# Supplementary material for: Swarm Reinforcement Learning For Adaptive Mesh Refinement
Source: arXiv:2304.00818 source file (2023-10-09)
Supplement: Supplementary file 1 [file group_element_penalties_1.tex]

\nextgroupplot[
ylabel shift = -0.2cm,
clip marker paths=true,
width=0.52\textwidth,
title style={yshift=-0.2cm},
height=4.5cm,
legend cell align={left},
clip marker paths=true,
log basis y={10},
tick align=outside,
tick pos=left,
title={ASMR},
x grid style={darkgray176},
xlabel={\empty},
xmajorgrids,
scaled x ticks=false,
xmin=-443.68, xmax=11364.16,
xtick style={color=black},
xtick={-2000,0,2000,4000,6000,8000,10000,12000},
xticklabels={\empty},
y grid style={darkgray176},
ylabel={Squared Error},
ymajorgrids,
ymin=5.97669995924903e-05, ymax=1.4498394926404,
ymode=log,
ytick style={color=black},
ytick={1e-06,1e-05,0.0001,0.001,0.01,0.1,1,10},
yticklabels={
  \(\displaystyle {10^{-6}}\),
  \(\displaystyle {10^{-5}}\),
  \(\displaystyle {10^{-4}}\),
  \(\displaystyle {10^{-3}}\),
  \(\displaystyle {10^{-2}}\),
  \(\displaystyle {10^{-1}}\),
  \(\displaystyle {10^{0}}\),
  \(\displaystyle {10^{1}}\)
}
]
\addplot [draw=red, fill=red, mark=*, mark size=1.9, only marks]
table{%
x  y
10827.44 8.89832417778698e-05
8102.46 0.000157479398200219
10341.7 0.000103640696026909
8004.3 0.000391863603320476
8733.48 0.000199655586592603
8894.46 0.000120733973308103
9745.58 0.000137263281414931
9169.26 0.000158745960107538
8041.88 0.000200159312559241
9242.9 0.000115577429873696
};
\addplot [draw=crimson227028, fill=crimson227028, mark=*, mark size=1.8, only marks]
table{%
x  y
5933.14 0.000384271585655832
5190.18 0.000714319857965041
7558.78 0.000273103096464109
6383.84 0.000425994052896478
7147.82 0.000263167244281184
7028.12 0.000235637116652944
6601.32 0.000413662118391082
6250.5 0.000342723455901967
7285.5 0.000315641507489854
5808.88 0.000473097068654762
};
\addplot [draw=crimson198057, fill=crimson198057, mark=*, mark size=1.7, only marks]
table{%
x  y
4704.78 0.000721063730609188
4669.16 0.000702916465450353
4884.38 0.000629589007908922
5345.22 0.000492787375382855
4517.84 0.000729231750768611
4360.52 0.000744839177498326
5155.24 0.000623847279416359
4665.26 0.000715647837964524
5064.22 0.000494807528208721
4656.3 0.000594803554837518
};
\addplot [draw=crimson170085, fill=crimson170085, mark=*, mark size=1.6, only marks]
table{%
x  y
3545.92 0.00094465663554887
3252.52 0.00120634616889338
3738.74 0.00116756600742772
3633.94 0.00143286209006131
2924.44 0.00218190151356095
3373.44 0.000929808742658101
2999.66 0.00168118865716983
4836.92 0.000531359022049817
3276.08 0.00142284404994178
3485.36 0.00123109170905157
};
\addplot [draw=purple1420113, fill=purple1420113, mark=*, mark size=1.5, only marks]
table{%
x  y
2856.26 0.00212675556447228
2666.66 0.00166573301676033
3000.32 0.00151188517783369
2557.36 0.00278244203287864
2208.88 0.00313583887067082
2784.02 0.00172471763613014
3423.04 0.000989698762361364
2718.5 0.0021646288442573
2948.92 0.00158706243707568
3363.52 0.000928262795043815
};
\addplot [draw=purple1130142, fill=purple1130142, mark=*, mark size=1.4, only marks]
table{%
x  y
1806.88 0.0044637024662834
2008.82 0.00489464315558175
2085.8 0.00374242051697224
1968.74 0.00417206546008202
1712.64 0.00401535698884066
1963.48 0.00445307783055
1833.18 0.00375564190990526
2239.48 0.00270746409770763
1824.58 0.00343516920040012
2042.92 0.0033501886862271
};
\addplot [draw=indigo850170, fill=indigo850170, mark=*, mark size=1.3, only marks]
table{%
x  y
1602.44 0.00542384881451712
1520.52 0.00579018443419992
1574.84 0.00606940289360274
1620.96 0.00464812571882298
1330.3 0.0066866089449338
1273.96 0.0084972475828809
1371.44 0.00631169862976796
1302.6 0.00761078195621184
1330.1 0.00576122589767241
1257.78 0.00661872088880234
};
\addplot [draw=mediumblue570198, fill=mediumblue570198, mark=*, mark size=1.2, only marks]
table{%
x  y
880.84 0.0170371041140525
915.34 0.0180814111705197
664.06 0.0316445770336203
795.52 0.018652945406005
927.7 0.02233027863137
1061.54 0.0159290070530343
836.18 0.0206039417495388
879.9 0.0150285895250592
893.5 0.0138103743408145
819.34 0.0220466759858583
};
\addplot [draw=mediumblue280227, fill=mediumblue280227, mark=*, mark size=1.1, only marks]
table{%
x  y
666.78 0.0260319244636584
655.06 0.0318785490585947
645.96 0.0280494475577444
538.92 0.0293680372328286
733 0.0501426321115083
504.34 0.0423955248616776
581.72 0.0329062856737456
684.3 0.0246609401306
662.56 0.0329571701160841
635.4 0.0247245469615234
};
\addplot [draw=blue, fill=blue, mark=*, mark size=1, only marks]
table{%
x  y
341.82 0.0784128563878483
418.4 0.0606693803247372
353.26 0.0910435229176025
420.2 0.0493127232028312
366.52 0.0730320438086551
407.74 0.0584584914229364
456.92 0.051868355302182
488.56 0.0433722037434131
271.42 0.106605814000352
394.68 0.0650625149726096
};
\addplot [draw=black, fill=black, mark=x, very thick, mark size=2.5pt, only marks]
table{%
x  y
93.04 0.254825928505529
380.48 0.0734326103191988
1525.76 0.0220825055651117
6118.4 0.00618414503102848
};
