# Supplementary material for: Swarm Reinforcement Learning For Adaptive Mesh Refinement
Source: arXiv:2304.00818 source file (2023-10-09)
Supplement: Supplementary file 2 [file group_element_penalties_2.tex]

\nextgroupplot[
ylabel shift = -0.2cm,
clip marker paths=true,
width=0.52\textwidth,
title style={yshift=-0.2cm},
height=4.5cm,
legend cell align={left},
clip marker paths=true,
log basis y={10},
tick align=outside,
tick pos=left,
title={VDGN-like (PPO)},
x grid style={darkgray176},
xlabel={\empty},
xmajorgrids,
scaled x ticks=false,
xmin=-443.68, xmax=11364.16,
xtick style={color=black},
xtick={-2000,0,2000,4000,6000,8000,10000},
xticklabels={\empty},
y grid style={darkgray176},
ylabel={\empty},
ymajorgrids,
ymin=5.97669995924903e-05, ymax=1.4498394926404,
ymode=log,
ytick style={color=black},
ytick={1e-06,1e-05,0.0001,0.001,0.01,0.1,1,10},
yticklabels={ 
\empty
  % \(\displaystyle {10^{-5}}\),
  % \(\displaystyle {10^{-4}}\),
  % \(\displaystyle {10^{-3}}\),
  % \(\displaystyle {10^{-2}}\),
  % \(\displaystyle {10^{-1}}\),
  % \(\displaystyle {10^{0}}\),
  % \(\displaystyle {10^{1}}\),
  % \(\displaystyle {10^{2}}\)
}
]
\addplot [draw=red, fill=red, mark=*, mark size=1.9, only marks]
table{%
x  y
23.82 0.999999996122416
1169.46 0.0124217678717432
23.82 0.999999996122416
439.7 0.0361793532148775
773.72 0.0450680372166332
23.72 0.999999996023892
23.82 0.999999996122416
};
\addplot [draw=crimson227028, fill=crimson227028, mark=*, mark size=1.8, only marks]
table{%
x  y
23.82 0.999999996122416
8209.1 0.00168656097432665
23.82 0.999999996122416
23.82 0.999999996122416
23.82 0.999999996122416
23.82 0.999999996122416
23.82 0.999999996122416
23.82 0.999999996122416
868.66 0.0541760875458956
23.82 0.999999996122416
};
\addplot [draw=crimson198057, fill=crimson198057, mark=*, mark size=1.7, only marks]
table{%
x  y
23.82 0.999999996122416
23.82 0.999999996122416
23.82 0.999999996122416
8965.7 0.00337769826976722
23.82 0.999999996122416
270.68 0.76214180148582
23.46 0.999999995989741
};
\addplot [draw=crimson170085, fill=crimson170085, mark=*, mark size=1.6, only marks]
table{%
x  y
23.4 0.999999996039599
23.44 0.999999995975606
3536.34 0.0143793497458716
23.82 0.999999996122416
559.04 0.086311246620783
23.82 0.999999996122416
23.82 0.999999996122416
510.54 0.0341639546418358
23.82 0.999999996122416
23.82 0.999999996122416
};
\addplot [draw=purple1420113, fill=purple1420113, mark=*, mark size=1.5, only marks]
table{%
x  y
27.24 1.00230361365338
238.62 0.0760667122397123
611.06 0.0724988694693003
23.82 0.999999996122416
23.82 0.999999996122416
23.82 0.999999996122416
2170.06 0.0678777363276302
159.22 0.943242780959166
23.82 0.999999996122416
23.82 0.999999996122416
};
\addplot [draw=purple1130142, fill=purple1130142, mark=*, mark size=1.4, only marks]
table{%
x  y
23.82 0.999999996122416
648.18 0.044717108075816
1950.46 0.00733967057516051
2368.96 0.0141022316227945
23.82 0.999999996122416
23.82 0.999999996122416
1823.7 0.0101068973030538
23.82 0.999999996122416
419.06 0.0393665730695053
426.8 0.112860977014587
};
\addplot [draw=indigo850170, fill=indigo850170, mark=*, mark size=1.3, only marks]
table{%
x  y
23.82 0.999999996122416
432.28 0.070275067488921
2573.04 0.0116711840171314
4540.78 0.00368233037052443
125.68 0.360801411710085
408.36 0.0974609973383949
274.88 0.0653661043432944
};
\addplot [draw=mediumblue570198, fill=mediumblue570198, mark=*, mark size=1.2, only marks]
table{%
x  y
4046.7 0.00581642890690849
639.38 0.0432326393280082
2768.32 0.019533590035356
922.24 0.0366073868832422
110.94 0.192999000581388
376.28 0.0525078414187748
217.72 0.150380175357821
9354.4 0.00552173695693054
182.92 0.235941680625069
};
\addplot [draw=mediumblue280227, fill=mediumblue280227, mark=*, mark size=1.1, only marks]
table{%
x  y
128.22 0.216813395905554
6780.12 0.000623141549313094
23.82 0.999999996122416
235.1 0.068158327342096
165.4 0.153415532035507
420.76 0.0465388379969933
23.68 0.999999996020024
76.38 0.315633121529024
351.64 0.0603192573114466
};
\addplot [draw=blue, fill=blue, mark=*, mark size=1, only marks]
table{%
x  y
631.9 0.0303484204333282
1751.58 0.114399114366206
56.3 0.690964747053063
23.82 0.999999996122416
248.88 0.251583987724092
23.82 0.999999996122416
23.82 0.999999996122416
21.52 0.999999993258309
68 0.377521254558437
};
\addplot [draw=black, fill=black, mark=x, very thick, mark size=2.5pt, only marks]
table{%
x  y
93.04 0.254825928505529
380.48 0.0734326103191988
1525.76 0.0220825055651117
6118.4 0.00618414503102848
};
