# Supplementary material for: Swarm Reinforcement Learning For Adaptive Mesh Refinement
Source: arXiv:2304.00818 source file (2023-10-09)
Supplement: Supplementary file 3 [file group_element_penalties_3.tex]

\nextgroupplot[
ylabel shift = -0.2cm,
clip marker paths=true,
width=0.52\textwidth,
title style={yshift=-0.2cm},
height=4.5cm,
legend cell align={left},
clip marker paths=true,
log basis y={10},
tick align=outside,
tick pos=left,
title={Single Agent},
x grid style={darkgray176},
xlabel={Elements \(\displaystyle (\times 10^3)\)},
xmajorgrids,
scaled x ticks=false,
xmin=-443.68, xmax=11364.16,
xtick style={color=black},
xtick={-2000,0,2000,4000,6000,8000,10000,12000},
xticklabels={-2.0,0.0,2.0,4.0,6.0,8.0,10.0,12.0},
y grid style={darkgray176},
ylabel={Squared Error},
ymajorgrids,
ymin=5.97669995924903e-05, ymax=1.4498394926404,
ymode=log,
ytick style={color=black},
ytick={1e-06,1e-05,0.0001,0.001,0.01,0.1,1,10},
yticklabels={
  \(\displaystyle {10^{-6}}\),
  \(\displaystyle {10^{-5}}\),
  \(\displaystyle {10^{-4}}\),
  \(\displaystyle {10^{-3}}\),
  \(\displaystyle {10^{-2}}\),
  \(\displaystyle {10^{-1}}\),
  \(\displaystyle {10^{0}}\),
  \(\displaystyle {10^{1}}\)
}
]
\addplot [draw=red, fill=red, mark=*, mark size=1.9, only marks]
table{%
x  y
1217.92 0.0151480732941594
2082.8 0.00636458856913025
1740.02 0.027961273253409
1608.66 0.00980825397069075
3598.8 0.0399923163957668
2126.74 0.0179336217858102
1837.88 0.00837894522907555
2331.5 0.00494422627506986
2537.34 0.0109139011326656
3124.1 0.00769406064096164
};
\addplot [draw=crimson227028, fill=crimson227028, mark=*, mark size=1.8, only marks]
table{%
x  y
1849.36 0.00754303149139505
2782.82 0.00489130436951127
2132.64 0.00584370968576076
2657.46 0.0064978581554907
2272.28 0.077877386835798
2779.88 0.00460860593236314
2712.78 0.00367052958943131
1496.56 0.0177279003331272
1941.8 0.0110421683635074
2286.12 0.00518630204551364
};
\addplot [draw=crimson198057, fill=crimson198057, mark=*, mark size=1.7, only marks]
table{%
x  y
2924.14 0.00767270545665162
923.18 0.282285834621994
1961.34 0.00875723201138038
1697.24 0.00751764488463775
976.28 0.189276217718494
1260.38 0.0116947148111287
2382.48 0.00558137502883495
1256.94 0.0225245667989927
1650.44 0.0153180553126528
1552.58 0.0115135911313676
};
\addplot [draw=crimson170085, fill=crimson170085, mark=*, mark size=1.6, only marks]
table{%
x  y
1670.44 0.00834941372411557
603.12 0.221715819032469
1479.36 0.00802392554528171
1915.4 0.0481969451275689
1779.12 0.0792849270440343
1385.08 0.0252567151548092
1725.84 0.00871400900397147
1647.58 0.00831853749686704
1677.58 0.00855457851671469
1673 0.0131574009621213
};
\addplot [draw=purple1420113, fill=purple1420113, mark=*, mark size=1.5, only marks]
table{%
x  y
1385.58 0.0125764671658645
2132.04 0.017012417172795
1605.7 0.0502079312389834
1941.68 0.0174530773114027
836.06 0.0667373138416828
1247.3 0.0106765815388036
1513.98 0.0124381633920264
1582.54 0.0163142478698431
1142.46 0.0136783645022612
1092.08 0.0284957402032658
};
\addplot [draw=purple1130142, fill=purple1130142, mark=*, mark size=1.4, only marks]
table{%
x  y
1146.14 0.016456246549887
1180.64 0.0260161021616322
1670.8 0.0145099874588786
1591.22 0.0328118097534962
480.96 0.104073729985161
1213.58 0.0158373362081697
1253.84 0.0768511104369187
1045.54 0.0295932571499663
944.5 0.317157701536104
1184.62 0.0214334559173025
};
\addplot [draw=indigo850170, fill=indigo850170, mark=*, mark size=1.3, only marks]
table{%
x  y
908.4 0.0596720180871403
943.26 0.0249322756429858
890 0.0542169249092586
905.18 0.0261443544366584
1212.1 0.0376990656982806
1405.82 0.244790804923172
985.28 0.0229109291148013
728 0.0294974738190566
884.62 0.0262531667183055
1078.44 0.259842288786618
};
\addplot [draw=mediumblue570198, fill=mediumblue570198, mark=*, mark size=1.2, only marks]
table{%
x  y
525.54 0.0583366724679071
606.5 0.0940116679295074
602.36 0.190106452922885
736.64 0.155206773495116
699.74 0.107870257720654
709.5 0.0969458308342032
853.18 0.0462876834722416
635.2 0.0818369346604553
621.9 0.108467420901385
579.1 0.0583973546821304
};
\addplot [draw=mediumblue280227, fill=mediumblue280227, mark=*, mark size=1.1, only marks]
table{%
x  y
496.72 0.0433305514572823
430.14 0.0845480521629051
465.94 0.549161130928365
454.5 0.0798147414580984
391.78 0.0624949430996049
421.64 0.0542477714267245
467.56 0.311705695949139
531.64 0.0515798581734869
560.3 0.0707966559435389
421.76 0.0924687356128762
};
\addplot [draw=blue, fill=blue, mark=*, mark size=1, only marks]
table{%
x  y
208.92 0.153424445628512
224.08 0.178824970924827
284.3 0.27285798365575
209.86 0.14610570616009
218.24 0.14901677438442
290.94 0.366849744307524
329.72 0.200814980373319
231.88 0.148193303508201
211.28 0.119640619547173
262.32 0.147964848145385
};
\addplot [draw=black, fill=black, mark=x, very thick, mark size=2.5pt, only marks]
table{%
x  y
93.04 0.254825928505529
380.48 0.0734326103191988
1525.76 0.0220825055651117
6118.4 0.00618414503102848
};
