# Supplementary material for: Swarm Reinforcement Learning For Adaptive Mesh Refinement
Source: arXiv:2304.00818 source file (2023-10-09)
Supplement: Supplementary file 4 [file group_element_penalties_4.tex]

\nextgroupplot[
ylabel shift = -0.2cm,
clip marker paths=true,
width=0.52\textwidth,
title style={yshift=-0.2cm},
height=4.5cm,
legend cell align={left},
clip marker paths=true,
log basis y={10},
tick align=outside,
tick pos=left,
title={Sweep},
x grid style={darkgray176},
xlabel={Elements \(\displaystyle (\times 10^3)\)},
xmajorgrids,
scaled x ticks=false,
xmin=-443.68, xmax=11364.16,
xtick style={color=black},
xtick={-2000,0,2000,4000,6000,8000,10000,12000},
xticklabels={-2.0,0.0,2.0,4.0,6.0,8.0,10.0,12.0},
y grid style={darkgray176},
ylabel={\empty},
ymajorgrids,
ymin=5.97669995924903e-05, ymax=1.4498394926404,
ymode=log,
ytick style={color=black},
ytick={1e-06,1e-05,0.0001,0.001,0.01,0.1,1,10},
yticklabels={
\empty
  % \(\displaystyle {10^{-4}}\),
  % \(\displaystyle {10^{-3}}\),
  % \(\displaystyle {10^{-2}}\),
  % \(\displaystyle {10^{-1}}\),
  % \(\displaystyle {10^{0}}\),
  % \(\displaystyle {10^{1}}\)
}
]
\addplot [draw=red, fill=red, mark=*, mark size=1.9, only marks]
table{%
x  y
10538.18 0.00249046657129108
7217.34 0.00242802232322071
};
\addplot [draw=crimson227028, fill=crimson227028, mark=*, mark size=1.8, only marks]
table{%
x  y
6947.84 0.00576041962274625
6947.1 0.00576197983079482
6947.84 0.00576041962274625
6630.36 0.00576154578143396
6947.84 0.00576041962274625
6118.4 0.00618414503102881
6947.84 0.00576041962274625
6947.84 0.00576041962274625
6947.84 0.00576041962274625
6947.84 0.00576041962274625
};
\addplot [draw=crimson198057, fill=crimson198057, mark=*, mark size=1.7, only marks]
table{%
x  y
6118.4 0.00618414503102881
6118.4 0.00618414503102881
6118.4 0.00618414503102881
6118.4 0.00618414503102881
6118.4 0.00618414503102881
6118.4 0.00618414503102881
6118.4 0.00618414503102881
6118.4 0.00618414503102881
6118.4 0.00618414503102881
6118.4 0.00618414503102881
};
\addplot [draw=crimson170085, fill=crimson170085, mark=*, mark size=1.6, only marks]
table{%
x  y
6118.4 0.00618414503102881
6118.4 0.00618414503102881
6118.4 0.00618414503102881
6118.4 0.00618414503102881
6118.4 0.00618414503102881
6118.4 0.00618414503102881
6118.4 0.00618414503102881
6118.4 0.00618414503102881
6118.4 0.00618414503102881
6118.4 0.00618414503102881
};
\addplot [draw=purple1420113, fill=purple1420113, mark=*, mark size=1.5, only marks]
table{%
x  y
6118.4 0.00618414503102881
6118.4 0.00618414503102881
6118.4 0.00618414503102881
6108.3 0.00618836058589075
6118.4 0.00618414503102881
6118.26 0.00618535975880503
6118.4 0.00618414503102881
6118.4 0.00618414503102881
6118.4 0.00618414503102881
6118.4 0.00618414503102881
};
\addplot [draw=purple1130142, fill=purple1130142, mark=*, mark size=1.4, only marks]
table{%
x  y
5941.06 0.0062289827358909
2044.72 0.0210615214513479
3035.64 0.0096927394688761
3255.34 0.00654060589561155
5838.58 0.0066942900105509
5052.98 0.00865652993540068
5065.7 0.0062805279627293
6118.4 0.00618414503102881
6118.4 0.00618414503102881
6118.28 0.00618414284841863
};
\addplot [draw=indigo850170, fill=indigo850170, mark=*, mark size=1.3, only marks]
table{%
x  y
4396.38 0.0105585579200991
1591.12 0.0119115299943415
1903.68 0.0159554716555746
1978.66 0.016344123755007
2729.76 0.0110421539272058
1913.18 0.0119695633989661
1647.82 0.0123997491391439
4021.38 0.0105914273315205
4159.48 0.010595840704466
2347 0.0113417245256515
};
\addplot [draw=mediumblue570198, fill=mediumblue570198, mark=*, mark size=1.2, only marks]
table{%
x  y
1525.66 0.0220830665934843
1478.14 0.0222052664448807
1525.76 0.0220825055651083
1525.64 0.0220825066758445
1525.76 0.0220825055651083
1479.32 0.0223532988940319
1525.76 0.0220825055651083
1524.06 0.0221028347922318
1525.76 0.0220825055651083
1525.76 0.0220825055651083
};
\addplot [draw=mediumblue280227, fill=mediumblue280227, mark=*, mark size=1.1, only marks]
table{%
x  y
1396.26 0.0223672383981686
1340.9 0.0224270714826669
1451.96 0.023500019608051
1356.56 0.0222905770892828
945.22 0.0239228847037097
1213.38 0.0228873565005452
1318.94 0.0342337164764184
1164.1 0.0220029140452478
1249.96 0.0241539858289707
1358.82 0.0228538150551287
};
\addplot [draw=blue, fill=blue, mark=*, mark size=1, only marks]
table{%
x  y
395.94 0.0564679564112043
453 0.0369175544961218
363.62 0.0662187701855255
378.66 0.0721057696638585
466.94 0.0483593302840383
419.04 0.0577192964994661
441.44 0.0514797915392547
336.66 0.0680162646963843
391.66 0.0520091287608055
382.46 0.0607247473558358
};
\addplot [draw=black, fill=black, mark=x, very thick, mark size=2.5pt, only marks]
table{%
x  y
93.04 0.254825928505529
380.48 0.0734326103191988
1525.76 0.0220825055651117
6118.4 0.00618414503102848
};
