# Supplementary material for: Swarm Reinforcement Learning For Adaptive Mesh Refinement
Source: arXiv:2304.00818 source file (2023-10-09)
Supplement: Supplementary file 5 [file group_ablations_1.tex]

\nextgroupplot[
ylabel shift = -0.2cm,
clip marker paths=true,
width=0.52\textwidth,
height=4.5cm,
title style={yshift=-0.2cm},
scaled x ticks=false,
legend cell align={left},
legend style={fill opacity=0.8, draw opacity=1, text opacity=1, draw=lightgray204},
log basis y={10},
tick align=outside,
tick pos=left,
title={Poisson - Node Features},
x grid style={darkgray176},
xlabel={Elements \(\displaystyle (\times 10^3)\)},
xmajorgrids,
xmin=-419.152, xmax=9281.792,
xtick style={color=black},
xtick={-1000,0,1000,2000,3000,4000,5000,6000,7000,8000,9000},
xticklabels={-1.0,0.0,1.0,2.0,3.0,4.0,5.0,6.0,7.0,8.0,9.0},
y grid style={darkgray176},
ylabel={Squared Error},
ymajorgrids,
ymin=3.2945347498023e-06, ymax=2.41273251028282,
ymode=log,
ytick style={color=black},
ytick={1e-07,1e-06,1e-05,0.0001,0.001,0.01,0.1,1,10,100},
yticklabels={
  \(\displaystyle {10^{-7}}\),
  \(\displaystyle {10^{-6}}\),
  \(\displaystyle {10^{-5}}\),
  \(\displaystyle {10^{-4}}\),
  \(\displaystyle {10^{-3}}\),
  \(\displaystyle {10^{-2}}\),
  \(\displaystyle {10^{-1}}\),
  \(\displaystyle {10^{0}}\),
  \(\displaystyle {10^{1}}\),
  \(\displaystyle {10^{2}}\)
}
]
\addplot [
  draw=royalblue28108204,
  fill=royalblue28108204,
  forget plot,
  mark=*, mark size=1,
  only marks,
  draw opacity=0,
 fill opacity=0.5
]
table{%
x  y
219.22 0.0116380025783674
236.58 0.00893751131252496
255.06 0.00757221773421185
266.3 0.00695152587324572
277.02 0.00870449843080493
289.06 0.00650849332548639
301.82 0.00650772537377039
309.02 0.00632830538267971
313.48 0.00852456067483164
317.48 0.00503420224308783
366.78 0.00472734343816265
384.24 0.00384945126787151
427.52 0.00440570193112838
431.14 0.00387196288409598
433.8 0.0031068838328975
438.92 0.0033561305566538
446.06 0.00325148782214415
485 0.00270934352590588
524.5 0.0019590317268996
530.98 0.0024847849713976
530.98 0.0024462804500235
542.2 0.00339373662958677
568.26 0.00191195330793864
569.1 0.00200759214947172
579.8 0.00192121084682089
587.66 0.00166535004820132
612.06 0.00170099739413765
628 0.00142557999535175
636.98 0.00193167521782833
648.04 0.00147630841918046
648.78 0.00196488850395651
684.76 0.00192456325257735
704.12 0.00152017798836435
708.02 0.00171515266408961
724.56 0.00106290863523144
740.7 0.00145038634314574
740.82 0.00126611233262213
754.68 0.0010958404611985
776.14 0.00136681288549904
861 0.00122261947029662
866.82 0.0012376456173406
951.18 0.000684639740045543
978.82 0.000682995459645206
1030.58 0.000639142132617508
1031.2 0.000608987227553708
1080.16 0.000534351174466062
1116.56 0.000522936657826564
1126.22 0.00047220578013082
1173.32 0.000587407673606018
1183.24 0.000496992672901857
1212.6 0.000433759599768057
1270.84 0.000477030829124065
1271.28 0.00057574970357699
1312.64 0.000295338105933881
1334.88 0.0003688460635094
1390.92 0.000632823129081481
1414.42 0.000439822660083419
1465.2 0.000380405825070989
1546.18 0.000259777992401812
1645.64 0.000189432782231567
1650.1 0.00040730379394757
1712.26 0.000225696747843442
1799.62 0.000205137266591349
1800.64 0.000149688394684308
1820.82 0.00022968203197516
1908.42 0.000134858938308452
1925.1 0.000231468966668099
2020.12 0.000123482420852495
2156.38 0.000114435638078513
2168.78 0.000132258579214635
2169 0.000101440195225082
2212 0.000202015930911123
2238.3 0.000100444720362762
2307.32 0.00010430451268494
2321.26 0.000101348576943888
2363.12 7.85396281013735e-05
2399.82 8.97496755911525e-05
2432.68 0.000175103698214891
2457.16 9.48685731254995e-05
2655.7 7.07642905549767e-05
2715.22 5.85765922707877e-05
3044.4 5.85685554721719e-05
3414.76 4.01750628140733e-05
3545.46 3.80019302781983e-05
3591.66 3.62548169075136e-05
3997.22 3.19018762058348e-05
4033.6 2.70246768067793e-05
4075.94 2.55319826966762e-05
4148.74 2.90210310242148e-05
4304.56 2.36833753484687e-05
4311.96 4.28165553247746e-05
4611.22 2.13677683411378e-05
5764.26 1.3085878413959e-05
6013.74 1.0832458588431e-05
6168.52 9.73742044189171e-06
6591.82 8.02970379055727e-06
6800.42 8.43665609892419e-06
6819.78 8.29434337198603e-06
7381.26 8.13257734004449e-06
7648.78 6.34432528857979e-06
};
\addplot [
  draw=cadetblue80178158,
  fill=cadetblue80178158,
  forget plot,
  mark=*, mark size=1,
  only marks,
  draw opacity=0,
 fill opacity=0.5
]
table{%
x  y
76.46 0.324649302372107
77.5 0.363369193841061
94.42 0.24666180724943
109.32 0.186174674092117
110.94 0.185758438075802
111.32 0.166867049907532
114.52 0.193110987959021
116.34 0.182870870946333
128.02 0.216054774613969
128.74 0.191873741961263
160.54 0.0871121902170006
161.12 0.12367804129538
180.3 0.100333740127915
182.46 0.0987065319678356
184.3 0.0845749597726281
187.18 0.072656583580787
193.96 0.058587626881626
217.16 0.0441984057022334
227.64 0.0702184734275756
245.2 0.0459038035787503
251.72 0.0364126826407728
270.62 0.0333469037437763
275.68 0.0280778280906009
276.3 0.0185992987592233
286.98 0.0186839325234224
297.22 0.0229991292830044
374.16 0.00916725420617235
411.3 0.0068200642980895
416.82 0.006665914580277
421.16 0.00514742100268873
432.88 0.00555861349482553
490.84 0.00387737700361097
496.04 0.00432851803548351
501.92 0.00383649638853136
636.54 0.0020307954085463
639.18 0.00193599862440002
663.1 0.00171575344957506
665.84 0.00191644234451826
698.38 0.00158029097400022
703.04 0.0014770938803194
704.94 0.00180196329463034
715.04 0.00144474522374639
728.46 0.00171062512691464
729.26 0.0013887856355886
788.6 0.00130842346985013
791.88 0.00118532851883899
797.48 0.00105772942814475
830.16 0.00116439903223206
849.06 0.00114524993177717
852.56 0.00100568639167076
928.34 0.000990808504017271
930.24 0.000886249281054975
1006.52 0.000647856014189414
1033 0.000804580312705349
1084.08 0.000638994012723058
1087.1 0.000681308928549735
1108.36 0.000495110341753963
1161.04 0.000488539105425854
1183.06 0.000410291838535373
1188.32 0.000454615240690676
1200.34 0.000461871263155013
1239.4 0.000402622903457912
1255.4 0.000819911577209595
1319.54 0.000404042176953841
1394.64 0.000324528340997405
1511.18 0.000243331920103783
1514.18 0.0003223886931292
1535.64 0.00024037469129075
1604.5 0.000249324466879171
1625.16 0.000239152934927504
1644.04 0.000196462447171108
1694.08 0.000183067040710325
1757.98 0.00018988441938983
1794.96 0.000177224380025814
1809.84 0.000186749426384397
1844.6 0.000170559874173604
1857.88 0.0001723375898085
1860.42 0.000158853823233923
1875.1 0.00016111954340722
1989.2 0.000146226604068255
2079.74 0.000149445578197006
2098.7 0.000134224009434416
2199.82 0.000118600884416034
2460.68 8.87412950988705e-05
2511.48 8.99145953343811e-05
2557.66 8.17451688004562e-05
2627.46 8.88026305170725e-05
3207.22 4.95867110213706e-05
3276.24 5.22284198942497e-05
3305.94 4.96763723538134e-05
3348.84 5.09793289987068e-05
3548.44 4.34945252685227e-05
3983.08 3.44413145781619e-05
4278.66 2.83552596125645e-05
5075.22 2.21270687556576e-05
5464.24 1.63086735125538e-05
5543.18 1.63583027354058e-05
5917.9 1.57051697641336e-05
6158.94 1.70354492778014e-05
6346.56 1.68050666873237e-05
};
\addplot [
  draw=yellowgreen18420623,
  fill=yellowgreen18420623,
  forget plot,
  mark=*, mark size=1,
  only marks,
  draw opacity=0,
 fill opacity=0.5
]
table{%
x  y
232.32 0.00972972749178268
236.92 0.00939851974187336
258.64 0.00855109131137597
269.3 0.00751516813140444
274.38 0.00723881601168976
280.12 0.00761510592003331
282.26 0.00672619030765893
301.82 0.00626745768612525
302.24 0.00762010549300113
312 0.00711630238248691
373.4 0.00448421919256764
375.1 0.00437652863607603
376.02 0.00520630933550564
386.72 0.0033251438475346
398.02 0.00356680356807807
422.9 0.00430357474285149
429.22 0.00330727325184691
434.4 0.00362172198767669
438.9 0.00340082707451565
466.98 0.00264467982389246
532.88 0.0025399486030681
533.24 0.00203606035088114
541.98 0.00200211193041517
567 0.0021699032340457
583.28 0.00239043670944809
588.48 0.00167119438437892
597.12 0.00253526944919157
605.12 0.001822693559239
614.26 0.00150790590744772
614.98 0.00198819632928885
623.46 0.00192438176373624
642.02 0.00198006783993482
664.2 0.00137312725228689
697.38 0.00160178893032639
710.38 0.00121844386732602
741.88 0.00131564448935872
762.5 0.00166827981802596
776.4 0.00164881432118705
794.86 0.00113260725057376
801.12 0.00114548928864236
823.3 0.00138304615302644
895.36 0.000954945550980965
965.54 0.00089384133267044
971.76 0.000795488827859309
1023.22 0.000630956453768671
1027.22 0.000566269014761171
1144.84 0.000557587023543132
1159.14 0.000492978921053553
1183.98 0.000535067426151905
1206.82 0.000508165557992129
1230.1 0.000536549124900031
1257.68 0.00061579369658109
1300.84 0.000360249901762512
1376.96 0.000444693820344096
1401.66 0.000364337388690847
1435.96 0.000305214410009089
1436.02 0.000372361652686717
1446.1 0.000310634936393891
1448.84 0.000290067030172305
1455.12 0.000554506960536
1491.12 0.000324064897307907
1584.46 0.000274183719896366
1686.1 0.000241929349106663
1707.42 0.000226777199339877
1787.04 0.00020915776595312
1862.9 0.000148540046571892
1928.94 0.000162934668966511
1962.54 0.000238168585805641
2041.88 0.000147436309732292
2042.8 0.000152662606194393
2058.76 0.000123061762508607
2119.94 0.000220537378219434
2171.1 0.000142758798946366
2244.48 0.000146276332772705
2302.6 0.000378780970703722
2392.78 0.000108879308313787
2495.72 0.000187049885499844
2518.06 0.000163331073874347
2654.08 0.000192056675384633
2809.7 8.57776276420434e-05
2819.4 6.45700158265773e-05
2929.04 0.000119940093378474
3026.26 7.11318606580667e-05
3262.38 4.25935338820714e-05
3264.9 5.12294186633602e-05
3402.88 6.61360408573708e-05
3433.5 4.99070679689521e-05
3949.42 4.63931544667156e-05
4481.16 3.83950495461031e-05
4748.4 2.45958446205938e-05
4757.62 3.97676453277772e-05
5473.42 3.18924472206022e-05
5484.86 1.66897225815467e-05
5817.68 2.06111107411429e-05
6187.98 1.61118606198381e-05
6395.9 1.26910847993608e-05
6599.22 1.29057437505192e-05
6706.72 1.47270296604059e-05
6836.5 1.39321658050796e-05
7183.04 1.32441458177349e-05
};
\addplot [
  draw=sandybrown24422769,
  fill=sandybrown24422769,
  forget plot,
  mark=*, mark size=1,
  only marks,
  draw opacity=0,
 fill opacity=0.5
]
table{%
x  y
190.06 0.0160506438754664
211.38 0.0175674771240263
236.2 0.0157920133719396
240.66 0.00996396170307461
247.76 0.0211532431545219
276.1 0.011506231997328
311.16 0.00933255400159171
331.66 0.00667299865068799
346.18 0.00834977079606523
395.6 0.00665471002911091
446.86 0.00433029362616953
458.54 0.00400987552984578
467.46 0.00400374538271125
475.38 0.00373435261828123
476.88 0.00406702048468009
478.74 0.0037028657796726
481.68 0.0036183395494554
494.14 0.00365666991457534
504.48 0.00346170326388388
508.82 0.00336940773468552
586.52 0.00261023863301834
590.78 0.00268199311566163
596.84 0.002941737668219
605.46 0.00251960996948417
621.28 0.00257027926641862
624.16 0.00239843612038315
670.82 0.00235446004931542
675.52 0.00233320464979304
717.7 0.00213556417812113
725.62 0.00208735064231013
743.52 0.00209348105820297
746.38 0.00211428757333376
760.64 0.00239306409536522
765.8 0.00221260846111945
798.8 0.00203337394547253
816.88 0.00188056666575394
859.54 0.00182090031768361
890.82 0.00186826096277136
913.8 0.00182015423435024
935.06 0.00220674968803355
1017.72 0.00207275297147396
1168.64 0.00192689680209973
1260.06 0.0010033761560263
1286.78 0.000916784213120534
1477.58 0.000966545721555283
1529.7 0.00170037911601046
1597.94 0.000549180616811459
1785.02 0.000500740280858601
1803.82 0.000474791929576806
1810.5 0.000452331642721943
1839.3 0.000475503594071749
1862.72 0.000426849990506186
1909.42 0.000488318036644794
1911.62 0.000394069213857266
1970.12 0.000370050178508785
2006.02 0.000363466976332125
2069.36 0.000360415408268616
2072.36 0.000362543496919579
2073.2 0.000347363442431046
2087.24 0.000741690781816842
2103.62 0.000367202424182477
2155.76 0.000343387993473352
2162.12 0.000362599779749814
2186.1 0.000323342727758768
2241.38 0.000273430355759432
2244.22 0.000429548329799723
2293.66 0.000280905708693901
2326.34 0.000315943143494894
2370.78 0.00033861184415235
2391.56 0.000274854940602764
2418.9 0.000413276885974003
2542.56 0.000425797618038134
2575.9 0.000379140788236466
2601.02 0.00038773696582266
2649.06 0.000291039358976014
2721.76 0.000400538215384972
2746.04 0.000325153636313231
2780.48 0.000239372988734078
2783.68 0.000335510783341945
2815.3 0.000291752831175176
2840.58 0.000278349073291838
2887.28 0.000263012767044535
2973.64 0.000323469987548169
3037.2 0.000314931162447476
3087.74 0.000314660214461137
3184.8 0.000300192431583708
3277.12 0.000217235375225012
3461.5 0.000249878617126562
4182.7 0.000181467140309587
4234.28 0.000162297122249636
4386.94 0.000187534382180038
5903.14 7.69115291142625e-05
6369.18 6.50302348131615e-05
6884.14 4.52439969624826e-05
6964.64 4.65331359997054e-05
7134.94 4.10527289801623e-05
7140.8 4.35938245381886e-05
7658.3 3.33472062825622e-05
7689.92 3.56217928671189e-05
7780.94 3.62506780197039e-05
};
\addplot [very thick, royalblue28108204]
table {%
219.22 0.011036362330508
294.266060606061 0.00683752177615596
369.312121212121 0.00464144864349475
444.358181818182 0.00334666716525019
519.404242424242 0.0025193038327363
594.450303030303 0.00195898836228103
669.496363636364 0.00156242272863255
744.542424242424 0.00127184853740656
819.588484848485 0.00105288309708372
894.634545454545 0.000884011430865333
969.680606060606 0.000751210162546177
1044.72666666667 0.000645022898528129
1119.77272727273 0.000558886634562944
1194.81878787879 0.000488132454642395
1269.86484848485 0.000429366813814566
1344.91090909091 0.000380076270852898
1419.95696969697 0.000338367971794018
1495.00303030303 0.0003027951072934
1570.04909090909 0.000272236981973959
1645.09515151515 0.000245815016365929
1720.14121212121 0.000222832893735278
1795.18727272727 0.000202733241627402
1870.23333333333 0.000185065832838411
1945.27939393939 0.000169463938324359
2020.32545454545 0.000155626532140522
2095.37151515152 0.000143304752953709
2170.41757575758 0.00013229149937599
2245.46363636364 0.000122413358503866
2320.5096969697 0.00011352428972744
2395.55575757576 0.00010550064185257
2470.60181818182 9.82371921850629e-05
2545.64787878788 9.16439755603686e-05
2620.69393939394 8.56437288176314e-05
2695.74 8.01698183332399e-05
2770.78606060606 7.51645493600184e-05
2845.83212121212 7.05777791330937e-05
2920.87818181818 6.63657731597201e-05
2995.92424242424 6.24902573397632e-05
3070.9703030303 5.89176286642295e-05
3146.01636363636 5.56182950054424e-05
3221.06242424242 5.25661205236171e-05
3296.10848484848 4.97379578968152e-05
3371.15454545455 4.71132522503113e-05
3446.20060606061 4.46737045530535e-05
3521.24666666667 4.24029845402706e-05
3596.29272727273 4.02864850465218e-05
3671.33878787879 3.83111110946094e-05
3746.38484848485 3.64650982610337e-05
3821.43090909091 3.47378557882919e-05
3896.47696969697 3.31198306849694e-05
3971.52303030303 3.16023896826275e-05
4046.56909090909 3.01777164323574e-05
4121.61515151515 2.88387217459749e-05
4196.66121212121 2.75789650348172e-05
4271.70727272727 2.63925853870252e-05
4346.75333333333 2.52742409632466e-05
4421.79939393939 2.42190555898078e-05
4496.84545454546 2.32225715948118e-05
4571.89151515152 2.22807080720926e-05
4646.93757575758 2.13897238752291e-05
4721.98363636364 2.05461847426933e-05
4797.0296969697 1.97469340388092e-05
4872.07575757576 1.89890666660709e-05
4947.12181818182 1.8269905764614e-05
5022.16787878788 1.75869818659648e-05
5097.21393939394 1.69380142120492e-05
5172.26 1.63208939879861e-05
5247.30606060606 1.57336692494166e-05
5322.35212121212 1.51745313528374e-05
5397.39818181818 1.46418027212986e-05
5472.44424242424 1.41339257984621e-05
5547.4903030303 1.3649453061884e-05
5622.53636363636 1.31870379818742e-05
5697.58242424242 1.2745426825751e-05
5772.62848484848 1.23234512190284e-05
5847.67454545455 1.19200213852963e-05
5922.72060606061 1.15341199954871e-05
5997.76666666667 1.1164796565038e-05
6072.81272727273 1.08111623443141e-05
6147.85878787879 1.04723856536745e-05
6222.90484848485 1.0147687619861e-05
6297.95090909091 9.83633827504848e-06
6372.99696969697 9.53765298401601e-06
6448.04303030303 9.25098916853041e-06
6523.08909090909 8.97574330125288e-06
6598.13515151515 8.71134814433109e-06
6673.18121212121 8.45727021036785e-06
6748.22727272727 8.21300742570822e-06
6823.27333333333 7.97808697798452e-06
6898.31939393939 7.75206333164318e-06
6973.36545454545 7.53451639676642e-06
7048.41151515152 7.32504983792122e-06
7123.45757575758 7.12328951103846e-06
7198.50363636364 6.92888201746202e-06
7273.5496969697 6.74149336532551e-06
7348.59575757576 6.56080772932964e-06
7423.64181818182 6.38652630081431e-06
7498.68787878788 6.21836622075785e-06
7573.73393939394 6.05605958900093e-06
7648.78 5.89935254359227e-06
};
\addplot [very thick, cadetblue80178158]
table {%
76.46 0.677656332403636
139.794343434343 0.12410869627174
203.128686868687 0.0448160127030978
266.46303030303 0.02172340137052
329.797373737374 0.0124113785764754
393.131717171717 0.00787409660270458
456.466060606061 0.00537089964604743
519.800404040404 0.00386299311087674
583.134747474748 0.00289313397277987
646.469090909091 0.00223688438212706
709.803434343434 0.00177452226979323
773.137777777778 0.00143784834851217
836.472121212121 0.00118588907159839
899.806464646465 0.000992919624209993
963.140808080808 0.000842179354001275
1026.47515151515 0.000722397402507939
1089.8094949495 0.000625784900404476
1153.14383838384 0.000546829608836101
1216.47818181818 0.000481547922893543
1279.81252525253 0.000427006999672884
1343.14686868687 0.000381011502537523
1406.48121212121 0.00034189349060797
1469.81555555556 0.000308368561340635
1533.1498989899 0.000279435509534399
1596.48424242424 0.000254305151122737
1659.81858585859 0.000232349054624155
1723.15292929293 0.00021306209045673
1786.48727272727 0.000196034719213095
1849.82161616162 0.000180932241399142
1913.15595959596 0.000167479088354773
1976.4903030303 0.00015544680795398
2039.82464646465 0.000144644788690708
2103.15898989899 0.000134913034527422
2166.49333333333 0.000126116490520012
2229.82767676768 0.000118140551820875
2293.16202020202 0.000110887483416633
2356.49636363636 0.000104273546394615
2419.83070707071 9.82266764560167e-05
2483.16505050505 9.26845971543255e-05
2546.49939393939 8.75932776453442e-05
2609.83373737374 8.29056651904146e-05
2673.16808080808 7.85806380977513e-05
2736.50242424242 7.45821365334437e-05
2799.83676767677 7.08784376319324e-05
2863.17111111111 6.74415482750667e-05
2926.50545454545 6.42466942946641e-05
2989.8397979798 6.12718890590317e-05
3053.17414141414 5.84975677069403e-05
3116.50848484848 5.59062759011473e-05
3179.84282828283 5.34824040446211e-05
3243.17717171717 5.12119595552539e-05
3306.51151515152 4.90823711200009e-05
3369.84585858586 4.70823199168484e-05
3433.1802020202 4.52015936567783e-05
3496.51454545455 4.34309599997769e-05
3559.84888888889 4.17620564716606e-05
3623.18323232323 4.01872944776234e-05
3686.51757575758 3.8699775394199e-05
3749.85191919192 3.72932170396955e-05
3813.18626262626 3.59618890868523e-05
3876.52060606061 3.47005562005812e-05
3939.85494949495 3.35044278663561e-05
4003.18929292929 3.23691140276103e-05
4066.52363636364 3.12905857786928e-05
4129.85797979798 3.02651404677986e-05
4193.19232323232 2.92893706553024e-05
4256.52666666667 2.83601364499405e-05
4319.86101010101 2.74745408106248e-05
4383.19535353535 2.66299074572583e-05
4446.5296969697 2.58237610813081e-05
4509.86404040404 2.50538095874207e-05
4573.19838383838 2.43179281320715e-05
4636.53272727273 2.36141447550625e-05
4699.86707070707 2.29406274253397e-05
4763.20141414141 2.22956723447491e-05
4826.53575757576 2.16776933724728e-05
4889.8701010101 2.10852124494744e-05
4953.20444444444 2.05168509166606e-05
5016.53878787879 1.99713216329784e-05
5079.87313131313 1.94474218105659e-05
5143.20747474748 1.89440264935851e-05
5206.54181818182 1.8460082615685e-05
5269.87616161616 1.79946035783267e-05
5333.21050505051 1.75466642985938e-05
5396.54484848485 1.71153966807291e-05
5459.87919191919 1.66999854705844e-05
5523.21353535354 1.62996644565254e-05
5586.54787878788 1.59137129841886e-05
5649.88222222222 1.55414527558845e-05
5713.21656565657 1.51822448884611e-05
5776.55090909091 1.48354872061108e-05
5839.88525252525 1.45006117469809e-05
5903.2195959596 1.41770824645573e-05
5966.55393939394 1.38643931066716e-05
6029.88828282828 1.35620652566582e-05
6093.22262626263 1.32696465226848e-05
6156.55696969697 1.29867088626171e-05
6219.89131313131 1.27128470329757e-05
6283.22565656566 1.24476771516162e-05
6346.56 1.21908353647274e-05
};
\addplot [very thick, yellowgreen18420623]
table {%
232.32 0.0100580122198055
302.529292929293 0.00646236374292496
372.738585858586 0.00451507008128169
442.947878787879 0.00333657830941516
513.157171717172 0.00256716559165183
583.366464646465 0.00203628090564721
653.575757575758 0.0016541963773395
723.785050505051 0.00136989530996803
793.994343434343 0.0011525676388345
864.203636363636 0.000982685514672074
934.412929292929 0.000847371700575487
1004.62222222222 0.000737848694797621
1074.83151515152 0.000647962957864478
1145.04080808081 0.000573294971197859
1215.2501010101 0.000510603199843592
1285.45939393939 0.000457465852183147
1355.66868686869 0.000412043797923882
1425.87797979798 0.000372919909754691
1496.08727272727 0.000338987877971566
1566.29656565657 0.000309373800178555
1636.50585858586 0.000283379938604623
1706.71515151515 0.000260443753519181
1776.92444444444 0.000240107643645771
1847.13373737374 0.000221996307903644
1917.34303030303 0.00020579960928753
1987.55232323232 0.000191259462867488
2057.76161616162 0.000178159702365385
2127.97090909091 0.000166318175961758
2198.1802020202 0.000155580527732065
2268.3894949495 0.00014581526590801
2338.59878787879 0.000136909822308812
2408.80808080808 0.000128767381605222
2479.01737373737 0.00012130431319388
2549.22666666667 0.000114448078255991
2619.43595959596 0.000108135514114246
2689.64525252525 0.00010231142012121
2759.85454545455 9.69273860123921e-05
2830.06383838384 9.19408163638398e-05
2900.27313131313 8.73141145337377e-05
2970.48242424242 8.30139969850347e-05
3040.69171717172 7.90109147269267e-05
3110.90101010101 7.52785631796376e-05
3181.1103030303 7.17934653586495e-05
3251.3195959596 6.85346161155714e-05
3321.52888888889 6.54831774322116e-05
3391.73818181818 6.26222165706067e-05
3461.94747474747 5.9936480332711e-05
3532.15676767677 5.74121998545977e-05
3602.36606060606 5.50369213095774e-05
3672.57535353535 5.27993586678654e-05
3742.78464646465 5.06892652926938e-05
3812.99393939394 4.86973216718262e-05
3883.20323232323 4.68150370111898e-05
3953.41252525253 4.50346627711535e-05
4023.62181818182 4.33491165196727e-05
4093.83111111111 4.17519147211395e-05
4164.0404040404 4.02371132841867e-05
4234.2496969697 3.87992548630519e-05
4304.45898989899 3.74333220511964e-05
4374.66828282828 3.61346957273894e-05
4444.87757575757 3.48991179172347e-05
4515.08686868687 3.37226586202828e-05
4585.29616161616 3.2601686126983e-05
4655.50545454545 3.15328404129137e-05
4725.71474747475 3.05130092517396e-05
4795.92404040404 2.95393067346068e-05
4866.13333333333 2.86090539234219e-05
4936.34262626263 2.77197613996598e-05
5006.55191919192 2.68691134998423e-05
5076.76121212121 2.6054954054336e-05
5146.9705050505 2.52752734682053e-05
5217.1797979798 2.45281970020341e-05
5287.38909090909 2.38119741273054e-05
5357.59838383838 2.31249688454629e-05
5427.80767676768 2.24656508724648e-05
5498.01696969697 2.18325876017346e-05
5568.22626262626 2.12244367681361e-05
5638.43555555555 2.06399397441333e-05
5708.64484848485 2.00779154067927e-05
5778.85414141414 1.95372545208918e-05
5849.06343434343 1.90169145892228e-05
5919.27272727273 1.85159151263222e-05
5989.48202020202 1.8033333316411e-05
6059.69131313131 1.7568300020361e-05
6129.90060606061 1.71199961000776e-05
6200.1098989899 1.6687649031873e-05
6270.31919191919 1.62705297832238e-05
6340.52848484848 1.5867949929832e-05
6410.73777777778 1.54792589921518e-05
6480.94707070707 1.51038419725527e-05
6551.15636363636 1.47411170760821e-05
6621.36565656566 1.4390533599401e-05
6691.57494949495 1.40515699739018e-05
6761.78424242424 1.37237319503153e-05
6831.99353535353 1.34065509132703e-05
6902.20282828283 1.30995823153188e-05
6972.41212121212 1.28024042208767e-05
7042.62141414141 1.25146159513811e-05
7112.83070707071 1.22358368237275e-05
7183.04 1.1965704974746e-05
};
\addplot [very thick, sandybrown24422769]
table {%
190.06 0.0162301073621367
266.735555555556 0.0101892958710407
343.411111111111 0.00713180477239224
420.086666666667 0.00533373331109382
496.762222222222 0.00417184986680016
573.437777777778 0.00337064048213377
650.113333333333 0.00279115629544005
726.788888888889 0.00235643366926813
803.464444444444 0.00202073135938205
880.14 0.00175532720052806
956.815555555555 0.00154137051698603
1033.49111111111 0.00136603136260117
1110.16666666667 0.00122030761767886
1186.84222222222 0.00109771732616582
1263.51777777778 0.000993487980653328
1340.19333333333 0.000904036869920372
1416.86888888889 0.000826628231721498
1493.54444444444 0.000759141263166718
1570.22 0.000699909599413131
1646.89555555556 0.000647608015119312
1723.57111111111 0.000601171020747678
1800.24666666667 0.000559733429544264
1876.92222222222 0.000522586330430418
1953.59777777778 0.000489144039242439
2030.27333333333 0.000458918989099314
2106.94888888889 0.000431502439858749
2183.62444444444 0.000406549505843342
2260.3 0.000383767424869535
2336.97555555556 0.000362906286023649
2413.65111111111 0.000343751640924313
2490.32666666667 0.000326118571014068
2567.00222222222 0.00030984689004785
2643.67777777778 0.000294797238707903
2720.35333333333 0.000280847885567122
2797.02888888889 0.000267892091238778
2873.70444444444 0.000255835924534755
2950.38 0.000244596443662222
3027.05555555556 0.000234100173956748
3103.73111111111 0.00022428182784508
3180.40666666667 0.000215083223719205
3257.08222222222 0.000206452368966692
3333.75777777778 0.000198342679118299
3410.43333333333 0.000190712310372976
3487.10888888889 0.000183523586965595
3563.78444444444 0.000176742508198227
3640.46 0.000170338322647148
3717.13555555556 0.000164283159227277
3793.81111111111 0.000158551706552902
3870.48666666667 0.000153120933463241
3947.16222222222 0.000147969844749638
4023.83777777778 0.000143079267079923
4100.51333333333 0.000138431660905273
4177.18888888889 0.000134010954788135
4253.86444444444 0.000129802399132077
4330.54 0.000125792436746081
4407.21555555556 0.000121968588053457
4483.89111111111 0.000118319349072181
4560.56666666667 0.000114834100559913
4637.24222222222 0.000111503026941754
4713.91777777778 0.000108317043829109
4790.59333333333 0.00010526773309953
4867.26888888889 0.000102347284644886
4943.94444444444 9.95484440125243e-05
5020.62 9.68644652644515e-05
5097.29555555556 9.42890684656693e-05
5173.97111111111 9.18164012868122e-05
5250.64666666667 8.94410042700267e-05
5327.32222222222 8.71577793621309e-05
5403.99777777778 8.49619613667946e-05
5480.67333333333 8.28490920088453e-05
5557.34888888889 8.08149963397878e-05
5634.02444444444 7.88557612449387e-05
5710.7 7.69677158399337e-05
5787.37555555556 7.51474135682595e-05
5864.05111111111 7.33916158324103e-05
5940.72666666667 7.16972770096523e-05
6017.40222222222 7.00615307195232e-05
6094.07777777778 6.84816772244376e-05
6170.75333333333 6.69551718573003e-05
6247.42888888889 6.54796143811315e-05
6324.10444444444 6.40527391955093e-05
6400.78 6.26724063133305e-05
6477.45555555556 6.13365930391104e-05
6554.13111111111 6.00433862868941e-05
6630.80666666667 5.87909754819618e-05
6707.48222222222 5.75776459959493e-05
6784.15777777778 5.64017730698612e-05
6860.83333333333 5.52618161837955e-05
6937.50888888889 5.41563138360774e-05
7014.18444444444 5.30838786979904e-05
7090.86 5.20431931134003e-05
7167.53555555556 5.1033004915384e-05
7244.21111111111 5.00521235344894e-05
7320.88666666667 4.90994163755232e-05
7397.56222222222 4.81738054418133e-05
7474.23777777778 4.72742641877312e-05
7550.91333333333 4.63998145819364e-05
7627.58888888889 4.55495243653012e-05
7704.26444444444 4.47225044888507e-05
7780.94 4.3917906718279e-05
};
\addplot [draw=black, fill=black, mark=x, very thick, mark size=2.5pt, only marks]
table{%
x  y
87.6 0.272343533408822
351.36 0.0259470568426133
1450.24 0.00189066552594397
5765.12 0.000144604747120979
};
