# Supplementary material for: Swarm Reinforcement Learning For Adaptive Mesh Refinement
Source: arXiv:2304.00818 source file (2023-10-09)
Supplement: Supplementary file 6 [file group_ablations_2.tex]

\nextgroupplot[
ylabel shift = -0.2cm,
clip marker paths=true,
width=0.52\textwidth,
height=4.5cm,
title style={yshift=-0.2cm},
scaled x ticks=false,
legend cell align={left},
legend style={fill opacity=0.8, draw opacity=1, text opacity=1, draw=lightgray204},
log basis y={10},
tick align=outside,
tick pos=left,
title={Poisson - Num. Training PDEs},
x grid style={darkgray176},
xlabel={Elements \(\displaystyle (\times 10^3)\)},
xmajorgrids,
xmin=-419.152, xmax=9281.792,
xtick style={color=black},
xtick={-2000,0,2000,4000,6000,8000,10000},
xticklabels={-2.0,0.0,2.0,4.0,6.0,8.0,10.0},
y grid style={darkgray176},
ylabel={\empty},
ymajorgrids,
ymin=3.2945347498023e-06, ymax=2.41273251028282,
ymode=log,
ytick style={color=black},
ytick={1e-07,1e-06,1e-05,0.0001,0.001,0.01,0.1,1,10,100},
yticklabels={
\empty
  % \(\displaystyle {10^{-7}}\),
  % \(\displaystyle {10^{-6}}\),
  % \(\displaystyle {10^{-5}}\),
  % \(\displaystyle {10^{-4}}\),
  % \(\displaystyle {10^{-3}}\),
  % \(\displaystyle {10^{-2}}\),
  % \(\displaystyle {10^{-1}}\),
  % \(\displaystyle {10^{0}}\),
  % \(\displaystyle {10^{1}}\),
  % \(\displaystyle {10^{2}}\)
}
]
\addplot [
  draw=royalblue28108204,
  fill=royalblue28108204,
  forget plot,
  mark=*, mark size=1,
  only marks,
  draw opacity=0,
 fill opacity=0.5
]
table{%
x  y
219.22 0.0116380025783674
236.58 0.00893751131252496
255.06 0.00757221773421185
266.3 0.00695152587324572
277.02 0.00870449843080493
289.06 0.00650849332548639
301.82 0.00650772537377039
309.02 0.00632830538267971
313.48 0.00852456067483164
317.48 0.00503420224308783
366.78 0.00472734343816265
384.24 0.00384945126787151
427.52 0.00440570193112838
431.14 0.00387196288409598
433.8 0.0031068838328975
438.92 0.0033561305566538
446.06 0.00325148782214415
485 0.00270934352590588
524.5 0.0019590317268996
530.98 0.0024847849713976
530.98 0.0024462804500235
542.2 0.00339373662958677
568.26 0.00191195330793864
569.1 0.00200759214947172
579.8 0.00192121084682089
587.66 0.00166535004820132
612.06 0.00170099739413765
628 0.00142557999535175
636.98 0.00193167521782833
648.04 0.00147630841918046
648.78 0.00196488850395651
684.76 0.00192456325257735
704.12 0.00152017798836435
708.02 0.00171515266408961
724.56 0.00106290863523144
740.7 0.00145038634314574
740.82 0.00126611233262213
754.68 0.0010958404611985
776.14 0.00136681288549904
861 0.00122261947029662
866.82 0.0012376456173406
951.18 0.000684639740045543
978.82 0.000682995459645206
1030.58 0.000639142132617508
1031.2 0.000608987227553708
1080.16 0.000534351174466062
1116.56 0.000522936657826564
1126.22 0.00047220578013082
1173.32 0.000587407673606018
1183.24 0.000496992672901857
1212.6 0.000433759599768057
1270.84 0.000477030829124065
1271.28 0.00057574970357699
1312.64 0.000295338105933881
1334.88 0.0003688460635094
1390.92 0.000632823129081481
1414.42 0.000439822660083419
1465.2 0.000380405825070989
1546.18 0.000259777992401812
1645.64 0.000189432782231567
1650.1 0.00040730379394757
1712.26 0.000225696747843442
1799.62 0.000205137266591349
1800.64 0.000149688394684308
1820.82 0.00022968203197516
1908.42 0.000134858938308452
1925.1 0.000231468966668099
2020.12 0.000123482420852495
2156.38 0.000114435638078513
2168.78 0.000132258579214635
2169 0.000101440195225082
2212 0.000202015930911123
2238.3 0.000100444720362762
2307.32 0.00010430451268494
2321.26 0.000101348576943888
2363.12 7.85396281013735e-05
2399.82 8.97496755911525e-05
2432.68 0.000175103698214891
2457.16 9.48685731254995e-05
2655.7 7.07642905549767e-05
2715.22 5.85765922707877e-05
3044.4 5.85685554721719e-05
3414.76 4.01750628140733e-05
3545.46 3.80019302781983e-05
3591.66 3.62548169075136e-05
3997.22 3.19018762058348e-05
4033.6 2.70246768067793e-05
4075.94 2.55319826966762e-05
4148.74 2.90210310242148e-05
4304.56 2.36833753484687e-05
4311.96 4.28165553247746e-05
4611.22 2.13677683411378e-05
5764.26 1.3085878413959e-05
6013.74 1.0832458588431e-05
6168.52 9.73742044189171e-06
6591.82 8.02970379055727e-06
6800.42 8.43665609892419e-06
6819.78 8.29434337198603e-06
7381.26 8.13257734004449e-06
7648.78 6.34432528857979e-06
};
\addplot [draw=purple11522131, fill=purple11522131, forget plot, mark=*, mark size=1, only marks, draw opacity=0,
 fill opacity=0.5]
table{%
x  y
21.8 0.999999998844615
21.92 0.999999998950274
21.94 0.999999998905941
21.96 0.99999999888399
21.96 0.99999999888399
30.3 0.955115926525863
97.88 0.287048732748639
99.32 0.181889060496395
169.12 0.531132366867216
177.6 0.545020912138967
187.64 0.376775872350981
420.22 0.438636973557918
501.16 0.0250090737165922
591.34 0.267126864756588
631.64 0.0115761597308923
724.44 0.0031624616802585
761.36 0.00391950049930072
790.68 0.225096761541945
809.56 0.00254649272528214
833.22 0.00148358504568688
840.98 0.0018855619100576
852.94 0.00173984633925338
863.34 0.00137587777389848
885.1 0.00152978362809917
893.8 0.00283159716841115
900.12 0.0011581645530242
981.86 0.00100371705184928
1091.92 0.00148852079076812
1135.62 0.00108166711135929
1202.06 0.000689375037398485
1215.78 0.0014180334877725
1255.86 0.00151518966363459
1267.08 0.134157054547184
1272.68 0.000942390441828918
1275.54 0.00174992946883269
1313.62 0.000840331900689179
1331.7 0.000593727400159513
1343.48 0.000512112134314816
1373.44 0.00951457393453667
1386.3 0.313665674559799
1388.32 0.260162263083804
1500.86 0.00047713348638261
1520.3 0.00071738520325115
1610.24 0.000318674290798788
1767.14 0.000332371371964025
1814.58 0.000526983911996808
1830.68 0.00038142972209416
1917.46 0.00156015840477675
1928.32 0.000202250054529467
2249.24 0.000232164733573201
2803.34 0.000154596173220414
2809.94 0.000125463231975432
2979.76 0.000163825748619834
3013.06 0.00025215070873185
3232.68 0.00439376692350953
3324.9 0.00047979742396379
3894.5 0.000132072282354921
3984.48 0.00019801196014849
4162.44 0.000172169579399523
4202.02 9.96813532467877e-05
4302.44 8.56922150846815e-05
4385.92 0.000246344465972347
4424.12 6.06989680535098e-05
4504.42 6.35874216163741e-05
4516.44 0.11409288261005
4608.02 0.000104676671106279
4688.64 4.16809849734583e-05
4720.12 3.87609921791037e-05
5071.76 0.000137166384561248
5109.36 2.28042951428577e-05
5343.86 1.85296476023598e-05
5382.82 6.95841144613072e-05
5399.52 2.65494439641189e-05
5405.74 3.42114285184063e-05
5410.32 3.23869934707441e-05
5898.44 3.94790229070543e-05
6086.36 2.37045127328663e-05
6397.04 3.21805719181968e-05
7619.2 1.53937665295237e-05
8193.36 1.87380663194453e-05
8840.84 1.9440339417203e-05
};
\addplot [draw=plum223165229, fill=plum223165229, forget plot, mark=*, mark size=1, only marks, draw opacity=0,
 fill opacity=0.5]
table{%
x  y
193.86 0.0135415011326246
210.48 0.0133710055152162
244.9 0.0136773227294141
253.7 0.010960960859964
300.6 0.0072624613018336
316.1 0.00641642234906269
340.98 0.00489862538737564
355.02 0.00584426748373136
355.86 0.00622645252042319
402.12 0.00380434456742319
428.02 0.00403767442585351
438.52 0.0233335234028789
451.34 0.00300906110136661
458.9 0.00361487100077389
459 0.00772124755353511
464.58 0.00343112202154649
466.18 0.00411922433967292
470.1 0.00420567235154739
473.56 0.00301727351835417
479.92 0.00332395055076257
497.58 0.00279558307955556
501.4 0.00430373725343986
522.26 0.00245476448728294
537.16 0.00222388942549427
548.72 0.00225110030551122
578.98 0.00238750312607103
593.86 0.00249013647725441
619.48 0.00213143560649043
621.54 0.00180165485655061
666.96 0.00169777341298222
690.62 0.00180508854245135
697.08 0.00161761935591147
725.74 0.00118851086311835
755.36 0.00139724781523819
796.12 0.00105224879753276
864.56 0.00109129192905817
892.08 0.00121098460348252
997.2 0.000760614571734043
1113.72 0.00080070588524008
1165.04 0.000698275056820021
1185.68 0.000693671377303586
1197.78 0.000734372963201111
1198.28 0.000553227429281712
1220.96 0.0005934125405331
1286.3 0.000363492283277366
1290.48 0.000374817375794496
1292.08 0.00246719176871407
1320.36 0.000482189705198149
1353 0.000624893268603678
1366.58 0.000501786537945663
1476.04 0.000268160060864321
1476.5 0.000366435935152945
1517.22 0.000449688083441169
1519.86 0.00030641780880371
1551.72 0.000312624339322874
1592.88 0.000324851450331191
1610.46 0.000361379802542127
1702.22 0.000219144137453209
1855.12 0.000232703372551635
1869.96 0.000229071269121167
1876.64 0.000184857505007458
1898.06 0.000158339687197343
1949.52 0.00020784903630608
1983.56 0.000187866894438557
2105.16 0.000623088621498017
2159.72 0.000128840100125129
2185.92 0.000172012947549241
2264.48 0.000221620746580485
2278.5 0.000794745244387168
2327.34 0.000123061695274915
2362.38 0.000105190722944063
2384.5 0.000128881704865874
2505.62 0.000107977825671389
2839.88 7.85645407394983e-05
2901.06 5.37839754701565e-05
2931.22 6.41154148887755e-05
2973.42 6.31142345910785e-05
3064.36 0.000118807318695851
3401.34 5.56060369215685e-05
3592.34 4.16819804803639e-05
3623.66 4.26596179645136e-05
3771.28 5.75995135710313e-05
3815.46 3.92867780698185e-05
3984.5 7.29536406153362e-05
4174.92 2.99129487155668e-05
4367.86 2.61552673993048e-05
4787.46 2.86797501602571e-05
4862.82 2.04005534695789e-05
4920.36 5.56959098657463e-05
5169.2 7.82894062317636e-05
5378.96 2.03729893155251e-05
6153.86 1.1748414787208e-05
6383.74 2.55017944296395e-05
7022.32 1.10217139511226e-05
7133.76 1.21421800173281e-05
7183.26 8.86532175214317e-06
7664.92 9.30597932513595e-06
};
\addplot [
  draw=deepskyblue33188255,
  fill=deepskyblue33188255,
  forget plot,
  mark=*, mark size=1,
  only marks,
  draw opacity=0,
 fill opacity=0.5
]
table{%
x  y
232.44 0.0102145056237603
242.06 0.00772937514502982
248.28 0.00803684823057169
256.82 0.00910298830885816
263.6 0.00703046042465421
267.48 0.00757499472990293
267.52 0.00698477290863836
274.18 0.00744377881991286
275.66 0.00687043198379113
284.46 0.00594327768745318
350.06 0.00463677884014436
373.2 0.00456881637759607
380 0.00372822518800129
381.98 0.00370373800394192
392.4 0.00333597564313756
396.06 0.00408528583696487
412.84 0.00355461995691588
419.26 0.00366055746249258
437.06 0.00293642549508351
463.2 0.00281193912922212
465.54 0.00307584043220076
489.16 0.00245114524409103
534.92 0.00223994923314306
537.2 0.0021355213003277
541.56 0.00179825364400211
552.74 0.00212799575211299
582.78 0.0021756890699821
592.42 0.00202939414947846
596.72 0.00203464478710716
609.06 0.0017681140583195
624.1 0.00215425571005315
626.06 0.00208709310640201
675.7 0.00154354837750689
678.62 0.00161901883638993
689.66 0.00144212357805865
698.44 0.00134931503424467
740.28 0.00141358186689218
743.84 0.00123604062745275
762.3 0.00150676113145924
816.32 0.00112667348078017
890.56 0.000851316777752317
960.56 0.000834782689664723
973.34 0.000755399539137546
990.58 0.000693478583386397
1018.16 0.000744236542086434
1033.9 0.000600214963632465
1101.54 0.000562729514020439
1154.26 0.000526793508728487
1199.76 0.000426705334038905
1217.12 0.000536742890617672
1223.2 0.000412563326452338
1275.9 0.000404149229376146
1335.04 0.000330030099916982
1392.14 0.00053617071337871
1399.62 0.000324153042156614
1420.06 0.000331443383683338
1424.58 0.000478012557117557
1461.82 0.000313277359416343
1501.84 0.000396548791601051
1536.84 0.000218580751719588
1696.48 0.000248870857910407
1698.68 0.000202708199799553
1709.08 0.000199398799386926
1800.3 0.00015275069897752
1811.8 0.000216410091258093
1816.3 0.000166791361429974
1853.32 0.000176270720003868
1899.86 0.000153682942243057
1938.36 0.000137717594517831
1944.9 0.000140174870352484
1951 0.000150236463461802
1975.1 0.000184518186328756
1988.46 0.000242368453271074
2095.88 0.000133788776859591
2128.5 0.000138464242013216
2170.96 0.000108966782016599
2314.4 0.00010522389511318
2324.46 8.41675506536385e-05
2549.94 7.16980897789443e-05
2561.92 8.76552224788918e-05
2569.88 6.41382470264373e-05
2694.5 6.39339258260217e-05
2918.52 4.84825687703924e-05
3173.5 4.76670716880777e-05
3187.34 4.61559461763136e-05
3233.92 4.08347107180672e-05
3309.8 4.05565351329935e-05
3394.18 4.0982871584673e-05
3816.7 3.28791274408339e-05
4309.94 2.17692694880159e-05
4662.52 1.81739750528463e-05
4687.66 2.05262043066135e-05
4737.86 2.02478682764166e-05
4949.1 2.06803355923794e-05
5130.7 1.6943903738377e-05
5155.34 1.93704974021588e-05
5844.32 1.04522223392946e-05
6036.84 1.23957439159868e-05
6111.74 1.10251960008151e-05
7179.9 7.73442165846026e-06
};
\addplot [very thick, royalblue28108204]
table {%
219.22 0.011036362330508
294.266060606061 0.00683752177615596
369.312121212121 0.00464144864349475
444.358181818182 0.00334666716525019
519.404242424242 0.0025193038327363
594.450303030303 0.00195898836228103
669.496363636364 0.00156242272863255
744.542424242424 0.00127184853740656
819.588484848485 0.00105288309708372
894.634545454545 0.000884011430865333
969.680606060606 0.000751210162546177
1044.72666666667 0.000645022898528129
1119.77272727273 0.000558886634562944
1194.81878787879 0.000488132454642395
1269.86484848485 0.000429366813814566
1344.91090909091 0.000380076270852898
1419.95696969697 0.000338367971794018
1495.00303030303 0.0003027951072934
1570.04909090909 0.000272236981973959
1645.09515151515 0.000245815016365929
1720.14121212121 0.000222832893735278
1795.18727272727 0.000202733241627402
1870.23333333333 0.000185065832838411
1945.27939393939 0.000169463938324359
2020.32545454545 0.000155626532140522
2095.37151515152 0.000143304752953709
2170.41757575758 0.00013229149937599
2245.46363636364 0.000122413358503866
2320.5096969697 0.00011352428972744
2395.55575757576 0.00010550064185257
2470.60181818182 9.82371921850629e-05
2545.64787878788 9.16439755603686e-05
2620.69393939394 8.56437288176314e-05
2695.74 8.01698183332399e-05
2770.78606060606 7.51645493600184e-05
2845.83212121212 7.05777791330937e-05
2920.87818181818 6.63657731597201e-05
2995.92424242424 6.24902573397632e-05
3070.9703030303 5.89176286642295e-05
3146.01636363636 5.56182950054424e-05
3221.06242424242 5.25661205236171e-05
3296.10848484848 4.97379578968152e-05
3371.15454545455 4.71132522503113e-05
3446.20060606061 4.46737045530535e-05
3521.24666666667 4.24029845402706e-05
3596.29272727273 4.02864850465218e-05
3671.33878787879 3.83111110946094e-05
3746.38484848485 3.64650982610337e-05
3821.43090909091 3.47378557882919e-05
3896.47696969697 3.31198306849694e-05
3971.52303030303 3.16023896826275e-05
4046.56909090909 3.01777164323574e-05
4121.61515151515 2.88387217459749e-05
4196.66121212121 2.75789650348172e-05
4271.70727272727 2.63925853870252e-05
4346.75333333333 2.52742409632466e-05
4421.79939393939 2.42190555898078e-05
4496.84545454546 2.32225715948118e-05
4571.89151515152 2.22807080720926e-05
4646.93757575758 2.13897238752291e-05
4721.98363636364 2.05461847426933e-05
4797.0296969697 1.97469340388092e-05
4872.07575757576 1.89890666660709e-05
4947.12181818182 1.8269905764614e-05
5022.16787878788 1.75869818659648e-05
5097.21393939394 1.69380142120492e-05
5172.26 1.63208939879861e-05
5247.30606060606 1.57336692494166e-05
5322.35212121212 1.51745313528374e-05
5397.39818181818 1.46418027212986e-05
5472.44424242424 1.41339257984621e-05
5547.4903030303 1.3649453061884e-05
5622.53636363636 1.31870379818742e-05
5697.58242424242 1.2745426825751e-05
5772.62848484848 1.23234512190284e-05
5847.67454545455 1.19200213852963e-05
5922.72060606061 1.15341199954871e-05
5997.76666666667 1.1164796565038e-05
6072.81272727273 1.08111623443141e-05
6147.85878787879 1.04723856536745e-05
6222.90484848485 1.0147687619861e-05
6297.95090909091 9.83633827504848e-06
6372.99696969697 9.53765298401601e-06
6448.04303030303 9.25098916853041e-06
6523.08909090909 8.97574330125288e-06
6598.13515151515 8.71134814433109e-06
6673.18121212121 8.45727021036785e-06
6748.22727272727 8.21300742570822e-06
6823.27333333333 7.97808697798452e-06
6898.31939393939 7.75206333164318e-06
6973.36545454545 7.53451639676642e-06
7048.41151515152 7.32504983792122e-06
7123.45757575758 7.12328951103846e-06
7198.50363636364 6.92888201746202e-06
7273.5496969697 6.74149336532551e-06
7348.59575757576 6.56080772932964e-06
7423.64181818182 6.38652630081431e-06
7498.68787878788 6.21836622075785e-06
7573.73393939394 6.05605958900093e-06
7648.78 5.89935254359227e-06
};
\addplot [very thick, purple11522131]
table {%
21.8 1.30402265583594
110.881212121212 0.238634521213421
199.962424242424 0.0990394814912923
289.043636363636 0.0532385225907315
378.124848484849 0.0327087595346647
467.206060606061 0.021835646412651
556.287272727273 0.0154342026085804
645.368484848485 0.0113769729919177
734.449696969697 0.00866113396382379
823.530909090909 0.00676478180132582
912.612121212121 0.00539524724884808
1001.69333333333 0.00437852071229657
1090.77454545455 0.00360614215127733
1179.85575757576 0.00300782300867438
1268.93696969697 0.00253649616883847
1358.01818181818 0.00215975161231506
1447.09939393939 0.00185472715047158
1536.18060606061 0.00160495242311992
1625.26181818182 0.00139833961989424
1714.34303030303 0.00122586991053743
1803.42424242424 0.00108071432443984
1892.50545454545 0.000957632965077436
1981.58666666667 0.000852556665456269
2070.66787878788 0.00076229071038531
2159.74909090909 0.000684301761113716
2248.8303030303 0.000616562456477102
2337.91151515152 0.000557436616138867
2426.99272727273 0.00050559343237819
2516.07393939394 0.000459942629218054
2605.15515151515 0.000419584970083174
2694.23636363636 0.000383774126365876
2783.31757575758 0.00035188704248826
2872.39878787879 0.000323400716615054
2961.48 0.000297873869463851
3050.56121212121 0.000274932368793451
3139.64242424243 0.000254257562336432
3228.72363636364 0.000235576879823312
3317.80484848485 0.000218656217694678
3406.88606060606 0.000203293733620788
3495.96727272727 0.000189314762907417
3585.04848484849 0.000176567632947309
3674.1296969697 0.000164920200567748
3763.21090909091 0.000154256974382157
3852.29212121212 0.000144476712952118
3941.37333333333 0.000135490411811913
4030.45454545455 0.000127219609755424
4119.53575757576 0.000119594958390894
4208.61696969697 0.00011255500969846
4297.69818181818 0.000106045184830526
4386.7793939394 0.000100016894170939
4475.86060606061 9.44267840927983e-05
4564.94181818182 8.9236090216322e-05
4654.02303030303 8.44100804908751e-05
4743.10424242424 7.99175742824443e-05
4832.18545454546 7.57305259745404e-05
4921.26666666667 7.18236634926618e-05
5010.34787878788 6.81741737232775e-05
5099.42909090909 6.47614280836671e-05
5188.5103030303 6.15667425611942e-05
5277.59151515152 5.85731674213007e-05
5366.67272727273 5.57653025161336e-05
5455.75393939394 5.3129134737009e-05
5544.83515151515 5.0651894665515e-05
5633.91636363636 4.83219299074787e-05
5722.99757575758 4.61285929554635e-05
5812.07878787879 4.40621417305171e-05
5901.16 4.21136512120436e-05
5990.24121212121 4.02749347836778e-05
6079.32242424242 3.85384741092998e-05
6168.40363636364 3.68973565121246e-05
6257.48484848485 3.53452189654854e-05
6346.56606060606 3.38761979201382e-05
6435.64727272727 3.24848842926564e-05
6524.72848484849 3.11662830252813e-05
6613.8096969697 2.99157767015315e-05
6702.89090909091 2.87290927657454e-05
6791.97212121212 2.76022739499926e-05
6881.05333333333 2.65316515597017e-05
6970.13454545455 2.55138213109715e-05
7059.21575757576 2.45456214487491e-05
7148.29696969697 2.36241129066201e-05
7237.37818181818 2.27465612965301e-05
7326.4593939394 2.19104205408569e-05
7415.54060606061 2.11133179803847e-05
7504.62181818182 2.03530408102559e-05
7593.70303030303 1.96275237122743e-05
7682.78424242424 1.89348375662587e-05
7771.86545454546 1.82731791357952e-05
7860.94666666667 1.76408616348797e-05
7950.02787878788 1.70363060918102e-05
8039.10909090909 1.64580334354166e-05
8128.1903030303 1.59046572364485e-05
8217.27151515151 1.53748770438133e-05
8306.35272727273 1.48674722614556e-05
8395.43393939394 1.4381296517104e-05
8484.51515151515 1.39152724789419e-05
8573.59636363636 1.34683870805841e-05
8662.67757575758 1.30396871185839e-05
8751.75878787879 1.26282751901492e-05
8840.84 1.22333059418281e-05
};
\addplot [very thick, plum223165229]
table {%
193.86 0.0166040029641322
269.325252525253 0.00966186218446921
344.790505050505 0.00633066500716282
420.255757575758 0.00446714962096038
495.72101010101 0.00331711699355545
571.186262626263 0.00255695405044143
646.651515151515 0.00202825860221528
722.116767676768 0.00164580230170857
797.58202020202 0.00136032514753332
873.047272727273 0.00114170988554647
948.512525252525 0.000970687959193349
1023.97777777778 0.000834460947388817
1099.44303030303 0.000724256042928448
1174.90828282828 0.000633896181102737
1250.37353535354 0.000558929994148779
1325.83878787879 0.000496084160004859
1401.30404040404 0.000442908386610125
1476.76929292929 0.000397539254801897
1552.23454545455 0.000358539498196156
1627.6997979798 0.000324786374446476
1703.16505050505 0.000295392704997865
1778.6303030303 0.000269650095378513
1854.09555555556 0.000246987490874291
1929.56080808081 0.000226940511105752
2005.02606060606 0.000209128475657853
2080.49131313131 0.000193236993643568
2155.95656565657 0.000179004629728105
2231.42181818182 0.000166212591954657
2306.88707070707 0.00015467668397422
2382.35232323232 0.000144240971279289
2457.81757575758 0.000134772757038884
2533.28282828283 0.000126158567339109
2608.74808080808 0.000118300920841763
2684.21333333333 0.000111115712719455
2759.67858585859 0.000104530083113113
2835.14383838384 9.84806703711542e-05
2910.60909090909 9.29121718262493e-05
2986.07434343434 8.77761518651555e-05
3061.5395959596 8.30300499914968e-05
3137.00484848485 7.86363515095437e-05
3212.4701010101 7.45618911241958e-05
3287.93535353535 7.07772657120788e-05
3363.40060606061 6.72563371798834e-05
3438.86585858586 6.39758099932208e-05
3514.33111111111 6.09148708605406e-05
3589.79636363636 5.80548803643048e-05
3665.26161616162 5.5379108176467e-05
3740.72686868687 5.28725049774002e-05
3816.19212121212 5.05215053936384e-05
3891.65737373737 4.83138572395993e-05
3967.12262626263 4.62384731380871e-05
4042.58787878788 4.428530123993e-05
4118.05313131313 4.24452122929752e-05
4193.51838383838 4.07099007472247e-05
4268.98363636364 3.90717979438895e-05
4344.44888888889 3.75239957356966e-05
4419.91414141414 3.60601791352056e-05
4495.37939393939 3.46745667962424e-05
4570.84464646465 3.33618583081468e-05
4646.3098989899 3.21171874292814e-05
4721.77515151515 3.0936080509948e-05
4797.2404040404 2.98144194594389e-05
4872.70565656566 2.87484087005936e-05
4948.17090909091 2.77345456305755e-05
5023.63616161616 2.67695941707891e-05
5099.10141414141 2.58505610436929e-05
5174.56666666667 2.49746744612326e-05
5250.03191919192 2.41393649499209e-05
5325.49717171717 2.33422480722624e-05
5400.96242424242 2.25811088341165e-05
5476.42767676768 2.18538875934148e-05
5551.89292929293 2.11586673080085e-05
5627.35818181818 2.04936619798156e-05
5702.82343434343 1.98572061692996e-05
5778.28868686869 1.92477454689878e-05
5853.75393939394 1.86638278375497e-05
5929.21919191919 1.81040957071508e-05
6004.68444444444 1.75672787865961e-05
6080.1496969697 1.70521874913787e-05
6155.61494949495 1.65577069392984e-05
6231.0802020202 1.60827914569634e-05
6306.54545454545 1.5626459548343e-05
6382.01070707071 1.51877892817117e-05
6457.47595959596 1.47659140558938e-05
6532.94121212121 1.43600187107659e-05
6608.40646464646 1.39693359505603e-05
6683.87171717172 1.35931430516982e-05
6759.33696969697 1.32307588297139e-05
6834.80222222222 1.28815408423519e-05
6910.26747474747 1.25448828081636e-05
6985.73272727273 1.22202122219408e-05
7061.19797979798 1.190698815011e-05
7136.66323232323 1.16046991908189e-05
7212.12848484848 1.13128615848821e-05
7287.59373737374 1.10310174650403e-05
7363.05898989899 1.07587332321457e-05
7438.52424242424 1.04955980479245e-05
7513.98949494949 1.02412224349055e-05
7589.45474747475 9.99523697494286e-06
7664.92 9.75729109852603e-06
};
\addplot [very thick, deepskyblue33188255]
table {%
232.44 0.00931172631524898
302.616363636364 0.00611550288115463
372.792727272727 0.00431474568624407
442.969090909091 0.00319832687490688
513.145454545455 0.0024583845712418
583.321818181818 0.0019430855873874
653.498181818182 0.00157023233565497
723.674545454545 0.00129208227030546
793.850909090909 0.00107933239621526
864.027272727273 0.000913178526398494
934.203636363636 0.000781102063186298
1004.38 0.000674507573889738
1074.55636363636 0.000587335812006033
1144.73272727273 0.000515217107643439
1214.90909090909 0.000454937046606103
1285.08545454545 0.000404089320820817
1355.26181818182 0.000360844374184988
1425.43818181818 0.000323791710757476
1495.61454545455 0.00029183023444664
1565.79090909091 0.000264090605922216
1635.96727272727 0.000239879368963823
1706.14363636364 0.00021863814595512
1776.32 0.000199913435573804
1846.49636363636 0.000183333981452477
1916.67272727273 0.000168593621303701
1986.84909090909 0.000155438153215609
2057.02545454545 0.0001436551807577
2127.20181818182 0.000133066190704671
2197.37818181818 0.000123520320829821
2267.55454545455 0.000114889418969037
2337.73090909091 0.00010706409722948
2407.90727272727 9.99505593614532e-05
2478.08363636364 9.34680334075089e-05
2548.26 8.75466815927087e-05
2618.43636363636 8.21258890423123e-05
2688.61272727273 7.71528551211169e-05
2758.78909090909 7.25814279721806e-05
2828.96545454545 6.83711356131643e-05
2899.14181818182 6.44863767508182e-05
2969.31818181818 6.08957420434664e-05
3039.49454545455 5.75714424241732e-05
3109.67090909091 5.44888256974873e-05
3179.84727272727 5.16259662408875e-05
3250.02363636364 4.89633155037983e-05
3320.2 4.64834032724687e-05
3390.37636363636 4.41705814874022e-05
3460.55272727273 4.20108038602519e-05
3530.72909090909 3.99914357151099e-05
3600.90545454545 3.81010894337082e-05
3671.08181818182 3.63294816608575e-05
3741.25818181818 3.46673090611879e-05
3811.43454545455 3.31061399389277e-05
3881.61090909091 3.16383194611744e-05
3951.78727272727 3.0256886579396e-05
4021.96363636364 2.89555010376975e-05
4092.14 2.77283791008356e-05
4162.31636363636 2.65702368390225e-05
4232.49272727273 2.54762399774225e-05
4302.66909090909 2.44419594617584e-05
4372.84545454545 2.34633320123182e-05
4443.02181818182 2.25366250407656e-05
4513.19818181818 2.16584053906444e-05
4583.37454545455 2.08255114359085e-05
4653.55090909091 2.00350281343481e-05
4723.72727272727 1.92842646861501e-05
4793.90363636364 1.8570734493497e-05
4864.08 1.78921371562622e-05
4934.25636363636 1.72463422725184e-05
5004.43272727273 1.66313748415596e-05
5074.60909090909 1.60454020921629e-05
5144.78545454545 1.54867215804576e-05
5214.96181818182 1.49537504205269e-05
5285.13818181818 1.44450155271566e-05
5355.31454545454 1.39591447643175e-05
5425.49090909091 1.34948589053188e-05
5495.66727272727 1.30509643213601e-05
5565.84363636364 1.26263463246375e-05
5636.02 1.22199631004343e-05
5706.19636363636 1.1830840169876e-05
5776.37272727273 1.14580653314103e-05
5846.54909090909 1.11007840346882e-05
5916.72545454545 1.07581951454745e-05
5986.90181818182 1.04295470645897e-05
6057.07818181818 1.011413416775e-05
6127.25454545454 9.81129353660611e-06
6197.43090909091 9.52040195430912e-06
6267.60727272727 9.24087314164019e-06
6337.78363636364 8.97215521213492e-06
6407.96 8.71372832677232e-06
6478.13636363636 8.46510253070449e-06
6548.31272727273 8.22581575620282e-06
6618.48909090909 7.99543197751801e-06
6688.66545454545 7.77353950471196e-06
6758.84181818182 7.55974940473763e-06
6829.01818181818 7.35369403913752e-06
6899.19454545454 7.15502570871297e-06
6969.37090909091 6.96341539639849e-06
7039.54727272727 6.77855160037018e-06
7109.72363636364 6.60013925013311e-06
7179.9 6.42789869897669e-06
};
\addplot [draw=black, fill=black, mark=x, very thick, mark size=2.5pt, only marks]
table{%
x  y
87.6 0.272343533408822
351.36 0.0259470568426133
1450.24 0.00189066552594397
5765.12 0.000144604747120979
};
