# Supplementary material for: Swarm Reinforcement Learning For Adaptive Mesh Refinement
Source: arXiv:2304.00818 source file (2023-10-09)
Supplement: Supplementary file 7 [file group_additional_metrics_l1.tex]

\nextgroupplot[
ylabel shift = -0.2cm,
clip marker paths=true,
title style={yshift=-0.2cm},
height=4.5cm,
width=0.50\textwidth,
legend cell align={left},
legend style={fill opacity=0.8, draw opacity=1, text opacity=1, draw=lightgray204},
log basis y={10},
tick align=outside,
tick pos=left,
x grid style={darkgray176},
xlabel={\empty},
title={Laplace's Equation},
xmajorgrids,
xmin=-411.724, xmax=9371.324,
xtick style={color=black},
xtick={-2000,0,2000,4000,6000,8000,10000},
xticklabels={-2.0,0.0,2.0,4.0,6.0,8.0,10.0},
y grid style={darkgray176},
ylabel={Mean Error},
ymajorgrids,
ymin=0.00376150929044291, ymax=1.35511395197336,
ymode=log,
ytick style={color=black},
ytick={0.0001,0.001,0.01,0.1,1,10,100},
yticklabels={
  \(\displaystyle {10^{-4}}\),
  \(\displaystyle {10^{-3}}\),
  \(\displaystyle {10^{-2}}\),
  \(\displaystyle {10^{-1}}\),
  \(\displaystyle {10^{0}}\),
  \(\displaystyle {10^{1}}\),
  \(\displaystyle {10^{2}}\)
}
]
\addplot [
  draw=royalblue28108204,
  fill=royalblue28108204,
  forget plot,
  mark=*, mark size=1,
  only marks,
  draw opacity=0,
 fill opacity=0.5
]
table{%
x  y
32.96 0.999999999980335
66.36 0.430339546669326
66.46 0.426485917786622
66.6 0.450778962931904
66.68 0.435959598372274
67.8 0.429070790905372
69.64 0.413064658702576
71.28 0.412301699719357
71.6 0.39306276628447
75.74 0.383673649501318
101.7 0.315529746412287
118.94 0.239266352090949
121.06 0.222188965945495
125.6 0.260245269704668
126.22 0.23561952310194
130.86 0.246438327345172
132.76 0.245405522663286
135.62 0.228714931893102
136.7 0.223370731159634
138.02 0.235007538725717
273.4 0.110809627789383
274.06 0.109667636129185
292.52 0.103611623074567
298.58 0.103093796222904
300.48 0.108076401568397
314.24 0.0966511378794507
342.9 0.0964885903895576
344.6 0.09053803155886
348.22 0.104059768778813
352.16 0.0892794409093182
352.26 0.0976284462483978
352.8 0.092477892231664
387.38 0.0874291931030886
417.94 0.0822239582287599
426.8 0.0685309819570361
431.1 0.084754975736319
447.76 0.067628026300153
472.62 0.0752749556976965
519.64 0.0652314253734399
553.24 0.0658155655292609
587.06 0.0533863906396037
621.06 0.0539467127501229
640.9 0.0525548677763478
680.28 0.0530486419490799
689.02 0.0476028817203121
720.62 0.0480459326769567
766.08 0.0534517645679736
840.4 0.0426693089879357
930.4 0.0371760707908792
946.7 0.0342665390067617
1037.46 0.0362745953270279
1044.34 0.0355227074363928
1065.3 0.0324540692131355
1079.94 0.0322965244844643
1111.66 0.0326003621862768
1180.38 0.0327706539877276
1199.52 0.0316279434885521
1311.86 0.0245497489486174
1333.58 0.0313898834701562
1347.54 0.0318629843042994
1466.54 0.029940510266348
1494 0.0240121458559688
1534.04 0.0270845473663999
1550.9 0.0263821628243207
1684.28 0.0251464177537961
1754.78 0.0231526616569865
1878.7 0.0221944246001957
1893.14 0.0226232259276832
1953.44 0.0221060694935681
2045.58 0.0206606559081359
2259.26 0.0163766470815048
2289.34 0.0208315787036051
2536.3 0.0155158427938726
2925.5 0.0142036413178568
3209.28 0.0122733465909178
3236.04 0.011453090428979
3243.94 0.012377400270363
3293.3 0.0129644874369324
3538.9 0.0116319945206269
3617.08 0.0102859417266389
3679.3 0.0118131142811136
3765.68 0.0114625264847352
3798.76 0.0102239344578191
3816.32 0.0102591545717347
4032.16 0.0110243094255103
4347.24 0.0101336183148293
4379.48 0.0088066523633103
4509.78 0.00833486183273371
4519.06 0.0101600905893347
4784 0.0103358830821879
5117.82 0.0101273288041316
5276.84 0.00795231053887752
6151.78 0.0073081277459253
6857.24 0.00583462400631205
7125.34 0.00974155386862099
7174.8 0.00592616973394494
7392.48 0.00508041329062706
7461.92 0.0062046263159191
7851.68 0.00532292878827244
8408.56 0.00570902973794865
};
\addplot [
  draw=cadetblue80178158,
  fill=cadetblue80178158,
  forget plot,
  mark=*, mark size=1,
  only marks,
  draw opacity=0,
 fill opacity=0.5
]
table{%
x  y
268.78 0.161385620086291
274.26 0.153818037766715
279.9 0.132689566138063
284.84 0.13739950835545
285 0.14446394261981
286.36 0.14380483219367
297.24 0.151054310847592
302.38 0.172974330901603
309.04 0.138221716884235
330.78 0.126137454217282
472.7 0.0748524325464641
476.04 0.0743736018587619
508.96 0.10483028193192
516.56 0.135742099887855
521.14 0.0940186157187524
529.98 0.106840315720035
532.12 0.0832562344335797
538.56 0.0773985454041797
552.34 0.0996900570269834
608.08 0.0790023867072234
675.86 0.0860989262391039
707.88 0.088691407875646
723.56 0.08757238174092
742.4 0.0979001995031942
753.4 0.12412686250815
764.86 0.071526779694894
774.8 0.550085617653593
804.1 0.109047496565896
835.32 0.101688432459328
856.52 0.12836013355056
881.56 0.0738326419725011
887.64 0.119162520854932
891.82 0.101708019870122
904.2 0.116954082871802
908.08 0.0529117417226256
913.84 0.097526788969931
945.1 0.0501990239338428
958.36 0.0645462424878606
980.64 0.106412133446946
1000.58 0.110395897841918
1024.56 0.10725889100252
1031.5 0.106421090263841
1129.7 0.0529437314062433
1195 0.0528058616832717
1299.44 0.0293713117316865
1318.3 0.030015453539135
1328.56 0.027792081622906
1343.12 0.0425302098926684
1355.4 0.0894401928183229
1377.76 0.109024598292888
1426.62 0.0891206752096294
1453.92 0.0593330899150381
1582.56 0.0215459391095694
1633.74 0.0261081378419666
1636.12 0.0504681945144476
1641.32 0.0475052597320227
1682.42 0.0225424000353418
1702.24 0.0292369138282909
1729.48 0.0248223022019965
1784.38 0.0296986450055815
1870.06 0.0438263929297226
1878.72 0.0490276277254726
1896.8 0.0898894602737799
1946.16 0.0305705067731328
2076.58 0.0805572584837821
2097.52 0.0288868099750555
2105.22 0.200376570212317
2239.36 0.118981323704686
2264.62 0.0302794390524194
2289.72 0.0277573102156238
2316.66 0.0197100337053932
2355.28 0.0157963506363045
2374.32 0.0153451375351787
2399.96 0.083645082030987
2405.02 0.0319932806390875
2470.38 0.0202041792788868
2504.18 0.0292353686531664
2520.12 0.0164618816262922
2535.44 0.0131241475672375
2573.86 0.0176612716998016
2672.68 0.0361959195692772
2699.24 0.133590647304975
2717.02 0.0146412963961953
2738.82 0.0789639035746132
2781.02 0.0345590505072987
2817.26 0.0292203554852285
2831.28 0.0137384116292146
2831.48 0.0684628640844344
2849.98 0.0375026079311836
2910.08 0.097154443997046
2926.62 0.0152897324760686
2963.46 0.0195334288722926
3227.14 0.0135261771600207
3275.26 0.0559554818029536
3301 0.038763087781927
3367.86 0.0266376422900299
3386.36 0.0125135134778225
3411.62 0.0491674502531576
3505.26 0.0136750486677473
3695.54 0.0266213331404097
};
\addplot [
  draw=chocolate21910927,
  fill=chocolate21910927,
  forget plot,
  mark=*, mark size=1,
  only marks,
  draw opacity=0,
 fill opacity=0.5
]
table{%
x  y
32.96 0.999999999980335
32.96 0.999999999980335
32.96 0.999999999980335
32.96 0.999999999980335
32.96 0.999999999980335
32.96 0.999999999980335
32.96 0.999999999980335
32.96 0.999999999980335
32.96 0.999999999980335
32.96 0.999999999980335
32.96 0.999999999980335
32.96 0.999999999980335
32.96 0.999999999980335
32.96 0.999999999980335
32.96 0.999999999980335
32.96 0.999999999980335
32.96 0.999999999980335
32.96 0.999999999980335
32.96 0.999999999980335
32.96 0.999999999980335
32.96 0.999999999980335
32.96 0.999999999980335
32.96 0.999999999980335
32.96 0.999999999980335
32.96 0.999999999980335
33.64 0.991490642822235
50.92 0.788171280544929
57.82 0.776034853371592
65.62 0.492724202362264
115.96 0.275145411368273
125.98 0.248601757307911
127.78 0.393575482167479
130.88 0.391101139767186
141.2 0.249602092607236
168.04 0.265043394456105
174.94 0.183148725766233
175.56 0.182442976707885
176.98 0.18730481568622
190.02 0.179911627827663
204.66 0.189290537712779
207.72 0.161924626116643
207.86 0.183252547205863
216.14 0.20131660852059
260 0.143621880535998
293.08 0.134127433137295
327.14 0.110030313224311
330.88 0.0981610567195527
357.84 0.151721543502832
371.96 0.1018664435134
410.72 0.0874567457818312
417.18 0.0900415324029797
492.18 0.0699819314808662
529.6 0.0714473817963791
553.6 0.120667367625927
588.8 0.0581344847584519
608.58 0.117830384737993
647.74 0.0953023925893269
653.32 0.0695758313954637
676.38 0.078237501537757
677.64 0.0644138707429182
824.32 0.0589903214577183
938.4 0.0660881159477072
962.54 0.0430247565151487
1070.74 0.037444367680825
1071.96 0.0402578851569897
1275.3 0.0500230955751976
1349.56 0.0370105270442681
1586.58 0.0323888476724747
2637.64 0.0217103692879325
3043.06 0.0611853940831014
4747.98 0.0870278367524813
4755.04 0.818563688301899
8770.08 0.0069048421548667
};
\addplot [draw=purple11522131, fill=purple11522131, forget plot, mark=*, mark size=1, only marks, draw opacity=0,
 fill opacity=0.5]
table{%
x  y
107.26 0.40810330848494
122.94 0.311592499411245
154.68 0.270317930952998
174.7 0.210268187160215
176.84 0.219311988015121
179.42 0.19813065671728
188.94 0.199824129535235
193.8 0.18485650364839
210.94 0.253331077622085
220.76 0.167379440382471
276.34 0.159282649923193
303.26 0.150324533889584
305.16 0.142148902646402
324.84 0.149919604234704
331.72 0.148056194450133
342.26 0.146975831931965
345.74 0.15076699436899
349.48 0.148083764111394
352.96 0.147232282160267
390.82 0.142296837644272
394.62 0.123284489814973
429.04 0.136436289798182
434.36 0.148564911070371
441.04 0.135049187062166
460.3 0.149944739592598
460.5 0.150017663654099
467.64 0.150545239094115
475.62 0.151056365800289
485.12 0.151357084129822
486.28 0.15150564949051
500.7 0.15130505699795
510.3 0.127584649995831
516.4 0.153547746466055
517.54 0.153441004517466
521.7 0.153799516044374
532.16 0.148015883100912
540.32 0.07398982309607
551.58 0.0823873040931089
569.44 0.0733874845682196
675.16 0.0700522408046231
856.1 0.0688954253143714
911.44 0.0718594537178904
913.1 0.0626943831182554
943.64 0.0610407080474825
1057.96 0.0587261236514985
1086.08 0.0600517940645992
1097.22 0.0582255124136369
1178.62 0.0578205805885343
1276.36 0.0571862420357081
1383.96 0.0567749753142874
1406.36 0.0565834295719331
1490.4 0.0564312114035511
1664.1 0.0571003860135792
1798.62 0.0573436259620902
1954.9 0.0580643736635588
2055.34 0.0586756033976203
2065.4 0.0587734743962272
2070.7 0.0587526782918642
2071.22 0.0587675160842404
2088.98 0.0588734862477912
2092.48 0.0588864813979421
2092.8 0.0588871153876441
2092.8 0.0588871153876441
2092.8 0.0588871153876441
2092.8 0.0588871153876441
2092.8 0.0588871153876441
2092.8 0.0588871153876441
2092.8 0.0588871153876441
2092.8 0.0588871153876441
2092.8 0.0588871153876441
2139.08 0.0552346317305046
2285.72 0.0524261134110556
2313.76 0.0523162745083575
2356.38 0.0522118369638222
2463.18 0.0520491720513853
2493.88 0.0522582504000166
2618.06 0.0519997899035233
2641.54 0.052001704258203
2732.6 0.0520109358383984
3065.6 0.0521637125184354
5524.28 0.0205256756128556
6985.64 0.0204413660898113
7016.58 0.0206175018283706
7497.12 0.0206383478143084
7534.84 0.0206955915765632
8041.54 0.0208916954347581
8062.38 0.0208819630368516
8152.72 0.0209207150084562
8257.12 0.0209321257026056
8313.02 0.0209487911760055
8370.58 0.0209850149871891
8385.02 0.0209819237778679
8396.38 0.0209850610344135
8396.72 0.0209851715659037
8396.8 0.0209852007617076
8396.8 0.0209852007617076
8396.8 0.0209852007617076
8396.8 0.0209852007617076
8396.8 0.0209852007617076
8396.8 0.0209852007617076
};
\addplot [draw=black18, fill=black18, forget plot, mark=*, mark size=1, only marks, draw opacity=0,
 fill opacity=0.5]
table{%
x  y
32.96 0.999999999980335
89.06 0.346062565948644
90.96 0.336120606150106
93.58 0.327642333834431
96.22 0.320660086742732
99.24 0.315129348103591
104.52 0.297958376647911
108.84 0.291731362315642
110.92 0.285879085319973
112.6 0.28290787013254
117.76 0.276930887889205
121.46 0.266971807646307
127.7 0.262503314080789
130.44 0.251698308971446
136.98 0.241818332120912
143.22 0.238310441125782
144.82 0.235361850717918
149.5 0.226747887894884
158.28 0.220700970006049
162.46 0.215459067842928
166.12 0.20813677423522
168 0.202010512459825
178.14 0.19559339670512
184.76 0.19256687365078
200.02 0.185204854032834
209.14 0.181561855297813
213.16 0.17384929405806
216.34 0.177681329728982
223.04 0.169350045775965
238.2 0.160762651367098
253.28 0.154978716532749
259.44 0.152492628476801
273.76 0.146278872998635
297.88 0.136236713200526
315.18 0.129127629381908
326.62 0.124230554403099
351.16 0.11792035641183
367.58 0.114739276928865
376.04 0.112864946595617
390.6 0.106723381896161
422.94 0.101276475050717
459.34 0.0947866161903031
483.24 0.090930643923036
505.86 0.0879615707824792
533.24 0.0832902519649282
545.34 0.0815870909216827
584.7 0.0788636525124246
620.8 0.0737715896872021
695.34 0.068155541423808
762.24 0.0647659926137724
823.28 0.0597971945233343
883.4 0.0574464812361362
972.46 0.0511046834144224
1038.98 0.0470575219042502
1141.84 0.0446228912035317
1168.9 0.0427513135835954
1267.18 0.039727480151132
1284.34 0.0386382248886144
1352.86 0.0373435495529734
1508.42 0.0346526946849873
1536.88 0.0330919969373693
1685.88 0.0315126255872096
1844.38 0.0300678436912733
2001.12 0.0275442411118681
2183.96 0.0246631773177478
2453.52 0.022278932168902
2768.52 0.0202270835244657
3069.7 0.0175168013408616
3465.42 0.015705714000706
3714.94 0.0144715321268347
4067.96 0.0133797711900245
4476.74 0.0123448945757583
4938.1 0.0114806563663294
5529.96 0.0106463788624841
5967.68 0.00994329993079568
6922.62 0.00856780572165731
7245.56 0.00776742554442552
7993.36 0.00654056566540328
8673.04 0.00563291482250417
8926.64 0.0049155469827446
};
\addplot [draw=darkgray153, fill=darkgray153, forget plot, mark=*, mark size=1, only marks, draw opacity=0,
 fill opacity=0.5]
table{%
x  y
32.96 0.999999999980335
129.58 0.258246221600811
138.62 0.242970451902533
146.44 0.228350469141208
155.44 0.214832023431631
161.06 0.203065109413656
166.38 0.193474932691583
176.76 0.185285555593526
189.3 0.17805528241755
198.7 0.16799270519411
206.6 0.163048583911212
217.88 0.155602026446508
225.66 0.149541068203233
231.4 0.143932901387223
236.84 0.140849989535587
247.16 0.136312035338192
260.6 0.13055554537897
262.04 0.127973040817812
279.86 0.124049062603987
286.74 0.122426692341225
310.6 0.114575989758087
335.1 0.108699797298728
357.44 0.104505308325835
381.94 0.0990426629787996
405.98 0.0936990179583862
434.78 0.0890283309560312
475.36 0.0836240638978639
491.06 0.08113922522792
511.42 0.0774697614197355
548.62 0.0723773370097717
574.1 0.0693513007115915
597.12 0.0664829675685085
640.9 0.0615637059753741
680.84 0.0578182976330285
721.96 0.0547530430403681
758.26 0.0525858488498398
793.72 0.0499195904525219
836.18 0.0476748449555085
890.94 0.0451891332544572
930.62 0.0427713805323351
959.78 0.0419262405037161
997.54 0.040387433551011
1011.46 0.03914394511346
1068.4 0.0376703697124312
1136.66 0.0362840719288813
1181.46 0.0346158240477405
1240.54 0.0330628703888007
1273.5 0.0319509402734953
1350.56 0.0310455267451471
1426.38 0.0296663544395104
1481.76 0.0282576241309186
1560 0.0267744318593458
1672.96 0.025607856244556
1756.36 0.0245543477915938
1883.66 0.0231008314595368
1961.16 0.0223849081018885
2155.82 0.0203317595770839
2207.68 0.0194018495445246
2356.62 0.018187505084057
2505.78 0.0174744647415106
2670.38 0.0164146923180339
2755.8 0.0157443269292926
2874.8 0.0149986762773821
3049.02 0.014245839140203
3121.64 0.0137244453371722
3221.1 0.0131789701943614
3356 0.0126568272665105
3428.14 0.0124828950244923
3537.94 0.0120610411418207
3708.66 0.0115096902795757
3826.62 0.0111583662561134
3999.1 0.0107545554303015
4094 0.0103523649380904
4297.04 0.00996371017278845
4486.4 0.00960611191446247
4681.36 0.0092834214545766
4899.18 0.00895533956126858
5148.3 0.00854772186362389
5449.08 0.00815118520608631
5774.46 0.00778092535325896
6074.34 0.0074176280312051
6298.74 0.00710368336956384
6602.58 0.00677813705746091
7168.94 0.00637408604599968
7672.1 0.00601560285765009
8338.74 0.00561585020950441
};
\addplot [
  draw=saddlebrown1356716,
  fill=saddlebrown1356716,
  forget plot,
  mark=*, mark size=1,
  only marks,
  draw opacity=0,
 fill opacity=0.5
]
table{%
x  y
524.8 0.153946237773234
568.06 0.129573538061446
569.2 0.131612619541574
571.26 0.12668831986658
580.66 0.122908070539186
595.4 0.119486159812
605.54 0.115593396996593
616.48 0.111903149971852
633.1 0.106474630977512
649.08 0.102126890388985
660.02 0.0968483939190579
680.48 0.0907938619431612
687.5 0.0871372630590944
703.5 0.0809847621710623
721.86 0.0759326973088154
746 0.0718130192372387
761.7 0.0680340505675814
789.72 0.0624193381015835
804.46 0.0592853185954481
818.48 0.0560153128767777
842.16 0.0530927249231236
856.52 0.050918833773716
865.52 0.0494886626069736
886.3 0.0471633040154632
897.68 0.0463346722466286
903.12 0.045353639073169
903.14 0.0457340127901173
918 0.0448148202211418
932.1 0.0442238127281589
939.56 0.0434243176703382
949.54 0.0431833168813815
951.26 0.0423295353332846
953.9 0.0421000090086311
956.82 0.0427915699632023
959.26 0.0418286542086953
962.48 0.0413356539381481
967.4 0.0410915787855189
974.96 0.040360363710313
982.28 0.0407413411277442
988.46 0.0401575533633853
999.06 0.0395981208497352
1001.94 0.0393872871064227
1008.4 0.0390220657310609
1024.18 0.0385923836886959
1029.78 0.0382105872946599
1042.52 0.0378124829138433
1067.82 0.0372612573373586
1089.28 0.0367946418348373
1101.42 0.0363207357684195
1124.76 0.0358808415563502
1138.58 0.0353329308212251
1157.14 0.034912904705656
1187.18 0.0343277726499084
1204.06 0.033693328068574
1239.96 0.0329845091165643
1273.34 0.0323784960467983
1296.6 0.0316588145699229
1328.82 0.0310492434948404
1365.52 0.0303382319444808
1405.72 0.0297530072503556
1448.44 0.0291493408712959
1495.38 0.0284946190920433
1527.28 0.0278962416509419
1576.62 0.0271790438691756
1623.02 0.0264684408163017
1667.08 0.0257747298206779
1738.72 0.0249790883883493
1802.3 0.0243027864438798
1846.38 0.0236130803435218
1894.7 0.0227758132499567
1956.52 0.0221244662749673
2019.44 0.0214044030426906
2085.34 0.0207018743113742
2160.1 0.0200909758463748
2230.14 0.0195946909941539
2306.68 0.0190355312936448
2374.76 0.0184786072917017
2476.64 0.0179192285403796
2554.82 0.017334702322679
2617.3 0.0167533712888482
2698.8 0.0161769824082982
2795.52 0.0156397937333328
2918.56 0.0151245774676437
3056.16 0.0146218926633913
3151.92 0.0141431778814755
3267.62 0.0137176577309027
3356.14 0.0132482302491231
3481.66 0.0128603403543292
3604.74 0.0124645411243151
3728.02 0.0120359806784407
3878.8 0.0116614837039054
4053.68 0.0112372859854573
4208.3 0.0109203280983023
4352.96 0.0105765060926642
4511.16 0.0101892657295551
4669.8 0.00982823653695019
4823.04 0.00949810895593998
4996.94 0.00915235117432221
5183.88 0.00889546978734926
5395.36 0.00862219383769416
};
\addplot [very thick, royalblue28108204]
table {%
32.96 0.859244118712896
117.56202020202 0.258246279118756
202.16404040404 0.156029533259016
286.766060606061 0.113052041988605
371.368080808081 0.0892063824552026
455.970101010101 0.0739747635245339
540.572121212121 0.06337147577157
625.174141414141 0.0555479632064487
709.776161616162 0.0495276844386657
794.378181818182 0.0447452909463709
878.980202020202 0.040850391720786
963.582222222222 0.0376140354962842
1048.18424242424 0.034880169865258
1132.78626262626 0.0325386925155342
1217.38828282828 0.0305096523184967
1301.9903030303 0.0287335601135408
1386.59232323232 0.0271652166769536
1471.19434343434 0.0257696516533965
1555.79636363636 0.0245193755562677
1640.39838383838 0.0233924742365274
1725.0004040404 0.0223712587533544
1809.60242424242 0.0214412902813789
1894.20444444444 0.0205906637245227
1978.80646464646 0.0198094732348723
2063.40848484848 0.0190894078579028
2148.0105050505 0.0184234417286473
2232.61252525253 0.0178055939527636
2317.21454545455 0.0172307405176854
2401.81656565657 0.016694465518024
2486.41858585859 0.0161929424152156
2571.02060606061 0.0157228384760851
2655.62262626263 0.0152812372688996
2740.22464646465 0.0148655753507087
2824.82666666667 0.0144735901988734
2909.42868686869 0.014103277119854
2994.03070707071 0.0137528533766854
3078.63272727273 0.0134207281600573
3163.23474747475 0.0131054773197297
3247.83676767677 0.0128058219968964
3332.43878787879 0.0125206104711962
3417.04080808081 0.0122488026708632
3501.64282828283 0.0119894569002035
3586.24484848485 0.011741718422001
3670.84686868687 0.0115048095986944
3755.44888888889 0.0112780213490807
3840.05090909091 0.0110607057197927
3924.65292929293 0.0108522694051165
4009.25494949495 0.0106521680765577
4093.85696969697 0.0104599014062753
4178.45898989899 0.0102750086871008
4263.06101010101 0.0100970649671658
4347.66303030303 0.00992567762980655
4432.26505050505 0.00976048335990151
4516.86707070707 0.00960114544653748
4601.46909090909 0.00944735137919718
4686.07111111111 0.00929881070078828
4770.67313131313 0.0091552530859878
4855.27515151515 0.00901642661772957
4939.87717171717 0.00888209623834887
5024.47919191919 0.00875204235503301
5109.08121212121 0.00862605958189577
5193.68323232323 0.00850395560327606
5278.28525252525 0.00838555014481645
5362.88727272727 0.0082706740405576
5447.48929292929 0.00815916838573195
5532.09131313131 0.00805088376618935
5616.69333333333 0.00794567955646963
5701.29535353535 0.00784342327947577
5785.89737373737 0.00774399002151634
5870.49939393939 0.00764726189719873
5955.10141414141 0.00755312755927399
6039.70343434343 0.00746148174907889
6124.30545454545 0.00737222488369594
6208.90747474747 0.00728526267637206
6293.5094949495 0.0072005057871034
6378.11151515152 0.00711786950061975
6462.71353535354 0.0070372734292881
6547.31555555555 0.0069586412387089
6631.91757575758 0.00688190039400345
6716.5195959596 0.00680698192499032
6801.12161616162 0.00673382020862647
6885.72363636364 0.00666235276724626
6970.32565656566 0.00659252008127303
7054.92767676768 0.00652426541520329
7139.5296969697 0.00645753465577628
7224.13171717172 0.0063922761613426
7308.73373737374 0.00632844062153575
7393.33575757576 0.00626598092643159
7477.93777777778 0.00620485204445393
7562.5397979798 0.00614501090834996
7647.14181818182 0.00608641630861845
7731.74383838384 0.00602902879382707
7816.34585858586 0.00597281057730369
7900.94787878788 0.00591772544972977
7985.5498989899 0.00586373869720394
8070.15191919192 0.00581081702437931
8154.75393939394 0.00575892848231091
8239.35595959596 0.0057080424006791
8323.95797979798 0.00565812932408139
8408.56 0.00560916095211023
};
\addplot [very thick, cadetblue80178158]
table {%
268.78 0.148980186422425
303.393737373737 0.142300369449721
338.007474747475 0.136123666220473
372.621212121212 0.130413976978581
407.234949494949 0.125130477643123
441.848686868687 0.120232919669751
476.462424242424 0.115683804873284
511.076161616162 0.111449129620246
545.689898989899 0.107498474479684
580.303636363636 0.103804805886122
614.917373737374 0.10034416563485
649.531111111111 0.0970953322849848
684.144848484849 0.0940394934459117
718.758585858586 0.0911599455204711
753.372323232323 0.0884418263915817
787.986060606061 0.0858718811864687
822.599797979798 0.0834382588278133
857.213535353535 0.0811303361457078
891.827272727273 0.0789385661316758
926.44101010101 0.0768543470763755
961.054747474748 0.0748699096430882
995.668484848485 0.0729782192857904
1030.28222222222 0.0711728917722724
1064.89595959596 0.0694481198960744
1099.5096969697 0.0677986097472524
1134.12343434343 0.0662195251598951
1168.73717171717 0.0647064391661765
1203.35090909091 0.0632552914663139
1237.96464646465 0.0618623510752969
1272.57838383838 0.0605241834347135
1307.19212121212 0.0592376213851185
1341.80585858586 0.0579997394844051
1376.4195959596 0.0568078312333326
1411.03333333333 0.0556593888330823
1445.64707070707 0.0545520851534442
1480.26080808081 0.0534837576356189
1514.87454545455 0.0524523938920313
1549.48828282828 0.0514561187981323
1584.10202020202 0.0504931828988613
1618.71575757576 0.0495619519760387
1653.3294949495 0.048660897643105
1687.94323232323 0.0477885888508736
1722.55696969697 0.0469436842027578
1757.17070707071 0.0461249249906532
1791.78444444444 0.045331128873621
1826.39818181818 0.0445611841309877
1861.01191919192 0.0438140444296669
1895.62565656566 0.0430887240526266
1930.23939393939 0.0423842935415944
1964.85313131313 0.0416998757124853
1999.46686868687 0.041034642006728
2034.08060606061 0.0403878091457754
2068.69434343434 0.0397586360596875
2103.30808080808 0.0391464210638302
2137.92181818182 0.0385504992605147
2172.53555555556 0.037970240144852
2207.14929292929 0.0374050453962534
2241.76303030303 0.0368543468389232
2276.37676767677 0.0363176045563769
2310.99050505051 0.035794305146522
2345.60424242424 0.0352839601051695
2380.21797979798 0.0347861043270302
2414.83171717172 0.0343002947143091
2449.44545454545 0.0338261088839509
2484.05919191919 0.0333631439654339
2518.67292929293 0.0329110154817676
2553.28666666667 0.0324693563070174
2587.9004040404 0.0320378156942947
2622.51414141414 0.0316160583686923
2657.12787878788 0.0312037636801333
2691.74161616162 0.0308006248115476
2726.35535353535 0.0304063480381884
2760.96909090909 0.0300206520342559
2795.58282828283 0.0296432672233284
2830.19656565657 0.029273935169389
2864.8103030303 0.0289124080055075
2899.42404040404 0.0285584478974752
2934.03777777778 0.0282118265399151
2968.65151515152 0.0278723246825847
3003.26525252525 0.0275397316847732
3037.87898989899 0.0272138450958622
3072.49272727273 0.0268944702602644
3107.10646464646 0.0265814199451003
3141.7202020202 0.026274513989092
3176.33393939394 0.0259735789712716
3210.94767676768 0.0256784478982083
3245.56141414141 0.0253889599085516
3280.17515151515 0.0251049599937779
3314.78888888889 0.0248262987341114
3349.40262626263 0.0245528320486599
3384.01636363636 0.0242844209588794
3418.6301010101 0.0240209313645418
3453.24383838384 0.023762233831438
3487.85757575758 0.0235082033901041
3522.47131313131 0.0232587193449062
3557.08505050505 0.0230136650928636
3591.69878787879 0.0227729279516364
3626.31252525253 0.0225363989961372
3660.92626262626 0.0223039729032666
3695.54 0.0220755478043019
};
\addplot [very thick, chocolate21910927]
table {%
32.96 1.03696978949646
121.213737373737 0.263092734045391
209.467474747475 0.165309068533259
297.721212121212 0.126968929630522
385.974949494949 0.106332952488462
474.228686868687 0.0933591090072072
562.482424242424 0.084409884326951
650.736161616162 0.0778444304080863
738.989898989899 0.0728117716736733
827.243636363636 0.0688255002736207
915.497373737374 0.0655868616167705
1003.75111111111 0.0629019006637569
1092.00484848485 0.0606390260383264
1180.25858585859 0.0587056946103167
1268.51232323232 0.0570348547868988
1356.76606060606 0.0555766868995572
1445.0197979798 0.05429336953
1533.27353535354 0.0531556504542244
1621.52727272727 0.0521405342135528
1709.78101010101 0.0512296829951191
1798.03474747475 0.0504082860617305
1886.28848484849 0.0496642446184164
1974.54222222222 0.0489875737296098
2062.79595959596 0.0483699565375877
2151.0496969697 0.0478044072465493
2239.30343434343 0.0472850130289506
2327.55717171717 0.0468067340350112
2415.81090909091 0.0463652467480872
2504.06464646465 0.0459568200715533
2592.31838383838 0.0455782164096449
2680.57212121212 0.0452266120316932
2768.82585858586 0.0448995324567359
2857.0795959596 0.0445947996422122
2945.33333333333 0.0443104885261406
3033.58707070707 0.0440448910383506
3121.84080808081 0.0437964861192216
3210.09454545455 0.0435639146032098
3298.34828282828 0.0433459580669526
3386.60202020202 0.0431415209277392
3474.85575757576 0.0429496152218925
3563.1094949495 0.0427693476045564
3651.36323232323 0.0425999082001455
3739.61696969697 0.0424405610019866
3827.87070707071 0.0422906355746953
3916.12444444444 0.0421495198567705
4004.37818181818 0.0420166538961994
4092.63191919192 0.0418915243803738
4180.88565656566 0.0417736598447631
4269.13939393939 0.0416626264636713
4357.39313131313 0.0415580243418711
4445.64686868687 0.0414594842386463
4533.90060606061 0.0413666646662948
4622.15434343434 0.0412792493138837
4710.40808080808 0.041196944754321
4798.66181818182 0.0411194783989006
4886.91555555556 0.0410465966685773
4975.16929292929 0.0409780633555366
5063.42303030303 0.0409136581522546
5151.67676767677 0.0408531753283252
5239.93050505051 0.040796422537948
5328.18424242424 0.0407432197432079
5416.43797979798 0.0406933982401833
5504.69171717172 0.0406467997765586
5592.94545454545 0.0406032757508233
5681.19919191919 0.0405626864843568
5769.45292929293 0.0405249005587417
5857.70666666667 0.0404897942115597
5945.9604040404 0.0404572507847123
6034.21414141414 0.0404271602199942
6122.46787878788 0.0403994185972435
6210.72161616162 0.04037392771092
6298.97535353535 0.0403505946814154
6387.22909090909 0.0403293315978053
6475.48282828283 0.0403100551891017
6563.73656565657 0.0402926865213805
6651.9903030303 0.0402771507184269
6740.24404040404 0.0402633767037889
6828.49777777778 0.0402512969623419
6916.75151515152 0.0402408473196565
7005.00525252525 0.0402319667376332
7093.25898989899 0.0402245971250153
7181.51272727273 0.0402186831615279
7269.76646464647 0.0402141721345088
7358.0202020202 0.0402110137870046
7446.27393939394 0.0402091601764
7534.52767676768 0.0402085655427369
7622.78141414141 0.0402091861859519
7711.03515151515 0.0402109803513345
7799.28888888889 0.0402139081225695
7887.54262626263 0.0402179313217796
7975.79636363636 0.0402230134160397
8064.0501010101 0.0402291194298777
8152.30383838384 0.0402362158633158
8240.55757575758 0.0402442706150489
8328.81131313131 0.0402532529103843
8417.06505050505 0.0402631332336033
8505.31878787879 0.0402738832644282
8593.57252525252 0.0402854758183075
8681.82626262626 0.0402978847902531
8770.08 0.0403110851019846
};
\addplot [very thick, purple11522131]
table {%
107.26 0.296373545116789
190.992727272727 0.214307601983536
274.725454545455 0.174019266703624
358.458181818182 0.14913071631695
442.190909090909 0.131877255787574
525.923636363636 0.119048850008474
609.656363636364 0.109048913978999
693.389090909091 0.100983296449741
777.121818181818 0.0943077427019061
860.854545454545 0.0886698109483357
944.587272727273 0.0838300602105327
1028.32 0.079619471571292
1112.05272727273 0.0759149433744818
1195.78545454545 0.0726244480317994
1279.51818181818 0.0696776526005872
1363.25090909091 0.0670197771244018
1446.98363636364 0.0646074489601636
1530.71636363636 0.0624058299425741
1614.44909090909 0.0603865794089722
1698.18181818182 0.0585263804139424
1781.91454545455 0.0568058541231566
1865.64727272727 0.0552087472188514
1949.38 0.0537213148237317
2033.11272727273 0.0523318457479122
2116.84545454545 0.0510302928782232
2200.57818181818 0.0498079822937905
2284.31090909091 0.0486573820576886
2368.04363636364 0.047571916757499
2451.77636363636 0.0465458174843152
2535.50909090909 0.0455739995283502
2619.24181818182 0.0446519619457261
2702.97454545455 0.0437757045272623
2786.70727272727 0.0429416587205555
2870.44 0.042146629821036
2954.17272727273 0.0413877483257311
3037.90545454545 0.0406624287844881
3121.63818181818 0.0399683348226987
3205.37090909091 0.0393033492726573
3289.10363636364 0.0386655485561772
3372.83636363636 0.0380531806227392
3456.56909090909 0.037464645875421
3540.30181818182 0.0368984806188233
3624.03454545454 0.0363533426449194
3707.76727272727 0.0358279986386111
3791.5 0.0353213131381279
3875.23272727273 0.0348322388288518
3958.96545454545 0.0343598079847078
4042.69818181818 0.0339031249004741
4126.43090909091 0.0334613591825047
4210.16363636364 0.0330337397853542
4293.89636363636 0.032619549698453
4377.62909090909 0.0322181212008952
4461.36181818182 0.0318288316140751
4545.09454545455 0.0314510994917334
4628.82727272727 0.0310843811952716
4712.56 0.0307281678092256
4796.29272727273 0.0303819823577675
4880.02545454545 0.0300453772881965
4963.75818181818 0.0297179321917441
5047.49090909091 0.0293992517357486
5131.22363636364 0.0290889637844721
5214.95636363636 0.0287867176885983
5298.68909090909 0.0284921827258486
5382.42181818182 0.0282050466772225
5466.15454545454 0.0279250145251723
5549.88727272727 0.0276518072615898
5633.62 0.0273851607948486
5717.35272727273 0.0271248249463427
5801.08545454545 0.0268705625280082
5884.81818181818 0.0266221484932342
5968.55090909091 0.0263793691543793
6052.28363636364 0.0261420214608192
6136.01636363636 0.0259099123320834
6219.74909090909 0.0256828580411921
6303.48181818182 0.0254606836437999
6387.21454545454 0.0252432224491878
6470.94727272727 0.0250303155295347
6554.68 0.0248218112642464
6638.41272727273 0.0246175649164269
6722.14545454545 0.0244174382388533
6805.87818181818 0.0242212991070631
6889.61090909091 0.02402902117738
6973.34363636364 0.0238404835679066
7057.07636363636 0.0236555705606867
7140.80909090909 0.0234741713234013
7224.54181818182 0.0232961796491059
7308.27454545454 0.0231214937126475
7392.00727272727 0.0229500158425145
7475.74 0.0227816523069811
7559.47272727273 0.0226163131135021
7643.20545454545 0.0224539118204015
7726.93818181818 0.0222943653599767
7810.67090909091 0.0221375938722107
7894.40363636364 0.0219835205483521
7978.13636363636 0.0218320714836795
8061.86909090909 0.0216831755388202
8145.60181818182 0.0215367642090456
8229.33454545454 0.0213927715010075
8313.06727272727 0.0212511338164197
8396.8 0.021111789842231
};
\addplot [very thick, black18]
table {%
32.96 0.717040204829599
122.795151515152 0.27358978470612
212.630303030303 0.178035660676334
302.465454545455 0.13398009205738
392.300606060606 0.108161910251447
482.135757575758 0.0910425590985419
571.970909090909 0.0787930363884724
661.806060606061 0.069561283576642
751.641212121212 0.0623364465649462
841.476363636364 0.0565176588718438
931.311515151515 0.0517242534396243
1021.14666666667 0.04770282108145
1110.98181818182 0.0442778440533321
1200.81696969697 0.0413237388110572
1290.65212121212 0.0387481783527894
1380.48727272727 0.0364817054341133
1470.32242424242 0.0344710245639802
1560.15757575758 0.0326745332728336
1649.99272727273 0.0310592641152129
1739.82787878788 0.0295987423557492
1829.66303030303 0.028271453761789
1919.49818181818 0.0270597284104693
2009.33333333333 0.0259489140665739
2099.16848484849 0.0249267548745586
2189.00363636364 0.023982918068145
2278.83878787879 0.0231086290131551
2368.67393939394 0.0222963866362137
2458.50909090909 0.0215397392563827
2548.34424242424 0.0208331063313595
2638.17939393939 0.0201716354784152
2728.01454545455 0.0195510868637433
2817.8496969697 0.0189677390205925
2907.68484848485 0.0184183115885642
2997.52 0.0178999015207738
3087.35515151515 0.017409930089877
3177.1903030303 0.016946098613078
3267.02545454545 0.0165063512627411
3356.86060606061 0.0160888436705408
3446.69575757576 0.0156919162960718
3536.53090909091 0.0153140717349972
3626.36606060606 0.014953955301443
3716.20121212121 0.0146103383449783
3806.03636363636 0.0142821038620447
3895.87151515152 0.0139682340409991
3985.70666666667 0.0136677994434927
4075.54181818182 0.0133799495761221
4165.37696969697 0.0131039046477717
4255.21212121212 0.0128389483418288
4345.04727272727 0.0125844214600657
4434.88242424242 0.0123397163176663
4524.71757575758 0.0121042717875863
4614.55272727273 0.0118775689079375
4704.38787878788 0.011659126978979
4794.22303030303 0.0114485000870596
4884.05818181818 0.0112452740018714
4973.89333333333 0.011049063400955
5063.72848484849 0.0108595093817926
5153.56363636364 0.0106762772272318
5243.39878787879 0.0104990543945833
5333.23393939394 0.0103275487026389
5423.06909090909 0.0101614866942011
5512.90424242424 0.0100006121545719
5602.73939393939 0.00984468476890361
5692.57454545455 0.00969347890342761
5782.4096969697 0.00954678249740025
5872.24484848485 0.00940439605418054
5962.08 0.00926613172122367
6051.91515151515 0.00913181244996084
6141.7503030303 0.00900127122757109
6231.58545454545 0.00887435037355383
6321.42060606061 0.00875090089480034
6411.25575757576 0.00863078189355438
6501.09090909091 0.00851386002325972
6590.92606060606 0.00840000898782666
6680.76121212121 0.00828910908032072
6770.59636363636 0.0081810467574921
6860.43151515152 0.00807571424693244
6950.26666666667 0.007973009183971
7040.10181818182 0.00787283427571127
7129.93696969697 0.00777509698986571
7219.77212121212 0.00767970926627531
7309.60727272727 0.00758658724920375
7399.44242424242 0.00749565103867827
7489.27757575758 0.00740682445931201
7579.11272727273 0.00732003484518761
7668.94787878788 0.00723521283951299
7758.78303030303 0.00715229220787691
7848.61818181818 0.00707120966403746
7938.45333333333 0.00699190470727114
8028.28848484849 0.00691431947039576
8118.12363636364 0.00683839857765749
8207.95878787879 0.00676408901174155
8297.79393939394 0.00669133998922929
8387.62909090909 0.00662010284388146
8477.46424242424 0.0065503309171786
8567.29939393939 0.00648197945559686
8657.13454545454 0.00641500551413957
8746.9696969697 0.00634936786568401
8836.80484848485 0.00628502691573778
8926.64 0.00622194462223102
};
\addplot [very thick, darkgray153]
table {%
32.96 0.862526056670901
116.856767676768 0.281249824832813
200.753535353535 0.173055297766003
284.650303030303 0.126237951177448
368.547070707071 0.0998606999856956
452.443838383838 0.0828503674082188
536.340606060606 0.0709325262786799
620.237373737374 0.0620992830448579
704.134141414141 0.0552798422882397
788.030909090909 0.0498497231592788
871.927676767677 0.0454196077782371
955.824444444445 0.0417338863804093
1039.72121212121 0.0386176405070331
1123.61797979798 0.0359470423452813
1207.51474747475 0.0336319172120443
1291.41151515152 0.0316050047725465
1375.30828282828 0.0298150935360505
1459.20505050505 0.0282224890356027
1543.10181818182 0.0267959385912492
1626.99858585859 0.0255104934781161
1710.89535353535 0.0243459907784264
1794.79212121212 0.0232859547114142
1878.68888888889 0.0223167879741914
1962.58565656566 0.0214271674138875
2046.48242424242 0.0206075861402822
2130.37919191919 0.019850002224183
2214.27595959596 0.0191475660729156
2298.17272727273 0.0184944066341251
2382.0694949495 0.0178854621093249
2465.96626262626 0.0173163447122763
2549.86303030303 0.0167832317310807
2633.7597979798 0.0162827771035281
2717.65656565657 0.0158120391293194
2801.55333333333 0.015368420979519
2885.4501010101 0.0149496214317369
2969.34686868687 0.0145535938342922
3053.24363636364 0.0141785117366426
3137.1404040404 0.0138227399539646
3221.03717171717 0.0134848100876478
3304.93393939394 0.013163399719913
3388.83070707071 0.0128573146538787
3472.72747474747 0.0125654736905519
3556.62424242424 0.0122868955291174
3640.52101010101 0.0120206874523101
3724.41777777778 0.0117660355189285
3808.31454545455 0.0115221960339879
3892.21131313131 0.0112884881061518
3976.10808080808 0.0110642871338554
4060.00484848485 0.0108490190874636
4143.90161616162 0.0106421554760563
4227.79838383838 0.0104432089049217
4311.69515151515 0.0102517291443013
4395.59191919192 0.0100672996419277
4479.48868686869 0.00988953442189133
4563.38545454546 0.00971807532073507
4647.28222222222 0.00955258951868622
4731.17898989899 0.00939276732984251
4815.07575757576 0.00923832022011737
4898.97252525253 0.00908897902597657
4982.86929292929 0.00894449235059157
5066.76606060606 0.00880462511709736
5150.66282828283 0.00866915726126108
5234.5595959596 0.0085378825481113
5318.45636363636 0.00841060749900704
5402.35313131313 0.008287150417287
5486.2498989899 0.00816734050207445
5570.14666666667 0.00805101704105639
5654.04343434343 0.00793802867413319
5737.9402020202 0.007828232720773
5821.83696969697 0.00772149456472224
5905.73373737374 0.00761768709043741
5989.63050505051 0.00751669016622804
6073.52727272727 0.00741839016964844
6157.42404040404 0.0073226795511569
6241.32080808081 0.00722945643248496
6325.21757575758 0.00713862423653229
6409.11434343434 0.00705009134593327
6493.01111111111 0.0069637707877327
6576.90787878788 0.00687957994186723
6660.80464646465 0.00679744027137835
6744.70141414141 0.00671727707248725
6828.59818181818 0.00663901924284395
6912.49494949495 0.00656259906642431
6996.39171717172 0.00648795201369472
7080.28848484849 0.00641501655579248
7164.18525252525 0.00634373399158682
7248.08202020202 0.00627404828658912
7331.97878787879 0.00620590592277435
7415.87555555556 0.0061392557584598
7499.77232323232 0.0060740488974629
7583.66909090909 0.00601023856682783
7667.56585858586 0.0059477800024724
7751.46262626263 0.00588663034216202
7835.35939393939 0.00582674852526819
7919.25616161616 0.00576809519881401
8003.15292929293 0.00571063262935091
8087.0496969697 0.00565432462024792
8170.94646464646 0.00559913643400911
8254.84323232323 0.0055450347192655
8338.74 0.0054919874421161
};
\addplot [very thick, saddlebrown1356716]
table {%
524.8 0.131013990348183
573.997575757576 0.110917427013304
623.195151515151 0.0956592066861799
672.392727272727 0.0837763668233974
721.590303030303 0.0743224453038062
770.787878787879 0.066662940204372
819.985454545455 0.0603593644714162
869.18303030303 0.055100639313958
918.380606060606 0.050660970181098
967.578181818182 0.046873137391238
1016.77575757576 0.0436110753694947
1065.97333333333 0.040778222458202
1115.17090909091 0.0382995541385829
1164.36848484848 0.0361160250165318
1213.56606060606 0.0341806206779963
1262.76363636364 0.0324555068610267
1311.96121212121 0.0309099400672176
1361.15878787879 0.0295187152307087
1410.35636363636 0.0282609978850923
1459.55393939394 0.0271194354124521
1508.75151515151 0.0260794734429982
1557.94909090909 0.0251288248375279
1607.14666666667 0.024257053396491
1656.34424242424 0.0234552447095205
1705.54181818182 0.0227157438204789
1754.73939393939 0.0220319445781265
1803.93696969697 0.0213981193007431
1853.13454545455 0.0208092801301962
1902.33212121212 0.0202610654786991
1951.5296969697 0.0197496464820226
2000.72727272727 0.0192716495079079
2049.92484848485 0.0188240916282029
2099.12242424242 0.0184043266195944
2148.32 0.0180099995625342
2197.51757575758 0.0176390084987565
2246.71515151515 0.0172894719124024
2295.91272727273 0.0169597010386634
2345.1103030303 0.0166481761923461
2394.30787878788 0.0163535264583193
2443.50545454545 0.0160745122051144
2492.70303030303 0.015810009978625
2541.90060606061 0.0155589994099498
2591.09818181818 0.0153205518338483
2640.29575757576 0.0150938203650491
2689.49333333333 0.0148780312211296
2738.69090909091 0.0146724761147004
2787.88848484848 0.0144765055656528
2837.08606060606 0.0142895230073861
2886.28363636364 0.0141109795801557
2935.48121212121 0.0139403695206895
2984.67878787879 0.013777226070592
3033.87636363636 0.0136211178372749
3083.07393939394 0.013471645550577
3132.27151515151 0.0133284391661984
3181.46909090909 0.0131911552738027
3230.66666666667 0.0130594747733552
3279.86424242424 0.0129331007881266
3329.06181818182 0.0128117567869364
3378.25939393939 0.0126951848917642
3427.45696969697 0.0125831443498926
3476.65454545454 0.012475410152367
3525.85212121212 0.0123717717828091
3575.0496969697 0.0122720320825673
3624.24727272727 0.0121760062198746
3673.44484848485 0.0120835207521434
3722.64242424242 0.0119944127718004
3771.84 0.0119085291271698
3821.03757575758 0.0118257257108794
3870.23515151515 0.0117458668091102
3919.43272727273 0.0116688245057477
3968.6303030303 0.0115944781361472
4017.82787878788 0.0115227137857911
4067.02545454545 0.0114534238296231
4116.22303030303 0.0113865065082883
4165.42060606061 0.0113218655378963
4214.61818181818 0.0112594097502778
4263.81575757576 0.0111990527610065
4313.01333333333 0.0111407126627366
4362.21090909091 0.0110843117416464
4411.40848484848 0.0110297762149948
4460.60606060606 0.0109770359879913
4509.80363636364 0.0109260244283533
4559.00121212121 0.0108766781570752
4608.19878787879 0.0108289368540752
4657.39636363636 0.0107827430775073
4706.59393939394 0.010738042095638
4755.79151515152 0.0106947817302853
4804.98909090909 0.0106529122109094
4854.18666666667 0.0106123860385243
4903.38424242424 0.010573157858671
4952.58181818182 0.0105351843427622
5001.77939393939 0.0104984240771634
5050.97696969697 0.0104628374594341
5100.17454545455 0.0104283866011963
5149.37212121212 0.0103950352371464
5198.5696969697 0.0103627486397636
5247.76727272727 0.0103314935393049
5296.96484848485 0.010301238048712
5346.16242424242 0.0102719515930819
5395.36 0.0102436048433839
};
\addplot [draw=black, fill=black, mark=x, very thick, mark size=2.5pt, only marks]
table{%
x  y
130.88 0.391101139767192
524.8 0.153946237773243
2092.8 0.058887115387654
8396.8 0.0209852007617188
};
