# Supplementary material for: Swarm Reinforcement Learning For Adaptive Mesh Refinement
Source: arXiv:2304.00818 source file (2023-10-09)
Supplement: Supplementary file 8 [file group_additional_metrics_l2.tex]

\nextgroupplot[
ylabel shift = -0.2cm,
clip marker paths=true,
title style={yshift=-0.2cm},
height=4.5cm,
width=0.50\textwidth,
ylabel={Mean Error},
xlabel={\empty},
title={Poisson's Equation},
clip marker paths=true,
legend cell align={left},
legend style={fill opacity=0.8, draw opacity=1, text opacity=1, draw=lightgray204},
log basis y={10},
tick align=outside,
tick pos=left,
x grid style={darkgray176},
xmajorgrids,
xmin=-423.163, xmax=9362.063,
xtick style={color=black},
xtick={-2000,0,2000,4000,6000,8000,10000},
xticklabels={-2.0,0.0,2.0,4.0,6.0,8.0,10.0},
y grid style={darkgray176},
ymajorgrids,
ymin=0.00154337441262742, ymax=1.38143703176154,
ymode=log,
ytick style={color=black},
ytick={0.0001,0.001,0.01,0.1,1,10,100},
yticklabels={
  \(\displaystyle {10^{-4}}\),
  \(\displaystyle {10^{-3}}\),
  \(\displaystyle {10^{-2}}\),
  \(\displaystyle {10^{-1}}\),
  \(\displaystyle {10^{0}}\),
  \(\displaystyle {10^{1}}\),
  \(\displaystyle {10^{2}}\)
}
]
\addplot [
  draw=royalblue28108204,
  fill=royalblue28108204,
  forget plot,
  mark=*, mark size=1,
  only marks,
  draw opacity=0,
 fill opacity=0.5
]
table{%
x  y
219.18 0.0973460605904213
238.12 0.0828171588902105
256.42 0.0764336144461117
269.14 0.0743667671297548
270.9 0.0847702645880351
289.76 0.069106250844752
296.86 0.0700802124232011
308.4 0.0679916258588892
318.42 0.0625990000766591
319.3 0.0722947064621217
364.1 0.0637420133392389
387.18 0.0578994257562097
421.68 0.0576495894912367
428.8 0.0556658049844392
430.52 0.0484236178734979
443.06 0.0505658468380969
444.62 0.0496419776038366
488.12 0.0452183097007982
522.86 0.0388237909790696
526.8 0.044855033137476
532.74 0.0425347133138973
552.8 0.0541295863194595
568.08 0.0386437176107787
569.44 0.0365997612901989
582.28 0.0379112238951454
583.36 0.0355758933210149
602.7 0.03227206197186
623.54 0.0319918151592389
637.42 0.0377349868678218
644.34 0.0323096946243004
653.44 0.0427406491222493
678.4 0.0416487168990661
707.2 0.0371426713064119
711.02 0.0346853774114005
722.84 0.0277041427908148
732.02 0.0299869052483896
742.58 0.0322260466984204
742.84 0.0292084032074518
785.28 0.0317270082173172
844.36 0.0317352387841973
863.74 0.0304513232948253
938.58 0.0231025993935928
971.44 0.0232661728522498
1026.4 0.0224737755310224
1032.16 0.0224869006317207
1071.44 0.0207402229497386
1105.18 0.0204909650311651
1124.78 0.0197459087283982
1166.14 0.0236538530028521
1187.8 0.0205945538505842
1218.42 0.0189204001805537
1271.18 0.0227837189645915
1272.82 0.0208832620813238
1302.62 0.0160525301826294
1328.46 0.0181214243938365
1371.06 0.0230850152030672
1401.4 0.0199300579202321
1461.14 0.0185117389358533
1524.62 0.0145677645570796
1631.76 0.0188167405417521
1636.42 0.0132012503121757
1705.86 0.014154970792085
1798.86 0.0113957405359571
1802.26 0.0141460656273328
1810.42 0.0149182014160916
1923.8 0.0110336427102804
1945.04 0.0154936896200427
2051.26 0.010333728454396
2141.42 0.00956364681040405
2172.76 0.00844525114109571
2173.16 0.0104173561082714
2242.86 0.00947402907486066
2253.86 0.0141391371368927
2308.98 0.00967677458370818
2325.48 0.00963007464020311
2359.3 0.0081740250343516
2408.1 0.00847261497609961
2427.24 0.0138194545042532
2443.1 0.00933112240586968
2651.56 0.00712923348756251
2696.22 0.0069301813180975
3027.66 0.0067944999318388
3398.78 0.00548665162703757
3489.78 0.00527389092566379
3531.94 0.00562434342354557
3963.3 0.00523940778424421
3997.38 0.00501525100086509
4097.8 0.00452941858916101
4138.2 0.00481802298554439
4315.98 0.00601989910723352
4341.64 0.00445494285048377
4679.2 0.00432566893319388
5776.4 0.00336374927844625
6066.6 0.00334928797252867
6255.62 0.00296002159965198
6562.2 0.00262723242046187
6823.92 0.00276941926752202
6846.44 0.00258891956214876
7379.64 0.00240007119249415
7634.56 0.00210206790454559
};
\addplot [
  draw=cadetblue80178158,
  fill=cadetblue80178158,
  forget plot,
  mark=*, mark size=1,
  only marks,
  draw opacity=0,
 fill opacity=0.5
]
table{%
x  y
238.98 0.143825713258587
259.78 0.139858957610943
267.04 0.180777238890059
268.12 0.152490583685837
275.28 0.206080368035307
295.34 0.12436814766539
300.12 0.137649327771952
305.7 0.129022719716798
331.22 0.228414407760491
350.88 0.253142757804266
387.16 0.213027315916884
427.04 0.0635670549360187
440.72 0.0595171108740263
456.08 0.0784599679273928
499.3 0.0999574116622761
528.08 0.0677847591423064
564.48 0.135851502938688
578.7 0.0743033737608325
622.44 0.0834771732348492
656.82 0.123371795538666
676.44 0.0814892647812072
689.72 0.0388964224509415
697.62 0.0553509621021876
704.3 0.15941186715911
713.46 0.0743238884453014
763.12 0.069072597095672
783.02 0.0847574112178445
788.52 0.0594409518411156
797.78 0.22479240763318
856.48 0.377200147695946
880.18 0.328782694147163
955.78 0.0765958055004915
959.62 0.04143299370588
961.92 0.0827442139632796
966 0.0408621994521437
1003.44 0.048507646382652
1009.66 0.0560038505357456
1033.92 0.0369361152584984
1125.42 0.0425206534702089
1135.5 0.0442110343451333
1198.22 0.0234551413985928
1199.62 0.314488743490787
1237.68 0.100904483726611
1260.02 0.0305624903599764
1305.24 0.0825167644872072
1343.34 0.033100073298613
1442.5 0.350764088498612
1465.78 0.058471625573805
1478.56 0.0383517098005549
1501.94 0.0469341095249521
1551 0.295768195417903
1576.48 0.0363131267180406
1613.9 0.0502024451444174
1652.34 0.04808697305604
1687.7 0.0221681509618419
1764.26 0.0166283335102832
1779.94 0.018200466675005
1959.6 0.0266688907612151
1987.8 0.0393580944899701
2001.56 0.0794422754155379
2014.44 0.0247196544746411
2151.74 0.021166249700584
2211.04 0.0169179910678441
2267.1 0.0537043519078183
2276.52 0.0371492388318527
2316.48 0.416689598180732
2333.88 0.01665421228074
2460.98 0.0183656499947459
2478.84 0.029024267514846
2487.08 0.0172227680796079
2509.94 0.0164654623186325
2511.8 0.0185807039894257
2514 0.0258170592055591
2697.92 0.0352429807289074
2741.78 0.0531862015961485
2796.16 0.0213369103669072
2796.46 0.0188628470002769
2805.52 0.0240913288444364
2809.04 0.263312050828101
2897.04 0.0153956577509994
2953.92 0.12634838033186
2990.56 0.0758824686350854
2995.6 0.0217804602368318
3023.3 0.0333050079788646
3044.72 0.0572698852663463
3141.72 0.0098153648224868
3184.04 0.0300996870636207
3187.12 0.098527017880148
3280.98 0.0108667151880465
3281.92 0.0122779601890539
3290.56 0.00762841483486953
3305.14 0.0221903239007364
3339.4 0.0219211257936046
3372.38 0.0086067821218794
3460.44 0.0108813957845498
3692.98 0.0119818497514704
3707.82 0.0171350201697883
3788.4 0.141162709501631
3851.82 0.0148655891106172
4036.14 0.0542085226729007
};
\addplot [
  draw=chocolate21910927,
  fill=chocolate21910927,
  forget plot,
  mark=*, mark size=1,
  only marks,
  draw opacity=0,
 fill opacity=0.5
]
table{%
x  y
21.62 0.999999999946257
21.94 0.99999999994621
21.94 0.99999999994621
21.94 0.99999999994621
21.94 0.99999999994621
21.98 0.999999999947385
21.98 0.999999999947385
21.98 0.999999999947385
21.98 0.999999999947385
21.98 0.999999999947385
21.98 0.999999999947385
21.98 0.999999999947385
21.98 0.999999999947385
21.98 0.999999999947385
21.98 0.999999999947385
21.98 0.999999999947385
21.98 0.999999999947385
21.98 0.999999999947385
21.98 0.999999999947385
21.98 0.999999999947385
21.98 0.999999999947385
21.98 0.999999999947385
21.98 0.999999999947385
21.98 0.999999999947385
21.98 0.999999999947385
21.98 0.999999999947385
21.98 0.999999999947385
21.98 0.999999999947385
21.98 0.999999999947385
21.98 0.999999999947385
21.98 0.999999999947385
21.98 0.999999999947385
21.98 0.999999999947385
21.98 0.999999999945819
21.98 0.999999999947385
21.98 0.999999999947385
22.02 0.99999999994686
22.06 0.999999999935702
22.06 0.999999999940137
22.1 0.999999999946792
26.76 0.983487948423689
29.44 0.945915160040805
32.74 0.916582483151734
92.76 0.777688326991958
98.12 0.379800795652663
127.7 0.774117578836904
136.86 0.224305992688413
137.28 0.205526744544644
149.08 0.19425357113539
203.62 0.370669156906357
253.14 0.172528553651518
269.48 0.131545159456555
271.84 0.180563785120998
276.02 0.164437579325448
308.32 0.398630778220885
338.74 0.138354631854554
342.64 0.101627235703601
354.8 0.0792026947001298
386.76 0.0532886091577981
401.7 0.0773342094271383
418.92 0.0886991411158758
430.88 0.125619228615446
527.84 0.280686934351854
631.64 0.0457892612138262
680.68 0.0470901957437581
700.04 0.0408753429140694
708.38 0.648228000612585
782.36 0.0539846853461908
1009.7 0.134989190902982
1168.3 0.115031026940184
1243.2 0.0236954460432344
1262.06 0.025579109317322
1269.36 0.0205551497143709
1346.86 0.019260675442718
1386.16 0.0255964184181269
1648.32 0.120155067349954
1929.3 0.0829202290487376
2006.58 0.0109415720325125
2041.68 0.0131605937162021
2114.96 0.310559819285065
2245.4 0.391014541350035
3247.16 0.00805620407251461
3548.74 0.0150944719536972
4152.08 0.021459538440929
4432.4 0.0112210129910777
4885.76 0.00947819198197417
5010.6 0.00531992010846068
7456.42 0.00559030970195098
};
\addplot [draw=purple11522131, fill=purple11522131, forget plot, mark=*, mark size=1, only marks, draw opacity=0,
 fill opacity=0.5]
table{%
x  y
78.62 0.481924214270777
85.94 0.441572369286234
87.34 0.456407908815635
104.64 0.306662588413135
115.14 0.310411931588745
116.28 0.353610364865927
121.46 0.265138267272263
125.6 0.268660309185678
137.24 0.285770570719013
195.76 0.2432208483152
209.7 0.202164332051236
223.68 0.196581871554813
240.72 0.173988832224467
306.04 0.186114528199343
306.56 0.156082056871787
323.62 0.107549331495117
334.42 0.120391097577896
340.56 0.118393185863639
341.82 0.0764994449591297
342.12 0.121666274841628
343.48 0.117824081118163
349.4 0.116121814349164
350.84 0.117636857252407
352.78 0.0997981111482906
353.14 0.111463990590858
354.44 0.108117744770901
362.32 0.106362620393784
369.56 0.101880287571261
371.1 0.0843169445794885
380.18 0.0815138749464122
383.12 0.0887991530471418
386.72 0.0706579247757746
406.94 0.0824250631705898
412.86 0.107801143323242
416.88 0.0691768057851023
489.4 0.0544907379051131
499.46 0.0581614031310985
534.34 0.0654923370257837
569.52 0.048969602510271
816.36 0.0325436096179492
852.6 0.0361034678145522
1274.1 0.0276374747108567
1342.96 0.0261720428951532
1349.4 0.027021310614697
1370 0.0283038424214603
1386.12 0.0258130586231484
1410.64 0.0246443264963626
1415.08 0.0256579857400617
1419.32 0.0256490158956209
1420.66 0.0251260051819445
1422.82 0.0249751576228517
1425.14 0.0249351425676609
1429.98 0.0248439725357445
1437.36 0.0259449800967554
1439.04 0.0255217096438388
1439.14 0.0255112520015534
1440 0.0255075439960815
1443.8 0.02565586437886
1443.98 0.0256403901265642
1447.08 0.0237413127241956
1461.84 0.026124661371356
1469.12 0.0215189720621686
1503.92 0.0188899237325762
1566.5 0.0193167897287452
1577.76 0.0180663205912007
1620.2 0.0162374983902101
1779.1 0.015251538647712
1804.8 0.0149422217192281
2036.18 0.0150389543055448
2147.06 0.0130414981185798
2339.06 0.0154159553579408
2551.78 0.0106063853481468
3066.58 0.00945595827319231
3334.22 0.00833544532972316
3472.28 0.00830266739197611
3602.5 0.00881725788634855
3678.74 0.00832770650080229
3850.04 0.00798486179326709
4650.46 0.00815659240761659
5706.3 0.00653149911888382
5716.16 0.0066799770786643
5718.68 0.00651844146052833
5744.66 0.00649749396420267
5765.12 0.00649169936135551
5765.12 0.00649169936135551
5765.12 0.00649169936135551
5765.12 0.00649169936135551
5765.12 0.00649169936135551
5765.12 0.00649169936135551
5765.12 0.00649169936135551
5765.12 0.00649169936135551
5765.12 0.00649169936135551
5765.12 0.00649169936135551
5765.12 0.00649169936135551
5765.12 0.00649169936135551
5765.12 0.00649169936135551
5765.12 0.00649169936135551
5765.12 0.00649169936135551
5765.12 0.00649169936135551
5765.12 0.00649169936135551
};
\addplot [draw=black18, fill=black18, forget plot, mark=*, mark size=1, only marks, draw opacity=0,
 fill opacity=0.5]
table{%
x  y
21.98 0.999999999947385
83.6 0.216859574551975
83.82 0.220768214788371
87.04 0.214215829663614
88.88 0.210075035411911
91.06 0.207084984632005
93.62 0.201061597345765
96.78 0.197873074053071
100.7 0.191227967089493
102.46 0.186451272403011
104.82 0.17930705610045
107.12 0.176064465033177
109 0.172787411617989
114.52 0.162115359286375
117.18 0.154829535763223
119.36 0.150104432625156
121.74 0.145883118788123
124.56 0.140497249282753
128.86 0.139139185370573
137.16 0.129266666598339
138.62 0.125067404748617
138.92 0.125195090758912
141.96 0.124231648340818
145.12 0.122374364955692
147.8 0.119459427804562
156.86 0.115877781175623
166.12 0.111145603826631
167.52 0.109209373296553
168.76 0.107812085242885
175.3 0.103385911193226
184.72 0.101283682553239
189.7 0.0968201297174157
201.52 0.0933420379383003
209.5 0.0885477626788509
214.66 0.0858881274271091
219.1 0.085965672986357
230.78 0.0824925691029951
246.28 0.0757411504956655
248.04 0.0785500130926959
249.26 0.0735242268263356
262.62 0.0700545343893039
276.18 0.0681281506793115
295.06 0.0647789689009969
304.64 0.0624594644410947
320.28 0.0586215290956634
348.44 0.0547850066614873
351.9 0.0536470981355772
383.54 0.0494312583402877
389.74 0.047806412747984
417.82 0.044705909537518
434.08 0.0431620979732259
458.8 0.0428776847521109
487.8 0.0399062329511601
502.38 0.0376349239479182
534.02 0.0360550666802545
563.48 0.034257332544781
589.22 0.0340938987809781
617.92 0.0325158826401245
658.84 0.0309891996762087
703.16 0.0291722636197349
782.5 0.026748871187484
802.04 0.0254817658214125
861.4 0.0241051290961275
906.18 0.0233269769633477
1001.12 0.0214539840724776
1066.84 0.0202030934592432
1103.22 0.0194492948883254
1206.54 0.0178205430328861
1366.18 0.0160885786927875
1468.58 0.0148306420215289
1533.28 0.0140967651573949
1702.38 0.0129599420558137
1835.82 0.0120194532021755
2029.18 0.0109133709703438
2203.16 0.0102021832576779
2415.3 0.00950739488370429
2666.86 0.00856015868443402
2924.44 0.0077075181879002
3125.82 0.00717521635432423
3402.44 0.00652249414926455
4035.94 0.00581538821469147
4343.92 0.00532903629345964
4935.7 0.0046575667115001
5366.02 0.00423202835218428
6188.42 0.00365222546753481
7006.22 0.00317739406023101
7954.68 0.00272294164993118
};
\addplot [draw=darkgray153, fill=darkgray153, forget plot, mark=*, mark size=1, only marks, draw opacity=0,
 fill opacity=0.5]
table{%
x  y
21.98 0.999999999947385
113.72 0.167828351208239
119.72 0.1626531271485
123.54 0.15856109603795
127.16 0.153318916428482
137.02 0.148418294191455
145.64 0.14295743271828
151.5 0.142674417185087
156.26 0.139439759005705
161.06 0.136413779307276
167.08 0.133114357649189
173.14 0.128894777034428
189.78 0.127675815358615
195.04 0.123555188221683
208.76 0.121550598466561
214.52 0.118266017296527
215.84 0.118313234142643
224.9 0.117362180139956
232.5 0.114557952197078
242.5 0.11315233084572
266.14 0.109903824857124
280.76 0.108907391216131
299.3 0.107483825770378
315.1 0.103986478396502
341.18 0.102057115973005
346.6 0.0997649125035175
373.22 0.0996182674286178
398.1 0.0975129603570072
420.74 0.0924029777164064
425.06 0.0947812265353881
445.56 0.0882452793601257
476.08 0.086415975221954
486.2 0.0851261133548827
527.24 0.083069421092638
543.72 0.0824170762549643
603.82 0.0782145896197071
620.82 0.0790767924484242
623.38 0.0760115295906866
723.6 0.0746662359690757
804.04 0.0708056875961543
818.4 0.0723982174244424
839.08 0.0665095570759907
888.56 0.0681803256982436
903.82 0.0641989085106146
1015.22 0.0626576888556664
1063.68 0.0592203491889917
1137.64 0.0570750307710089
1164.92 0.055782991077672
1220.38 0.0544706674798049
1262.98 0.0517344531052983
1402.24 0.0500194509579525
1426.1 0.0486985691513412
1514.66 0.0463331881175779
1615.22 0.0426923004548512
1619.84 0.0435128832353502
1818.94 0.0413481817076679
1901.54 0.0397749779858676
2071.48 0.0371046343404933
2217.96 0.0362200947440547
2455.82 0.0327207133023817
2643.18 0.0303240892813645
2685.96 0.031321407653412
2867.72 0.0289850284093498
3060.68 0.0274122430864282
3126.12 0.0255560190533195
3213.62 0.0239485895148934
3532.36 0.0219099266717966
3673.58 0.0205574879578213
3880.3 0.0197295142262163
4124.7 0.0186908631272774
4349.1 0.0177047810116271
4738.9 0.0159813218833528
4835.54 0.0151958073756304
5322.76 0.0141008463637272
5526.3 0.0128171106852104
6003.8 0.0115574120106834
6287.8 0.0107548543024724
6877.04 0.0099677896936706
7154.58 0.00924271909328716
7496.94 0.00860573826762663
7944.1 0.00792512047935174
8325 0.00749925407619285
};
\addplot [
  draw=saddlebrown1356716,
  fill=saddlebrown1356716,
  forget plot,
  mark=*, mark size=1,
  only marks,
  draw opacity=0,
 fill opacity=0.5
]
table{%
x  y
352.64 0.115810698329374
420.3 0.072943573236752
423.92 0.0708526757280854
429.3 0.0659374930887923
434.5 0.0640368931543155
448.26 0.0631939845696464
460.02 0.0600265365317044
471.88 0.0594895758336944
492.54 0.0576357384008479
499.96 0.0564735997769635
520.64 0.0552989362665888
532.5 0.0533504446082853
557.42 0.0520929127654776
594.42 0.0490890970999152
615.56 0.0470342341076481
642.18 0.0456608931103481
661.12 0.0437185787610735
706.48 0.0422591062998619
742.04 0.041187021003962
782.36 0.0409409454097096
842.88 0.0392306688378648
867.38 0.0367507782552912
935.76 0.0352945126416183
968.48 0.034828382604473
999.86 0.0331147438443775
1060.74 0.0320171349754345
1150.38 0.0303739643460791
1206.26 0.0293160532741253
1258.96 0.0281869218201989
1316.1 0.0280278679408542
1352.1 0.0274289742498982
1371.24 0.0267979375507611
1414.32 0.026558370294256
1499.12 0.0252948845807659
1513.7 0.0241201970010159
1539.96 0.0247626406658842
1574.36 0.0237138415346201
1627.12 0.0233482289924972
1642.76 0.0230384364960747
1684.06 0.0225788353226009
1728.04 0.0222380469420213
1841.84 0.0218581818944938
1881.2 0.0216426373505097
1992.1 0.021198513342141
2017.18 0.0207344651447166
2063.52 0.0200429807594121
2082.88 0.0202556998605457
2210.98 0.0196759202519187
2320.92 0.0192662110846896
2369.56 0.018836322185549
2399.66 0.0185911697351927
2510.78 0.0181920461122671
2606.4 0.0178891611536655
2704.08 0.0176314507229758
2833.72 0.0172671164339665
2910.86 0.0169626180667063
3026.3 0.0166702284464808
3142.96 0.0163376649957944
3244.78 0.015958969591004
3331.44 0.0156544651076758
3467.94 0.0153433308914886
3555.34 0.0149413841054458
3686.8 0.0145385449232997
3814.68 0.0143239196880474
4045.88 0.0139867903952909
4120.52 0.0135880901972672
4338.6 0.0132278754817566
4492.16 0.0129225602040127
4611.86 0.0126647319017288
4787.3 0.0123721401970069
4910.24 0.0120236709519004
5106.56 0.0117318174471506
5271.2 0.0114278427416402
5495.14 0.011182327298018
5708.76 0.0108473357811736
5892.22 0.0105797329347381
6105.14 0.0102888174868082
6361.26 0.0100036293272793
6656.64 0.00975261202697022
6846.94 0.00947626480181539
7004.84 0.00922599340943092
7199.22 0.00898220184266001
7437.2 0.00879632796796801
7680.98 0.00856613886991631
7951.38 0.00826962326397874
8093.9 0.00805509646824421
8253.78 0.00783651175388411
8529.36 0.00759099431180159
8917.28 0.00735248917594816
};
\addplot [very thick, royalblue28108204]
table {%
219.18 0.0891362063366321
294.082828282828 0.0713277049141561
368.985656565657 0.0594496080672549
443.888484848485 0.0509189799177026
518.791313131313 0.0444782225875309
593.694141414141 0.0394357691427466
668.59696969697 0.0353776338679245
743.499797979798 0.0320399083836679
818.402626262626 0.0292459706391705
893.305454545454 0.0268729368249329
968.208282828283 0.0248325537929066
1043.11111111111 0.0230597395056256
1118.01393939394 0.021505410878471
1192.91676767677 0.0201318310689755
1267.8195959596 0.0189094973770176
1342.72242424242 0.0178150038477281
1417.62525252525 0.0168295390129009
1492.52808080808 0.0159378083347961
1567.43090909091 0.0151272471924143
1642.33373737374 0.0143874367072462
1717.23656565657 0.0137096637791332
1792.13939393939 0.0130865853442263
1867.04222222222 0.0125119690827872
1941.94505050505 0.0119804909689263
2016.84787878788 0.0114875756095612
2091.75070707071 0.0110292691620476
2166.65353535354 0.0106021373174332
2241.55636363636 0.0102031827564383
2316.45919191919 0.00982977786959832
2391.36202020202 0.00947960954287399
2466.26484848485 0.00915063355486207
2541.16767676768 0.00884103668670827
2616.0705050505 0.00854920506330454
2690.97333333333 0.0082736975612113
2765.87616161616 0.00801322336126169
2840.77898989899 0.00776662291088554
2915.68181818182 0.00753285170658213
2990.58464646465 0.00731096642075596
3065.48747474747 0.00710011298676944
3140.3903030303 0.00689951632712883
3215.29313131313 0.0067084714663884
3290.19595959596 0.00652633581580555
3365.09878787879 0.00635252245342153
3440.00161616162 0.00618649425293811
3514.90444444444 0.00602775873894191
3589.80727272727 0.00587586356581207
3664.7101010101 0.00573039253390426
3739.61292929293 0.00559096207001993
3814.51575757576 0.00545721811028662
3889.41858585859 0.00532883333282173
3964.32141414141 0.00520550469527263
4039.22424242424 0.00508695123879463
4114.12707070707 0.00497291212546786
4189.0298989899 0.0048631448807415
4263.93272727273 0.00475742381637701
4338.83555555556 0.0046555386126576
4413.73838383838 0.0045572930414369
4488.64121212121 0.0044625038139955
4563.54404040404 0.00437099953972457
4638.44686868687 0.00428261978341652
4713.3496969697 0.00419721421045702
4788.25252525253 0.00411464181052022
4863.15535353535 0.00403477019149876
4938.05818181818 0.00395747493637981
5012.96101010101 0.0038826390166297
5087.86383838384 0.00381015225638996
5162.76666666667 0.00373991084243455
5237.66949494949 0.00367181687540274
5312.57232323232 0.00360577795831706
5387.47515151515 0.00354170681883029
5462.37797979798 0.00347952096202728
5537.28080808081 0.00341914235094367
5612.18363636364 0.00336049711226076
5687.08646464647 0.00330351526489792
5761.98929292929 0.00324813046945627
5836.89212121212 0.00319427979667355
5911.79494949495 0.00314190351323306
5986.69777777778 0.00309094488343205
6061.60060606061 0.00304134998536056
6136.50343434343 0.00299306754037049
6211.40626262626 0.0029460487547308
6286.30909090909 0.00290024717246785
6361.21191919192 0.0028556185384828
6436.11474747475 0.00281212067112102
6511.01757575758 0.00276971334344319
6585.9204040404 0.00272835817251493
6660.82323232323 0.00268801851609234
6735.72606060606 0.00264865937613527
6810.62888888889 0.0026102473086296
6885.53171717172 0.00257275033924386
6960.43454545455 0.00253613788438631
7035.33737373737 0.00250038067726475
7110.2402020202 0.00246545069858418
7185.14303030303 0.00243132111154797
7260.04585858586 0.00239796620085495
7334.94868686869 0.00236536131540991
7409.85151515151 0.00233348281448737
7484.75434343434 0.00230230801710919
7559.65717171717 0.00227181515441523
7634.56 0.00224198332482353
};
\addplot [very thick, cadetblue80178158]
table {%
238.98 0.164422139930838
277.335151515151 0.152982404622388
315.690303030303 0.143190954360821
354.045454545455 0.134693222892593
392.400606060606 0.127232814680895
430.755757575758 0.120619179696807
469.110909090909 0.114707359003211
507.466060606061 0.109384846462464
545.821212121212 0.104562798793528
584.176363636364 0.100169992159968
622.531515151515 0.0961485659579892
660.886666666667 0.0924509608572821
699.241818181818 0.0890376739963059
737.59696969697 0.0858755852682325
775.952121212121 0.0829366903814056
814.307272727273 0.0801971286557388
852.662424242424 0.077636427707144
891.017575757576 0.0752369099945222
929.372727272727 0.0729832217238419
967.727878787879 0.0708619553387893
1006.08303030303 0.0688613443692667
1044.43818181818 0.0669710147839019
1082.79333333333 0.0651817808742511
1121.14848484848 0.0634854765359142
1159.50363636364 0.0618748149097634
1197.85878787879 0.0603432709141127
1236.21393939394 0.0588849823815478
1274.56909090909 0.0574946664149559
1312.92424242424 0.0561675482692265
1351.27939393939 0.0548993006008707
1389.63454545455 0.0536859913458423
1427.9896969697 0.0525240388143283
1466.34484848485 0.0514101728511624
1504.7 0.0503414011174175
1543.05515151515 0.0493149797144698
1581.4103030303 0.0483283875053313
1619.76545454545 0.0473793035961886
1658.12060606061 0.0464655875291191
1696.47575757576 0.0455852618089852
1734.83090909091 0.0447364964467098
1773.18606060606 0.043917595250018
1811.54121212121 0.0431269836332604
1849.89636363636 0.0423631977516758
1888.25151515151 0.041624874793654
1926.60666666667 0.0409107442882176
1964.96181818182 0.0402196203048617
2003.31696969697 0.0395503944397168
2041.67212121212 0.0389020294962642
2080.02727272727 0.0382735537809597
2118.38242424242 0.0376640559444657
2156.73757575758 0.0370726803080387
2195.09272727273 0.0364986226222083
2233.44787878788 0.0359411262114121
2271.80303030303 0.0353994784638803
2310.15818181818 0.0348730076309307
2348.51333333333 0.0343610799040539
2386.86848484848 0.033863096741833
2425.22363636364 0.0333784924219334
2463.57878787879 0.0329067317961817
2501.93393939394 0.0324473082291924
2540.28909090909 0.0319997417031289
2578.64424242424 0.0315635770730662
2616.99939393939 0.0311383824590668
2655.35454545455 0.0307237477625386
2693.7096969697 0.0303192832957233
2732.06484848485 0.0299246185143053
2770.42 0.0295394008441305
2808.77515151515 0.0291632945939249
2847.1303030303 0.0287959799466921
2885.48545454545 0.0284371520231796
2923.84060606061 0.0280865200114341
2962.19575757576 0.0277438063570283
3000.55090909091 0.0274087460090492
3038.90606060606 0.0270810857173863
3077.26121212121 0.026760583377267
3115.61636363636 0.0264470074173474
3153.97151515151 0.0261401362279976
3192.32666666667 0.0258397576267123
3230.68181818182 0.0255456683578476
3269.03696969697 0.0252576736241203
3307.39212121212 0.0249755866475294
3345.74727272727 0.0246992282575502
3384.10242424242 0.0244284265046326
3422.45757575758 0.0241630162971976
3460.81272727273 0.0239028390604714
3499.16787878788 0.0236477424156285
3537.52303030303 0.0233975798778408
3575.87818181818 0.023152210571936
3614.23333333333 0.0229114989644727
3652.58848484848 0.0226753146111295
3690.94363636364 0.0224435319183911
3729.29878787879 0.02221602991859
3767.65393939394 0.0219926920574344
3806.00909090909 0.0217734059932156
3844.36424242424 0.0215580634069494
3882.71939393939 0.0213465598227583
3921.07454545455 0.0211387944378526
3959.4296969697 0.0209346699615143
3997.78484848485 0.0207340924625281
4036.14 0.0205369712245462
};
\addplot [very thick, chocolate21910927]
table {%
21.62 1.0142748304497
96.7189898989899 0.39913797745739
171.81797979798 0.263224571959248
246.91696969697 0.199055408524069
322.01595959596 0.160894817252106
397.114949494949 0.135346818402912
472.213939393939 0.116945500727082
547.312929292929 0.103013478427026
622.411919191919 0.0920747601818243
697.510909090909 0.0832448792390614
772.609898989899 0.0759597663186075
847.708888888889 0.0698418399044139
922.807878787879 0.0646283579914607
997.906868686869 0.0601305846845453
1073.00585858586 0.0562092963994689
1148.10484848485 0.0527594528658055
1223.20383838384 0.0497002546382574
1298.30282828283 0.0469684942023332
1373.40181818182 0.0445139904666502
1448.50080808081 0.0422963805048886
1523.5997979798 0.0402828186177283
1598.69878787879 0.038446295938455
1673.79777777778 0.0367643931624341
1748.89676767677 0.0352183411463191
1823.99575757576 0.0337923039715859
1899.09474747475 0.0324728251725852
1974.19373737374 0.0312483952718113
2049.29272727273 0.0301091106299468
2124.39171717172 0.0290464018222012
2199.49070707071 0.0280528155108373
2274.5896969697 0.0271218378818335
2349.68868686869 0.0262477506675287
2424.78767676768 0.0254255129316168
2499.88666666667 0.0246506633816821
2574.98565656566 0.0239192391581863
2650.08464646465 0.0232277079391984
2725.18363636364 0.0225729108759144
2800.28262626263 0.0219520143912094
2875.38161616162 0.0213624692724398
2950.48060606061 0.0208019757997974
3025.5795959596 0.0202684538942002
3100.67858585859 0.0197600174599168
3175.77757575758 0.0192749522487157
3250.87656565657 0.0188116966932411
3325.97555555556 0.0183688252543
3401.07454545455 0.0179450339049517
3476.17353535354 0.0175391274376857
3551.27252525253 0.0171500083326064
3626.37151515152 0.0167766669668
3701.4705050505 0.0164181729797885
3776.5694949495 0.0160736676386452
3851.66848484848 0.0157423570701127
3926.76747474747 0.0154235062468311
4001.86646464646 0.0151164336313029
4076.96545454545 0.0148205063950612
4152.06444444444 0.014535136142147
4227.16343434343 0.0142597750758321
4302.26242424242 0.0139939125558353
4377.36141414141 0.0137370720003453
4452.4604040404 0.0134888080931797
4527.55939393939 0.0132487042615448
4602.65838383838 0.0130163703942631
4677.75737373737 0.0127914407741147
4752.85636363636 0.01257357220119
4827.95535353535 0.0123624422869617
4903.05434343434 0.0121577479012117
4978.15333333333 0.0119592037560569
5053.25232323232 0.0117665411131462
5128.35131313131 0.0115795066017001
5203.4503030303 0.0113978611364523
5278.54929292929 0.0112213789257722
5353.64828282828 0.0110498465613155
5428.74727272727 0.0108830621814839
5503.84626262626 0.0107208347018029
5578.94525252525 0.0105629831060501
5654.04424242424 0.0104093357926097
5729.14323232323 0.0102597299710957
5804.24222222222 0.0101140111047875
5879.34121212121 0.00997203239487104
5954.4402020202 0.00983365430286952
6029.53919191919 0.00969874410800587
6104.63818181818 0.00956717549655
6179.73717171717 0.0094388281804856
6254.83616161616 0.00931358754308315
6329.93515151515 0.00919134430918844
6405.03414141414 0.00907199423823951
6480.13313131313 0.00895543783820399
6555.23212121212 0.00884158009879199
6630.33111111111 0.00873033024244632
6705.4301010101 0.00862160149174246
6780.52909090909 0.00851531085195091
6855.62808080808 0.00841137890762056
6930.72707070707 0.00830972963214
7005.82606060606 0.00821029020932065
7080.92505050505 0.0081129908661257
7156.02404040404 0.00801776471574097
7231.12303030303 0.00792454761024934
7306.22202020202 0.00783327800223016
7381.32101010101 0.00774389681465916
7456.42 0.00765634731853418
};
\addplot [very thick, purple11522131]
table {%
78.62 0.531161263146081
136.059393939394 0.284326992808518
193.498787878788 0.192025406662749
250.938181818182 0.144364818034008
308.377575757576 0.115444095682803
365.81696969697 0.0960924443935335
423.256363636364 0.0822636394490443
480.695757575758 0.0719027553966569
538.135151515152 0.0638581258703471
595.574545454546 0.0574353479070452
653.013939393939 0.0521913732325861
710.453333333333 0.0478304897683476
767.892727272727 0.0441479232779518
825.332121212121 0.0409974591514945
882.771515151515 0.0382719549704355
940.210909090909 0.0358911363520282
997.650303030303 0.0337936905377313
1055.0896969697 0.0319319921182494
1112.52909090909 0.0302684936001255
1169.96848484848 0.0287731991182353
1227.40787878788 0.0274218606104815
1284.84727272727 0.0261946666701043
1342.28666666667 0.0250752741064759
1399.72606060606 0.024050082193157
1457.16545454545 0.0231076815773769
1514.60484848485 0.0222384307576825
1572.04424242424 0.0214341269965051
1629.48363636364 0.0206877480087291
1686.92303030303 0.019993247301314
1744.36242424242 0.0193453906121403
1801.80181818182 0.0187396241408606
1859.24121212121 0.0181719675957986
1916.68060606061 0.0176389267756749
1974.12 0.0171374216504712
2031.55939393939 0.0166647268304972
2088.99878787879 0.0162184220058859
2146.43818181818 0.0157963504629789
2203.87757575758 0.0153965841838796
2261.31696969697 0.0150173943427992
2318.75636363636 0.0146572262508519
2376.19575757576 0.0143146779866094
2433.63515151515 0.0139884820954896
2491.07454545455 0.0136774898562315
2548.51393939394 0.0133806577042572
2605.95333333333 0.0130970354749144
2663.39272727273 0.0128257561884138
2720.83212121212 0.0125660271458084
2778.27151515151 0.0123171221439481
2835.71090909091 0.0120783746488216
2893.1503030303 0.011849171792492
2950.5896969697 0.0116289490800602
3008.02909090909 0.0114171857106302
3065.46848484848 0.0112134004308042
3122.90787878788 0.0110171478513522
3180.34727272727 0.0108280151678319
3237.78666666667 0.0106456192344277
3295.22606060606 0.0104696039474282
3352.66545454545 0.0102996379007972
3410.10484848485 0.0101354122814037
3467.54424242424 0.00997663897582236
3524.98363636364 0.00982304886430923
3582.42303030303 0.00967439028072501
3639.86242424242 0.00953042761987891
3697.30181818182 0.00939094007609583
3754.74121212121 0.00925572049880917
3812.18060606061 0.00912457435271035
3869.62 0.00899731877148136
3927.05939393939 0.0088737816954325
3984.49878787879 0.00875380108449443
4041.93818181818 0.00863722419899529
4099.37757575758 0.0085239069415093
4156.81696969697 0.0084137132538129
4214.25636363636 0.00830651456364063
4271.69575757576 0.00820218927650871
4329.13515151515 0.00810062230838187
4386.57454545454 0.00800170465540459
4444.01393939394 0.00790533299731293
4501.45333333333 0.00781140933149087
4558.89272727273 0.00771984063494434
4616.33212121212 0.00763053855173958
4673.77151515151 0.00754341910369584
4731.21090909091 0.00745840242233901
4788.6503030303 0.00737541250031531
4846.0896969697 0.00729437696063681
4903.52909090909 0.00721522684228416
4960.96848484848 0.00713789640082963
5018.40787878788 0.00706232292286692
5075.84727272727 0.00698844655314512
5133.28666666667 0.0069162101334036
5190.72606060606 0.0068455590519941
5248.16545454545 0.00677644110345691
5305.60484848485 0.00670880635729086
5363.04424242424 0.00664260703522236
5420.48363636364 0.00657779739633817
5477.92303030303 0.00651433362950025
5535.36242424242 0.00645217375250962
5592.80181818182 0.00639127751753053
5650.24121212121 0.00633160632232583
5707.68060606061 0.00627312312689141
5765.12 0.00621579237511013
};
\addplot [very thick, black18]
table {%
21.98 0.840835995878117
102.108282828283 0.180861365418746
182.236565656566 0.102708368590372
262.364848484848 0.0722236107593054
342.493131313131 0.0559317912054236
422.621414141414 0.0457692953833874
502.749696969697 0.0388131731729659
582.87797979798 0.0337462783407002
663.006262626263 0.0298871033729669
743.134545454546 0.0268473499305143
823.262828282828 0.0243894193210697
903.391111111111 0.0223596956459916
983.519393939394 0.020654409478153
1063.64767676768 0.0192009107739129
1143.77595959596 0.0179468006048554
1223.90424242424 0.0168533239266552
1304.03252525253 0.0158911929589899
1384.16080808081 0.015037857709158
1464.28909090909 0.014275670255435
1544.41737373737 0.0135906188139436
1624.54565656566 0.0129714352735959
1704.67393939394 0.0124089535930399
1784.80222222222 0.0118956404145529
1864.93050505051 0.0114252462330339
1945.05878787879 0.0109925424509922
2025.18707070707 0.0105931206012741
2105.31535353535 0.0102232372250658
2185.44363636364 0.00987969272481553
2265.57191919192 0.00955973580852305
2345.7002020202 0.00926098742702536
2425.82848484849 0.00898137971312525
2505.95676767677 0.00871910657707481
2586.08505050505 0.00847258343981718
2666.21333333333 0.0082404141891331
2746.34161616162 0.00802136388942246
2826.4698989899 0.00781433610802504
2906.59818181818 0.00761835397095108
2986.72646464647 0.00743254425066109
3066.85474747475 0.00725612393379868
3146.98303030303 0.00708838882884871
3227.11131313131 0.0069287038607872
3307.2395959596 0.00677649476794865
3387.36787878788 0.00663124097002644
3467.49616161616 0.00649246941868085
3547.62444444444 0.00635974927616197
3627.75272727273 0.00623268729456499
3707.88101010101 0.00611092379026876
3788.00929292929 0.00599412912588133
3868.13757575758 0.00588200062648525
3948.26585858586 0.00577425986881187
4028.39414141414 0.00567065029169763
4108.52242424242 0.00557093508419901
4188.65070707071 0.00547489531438942
4268.77898989899 0.00538232826738961
4348.90727272727 0.00529304596579777
4429.03555555556 0.00520687384955131
4509.16383838384 0.0051236495955029
4589.29212121212 0.00504322205973423
4669.4204040404 0.0049654503279507
4749.54868686869 0.00489020286126917
4829.67696969697 0.00481735672638639
4909.80525252525 0.00474679690054691
4989.93353535354 0.00467841564295399
5070.06181818182 0.00461211192531802
5150.1901010101 0.00454779091514233
5230.31838383838 0.0044853635061258
5310.44666666667 0.0044247458907377
5390.57494949495 0.00436585917060424
5470.70323232323 0.00430862900085526
5550.83151515152 0.00425298526502162
5630.9597979798 0.00419886177745988
5711.08808080808 0.00414619601061874
5791.21636363636 0.00409492884475702
5871.34464646465 0.00404500433798275
5951.47292929293 0.00399636951471092
6031.60121212121 0.00394897417083882
6111.7294949495 0.00390277069411519
6191.85777777778 0.00385771389833597
6271.98606060606 0.00381376087013907
6352.11434343434 0.00377087082729314
6432.24262626263 0.00372900498748503
6512.37090909091 0.00368812644670823
6592.49919191919 0.00364820006644098
6672.62747474747 0.00360919236888064
6752.75575757576 0.00357107143956988
6832.88404040404 0.0035338068368121
6913.01232323232 0.0034973695073295
6993.14060606061 0.00346173170766653
7073.26888888889 0.00342686693088647
7153.39717171717 0.00339274983814921
7233.52545454545 0.00335935619479457
7313.65373737374 0.00332666281058799
7393.78202020202 0.00329464748381545
7473.9103030303 0.00326328894894066
7554.03858585859 0.00323256682756216
7634.16686868687 0.00320246158242974
7714.29515151515 0.00317295447429927
7794.42343434343 0.00314402752142334
7874.55171717172 0.00311566346149148
7954.68 0.00308784571584842
};
\addplot [very thick, darkgray153]
table {%
21.98 0.358823339275112
105.848888888889 0.196285992717573
189.717777777778 0.147324383615972
273.586666666667 0.120930287729092
357.455555555556 0.103806615349578
441.324444444444 0.0915724444058115
525.193333333333 0.082291101897448
609.062222222222 0.0749538204532799
692.931111111111 0.0689759698748234
776.8 0.0639921138210037
860.668888888889 0.0597605217648995
944.537777777778 0.0561140844077467
1028.40666666667 0.0529331195202686
1112.27555555556 0.0501293868162951
1196.14444444444 0.0476362289888193
1280.01333333333 0.0454022438258805
1363.88222222222 0.0433870838093371
1447.75111111111 0.0415585865268138
1531.62 0.0398907647991966
1615.48888888889 0.0383623679427853
1699.35777777778 0.0369558318742093
1783.22666666667 0.0356564997547714
1867.09555555556 0.0344520345378124
1950.96444444444 0.0333319700201057
2034.83333333333 0.0322873634329249
2118.70222222222 0.0313105235370177
2202.57111111111 0.0303947955918997
2286.44 0.029534389676177
2370.30888888889 0.0287242424120714
2454.17777777778 0.0279599046887185
2538.04666666667 0.0272374498088595
2621.91555555556 0.0265533978176615
2705.78444444444 0.0259046527560926
2789.65333333333 0.0252884503143199
2873.52222222222 0.0247023139122592
2957.39111111111 0.0241440176534137
3041.26 0.0236115549191479
3125.12888888889 0.0231031116184683
3208.99777777778 0.0226170433013328
3292.86666666667 0.0221518554947479
3376.73555555556 0.0217061867402691
3460.60444444444 0.0212787939063109
3544.47333333333 0.0208685394244187
3628.34222222222 0.0204743801595276
3712.21111111111 0.0200953576734197
3796.08 0.0197305896805455
3879.94888888889 0.0193792625279846
3963.81777777778 0.01904062455807
4047.68666666667 0.0187139802342273
4131.55555555555 0.018398684928816
4215.42444444444 0.0180941402868961
4299.29333333333 0.0177997900924786
4383.16222222222 0.0175151165743886
4467.03111111111 0.0172396370977528
4550.9 0.0169729011946141
4634.76888888889 0.016714487893508
4718.63777777778 0.0164640033132169
4802.50666666667 0.0162210784904866
4886.37555555556 0.015985367415406
4970.24444444444 0.0157565452514855
5054.11333333333 0.0155343067203515
5137.98222222222 0.0153183646334382
5221.85111111111 0.0151084485551967
5305.72 0.0149043035841861
5389.58888888889 0.0147056892400104
5473.45777777778 0.0145123784454581
5557.32666666667 0.0143241565944151
5641.19555555556 0.0141408206971762
5725.06444444444 0.0139621785957101
5808.93333333333 0.013788048242244
5892.80222222222 0.0136182570352449
5976.67111111111 0.013452641207506
6060.54 0.0132910452615977
6144.40888888889 0.0131333214484322
6228.27777777778 0.0129793292851236
6312.14666666667 0.0128289351087102
6396.01555555555 0.0126820116626431
6479.88444444444 0.0125384377132517
6563.75333333333 0.0123980976936645
6647.62222222222 0.0122608813729045
6731.49111111111 0.0121266835480932
6815.36 0.0119954037578921
6899.22888888889 0.0118669460154783
6983.09777777778 0.0117412185595105
7066.96666666667 0.0116181336216768
7150.83555555556 0.0114976072095435
7234.70444444444 0.0113795589035346
7318.57333333333 0.0112639116669737
7402.44222222222 0.0111505916682142
7486.31111111111 0.0110395281139615
7570.18 0.0109306530929715
7654.04888888889 0.0108239014293736
7737.91777777778 0.0107192105449305
7821.78666666667 0.0106165203296014
7905.65555555556 0.0105157730198274
7989.52444444444 0.0104169130840038
8073.39333333333 0.0103198871146454
8157.26222222222 0.0102246437267915
8241.13111111111 0.0101311334622297
8325 0.0100393086991512
};
\addplot [very thick, saddlebrown1356716]
table {%
352.64 0.077656518150213
439.151515151515 0.0649434267312972
525.66303030303 0.0562486002525156
612.174545454546 0.049897066778262
698.686060606061 0.0450363572298221
785.197575757576 0.0411855391738634
871.709090909091 0.0380520551097275
958.220606060606 0.0354473786492688
1044.73212121212 0.0332443558870569
1131.24363636364 0.0313539955515496
1217.75515151515 0.0297120788606005
1304.26666666667 0.0282710536029507
1390.77818181818 0.0269949253912801
1477.2896969697 0.0258559257448828
1563.80121212121 0.0248322740328248
1650.31272727273 0.0239066351240721
1736.82424242424 0.0230650322758878
1823.33575757576 0.0222960654621016
1909.84727272727 0.0215903392405808
1996.35878787879 0.0209400372538853
2082.8703030303 0.0203386011918089
2169.38181818182 0.019780485384798
2255.89333333333 0.0192609669642037
2342.40484848485 0.0187759973988016
2428.91636363636 0.0183220852216557
2515.42787878788 0.0178962025360532
2601.93939393939 0.0174957098402749
2688.45090909091 0.0171182951016644
2774.96242424242 0.0167619240143168
2861.47393939394 0.0164247991078456
2947.98545454546 0.0161053259159658
3034.49696969697 0.0158020848173352
3121.00848484849 0.0155138074650591
3207.52 0.0152393569521798
3294.03151515152 0.0149777110373502
3380.54303030303 0.0147279478914668
3467.05454545455 0.0144892339322539
3553.56606060606 0.0142608133970002
3640.07757575758 0.0140419993692412
3726.58909090909 0.0138321660272407
3813.10060606061 0.0136307419236562
3899.61212121212 0.0134372041391286
3986.12363636364 0.0132510731794365
4072.63515151515 0.013071908507686
4159.14666666667 0.0128993046207978
4245.65818181818 0.0127328875941161
4332.1696969697 0.0125723120299532
4418.68121212121 0.0124172583557753
4505.19272727273 0.0122674304259498
4591.70424242424 0.0121225533878049
4678.21575757576 0.0119823717784698
4764.72727272727 0.0118466478237529
4851.23878787879 0.0117151599143481
4937.7503030303 0.0115877012380685
5024.26181818182 0.011464078549688
5110.77333333333 0.011344111062426
5197.28484848485 0.0112276294472002
5283.79636363636 0.0111144749275558
5370.30787878788 0.0110044984597153
5456.8193939394 0.0108975599885039
5543.33090909091 0.010793527771042
5629.84242424243 0.0106922777610752
5716.35393939394 0.0105936930476581
5802.86545454546 0.0104976633426474
5889.37696969697 0.0104040845120954
5975.88848484849 0.0103128581471965
6062.4 0.0102238911709249
6148.91151515152 0.0101370954769284
6235.42303030303 0.0100523875976168
6321.93454545455 0.00996968839871465
6408.44606060606 0.00988892279783311
6494.95757575758 0.00981001950487589
6581.46909090909 0.00973291078231619
6667.98060606061 0.00965753222358292
6754.49212121212 0.00958382254797135
6841.00363636364 0.00951172341065002
6927.51515151515 0.00944117922647614
7014.02666666667 0.00937213700645611
7100.53818181818 0.00930454620579864
7187.0496969697 0.00923835858260767
7273.56121212121 0.00917352806635091
7360.07272727273 0.00911001063531957
7446.58424242424 0.00904776420236595
7533.09575757576 0.00898674850827024
7619.60727272727 0.00892692502214529
7706.11878787879 0.00886825684833991
7792.63030303031 0.0088107086393488
7879.14181818182 0.00875424651427885
7965.65333333334 0.00869883798246022
8052.16484848485 0.00864445187182532
8138.67636363637 0.00859105826170962
8225.18787878788 0.00853862841975763
8311.6993939394 0.00848713474264224
8398.21090909091 0.0084365507003299
8484.72242424243 0.00838685078364495
8571.23393939394 0.00833801045490626
8657.74545454546 0.00829000610142676
8744.25696969697 0.00824281499168309
8830.76848484849 0.00819641523397675
8917.28 0.00815078573742231
};
\addplot [draw=black, fill=black, mark=x, very thick, mark size=2.5pt, only marks]
table{%
x  y
87.12 0.462721827510279
352.64 0.115810698329374
1440 0.0255075439960804
5765.12 0.00649169936135397
};
