# Supplementary material for: Swarm Reinforcement Learning For Adaptive Mesh Refinement
Source: arXiv:2304.00818 source file (2023-10-09)
Supplement: Supplementary file 9 [file group_additional_metrics_l3.tex]

\nextgroupplot[
ylabel shift = -0.2cm,
title style={yshift=-0.2cm},
height=4.5cm,
width=0.50\textwidth,
ylabel={Mean Error},
xlabel={\empty},
title={Stokes Flow},
scaled x ticks=false,
clip marker paths=true,
legend cell align={left},
legend style={fill opacity=0.8, draw opacity=1, text opacity=1, draw=lightgray204},
log basis y={10},
tick align=outside,
tick pos=left,
x grid style={darkgray176},
xmajorgrids,
xmin=-460.664, xmax=10410.064,
xtick style={color=black},
xtick={-2000,0,2000,4000,6000,8000,10000,12000},
xticklabels={-2.0,0.0,2.0,4.0,6.0,8.0,10.0,12.0},
y grid style={darkgray176},
ymajorgrids,
ymin=0.000893892960125057, ymax=2.42343362744762,
ymode=log,
ytick style={color=black},
ytick={1e-05,0.0001,0.001,0.01,0.1,1,10,100},
yticklabels={
  \(\displaystyle {10^{-5}}\),
  \(\displaystyle {10^{-4}}\),
  \(\displaystyle {10^{-3}}\),
  \(\displaystyle {10^{-2}}\),
  \(\displaystyle {10^{-1}}\),
  \(\displaystyle {10^{0}}\),
  \(\displaystyle {10^{1}}\),
  \(\displaystyle {10^{2}}\)
}
]
\addplot [
  draw=royalblue28108204,
  fill=royalblue28108204,
  forget plot,
  mark=*, mark size=1,
  only marks,
  draw opacity=0,
 fill opacity=0.5
]
table{%
x  y
33.46 0.99999999998787
64.96 0.794966623258819
66.06 0.779610123685663
87.08 0.696507583089408
88.82 0.603860901553408
97.52 0.625250969139485
101.84 0.521094349017051
110.12 0.487564798136627
117.52 0.478381474500459
139.2 0.465914117352839
164.94 0.321141143596973
181.22 0.260738449510546
184.9 0.294164854721592
189.6 0.292021901824059
193.68 0.291948368528379
207.56 0.252190731294284
213.78 0.253107030618805
221.4 0.223376808240367
252.7 0.216814012341399
263 0.235415311751991
432.38 0.12787983984403
461.4 0.104277040715896
476.36 0.105474210968175
514.82 0.0963096979642699
522.78 0.0910064592652747
529.7 0.0905698911252434
546.54 0.0892185078858907
569.6 0.0843035184634867
576.48 0.0854228604199573
632.9 0.0724460931874423
715 0.0622165246384435
745.14 0.0639232232129843
767.72 0.0628812005750337
786.9 0.0641375160337999
817.82 0.0575673632549732
819.28 0.0508416143610307
842.64 0.0536311274484827
875.44 0.0500907577363107
893.08 0.0443053335366149
966.7 0.0548519369554346
1201.52 0.0363581171033462
1313.52 0.0327640120503603
1327.9 0.0344491247111212
1416.92 0.0334192179214046
1427.12 0.0342143386926798
1458.56 0.0341947257876818
1533.6 0.0312451780332479
1546.62 0.026632513281294
1579.18 0.0360530529292164
1676.48 0.0270226811924884
1689.34 0.0314212974090584
1748.78 0.02749757630383
1759.58 0.0257647137085898
1844.68 0.0267319212365777
2004.78 0.0215700826346497
2031.62 0.0227163084226214
2040.38 0.0214897245695974
2046.84 0.0237265330499898
2116.72 0.0208268988744373
2434.96 0.0189333188733516
2613.36 0.0176770291583836
2657.36 0.0167128227544137
2746.04 0.0134103490901508
2850.86 0.0162158236285356
2899.18 0.019232119773775
2990.4 0.0168009763745404
3031.56 0.0167387815484369
3169.78 0.0157291644051932
3196.82 0.0165667564106939
3227.86 0.013814245342193
3232.2 0.015046737444604
3263.36 0.0153557240687915
3543.22 0.0110324949741737
3715.14 0.0125362487548231
3869.32 0.0133996781058468
4032.2 0.0117590363583319
4047.56 0.0121428766602056
4090.68 0.0112624510767545
4158.36 0.012719939295131
4312.04 0.0106237254473418
4330.38 0.00820245881791757
4504.38 0.00933740798203205
4589.06 0.0101304689412865
4621.66 0.00979395541449275
4654.88 0.00923231341798101
4710.04 0.0101856925141477
4784.28 0.0103119884669118
5357.04 0.0091857805726361
5413.04 0.00903472669388869
5561.3 0.0103184574829582
5665.18 0.00853597047231892
5897.1 0.00799342938468795
5947.52 0.00789817451371855
6078.84 0.00904829432874153
6525.5 0.00729075453070402
6599.42 0.00855483515985166
6769.2 0.00740163554191098
6857.84 0.00783291771190483
7766.54 0.00746018359150048
8444.02 0.00653616707656115
};
\addplot [
  draw=cadetblue80178158,
  fill=cadetblue80178158,
  forget plot,
  mark=*, mark size=1,
  only marks,
  draw opacity=0,
 fill opacity=0.5
]
table{%
x  y
212.84 0.32135280628743
218.08 0.331492761153022
220.48 0.333966373415005
220.82 0.339149566877058
222.46 0.300369938141208
222.8 0.315149380476518
224.06 0.29992964338902
224.78 0.300865232312947
232.06 0.273755713240701
262.36 0.264172936767318
419.76 0.170983677153241
425.48 0.186946414139752
425.98 0.352412005287442
438.66 0.323754375826051
454.6 0.195704728117426
456.02 0.535248007936563
481.62 0.493209199554734
503.02 0.452869285594235
513.9 0.330555964300931
519.74 0.433914670087535
582.62 0.117825650056223
620.72 0.118521517482823
629.74 0.147567610250449
646.86 0.21867941411934
658.96 0.413754249573662
681 0.191343166236768
707.16 0.442791640753597
718.16 0.379739271457233
786.92 0.413815893554966
795.82 0.635850750548476
819.46 0.115981762196409
840.86 0.137539153135833
845.26 0.192838183104568
847.38 0.0877491929510416
916.56 0.083057572633441
946.82 0.192892706664612
957.68 0.340969967298046
1062.12 0.779644510375836
1070.16 0.193877101054835
1093.24 0.164595401975386
1093.82 0.143016174089176
1106.34 0.0964142711855821
1240.7 0.328966241585423
1254.04 0.0581776471375769
1266.58 0.0417593924744535
1375.3 0.0923498452509526
1427.56 0.129880529985074
1429.36 0.593420596707602
1434.42 0.0591438693814449
1440.34 0.579204134105714
1451.1 0.28638825477038
1489 0.266092212590387
1611.12 0.654552312656735
1615.8 0.0538006154094027
1623.14 0.22403180143834
1636.1 0.0907238504128445
1743.4 0.452281129819539
1758.36 0.199619785933458
1776.42 0.0230118895161876
1804.72 0.214931058650941
1811.7 0.50514449597778
1823.46 0.132946698045248
1865.74 0.159128477369764
1911.54 0.0458382480186223
2047.38 0.106130602974818
2139.58 0.0234520882208825
2141.04 0.258135363612793
2328.24 0.534813813838854
2516.04 0.0476812055920278
2532.06 0.0400592231696807
2540.18 0.267311120994856
2625.56 0.268354311344489
2626.92 0.111895480236098
2687.78 0.0836991440090808
2702.28 0.0918478952156633
2730.38 0.098040257366595
2767.92 0.0443302341231039
2807.7 0.654876756784378
2855.7 0.0237823333396244
2972.86 0.0195124566248723
3013.02 0.0397913254851273
3040.72 0.0416743548827885
3085.04 0.145440109700175
3135.12 0.099077987976883
3152.28 0.259858012509516
3167.68 0.0137476796640643
3231.24 0.0335640321064188
3390.32 0.0129127173344693
3411.66 0.15527723638709
3455.38 0.0169942463034064
3493.72 0.627461045435626
3599.94 0.0118693663656783
3732.46 0.489794200202897
4033 0.184966143192559
};
\addplot [
  draw=chocolate21910927,
  fill=chocolate21910927,
  forget plot,
  mark=*, mark size=1,
  only marks,
  draw opacity=0,
 fill opacity=0.5
]
table{%
x  y
33.46 0.99999999998787
33.46 0.99999999998787
33.46 0.99999999998787
33.46 0.99999999998787
33.46 0.99999999998787
33.46 0.99999999998787
33.46 0.99999999998787
33.46 0.99999999998787
33.46 0.99999999998787
33.46 0.99999999998787
33.46 0.99999999998787
33.46 0.99999999998787
33.46 0.99999999998787
33.46 0.99999999998787
33.46 0.99999999998787
33.46 0.99999999998787
33.46 0.99999999998787
33.46 0.99999999998787
33.46 0.99999999998787
33.46 0.99999999998787
33.46 0.99999999998787
33.46 0.99999999998787
33.46 0.99999999998787
33.46 0.99999999998787
33.46 0.99999999998787
33.46 0.99999999998787
33.46 0.99999999998787
33.46 0.99999999998787
33.46 0.99999999998787
33.46 0.99999999998787
33.46 0.99999999998787
33.46 0.99999999998787
33.46 0.99999999998787
33.46 0.99999999998787
33.46 0.99999999998787
33.46 0.99999999998787
40.24 0.958412724079648
43.08 0.947555656678652
56.88 0.879805939787418
83.2 0.889942511154493
88.82 0.588417842115723
92.44 0.583417762212731
96.78 0.535591952249442
97.04 0.535532289875897
99.24 0.509653179794803
99.78 0.755273348173172
101.92 0.553166057937973
108.56 0.546864835167736
110.34 0.482562925387569
111.1 0.540978431910548
113.22 0.692985965206655
116.44 0.563302625603061
119.48 0.433871924745008
125.78 0.509083313672148
127.26 0.381091021333006
134.96 0.338118374648499
138.44 0.484775624688607
141.5 0.572619345471829
153.92 0.443401522854608
155.38 0.468709434270532
155.84 0.454617595227495
156.58 0.339590396120175
176.48 0.354087202372516
193.98 0.361297847993498
221.78 0.479008372812416
276.52 0.249177361478775
285.3 0.520083946631924
286.88 0.237348912276257
324.04 0.157681798902576
350.5 0.62388676902221
380.4 0.158227156875303
418.38 0.188411284319286
458.6 0.129843596328473
496.32 0.107246619013471
675.68 0.118524319708766
828.5 0.157902303786514
960.88 0.11064400576642
1061.96 0.0696554340722227
1188.68 0.227533598382464
1399.94 0.0784281935790929
1578.68 0.05980081252041
1586.74 0.0482902271483096
1712.24 0.0341234828618733
1866.56 0.0408291807605406
2152.14 0.381583642252499
2568.38 0.0362754386511536
2764.74 0.0273067919063109
3140.76 0.309069663738016
3557.84 0.0247893958598572
3730.42 0.0275462533068987
4186.8 0.0135592944018877
4660.9 0.00495863310811784
6262.92 0.19789130899893
7068.34 0.0081849990439818
};
\addplot [draw=purple11522131, fill=purple11522131, forget plot, mark=*, mark size=1, only marks, draw opacity=0,
 fill opacity=0.5]
table{%
x  y
106.9 0.536466316270368
110.94 0.489696331231732
118.46 0.430208883080805
123.78 0.418044589775813
141.56 0.424218497980878
149.76 0.333251781352849
151.84 0.325739376840925
155.2 0.337157722753667
162.74 0.282614784514403
164.18 0.306680037508889
170.94 0.298020481321071
171.8 0.321915216032249
176.82 0.283415694163216
178.72 0.280117098884751
202.08 0.248006056173387
262.34 0.209658131015819
295.8 0.218831186204381
314.06 0.209262892193574
374.26 0.191917450402168
379.94 0.169978694875892
393.48 0.155304797194771
431.14 0.174983633286302
449.78 0.116974624301776
460.36 0.11249426938283
498.9 0.100879591501201
529.1 0.0986025691189157
535.98 0.0983885372250098
536 0.0983585902434125
536.08 0.0983862711646816
536.2 0.0983842333823283
536.2 0.0983835174897156
536.24 0.098386637393778
536.5 0.0983774705092026
536.56 0.0983729453909929
536.64 0.0983741953483196
536.64 0.0983741953483196
536.64 0.0983741953483196
536.64 0.0983741953483196
537.76 0.0982894950629496
537.92 0.0982871868955507
2036.44 0.0340125979485236
2084.2 0.0340740982826956
2135.64 0.0329828820353378
2142.12 0.0329836412873371
2144.2 0.0329850830266632
2145.04 0.0329826521811118
2145.28 0.032982511865441
2145.28 0.032982511865441
2145.28 0.032982511865441
2145.28 0.032982511865441
2145.28 0.032982511865441
2145.28 0.032982511865441
2145.28 0.032982511865441
2145.28 0.032982511865441
2145.28 0.032982511865441
2145.28 0.032982511865441
2145.28 0.032982511865441
2145.28 0.032982511865441
2145.28 0.032982511865441
2145.28 0.032982511865441
2168.76 0.0324587533692423
2178.56 0.0315217625878164
2178.56 0.0315217625878164
2178.56 0.0315217625878164
2178.56 0.0315217625878164
2178.56 0.0315217625878164
2178.56 0.0315217625878164
2178.56 0.0315217625878164
2178.56 0.0315217625878164
2252.44 0.031736409913519
8327.18 0.012044258334631
8375.32 0.0120465719688273
8490.84 0.0120732248516254
8551.3 0.011939098564105
8555.72 0.01193190475931
8558.24 0.0119319370922575
8559.24 0.0119319406640461
8560.48 0.0120425691830139
8560.64 0.0119319398987969
8560.64 0.0119319398987969
8560.64 0.0119319398987969
8560.64 0.0119319398987969
8560.64 0.0119319398987969
8560.64 0.0119319398987969
8560.64 0.0119319398987969
8560.64 0.0119319398987969
8560.64 0.0119319398987969
8560.64 0.0119319398987969
8560.64 0.0119319398987969
8560.64 0.0119319398987969
8560.64 0.0119319398987969
8560.64 0.0119319398987969
8560.64 0.0119319398987969
8570.88 0.0120424813908945
8570.88 0.0120424813908945
8570.88 0.0120424813908945
8570.88 0.0120424813908945
8570.88 0.0120424813908945
8570.88 0.0120424813908945
8585.52 0.0119501484232162
};
\addplot [draw=black18, fill=black18, forget plot, mark=*, mark size=1, only marks, draw opacity=0,
 fill opacity=0.5]
table{%
x  y
33.46 0.99999999998787
79.26 0.557977594934325
81.96 0.543303124806472
85.02 0.529115955156297
89.9 0.510628617570606
92.78 0.49336671894209
96.04 0.475296869653251
98.06 0.462915160491743
99.82 0.45117525110646
102.3 0.438266312186609
106.92 0.420425619893037
111.44 0.409245356508811
116.48 0.392847235488561
121.02 0.38112860182761
124.18 0.367653768289701
129.82 0.355468494732492
134.72 0.341336420934796
141.66 0.323440760018857
146.68 0.30789105220329
152.2 0.292512164593292
158.3 0.279487404389562
164.04 0.26836352833667
167.76 0.261675987761564
175.14 0.254091849933499
180.36 0.240172205097444
188.96 0.232655890921929
196.94 0.219470763233798
206.24 0.209992405322038
210.86 0.204437510832723
222.8 0.192649798798874
224.36 0.189667831860451
235.36 0.184410806479386
243.14 0.17557275711421
254.22 0.164141773670901
270.68 0.154786277869199
282.1 0.148172833506988
301.72 0.138288550759936
312 0.129784293300444
325.74 0.124235430620451
341.02 0.117401408087022
355.64 0.109556689931558
363.36 0.105979261357087
387.06 0.0994308781071243
409.18 0.092093138969042
434.98 0.0864860324795609
462.7 0.0793521371425046
488.84 0.0733663021360781
492.8 0.0711929131492074
518.98 0.0675048263666345
542.04 0.0641057508743184
585.44 0.0582091818720579
615.52 0.0551021654835362
680.08 0.0486042889713111
685.3 0.0470391860403103
717.8 0.0449200243684916
751.88 0.0422002792034109
810.56 0.0377578179923522
848.56 0.0354422900027783
919.6 0.0323040426924709
982.48 0.0301761323725828
1068.68 0.0270118751641665
1113.4 0.0254321975090708
1217.02 0.0238984821336962
1312.12 0.0210502243436265
1425.1 0.0186876875923264
1566.7 0.0165838706326232
1686.46 0.0153661693750526
1857.4 0.0133664525087314
1912.5 0.0123916913487644
2060.92 0.0111540448874587
2274.56 0.0100746369685574
2321.84 0.00899396095163764
2693.56 0.00786546212638548
2947.1 0.00688108933790973
3290.56 0.00584943796530894
3701.28 0.00464360908188495
3988.44 0.00432416633177911
4503.64 0.00372936054758154
5158.04 0.00325642840134679
5594.7 0.00285610095390129
5979.9 0.00266741034831772
6608.64 0.00246762878525333
7114.6 0.00238656448518115
7333.16 0.00230461987592059
7700.88 0.00223254771139725
8066.84 0.00213688836946819
8269.98 0.00205367747771717
8662.12 0.00197000267349547
9283.38 0.00189440796824074
9718.92 0.00181790813654742
};
\addplot [draw=darkgray153, fill=darkgray153, forget plot, mark=*, mark size=1, only marks, draw opacity=0,
 fill opacity=0.5]
table{%
x  y
33.46 0.99999999998787
105.22 0.516350028393451
114.84 0.482914145396095
122.5 0.457823085920236
129.82 0.426696876356409
139.38 0.405409901318726
148.46 0.385432613845023
157.78 0.362906474086134
162.72 0.350709540807902
180.5 0.327726196089315
191.68 0.303835908652141
202.26 0.283181052901277
222.34 0.260078822479622
229.58 0.246995972223367
244.66 0.229174151829273
269.9 0.208203455614653
286.46 0.200852868198735
303.06 0.188084657150798
326.52 0.174169591096697
340.96 0.162140138379211
359.86 0.15610534578047
384.02 0.145781652199329
396.92 0.134863060981767
420.46 0.126643794921641
451.42 0.118839016650845
474.82 0.113311188639173
510.72 0.101871139810333
532.74 0.0956781625888339
566.6 0.0883300881449651
602.16 0.0786745224699959
621.34 0.0752078171293834
632.86 0.0722764827080448
669.74 0.068196108752552
684 0.0660101432739054
721.64 0.0616739582696299
756.54 0.0585740930710847
774.66 0.05591699633592
799.86 0.053038188662944
835.84 0.0503446519683722
872.58 0.0486787627129453
898.1 0.0467447964344433
918.62 0.044943669038258
949.62 0.0426194720421062
964.08 0.0408116160929876
996.5 0.0381745064816794
1021.86 0.0360746805808819
1057.5 0.0341496527140785
1082.94 0.0334200975558145
1124.06 0.0320230759338757
1138.68 0.0308435188323597
1171.42 0.0297218818151027
1199.46 0.028621233040751
1260.32 0.0272068619051475
1282.48 0.026456517323812
1313.22 0.0254755261973134
1348.24 0.0240777334867999
1371.08 0.0233542395478935
1413.4 0.0224029331111788
1422.86 0.0219432992525787
1463.94 0.0212932242792785
1491.94 0.0202440222266589
1524.68 0.0196298434739734
1550.32 0.0190695697382172
1558.8 0.0186529545554306
1595.48 0.0181015191367999
1630.36 0.0173229752750418
1637.46 0.0168079985000023
1674.04 0.0163008531399759
1687.22 0.015710865933103
1727.24 0.0152685100931621
1753.98 0.0147310850430391
1785.86 0.0142668119491611
1819.24 0.0139265920581383
1843 0.0134568192268386
1893.46 0.0128940136409208
1911.64 0.0124667085353728
1980.24 0.0120903076848314
2002.44 0.0117314682611892
2030.36 0.0112521485158039
2068.02 0.0107474381865207
2111.64 0.0103922662654719
2197.16 0.009991898306606
2279.58 0.00955312450290415
2350.22 0.00923112451560228
2455.82 0.00882312206569614
2562.1 0.0084623857869774
2698.06 0.00787839598883674
2867.9 0.00739947518718363
3070.9 0.00685168288520462
3295.94 0.0063705072557461
3564.72 0.0057395047506942
3932.98 0.00526349308053081
4372.16 0.00470309973497842
4981 0.00414393512840152
5899.18 0.00355767919233107
7255.88 0.00304012389706951
9419.44 0.00250861240873134
};
\addplot [
  draw=saddlebrown1356716,
  fill=saddlebrown1356716,
  forget plot,
  mark=*, mark size=1,
  only marks,
  draw opacity=0,
 fill opacity=0.5
]
table{%
x  y
536.64 0.0983741953481614
601.54 0.0758075574347167
605.98 0.0743551514379984
622.1 0.0720247991577646
626.5 0.0712346989793696
634.88 0.0698027788710181
646.24 0.068574881687597
650.8 0.0678972702452076
671.14 0.0650328695656024
675.7 0.0640937800122216
682.92 0.0602198146112363
686.54 0.0617411208734235
700.96 0.0580644195600149
712.48 0.0565521220676408
732.92 0.0546282798184157
759.46 0.0529625200937498
773.06 0.0513375804050359
780.92 0.0497834833354104
809.18 0.0482153291441203
835.32 0.0461593861421519
844.88 0.0448321471687714
863.72 0.0438213931779754
873.42 0.0424823951646487
906.14 0.0402424828585582
923.08 0.0386999743962648
942.28 0.037284445606447
971.24 0.0354204850235839
1000.9 0.0345103905717458
1006.88 0.033753343613441
1021.78 0.0331228058296677
1051.22 0.0319047056058169
1074.76 0.0309892123577347
1101.76 0.0300382871443506
1137.56 0.0289668017065427
1166.6 0.0283480864366474
1188.06 0.0269594866827298
1209.38 0.0262524015252224
1249.14 0.0251142484884333
1276.62 0.0244562363905532
1305.34 0.0229560913335072
1329.12 0.0219295131433128
1368.1 0.02080777477216
1413.76 0.0199860447020218
1436.92 0.0194642893463472
1504.54 0.0182375292446639
1544.04 0.0172759873853777
1595.02 0.0168509187605283
1647.02 0.015906802084436
1735.22 0.0148159980786927
1813.62 0.0137476118442167
1886.72 0.0132276734345416
1942.18 0.0128170554766784
2041.12 0.0122812533563184
2102.48 0.0119214694458844
2162.96 0.0114946448926828
2245.82 0.0110105605951597
2323.72 0.0105656476057908
2393 0.0102523839122043
2490.44 0.00980792884686621
2577.62 0.00944381481053563
2689.42 0.00897081828532542
2765.06 0.00863674340986918
2869.32 0.00831051731364909
2960 0.00797507823452655
3062.46 0.00764736884948022
3193.26 0.00737066195777189
3359.02 0.00716067833850793
3458.44 0.00690546844623395
3588.72 0.00670201147223601
3678.78 0.00652146210156336
3812.02 0.00631707489683712
3928.8 0.00609773463518237
4089.42 0.00590894231537145
4173.6 0.00571288083891096
4322.68 0.00553567482726663
4456.78 0.00535503476247626
4641.36 0.00516057267762516
4760.24 0.00498088157026305
4962.34 0.00484973155755508
5171.96 0.00471486787620706
5329.68 0.00458739045934273
5576.74 0.00444280368252511
5742.9 0.00429590504226794
5913.02 0.00415609825060199
6171.14 0.00400275271040345
6413.76 0.00387066925385986
6744.18 0.00374487460663354
6900.66 0.00363910123242782
7044.16 0.00352861705671428
7325.66 0.00340395880866202
7664.22 0.00330013638813851
7970.24 0.0032020648380745
8133.3 0.00311500793808118
8447.46 0.00301743605019504
8809.56 0.00294664317875465
9097.24 0.0028685258006402
9567.2 0.00279483592134227
9915.94 0.00271345090165114
};
\addplot [very thick, royalblue28108204]
table {%
33.46 1.67900060170567
118.415151515152 0.437107546942947
203.370303030303 0.2479032518172
288.325454545455 0.172393875904882
373.280606060606 0.131952955027299
458.235757575758 0.10680677223613
543.190909090909 0.0896786051525251
628.146060606061 0.0772699614780849
713.101212121212 0.0678709683152558
798.056363636364 0.0605075762084314
883.011515151515 0.0545845415977001
967.966666666667 0.0497177648795855
1052.92181818182 0.0456483812381828
1137.87696969697 0.0421956135723157
1222.83212121212 0.0392294196738448
1307.78727272727 0.0366538767535185
1392.74242424242 0.0343966901712592
1477.69757575758 0.0324023465370068
1562.65272727273 0.0306275157699316
1647.60787878788 0.0290378854372416
1732.56303030303 0.0276059327866661
1817.51818181818 0.0263093258249105
1902.47333333333 0.0251297556442762
1987.42848484849 0.024052070198985
2072.38363636364 0.0230636225242094
2157.33878787879 0.0221537739442587
2242.29393939394 0.0213135109300696
2327.24909090909 0.0205351464008591
2412.20424242424 0.0198120845352644
2497.15939393939 0.0191386338837451
2582.11454545455 0.0185098575970225
2667.0696969697 0.0179214524497612
2752.02484848485 0.0173696504037019
2836.98 0.0168511379604278
2921.93515151515 0.0163629896640832
3006.8903030303 0.0159026129409719
3091.84545454546 0.0154677020842556
3176.80060606061 0.0150561996630857
3261.75575757576 0.0146662639956982
3346.71090909091 0.0142962416035635
3431.66606060606 0.0139446437791279
3516.62121212121 0.0136101265680986
3601.57636363636 0.0132914735997331
3686.53151515152 0.0129875813035007
3771.48666666667 0.0126974461340451
3856.44181818182 0.0124201534932953
3941.39696969697 0.0121548680924592
4026.35212121212 0.0119008255402497
4111.30727272727 0.0116573249791582
4196.26242424242 0.0114237226205767
4281.21757575758 0.0111994260533509
4366.17272727273 0.0109838892199514
4451.12787878788 0.0107766079706741
4536.08303030303 0.0105771161197584
4621.03818181818 0.0103849819385508
4705.99333333333 0.0101998050302484
4790.94848484849 0.0100212135386576
4875.90363636364 0.00984886165005749
4960.85878787879 0.0096824273528853
5045.81393939394 0.00952161042473311
5130.76909090909 0.00936613062019963
5215.72424242424 0.00921572603660393
5300.67939393939 0.00907015163752628
5385.63454545455 0.00892917791667862
5470.5896969697 0.00879258968679055
5555.54484848485 0.00866018498007538
5640.5 0.00853177404846704
5725.45515151515 0.00840717845322491
5810.4103030303 0.00828623023472493
5895.36545454546 0.00816877115431766
5980.32060606061 0.0080546520010604
6065.27575757576 0.00794373195693823
6150.23090909091 0.00783587801489856
6235.18606060606 0.00773096444464281
6320.14121212121 0.00762887230166577
6405.09636363636 0.0075294889755129
6490.05151515152 0.00743270777364858
6575.00666666667 0.0073384275377039
6659.96181818182 0.00724655228920211
6744.91696969697 0.00715699090215361
6829.87212121212 0.00706965680017326
6914.82727272727 0.0069844676760036
6999.78242424242 0.00690134523153389
7084.73757575758 0.00682021493658903
7169.69272727273 0.00674100580492623
7254.64787878788 0.00666365018602402
7339.60303030303 0.00658808357138018
7424.55818181818 0.00651424441415227
7509.51333333333 0.00644207396108133
7594.46848484849 0.00637151609573311
7679.42363636364 0.00630251719217825
7764.37878787879 0.0062350259783091
7849.33393939394 0.00616899340806072
7934.28909090909 0.00610437254186686
8019.24424242424 0.0060411184347382
8104.1993939394 0.00597918803140179
8189.15454545455 0.00591854006798749
8274.1096969697 0.00585913497978944
8359.06484848485 0.00580093481466895
8444.02 0.00574390315170049
};
\addplot [very thick, cadetblue80178158]
table {%
212.84 0.309668229593924
251.427474747475 0.30953297004364
290.01494949495 0.306700916127998
328.602424242424 0.302220509579732
367.189898989899 0.29673741838613
405.777373737374 0.290662288405579
444.364848484848 0.284262490553957
482.952323232323 0.277714960533494
521.539797979798 0.271137931411352
560.127272727273 0.264610659323292
598.714747474747 0.258186043894139
637.302222222222 0.251898901373672
675.889696969697 0.245771501040697
714.477171717172 0.239817335883911
753.064646464646 0.234043729449409
791.652121212121 0.228453661117926
830.239595959596 0.223047057847912
868.827070707071 0.217821716415029
907.414545454545 0.212773966478736
946.00202020202 0.207899149821116
984.589494949495 0.203191967916652
1023.17696969697 0.198646734385321
1061.76444444444 0.194257558228525
1100.35191919192 0.190018476382134
1138.93939393939 0.185923548969092
1177.52686868687 0.181966926991826
1216.11434343434 0.178142899604501
1254.70181818182 0.174445926232373
1293.28929292929 0.170870657445452
1331.87676767677 0.167411947498751
1370.46424242424 0.164064860718478
1409.05171717172 0.160824673370417
1447.63919191919 0.157686872241895
1486.22666666667 0.154647150865547
1524.81414141414 0.151701404084961
1563.40161616162 0.148845721489985
1601.98909090909 0.146076380118883
1640.57656565657 0.143389836725318
1679.16404040404 0.140782719832524
1717.75151515151 0.13825182173942
1756.33898989899 0.135794090599338
1794.92646464646 0.133406622658481
1833.51393939394 0.131086654715523
1872.10141414141 0.128831556844269
1910.68888888889 0.126638825406394
1949.27636363636 0.124506076370119
1987.86383838384 0.122431038942185
2026.45131313131 0.12041154951424
2065.03878787879 0.11844554592011
2103.62626262626 0.116531061997084
2142.21373737374 0.114666222441971
2180.80121212121 0.112849237951075
2219.38868686869 0.111078400632221
2257.97616161616 0.109352079676335
2296.56363636364 0.107668717275858
2335.15111111111 0.106026824777222
2373.73858585859 0.10442497905481
2412.32606060606 0.102861819094112
2450.91353535354 0.101336042772179
2489.50101010101 0.0998464038239405
2528.08848484848 0.0983917089834553
2566.67595959596 0.0969708152896676
2605.26343434343 0.0955826275467887
2643.85090909091 0.0942260959299458
2682.43838383838 0.0929002137272651
2721.02585858586 0.0916040152100605
2759.61333333333 0.0903365736232979
2798.20080808081 0.0890969992889674
2836.78828282828 0.0878844378154582
2875.37575757576 0.0866980684064501
2913.96323232323 0.0855371022632428
2952.55070707071 0.0844007810748365
2991.13818181818 0.0832883755904248
3029.72565656566 0.0821991842693147
3068.31313131313 0.0811325320035978
3106.90060606061 0.0800877689092028
3145.48808080808 0.0790642691812354
3184.07555555556 0.0780614300097793
3222.66303030303 0.0770786705525719
3261.25050505051 0.0761154309612024
3299.83797979798 0.0751711714576923
3338.42545454545 0.0742453714585193
3377.01292929293 0.0733375287433327
3415.6004040404 0.0724471586657809
3454.18787878788 0.0715737934040386
3492.77535353535 0.0707169812487685
3531.36282828283 0.0698762859263989
3569.9503030303 0.0690512859557267
3608.53777777778 0.0682415740359804
3647.12525252525 0.067446756464597
3685.71272727273 0.0666664525830658
3724.3002020202 0.0659002942493027
3762.88767676768 0.0651479253351023
3801.47515151515 0.0644090012473133
3840.06262626263 0.0636831884714553
3878.6501010101 0.0629701641365781
3917.23757575758 0.062269615600233
3955.82505050505 0.0615812400524933
3994.41252525253 0.0609047441380247
4033 0.0602398435952648
};
\addplot [very thick, chocolate21910927]
table {%
33.46 1.01500839203872
104.519393939394 0.54043138988337
175.578787878788 0.38965867997721
246.638181818182 0.310251012228245
317.697575757576 0.259981015386981
388.75696969697 0.224840416022255
459.816363636364 0.198686555108804
530.875757575758 0.178356833849184
601.935151515152 0.162040776013445
672.994545454545 0.148620278728776
744.053939393939 0.137364213665756
815.113333333333 0.12777263017195
886.172727272727 0.119491127791315
957.232121212121 0.112260927037017
1028.29151515152 0.105888318537467
1099.35090909091 0.100225205240615
1170.4103030303 0.0951562827492292
1241.4696969697 0.0905903442897781
1312.52909090909 0.0864542328498237
1383.58848484848 0.0826885407579076
1454.64787878788 0.0792444916487052
1525.70727272727 0.0760816401774333
1596.76666666667 0.0731661484462778
1667.82606060606 0.0704694763429539
1738.88545454545 0.0679673736855325
1809.94484848485 0.0656390956133123
1881.00424242424 0.0634667852886101
1952.06363636364 0.0614349835009419
2023.12303030303 0.0595302355905479
2094.18242424242 0.0577407737666106
2165.24181818182 0.0560562583864961
2236.30121212121 0.0544675657483978
2307.36060606061 0.0529666128767807
2378.42 0.0515462119524492
2449.47939393939 0.0501999486675749
2520.53878787879 0.0489220800182097
2591.59818181818 0.047707447987285
2662.65757575758 0.046551406294826
2733.71696969697 0.0454497579533359
2804.77636363636 0.0443987018046908
2875.83575757576 0.0433947865596675
2946.89515151515 0.0424348711341467
3017.95454545455 0.0415160902934086
3089.01393939394 0.0406358247900674
3160.07333333333 0.0397916753214636
3231.13272727273 0.0389814397459172
3302.19212121212 0.0382030930896824
3373.25151515152 0.0374547699520342
3444.31090909091 0.0367347489780042
3515.3703030303 0.0360414391195119
3586.4296969697 0.0353733674480705
3657.48909090909 0.0347291683175482
3728.54848484848 0.0341075737049307
3799.60787878788 0.0335074045817297
3870.66727272727 0.0329275631894488
3941.72666666667 0.0323670261100392
4012.78606060606 0.0318248380371092
4083.84545454545 0.031300106166252
4154.90484848485 0.0307919951335767
4225.96424242424 0.0302997224406951
4297.02363636364 0.0298225543122645
4368.08303030303 0.0293598019389251
4439.14242424242 0.0289108180642799
4510.20181818182 0.0284749938795707
4581.26121212121 0.0280517561940436
4652.32060606061 0.0276405648527584
4723.38 0.027240910376863
4794.43939393939 0.0268523118042082
4865.49878787879 0.0264743147106616
4936.55818181818 0.0261064893946572
5007.61757575758 0.0257484292094281
5078.67696969697 0.0253997490290398
5149.73636363636 0.0250600838358256
5220.79575757576 0.0247290874181168
5291.85515151515 0.0244064311683174
5362.91454545455 0.0240918029723841
5433.97393939394 0.0237849061826757
5505.03333333333 0.0234854586669356
5576.09272727273 0.0231931919268813
5647.15212121212 0.0229078502805095
5718.21151515152 0.0226291901027891
5789.27090909091 0.0223569791199178
5860.3303030303 0.0220909957527736
5931.3896969697 0.0218310285055902
6002.44909090909 0.0215768753962543
6073.50848484848 0.0213283434249432
6144.56787878788 0.0210852480781173
6215.62727272727 0.0208474128651445
6286.68666666667 0.0206146688850706
6357.74606060606 0.0203868544212655
6428.80545454546 0.0201638145618685
6499.86484848485 0.0199454008441308
6570.92424242424 0.0197314709209139
6641.98363636364 0.0195218882477431
6713.04303030303 0.0193165217889518
6784.10242424242 0.0191152457415646
6855.16181818182 0.018917939275681
6926.22121212121 0.0187244862902155
6997.28060606061 0.0185347751829429
7068.34 0.018348698633878
};
\addplot [very thick, purple11522131]
table {%
106.9 0.498800574534795
192.542626262626 0.274714168780336
278.185252525253 0.192060289373707
363.827878787879 0.149017615139884
449.470505050505 0.122554943904126
535.113131313131 0.104599698247241
620.755757575758 0.091592167417923
706.398383838384 0.0817183967338305
792.04101010101 0.07395647929024
877.683636363636 0.067686506976211
963.326262626263 0.0625104008532112
1048.96888888889 0.0581607055574666
1134.61151515152 0.0544509882017724
1220.25414141414 0.0512472597077997
1305.89676767677 0.0484507060599962
1391.53939393939 0.0459868285031698
1477.18202020202 0.04379837789038
1562.82464646465 0.041840620796722
1648.46727272727 0.0400780857888548
1734.1098989899 0.0384822762174509
1819.75252525253 0.0370300300741204
1905.39515151515 0.0357023227501416
1991.03777777778 0.0344833790228041
2076.6804040404 0.0333600048276136
2162.32303030303 0.0323210777883855
2247.96565656566 0.0313571541195392
2333.60828282828 0.0304601619831704
2419.25090909091 0.0296231598697469
2504.89353535354 0.0288401444406661
2590.53616161616 0.0281058963906726
2676.17878787879 0.0274158558194373
2761.82141414141 0.0267660207137088
2847.46404040404 0.0261528636812007
2933.10666666667 0.0255732632121498
3018.74929292929 0.0250244465893276
3104.39191919192 0.024503942202286
3190.03454545455 0.0240095395031574
3275.67717171717 0.023539255209568
3361.3197979798 0.0230913046440389
3446.96242424242 0.0226640773196333
3532.60505050505 0.0222561160539371
3618.24767676768 0.0218660990291088
3703.8903030303 0.021492824323187
3789.53292929293 0.0211351965234668
3875.17555555556 0.0207922151013726
3960.81818181818 0.0204629642835428
4046.46080808081 0.0201466041986112
4132.10343434343 0.0198423631156143
4217.74606060606 0.019549530619742
4303.38868686869 0.0192674515956209
4389.03131313131 0.018995520908505
4474.67393939394 0.0187331786904586
4560.31656565657 0.0184799061525209
4645.95919191919 0.0182352218554362
4731.60181818182 0.017998678381253
4817.24444444444 0.0177698593562577
4902.88707070707 0.0175483767826012
4988.5296969697 0.0173338686417952
5074.17232323232 0.0171259967382092
5159.81494949495 0.0169244447548989
5245.45757575758 0.0167289164976973
5331.1002020202 0.0165391343065704
5416.74282828283 0.0163548376158806
5502.38545454545 0.0161757816474753
5588.02808080808 0.0160017362224729
5673.67070707071 0.0158324846793169
5759.31333333333 0.0156678228871375
5844.95595959596 0.0155075583447346
5930.59858585859 0.0153515093566085
6016.24121212121 0.0151995042784344
6101.88383838384 0.0150513808252239
6187.52646464646 0.0149069854361597
6273.16909090909 0.0147661726907416
6358.81171717172 0.0146288047714556
6444.45434343434 0.0144947509686824
6530.09696969697 0.0143638872240084
6615.7395959596 0.0142360957084953
6701.38222222222 0.0141112644328161
6787.02484848485 0.0139892868864708
6872.66747474747 0.0138700617035752
6958.3101010101 0.0137534923529585
7043.95272727273 0.0136394868505226
7129.59535353535 0.0135279574920145
7215.23797979798 0.0134188206045336
7300.88060606061 0.0133119963152551
7386.52323232323 0.0132074083359867
7472.16585858586 0.0131049837623054
7557.80848484849 0.0130046528861298
7643.45111111111 0.0129063490206887
7729.09373737374 0.0128100083369351
7814.73636363636 0.0127155697105389
7900.37898989899 0.0126229745786654
7986.02161616162 0.0125321668058145
8071.66424242424 0.0124430925580561
8157.30686868687 0.0123557001850521
8242.94949494949 0.0122699401093073
8328.59212121212 0.012185764722134
8414.23474747475 0.0121031282858592
8499.87737373737 0.0120219868418405
8585.52 0.0119422981238888
};
\addplot [very thick, black18]
table {%
33.46 1.4593570153175
131.292929292929 0.33597457017964
229.125858585859 0.178302926498061
326.958787878788 0.117712488533604
424.791717171717 0.0862474322186312
522.624646464647 0.0672049903536047
620.457575757576 0.0545472261960417
718.290505050505 0.0455800366369735
816.123434343434 0.0389269904138078
913.956363636364 0.0338145777368928
1011.78929292929 0.0297761412578729
1109.62222222222 0.0265142126871966
1207.45515151515 0.0238306381086493
1305.28808080808 0.0215885759044768
1403.12101010101 0.0196906404305419
1500.95393939394 0.0180657363633063
1598.78686868687 0.0166608129314756
1696.6197979798 0.0154355246874236
1794.45272727273 0.0143586733198525
1892.28565656566 0.0134057759946624
1990.11858585859 0.0125573663072754
2087.95151515152 0.0117977835106241
2185.78444444444 0.0111142943620444
2283.61737373737 0.0104964460353602
2381.4503030303 0.00993558240977974
2479.28323232323 0.00942447773936005
2577.11616161616 0.00895705589430503
2674.94909090909 0.00852817282213617
2772.78202020202 0.00813344629032121
2870.61494949495 0.00776912139117889
2968.44787878788 0.00743196337974932
3066.28080808081 0.00711917160506123
3164.11373737374 0.00682830986658267
3261.94666666667 0.00655724966841214
3359.7795959596 0.00630412368095255
3457.61252525253 0.00606728734044046
3555.44545454546 0.00584528698116599
3653.27838383838 0.00563683324590884
3751.11131313131 0.00544077878712041
3848.94424242424 0.00525609947627353
3946.77717171717 0.0050818784971991
4044.6101010101 0.00491729282254375
4142.44303030303 0.00476160166912456
4240.27595959596 0.00461413660417032
4338.10888888889 0.00447429303490515
4435.94181818182 0.00434152286217244
4533.77474747475 0.00421532811749779
4631.60767676768 0.00409525543419369
4729.44060606061 0.00398089122839396
4827.27353535354 0.00387185748649008
4925.10646464647 0.00376780807227447
5022.93939393939 0.00366842548092028
5120.77232323232 0.00357341797832752
5218.60525252525 0.00348251707380363
5316.43818181818 0.00339547528189051
5414.27111111111 0.00331206413569213
5512.10404040404 0.0032320724195324
5609.93696969697 0.00315530459337188
5707.7698989899 0.00308157938528587
5805.60282828283 0.00301072853158087
5903.43575757576 0.00294259564690239
6001.26868686869 0.00287703520904634
6099.10161616162 0.00281391164519842
6196.93454545455 0.00275309850804533
6294.76747474748 0.00269447773167576
6392.60040404041 0.00263793895845547
6490.43333333333 0.00258337892915164
6588.26626262626 0.00253070092952346
6686.09919191919 0.00247981428741106
6783.93212121212 0.00243063391506161
6881.76505050505 0.00238307989204578
6979.59797979798 0.00233707708465291
7077.43090909091 0.00229255479812035
7175.26383838384 0.00224944645846043
7273.09676767677 0.00220768932100668
7370.9296969697 0.00216722420311484
7468.76262626263 0.0021279952387303
7566.59555555556 0.00208994965277688
7664.42848484849 0.0020530375535367
7762.26141414142 0.00201721174138034
7860.09434343434 0.00198242753237464
7957.92727272727 0.00194864259544441
8055.7602020202 0.00191581680189663
8153.59313131313 0.00188391208623302
8251.42606060606 0.0018528923172822
8349.25898989899 0.00182272317877572
8447.09191919192 0.00179337205857567
8544.92484848485 0.00176480794583656
8642.75777777778 0.00173700133545083
8740.59070707071 0.00170992413918718
8838.42363636364 0.00168354960298512
8936.25656565657 0.00165785222991718
9034.0894949495 0.00163280770837391
9131.92242424242 0.00160839284506623
9229.75535353535 0.00158458550247482
9327.58828282828 0.0015613645404084
9425.42121212121 0.00153870976136168
9523.25414141414 0.00151660185938986
9621.08707070707 0.00149502237224037
9718.92 0.00147395363650397
};
\addplot [very thick, darkgray153]
table {%
33.46 1.69191700933645
128.267878787879 0.447554457141191
223.075757575758 0.241440602556597
317.883636363636 0.159228389572664
412.691515151515 0.115921969415235
507.499393939394 0.0895704378379832
602.307272727273 0.0720345081062379
697.115151515152 0.0596270141082406
791.92303030303 0.0504459798882598
886.730909090909 0.043415892988359
981.538787878788 0.0378853117773912
1076.34666666667 0.0334379698522868
1171.15454545455 0.0297962154202134
1265.96242424242 0.0267682157259211
1360.7703030303 0.0242174705999559
1455.57818181818 0.0220443930755938
1550.38606060606 0.0201747475993993
1645.19393939394 0.0185521517543957
1740.00181818182 0.0171330738337915
1834.8096969697 0.0158834119175643
1929.61757575758 0.0147761028371819
2024.42545454546 0.0137894182202084
2119.23333333333 0.012905728892899
2214.04121212121 0.0121105947731601
2308.84909090909 0.0113920849433668
2403.65696969697 0.0107402630948168
2498.46484848485 0.0101467935062485
2593.27272727273 0.00960463604136062
2688.08060606061 0.00910780769115457
2782.88848484849 0.00865119441930351
2877.69636363636 0.0082304014276146
2972.50424242424 0.00784163304819024
3067.31212121212 0.00748159568600683
3162.12 0.00714741884508694
3256.92787878788 0.00683659045237515
3351.73575757576 0.00654690356866178
3446.54363636364 0.00627641223067544
3541.35151515152 0.00602339466264937
3636.15939393939 0.005786322471742
3730.96727272727 0.00556383473012844
3825.77515151515 0.0053547160694338
3920.58303030303 0.00515787808656469
4015.39090909091 0.00497234349578335
4110.19878787879 0.00479723256888124
4205.00666666667 0.00463175149014158
4299.81454545455 0.00447518232041443
4394.62242424243 0.00432687431883764
4489.4303030303 0.00418623641441085
4584.23818181818 0.0040527306549884
4679.04606060606 0.00392586649001609
4773.85393939394 0.00380519576683319
4868.66181818182 0.00369030833964093
4963.4696969697 0.00358082820612204
5058.27757575758 0.00347641009983327
5153.08545454546 0.00337673647740076
5247.89333333333 0.00328151484863574
5342.70121212121 0.00319047540528778
5437.50909090909 0.00310336891052816
5532.31696969697 0.0030199648166217
5627.12484848485 0.00294004958277589
5721.93272727273 0.00286342516899228
5816.74060606061 0.00278990768500364
5911.54848484849 0.00271932617615436
6006.35636363637 0.00265152153045174
6101.16424242424 0.00258634549304376
6195.97212121212 0.00252365977612041
6290.78 0.00246333525373401
6385.58787878788 0.00240525123232548
6480.39575757576 0.00234929478886095
6575.20363636364 0.00229536016945058
6670.01151515152 0.00224334824216127
6764.8193939394 0.00219316599846659
6859.62727272727 0.00214472609841353
6954.43515151515 0.00209794645514312
7049.24303030303 0.00205274985488863
7144.05090909091 0.00200906360900224
7238.85878787879 0.00196681923493641
7333.66666666667 0.00192595216343617
7428.47454545455 0.00188640146948952
7523.28242424243 0.00184810962484022
7618.0903030303 0.00181102227009419
7712.89818181818 0.00177508800465224
7807.70606060606 0.00174025819288011
7902.51393939394 0.00170648678508571
7997.32181818182 0.00167373015201416
8092.1296969697 0.00164194693169736
8186.93757575758 0.00161109788760671
8281.74545454545 0.00158114577715795
8376.55333333333 0.00155205522970673
8471.36121212121 0.00152379263325386
8566.16909090909 0.0014963260291511
8660.97696969697 0.00146962501416339
8755.78484848485 0.00144366064930098
8850.59272727273 0.00141840537488801
8945.40060606061 0.00139383293138072
9040.20848484849 0.00136991828549124
9135.01636363636 0.00134663756121141
9229.82424242424 0.00132396797536578
9324.63212121212 0.00130188777735451
9419.44 0.00128037619277517
};
\addplot [very thick, saddlebrown1356716]
table {%
536.64 0.0945091187652701
631.380404040404 0.0712776036769703
726.120808080808 0.0563763363038157
820.861212121212 0.046176013603196
915.601616161616 0.0388429947656358
1010.34202020202 0.0333660486878142
1105.08242424242 0.0291483732213797
1199.82282828283 0.0258181842722419
1294.56323232323 0.0231334234346699
1389.30363636364 0.0209305985650308
1484.04404040404 0.0190958030526896
1578.78444444444 0.0175475407165928
1673.52484848485 0.0162261475351318
1768.26525252525 0.0150870561362075
1863.00565656566 0.0140963808736072
1957.74606060606 0.0132279491516685
2052.48646464646 0.0124612595177057
2147.22686868687 0.0117800485109233
2241.96727272727 0.0111712663335959
2336.70767676768 0.0106243326050827
2431.44808080808 0.0101305874952887
2526.18848484849 0.0096828814069366
2620.92888888889 0.00927526439145746
2715.66929292929 0.00890274835213044
2810.4096969697 0.00856112304553423
2905.1501010101 0.00824681231399378
2999.8905050505 0.00795676073090159
3094.63090909091 0.00768834346936089
3189.37131313131 0.00743929407117366
3284.11171717172 0.00720764613452449
3378.85212121212 0.00699168591334336
3473.59252525253 0.00678991353690444
3568.33292929293 0.00660101108872631
3663.07333333333 0.00642381618075529
3757.81373737374 0.00625729995834341
3852.55414141414 0.00610054869941263
3947.29454545455 0.00595274834589541
4042.03494949495 0.00581317144044993
4136.77535353535 0.00568116604633799
4231.51575757576 0.00555614631044677
4326.25616161616 0.00543758439407625
4420.99656565657 0.00532500354732016
4515.73696969697 0.00521797214365464
4610.47737373737 0.00511609852401374
4705.21777777778 0.005019026525922
4799.95818181818 0.0049264315945215
4894.69858585859 0.00483801738961189
4989.43898989899 0.00475351281692986
5084.17939393939 0.00467266942345695
5178.9197979798 0.00459525910606554
5273.6602020202 0.00452107209067792
5368.40060606061 0.00444991514563927
5463.14101010101 0.0043816099984374
5557.88141414142 0.00431599192944217
5652.62181818182 0.00425290852014008
5747.36222222222 0.00419221853654207
5842.10262626263 0.0041337909311394
5936.84303030303 0.00407750394906896
6031.58343434344 0.00402324432608675
6126.32383838384 0.00397090656759887
6221.06424242424 0.00392039229940687
6315.80464646465 0.00387160968202974
6410.54505050505 0.00382447288149771
6505.28545454545 0.003778901590402
6600.02585858586 0.00373482059375088
6694.76626262626 0.00369215937484413
6789.50666666667 0.0036508517569513
6884.24707070707 0.00361083557707644
6978.98747474748 0.00357205238852469
7073.72787878788 0.00353444718936319
7168.46828282828 0.00349796817419773
7263.20868686869 0.00346256650697465
7357.94909090909 0.00342819611277031
7452.6894949495 0.00339481348675132
7547.4298989899 0.00336237751868471
7642.1703030303 0.00333084933154844
7736.91070707071 0.00330019213294445
7831.65111111111 0.00327037107815096
7926.39151515152 0.00324135314376899
8021.13191919192 0.00321310701102393
8115.87232323232 0.00318560295787628
8210.61272727273 0.00315881275917908
8305.35313131313 0.00313270959419384
8400.09353535354 0.00310726796084265
8494.83393939394 0.0030824635961339
8589.57434343434 0.00305827340225123
8684.31474747475 0.0030346753778432
8779.05515151515 0.00301164855409391
8873.79555555555 0.00298917293519197
8968.53595959596 0.00296722944285109
9063.27636363636 0.00294579986456496
9158.01676767677 0.00292486680530801
9252.75717171717 0.00290441364241837
9347.49757575758 0.00288442448342194
9442.23797979798 0.00286488412657748
9536.97838383838 0.00284577802394074
9631.71878787879 0.0028270922467627
9726.45919191919 0.00280881345305257
9821.1995959596 0.00279092885714956
9915.94 0.00277342620116039
};
\addplot [draw=black, fill=black, mark=x, very thick, mark size=2.5pt, only marks]
table{%
x  y
134.72 0.338602550307043
536.64 0.0983741953481614
2145.28 0.0329825118653072
8560.64 0.0119319398987522
};
