# Supplementary material for: Swarm Reinforcement Learning For Adaptive Mesh Refinement
Source: arXiv:2304.00818 source file (2023-10-09)
Supplement: Supplementary file 10 [file group_additional_metrics_l4.tex]

\nextgroupplot[
ylabel shift = -0.2cm,
title style={yshift=-0.2cm},
height=4.5cm,
width=0.50\textwidth,
ylabel={Mean Error},
xlabel={\empty},
title={Linear Elasticity},
scaled x ticks=false,
clip marker paths=true,
legend cell align={left},
legend style={fill opacity=0.8, draw opacity=1, text opacity=1, draw=lightgray204},
log basis y={10},
tick align=outside,
tick pos=left,
x grid style={darkgray176},
xmajorgrids,
xmin=-550.266, xmax=12033.866,
xtick style={color=black},
xtick={-2000,0,2000,4000,6000,8000,10000,12000,14000},
xticklabels={-2.0,0.0,2.0,4.0,6.0,8.0,10.0,12.0,14.0},
y grid style={darkgray176},
ymajorgrids,
ymin=0.00512852597236402, ymax=1.91827218862113,
ymode=log,
ytick style={color=black},
ytick={0.0001,0.001,0.01,0.1,1,10,100},
yticklabels={
  \(\displaystyle {10^{-4}}\),
  \(\displaystyle {10^{-3}}\),
  \(\displaystyle {10^{-2}}\),
  \(\displaystyle {10^{-1}}\),
  \(\displaystyle {10^{0}}\),
  \(\displaystyle {10^{1}}\),
  \(\displaystyle {10^{2}}\)
}
]
\addplot [
  draw=royalblue28108204,
  fill=royalblue28108204,
  forget plot,
  mark=*, mark size=1,
  only marks,
  draw opacity=0,
 fill opacity=0.5
]
table{%
x  y
270.98 0.299006061573925
348.2 0.25910997898235
355.54 0.270780517169287
368.46 0.242279850569682
392.84 0.232497464294626
411.22 0.218696524424197
430.54 0.195461296820753
438.8 0.225162801860571
450.28 0.204299439041497
493.32 0.184813361366991
520.12 0.178522433492857
577.34 0.148436805245509
590.26 0.158361331370352
654.84 0.13979890174314
660.6 0.145203202814009
673.62 0.152557421743582
677.66 0.15197419229147
678.16 0.152504557395195
678.84 0.14029219710301
727.34 0.134478945226562
736.68 0.196266704438969
813.18 0.126517488144663
825.78 0.10846346465524
852.48 0.115665189940684
879.7 0.104756126326896
890.76 0.0993327909194987
917.44 0.0951582498428127
921.42 0.111629588443845
954.82 0.11754964567202
1028.88 0.0999810311297168
1256.04 0.0705674798999759
1286.48 0.0660473456638291
1320.14 0.0695451923726273
1328.4 0.0683415467170694
1375.98 0.0617397779923147
1382.78 0.0647610403013882
1512.08 0.0622080923714642
1525.88 0.0611299784780744
1618.84 0.0549604042342549
1663.86 0.0575613107200808
1781.66 0.050291256163705
1799.02 0.0472829266881835
1866.16 0.046249910434352
1871 0.049134542306879
1961.86 0.0516948736651631
1997.84 0.0492271152061607
2031.54 0.0437458139728091
2158.14 0.0466103475311052
2171.98 0.0410526693793569
2196.22 0.0520267736018319
2228.22 0.0435309687019002
2490.8 0.0397071171973774
2663.6 0.029887926376111
2692.52 0.0342920487235238
2744.9 0.0295306048214588
2771.14 0.0350219596097533
2900.68 0.034171570411988
2956 0.0296789571889184
3026.28 0.0306715434279613
3090.62 0.0290326303292541
3186.12 0.0263200120690673
3332.02 0.0236894251797578
3375.18 0.0274515441172976
3470.52 0.0231770021376763
3495.26 0.0239798690318413
3517.2 0.0235313765523282
3595.28 0.0261818178266814
3673.24 0.02559545882007
3728.42 0.024168875887736
4392.22 0.0201922159190329
4562.48 0.019524600039237
4610.46 0.0192872339299318
4613.82 0.0203847444571053
4616.98 0.018338500763457
4629.7 0.0192138970890241
4716.78 0.0172022139460401
5013.8 0.0189164596546948
5042.36 0.0166924014491182
5056 0.0183534336509692
5118.94 0.0167616821310883
5226.12 0.0184256348661216
5715.7 0.0155768778803017
5749.24 0.0144318021501676
6195.3 0.0141120112533817
6327.42 0.01309494282439
6437.36 0.0147159038332097
7025.82 0.0115867912925645
7140.38 0.0126739951758384
7306.82 0.0107115747019937
7355.04 0.0119158910628391
7929.54 0.0126019936366407
7980.4 0.00892139531621997
8264.72 0.00858265877453217
8556.06 0.00976942271467917
8725.08 0.00756528324724917
8947.48 0.00757948543505046
9346.38 0.00812880156358449
9548.82 0.0087144673642854
9669.8 0.00714149769426307
10181.7 0.00671341295788591
};
\addplot [
  draw=cadetblue80178158,
  fill=cadetblue80178158,
  forget plot,
  mark=*, mark size=1,
  only marks,
  draw opacity=0,
 fill opacity=0.5
]
table{%
x  y
210.16 0.332268736165979
210.38 0.317315141169536
211.12 0.289276846672753
218.96 0.328699636997378
222.76 0.362931295536743
230.08 0.340753068271997
262.52 0.355924470619747
284.38 0.483756283419372
293.02 0.578814134875912
333.16 0.420777912097089
398.72 0.188952672876305
419.32 0.25060527276196
422.78 0.187107593345768
429.1 0.226283196001505
463.12 0.257622378276496
467.46 0.712551729523946
472.62 0.518955223531677
488.68 0.295888486797582
507.3 0.185559236738179
531.5 0.20141556688135
532.62 0.22156543309495
558.94 0.240179559069332
576.32 0.171552351768844
600.54 0.368151226359535
623.72 0.251358969002923
627.72 0.260390615232151
633.04 0.279131225865239
639.88 0.445350308963974
699.62 0.298452892635903
704.48 0.281948901310517
736.44 0.146331761174699
736.74 0.368835515055186
850.2 0.20264051504571
854.3 0.216432902563278
881.6 0.174981854528725
897.14 0.132683579888517
898.78 0.220219031769558
928.74 0.144941346432965
933.5 0.444370535597655
941.8 0.484397948622168
990.72 0.126453726388259
1001.7 0.11789679355132
1018.6 0.393981812268361
1049.98 0.111211595242318
1060.78 0.453768220535371
1083.74 0.153874663528964
1140.98 0.0834216615673218
1164.16 0.110246187697082
1208.06 0.0934353582347445
1208.48 0.0947716180716977
1209.98 0.163459163946469
1214.34 0.147675647114497
1229.14 0.134524515739899
1234.98 0.0993470238277686
1242.68 0.227303842142592
1279.76 0.0871680782245781
1324.9 0.0890078201376326
1329 0.118634493203949
1347.32 0.0836846482037108
1433.92 0.451124907525216
1500.2 0.0827941324827171
1526.04 0.066943441204665
1553.78 0.124037931286626
1574.08 0.0875457832880069
1580.3 0.118884175982181
1585.06 0.0810275546750743
1590.38 0.0766347181534238
1607.82 0.194626496027404
1608.16 0.0766338988255483
1646 0.0967918389550091
1658.72 0.063344067821623
1668.76 0.101940737223019
1717.86 0.0709787005532946
1739.64 0.0670968347551952
1742.52 0.223371620299426
1745.76 0.0678727453397716
1768.46 0.136765879429944
1807.02 0.0800742523115245
1813.7 0.0780491147314562
1875.24 0.0705447035433655
1883.7 0.169532662406632
1916.64 0.0707270273577733
2000.86 0.113482573286881
2025.18 0.0629921803673203
2059 0.0641103814456508
2153.04 0.0884066327780211
2209.04 0.0922537452233251
2224.6 0.0549229214547052
2261.1 0.0489666350206334
2311.82 0.238717482381688
2360.2 0.0459762169195444
2402.84 0.0555359081503642
2620.68 0.0846963765747154
2685.68 0.0567176170327627
2735.32 0.0475207056759815
2745.56 0.0473476301397378
2827.28 0.0397925071517442
2856.42 0.0500224631593903
3088.84 0.053050030524986
3508.24 0.17159950951218
};
\addplot [
  draw=chocolate21910927,
  fill=chocolate21910927,
  forget plot,
  mark=*, mark size=1,
  only marks,
  draw opacity=0,
 fill opacity=0.5
]
table{%
x  y
21.74 0.99999999991376
23.18 0.999999999931976
23.32 0.999999999930948
23.52 0.999999999932831
23.76 0.999999999931698
23.84 0.99999999993254
23.88 0.999999999932356
23.88 0.999999999932356
23.88 0.999999999932356
23.88 0.999999999932356
23.88 0.999999999932356
23.88 0.999999999932356
23.88 0.999999999932356
23.88 0.999999999932356
23.88 0.999999999932356
23.88 0.999999999932356
23.88 0.999999999932356
23.88 0.999999999932356
23.88 0.999999999932356
23.88 0.999999999932356
23.88 0.999999999932356
23.88 0.999999999932356
23.88 0.999999999932356
23.88 0.999999999932356
23.88 0.999999999932356
23.88 0.999999999932356
23.88 0.999999999932356
23.88 0.999999999932356
23.88 0.999999999932356
23.88 0.999999999932356
23.88 0.999999999932356
23.88 0.999999999932356
23.88 0.999999999932356
23.88 0.999999999932356
23.88 0.999999999932356
23.88 0.999999999932356
23.88 0.999999999932356
23.88 0.999999999932356
23.88 0.999999999932356
23.88 0.999999999932356
25.1 1.00049799544673
56.26 0.807772485914915
66.62 0.593331885521158
77.08 0.53386458837952
115.34 0.395650342103367
128.02 0.420962974054701
128.72 0.558091977956895
158.24 0.966357279930697
183.68 0.349069442270222
191.92 0.438294295664082
215.08 0.323725619004556
238.14 0.832254340231318
243.82 0.216023919002224
250.64 0.22961486835735
252.14 0.444741801560932
283.1 0.204157920436068
352.6 0.185502532377457
398.34 0.26160376451922
413.22 0.154265620351664
422.74 0.225315678088383
426.3 0.168657850518265
430.74 0.234214940119378
453.36 0.160598991331002
469.66 0.14726224426523
537.48 0.151841374296993
538.46 0.221098538075828
593.38 0.194756603799558
615.38 0.15228460585292
646.86 0.153347498377356
678.2 0.153791473103854
821.88 0.181590734711409
837 0.177820627575278
930.6 0.13342520046171
1158.44 0.080585490746031
1685.46 0.183404757764541
1723.26 0.0591105347698943
1732.58 0.272263542486899
1817.58 0.0574855119502551
2501.78 0.074027694751875
2660.7 0.0751060828888797
2718.8 0.086933085193926
3484.16 0.0832910752316459
3980.38 0.0523446471207853
4435.78 0.0329272859989326
8257.86 0.0144160201517144
9787.04 0.0327129396511796
10020.1 0.0331866901306974
10084.6 0.0492416897172995
};
\addplot [draw=purple11522131, fill=purple11522131, forget plot, mark=*, mark size=1, only marks, draw opacity=0,
 fill opacity=0.5]
table{%
x  y
333.1 0.200040316550262
354.14 0.197019354092078
363.12 0.202857413691859
364.34 0.187984804222347
386.28 0.174754566870086
391.9 0.171121677082445
415.7 0.173579634589385
432.94 0.161132607963896
450.06 0.151638096287692
450.98 0.137861982868126
969.68 0.0969916699830544
1091.02 0.0924146443420061
1183 0.0924851640569126
1251.1 0.0915005640570178
1288.3 0.10798287727823
1309.04 0.0887575782855517
1339.34 0.0889228290436248
1342.94 0.0875371728975888
1354.56 0.0879215345085591
1403.28 0.0889300844701582
1406.06 0.0870320094062931
1408.92 0.0876545231264563
1451.52 0.0862890974899711
1452.7 0.086254651185875
1452.8 0.0862508073444902
1452.8 0.0862508073444902
1452.8 0.0862508073444902
1452.98 0.0862035094363672
1453.68 0.086191280450082
1453.82 0.0859887733021502
1569.66 0.0592484908078443
1648.96 0.0591272173163831
1799.76 0.0684836959263313
1894.24 0.0567706731478341
1931.76 0.0670228553635988
2098.96 0.0784585228067788
2272.66 0.0526118321514547
2596.86 0.0525548085816587
2852.84 0.0501041529298205
3299.98 0.038058600595271
3921.54 0.047222853822651
4107.76 0.0472882559833154
4296.54 0.0467130808670481
4958.26 0.0399145156827133
5212.04 0.0339802039291702
5669.74 0.0336320968884412
5677.08 0.0344398829539787
5752.48 0.0333065661172312
5754.28 0.0332955408308812
5754.84 0.0332949267118625
5754.88 0.0332949259765874
5754.88 0.0332949259765874
5754.88 0.0332949259765874
5754.88 0.0332949259765874
5754.88 0.0332949259765874
5754.88 0.0332949259765874
5754.88 0.0332949259765874
5754.88 0.0332949259765874
5754.88 0.0332949259765874
5754.88 0.0332949259765874
5754.88 0.0332949259765874
5754.88 0.0332949259765874
5754.88 0.0332949259765874
5754.88 0.0332949259765874
5754.88 0.0332949259765874
5754.88 0.0332949259765874
5754.88 0.0332949259765874
5754.88 0.0332949259765874
5754.88 0.0332949259765874
5754.88 0.0332949259765874
5774.88 0.0332648993538906
5800.96 0.0331516466206832
5800.96 0.0331516466206832
5800.96 0.0331516466206832
5800.96 0.0331516466206832
5800.96 0.0331516466206832
5800.96 0.0331516466206832
5800.96 0.0331516466206832
5800.96 0.0331516466206832
5800.96 0.0331516466206832
5800.96 0.0331516466206832
6427.1 0.030740188382911
6742.3 0.0306833949762741
6743.04 0.0306686520831985
6743.04 0.0306686520831985
6743.04 0.0306686520831985
6743.04 0.0306686520831985
6743.04 0.0306686520831985
6743.04 0.0306686520831985
6743.04 0.0306686520831985
6952.3 0.0183039571016531
9174.24 0.0183543639726229
};
\addplot [draw=black18, fill=black18, forget plot, mark=*, mark size=1, only marks, draw opacity=0,
 fill opacity=0.5]
table{%
x  y
23.88 0.999999999932356
72.62 0.499894999848985
75.36 0.488888204876539
77.56 0.475268720720179
79.5 0.469922869230011
80.5 0.458220151268784
83.3 0.450675650073987
83.48 0.44209811146449
87.72 0.430758767765844
90.58 0.428376763392619
93.64 0.415991079612153
98 0.400960152331121
100.56 0.398808746949949
104.9 0.389418694511018
110.44 0.377771675476188
112.48 0.372161098435846
115.04 0.362366032590379
120.76 0.353559997112312
123.42 0.347327135917965
128.28 0.336111607231169
130.1 0.325415433937627
137.2 0.314582490019368
143.06 0.307972913936183
144.3 0.303194497671577
154.64 0.292881817567783
162.84 0.282378573812598
176.9 0.267562347841674
178.38 0.262442671875295
182.24 0.258514498321184
195.02 0.247153545528739
199.86 0.240868503037277
205.7 0.231189246262315
210.18 0.224184864660397
220.12 0.218920780619021
231.04 0.212855984641332
236.42 0.209372707570526
248.48 0.200239275797432
270.68 0.188996788124286
288.58 0.180815084245682
293.28 0.175228637661691
310.1 0.169809619047354
322.54 0.162981282925459
333.52 0.15720340136718
357.64 0.149704941795942
373.82 0.145414340162425
418.76 0.134778062850161
442.2 0.130016319904582
452.12 0.124641729649005
471.96 0.121348028919695
527 0.114836920438271
541.62 0.10929248159484
593.64 0.10215231400708
633.18 0.0988103156500331
677.56 0.0920845555586772
715.14 0.0869987759436776
757.32 0.0837532964333693
823.54 0.0798822619195245
916.86 0.0749503361528542
985.7 0.0698707005659376
1040.46 0.0660008146383564
1103.28 0.0643732613952269
1220.52 0.0597591687071404
1296.68 0.0577266756031318
1407.48 0.0550004599480541
1473.12 0.0520204129422505
1606.88 0.0493587202525797
1731.9 0.046863203717378
1870.26 0.0449742565986501
2027.5 0.0422304195377087
2173.94 0.039818231278175
2385.52 0.0376203007532197
2580.42 0.0359541407344651
2822.2 0.0339166921504596
3015.6 0.0315871998520886
3282.28 0.0299953869391551
3565.48 0.0282201078278197
3694.3 0.0274099849674566
3826.3 0.0263874199137818
4309.32 0.0249920994020705
4452.58 0.0240609761667179
4745.9 0.0227608938481156
5193.56 0.0215029263581305
5515.7 0.0206178478529835
5674.64 0.0199462419813897
6412.74 0.0188634899081182
6753.2 0.0179704687843063
7090.46 0.0173754391124696
7593.5 0.0166704787626988
7847.68 0.0158229511229201
8328.26 0.0151230806837575
8620.52 0.0145314223450918
9179.1 0.013848244764977
9914.3 0.0131003201677005
10560.44 0.0122962525056891
11461.86 0.0114373435661335
};
\addplot [draw=darkgray153, fill=darkgray153, forget plot, mark=*, mark size=1, only marks, draw opacity=0,
 fill opacity=0.5]
table{%
x  y
23.88 0.999999999932356
89.26 0.673919440125082
91.82 0.670146304050802
94.66 0.661109785159764
96.14 0.654203057702209
100.72 0.640329425751186
103.6 0.634767388422587
107.86 0.620383992280127
112.46 0.603254725369626
114.38 0.592805090182696
120.06 0.578919901618401
123.9 0.571290638965983
126.14 0.562303090732803
131.86 0.553135013610301
137.7 0.539355187187159
141.46 0.531423930687964
144.46 0.527935673247067
151.8 0.512524482735041
154 0.500033521277472
162.24 0.484504533845379
166.52 0.476137937939806
169.24 0.469700994944033
177.96 0.466710278818145
183.52 0.459939685958208
187.38 0.450561649112266
195.78 0.429637595802301
197.28 0.423781577017942
200.82 0.413650286069879
202.2 0.415191246251012
204.34 0.397367335158177
205.28 0.389609815912586
211.28 0.380321820110685
218.28 0.369031415347225
220.98 0.365273665361934
224.68 0.358040756142346
235.6 0.353674610831244
238.94 0.343915412024295
244.6 0.330639503132784
247.8 0.320297809355934
247.86 0.322943442630088
253.74 0.314156842891095
257.62 0.313973611344786
265.8 0.309585603237589
266.88 0.304350746858273
278.28 0.300479306408965
282.2 0.298297752889154
287.34 0.296555016614443
294.72 0.291914639067681
297.7 0.287406431758595
301.04 0.284621265191705
303.18 0.283007150613731
310.64 0.278801859836818
316.86 0.272738269501527
320.34 0.268477460057213
326.44 0.268252378813365
335.46 0.265882228273728
341.72 0.261160640799758
353.72 0.256824792871637
360.54 0.25133590439771
367.7 0.252020671041174
370.72 0.245394950535628
373.4 0.247278619078118
388.5 0.24042690352682
399.2 0.235288587327472
402.16 0.228861717806933
413.48 0.222069714939077
413.98 0.224481431496043
424.14 0.22024353156559
439.62 0.217231881949797
477.84 0.209515802953573
483.7 0.20327784852717
501.06 0.200582539635209
518.16 0.196453681853605
530.56 0.188715209721777
555.88 0.186392912608758
565.7 0.18132641739547
591.8 0.176322531596772
593.18 0.179135229954817
612 0.171376154395311
671.74 0.165168653575118
683.12 0.160724025359578
727 0.157426725474876
748.34 0.153591201896838
766.98 0.148697536502158
824.78 0.142279806796696
848.34 0.135649788421783
921.02 0.129393381350691
1053.46 0.123052378505931
1108.72 0.119311068244122
1219.66 0.111913946340447
1358.84 0.102255965156287
1596.92 0.09217698840241
1828.24 0.0815763894148244
2142.48 0.0711458182859118
2547.28 0.061696089958677
3166.32 0.0518774647542034
4185.08 0.0419060679751642
5918.84 0.0313467482941089
9460.12 0.0213872098694037
};
\addplot [
  draw=saddlebrown1356716,
  fill=saddlebrown1356716,
  forget plot,
  mark=*, mark size=1,
  only marks,
  draw opacity=0,
 fill opacity=0.5
]
table{%
x  y
363.84 0.205078607868437
399.38 0.175035509239552
402.9 0.173777077726886
406.92 0.17133857695525
412.34 0.16850881006454
422.04 0.166445467761985
422.54 0.165661007059518
429.64 0.163655497512343
434.58 0.162937703601283
445.48 0.15866398824917
453.08 0.157266770981932
460.9 0.156748023351489
474.72 0.151604335797452
483.7 0.144051715142428
484 0.147535614772079
497.5 0.141272006710443
504.7 0.139810684768669
520.86 0.136950289909771
537.82 0.13490526876602
553.66 0.132152557226614
563.66 0.126800980807656
586.54 0.121150701662675
603.3 0.118127006339945
628.3 0.115115915836676
641.24 0.114161333279785
667.46 0.111802490808047
695.26 0.108810937745185
706.32 0.105829138019718
731.52 0.101339633235354
764.02 0.099057176253021
779.2 0.0966918856156601
814.84 0.0946062168838224
833.48 0.093038491930836
857.8 0.0908276825562103
884.82 0.0882016589920194
913.86 0.0870724134449087
935.56 0.0847320525818932
948.68 0.082757547903139
965.96 0.0814665705353899
1007.24 0.0789834324934295
1069.5 0.0772120557892426
1075.5 0.0760404834542455
1107.92 0.0744359497532119
1143.7 0.0732219169598871
1185.7 0.0717303998918536
1218.8 0.0706724608286364
1241.9 0.0695270321106836
1293.92 0.0680899138026271
1317.48 0.0668439793708195
1358.84 0.0650855220932997
1413.44 0.0637476369448182
1475.76 0.0616140433977715
1533.86 0.0599105228541518
1590.08 0.0583740435800327
1675.08 0.0570376852198827
1712.6 0.0559092504490144
1743.44 0.0546742169347516
1818.62 0.0535884740208835
1886.2 0.0527313557062522
1950.28 0.051668050072977
2011.26 0.0504196702310596
2084.82 0.0494099061268732
2135.68 0.0484119077574593
2238.26 0.04738269055526
2287.24 0.0467461975338281
2358.22 0.0454915298135641
2475.74 0.0442693300092225
2562.84 0.0432842457703322
2749.56 0.0421480253339841
2846.26 0.0412801125224304
2994.6 0.0402515031944716
3062.04 0.039262254392545
3123.44 0.0382292345149242
3238.34 0.0372831790393866
3419.16 0.0362585187015204
3536.38 0.0357019313421746
3680.56 0.0346539766951266
3825.88 0.0338780268422605
3967.04 0.0331532474021288
4000.3 0.0326286665065875
4203.2 0.0318520170392422
4435.84 0.0310182163351307
4569.82 0.0302606109922938
4730.36 0.0296188099221471
4829.42 0.028958655591898
5033.48 0.0282207828364926
5285.1 0.027547014241235
5405.04 0.0268257998641409
5590.36 0.0259685027890771
5753.38 0.0251613212420855
6068.28 0.0243601094101947
6287 0.0237381601263643
6518.28 0.023090826595116
6939.46 0.0224164526946954
7135.8 0.0218411594889094
7397.82 0.0212860451144397
7476.64 0.0207640214107431
7803.18 0.0200908909169227
8069.98 0.0194770571542524
8357.72 0.0189320402662473
};
\addplot [very thick, royalblue28108204]
table {%
270.98 0.325049977402079
371.088282828283 0.24582469007255
471.196565656566 0.197603807427364
571.304848484849 0.16505481370187
671.413131313131 0.141567024759603
771.521414141414 0.123804592588687
871.629696969697 0.109896289688506
971.73797979798 0.0987089514573181
1071.84626262626 0.0895152769790348
1171.95454545455 0.0818265996219027
1272.06282828283 0.0753022088732241
1372.17111111111 0.0696971768286226
1472.27939393939 0.0648308466219454
1572.38767676768 0.0605670138405296
1672.49595959596 0.0568010267400102
1772.60424242424 0.0534511385470323
1872.71252525253 0.0504525597797475
1972.82080808081 0.0477532745678642
2072.92909090909 0.0453110386755503
2173.03737373737 0.0430911869256714
2273.14565656566 0.041065006125685
2373.25393939394 0.0392085101968252
2473.36222222222 0.0375015060093702
2573.47050505051 0.0359268724330504
2673.57878787879 0.0344699978699039
2773.68707070707 0.0331183370369858
2873.79535353535 0.0318610584938329
2973.90363636364 0.0306887619442125
3074.01191919192 0.029593249706136
3174.1202020202 0.0285673406117468
3274.22848484849 0.0276047174198456
3374.33676767677 0.0266998009040704
3474.44505050505 0.0258476453292759
3574.55333333333 0.0250438511938216
3674.66161616162 0.0242844919994188
3774.7698989899 0.0235660524863816
3874.87818181818 0.0228853762934679
3974.98646464647 0.0222396214064188
4075.09474747475 0.0216262220760073
4175.20303030303 0.0210428561357486
4275.31131313131 0.020487416846954
4375.4195959596 0.019957988556236
4475.52787878788 0.0194528255767299
4575.63616161616 0.0189703338059508
4675.74444444444 0.0185090546755254
4775.85272727273 0.0180676510950308
4875.96101010101 0.0176448951069428
4976.06929292929 0.0172396570146725
5076.17757575758 0.016850895782765
5176.28585858586 0.0164776505390442
5276.39414141414 0.0161190330340224
5376.50242424242 0.015774220934195
5476.61070707071 0.015442451843677
5576.71898989899 0.0151230179636312
5676.82727272727 0.014815261311569
5776.93555555556 0.0145185694332949
5877.04383838384 0.0142323715493322
5977.15212121212 0.0139561350853764
6077.2604040404 0.0136893625429117
6177.36868686869 0.0134315886717516
6277.47696969697 0.0131823779110983
6377.58525252525 0.0129413220698729
6477.69353535354 0.0127080382206475
6577.80181818182 0.0124821667846107
6677.9101010101 0.0122633697876791
6778.01838383838 0.0120513292701978
6878.12666666667 0.0118457458346987
6978.23494949495 0.0116463373179556
7078.34323232323 0.0114528375751157
7178.45151515152 0.0112649953650449
7278.5597979798 0.0110825733272046
7378.66808080808 0.0109053470414257
7478.77636363637 0.0107331041628599
7578.88464646465 0.0105656436251997
7678.99292929293 0.0104027749059752
7779.10121212121 0.010244317348365
7879.20949494949 0.0100900995345248
7979.31777777778 0.00993995870593286
8079.42606060606 0.009793740226695
8179.53434343434 0.00965129708614663
8279.64262626263 0.0095124894374428
8379.75090909091 0.0093771841691395
8479.85919191919 0.00924525450705271
8579.96747474747 0.00911657964393212
8680.07575757576 0.00899104439471368
8780.18404040404 0.00886853887531714
8880.29232323232 0.00874895820313763
8980.40060606061 0.00863220221754444
9080.50888888889 0.00851817521884833
9180.61717171717 0.00840678572433215
9280.72545454545 0.00829794624006029
9380.83373737374 0.00819157304729179
9480.94202020202 0.00808758600242074
9581.0503030303 0.00798590834945682
9681.15858585859 0.00788646654414097
9781.26686868687 0.00778919008886412
9881.37515151515 0.00769401137762476
9981.48343434343 0.00760086555032168
10081.5917171717 0.00750969035573455
10181.7 0.00742042602259513
};
\addplot [very thick, cadetblue80178158]
table {%
210.16 0.381826223973958
243.473939393939 0.36941611164339
276.787878787879 0.356300275546926
310.101818181818 0.343097414116343
343.415757575758 0.330144304574934
376.729696969697 0.317621327349656
410.043636363636 0.3056194773095
443.357575757576 0.294177709895105
476.671515151515 0.283304464155751
509.985454545455 0.272990391068336
543.299393939394 0.263216026022702
576.613333333333 0.253956473306233
609.927272727273 0.245184284322492
643.241212121212 0.236871223913598
676.555151515151 0.228989342535849
709.869090909091 0.22151161070058
743.18303030303 0.214412275739407
776.49696969697 0.207667042211139
809.810909090909 0.201253140806823
843.124848484848 0.19514932762307
876.438787878788 0.18933584098692
909.752727272727 0.183794333524207
943.066666666667 0.178507790971774
976.380606060606 0.173460445164773
1009.69454545455 0.168637685941592
1043.00848484848 0.16402597492685
1076.32242424242 0.159612762970943
1109.63636363636 0.155386412242762
1142.9503030303 0.15133612345824
1176.26424242424 0.147451868393684
1209.57818181818 0.143724327620346
1242.89212121212 0.1401448332659
1276.20606060606 0.136705316532472
1309.52 0.133398259661283
1342.83393939394 0.130216652018521
1376.14787878788 0.127153949977123
1409.46181818182 0.124204040278994
1442.77575757576 0.121361206577946
1476.0896969697 0.118620098882551
1509.40363636364 0.115975705638517
1542.71757575758 0.113423328210871
1576.03151515152 0.110958557546474
1609.34545454545 0.108577252816736
1642.65939393939 0.106275521858566
1675.97333333333 0.104049703248479
1709.28727272727 0.101896349860314
1742.60121212121 0.0998122137712751
1775.91515151515 0.0977942323939193
1809.22909090909 0.095839515723518
1842.54303030303 0.093945334600824
1875.85696969697 0.0921091098999154
1909.17090909091 0.0903284025594388
1942.48484848485 0.088600904383398
1975.79878787879 0.0869244295446682
2009.11272727273 0.0852969067307409
2042.42666666667 0.0837163718769184
2075.74060606061 0.0821809614372906
2109.05454545455 0.0806889061484602
2142.36848484848 0.0792385252451294
2175.68242424242 0.0778282210904136
2208.99636363636 0.0764564741871234
2242.3103030303 0.0751218385392989
2275.62424242424 0.0738229373360274
2308.93818181818 0.0725584589320632
2342.25212121212 0.0713271531019978
2375.56606060606 0.0701278275467682
2408.88 0.0689593446331135
2442.19393939394 0.0678206183482621
2475.50787878788 0.0667106114536256
2508.82181818182 0.0656283328226512
2542.13575757576 0.0645728349492139
2575.4496969697 0.0635432116140652
2608.76363636364 0.0625385956978687
2642.07757575758 0.0615581571302926
2675.39151515151 0.0606011009654718
2708.70545454545 0.0596666655749274
2742.01939393939 0.0587541209497354
2775.33333333333 0.0578627671043817
2808.64727272727 0.0569919325753237
2841.96121212121 0.0561409730078244
2875.27515151515 0.0553092698251054
2908.58909090909 0.0544962289743269
2941.90303030303 0.0537012797443065
2975.21696969697 0.0529238736502726
3008.53090909091 0.0521634833812905
3041.84484848485 0.0514196018063243
3075.15878787879 0.0506917410351838
3108.47272727273 0.0499794315308806
3141.78666666667 0.0492822212701625
3175.10060606061 0.0485996749492259
3208.41454545455 0.0479313732318131
3241.72848484848 0.0472769120371003
3275.04242424242 0.0466359018649567
3308.35636363636 0.0460079671563237
3341.6703030303 0.0453927456866146
3374.98424242424 0.0447898879901769
3408.29818181818 0.0441990568139892
3441.61212121212 0.043619926598891
3474.92606060606 0.0430521829867443
3508.24 0.0424955223520444
};
\addplot [very thick, chocolate21910927]
table {%
21.74 1.05108699683304
123.385050505051 0.446377698094598
225.030101010101 0.322182485372171
326.675151515152 0.261184691439491
428.320202020202 0.223408068201008
529.965252525252 0.197162152701875
631.610303030303 0.177613870041479
733.255353535354 0.162355820820794
834.900404040404 0.150037318276536
936.545454545455 0.139834734289043
1038.1905050505 0.131213810721222
1139.83555555556 0.123811024074162
1241.48060606061 0.117369409383245
1343.12565656566 0.111701577204496
1444.77070707071 0.106667283219968
1546.41575757576 0.102159236988844
1648.06080808081 0.0980937986536587
1749.70585858586 0.0944046922465218
1851.35090909091 0.0910386447083642
1952.99595959596 0.0879522907791123
2054.64101010101 0.0851099316266088
2156.28606060606 0.0824818824477863
2257.93111111111 0.0800432346554806
2359.57616161616 0.0777729152116474
2461.22121212121 0.0756529624256405
2562.86626262626 0.0736679617824577
2664.51131313131 0.0718046016757734
2766.15636363636 0.0700513200890575
2867.80141414141 0.0683980210412498
2969.44646464646 0.0668358451047339
3071.09151515152 0.0653569822361673
3172.73656565657 0.0639545180132532
3274.38161616162 0.0626223064639137
3376.02666666667 0.0613548642274084
3477.67171717172 0.060147281950914
3579.31676767677 0.0589951497057371
3680.96181818182 0.0578944938795587
3782.60686868687 0.0568417235185175
3884.25191919192 0.0558335844943113
3985.89696969697 0.0548671201851456
4087.54202020202 0.0539396376061745
4189.18707070707 0.0530486781205664
4290.83212121212 0.0521919920181394
4392.47717171717 0.051367516373415
4494.12222222222 0.0505733556956438
4595.76727272727 0.0498077649649685
4697.41232323232 0.0490691347153718
4799.05737373737 0.0483559778794689
4900.70242424242 0.0476669181549491
5002.34747474747 0.047000679689421
5103.99252525253 0.0463560779110625
5205.63757575758 0.045732011357992
5307.28262626263 0.0451274543806074
5408.92767676768 0.044541450609034
5510.57272727273 0.0439731070928864
5612.21777777778 0.043421589033276
5713.86282828283 0.0428861150377841
5815.50787878788 0.042365952838287
5917.15292929293 0.0418604154193455
6018.79797979798 0.0413688575115537
6120.44303030303 0.040890672409981
6222.08808080808 0.0404252890827752
6323.73313131313 0.0399721695392447
6425.37818181818 0.0395308064304162
6527.02323232323 0.0391007208582513
6628.66828282828 0.0386814603724675
6730.31333333333 0.0382725971363244
6831.95838383838 0.0378737262448306
6933.60343434343 0.0374844641806694
7035.24848484848 0.0371044473947482
7136.89353535354 0.0367333309996891
7238.53858585859 0.0363707875658247
7340.18363636364 0.036016506010354
7441.82868686869 0.035670190571284
7543.47373737374 0.0353315598586349
7645.11878787879 0.0350003459761485
7746.76383838384 0.0346762937074065
7848.40888888889 0.0343591597608694
7950.05393939394 0.0340487120688737
8051.69898989899 0.0337447291361032
8153.34404040404 0.0334469994334722
8254.98909090909 0.0331553208337389
8356.63414141414 0.0328695000855049
8458.27919191919 0.0325893523225644
8559.92424242424 0.0323147006058362
8661.56929292929 0.0320453754953622
8763.21434343434 0.0317812146500724
8864.85939393939 0.0315220624532222
8966.50444444444 0.0312677696615809
9068.1494949495 0.0310181930766219
9169.79454545455 0.030773195236103
9271.43959595959 0.030532644124568
9373.08464646465 0.0302964129014145
9474.7296969697 0.0300643796452874
9576.37474747475 0.0298364271136566
9678.0197979798 0.0296124425165258
9779.66484848485 0.0293923173033073
9881.3098989899 0.0291759469619676
9982.95494949495 0.0289632308296213
10084.6 0.0287540719138133
};
\addplot [very thick, purple11522131]
table {%
333.1 0.19112931307855
422.404444444444 0.168349491281721
511.708888888889 0.151555660634837
601.013333333333 0.138519536234909
690.317777777778 0.128026390872489
779.622222222222 0.119349207498934
868.926666666667 0.112022361837059
958.231111111111 0.105731860659457
1047.53555555556 0.100257181964824
1136.84 0.0954382719415691
1226.14444444444 0.0911557629842289
1315.44888888889 0.0873185724152916
1404.75333333333 0.0838558314267149
1494.05777777778 0.0807114626362394
1583.36222222222 0.0778404362040438
1672.66666666667 0.0752061227911937
1761.97111111111 0.0727783826157548
1851.27555555556 0.0705321602397061
1940.58 0.0684464341232386
2029.88444444444 0.0665034197171401
2119.18888888889 0.0646879568025054
2208.49333333333 0.0629870327619148
2297.79777777778 0.061389407522033
2387.10222222222 0.0598853155008073
2476.40666666667 0.0584662265500767
2565.71111111111 0.0571246525758159
2655.01555555556 0.0558539898708354
2744.32 0.0546483896217486
2833.62444444444 0.0535026508301163
2922.92888888889 0.0524121312048835
3012.23333333333 0.0513726725691421
3101.53777777778 0.0503805380693328
3190.84222222222 0.0494323590431685
3280.14666666667 0.0485250898394971
3369.45111111111 0.0476559692220001
3458.75555555556 0.046822487253109
3548.06 0.0460223567625269
3637.36444444444 0.0452534886694072
3726.66888888889 0.044513970558428
3815.97333333333 0.0438020480151272
3905.27777777778 0.0431161083105945
3994.58222222222 0.0424546660942656
4083.88666666667 0.0418163508094717
4173.19111111111 0.0411998955921518
4262.49555555556 0.0406041274507527
4351.8 0.0400279585563986
4441.10444444445 0.0394703784981788
4530.40888888889 0.0389304473798441
4619.71333333333 0.0384072896521318
4709.01777777778 0.0379000885899809
4798.32222222222 0.037408081336559
4887.62666666667 0.0369305544467223
4976.93111111111 0.0364668398715964
5066.23555555556 0.0360163113336754
5155.54 0.0355783810484119
5244.84444444444 0.0351524967538939
5334.14888888889 0.034738139015029
5423.45333333333 0.0343348187728052
5512.75777777778 0.0339420751127747
5602.06222222222 0.0335594732300009
5691.36666666667 0.0331866025703883
5780.67111111111 0.032823075130646
5869.97555555556 0.0324685239011582
5959.28 0.0321226014378099
6048.58444444444 0.0317849785503588
6137.88888888889 0.0314553430963014
6227.19333333333 0.0311333988703721
6316.49777777778 0.0308188645808608
6405.80222222222 0.0305114729048575
6495.10666666667 0.0302109696153475
6584.41111111111 0.0299171127738025
6673.71555555556 0.0296296719825504
6763.02 0.0293484276917761
6852.32444444444 0.0290731705565068
6941.62888888889 0.028803700839388
7030.93333333333 0.028539827855454
7120.23777777778 0.0282813694554556
7209.54222222222 0.0280281515446285
7298.84666666667 0.0277800076340714
7388.15111111111 0.0275367784221608
7477.45555555556 0.0272983114036604
7566.76 0.0270644605043912
7656.06444444444 0.0268350857395147
7745.36888888889 0.0266100528936517
7834.67333333333 0.026389233221211
7923.97777777778 0.026172503165439
8013.28222222222 0.0259597440948299
8102.58666666667 0.0257508420556429
8191.89111111111 0.0255456875393819
8281.19555555556 0.0253441752641819
8370.5 0.0251462039691324
8459.80444444444 0.0249516762206459
8549.10888888889 0.0247604982300481
8638.41333333333 0.0245725796816328
8727.71777777778 0.024387833570479
8817.02222222222 0.0242061760493867
8906.32666666667 0.0240275262843311
8995.63111111111 0.023851806317883
9084.93555555556 0.0236789409400838
9174.24 0.0235088575662989
};
\addplot [very thick, black18]
table {%
23.88 1.15314720107243
139.415151515152 0.307289410049633
254.950303030303 0.19600610102307
370.485454545455 0.148478979561632
486.020606060606 0.121400965775916
601.555757575758 0.103658600940886
717.090909090909 0.0910203821401157
832.626060606061 0.0815016618638986
948.161212121212 0.0740403488838084
1063.69636363636 0.0680134214787664
1179.23151515152 0.0630297627945993
1294.76666666667 0.0588306564141321
1410.30181818182 0.0552376951121767
1525.83696969697 0.0521236067959182
1641.37212121212 0.0493950012020487
1756.90727272727 0.0469816977676832
1872.44242424242 0.0448298705980253
1987.97757575758 0.0428975014306666
2103.51272727273 0.0411512786933121
2219.04787878788 0.0395644309780596
2334.58303030303 0.0381151807972823
2450.11818181818 0.0367856200007073
2565.65333333333 0.0355608779575356
2681.18848484849 0.0344284968921959
2796.72363636364 0.0333779563160476
2912.25878787879 0.0324003064370121
3027.79393939394 0.0314878823495727
3143.32909090909 0.0306340788763035
3258.86424242424 0.0298331714865991
3374.39939393939 0.0290801726015838
3489.93454545455 0.0283707153479909
3605.4696969697 0.0277009588024307
3721.00484848485 0.027067510206513
3836.54 0.026467360691759
3952.07515151515 0.0258978318400187
4067.6103030303 0.0253565309956824
4183.14545454546 0.0248413136933727
4298.68060606061 0.0243502519066519
4414.21575757576 0.0238816070866031
4529.75090909091 0.0234338071635345
4645.28606060606 0.0230054268448346
4760.82121212121 0.02259517066777
4876.35636363636 0.0222018583656392
4991.89151515152 0.0218244121850909
5107.42666666667 0.021461845856058
5222.96181818182 0.0211132549670529
5338.49696969697 0.0207778085401291
5454.03212121212 0.0204547416336541
5569.56727272727 0.0201433488287197
5685.10242424242 0.019842978477768
5800.63757575758 0.0195530276127907
5916.17272727273 0.0192729374260176
6031.70787878788 0.0190021892489645
6147.24303030303 0.0187403009665241
6262.77818181818 0.0184868238118499
6378.31333333333 0.0182413394954138
6493.84848484849 0.0180034576280514
6609.38363636364 0.0177728134032657
6724.91878787879 0.0175490655086865
6840.45393939394 0.0173318942405314
6955.98909090909 0.0171209997982841
7071.52424242424 0.0169161007396943
7187.05939393939 0.0167169325786847
7302.59454545455 0.0165232465108909
7418.1296969697 0.0163348082534018
7533.66484848485 0.0161513969868706
7649.2 0.0159728043895486
7764.73515151515 0.0157988337540038
7880.2703030303 0.0156292991783339
7995.80545454546 0.015464024824604
8111.34060606061 0.0153028442380402
8226.87575757576 0.0151455997212165
8342.41090909091 0.0149921417580915
8457.94606060606 0.014842328483294
8573.48121212121 0.0146960251925425
8689.01636363636 0.0145531038905008
8804.55151515152 0.0144134428727558
8920.08666666667 0.0142769263389311
9035.62181818182 0.0141434440342472
9151.15696969697 0.0140128909171056
9266.69212121212 0.0138851668505036
9382.22727272727 0.0137601763152986
9497.76242424242 0.0136378281435294
9613.29757575758 0.0135180352701632
9728.83272727273 0.0134007145017948
9844.36787878788 0.0132857863009517
9959.90303030303 0.0131731745847851
10075.4381818182 0.0130628065370313
10190.9733333333 0.0129546124322293
10306.5084848485 0.0128485254712659
10422.0436363636 0.0127444816274016
10537.5787878788 0.0126424195020007
10653.1139393939 0.0125422801892558
10768.6490909091 0.0124440071492547
10884.1842424242 0.0123475460887925
10999.7193939394 0.0122528448493798
11115.2545454545 0.0121598533019412
11230.7896969697 0.0120685232477405
11346.3248484848 0.0119788083251047
11461.86 0.0118906639215512
};
\addplot [very thick, darkgray153]
table {%
23.88 1.46541093228161
119.195555555556 0.550538885501558
214.511111111111 0.373246282641894
309.826666666667 0.290225828323933
405.142222222222 0.240576201328791
500.457777777778 0.20702107103274
595.773333333333 0.182593989143653
691.088888888889 0.163896898232998
786.404444444445 0.149057470450668
881.72 0.136952018240408
977.035555555556 0.12686193910967
1072.35111111111 0.118304525219694
1167.66666666667 0.110942547050817
1262.98222222222 0.104532726657578
1358.29777777778 0.0988948063663511
1453.61333333333 0.0938921652960099
1548.92888888889 0.0894192250878393
1644.24444444444 0.0853930102659423
1739.56 0.0817473397568796
1834.87555555556 0.078428735048252
1930.19111111111 0.075393477878083
2025.50666666667 0.0726054556063073
2120.82222222222 0.0700345574831346
2216.13777777778 0.0676554633389884
2311.45333333333 0.065446716466429
2406.76888888889 0.0633900054184308
2502.08444444445 0.061469601493425
2597.4 0.0596719136944672
2692.71555555556 0.0579851333485961
2788.03111111111 0.0563989478826336
2883.34666666667 0.0549043084624778
2978.66222222222 0.0534932399651897
3073.97777777778 0.0521586845019794
3169.29333333333 0.0508943717408237
3264.60888888889 0.0496947107930163
3359.92444444445 0.0485546995700039
3455.24 0.0474698483852111
3550.55555555556 0.0464361152413785
3645.87111111111 0.0454498507585247
3741.18666666667 0.0445077510983223
3836.50222222222 0.0436068175548584
3931.81777777778 0.0427443217297527
4027.13333333333 0.0419177754066044
4122.44888888889 0.0411249043971506
4217.76444444445 0.0403636257580228
4313.08 0.0396320278791919
4408.39555555556 0.0389283530281894
4503.71111111111 0.0382509820019281
4599.02666666667 0.0375984205934716
4694.34222222222 0.0369692876268341
4789.65777777778 0.0363623043507098
4884.97333333333 0.0357762850134326
4980.28888888889 0.0352101284676501
5075.60444444445 0.0346628106750941
5170.92 0.0341333780002269
5266.23555555556 0.0336209411970414
5361.55111111111 0.0331246700063948
5456.86666666667 0.0326437882923668
5552.18222222222 0.0321775696555908
5647.49777777778 0.0317253334695678
5742.81333333333 0.0312864412928763
5838.12888888889 0.030860293616114
5933.44444444445 0.0304463269074972
6028.76 0.030044010925442
6124.07555555556 0.029652846270245
6219.39111111111 0.0292723621502771
6314.70666666667 0.0289021143409617
6410.02222222222 0.0285416833172977
6505.33777777778 0.0281906725428619
6600.65333333333 0.0278487069001231
6695.96888888889 0.0275154312485645
6791.28444444445 0.0271905090985729
6886.6 0.0268736213903349
6981.91555555556 0.0265644653681175
7077.23111111111 0.0262627535413034
7172.54666666667 0.0259682127244426
7267.86222222222 0.0256805831493566
7363.17777777778 0.0253996176430339
7458.49333333333 0.0251250808656665
7553.80888888889 0.0248567486037318
7649.12444444445 0.0245944071135103
7744.44 0.0243378525108687
7839.75555555556 0.0240868902035298
7935.07111111111 0.0238413343623984
8030.38666666667 0.0236010074288295
8125.70222222222 0.0233657396550038
8221.01777777778 0.023135368674832
8316.33333333333 0.022909739103035
8411.64888888889 0.0226887021602537
8506.96444444445 0.0224721153222289
8602.28 0.0222598419912575
8697.59555555556 0.0220517511882832
8792.91111111111 0.0218477172641184
8888.22666666667 0.021647619628418
8983.54222222222 0.0214513424951371
9078.85777777778 0.0212587746433101
9174.17333333333 0.0210698091920801
9269.48888888889 0.0208843433889926
9364.80444444445 0.020702278410646
9460.12 0.0205235191748613
};
\addplot [very thick, saddlebrown1356716]
table {%
363.84 0.184417090227137
444.586262626263 0.15629070692929
525.332525252525 0.136524794224368
606.078787878788 0.121817961596472
686.825050505051 0.110413792622276
767.571313131313 0.101289631460834
848.317575757576 0.0938085544255805
929.063838383838 0.0875525686882791
1009.8101010101 0.0822356329655554
1090.55636363636 0.077655179082609
1171.30262626263 0.0736635931047318
1252.04888888889 0.0701506707966062
1332.79515151515 0.0670324098050176
1413.54141414141 0.0642436154806129
1494.28767676768 0.0617328848722944
1575.03393939394 0.0594591201679149
1655.7802020202 0.0573890526789706
1736.52646464646 0.0554954506461273
1817.27272727273 0.053755799715326
1898.01898989899 0.0521513164151243
1978.76525252525 0.0506662002991809
2059.51151515152 0.0492870598242067
2140.25777777778 0.0480024665021471
2221.00404040404 0.0468026049957608
2301.7503030303 0.045678995833814
2382.49656565657 0.0446242736974178
2463.24282828283 0.0436320086640524
2543.98909090909 0.0426965609719005
2624.73535353535 0.0418129621695903
2705.48161616162 0.0409768172047072
2786.22787878788 0.0401842232554766
2866.97414141414 0.0394317020462995
2947.7204040404 0.0387161430950334
3028.46666666667 0.0380347558787545
3109.21292929293 0.037385029318666
3189.95919191919 0.0367646973052242
3270.70545454545 0.0361717092343946
3351.45171717172 0.0356042047220763
3432.19797979798 0.0350604918187251
3512.94424242424 0.0345390281694141
3593.6905050505 0.0340384046631099
3674.43676767677 0.033557331194175
3755.18303030303 0.0330946242231609
3835.92929292929 0.032649195875992
3916.67555555556 0.0322200443631233
3997.42181818182 0.0318062455350958
4078.16808080808 0.0314069454196056
4158.91434343434 0.031021353608942
4239.66060606061 0.03064873738636
4320.40686868687 0.0302884164963859
4401.15313131313 0.0299397584778043
4481.89939393939 0.029602174489621
4562.64565656566 0.0292751155700238
4643.39191919192 0.0289580692765883
4724.13818181818 0.0286505566629471
4804.88444444444 0.0283521295530734
4885.63070707071 0.0280623680793917
4966.37696969697 0.0277808784552517
5047.12323232323 0.0275072909560215
5127.86949494949 0.0272412580862444
5208.61575757576 0.0269824529130588
5289.36202020202 0.0267305675484629
5370.10828282828 0.0264853117650641
5450.85454545455 0.0262464117317486
5531.60080808081 0.0260136088572609
5612.34707070707 0.0257866587310466
5693.09333333333 0.0255653301518969
5773.8395959596 0.025349404235977
5854.58585858586 0.0251386735967311
5935.33212121212 0.0249329415899625
6016.07838383838 0.024732021618094
6096.82464646465 0.0245357364882363
6177.57090909091 0.0243439178192468
6258.31717171717 0.0241564054934489
6339.06343434343 0.0239730471491145
6419.8096969697 0.0237936977101984
6500.55595959596 0.0236182189501574
6581.30222222222 0.0234464790869891
6662.04848484848 0.023278352406901
6742.79474747475 0.0231137189142636
6823.54101010101 0.0229524640057179
6904.28727272727 0.0227944781665041
6985.03353535353 0.0226396566872551
7065.7797979798 0.0224878993996541
7146.52606060606 0.0223391104294976
7227.27232323232 0.0221931979658356
7308.01858585859 0.0220500740449721
7388.76484848485 0.0219096543482174
7469.51111111111 0.0217718580123738
7550.25737373737 0.0216366074520258
7631.00363636364 0.0215038281927792
7711.7498989899 0.0213734487146668
7792.49616161616 0.021245400305
7873.24242424242 0.0211196169200048
7953.98868686869 0.0209960350546323
8034.73494949495 0.020874593619984
8115.48121212121 0.0207552338278314
8196.22747474747 0.0206378990817562
8276.97373737374 0.0205225348744671
8357.72 0.0204090886908869
};
\addplot [draw=black, fill=black, mark=x, very thick, mark size=2.5pt, only marks]
table{%
x  y
90.08 0.463967623588202
363.84 0.205078607868424
1452.8 0.0862508073444684
5754.88 0.0332949259765356
};
