# Supplementary material for: Swarm Reinforcement Learning For Adaptive Mesh Refinement
Source: arXiv:2304.00818 source file (2023-10-09)
Supplement: Supplementary file 11 [file group_additional_metrics_l5.tex]

\nextgroupplot[
ylabel shift = -0.2cm,
title style={yshift=-0.2cm},
height=4.5cm,
width=0.50\textwidth,
ylabel={Mean Error},
title={Heat Diffusion},
scaled x ticks=false,
clip marker paths=true,
legend cell align={left},
legend style={fill opacity=0.8, draw opacity=1, text opacity=1, draw=lightgray204},
log basis y={10},
tick align=outside,
tick pos=left,
x grid style={darkgray176},
xlabel={Elements \(\displaystyle (\times 10^3)\)},
xmajorgrids,
xmin=-326.981, xmax=7238.401,
xtick style={color=black},
xtick={-1000,0,1000,2000,3000,4000,5000,6000,7000,8000},
xticklabels={-1.0,0.0,1.0,2.0,3.0,4.0,5.0,6.0,7.0,8.0},
y grid style={darkgray176},
ymajorgrids,
ymin=0.00202351979418075, ymax=1.35840264521997,
ymode=log,
ytick style={color=black},
ytick={0.0001,0.001,0.01,0.1,1,10,100},
yticklabels={
  \(\displaystyle {10^{-4}}\),
  \(\displaystyle {10^{-3}}\),
  \(\displaystyle {10^{-2}}\),
  \(\displaystyle {10^{-1}}\),
  \(\displaystyle {10^{0}}\),
  \(\displaystyle {10^{1}}\),
  \(\displaystyle {10^{2}}\)
}
]
\addplot [
  draw=royalblue28108204,
  fill=royalblue28108204,
  forget plot,
  mark=*, mark size=1,
  only marks,
  draw opacity=0,
 fill opacity=0.5
]
table{%
x  y
134.88 0.229968188597145
136.92 0.247482366866981
140.68 0.230764052634291
144.68 0.218329661728041
148.58 0.228336958437283
151.16 0.240523574217139
160.7 0.218300680418605
161.58 0.205703991293262
166.68 0.192956734071841
186.8 0.220617294348231
211.54 0.151864421501522
211.56 0.138449094122903
235.68 0.141696698057511
236.12 0.139929091725578
249.78 0.139723378214435
252.72 0.136645750271135
255.58 0.130752196676432
261.98 0.172015950966048
263.58 0.123571576345143
268.44 0.140212570286989
274.56 0.104752849827404
279.72 0.14186958283084
281.38 0.128680720145284
290.34 0.10737380442499
293.24 0.125414790365955
306.62 0.0994924234737539
308.6 0.100393623726061
319.16 0.149155108264558
366.56 0.101935124984811
374.7 0.0921727833982031
378.94 0.063495268428199
403.42 0.111828787044388
411.48 0.0711753045914537
412.98 0.0825318050834778
414.08 0.123773065534188
415 0.0888800939334704
439 0.0687025115484986
455 0.0788936265240387
457.58 0.0686056780461258
481 0.090753643470921
507.76 0.0518917342226987
508.12 0.0607093694074221
518.28 0.0605340951770016
596.12 0.0612554952419007
631.2 0.059645616848858
684.24 0.0412430303897337
717.88 0.0383289725321252
749.4 0.0338514468019329
764.7 0.0495291783777241
800.08 0.0421889307311646
960.5 0.040211192001268
1017.62 0.0909675739085955
1169.94 0.0262040778777617
1308.38 0.0271389014074477
1422.2 0.0185813650708506
1483.84 0.0184299194700579
1514.78 0.0188206178256694
1557.08 0.0218302245925481
1561.08 0.0203842792009267
1585.78 0.0223523658857659
1626.3 0.0220448989226254
1629.44 0.019791570190636
1656.18 0.0206841821651404
1687.36 0.0179917082577097
1694.8 0.0152173761038888
1702.88 0.0163601321426527
1706 0.0174105013361674
1709.52 0.0199040846107135
1718.04 0.0165706094020128
1819.3 0.0142633749363136
1846.94 0.0168870906598096
1880.7 0.0184561313579887
1892.46 0.0185275160693602
1914.28 0.0146575244073988
1963.96 0.0136704173827464
1976.7 0.0126771266417378
2000.64 0.0143040418397014
2051.5 0.0155799160054725
2133.94 0.0157968684549234
2146.12 0.0196136166218795
2432.54 0.0127641141352575
2508.48 0.0131508221791704
2555.96 0.012486915346647
2604.64 0.0103454189426603
2630.82 0.0140617791948356
2750.6 0.0108442915420435
2766.8 0.00941491506949838
3062.26 0.00932064470598459
3203.74 0.00812278594090236
3540.68 0.00766112171503817
3542.88 0.00942626889642574
3699.44 0.0101636744624705
3780.26 0.00790843689291913
3910.68 0.00614163754183157
4150.42 0.00802959727519985
4165.94 0.00663495350730892
4722.46 0.00451662373928967
5140.76 0.00379636860399534
5754.9 0.00346190987666681
6212.24 0.00458426978556074
};
\addplot [
  draw=cadetblue80178158,
  fill=cadetblue80178158,
  forget plot,
  mark=*, mark size=1,
  only marks,
  draw opacity=0,
 fill opacity=0.5
]
table{%
x  y
241.02 0.128148240991119
242.42 0.113413087972827
246.08 0.104513196333517
280.66 0.136758015102382
283 0.110122873525341
285.6 0.157131021155156
292.08 0.132679634644969
295.56 0.126312355576448
403.64 0.241650068031214
428.2 0.137843373243482
464.24 0.0891061796143678
465.5 0.067104967895577
472.08 0.144271641464477
473.9 0.180391943200617
499.16 0.0745935413410905
521.66 0.120256548704903
538.92 0.20980249144724
552.68 0.0768675383568753
565.42 0.428630367941606
624.08 0.0648165604717722
626.94 0.806431989914857
647.16 0.341187855139783
673.66 0.0460754646737481
705.8 0.140078897666257
710.06 0.693904660129664
762.98 0.15309240711193
764.58 0.0783727645635267
772.88 0.0459523809009515
802.38 0.0880405393905423
828.36 0.0738131513398185
864.82 0.0671563784137888
882.14 0.128118204142887
903.56 0.440748487044327
939.3 0.629112103360385
941.96 0.0902001929707629
963.54 0.0840965736549744
965.02 0.267702929152013
975.9 0.0591030431820816
989.52 0.0709997990800259
997.02 0.23522013463426
1021.18 0.151691690336855
1134.24 0.109810674794594
1169.52 0.481312973642867
1238.14 0.0355533644918635
1269.8 0.799605846060443
1278.56 0.113984369556945
1340.92 0.84770628628293
1387.3 0.0667861498265316
1459.64 0.0941699703659385
1484.46 0.039113554147016
1490.98 0.0477782060367807
1500.8 0.271094727395275
1505.44 0.0907116268012138
1547.48 0.084986172713398
1651.48 0.210145592697733
1677.08 0.0262063541310689
1693.32 0.0358906077287285
1708.5 0.252291740918991
1731.68 0.0303101273276684
1774.74 0.199662273925217
1784.28 0.0272069847342685
1841.92 0.0900434685543469
1878.02 0.372222897353837
1973.82 0.0826478111845805
1993.98 0.466007925663124
2000 0.0148499497402732
2040.14 0.0311904862908043
2043.18 0.109727343299229
2058.24 0.0455626111281557
2093.26 0.0245865094612139
2180.78 0.0433310001844382
2229.96 0.1518519569068
2276.7 0.0443376189300637
2318.2 0.0593413221419744
2378.76 0.0488918368754557
2383.72 0.0656743362456901
2386.88 0.0486214711526844
2503.9 0.17008006079522
2516.66 0.0810101997764562
2554.2 0.014126000442229
2565 0.0259537986344119
2577.56 0.032707573403296
2622.78 0.0187555674507252
2641.06 0.0344780956956401
2679.5 0.721833661146086
2725.86 0.362009892406292
2781.9 0.0483921178835863
2813.24 0.0206608871558983
2832.16 0.0277444307626527
2837.8 0.0777656655995455
2936.54 0.250944765699977
2991.6 0.0927558760605114
3099.9 0.0710177166930924
3108.04 0.0535913160252595
3131.92 0.0221143914761767
3321.68 0.0212603642625764
3456.78 0.0350811251126185
3654.96 0.0127454699453917
3912.14 0.311700762000353
4212.62 0.0822795435248221
};
\addplot [
  draw=chocolate21910927,
  fill=chocolate21910927,
  forget plot,
  mark=*, mark size=1,
  only marks,
  draw opacity=0,
 fill opacity=0.5
]
table{%
x  y
16.9 0.999999999999784
16.9 0.999999999999787
16.92 0.999999999999781
16.96 0.999999999999784
17.04 0.999999999999785
17.04 0.999999999999785
17.04 0.999999999999785
17.04 0.999999999999785
17.04 0.999999999999785
17.04 0.999999999999785
17.04 0.999999999999785
17.04 0.999999999999785
17.04 0.999999999999785
17.04 0.999999999999785
17.04 0.999999999999785
17.04 0.999999999999785
17.08 0.999999999999727
17.12 0.999999999999776
17.28 0.999999999999726
17.36 0.999999999999758
21.96 0.889271206732765
25.1 0.926477888063115
96.34 0.243595469418368
127.92 0.319234383313305
134.24 0.464352039180842
136.58 0.215749118296018
140.86 0.223427329966401
148.98 0.185694544950981
202.7 0.112030224931173
215.06 0.108243030284617
219.04 0.554355853756161
220.34 0.122320442164047
244.04 0.116580587959138
250.14 0.113027499393677
250.72 0.122922144948342
262.18 0.100986444733323
271.06 0.113427966505389
271.5 0.0934116588020941
271.78 0.113488779706129
273.34 0.0942620790102527
303.22 0.0906361897223452
304.12 0.103783671147744
324.54 0.258393554377098
333.34 0.142962498731587
354.22 0.0723566294632999
360.26 0.0759761753928511
381.58 0.0825608044075494
409.2 0.106581002361721
436.04 0.0610029310516181
440.08 0.0704394814760409
537.46 0.0564801147246061
634.94 0.0384402832310594
671.66 0.0542658548782526
673.54 0.0438252415646254
1037.28 0.0601039305936212
1096.34 0.140596757840636
1205.54 0.0202083506471866
1431.94 0.0284268004763017
1502.14 0.0175914773083305
1532.86 0.0346118028575098
1648.54 0.646623606091061
1660.98 0.0378433820973277
1961.58 0.0380380054446884
1975.44 0.0228425048410865
2058.46 0.0264549641473372
2072.8 0.0348143604561529
2388.86 0.0247397044777072
2572.62 0.0234657750531741
2750.58 0.01601639102736
2890.28 0.0117042564463105
3055.76 0.0266376096356656
3264.02 0.0230211023740435
4095 0.00845854202660336
4299 0.00538538233250678
4337.48 0.0185336875406909
4429.88 0.00732164415556057
5311.04 0.0109780369646087
5687.56 0.00521293898722032
5939 0.0360005239331822
6427.48 0.00885619935846252
6477.06 0.00712451682506024
};
\addplot [draw=purple11522131, fill=purple11522131, forget plot, mark=*, mark size=1, only marks, draw opacity=0,
 fill opacity=0.5]
table{%
x  y
271.48 0.163370833559206
323.38 0.104966266875056
326.24 0.122578815880352
326.36 0.0930110009061243
343.56 0.0844518853391262
350 0.110496527236234
354.86 0.106775239092927
377.5 0.100941349861312
385.36 0.100486047508273
398.28 0.105590585696193
463.48 0.0811960312937949
480.48 0.0690385344627582
490.44 0.0704160134257457
552.56 0.0590024925891029
726.96 0.0818339469801299
740.86 0.0577646454723399
759.7 0.053728661404049
762.02 0.0590451328766667
805.5 0.0493584604772002
823.88 0.0480480463606977
870.76 0.0431938323553445
1014.18 0.044959391424089
1047.28 0.0440478402626565
1082.9 0.0434655894080289
1091.84 0.0436020304761975
1091.84 0.0436020304761975
1092.34 0.0435475495530989
1092.62 0.0432897017648935
1094.38 0.0433139003998465
1104.32 0.0434367654793026
1104.64 0.0434367654841564
1108.4 0.0429776109659873
1122.64 0.041889963263817
1127.46 0.04168911575981
1157.24 0.0386872703346303
1159.82 0.0430934508978524
1184.84 0.0425635049983894
1250.66 0.0415706786775793
1252.18 0.035095291660932
1264.66 0.0354497815033238
2094.7 0.0240785806070554
3057.84 0.013870513873668
3576.76 0.0126733530974142
3593.68 0.0141602248955579
3646.92 0.0121173421359783
3741.12 0.0118501519020265
4263.78 0.0135225019679018
4302.06 0.011232453589191
4348.72 0.0107013309049161
4379.54 0.0106876590322493
4382.68 0.0112321120625183
4382.72 0.0112321120624766
4419.88 0.0108078485310351
4444.78 0.010687238887644
4462.22 0.0107812671937807
4463.2 0.0106870375275198
4464.48 0.0108446532536478
4466.32 0.0106870250672756
4467.56 0.0106870257996064
4483.24 0.0106870281140026
4489.1 0.010687028098413
4491.54 0.0107054415882163
4506.58 0.0104123778660457
4515.84 0.0106870280954708
4515.84 0.0104123778656963
4515.84 0.0106870280954708
4515.84 0.0104123778656963
4515.84 0.0106870280954708
4515.84 0.0104123778656963
4515.84 0.0106870280954708
4515.84 0.0106870280954708
4515.84 0.0106870280954708
4515.84 0.0104123778656963
4515.84 0.0104123778656963
4515.84 0.0104123778656963
4515.84 0.0106870280954708
4515.84 0.0104123778656963
4515.84 0.0104123778656963
4515.84 0.0106870280954708
4515.84 0.0104123778656963
5611.56 0.00803855116345075
5824.58 0.00791298443084326
5905.82 0.00791258041715979
6048.94 0.00790904790078312
6085.04 0.00790906150503334
6087.68 0.00790904127258839
6087.68 0.00790904127258839
6087.68 0.00790904127258839
6087.68 0.00790904127258839
6087.68 0.00790904127258839
};
\addplot [draw=black18, fill=black18, forget plot, mark=*, mark size=1, only marks, draw opacity=0,
 fill opacity=0.5]
table{%
x  y
17.04 0.999999999999785
77.24 0.266068578731246
79.3 0.263402765895984
81.78 0.248092547979932
82.54 0.246708379046705
83.8 0.239163588972948
85.04 0.233327402416428
86.64 0.225776596044884
90.34 0.219343045937413
92.96 0.212676503372305
95.36 0.207587420984133
98.04 0.205213040732546
101.54 0.199538475867268
104.32 0.192630607277795
109.08 0.18324966626993
114.32 0.178725998237621
114.38 0.173189766423988
118.66 0.167231940386698
119.38 0.167158259245488
121.72 0.162062885609291
125.66 0.15986364659854
126.36 0.155779767975573
132.98 0.150143585875306
137 0.146255625688641
140.18 0.143671506362209
146.78 0.13694118142443
152 0.129877449263528
156.36 0.124779940803586
164.22 0.124341035016557
169.46 0.121900676931617
173.72 0.118862676890688
178.88 0.117335808286283
184.14 0.112984450321335
194.84 0.107658370490371
200.58 0.103769219436575
208.36 0.096172432401705
208.58 0.101761448190266
211.22 0.0931151603318588
217.6 0.0913695214093229
238.7 0.0877124512103094
255.24 0.0835386561120953
270.48 0.0791765427566728
271.78 0.0798824423620123
284.9 0.0773400433665993
294.62 0.0725956970977306
312.04 0.0712123622575832
328.88 0.0657650625511603
349.48 0.0618536360592338
376.42 0.0594377345367816
376.6 0.0595574177119559
397.08 0.054086153083988
398.62 0.0553606297481066
431.04 0.0503562425995996
435.12 0.051610566789835
446.98 0.0509497300595155
476.08 0.047759854672179
503.98 0.0441723590124513
531.64 0.0426203603174572
547.62 0.0384099590502216
548.66 0.0393882821081998
585.22 0.0369584403361492
619.14 0.0347657832825933
661 0.032131787281564
708.6 0.0298919011587729
759.88 0.0279264590725743
823.92 0.0269369016666711
859.32 0.0264450556881751
895.84 0.0232832469043444
959.38 0.0226484458858513
1088.28 0.0208310894644976
1163.28 0.0190991637128258
1220.84 0.0177682551895876
1227.44 0.0183226012209086
1290.82 0.0165969974850226
1415.38 0.015568054222409
1517.88 0.0139534249086142
1701.32 0.0131505025173152
1829.64 0.0126252553723732
1905.2 0.0116922567297305
2059.08 0.0105119556945572
2289 0.00968322257482939
2460.04 0.00873536569995299
2530.3 0.00852076725468386
2907.64 0.00742831393153313
3043.44 0.0067306775997403
3252.04 0.00656349906930804
3606 0.00591323003802982
3835.24 0.00547703931900739
4135.54 0.00477365128126506
4811.88 0.00412401463234102
5381.92 0.0036626235260746
5575.76 0.00347250945906039
6012.9 0.00313689292846319
6157.76 0.00272021899505656
};
\addplot [draw=darkgray153, fill=darkgray153, forget plot, mark=*, mark size=1, only marks, draw opacity=0,
 fill opacity=0.5]
table{%
x  y
17.04 0.999999999999785
124.36 0.246942147992851
131.24 0.242419142168385
137.02 0.236887645071227
143.78 0.234658584996877
146.2 0.23269532094878
151.74 0.219664945744679
155.86 0.213587495665484
163.64 0.208978231970141
166.16 0.206888820038483
175.24 0.199317456189227
179.82 0.197427305689721
186.34 0.181879019880912
187.14 0.19023706801612
188.5 0.187460588009462
195.52 0.17939944167316
204.1 0.170787569623813
212.08 0.168520516815102
219.82 0.162190004237973
224.74 0.157094815421346
228.76 0.154019149634303
233.78 0.151578500526628
249.18 0.145316824038347
250.02 0.148886350943762
262.94 0.139056618393962
270.38 0.132877054254361
279.66 0.132205842166383
286 0.132350587403759
290.02 0.13084907689075
300.48 0.127645360076798
309.02 0.126177215893716
317.78 0.122269733890316
342.62 0.120835706675875
357.14 0.118425876488182
373.68 0.116816121392983
378.7 0.110364453905073
381.1 0.113945523805027
396.86 0.106249662843278
431.52 0.102664011393611
431.98 0.0970278864603355
434.98 0.098102901534108
450.5 0.0945179505511729
463.3 0.0914392780105597
476.02 0.0894797685099414
511.34 0.0842347651380631
529.58 0.0818293742966073
532.58 0.0822002337585193
548.94 0.0792507758694347
558.32 0.0780914332119853
587.24 0.0753652836004985
591.06 0.0756509932882013
622.62 0.0719558605595588
639.04 0.0709138955959085
663.16 0.0672538564895584
707.54 0.0664901009391193
718.34 0.0637982350469954
762.64 0.0616480626529974
772.3 0.0613020482334426
806.28 0.0576881713158385
819.64 0.0559914922540502
855.74 0.0547755256311506
869.96 0.0502664339437056
903.04 0.0493343469987426
918.54 0.048147373433969
941.12 0.0462058885821962
999.58 0.0438960761306638
1008.32 0.0409286850413342
1054.24 0.0396998094943577
1089 0.0364688516038999
1094.58 0.0356268344634389
1166.82 0.0359073043073878
1221.04 0.0339675074657702
1269.78 0.0322036993982737
1326.02 0.0318382288748641
1374.1 0.0302680895026589
1435.74 0.0279657058840187
1451.06 0.0274575514807547
1499.88 0.0261837588511252
1510.66 0.0257980438864228
1589.5 0.0237886757626284
1615.32 0.0219416830056942
1825.06 0.0195613662924989
1829.46 0.0203416284052703
1964.48 0.0185004966529968
2075.06 0.0176898125339507
2168.46 0.016352737546978
2286.68 0.0149388710033452
2462.88 0.013710211382883
2629.48 0.0126010974996551
2848.06 0.0115704586186715
3084.22 0.0106791840920614
3275.22 0.00938659652365044
3617 0.00896468080187459
3782.56 0.00786855073804499
4342.1 0.00676238895587814
4959.16 0.00544743031171896
5826.28 0.00443325517895546
6894.52 0.00345510304358035
};
\addplot [
  draw=saddlebrown1356716,
  fill=saddlebrown1356716,
  forget plot,
  mark=*, mark size=1,
  only marks,
  draw opacity=0,
 fill opacity=0.5
]
table{%
x  y
274.56 0.160676273820693
329.78 0.0961034897867873
333.46 0.0950983292592743
336.7 0.0954596141375509
339.98 0.0939811119760826
349.52 0.092125053199785
357.28 0.0913618785951833
363.48 0.0906381540532084
369.5 0.0897753479365617
378.88 0.088085317056371
381.78 0.0877109416870239
391.34 0.0865859313712926
402.16 0.0858308465565879
409.54 0.0849170124032236
425.96 0.083357223940755
432.18 0.0833209332532042
443.84 0.0825328697882807
457.3 0.0814325736401324
464.5 0.0803148336310652
484.54 0.0801291021792992
496.2 0.0789501074019127
510.66 0.0783327460341655
530 0.0777118926251167
542.72 0.0772956431875477
555.42 0.0761337504554322
567.32 0.0757483453973276
577.74 0.0748593772068245
599.12 0.0732620804431402
622.84 0.0728919249654411
637.98 0.0699824001261837
645.72 0.069900842120727
656.58 0.0694714017705556
681.24 0.0688521751576069
700.04 0.0683040734705871
719.8 0.0674084223261883
733.36 0.066854686808223
756.86 0.0666830341463277
771.08 0.0663931059042844
788.88 0.0664547071467681
811.94 0.0656445751623344
834.48 0.0645315156034688
868.2 0.0642435221056465
887.54 0.0638176127017592
908.74 0.0633208652268299
938.88 0.0631277936468166
971.68 0.0626825852651677
998.62 0.0617596477373443
1017.52 0.0615400730089785
1044.62 0.0598517080637559
1075 0.0592044305048184
1099.88 0.0583958381415738
1115.38 0.057754626958315
1163.6 0.0563849231690622
1191.52 0.0558294049626599
1214.18 0.0550682478705333
1250.44 0.0543684315063204
1273.8 0.0542769891914193
1320.02 0.0529524042222122
1348.86 0.0510678739250316
1381.28 0.0497579217856394
1419.2 0.0495091012524242
1454.14 0.0492151371580982
1489.52 0.0480027766415077
1547.72 0.0464719675763181
1610.68 0.0449913213688066
1634.42 0.0431324050054136
1682.78 0.0428052169277452
1718.32 0.0416033296051277
1745.56 0.0417289813907315
1854.32 0.0398077563527018
1878.62 0.0384112505411913
1924.54 0.0382038793308905
1972.58 0.0378885025515901
2015.78 0.0373870617117983
2072.82 0.0371005743950363
2126.78 0.0364236880231272
2200.28 0.0349750636140511
2212.1 0.0353754627700134
2295.58 0.0341054609739773
2390.64 0.0327536747181491
2462.5 0.0315082848548305
2501.9 0.0306364059686547
2552.72 0.0297553679220645
2599.8 0.0288639024733818
2620.04 0.0282646520577079
2723.1 0.0275734089461694
2762.4 0.0263675400258431
2811.56 0.024503256173126
2918.68 0.0236725950917799
2978.94 0.0232528794551627
3061.4 0.0217988925199399
3141 0.0208685494723409
3253.48 0.0206011148317047
3377.84 0.0204027368111624
3484.94 0.0198889657310008
3608.16 0.019148159076109
3744.22 0.0180169420148316
3770.02 0.0171822906571962
3914.58 0.0165972758419086
4083.74 0.0158856769487742
};
\addplot [very thick, royalblue28108204]
table {%
134.88 0.242862938196885
196.267474747475 0.173124710996861
257.65494949495 0.134218308313717
319.042424242424 0.109322413975728
380.429898989899 0.0920069543795677
441.817373737374 0.0792653587477838
503.204848484848 0.0694989375469172
564.592323232323 0.0617775415149305
625.979797979798 0.0555225667610392
687.367272727273 0.0503549657710128
748.754747474747 0.046015941584323
810.142222222222 0.042322722683932
871.529696969697 0.0391425387862191
932.917171717172 0.0363766111199504
994.304646464646 0.0339499282799642
1055.69212121212 0.0318045050957605
1117.0795959596 0.0298948136534801
1178.46707070707 0.0281846110435338
1239.85454545455 0.0266446896047914
1301.24202020202 0.0252512510379704
1362.62949494949 0.0239847114098992
1424.01696969697 0.0228288094315075
1485.40444444444 0.021769931849661
1546.79191919192 0.0207965966845129
1608.17939393939 0.0198990528446038
1669.56686868687 0.0190689666538676
1730.95434343434 0.0182991740541754
1792.34181818182 0.0175834829775066
1853.72929292929 0.0169165144291465
1915.11676767677 0.0162935737195602
1976.50424242424 0.0157105453804277
2037.89171717172 0.0151638068370931
2099.27919191919 0.0146501570473091
2160.66666666667 0.0141667571666228
2222.05414141414 0.0137110809423935
2283.44161616162 0.0132808730267225
2344.82909090909 0.0128741137731788
2406.21656565657 0.0124889893717875
2467.60404040404 0.0121238664022314
2528.99151515152 0.0117772700619735
2590.37898989899 0.0114478654654749
2651.76646464646 0.0111344415213915
2713.15393939394 0.0108358969830264
2774.54141414141 0.0105512283382806
2835.92888888889 0.0102795192626196
2897.31636363636 0.0100199314050252
2958.70383838384 0.00977169631476125
3020.09131313131 0.00953410834777443
3081.47878787879 0.00930651841703759
3142.86626262626 0.00908832847218261
3204.25373737374 0.00887898661121444
3265.64121212121 0.00867798274161208
3327.02868686869 0.00848484472024654
3388.41616161616 0.00829913491170584
3449.80363636364 0.00812044711316348
3511.19111111111 0.0079484038011363
3572.57858585859 0.00778265366158094
3633.96606060606 0.00762286936995854
3695.35353535353 0.00746874559230882
3756.74101010101 0.00731999718214105
3818.12848484848 0.00717635755117383
3879.51595959596 0.00703757719472404
3940.90343434343 0.00690342235492718
4002.29090909091 0.00677367380702608
4063.67838383838 0.00664812575574283
4125.06585858586 0.00652658483028775
4186.45333333333 0.00640886916789847
4247.84080808081 0.0062948075769657
4309.22828282828 0.00618423877181935
4370.61575757576 0.00607701067213557
4432.00323232323 0.0059729797607044
4493.39070707071 0.00587201049397938
4554.77818181818 0.00577397476043077
4616.16565656566 0.00567875138225287
4677.55313131313 0.00558622565644187
4738.94060606061 0.00549628893167259
4800.32808080808 0.00540883821776806
4861.71555555556 0.00532377582487831
4923.10303030303 0.00524100902977297
4984.4905050505 0.00516044976690703
5045.87797979798 0.00508201434214713
5107.26545454545 0.00500562316724883
5168.65292929293 0.00493120051335624
5230.0404040404 0.00485867428195799
5291.42787878788 0.00478797579187898
5352.81535353535 0.00471903958101718
5414.20282828283 0.00465180322165235
5475.5903030303 0.00458620714825855
5536.97777777778 0.00452219449684713
5598.36525252525 0.00445971095495246
5659.75272727273 0.0043987046214495
5721.1402020202 0.00433912587546227
5782.52767676768 0.0042809272536851
5843.91515151515 0.00422406333549569
5905.30262626263 0.00416849063529061
5966.6901010101 0.00411416750152104
6028.07757575757 0.00406105402194878
6089.46505050505 0.00400911193468194
6150.85252525253 0.00395830454458424
6212.24 0.00390859664468467
};
\addplot [very thick, cadetblue80178158]
table {%
241.02 0.123615779601643
281.137171717172 0.131733343021864
321.254343434343 0.137537024027132
361.371515151515 0.141554571180873
401.488686868687 0.144185659198337
441.605858585859 0.145734929119424
481.72303030303 0.1464364857029
521.840202020202 0.146471748431619
561.957373737374 0.14598244539285
602.074545454545 0.145080124500493
642.191717171717 0.143853173781427
682.308888888889 0.14237205179191
722.426060606061 0.140693221865716
762.543232323232 0.13886213912467
802.660404040404 0.13691553862015
842.777575757576 0.134883202937277
882.894747474747 0.132789338504872
923.011919191919 0.13065365516552
963.129090909091 0.128492218825769
1003.24626262626 0.12631812920632
1043.36343434343 0.124142061783687
1083.48060606061 0.121972703540151
1123.59777777778 0.119817105134944
1163.71494949495 0.11768096688887
1203.83212121212 0.115568872052168
1243.94929292929 0.113484477856042
1284.06646464646 0.111430672584314
1324.18363636364 0.109409705163601
1364.30080808081 0.10742329242757
1404.41797979798 0.105472708166837
1444.53515151515 0.10355885725978
1484.65232323232 0.101682337537638
1524.76949494949 0.0998434915299525
1564.88666666667 0.0980424498333189
1605.00383838384 0.0962791675247727
1645.12101010101 0.0945534547831362
1685.23818181818 0.0928650026739802
1725.35535353535 0.0912134048858723
1765.47252525253 0.0895981760692599
1805.5896969697 0.0880187673182363
1845.70686868687 0.0864745792445994
1885.82404040404 0.0849649730190826
1925.94121212121 0.0834892796932765
1966.05838383838 0.0820468080650971
2006.17555555556 0.0806368513087041
2046.29272727273 0.0792586925549125
2086.4098989899 0.0779116095791291
2126.52707070707 0.0765948787296094
2166.64424242424 0.0753077782085409
2206.76141414141 0.074049590801454
2246.87858585859 0.0728196061361364
2286.99575757576 0.0716171225401763
2327.11292929293 0.0704414485560721
2367.2301010101 0.0692919041642261
2407.34727272727 0.0681678217568375
2447.46444444444 0.067068546899505
2487.58161616162 0.0659934389120682
2527.69878787879 0.0649418712957242
2567.81595959596 0.0639132320296154
2607.93313131313 0.0629069237568037
2648.0503030303 0.0619223638767415
2688.16747474747 0.0609589845589427
2728.28464646465 0.0600162326904931
2768.40181818182 0.0590935697682698
2808.51898989899 0.0581904717452106
2848.63616161616 0.0573064288386664
2888.75333333333 0.0564409453077367
2928.87050505051 0.0555935392055174
2968.98767676768 0.0547637421113445
3009.10484848485 0.0539510988473979
3049.22202020202 0.0531551671833958
3089.33919191919 0.0523755175325737
3129.45636363636 0.0516117326416707
3169.57353535354 0.0508634072772421
3209.69070707071 0.0501301479102656
3249.80787878788 0.0494115724007058
3289.92505050505 0.0487073096834403
3330.04222222222 0.0480169994567225
3370.15939393939 0.0473402918741612
3410.27656565657 0.0466768472410285
3450.39373737374 0.0460263357155567
3490.51090909091 0.0453884370157657
3530.62808080808 0.044762840132249
3570.74525252525 0.0441492430472518
3610.86242424242 0.0435473524602972
3650.9795959596 0.042956883520548
3691.09676767677 0.0423775595660259
3731.21393939394 0.0418091118697709
3771.33111111111 0.0412512793929659
3811.44828282828 0.04070380854503
3851.56545454545 0.0401664529506425
3891.68262626263 0.0396389732236378
3931.7997979798 0.0391211367476903
3971.91696969697 0.0386127174636887
4012.03414141414 0.0381134956636863
4052.15131313131 0.0376232577912992
4092.26848484848 0.0371417962484193
4132.38565656566 0.0366689092080957
4172.50282828283 0.0362044004334382
4212.62 0.0357480791023894
};
\addplot [very thick, chocolate21910927]
table {%
16.9 1.01049020173207
82.1541414141414 0.320561653957869
147.408282828283 0.206402444440932
212.662424242424 0.155942286786061
277.916565656566 0.126807186027614
343.170707070707 0.107599552389042
408.424848484848 0.0938793417957881
473.67898989899 0.0835354156520529
538.933131313131 0.0754277768996142
604.187272727273 0.0688835171195139
669.441414141414 0.0634783111036655
734.695555555556 0.0589305617328485
799.949696969697 0.0550456202935834
865.203838383838 0.0516843863092689
930.45797979798 0.0487446618402863
995.712121212121 0.0461495800653194
1060.96626262626 0.0438401526681673
1126.2204040404 0.0417703155572343
1191.47454545455 0.0399035440927263
1256.72868686869 0.038210484743172
1321.98282828283 0.0366672627393692
1387.23696969697 0.0352542500000516
1452.49111111111 0.0339551530643761
1517.74525252525 0.0327563277145495
1582.99939393939 0.0316462569147605
1648.25353535354 0.0306151482204107
1713.50767676768 0.0296546198065354
1778.76181818182 0.0287574530717041
1844.01595959596 0.0279173958436688
1909.2701010101 0.0271290044609968
1974.52424242424 0.0263875160200224
2039.77838383838 0.0256887442445272
2105.03252525253 0.0250289940134713
2170.28666666667 0.0244049907434256
2235.54080808081 0.0238138216860423
2300.79494949495 0.0232528868495132
2366.04909090909 0.0227198577445177
2431.30323232323 0.0222126425308903
2496.55737373737 0.0217293564307377
2561.81151515152 0.0212682964985008
2627.06565656566 0.020827920014202
2692.3197979798 0.0204068259044733
2757.57393939394 0.0200037387055657
2822.82808080808 0.0196174946699071
2888.08222222222 0.0192470296878108
2953.33636363636 0.0188913687523849
3018.59050505051 0.0185496167414301
3083.84464646465 0.0182209503273523
3149.09878787879 0.0179046108565844
3214.35292929293 0.0175998980650419
3279.60707070707 0.0173061645168049
3344.86121212121 0.0170228106703372
3410.11535353535 0.0167492804908034
3475.3694949495 0.0164850575389393
3540.62363636364 0.0162296614769072
3605.87777777778 0.0159826449399525
3671.13191919192 0.0157435907297594
3736.38606060606 0.0155121092913955
3801.6402020202 0.0152878364408261
3866.89434343434 0.0150704313143151
3932.14848484849 0.0148595745147327
3997.40262626263 0.014654966432965
4062.65676767677 0.0144563257253433
4127.91090909091 0.0142633879303631
4193.16505050505 0.0140759042099835
4258.41919191919 0.0138936402025566
4323.67333333333 0.0137163749759544
4388.92747474747 0.0135439000707866
4454.18161616162 0.0133760186247521
4519.43575757576 0.0132125445701758
4584.6898989899 0.0130533018976622
4649.94404040404 0.012898123979569
4715.19818181818 0.0127468529476832
4780.45232323232 0.0125993391200779
4845.70646464646 0.0124554404726553
4910.96060606061 0.0123150221513459
4976.21474747475 0.0121779560213463
5041.46888888889 0.0120441202501399
5106.72303030303 0.0119133989213719
5171.97717171717 0.011785681676936
5237.23131313131 0.0116608633848866
5302.48545454545 0.0115388438310181
5367.7395959596 0.0114195274321603
5432.99373737374 0.0113028229694171
5498.24787878788 0.0111886433397434
5563.50202020202 0.0110769053243985
5628.75616161616 0.0109675293729483
5694.0103030303 0.0108604394016074
5759.26444444444 0.0107555626048159
5824.51858585859 0.0106528292790462
5889.77272727273 0.0105521726579186
5955.02686868687 0.0104535287577842
6020.28101010101 0.0103568362330055
6085.53515151515 0.0102620362402281
6150.78929292929 0.0101690723109952
6216.04343434343 0.0100778902321111
6281.29757575758 0.00998843793320686
6346.55171717172 0.00990066538100378
6411.80585858586 0.00981452447981433
6477.06 0.00972996897785126
};
\addplot [very thick, purple11522131]
table {%
271.48 0.124646774651517
330.229494949495 0.108540666047395
388.97898989899 0.0963184344669057
447.728484848485 0.0866825357103684
506.47797979798 0.0788658331766388
565.227474747475 0.0723827034444968
623.97696969697 0.0669092993620967
682.726464646465 0.0622205990214981
741.47595959596 0.058154954100573
800.225454545455 0.0545929965738806
858.97494949495 0.0514445102266484
917.724444444445 0.0486399460942849
976.47393939394 0.0461247611453029
1035.22343434343 0.0438555355465756
1093.97292929293 0.0417972453478111
1152.72242424242 0.0399213061383828
1211.47191919192 0.038204143421952
1270.22141414141 0.0366261304453583
1328.97090909091 0.0351707872124178
1387.7204040404 0.0338241682942617
1446.4698989899 0.0325743892010176
1505.21939393939 0.0314112558609328
1563.96888888889 0.0303259717984829
1622.71838383838 0.0293109045451846
1681.46787878788 0.0283593976885111
1740.21737373737 0.0274656184314793
1798.96686868687 0.0266244330353109
1857.71636363636 0.0258313043417318
1916.46585858586 0.0250822069175078
1975.21535353535 0.0243735563673994
2033.96484848485 0.0237021501172497
2092.71434343434 0.0230651175428836
2151.46383838384 0.0224598777602348
2210.21333333333 0.0218841037317188
2268.96282828283 0.0213356916081128
2327.71232323232 0.0208127344322585
2386.46181818182 0.0203134994942501
2445.21131313131 0.019836408757435
2503.96080808081 0.0193800218781101
2562.7103030303 0.0189430214249721
2621.4597979798 0.0185241999715374
2680.20929292929 0.018122448789264
2738.95878787879 0.0177367479135682
2797.70828282828 0.0173661573913644
2856.45777777778 0.0170098095487461
2915.20727272727 0.0166669021422159
2973.95676767677 0.0163366922774468
3032.70626262626 0.0160184909967024
3091.45575757576 0.0157116584503782
3150.20525252525 0.0154155995801649
3208.95474747475 0.015129760251467
3267.70424242424 0.0148536237812754
3326.45373737374 0.0145867078149566
3385.20323232323 0.0143285615115896
3443.95272727273 0.0140787630027526
3502.70222222222 0.0138369170941604
3561.45171717172 0.0136026531834171
3620.20121212121 0.0133756233704704
3678.95070707071 0.0131555007402147
3737.7002020202 0.0129419777991651
3796.4496969697 0.0127347650502675
3855.19919191919 0.0125335896917713
3913.94868686869 0.0123381944277101
3972.69818181818 0.0121483363789475
4031.44767676768 0.0119637860849808
4090.19717171717 0.0117843265877746
4148.94666666667 0.0116097525898459
4207.69616161616 0.011439869679656
4266.44565656566 0.0112744936180971
4325.19515151515 0.0111134496805125
4383.94464646465 0.010956572049259
4442.69414141414 0.0108037032523287
4501.44363636364 0.0106546936439982
4560.19313131313 0.0105094009238689
4618.94262626263 0.0103676896910233
4677.69212121212 0.0102294310303328
4736.44161616162 0.0100945021282401
4795.19111111111 0.00996278591558857
4853.94060606061 0.00983417073529973
4912.6901010101 0.0097085500328994
4971.4395959596 0.00958582206807847
5030.18909090909 0.00946588964563466
5088.93858585859 0.00934865986429039
5147.68808080808 0.00923404388201352
5206.43757575758 0.00912195669658737
5265.18707070707 0.00901231694028437
5323.93656565657 0.00890504668759518
5382.68606060606 0.0088000712750529
5441.43555555556 0.00869731913227306
5500.18505050505 0.00859672162340113
5558.93454545455 0.00849821289822685
5617.68404040404 0.00840172975228257
5676.43353535354 0.00830721149529967
5735.18303030303 0.00821459982744426
5793.93252525253 0.00812383872280056
5852.68202020202 0.00803487431961075
5911.43151515152 0.00794765481681761
5970.18101010101 0.00786213037649167
6028.93050505051 0.00777825303175499
6087.68 0.00769597659984356
};
\addplot [very thick, black18]
table {%
17.04 0.932717267872456
79.0674747474747 0.247674448608199
141.09494949495 0.145992801595961
203.122424242424 0.103863999830355
265.149898989899 0.080656823653117
327.177373737374 0.0659186834890728
389.204848484849 0.055714600939436
451.232323232323 0.0482256307167465
513.259797979798 0.0424930350050827
575.287272727273 0.0379628079173876
637.314747474747 0.0342921883850146
699.342222222222 0.0312575993984191
761.369696969697 0.0287069207549414
823.397171717172 0.0265330188538077
885.424646464646 0.0246582428215552
947.452121212121 0.023024924883583
1009.4795959596 0.021589334639344
1071.50707070707 0.0203177048282383
1133.53454545455 0.0191835446862009
1195.56202020202 0.0181657788197237
1257.5894949495 0.0172474298974436
1319.61696969697 0.0164146682708938
1381.64444444444 0.0156561145061229
1443.67191919192 0.014962319597827
1505.69939393939 0.0143253721806966
1567.72686868687 0.0137385979370215
1629.75434343434 0.0131963268925689
1691.78181818182 0.0126937113543846
1753.80929292929 0.0122265820779414
1815.83676767677 0.0117913336117289
1877.86424242424 0.0113848321375829
1939.89171717172 0.0110043408189513
2001.91919191919 0.0106474588947736
2063.94666666667 0.0103120716533946
2125.97414141414 0.00999630908410932
2188.00161616162 0.00969851149925658
2250.02909090909 0.00941720079317357
2312.05656565657 0.00915105628825643
2374.08404040404 0.00889889433605097
2436.11151515152 0.008659651009466
2498.13898989899 0.00843236735306973
2560.16646464646 0.0082161767609678
2622.19393939394 0.00801029413262752
2684.22141414141 0.00781400652117835
2746.24888888889 0.00762666503993279
2808.27636363636 0.00744767783397348
2870.30383838384 0.00727650395681501
2932.33131313131 0.00711264801903989
2994.35878787879 0.00695565549771799
3056.38626262626 0.00680510861335332
3118.41373737374 0.00666062269584577
3180.44121212121 0.0065218429731277
3242.46868686869 0.00638844172622472
3304.49616161616 0.00626011576288528
3366.52363636364 0.0061365841689352
3428.55111111111 0.00601758630238964
3490.57858585859 0.00590288000029753
3552.60606060606 0.00579223997246298
3614.63353535354 0.00568545635971803
3676.66101010101 0.00558233343741786
3738.68848484848 0.00548268844738088
3800.71595959596 0.00538635054367493
3862.74343434343 0.00529315983951697
3924.77090909091 0.00520296654415457
3986.79838383838 0.00511563017997647
4048.82585858586 0.00503101887128872
4110.85333333333 0.0049490086972217
4172.88080808081 0.00486948310212484
4234.90828282828 0.00479233235758085
4296.93575757576 0.0047174530708458
4358.96323232323 0.00464474773510978
4420.99070707071 0.00457412431748768
4483.01818181818 0.00450549588110049
4545.04565656566 0.00443878023800289
4607.07313131313 0.00437389963006113
4669.10060606061 0.00431078043519187
4731.12808080808 0.00424935289664253
4793.15555555556 0.00418955087323354
4855.18303030303 0.00413131160869437
4917.21050505051 0.00407457551841281
4979.23797979798 0.00401928599208401
5041.26545454545 0.00396538921089453
5103.29292929293 0.00391283397800814
5165.3204040404 0.00386157156123891
5227.34787878788 0.00381155554690216
5289.37535353535 0.00376274170392822
5351.40282828283 0.00371508785740882
5413.4303030303 0.00366855377082141
5475.45777777778 0.00362310103624512
5537.48525252525 0.00357869297194334
5599.51272727273 0.00353529452674306
5661.5402020202 0.00349287219069102
5723.56767676768 0.00345139391151151
5785.59515151515 0.0034108290164315
5847.62262626263 0.00337114813897532
5909.6501010101 0.00333232315036458
5971.67757575758 0.0032943270951892
6033.70505050505 0.00325713413104272
6095.73252525253 0.00322071947183999
6157.76 0.0031850593345583
};
\addplot [very thick, darkgray153]
table {%
17.04 0.759016557624628
86.509494949495 0.34025082237529
155.97898989899 0.225950429277701
225.448484848485 0.169443929528277
294.91797979798 0.135255781651643
364.387474747475 0.112224827089551
433.85696969697 0.0956226637016561
503.326464646465 0.0830794622714685
572.79595959596 0.0732691386745628
642.265454545455 0.0653890703073975
711.73494949495 0.0589239265065404
781.204444444445 0.0535272122085044
850.673939393939 0.0489571418335356
920.143434343434 0.0450397613899738
989.612929292929 0.041646671345177
1059.08242424242 0.0386810081361487
1128.55191919192 0.0360683126797267
1198.02141414141 0.0337504035617864
1267.49090909091 0.0316811593837038
1336.9604040404 0.0298235493756608
1406.4298989899 0.0281475009200204
1475.89939393939 0.0266283408018333
1545.36888888889 0.0252456376431411
1614.83838383838 0.0239823299068171
1684.30787878788 0.0228240604671117
1753.77737373737 0.0217586627957565
1823.24686868687 0.0207757599207151
1892.71636363636 0.019866448293877
1962.18585858586 0.0190230463083144
2031.65535353535 0.0182388925506849
2101.12484848485 0.0175081826825503
2170.59434343434 0.0168258365918839
2240.06383838384 0.0161873894614641
2309.53333333333 0.0155889018805266
2379.00282828283 0.0150268852288785
2448.47232323232 0.0144982393924045
2517.94181818182 0.0140002004986889
2587.41131313131 0.0135302968434885
2656.88080808081 0.0130863115505838
2726.3503030303 0.0126662507964212
2795.8197979798 0.0122683166569964
2865.28929292929 0.0118908838124413
2934.75878787879 0.0115324794858532
3004.22828282828 0.0111917661053599
3073.69777777778 0.010867526268563
3143.16727272727 0.0105586496611517
3212.63676767677 0.0102641216403259
3282.10626262626 0.00998301324156105
3351.57575757576 0.00971447240641304
3421.04525252525 0.00945771626122201
3490.51474747475 0.00921202430310304
3559.98424242424 0.00897673237157738
3629.45373737374 0.00875122730245869
3698.92323232323 0.0085349421758453
3768.39272727273 0.00832735208282715
3837.86222222222 0.00812797034623654
3907.33171717172 0.00793634513980794
3976.80121212121 0.00775205645775455
4046.27070707071 0.00757471339325137
4115.7402020202 0.00740395168982957
4185.2096969697 0.00723943153439219
4254.67919191919 0.00708083556458569
4324.14868686869 0.00692786706671561
4393.61818181818 0.00678024834336237
4463.08767676768 0.00663771923241399
4532.55717171717 0.00650003576144388
4602.02666666667 0.00636696892327711
4671.49616161616 0.0062383035602527
4740.96565656566 0.0061138373461352
4810.43515151515 0.00599337985589061
4879.90464646465 0.00587675171464338
4949.37414141414 0.00576378381809582
5018.84363636364 0.0056543166175365
5088.31313131313 0.00554819946330797
5157.78262626263 0.00544529000125795
5227.25212121212 0.00534545361727451
5296.72161616162 0.00524856292551606
5366.19111111111 0.00515449729639674
5435.66060606061 0.00506314242078795
5505.1301010101 0.00497438990725073
5574.5995959596 0.0048881369094295
5644.06909090909 0.00480428578101719
5713.53858585859 0.00472274375595325
5783.00808080808 0.00464342265173839
5852.47757575758 0.00456623859394975
5921.94707070707 0.00449111176021946
5991.41656565657 0.00441796614209939
6060.88606060606 0.0043467293233787
6130.35555555556 0.00427733227355054
6199.82505050505 0.0042097091552401
6269.29454545455 0.00414379714451159
6338.76404040404 0.00407953626306556
6408.23353535354 0.00401686922142425
6477.70303030303 0.00395574127227903
6547.17252525253 0.00389610007324456
6616.64202020202 0.0038378955583269
6686.11151515152 0.00378107981747105
6755.58101010101 0.00372560698360466
6825.05050505051 0.00367143312664264
6894.52 0.0036185161539604
};
\addplot [very thick, saddlebrown1356716]
table {%
274.56 0.0941615841758089
313.036565656566 0.0928074691522695
351.513131313131 0.0910955361022653
389.989696969697 0.0891741865136961
428.466262626263 0.0871386540263313
466.942828282828 0.0850511493872246
505.419393939394 0.0829527470907495
543.89595959596 0.080870662765746
582.372525252525 0.0788228472479106
620.849090909091 0.0768209622533218
659.325656565657 0.0748723501087257
697.802222222222 0.072981361842065
736.278787878788 0.0711502667389212
774.755353535353 0.0693798835195913
813.231919191919 0.0676700231738313
851.708484848485 0.0660198024502866
890.18505050505 0.0644278673447908
928.661616161616 0.0628925532408186
967.138181818182 0.0614120000136561
1005.61474747475 0.0599842348384178
1044.09131313131 0.058607231666599
1082.56787878788 0.0572789537435819
1121.04444444444 0.0559973837381779
1159.52101010101 0.0547605447898513
1197.99757575758 0.0535665148813977
1236.47414141414 0.0524134363019745
1274.95070707071 0.0512995215012507
1313.42727272727 0.050223056297835
1351.90383838384 0.0491824011578695
1390.3804040404 0.0481759910774515
1428.85696969697 0.0472023344675113
1467.33353535354 0.0462600113392064
1505.8101010101 0.0453476710126761
1544.28666666667 0.0444640295155303
1582.76323232323 0.0436078667949163
1621.2397979798 0.0427780238349008
1659.71636363636 0.0419733997466181
1698.19292929293 0.0411929488802471
1736.66949494949 0.0404356779939525
1775.14606060606 0.0397006435043819
1813.62262626263 0.0389869488353486
1852.09919191919 0.0382937418753227
1890.57575757576 0.0376202125498575
1929.05232323232 0.0369655905117223
1967.52888888889 0.0363291429490402
2006.00545454545 0.0357101725099226
2044.48202020202 0.0351080153408084
2082.95858585859 0.0345220392348141
2121.43515151515 0.0339516418858025
2159.91171717172 0.0333962492435075
2198.38828282828 0.0328553139648438
2236.86484848485 0.0323283139564597
2275.34141414141 0.0318147510036052
2313.81797979798 0.0313141494804759
2352.29454545455 0.0308260551373265
2390.77111111111 0.0303500339598182
2429.24767676768 0.0298856710962528
2467.72424242424 0.0294325698485501
2506.20080808081 0.0289903507230389
2544.67737373737 0.0285586505373391
2583.15393939394 0.0281371215798269
2621.6305050505 0.0277254308183785
2660.10707070707 0.0273232591552875
2698.58363636364 0.0269303007254433
2737.0602020202 0.026546262235039
2775.53676767677 0.0261708623382544
2814.01333333333 0.0258038310495189
2852.4898989899 0.0254449091891223
2890.96646464646 0.0250938478600786
2929.44303030303 0.0247504079542941
2967.9195959596 0.024414359686212
3006.39616161616 0.0240854821522333
3044.87272727273 0.02376356291432
3083.34929292929 0.0234483976062978
3121.82585858586 0.023139789561468
3160.30242424242 0.0228375494602356
3198.77898989899 0.0225414949965409
3237.25555555556 0.0222514505619655
3275.73212121212 0.0219672469464542
3314.20868686869 0.0216887210546673
3352.68525252525 0.0214157156370379
3391.16181818182 0.021148079034672
3429.63838383838 0.0208856649372833
3468.11494949495 0.0206283321534069
3506.59151515152 0.0203759443921839
3545.06808080808 0.020128370056056
3583.54464646465 0.0198854820437476
3622.02121212121 0.0196471575629561
3660.49777777778 0.0194132779522035
3698.97434343434 0.0191837285113406
3737.45090909091 0.0189583983402222
3775.92747474747 0.0187371801851051
3814.40404040404 0.0185199702923467
3852.88060606061 0.0183066682690072
3891.35717171717 0.0180971769499827
3929.83373737374 0.0178914022713203
3968.3103030303 0.0176892531493859
4006.78686868687 0.017490641365574
4045.26343434343 0.01729548145627
4083.74 0.0171036906077902
};
\addplot [draw=black, fill=black, mark=x, very thick, mark size=2.5pt, only marks]
table{%
x  y
69.92 0.473622812407748
274.56 0.160676273820694
1091.84 0.0436020304761968
4515.84 0.0106870280954713
};
