# Supplementary material for: Swarm Reinforcement Learning For Adaptive Mesh Refinement
Source: arXiv:2304.00818 source file (2023-10-09)
Supplement: Supplementary file 12 [file group_additional_metrics_r1.tex]

\nextgroupplot[
ylabel shift = -0.2cm,
clip marker paths=true,
title style={yshift=-0.2cm},
height=4.5cm,
width=0.50\textwidth,
legend cell align={left},
legend style={fill opacity=0.8, draw opacity=1, text opacity=1, draw=lightgray204},
log basis y={10},
tick align=outside,
tick pos=left,
x grid style={darkgray176},
xlabel={\empty},
title={Laplace's Equation},
xmajorgrids,
xmin=-411.724, xmax=9371.324,
xtick style={color=black},
xtick={-2000,0,2000,4000,6000,8000,10000},
xticklabels={-2.0,0.0,2.0,4.0,6.0,8.0,10.0},
y grid style={darkgray176},
ylabel={Top $0.1\,\%$ Error},
ymajorgrids,
ymin=0.00392430215125743, ymax=1.93038921171556,
ymode=log,
ytick style={color=black},
ytick={0.0001,0.001,0.01,0.1,1,10,100},
yticklabels={
  \(\displaystyle {10^{-4}}\),
  \(\displaystyle {10^{-3}}\),
  \(\displaystyle {10^{-2}}\),
  \(\displaystyle {10^{-1}}\),
  \(\displaystyle {10^{0}}\),
  \(\displaystyle {10^{1}}\),
  \(\displaystyle {10^{2}}\)
}
]
\addplot [
  draw=royalblue28108204,
  fill=royalblue28108204,
  forget plot,
  mark=*, mark size=1,
  only marks,
  draw opacity=0,
 fill opacity=0.5
]
table{%
x  y
33.52 0.999999999999973
64.5 0.590307097630691
66.7 0.584821862550677
66.84 0.573517519579107
67.12 0.580596188549328
68.4 0.572854624886529
69.82 0.562902959861192
71 0.55445826701756
74.16 0.539377402759181
77.38 0.511146856423738
103.38 0.429051741330797
119.78 0.332665622626089
121.5 0.325662556196854
125 0.352907459325499
126.64 0.364988068339992
132.94 0.370451996510936
133.4 0.327296482975018
134.7 0.353120509577495
137 0.336078231063038
137.36 0.328797463085102
273.2 0.160403191857739
275.38 0.17612264079397
295.62 0.175690557732173
298.38 0.194824589780441
300.16 0.1840808740023
319.06 0.187880733244981
336.12 0.230538961010179
342.78 0.170011423881145
342.84 0.157271299474451
352.5 0.167185359283964
352.64 0.171827508480486
357.9 0.144685026118205
397.32 0.1713234206091
424.78 0.145044395277693
435.3 0.0979279711158779
439.5 0.167541476790286
456.44 0.09810709802364
476.38 0.139517068715451
529.26 0.114638014276998
567.42 0.124573521619638
588.94 0.0873803944159866
636.84 0.0884148641482334
647.28 0.0864326813431003
685.24 0.096564621651327
704.48 0.0731669017393685
732.98 0.0903577108518634
766.9 0.118859856677266
861.08 0.0845386257605314
937.42 0.0759786368095192
958.02 0.0543289490792487
1037.64 0.0744031176193805
1049.72 0.0768770469804815
1074.48 0.062341756780888
1083.2 0.0648491599189358
1122.5 0.0676988638595765
1200.18 0.0701528864380032
1206.6 0.0661011906536927
1326.24 0.0401067634680085
1338.1 0.069108360034423
1379.32 0.06769672223611
1477.24 0.0632256019322069
1512.34 0.0452657549424769
1548.6 0.0574778321836805
1559.88 0.0532763165390679
1696.38 0.054587090614858
1761.28 0.0495713727366948
1900.52 0.0437138883501228
1976.5 0.0452905498125134
1983.22 0.043812339525152
2101.32 0.0373264884309285
2267.26 0.0324307275714326
2352.6 0.0383462478554905
2539.9 0.0296103988952919
2973.28 0.0318406269398944
3234.38 0.0251044691359993
3257.34 0.0270554155209388
3275.22 0.023710424416294
3281.68 0.0305181554481558
3651.98 0.0244791935274518
3719.78 0.0240843389142087
3742.06 0.0269863675428058
3794.42 0.0250175611846564
3847.78 0.0228510068362316
3901.08 0.025952130310459
4076.68 0.0255523933929157
4415.34 0.0245845136451815
4486.44 0.0187657377830195
4521.46 0.017799799734637
4575.16 0.0216367725722062
4840.32 0.0242319368199741
5145.86 0.023727072782864
5409.52 0.0183789200048805
6412.3 0.0174233197872813
6944.16 0.0117267110214251
7383.8 0.0135610601278447
7428.84 0.0146640907818188
7474.62 0.0213328539585994
7594.52 0.0110004906469171
7962.56 0.012657312403401
8690.78 0.0139729712777573
};
\addplot [
  draw=cadetblue80178158,
  fill=cadetblue80178158,
  forget plot,
  mark=*, mark size=1,
  only marks,
  draw opacity=0,
 fill opacity=0.5
]
table{%
x  y
269.44 0.297100307573756
272.24 0.170298924036845
275.86 0.173318868291168
284.14 0.162839570975744
287.14 0.255411328443363
287.2 0.198257478287267
300.54 0.305502293171858
307.94 0.260833020828009
309.96 0.173393835686084
334.24 0.199112338309936
466.3 0.139276503030591
478.1 0.120496538390909
505 0.153702923028779
520.32 0.119572417194979
525.22 0.261702495022289
530.82 0.119439929537667
534.2 0.152175020953633
536.38 0.10289235199797
552.12 0.135359307642963
607.06 0.101131913713388
673.98 0.111879379170428
708.56 0.112462293307713
717.22 0.142698924255519
729.58 0.0999899022814592
741.8 0.114260045830483
747.26 0.149372765281708
778.92 0.75682233007154
808.72 0.132781402030934
830.16 0.120917796900537
858.02 0.150720016366526
876.44 0.124100872282018
882.26 0.137307489021787
886.06 0.11455750078349
904.82 0.131913029046941
906.2 0.076325695305403
909.58 0.119359478832882
950.58 0.0695661544706626
960.66 0.0861436353707652
985.38 0.123681129833706
1005.86 0.125258986123118
1030.08 0.134007310272221
1032.84 0.118726993636174
1131.02 0.0861181726735627
1192.64 0.116479471890105
1294.02 0.048114186011647
1325.06 0.0473687628573225
1330 0.0438182952395323
1349.98 0.060293101575095
1363 0.100591273174827
1378.7 0.121526434550626
1436.98 0.0996653226385506
1456.72 0.0720970719087714
1579 0.0331284963333917
1637.16 0.0536047440975469
1638.58 0.112293488543181
1642.26 0.103681806030008
1678.86 0.04889774125936
1681.64 0.0317884632492597
1738.32 0.0433661921425468
1769.26 0.0561136387451088
1870.28 0.0594286944530067
1871.1 0.0982805539246491
1902.4 0.0975668681348573
1936.64 0.060936928729611
2094.1 0.0939058260429389
2098.04 0.0590216433332079
2158.68 0.301501742001208
2238.24 0.282545947568553
2246.4 0.061264335580051
2283.88 0.0454303944307129
2310.02 0.0324096117387761
2355.52 0.023577188089178
2379.12 0.0208966118490871
2400.7 0.0897573423881581
2404.84 0.0503617630632151
2464.98 0.0402951360641627
2511.58 0.0299957839275513
2522.54 0.0511854539945445
2529.9 0.0186731585348783
2573.18 0.0285245573205758
2668.36 0.0535453801313554
2687.78 0.309700147414061
2725.32 0.0241968512427376
2729.02 0.159835508067205
2787.66 0.0519631228000824
2809.5 0.159833859816756
2812.78 0.0992273925252277
2835.22 0.0227513198107071
2858.06 0.0843388015374389
2905.88 0.228603841335432
2930.08 0.0253272896674337
2964.5 0.0584889385797267
3234.66 0.0313226812967626
3280.22 0.149708713825751
3292.32 0.0551175681188116
3365.02 0.054021785829993
3402.36 0.0233244150204179
3434.26 0.0659476642271265
3512.42 0.0200384137884442
3707.38 0.0449747090448398
};
\addplot [
  draw=chocolate21910927,
  fill=chocolate21910927,
  forget plot,
  mark=*, mark size=1,
  only marks,
  draw opacity=0,
 fill opacity=0.5
]
table{%
x  y
33.46 0.999184598070221
33.52 0.999999999999973
33.52 0.999999999999973
33.52 0.999999999999973
33.52 0.999999999999973
33.52 0.999999999999973
33.52 0.999999999999973
33.52 0.999999999999973
33.52 0.999999999999973
33.52 0.999999999999973
33.52 0.999999999999973
33.52 0.999999999999973
33.52 0.999999999999973
33.52 0.999999999999973
33.52 0.999999999999973
33.52 0.999999999999973
33.52 0.999999999999973
33.52 0.999999999999973
33.52 0.999999999999973
33.52 0.999999999999973
33.52 0.999999999999973
33.52 0.999999999999973
33.52 0.999999999999973
33.52 0.999999999999973
33.52 0.999999999999973
33.52 0.999999999999973
48.14 0.887232592232888
52.94 0.872471593315088
66 0.624293708146199
115.74 0.431464318836701
127.16 0.565677836617328
127.28 0.358046126432196
130.88 0.563302347042076
143.54 0.424140681205008
169.5 0.399108511484289
173.28 0.280780780698862
173.78 0.299673996968085
176.6 0.305288576140012
189.96 0.30240892090987
200.32 0.324068897570556
204.38 0.312076657104999
206.98 0.256290414709792
212.8 0.30821705843723
263.3 0.239598880064493
296.32 0.230650128524209
320.78 0.171481052881912
327.3 0.161257803268653
350.36 0.295859968985553
370.7 0.199730055405593
402.48 0.16644285201283
414.94 0.155300813148035
495.62 0.120392312078816
525.48 0.125240246653157
559.5 0.227317882401884
590.34 0.0931722817281173
609.68 0.279803527340112
650.54 0.0931331601826804
658.54 0.0925829614778802
664.2 0.194789273524853
690.1 0.186129561833358
809.38 0.15293598399774
921.94 0.13836856828343
954.5 0.0595535955384117
1069.72 0.0577832104935349
1080 0.0936408376027754
1287.14 0.108393617462772
1345.3 0.0956287335406013
1555.08 0.0684147310191712
2699.3 0.070989502537546
2977.26 0.0741850567934974
3450.04 0.99669629325775
4769.56 0.0940672579197273
8798.68 0.0230023001229247
};
\addplot [draw=purple11522131, fill=purple11522131, forget plot, mark=*, mark size=1, only marks, draw opacity=0,
 fill opacity=0.5]
table{%
x  y
107.5 0.57199530780242
124.98 0.458432331203362
155.66 0.395496860823082
175.74 0.336310915725707
177.34 0.344906321527062
182.6 0.324104423626245
192.86 0.322602120733883
195.3 0.308014175172717
203.86 0.388679978986547
220.06 0.297712859136943
276.34 0.303212522194285
303.3 0.291604793108804
306.26 0.302885428711274
326.26 0.305808006079182
339.86 0.303410069710087
347.84 0.303265136973907
350.54 0.306307185849673
352.08 0.303713197234736
353 0.303442700701954
395.1 0.243509694614683
399.8 0.286985718155311
431.72 0.276747891430341
444.3 0.303891567771138
445.02 0.278314121626174
467.38 0.304244256248771
468.18 0.304264945300126
472.34 0.304280245814863
483.5 0.304309506282045
491.4 0.304330552735115
496.02 0.303892270975126
513.88 0.246937650524519
514.52 0.300552671146966
523.48 0.304387702074228
525.9 0.304295178079806
530.68 0.304302867074118
535.64 0.286611664897466
548.02 0.148064872728711
549.32 0.15868992060578
580.12 0.158449475755703
691.64 0.155502187569301
863.74 0.153799074785315
883.24 0.151265660464086
915.68 0.151231569047558
934.3 0.162843079977879
1025.08 0.155492455600128
1028.84 0.149909469274883
1045.32 0.150665341735532
1100.4 0.150750259329824
1216.56 0.1509059502358
1323.88 0.150695604934678
1370.56 0.150703856683975
1443.32 0.150734141412457
1576.64 0.150807650484798
1711.44 0.150847025031164
1951.6 0.150948660971937
2101.98 0.150969718592951
2107.08 0.150969001601357
2116.6 0.150968880213481
2124.44 0.150971495025919
2160.54 0.150973996812031
2163 0.150974297828352
2163.2 0.150974298879811
2163.2 0.150974298879811
2163.2 0.150974298879811
2163.2 0.150974298879811
2163.2 0.150974298879811
2163.2 0.150974298879811
2163.2 0.150974298879811
2163.2 0.150974298879811
2163.2 0.150974298879811
2163.46 0.134724242236428
2316 0.129353199026885
2338.56 0.129359983236602
2389.08 0.129382279827112
2491.92 0.129398553228173
2614.66 0.129497527130674
2652 0.129423456911059
2673.04 0.129421978400302
2751.68 0.129429102394223
3077.12 0.129435867022172
5155.06 0.063133389084074
6382.64 0.0632428500847893
6868.22 0.0632810208303107
7456.82 0.0632925874015059
7472.48 0.0632922178159606
7958.54 0.0632942773603342
8034.76 0.063297195049943
8217.14 0.0632986691795784
8435.38 0.0633006008178964
8518.96 0.0628417386740761
8638.98 0.0633014516807851
8668.74 0.0628422856293142
8693.24 0.0628423482634744
8693.68 0.0628423489672365
8693.76 0.062842349125676
8693.76 0.062842349125676
8693.76 0.062842349125676
8693.76 0.062842349125676
8693.76 0.062842349125676
8693.76 0.062842349125676
};
\addplot [draw=black18, fill=black18, forget plot, mark=*, mark size=1, only marks, draw opacity=0,
 fill opacity=0.5]
table{%
x  y
33.52 0.999999999999973
90.28 0.508373189067336
93.22 0.491384719949108
96.66 0.46917845960566
98.68 0.460165737996287
101.4 0.451566736195257
109.14 0.429003749948867
111.82 0.413738326916479
114.12 0.406507906005402
115 0.401670196009024
121.3 0.395052068839892
124.62 0.386326221014564
129.78 0.382204880370122
133.82 0.374368122870413
137.68 0.360372156599402
144 0.359855367704484
147.76 0.350409753700469
148.14 0.358320327437816
153.46 0.346291317870336
160.98 0.338472916417558
167.72 0.33435402513411
175.38 0.330265177031243
184.02 0.321751866208178
187.2 0.318113979555778
196.24 0.310599850823828
202.46 0.31137672996195
208.72 0.306312746979744
211.82 0.297974391064646
220.04 0.289709310450746
235.34 0.279858213619542
265.66 0.264975360405286
273.88 0.261047784750391
290.98 0.252604377942575
318.7 0.241215802745467
333.9 0.224053381374907
337.58 0.232316604755628
356.96 0.214627019216544
364.38 0.210307305210649
382.46 0.208600949888548
405.24 0.198743144974719
445.06 0.192144181116989
462.48 0.180753323173122
483.12 0.17673302477131
503.26 0.171814156459525
512.96 0.168359217905497
534.74 0.16670542067382
581.92 0.15934234817807
633.58 0.152737462554005
688.04 0.140707548484303
749.54 0.135718772465614
794.28 0.127757397124167
870.22 0.123814014536384
964.72 0.112595329957665
1058.96 0.104048156774752
1118.36 0.101428295171905
1155.12 0.096792879994904
1313.76 0.0914550604644922
1357.34 0.0886268105050537
1387.24 0.0852040179746643
1540.74 0.081790913624287
1626.52 0.0730907904019229
1629.64 0.0767277820894061
1814.76 0.0710756788678449
2014.46 0.0631236126106223
2262.76 0.0568575146374131
2495.68 0.0495139250141562
2809.94 0.0458511623039902
3048.9 0.0404502266422837
3469.5 0.0353899925726177
3789.32 0.0340660035535036
4193.42 0.0316376545508888
4691.22 0.0294339031379992
5135.12 0.0282439516651055
5607.22 0.0263533068407911
5731.56 0.0243525102509045
6838.66 0.0214327105426079
7345.94 0.0193590602863731
7867.86 0.0162875426728936
8359.56 0.0140862205368887
};
\addplot [draw=darkgray153, fill=darkgray153, forget plot, mark=*, mark size=1, only marks, draw opacity=0,
 fill opacity=0.5]
table{%
x  y
33.52 0.999999999999973
131.76 0.365678045565616
138.54 0.339650449129161
144.04 0.318804733301649
151.6 0.300627307689338
155.1 0.289138794291182
165.02 0.271359398875248
173.64 0.260168284867575
190.04 0.237821221404353
203.2 0.221305929183878
207.84 0.208501382539354
214.98 0.198550670085868
223.72 0.188287320655542
228.14 0.177449567535533
230.38 0.168672001786097
244.6 0.157777675552382
257.66 0.146156579474109
259.08 0.142443903584446
275.94 0.135529806061058
294.82 0.129383141402107
309.34 0.119028081644409
349.12 0.105880631139978
371.72 0.097971180260995
407.06 0.0907130190098807
434.38 0.0859897050542244
445.2 0.0799901355987584
477.9 0.0715965993489918
496.42 0.0696146704441919
526.46 0.0663450575891753
543.76 0.0629239805236287
589.5 0.059888873763534
602.58 0.0572509384676563
670.8 0.0532044118966826
701.96 0.0515719812598101
717.1 0.048967086557189
728.2 0.0471076579263354
769.6 0.0452595588551466
827.28 0.044045448944142
887.28 0.0415370012400482
924.92 0.0399187606305244
962.38 0.0385069428445061
988.38 0.0371059851146981
1034.58 0.0356491261194551
1127.64 0.034491019700124
1168.68 0.032553351792036
1199.16 0.0316641253440086
1232.96 0.0300647220596885
1289.2 0.0291158888250269
1349.18 0.0282911098764365
1415.18 0.0268325296856616
1455.4 0.0254323236706423
1555.92 0.0240242701369204
1663 0.0228876139443805
1774.14 0.0219853833859954
1920.78 0.0204482157725003
1957.1 0.0195389330916438
2167.12 0.0181679289101386
2220.52 0.0173604638071523
2371.72 0.0162573330567243
2480.84 0.015533732112357
2663.9 0.0147017754946076
2789.4 0.0140777958708976
2901.78 0.0137161341975242
3067.48 0.0129568624892111
3174.24 0.0125216451110658
3339.9 0.012102706107191
3435.78 0.0116367377597849
3504.8 0.0113651977463166
3604.74 0.0109640246455063
3718.7 0.0106060035276789
3885.76 0.0101351703015346
4076.34 0.00984517884542856
4294.68 0.00935331612172213
4464.18 0.00906735471221163
4612.5 0.00873172273731122
4969.58 0.00848109218652231
5134.52 0.00823794777829721
5294.96 0.00779042582756709
5534.32 0.00748509900272416
5820.28 0.00717278706431979
6110.38 0.00687361306914053
6431.96 0.00651441755173665
6791.46 0.00625485058239542
7221.72 0.00583014307564436
7633.88 0.0055420856083271
8232.18 0.0052369676802253
};
\addplot [
  draw=saddlebrown1356716,
  fill=saddlebrown1356716,
  forget plot,
  mark=*, mark size=1,
  only marks,
  draw opacity=0,
 fill opacity=0.5
]
table{%
x  y
532.48 0.304397222279069
582.08 0.286688153269027
588.36 0.281759125198257
591.48 0.274442701357363
597 0.265716761960643
601.64 0.25074821174796
618.72 0.244968453854984
623.06 0.240894744063962
633.32 0.218481308371691
639.1 0.210329421333192
649.06 0.19907856923048
668.64 0.184185507841204
684.26 0.173223980465054
693.56 0.152139485432754
709.16 0.141321895255203
736.4 0.130824997509604
758.04 0.121794770734404
792.58 0.107810839975017
813.1 0.0990856787576112
840.7 0.0939989892400019
861.96 0.0842279193748491
878.3 0.0763958569732237
888.06 0.070986919471293
904.92 0.0656564338693791
906.82 0.0628589186394916
911.76 0.0623255993178547
912.72 0.0640163595589718
927.02 0.0612990743266014
938.42 0.0600976107600948
954.9 0.0589287111966402
959.94 0.0586277075005384
963.1 0.0556500776669849
965.22 0.0574026683866941
965.44 0.0552253977539238
970.62 0.0562105937655071
972.64 0.0546584319530623
983.96 0.0543524018918829
997.18 0.0536070538211599
1004.38 0.0527349937274907
1009.18 0.052224790712897
1011.8 0.0513152845579338
1022.8 0.0508658306259448
1031.44 0.0497445372295701
1051.84 0.0488584940166709
1061.34 0.0473173249837277
1077.9 0.0464709387374728
1099 0.0457871312048541
1106.62 0.0450218300770056
1123.52 0.0445758893106944
1139.34 0.0437343045346661
1153.88 0.0429509761836559
1166.16 0.0423503393443485
1186.1 0.0417763593128315
1208.6 0.040741812309549
1229.26 0.0397856611642237
1268.06 0.0392161846946114
1289.32 0.0383881105864112
1325.24 0.0375560907870037
1381.18 0.0365972792258031
1412.08 0.0358227868551868
1437.7 0.0348273613098283
1494.24 0.0338063170289925
1538.54 0.0329787314830246
1576.7 0.0321156227558554
1632.66 0.0311194183222738
1683.3 0.0301306696783026
1706.66 0.0289160980903111
1746.78 0.0283312388231913
1788.94 0.0274828391176859
1858.14 0.0265860105376705
1930.32 0.0257088817003409
1986.94 0.0248486672997479
2067.68 0.0240235140303854
2121.76 0.0233359569600529
2199.78 0.0227358751785204
2264.36 0.0221507181742386
2342.82 0.0215833416121673
2415.58 0.0207238254642913
2515.54 0.0200145174412796
2583.28 0.0191961033426783
2639.56 0.0184318466052882
2736.12 0.0176739007191108
2886.56 0.0170891704131265
2982.66 0.0163500292055542
3136.08 0.015868005663986
3154.38 0.0153864320203464
3281.68 0.0149317621280108
3394.84 0.0146176343720682
3577.98 0.0141092249774065
3647.96 0.0136520882664115
3776.78 0.0131590793228492
3920.28 0.0126097496582266
4086.18 0.0122152030689076
4266.64 0.0117850729234692
4360.58 0.0112497513009928
4513.7 0.0109114150538168
4756.22 0.0105851757590359
4840.44 0.0101736214707256
5005.86 0.00972872004870676
5262.7 0.00944003116552999
};
\addplot [very thick, royalblue28108204]
table {%
33.52 0.971343630393969
120.967070707071 0.366131371855682
208.414141414141 0.241089692337927
295.861212121212 0.183963585210654
383.308282828283 0.150534545249998
470.755353535353 0.12833386612587
558.202424242424 0.112400676348564
645.649494949495 0.100347726271985
733.096565656566 0.0908759327663458
820.543636363636 0.0832143542692945
907.990707070707 0.076874923187141
995.437777777778 0.071532757166124
1082.88484848485 0.0669627461147499
1170.33191919192 0.0630037046201528
1257.77898989899 0.0595370140311907
1345.22606060606 0.0564733317306326
1432.67313131313 0.0537440118461098
1520.1202020202 0.0512953911180884
1607.56727272727 0.0490848786306115
1695.01434343434 0.0470782159110439
1782.46141414141 0.045247516658371
1869.90848484848 0.0435698380488103
1957.35555555556 0.0420261220818804
2044.80262626263 0.0406003993490838
2132.2496969697 0.0392791820489095
2219.69676767677 0.0380509955642936
2307.14383838384 0.0369060129046624
2394.59090909091 0.0358357664827448
2482.03797979798 0.0348329187110401
2569.48505050505 0.0338910778164037
2656.93212121212 0.0330046487616275
2744.37919191919 0.0321687116746633
2831.82626262626 0.0313789220154824
2919.27333333333 0.0306314280578127
3006.7204040404 0.0299228022655632
3094.16747474747 0.0292499838970778
3181.61454545455 0.0286102307415808
3269.06161616162 0.0280010783290096
3356.50868686869 0.0274203052911802
3443.95575757576 0.0268659038137848
3531.40282828283 0.0263360543233291
3618.8498989899 0.0258291037142438
3706.29696969697 0.0253435465491149
3793.74404040404 0.0248780087667965
3881.19111111111 0.0244312335148296
3968.63818181818 0.0240020687884255
4056.08525252525 0.0235894566116308
4143.53232323232 0.0231924235397543
4230.97939393939 0.0228100722976976
4318.42646464647 0.0224415743980672
4405.87353535354 0.0220861636070774
4493.32060606061 0.0217431301462639
4580.76767676768 0.0214118155346695
4668.21474747475 0.0210916079900793
4755.66181818182 0.0207819383195365
4843.10888888889 0.0204822762391841
4930.55595959596 0.0201921270717561
5018.00303030303 0.0199110287770564
5105.4501010101 0.0196385492767186
5192.89717171717 0.0193742840396174
5280.34424242424 0.0191178538986383
5367.79131313131 0.0188689030732273
5455.23838383838 0.0186270973753369
5542.68545454546 0.0183921225791336
5630.13252525253 0.0181636829372053
5717.5795959596 0.0179414998280662
5805.02666666667 0.0177253105215355
5892.47373737374 0.0175148670501211
5979.92080808081 0.0173099351758886
6067.36787878788 0.0171102934434779
6154.81494949495 0.0169157323109608
6242.26202020202 0.0167260533511412
6329.70909090909 0.0165410685166941
6417.15616161616 0.0163605994632395
6504.60323232323 0.0161844769250674
6592.0503030303 0.0160125401387742
6679.49737373737 0.0158446363105533
6766.94444444445 0.0156806201233144
6854.39151515152 0.0155203532801808
6941.83858585859 0.0153637040812573
7029.28565656566 0.0152105470308594
7116.73272727273 0.0150607624726644
7204.1797979798 0.014914236250484
7291.62686868687 0.0147708593925747
7379.07393939394 0.0146305278175915
7466.52101010101 0.0144931420604668
7553.96808080808 0.0143586070166484
7641.41515151515 0.0142268317032703
7728.86222222222 0.0140977290359587
7816.30929292929 0.0139712156200833
7903.75636363636 0.0138472115553715
7991.20343434344 0.0137256402528933
8078.65050505051 0.0136064282635067
8166.09757575758 0.0134895051169325
8253.54464646465 0.0133748031706934
8340.99171717172 0.0132622574682164
8428.43878787879 0.0131518056054523
8515.88585858586 0.0130433876054208
8603.33292929293 0.0129369458001314
8690.78 0.0128324247193807
};
\addplot [very thick, cadetblue80178158]
table {%
269.44 0.225723806531321
304.166666666667 0.209293073052946
338.893333333333 0.195682936817114
373.62 0.184186415788222
408.346666666667 0.17431976569085
443.073333333333 0.165739785552804
477.8 0.158195607332234
512.526666666667 0.15149920473267
547.253333333333 0.14550661500813
581.98 0.14010556920714
616.706666666667 0.135207102883108
651.433333333333 0.130739720619025
686.16 0.126645245937266
720.886666666667 0.122875811406257
755.613333333333 0.119391637252582
790.34 0.116159366066006
825.066666666667 0.113150796658037
859.793333333333 0.110341909020394
894.52 0.107712104668902
929.246666666667 0.105243608464309
963.973333333333 0.102920992963094
998.7 0.100730796781498
1033.42666666667 0.0986612158342021
1068.15333333333 0.0967018515990751
1102.88 0.0948435043996879
1137.60666666667 0.0930780025175951
1172.33333333333 0.0913980600398497
1207.06 0.0897971579168978
1241.78666666667 0.0882694438939381
1276.51333333333 0.0868096478858077
1311.24 0.0854130100636356
1345.96666666667 0.0840752194631208
1380.69333333333 0.0827923613475342
1415.42 0.0815608718915682
1450.14666666667 0.0803774990158949
1484.87333333333 0.0792392684124647
1519.6 0.0781434539690285
1554.32666666667 0.0770875519371449
1589.05333333333 0.0760692582979381
1623.78 0.0750864488694642
1658.50666666667 0.0741371617728441
1693.23333333333 0.0732195819345741
1727.96 0.0723320273521741
1762.68666666667 0.0714729368915703
1797.41333333333 0.0706408594189399
1832.14 0.0698344440984268
1866.86666666667 0.0690524317111881
1901.59333333333 0.0682936468714804
1936.32 0.0675569910325829
1971.04666666667 0.0668414361898424
2005.77333333333 0.0661460192004293
2040.5 0.065469836649887
2075.22666666667 0.0648120402045259
2109.95333333333 0.0641718323964029
2144.68 0.0635484627942374
2179.40666666667 0.0629412245193104
2214.13333333333 0.062349451070318
2248.86 0.0617725134254122
2283.58666666667 0.0612098173933643
2318.31333333333 0.0606608011890073
2353.04 0.060124933210923
2387.76666666667 0.0596017100017944
2422.49333333333 0.0590906543739932
2457.22 0.0585913136848617
2491.94666666667 0.0581032582478037
2526.67333333333 0.0576260798667644
2561.4 0.0571593904829659
2596.12666666667 0.0567028209239071
2630.85333333333 0.0562560197456474
2665.58 0.0558186521602858
2700.30666666667 0.0553903990413496
2735.03333333333 0.0549709560005094
2769.76 0.0545600325296718
2804.48666666667 0.054157351203066
2839.21333333333 0.0537626469344422
2873.94 0.0533756662849524
2908.66666666667 0.0529961668176908
2943.39333333333 0.0526239164952306
2978.12 0.0522586931168241
3012.84666666667 0.0519002837922263
3047.57333333333 0.0515484844493658
3082.3 0.0512030993733282
3117.02666666667 0.0508639407743321
3151.75333333333 0.0505308283825743
3186.48 0.0502035890679967
3221.20666666667 0.0498820564831886
3255.93333333333 0.0495660707277853
3290.66 0.0492554780328528
3325.38666666667 0.0489501304638738
3360.11333333333 0.0486498856410543
3394.84 0.0483546064757759
3429.56666666667 0.0480641609221048
3464.29333333333 0.0477784217423561
3499.02 0.0474972662857854
3533.74666666667 0.0472205762795503
3568.47333333333 0.0469482376311487
3603.2 0.0466801402415988
3637.92666666667 0.0464161778286794
3672.65333333333 0.0461562477595978
3707.38 0.0459002508924993
};
\addplot [very thick, chocolate21910927]
table {%
33.46 1.02791458594879
121.997575757576 0.389128586612746
210.535151515152 0.273667965019851
299.072727272727 0.2221985611229
387.610303030303 0.192244507271539
476.147878787879 0.172326375903938
564.685454545455 0.157970945392641
653.22303030303 0.147050430805012
741.760606060606 0.138414617698462
830.298181818182 0.131383415237399
918.835757575758 0.125527025027741
1007.37333333333 0.120559478870369
1095.91090909091 0.116282536462709
1184.44848484848 0.112554090965966
1272.98606060606 0.10926939464395
1361.52363636364 0.106349396269972
1450.06121212121 0.103733220824964
1538.59878787879 0.101373163322766
1627.13636363636 0.0992312633340739
1715.67393939394 0.0972769041739735
1804.21151515152 0.095485094314592
1892.74909090909 0.0938352138770453
1981.28666666667 0.0923100849005868
2069.82424242424 0.0908952712963605
2158.36181818182 0.0895785445206275
2246.89939393939 0.0883494706641622
2335.43696969697 0.0871990877487482
2423.97454545455 0.0861196509040071
2512.51212121212 0.0851044292250129
2601.0496969697 0.0841475424033906
2689.58727272727 0.0832438282742595
2778.12484848485 0.0823887346166831
2866.66242424242 0.0815782301448146
2955.2 0.0808087308055208
3043.73757575758 0.0800770383758476
3132.27515151515 0.0793802890135373
3220.81272727273 0.0787159099145056
3309.3503030303 0.078081582614383
3397.88787878788 0.0774752117668718
3486.42545454546 0.0768948984614988
3574.96303030303 0.0763389173232924
3663.50060606061 0.0758056967787674
3752.03818181818 0.0752938019851242
3840.57575757576 0.074801920009392
3929.11333333333 0.0743288469163422
4017.65090909091 0.0738734764821906
4106.18848484849 0.0734347902983265
4194.72606060606 0.0730118490677966
4283.26363636364 0.0726037849288169
4371.80121212121 0.0722097946655333
4460.33878787879 0.0718291336877043
4548.87636363636 0.0714611106787772
4637.41393939394 0.0711050828266636
4725.95151515152 0.0707604515639189
4814.48909090909 0.0704266587544452
4903.02666666667 0.0701031832726045
4991.56424242424 0.0697895379280395
5080.10181818182 0.0694852666957851
5168.63939393939 0.0691899422165935
5257.17696969697 0.0689031635369587
5345.71454545455 0.0686245540622225
5434.25212121212 0.06835375969949
5522.7896969697 0.0680904471699632
5611.32727272727 0.0678343024727764
5699.86484848485 0.0675850294845707
5788.40242424242 0.0673423486808951
5876.94 0.0671059959671464
5965.47757575758 0.0668757216081568
6054.01515151515 0.0666512892467716
6142.55272727273 0.0664324750028311
6231.0903030303 0.0662190666449061
6319.62787878788 0.0660108628279689
6408.16545454545 0.0658076723909016
6496.70303030303 0.0656093137083862
6585.24060606061 0.0654156140922858
6673.77818181818 0.0652264092381234
6762.31575757576 0.065041542712711
6850.85333333333 0.064860865479372
6939.39090909091 0.0646842354575494
7027.92848484849 0.0645115171139037
7116.46606060606 0.0643425810822826
7205.00363636364 0.0641773038101892
7293.54121212121 0.0640155672296011
7382.07878787879 0.0638572584501863
7470.61636363636 0.0637022694731443
7559.15393939394 0.0635504969240576
7647.69151515152 0.0634018418032825
7736.22909090909 0.0632562092525407
7824.76666666667 0.0631135083364844
7913.30424242424 0.0629736518381182
8001.84181818182 0.062836556067053
8090.37939393939 0.062702140679655
8178.91696969697 0.062570328510229
8267.45454545455 0.0624410454124474
8355.99212121212 0.0623142201103016
8444.5296969697 0.0621897840579077
8533.06727272727 0.0620676713075534
8621.60484848485 0.061947818385423
8710.14242424242 0.0618301641744775
8798.68 0.0617146498040112
};
\addplot [very thick, purple11522131]
table {%
107.5 0.430465582862106
194.229898989899 0.35743568940578
280.959797979798 0.314604587296576
367.689696969697 0.285053666815582
454.419595959596 0.262878617116164
541.149494949495 0.245350045740973
627.879393939394 0.230992537937748
714.609292929293 0.218923244888951
801.339191919192 0.208574537346211
888.069090909091 0.19956131439034
974.79898989899 0.191611161278279
1061.52888888889 0.18452481563072
1148.25878787879 0.178152467112893
1234.98868686869 0.172378871664273
1321.71858585859 0.167113633948612
1408.44848484848 0.16228465374459
1495.17838383838 0.157833581351809
1581.90828282828 0.153712589294938
1668.63818181818 0.149882030254426
1755.36808080808 0.14630870607526
1842.09797979798 0.142964567113609
1928.82787878788 0.139825720387255
2015.55777777778 0.136871663083721
2102.28767676768 0.134084683047052
2189.01757575758 0.131449384703515
2275.74747474747 0.128952310410379
2362.47737373737 0.126581635232442
2449.20727272727 0.124326918819849
2535.93717171717 0.122178902124471
2622.66707070707 0.120129339643421
2709.39696969697 0.118170860047513
2796.12686868687 0.116296849664781
2882.85676767677 0.114501354500017
2969.58666666667 0.112778997389359
3056.31656565657 0.111124907591489
3143.04646464646 0.109534660658983
3229.77636363636 0.108004226854927
3316.50626262626 0.106529926710213
3403.23616161616 0.105108392577556
3489.96606060606 0.103736535245264
3576.69595959596 0.102411514839252
3663.42585858586 0.101130715374836
3750.15575757576 0.0998917224273523
3836.88565656566 0.0986923034781102
3923.61555555556 0.0975303905635809
4010.34545454546 0.0964040649143693
4097.07535353535 0.0953115433188599
4183.80525252525 0.0942511659864795
4270.53515151515 0.0932213857188344
4357.26505050505 0.0922207582247952
4443.99494949495 0.0912479334389291
4530.72484848485 0.0903016477222996
4617.45474747475 0.0893807168412244
4704.18464646465 0.0884840296336203
4790.91454545455 0.0876105422844942
4877.64444444445 0.0867592731423152
4964.37434343434 0.0859292980167022
5051.10424242424 0.0851197459053222
5137.83414141414 0.0843297951043149
5224.56404040404 0.0835586696620911
5311.29393939394 0.0828056361411397
5398.02383838384 0.082070000656625
5484.75373737374 0.0813511061641576
5571.48363636364 0.0806483299722662
5658.21353535354 0.0799610814578299
5744.94343434344 0.0792887999651332
5831.67333333333 0.0786309528713026
5918.40323232323 0.077987033802731
6005.13313131313 0.0773565609887201
6091.86303030303 0.0767390757400019
6178.59292929293 0.0761341410410679
6265.32282828283 0.0755413402463526
6352.05272727273 0.0749602758713138
6438.78262626263 0.0743905684703296
6525.51252525253 0.0738318555941229
6612.24242424242 0.0732837908201177
6698.97232323232 0.0727460428497598
6785.70222222222 0.0722182946673891
6872.43212121212 0.0717002427557535
6959.16202020202 0.0711915963636994
7045.89191919192 0.0706920768219757
7132.62181818182 0.0702014169034522
7219.35171717172 0.0697193602243765
7306.08161616162 0.0692456606835855
7392.81151515152 0.0687800819368558
7479.54141414141 0.0683223969038127
7566.27131313131 0.0678723873050373
7653.00121212121 0.067429843227203
7739.73111111111 0.0669945627142551
7826.46101010101 0.0665663513828047
7913.19090909091 0.0661450220600568
7999.92080808081 0.0657303944427256
8086.65070707071 0.0653222947755105
8173.38060606061 0.0649205555478183
8260.11050505051 0.064525015207519
8346.84040404041 0.0641355178906117
8433.5703030303 0.0637519131657645
8520.3002020202 0.0633740557927705
8607.0301010101 0.0630018054940276
8693.76 0.0626350267382229
};
\addplot [very thick, black18]
table {%
33.52 0.754487895399919
117.621414141414 0.419962475316073
201.722828282828 0.310443935667809
285.824242424242 0.251310109226916
369.925656565656 0.213180941558186
454.027070707071 0.186143073369503
538.128484848485 0.165784510053839
622.229898989899 0.149804830027715
706.331313131313 0.136872730881886
790.432727272727 0.126158198474004
874.534141414141 0.117113916092541
958.635555555555 0.1093628103653
1042.73696969697 0.102635772940125
1126.83838383838 0.096735093274769
1210.9397979798 0.0915119410430508
1295.04121212121 0.0868519404316541
1379.14262626263 0.0826656141358836
1463.24404040404 0.0788818691422331
1547.34545454545 0.0754434443411975
1631.44686868687 0.072303659164062
1715.54828282828 0.0694240463665444
1799.6496969697 0.066772598802261
1883.75111111111 0.06432245088534
1967.85252525252 0.0620508731789274
2051.95393939394 0.0599384960969879
2136.05535353535 0.0579687036433809
2220.15676767677 0.0561271549878223
2304.25818181818 0.0544014032968228
2388.3595959596 0.0527805893634408
2472.46101010101 0.0512551933452409
2556.56242424242 0.049816832065461
2640.66383838384 0.0484580923500381
2724.76525252525 0.0471723930948826
2808.86666666667 0.0459538704109472
2892.96808080808 0.0447972814369194
2977.06949494949 0.0436979233515376
3061.17090909091 0.0426515648382976
3145.27232323232 0.0416543878111835
3229.37373737374 0.0407029376420429
3313.47515151515 0.0397940804683539
3397.57656565656 0.0389249664265933
3481.67797979798 0.0380929978677567
3565.77939393939 0.037295801780221
3649.88080808081 0.0365312057804815
3733.98222222222 0.0357972171415176
3818.08363636364 0.0350920044171311
3902.18505050505 0.0344138812928292
3986.28646464646 0.0337612923529704
4070.38787878788 0.033132800502568
4154.48929292929 0.0325270758223565
4238.59070707071 0.0319428856690938
4322.69212121212 0.031379085860868
4406.79353535353 0.0308346128104153
4490.89494949495 0.0303084764889581
4574.99636363636 0.0297997541194955
4659.09777777778 0.0293075845123531
4743.19919191919 0.0288311629675602
4827.30060606061 0.0283697366786237
4911.40202020202 0.0279226005807929
4995.50343434343 0.0274890935942075
5079.60484848485 0.0270685952185701
5163.70626262626 0.0266605224413676
5247.80767676768 0.0262643269262993
5331.90909090909 0.0258794924525799
5416.0105050505 0.025505532579254
5500.11191919192 0.0251419885116761
5584.21333333333 0.0247884271499322
5668.31474747475 0.0244444393012693
5752.41616161616 0.024109638040596
5836.51757575758 0.0237836572048745
5920.61898989899 0.0234661500087561
6004.7204040404 0.0231567877701693
6088.82181818182 0.0228552587357559
6172.92323232323 0.0225612669971062
6257.02464646465 0.0222745314896696
6341.12606060606 0.0219947850670414
6425.22747474747 0.0217217736440586
6509.32888888889 0.0214552554027817
6593.4303030303 0.0211950000560214
6677.53171717172 0.0209407881635796
6761.63313131313 0.0206924104968374
6845.73454545454 0.0204496674477291
6929.83595959596 0.0202123684785119
7013.93737373737 0.0199803316090698
7098.03878787879 0.0197533829387841
7182.1402020202 0.0195313562002717
7266.24161616161 0.0193140923425292
7350.34303030303 0.0191014391412374
7434.44444444444 0.0188932508341763
7518.54585858586 0.0186893877798731
7602.64727272727 0.0184897161377697
7686.74868686869 0.0182941075683347
7770.8501010101 0.0181024389516797
7854.95151515151 0.017914592123355
7939.05292929293 0.0177304536261089
8023.15434343434 0.0175499144764921
8107.25575757576 0.0173728699452778
8191.35717171717 0.0171992193507487
8275.45858585859 0.0170288658639768
8359.56 0.0168617163252883
};
\addplot [very thick, darkgray153]
table {%
33.52 1.45641984821827
116.334747474747 0.356360326080105
199.149494949495 0.198725187420234
281.964242424242 0.137267973998081
364.77898989899 0.104780872115076
447.593737373737 0.0847487509244657
530.408484848485 0.0711819808648222
613.223232323232 0.0613934617229122
696.03797979798 0.0540011162514459
778.852727272727 0.0482224595876993
861.667474747475 0.043581685558453
944.482222222222 0.0397730203228402
1027.29696969697 0.0365910914042879
1110.11171717172 0.0338928926419672
1192.92646464646 0.0315758063993955
1275.74121212121 0.0295642997427046
1358.55595959596 0.0278015499100981
1441.37070707071 0.0262439936379815
1524.18545454545 0.0248576756389799
1607.0002020202 0.0236157399511502
1689.81494949495 0.0224966677785725
1772.6296969697 0.0214830150632117
1855.44444444444 0.0205604920010021
1938.25919191919 0.0197172811686636
2021.07393939394 0.0189435251225866
2103.88868686869 0.0182309363063919
2186.70343434343 0.0175724965244585
2269.51818181818 0.0169622228833721
2352.33292929293 0.0163949836664812
2435.14767676768 0.0158663521446162
2517.96242424242 0.0153724895097589
2600.77717171717 0.0149100503824894
2683.59191919192 0.0144761059743135
2766.40666666667 0.014068081173612
2849.22141414141 0.0136837026985339
2932.03616161616 0.0133209561107456
3014.85090909091 0.0129780499724988
3097.66565656566 0.0126533857996281
3180.4804040404 0.012345532745865
3263.29515151515 0.0120532061715865
3346.1098989899 0.0117752494190145
3428.92464646465 0.0115106182478112
3511.73939393939 0.0112583674887544
3594.55414141414 0.0110176395552642
3677.36888888889 0.0107876545178893
3760.18363636364 0.010567701499165
3842.99838383838 0.0103571311883523
3925.81313131313 0.0101553493096157
4008.62787878788 0.0099618109048843
4091.44262626263 0.00977601531524465
4174.25737373737 0.00959750176326446
4257.07212121212 0.00942584545392545
4339.88686868687 0.00926065412448519
4422.70161616162 0.00910156498408644
4505.51636363636 0.00894824199268434
4588.33111111111 0.00880037343618486
4671.14585858586 0.00865766976083441
4753.96060606061 0.00851986163508018
4836.77535353535 0.00838669821149669
4919.5901010101 0.00825794556508389
5002.40484848485 0.0081333852873961
5085.2195959596 0.0080128132186512
5168.03434343434 0.00789603830226922
5250.84909090909 0.00778288154825999
5333.66383838384 0.0076731750935765
5416.47858585859 0.00756676134900873
5499.29333333333 0.00746349222345618
5582.10808080808 0.00736322841750881
5664.92282828283 0.00726583877921426
5747.73757575758 0.00717119971573379
5830.55232323232 0.007079194655308
5913.36707070707 0.00698971355458129
5996.18181818182 0.00690265244688291
6078.99656565657 0.00681791302754443
6161.81131313131 0.00673540227275669
6244.62606060606 0.00665503208884156
6327.44080808081 0.00657671898914238
6410.25555555556 0.00650038379602695
6493.0703030303 0.00642595136575372
6575.88505050505 0.00635335033417905
6658.6997979798 0.00628251288148554
6741.51454545455 0.00621337451429098
6824.32929292929 0.00614587386365668
6907.14404040404 0.00607995249765741
6989.95878787879 0.00601555474730168
7072.77353535354 0.00595262754470499
7155.58828282828 0.00589112027252112
7238.40303030303 0.00583098462372719
7321.21777777778 0.00577217447094071
7404.03252525253 0.00571464574452065
7486.84727272727 0.00565835631877046
7569.66202020202 0.00560326590562145
7652.47676767677 0.00554933595522841
7735.29151515152 0.00549652956295861
7818.10626262626 0.00544481138229864
7900.92101010101 0.00539414754324462
7983.73575757576 0.0053445055757764
8066.55050505051 0.00529585433804989
8149.36525252525 0.00524816394897136
8232.18 0.00520140572484439
};
\addplot [very thick, saddlebrown1356716]
table {%
532.48 0.296996489182299
580.26 0.233235592255375
628.04 0.188293343038197
675.82 0.15554283880814
723.6 0.130998891021267
771.38 0.112161343851696
819.16 0.0974039545598236
866.94 0.0856353752430239
914.72 0.0761030060808502
962.5 0.0682752773535391
1010.28 0.0617686905367114
1058.06 0.0563012931694032
1105.84 0.0516622469458247
1153.62 0.0476914635298503
1201.4 0.0442656944382635
1249.18 0.0412888508293688
1296.96 0.0386851517024592
1344.74 0.0363941983100993
1392.52 0.0343673825431506
1440.3 0.032565233486799
1488.08 0.0309554332273771
1535.86 0.0295113163915061
1583.64 0.0282107236155115
1631.42 0.0270351169276186
1679.2 0.0259688910096791
1726.98 0.024998832408612
1774.76 0.0241136915349971
1822.54 0.0233038413933743
1870.32 0.0225610035549834
1918.1 0.021878026665664
1965.88 0.0212487062973998
2013.66 0.020667637560032
2061.44 0.020130093840741
2109.22 0.0196319265102221
2157 0.0191694815524628
2204.78 0.0187395299306547
2252.56 0.0183392091611088
2300.34 0.0179659740784186
2348.12 0.0176175551742261
2395.9 0.0172919232052609
2443.68 0.0169872590136875
2491.46 0.0167019276991551
2539.24 0.0164344564386041
2587.02 0.0161835153755084
2634.8 0.0159479011014363
2682.58 0.0157265223347158
2730.36 0.01551838746757
2778.14 0.0153225937074308
2825.92 0.0151383175826746
2873.7 0.0149648066196692
2921.48 0.0148013720282776
2969.26 0.0146473822580461
3017.04 0.0145022573081598
3064.82 0.0143654636916529
3112.6 0.0142365099689321
3160.38 0.0141149427779071
3208.16 0.0140003432983267
3255.94 0.013892324096627
3303.72 0.0137905263049724
3351.5 0.0136946170944352
3399.28 0.0136042874075989
3447.06 0.0135192499204197
3494.84 0.0134392372070899
3542.62 0.013364000084988
3590.4 0.0132933061196807
3638.18 0.0132269382724242
3685.96 0.0131646936747563
3733.74 0.0131063825166259
3781.52 0.0130518270361191
3829.3 0.0130008606002383
3877.08 0.0129533268674148
3924.86 0.0129090790234947
3972.64 0.0128679790838743
4020.42 0.01282989725527
4068.2 0.0127947113513309
4115.98 0.0127623062569235
4163.76 0.0127325734364781
4211.54 0.0127054104822702
4259.32 0.012680720698945
4307.1 0.0126584127209727
4354.88 0.0126384001600618
4402.66 0.0126206012798574
4450.44 0.0126049386955174
4498.22 0.0125913390959981
4546 0.0125797329870927
4593.78 0.0125700544534523
4641.56 0.0125622409379917
4689.34 0.0125562330372295
4737.12 0.0125519743112489
4784.9 0.012549411107089
4832.68 0.0125484923944786
4880.46 0.012549169612934
4928.24 0.0125513965293149
4976.02 0.0125551291050286
5023.8 0.0125603253721307
5071.58 0.0125669453176434
5119.36 0.0125749507754681
5167.14 0.0125843053253219
5214.92 0.0125949741981759
5262.7 0.0126069241877179
};
\addplot [draw=black, fill=black, mark=x, very thick, mark size=2.5pt, only marks]
table{%
x  y
130.88 0.563302347042077
532.48 0.304397222279069
2163.2 0.150974298879811
8693.76 0.0628423491256762
};
