# Supplementary material for: Swarm Reinforcement Learning For Adaptive Mesh Refinement
Source: arXiv:2304.00818 source file (2023-10-09)
Supplement: Supplementary file 13 [file group_additional_metrics_r2.tex]

\nextgroupplot[
ylabel shift = -0.2cm,
title style={yshift=-0.2cm},
height=4.5cm,
width=0.50\textwidth,
ylabel={Top $0.1\,\%$ Error},
xlabel={\empty},
title={Poisson's Equation},
clip marker paths=true,
legend cell align={left},
legend style={fill opacity=0.8, draw opacity=1, text opacity=1, draw=lightgray204},
log basis y={10},
tick align=outside,
tick pos=left,
x grid style={darkgray176},
xmajorgrids,
xmin=-425.719, xmax=9421.899,
xtick style={color=black},
xtick={-2000,0,2000,4000,6000,8000,10000},
xticklabels={-2.0,0.0,2.0,4.0,6.0,8.0,10.0},
y grid style={darkgray176},
ymajorgrids,
ymin=0.00252051809300322, ymax=1.32965380294905,
ymode=log,
ytick style={color=black},
ytick={0.0001,0.001,0.01,0.1,1,10,100},
yticklabels={
  \(\displaystyle {10^{-4}}\),
  \(\displaystyle {10^{-3}}\),
  \(\displaystyle {10^{-2}}\),
  \(\displaystyle {10^{-1}}\),
  \(\displaystyle {10^{0}}\),
  \(\displaystyle {10^{1}}\),
  \(\displaystyle {10^{2}}\)
}
]
\addplot [
  draw=royalblue28108204,
  fill=royalblue28108204,
  forget plot,
  mark=*, mark size=1,
  only marks,
  draw opacity=0,
 fill opacity=0.5
]
table{%
x  y
219.44 0.144943315012232
253.72 0.135063787446789
264.04 0.121975720793038
276.92 0.116228235908273
280.58 0.110562874588746
304.86 0.114871093976589
309.34 0.11423090203441
310.42 0.120666844010388
321.76 0.158880317511244
326.62 0.0999213668833362
381.9 0.08384890821968
391.58 0.077786853057476
432.4 0.0745352397856568
435.4 0.0787505973314633
439.36 0.0897552404983674
460.02 0.0740149868397821
467.2 0.0759026471800116
513.26 0.0695317573237953
548.58 0.0593945930250203
550.98 0.0627135386379849
552.82 0.0677099252892207
569.98 0.0684196320114038
575.02 0.0594331013039196
586.42 0.0604078720519802
594.7 0.0578275499983459
604.74 0.0563793962247504
616.96 0.0638000261222975
636.66 0.0527699320251235
648.96 0.0576258902302889
667.72 0.0518169242231017
680.38 0.0503845411649547
721.5 0.05222069093053
728.42 0.051379274350617
735.12 0.0506161945418661
744.48 0.0447839749920601
744.64 0.0455927517635886
749.68 0.0442318722879005
750.54 0.0484083829383322
814.88 0.0489321696618264
880.52 0.0431433188626397
900 0.0476579667418267
959.06 0.0324328683876128
1000.06 0.0314108130798124
1055.58 0.0297235192381075
1057.24 0.0303554088997409
1099.06 0.029104061779677
1123.62 0.0286557876962508
1124.12 0.0273955885060394
1187.06 0.025234069387518
1189.3 0.0267990724323369
1263.58 0.0264733075124408
1283.62 0.0264660506501021
1283.68 0.0237249464731312
1327.76 0.021312907985604
1341.18 0.0218229442697872
1398.48 0.0281344099091287
1414.68 0.0239628701671583
1482.28 0.0222105815934702
1589.06 0.0208293374482413
1685 0.0229308508601196
1713.06 0.0173558589954624
1739.68 0.0179029435672331
1822.1 0.0168285010321951
1838.52 0.0164269473963722
1867.06 0.0167997084733952
1947.9 0.0149075979280466
1953.1 0.0145798590104653
2080.9 0.0143145031796558
2218.72 0.013806012277804
2227.28 0.0149100525289481
2251.12 0.0142204727999416
2266 0.0147963866109884
2316.3 0.0121604657779952
2364.92 0.0120116800785737
2380.18 0.0124819339843187
2441.04 0.0131830177781086
2442.48 0.011906946326896
2479.4 0.0120114408727239
2526.6 0.0117800198170452
2726.56 0.0111687373529929
2842.12 0.0101815775077515
3139.84 0.0111766226158419
3446.8 0.00848818161990444
3638.76 0.00764112320263953
3689.8 0.00810204964084976
4066.44 0.00698693368378327
4107.14 0.00664354334527057
4240.6 0.0073792628889566
4343.22 0.00768629133570437
4397.24 0.00732712892328073
4501.08 0.00677250298491408
4667.26 0.00604493063659663
5928.04 0.00456256999981585
6163.7 0.00390589640264517
6435.52 0.00412076869528313
6826.82 0.00369439705450541
7019.62 0.00390175920699876
7050.18 0.00423886433598527
7544.28 0.00429553928223084
7854.52 0.00383995964955601
};
\addplot [
  draw=cadetblue80178158,
  fill=cadetblue80178158,
  forget plot,
  mark=*, mark size=1,
  only marks,
  draw opacity=0,
 fill opacity=0.5
]
table{%
x  y
235.24 0.296444164542315
257.6 0.250988693267948
266.36 0.290421819487767
274.1 0.240873438642678
276.6 0.351883719282123
293.48 0.192258890836193
295.44 0.207299629460545
309.3 0.206377008149073
333.3 0.30955017926646
348.28 0.352479604139424
395.76 0.326090209019444
424.72 0.139205093978138
442.82 0.112716795815398
447.86 0.164858566131203
495.5 0.163428105891043
533.66 0.163748430969141
565.44 0.236088805970188
582.84 0.122504237366658
634.02 0.183517887713767
659.12 0.243789901900965
671.76 0.12414884750664
684.08 0.0931305248337605
694.72 0.116704822435766
698.34 0.221972056116065
713.92 0.132298398095599
765.18 0.0864562454021844
785.52 0.113951632751975
788.5 0.181185521148105
798.32 0.323010302935586
875.62 0.53116629569682
881.52 0.571433451922073
952.64 0.0813625299245541
953.16 0.125039527699667
964.52 0.0733105538850519
964.82 0.130367054479434
1000.92 0.0985687211618715
1006 0.092792495277612
1055.92 0.0938687026417912
1142.22 0.0670876938133656
1155.94 0.0929813177966107
1203.38 0.522149036062597
1206.96 0.0673343877077447
1242.58 0.156716982415953
1265.82 0.0789295073665014
1317.42 0.0895388940451156
1340.28 0.169106355539184
1474.38 0.511954666435441
1492.48 0.0465769150071352
1495.42 0.104104970380832
1505.24 0.0791199074094508
1570 0.068020796208626
1596.12 0.35773207122291
1625.54 0.072087556430034
1694.78 0.0976222185380507
1698.2 0.0819529098978446
1775.42 0.0457791144944519
1776.42 0.0483247462089244
1967.42 0.0443915579236676
1970.72 0.0482314224973151
2015.62 0.0571670445393776
2034.78 0.124982831341729
2149.06 0.0442945204496035
2227.18 0.0360047101437704
2284.46 0.059149180687969
2306.78 0.123001832008815
2342.5 0.0310173353761501
2424.16 0.575194065834085
2439.08 0.0730172063009628
2484.8 0.0620788051221046
2491.82 0.0357296175407991
2505.68 0.0313217557281276
2512.38 0.0391161410109745
2575.44 0.0518434611316117
2736.88 0.0632424486222121
2750.2 0.147540581761354
2771.74 0.0399599693764378
2803 0.036496951292338
2810.54 0.035431985779636
2829.18 0.366339933833245
2894.44 0.0359860849615794
2947.76 0.0794133546787386
2949.72 0.157567955715677
2961.5 0.0690749340839244
2976.14 0.112161985721538
3096.24 0.162261262432002
3144.04 0.0379850998081007
3174.96 0.0452559971658699
3179.52 0.295089689792815
3276.54 0.0263813574859573
3298.1 0.0228847095864752
3301.58 0.0377823658508824
3337.66 0.0296143928735442
3341.84 0.0293873535888986
3378.24 0.0271136167292589
3461.62 0.0239404544491837
3712.1 0.276386846460207
3722.84 0.0227357968174522
3725.54 0.0708257073846199
3871.68 0.0423020110246673
4048.68 0.0759216981537061
};
\addplot [
  draw=chocolate21910927,
  fill=chocolate21910927,
  forget plot,
  mark=*, mark size=1,
  only marks,
  draw opacity=0,
 fill opacity=0.5
]
table{%
x  y
21.86 0.999999999999927
22.2 0.999999999999929
22.46 0.999999999999934
22.46 0.999999999999934
22.46 0.999999999999934
22.46 0.999999999999934
22.5 0.999999999999934
22.56 0.999999999999935
22.64 0.999999999999934
22.66 0.999999999999936
22.66 0.999999999999936
22.66 0.999999999999936
22.66 0.999999999999936
22.66 0.999999999999936
22.66 0.999999999999936
22.66 0.999999999999936
22.66 0.999999999999936
22.66 0.999999999999936
22.66 0.999999999999936
22.66 0.999999999999936
22.66 0.999999999999936
22.66 0.999999999999936
22.66 0.999999999999936
22.66 0.999999999999936
22.66 0.999999999999936
22.66 0.999999999999936
22.66 0.999999999999933
22.66 0.999999999999936
22.66 0.999999999999936
22.66 0.999999999999936
22.66 0.999999999999936
22.66 0.999999999999936
22.66 0.999999999999936
22.66 0.999999999999936
22.66 0.999999999999936
22.66 0.999999999999936
22.66 0.999999999999936
22.66 0.999999999999936
22.66 0.999999999999936
22.66 0.999999999999936
25.08 0.997276757207327
30.06 0.991513747074262
33.78 0.964954450024066
76.92 0.912448702535122
98.3 0.519306531503057
136.64 0.371321309620658
139.8 0.387615644597802
139.98 0.890453665830885
159.56 0.330066175574826
207.44 0.572693520631197
222.76 0.317532897620117
266.3 0.37454086907836
268.72 0.306075867886978
290.96 0.339911421393067
292.22 0.217791774022915
342.12 0.319622138081555
343.9 0.620175465426788
362.86 0.193297756938743
396.96 0.225302620156313
403.12 0.112877542138478
404.74 0.230389550510629
428.58 0.301208874589376
541.12 0.447745940341116
546.56 0.76157590066463
656.94 0.118475569439025
714.8 0.089566798009849
718.16 0.129207484599479
719.82 0.0990156119182967
751.34 0.273496270072129
1144.26 0.2923179620922
1234.4 0.0644516228271708
1245.46 0.0667442558656033
1320.64 0.0648467022346733
1333.36 0.0401374228754001
1357.92 0.089845676804021
1641.52 0.277102646552267
1814.76 0.467130154977931
1854.84 0.120679292449578
2050.82 0.0387547016208826
2127.6 0.0423799354351745
2312.18 0.554342342421127
3274 0.0209453381290893
3688.92 0.0647134616305028
3791.06 0.0574271719675217
4690.88 0.0432569515303263
4714.86 0.0103957688163848
4960.8 0.0134003082346279
8218.76 0.00714301137004513
};
\addplot [draw=purple11522131, fill=purple11522131, forget plot, mark=*, mark size=1, only marks, draw opacity=0,
 fill opacity=0.5]
table{%
x  y
80.24 0.68799074441649
81.48 0.651277667432901
86.82 0.672534412077198
107.5 0.466493143315974
119.46 0.486971060442545
122.44 0.443741368311865
124.34 0.575952128568215
125 0.450054388239001
134.3 0.470590673510439
189.2 0.405024738507333
206.36 0.396907563546202
211.82 0.385961163853044
239.22 0.382444984461522
289.98 0.379848140100621
302.38 0.338661501733987
320.08 0.285591878468831
338.06 0.299326710949262
340.16 0.299977364773732
342.3 0.172483102304328
346.82 0.293197332011277
348.66 0.287175509868334
348.86 0.295420242468826
349.44 0.289841560897337
349.78 0.287659846040053
353.82 0.279798414811555
361.96 0.257259313961172
365.46 0.277182018064868
369.04 0.270266183023514
379.3 0.221296660034848
383.96 0.220637426606393
388.46 0.23271173684209
411.08 0.227323894676635
420.8 0.191815896438625
445 0.279641784770674
488.72 0.194528930129648
489.88 0.160131768310577
512.92 0.17333250514612
563.5 0.20169152325754
590.4 0.163560494467941
797.8 0.122611718990094
834.88 0.135085719538793
1223.5 0.117970837632403
1303.78 0.111424049887386
1333.96 0.116427237023529
1340.08 0.119974293264521
1400.82 0.111004517982763
1432.72 0.110960555812464
1439.92 0.115256667823096
1444.68 0.110995845514989
1449.2 0.105785927369463
1459.12 0.113114495269336
1459.2 0.112179289791658
1459.38 0.112108373550698
1460.12 0.105438020697108
1461.46 0.106732783175285
1465.96 0.110932276837285
1465.98 0.110924945038416
1466.88 0.110924073157526
1473.76 0.105886282041797
1480.54 0.104196903626139
1483.84 0.104517444742208
1513.46 0.0955336454851905
1513.88 0.0858645089199863
1551.96 0.0849296936848488
1579.32 0.0862443540179776
1660.16 0.0590835109350209
1939.38 0.0616893241907718
1981.56 0.0599525612475801
2019.96 0.0697942845033955
2128.52 0.0820851521011671
2196.34 0.0569407472809766
2576.26 0.0292192838220514
3286.08 0.0436024219549258
3371.78 0.0347412210732334
3529 0.0337328295735746
3602.92 0.0355800024508535
3790.2 0.0313221847100689
3979.52 0.0355628650145878
4716.4 0.0403795418011725
5726.56 0.0352832907138029
5758.06 0.0332925956408714
5759.78 0.0332925453224229
5759.8 0.0332925444887448
5760 0.0332925439690838
5760 0.0332925439690838
5760 0.0332925439690838
5760 0.0332925439690838
5760 0.0332925439690838
5760 0.0332925439690838
5760 0.0332925439690838
5760 0.0332925439690838
5760 0.0332925439690838
5760 0.0332925439690838
5760 0.0332925439690838
5760 0.0332925439690838
5760 0.0332925439690838
5760 0.0332925439690838
5760 0.0332925439690838
5760 0.0332925439690838
5760 0.0332925439690838
};
\addplot [draw=black18, fill=black18, forget plot, mark=*, mark size=1, only marks, draw opacity=0,
 fill opacity=0.5]
table{%
x  y
22.66 0.999999999999936
85.1 0.340930318732509
85.96 0.333739230671782
87.38 0.324555994855364
89.96 0.328816049745124
91.96 0.32327189587101
93.86 0.316949861078163
96.14 0.315292987934514
99.06 0.30349339057922
102.2 0.294568344807327
105.82 0.27771527522461
106.14 0.283139482667051
108.54 0.268093367453753
112.12 0.259484124864678
115.4 0.257040014382844
118.46 0.252716187662168
121.62 0.240715985779485
125.48 0.238801014262909
128.9 0.237922337737465
134.96 0.224243630619714
139.88 0.216296590510095
140.42 0.215811502737629
143.92 0.212775549481674
147.62 0.208611358020482
151.7 0.208242659956059
159.72 0.203005207982871
163.02 0.192910681043621
163.76 0.194976483511209
168.34 0.187694413818644
172.24 0.179981147032624
183.24 0.17865332933649
183.5 0.173214361957619
196.68 0.16712218987477
209.02 0.159838477096969
210.4 0.155073404849216
219.36 0.149428432649749
231.58 0.151094263677121
244.98 0.145606924857294
250.98 0.141728413004881
257.32 0.136299866231376
278.58 0.129934566674791
290.34 0.124325397375082
308.16 0.11886456525884
324.9 0.113290174264668
337.94 0.109555950174971
358.3 0.102610587428143
363.62 0.102939940338396
406.6 0.0956071709985471
411.18 0.0919543287273845
432.74 0.0844575996217349
450.54 0.0815570211818348
462.72 0.0803324633099801
491.42 0.0756748715840035
501.72 0.0724529894525083
535.34 0.0699832296910562
561.9 0.0660379319904319
597.86 0.0647254880111427
608.08 0.0620802649729884
671.22 0.0601038504523448
700.54 0.0570985899996448
748.28 0.0508986969552462
811.92 0.04798425330444
876.26 0.0457934145257443
931.58 0.0436995202703314
1044.3 0.0396185921989008
1130.38 0.0360328385300858
1165.74 0.0352178432046993
1306.64 0.0327195167519296
1367.4 0.030307115764422
1483.76 0.0259403690906863
1497.6 0.0274740804059503
1671.96 0.0227451120841565
1788.24 0.0208533353460278
1875.62 0.0182279967890015
2167.76 0.0168676146937989
2351.96 0.0158240404712896
2623.48 0.0142723287905577
2728.28 0.0134422830930509
3123.68 0.0119868224944522
3452.06 0.0108497815662517
4044.96 0.00933970717065937
4213.28 0.0084115407232803
4861.7 0.00702428944863693
5544.78 0.00615475485034355
6211.4 0.00497483455833236
7156.06 0.00434736497364397
8324.8 0.00364783835689206
};
\addplot [draw=darkgray153, fill=darkgray153, forget plot, mark=*, mark size=1, only marks, draw opacity=0,
 fill opacity=0.5]
table{%
x  y
22.66 0.999999999999936
115.26 0.206940509912184
122.36 0.195623593101067
125.7 0.191500003829072
130.72 0.185067298285086
140.3 0.175371475638895
147.08 0.163831950277733
151.92 0.161004376935183
159.5 0.155200431222691
163.6 0.150359028955833
164.14 0.145921689053331
177.6 0.140188542252786
187.48 0.13232127651925
188.62 0.133622806182694
199.2 0.126964449404207
210.68 0.124054774156527
213.12 0.121568480542518
220.5 0.120625497133104
234.9 0.115929387686542
240.6 0.115810925075792
250.84 0.111588817756318
251.82 0.108937802773734
286.38 0.102363683223508
312.52 0.0980170375524338
318.82 0.0923376651464658
328.34 0.089342105017807
338.7 0.0885550008887694
374.52 0.085485812829237
409.86 0.0834668073772506
437.4 0.0802356432281371
438.06 0.073748559320812
476.72 0.0708818828385713
520.66 0.0679468581566126
579.54 0.0637347075698805
617.3 0.0635679408504219
686.2 0.0592774935229168
687.06 0.055367309103769
710.28 0.0567428228655622
733.44 0.051505818939037
836.86 0.0486921270882633
878.3 0.047704329349688
912 0.0440557918955539
999.1 0.0419349400836734
1007.56 0.0431810014091504
1054.18 0.0407204792664118
1211.96 0.0382485719376418
1298.76 0.0355378136523808
1313.7 0.0312189956008068
1314.04 0.0350063395597176
1365.02 0.0334257706886494
1557.8 0.0294385181820639
1624.8 0.0283464900234501
1649.88 0.0267776357979007
1770.8 0.0245387284263508
1850.72 0.0238930168647132
1911.38 0.0232976708184229
2026.18 0.0217751359433226
2110.24 0.0208510372696412
2281.4 0.0194330436623577
2513.68 0.016753053845529
2551.96 0.0177369339418833
2739.16 0.0157596277176051
2916.24 0.0148469106706693
2991.16 0.0141121147587521
3133.36 0.0133102379662488
3426.82 0.0122994264310742
3741.14 0.0108615233707984
3927 0.0103953667190799
3990.48 0.00996277401027567
4196.4 0.00957307858110529
4298.12 0.00909231874675954
4800.48 0.00825796833786333
4956.4 0.00781010662747273
5420.84 0.0071204097188724
5698.68 0.00629405791519859
6216.22 0.00567163830458552
6556.28 0.00529464781836694
7008.76 0.00478167560703381
7224.12 0.00453951811930891
7683.76 0.00425193454332412
7871.12 0.00397907825527687
8518 0.00373355580594418
8993.26 0.00335141646776385
};
\addplot [
  draw=saddlebrown1356716,
  fill=saddlebrown1356716,
  forget plot,
  mark=*, mark size=1,
  only marks,
  draw opacity=0,
 fill opacity=0.5
]
table{%
x  y
351.04 0.289670262204928
413.5 0.17427498444696
428.7 0.168985102304683
442.36 0.158011150600203
447.02 0.150654638549678
451.16 0.144176523415503
465.32 0.132759072263851
474.98 0.12943289319522
501.74 0.122800738220918
513.78 0.118459792437601
530.2 0.111510247732214
547.48 0.108091572770353
571.1 0.105555434151552
614.88 0.0981687666132477
642.4 0.0902561812663924
652.32 0.0878806211262759
657.58 0.0858184148650825
684.98 0.0827599787339127
719.7 0.0777454181924096
761.22 0.0719223860749818
804.68 0.0682414807409437
831.14 0.0622072835649622
900.9 0.0606125099959661
904.58 0.0554613251784369
958.26 0.0510567425291437
1011.42 0.0470363671804819
1061.72 0.045006391611451
1119.34 0.0417687618352584
1140.86 0.0393631324943412
1196.52 0.0377048387502478
1220.72 0.0359284643243843
1281.3 0.0338907793334748
1314.04 0.0329856389522081
1405.3 0.0306799479968864
1464.92 0.0293625089012683
1514.32 0.0288279784068672
1575.72 0.0267177802971102
1584.78 0.0276038377219674
1661.76 0.0250932418569105
1709.24 0.0240351870063441
1713.04 0.0229272577107929
1788.2 0.0221310052768167
1904.34 0.0215103987103935
1993.24 0.0205804744000434
2122.46 0.0199149601104335
2206.32 0.0190899575612174
2271.92 0.0185980460073239
2351.86 0.017608880681521
2426.4 0.01693398866301
2428.56 0.0160330065001608
2516.2 0.0157856959415922
2685.8 0.01488909165406
2747.8 0.014431637549258
2864.14 0.0139977209087834
2965.74 0.0134825516283164
3062.98 0.0131816741269956
3198.44 0.0127377666078033
3344.96 0.0123907746615077
3440.58 0.0119131421434116
3582.66 0.0114683780178327
3705.42 0.0112153875597887
3869.82 0.0108891272282002
4057.72 0.0104664330222589
4173.64 0.0101060891669829
4414.5 0.00965802347631014
4580.56 0.00919578037616662
4758.46 0.00899463890129554
4921.2 0.00865854239519009
4996.42 0.00842289890039956
5254.84 0.00815550436856171
5470.84 0.00784723840335872
5657.92 0.00769797187141175
5830.84 0.00741721302917526
6031.94 0.00719073480290081
6215.8 0.00693357394091549
6398.38 0.00670353483635559
6742 0.00645997200029367
6811.28 0.00628412168459007
7049.1 0.00599077965021512
7317.02 0.00581297852924111
7560.1 0.00553617381403966
7953.56 0.00518346985953033
7988.2 0.00535602051969104
8134.04 0.00504802765963061
8429.02 0.0049324192697584
8795.2 0.00476331641282085
};
\addplot [very thick, royalblue28108204]
table {%
219.44 0.161596257025093
296.56202020202 0.119000744475274
373.68404040404 0.0938841327750076
450.806060606061 0.0773396870074016
527.928080808081 0.0656312277779133
605.050101010101 0.0569167819505447
682.172121212121 0.0501834274968272
759.294141414141 0.0448282055995155
836.416161616162 0.040469880671679
913.538181818182 0.0368556743847605
990.660202020202 0.0338114102159782
1067.78222222222 0.0312131957385864
1144.90424242424 0.0289705186519131
1222.02626262626 0.0270157285364224
1299.14828282828 0.0252972575064084
1376.2703030303 0.0237751164530031
1453.39232323232 0.0224178233003731
1530.51434343434 0.0212002590351447
1607.63636363636 0.0201021404148295
1684.75838383838 0.0191069119921066
1761.8804040404 0.0182009291000745
1839.00242424242 0.0173728464492539
1916.12444444444 0.0166131544377973
1993.24646464646 0.0159138231808957
2070.36848484848 0.0152680261745246
2147.49050505051 0.0146699235726407
2224.61252525253 0.0141144906071545
2301.73454545455 0.0135973805578003
2378.85656565657 0.0131148144260648
2455.97858585859 0.0126634914384041
2533.10060606061 0.0122405159351444
2610.22262626263 0.0118433372521455
2687.34464646465 0.0114696999816451
2764.46666666667 0.0111176025823651
2841.58868686869 0.0107852627500334
2918.71070707071 0.0104710882956337
2995.83272727273 0.0101736525369409
3072.95474747475 0.00989167340878614
3150.07676767677 0.00962399565331473
3227.19878787879 0.00936957557378269
3304.32080808081 0.00912746793201176
3381.44282828283 0.00889681464635871
3458.56484848485 0.00867683500837321
3535.68686868687 0.00846681718558739
3612.80888888889 0.0082661108176722
3689.93090909091 0.00807412054549262
3767.05292929293 0.00789030033893243
3844.17494949495 0.00771414851093459
3921.29696969697 0.00754520332295443
3998.41898989899 0.00738303910168687
4075.54101010101 0.00722726279909195
4152.66303030303 0.00707751093786852
4229.78505050505 0.00693344689298764
4306.90707070707 0.00679475846699205
4384.02909090909 0.00666115572273746
4461.15111111111 0.00653236904229007
4538.27313131313 0.00640814738496142
4615.39515151515 0.00628825672108427
4692.51717171717 0.00617247862122023
4769.63919191919 0.00606060898312484
4846.76121212121 0.00595245688105419
4923.88323232323 0.00584784352393478
5001.00525252525 0.0057466013105878
5078.12727272727 0.00564857297163835
5155.24929292929 0.00555361078898633
5232.37131313131 0.00546157588479493
5309.49333333333 0.00537233757289186
5386.61535353535 0.00528577276629444
5463.73737373737 0.00520176543528362
5540.85939393939 0.00512020611107462
5617.98141414141 0.00504099143067844
5695.10343434343 0.00496402371902756
5772.22545454545 0.00488921060486073
5849.34747474747 0.0048164646672331
5926.4694949495 0.00474570310984562
6003.59151515152 0.00467684746067732
6080.71353535354 0.00460982329466038
6157.83555555556 0.0045445599773658
6234.95757575758 0.00448099042786898
6312.0795959596 0.0044190508991449
6389.20161616162 0.0043586807745021
6466.32363636364 0.00429982237870815
6543.44565656566 0.00424242080258667
6620.56767676768 0.00418642373998003
6697.6896969697 0.00413178133607492
6774.81171717172 0.00407844604617886
6851.93373737374 0.00402637250411906
6929.05575757576 0.00397551739950865
7006.17777777778 0.00392583936319251
7083.2997979798 0.00387729886024493
7160.42181818182 0.00382985808994566
7237.54383838384 0.00378348089221047
7314.66585858586 0.00373813265999615
7391.78787878788 0.00369378025724077
7468.9098989899 0.00365039194193601
7546.03191919192 0.00360793729396191
7623.15393939394 0.00356638714734426
7700.27595959596 0.00352571352662222
7777.39797979798 0.00348588958703882
7854.52 0.00344688955828967
};
\addplot [very thick, cadetblue80178158]
table {%
235.24 0.278863684608127
273.759595959596 0.25966271537854
312.279191919192 0.243530697006608
350.798787878788 0.229720812777524
389.318383838384 0.217721000424736
427.83797979798 0.207166110977238
466.357575757576 0.197787392519666
504.877171717172 0.18938181939613
543.396767676768 0.181792627950463
581.916363636364 0.174896500703986
620.43595959596 0.168594860965712
658.955555555556 0.162807799365701
697.475151515151 0.157469737201591
735.994747474747 0.152526266377269
774.514343434343 0.147931804996503
813.033939393939 0.143647830056434
851.553535353535 0.139641525959359
890.073131313131 0.135884737573375
928.592727272727 0.132353149665058
967.112323232323 0.129025636865439
1005.63191919192 0.125883743683922
1044.15151515152 0.122911264812395
1082.67111111111 0.120093903570851
1121.19070707071 0.117418991817884
1159.7103030303 0.114875258635036
1198.2298989899 0.112452638031205
1236.74949494949 0.110142108101676
1275.26909090909 0.10793555572339
1313.78868686869 0.105825662119383
1352.30828282828 0.103805805584561
1390.82787878788 0.101869978406282
1429.34747474747 0.100012715590656
1467.86707070707 0.0982290334585355
1506.38666666667 0.0965143765330993
1544.90626262626 0.0948645714255587
1583.42585858586 0.0932757866532375
1621.94545454545 0.0917444975075391
1660.46505050505 0.0902674552376121
1698.98464646465 0.0888416599361608
1737.50424242424 0.0874643366124684
1776.02383838384 0.0861329140187106
1814.54343434343 0.0848450058624862
1853.06303030303 0.0835983940938817
1891.58262626263 0.0823910140014897
1930.10222222222 0.0812209408903091
1968.62181818182 0.0800863781467534
2007.14141414141 0.0789856465231719
2045.66101010101 0.0779171744972503
2084.18060606061 0.0768794895811058
2122.7002020202 0.0758712104714332
2161.2197979798 0.0748910399461588
2199.73939393939 0.0739377584251227
2238.25898989899 0.0730102181226527
2276.77858585859 0.0721073377287918
2315.29818181818 0.0712280975636172
2353.81777777778 0.0703715351557181
2392.33737373737 0.0695367412016527
2430.85696969697 0.0687228558681998
2469.37656565657 0.0679290654035705
2507.89616161616 0.0671545990275414
2546.41575757576 0.066398726073791
2584.93535353535 0.0656607533606338
2623.45494949495 0.0649400227689007
2661.97454545455 0.0642359090079631
2700.49414141414 0.063547817552883
2739.01373737374 0.0628751827374235
2777.53333333333 0.0622174659892011
2816.05292929293 0.0615741541946389
2854.57252525252 0.0609447581825981
2893.09212121212 0.0603288113166494
2931.61171717172 0.0597258681869158
2970.13131313131 0.0591355033932761
3008.65090909091 0.0585573104124948
3047.1705050505 0.0579909005425276
3085.6901010101 0.0574359019178755
3124.2096969697 0.0568919585904105
3162.72929292929 0.0563587296705984
3201.24888888889 0.0558358885244893
3239.76848484848 0.0553231220222529
3278.28808080808 0.0548201298343995
3316.80767676768 0.0543266237721568
3355.32727272727 0.0538423271687708
3393.84686868687 0.0533669742987685
3432.36646464646 0.0529003098324655
3470.88606060606 0.0524420883232216
3509.40565656566 0.051992073725151
3547.92525252525 0.051550038939176
3586.44484848485 0.0511157653854804
3624.96444444444 0.0506890426005699
3663.48404040404 0.0502696678572877
3702.00363636364 0.0498574458062578
3740.52323232323 0.0494521881373455
3779.04282828283 0.0490537132598315
3817.56242424242 0.0486618460000903
3856.08202020202 0.0482764173156556
3894.60161616162 0.047897264024635
3933.12121212121 0.0475242285495121
3971.64080808081 0.047157158674443
4010.1604040404 0.0467959073152154
4048.68 0.046440332301102
};
\addplot [very thick, chocolate21910927]
table {%
21.86 0.998701348584803
104.65696969697 0.612236451968522
187.453939393939 0.454119924332109
270.250909090909 0.364501616848261
353.047878787879 0.305568885354037
435.844848484849 0.263425925584329
518.641818181818 0.231604202818921
601.438787878788 0.206635193761077
684.235757575758 0.186473348473441
767.032727272727 0.169826340167991
849.829696969697 0.155833863606171
932.626666666667 0.143899125472908
1015.42363636364 0.133594095388826
1098.22060606061 0.124603201514421
1181.01757575758 0.116688323332589
1263.81454545455 0.109666188624782
1346.61151515152 0.103393304759169
1429.40848484848 0.0977556327130149
1512.20545454545 0.09266133990564
1595.00242424242 0.0880356060244563
1677.79939393939 0.0838168305036967
1760.59636363636 0.0799538172007506
1843.39333333333 0.076403653206059
1926.1903030303 0.073130089072978
2008.98727272727 0.0701022868016849
2091.78424242424 0.0672938412916417
2174.58121212121 0.0646820077282037
2257.37818181818 0.0622470858478054
2340.17515151515 0.0599719249878873
2422.97212121212 0.0578415230484223
2505.76909090909 0.0558426991369928
2588.56606060606 0.0539638245161118
2671.36303030303 0.052194600046158
2754.16 0.0505258709812309
2836.95696969697 0.0489494719797341
2919.75393939394 0.0474580967135029
3002.55090909091 0.0460451876247823
3085.34787878788 0.0447048422799508
3168.14484848485 0.0434317334684876
3250.94181818182 0.0422210407435771
3333.73878787879 0.0410683915327293
3416.53575757576 0.03996981028952
3499.33272727273 0.0389216744311119
3582.1296969697 0.0379206760257993
3664.92666666667 0.03696378837202
3747.72363636364 0.0360482367540327
3830.52060606061 0.0351714727766227
3913.31757575758 0.0343311517771637
3996.11454545455 0.0335251128922943
4078.91151515152 0.0327513614216762
4161.70848484848 0.0320080531853886
4244.50545454545 0.0312934806165475
4327.30242424242 0.0306060603683854
4410.09939393939 0.0299443222465974
4492.89636363636 0.0293068993043356
4575.69333333333 0.0286925189596788
4658.4903030303 0.0280999950144138
4741.28727272727 0.0275282204691206
4824.08424242424 0.0269761610433247
4906.88121212121 0.0264428493212433
4989.67818181818 0.0259273794537428
5072.47515151515 0.0254289023557872
5155.27212121212 0.0249466213461245
5238.06909090909 0.0244797881824052
5320.86606060606 0.0240276994505103
5403.66303030303 0.0235896932717064
5486.46 0.0231651462954604
5569.25696969697 0.0227534709494134
5652.05393939394 0.0223541129212217
5734.85090909091 0.0219665488497765
5817.64787878788 0.0215902842057741
5900.44484848485 0.0212248513437688
5983.24181818182 0.0208698077097432
6066.03878787879 0.0205247341899076
6148.83575757576 0.020189233587921
6231.63272727273 0.0198629292190363
6314.4296969697 0.0195454636108366
6397.22666666667 0.019236497301256
6480.02363636364 0.0189357077255004
6562.82060606061 0.0186427881842951
6645.61757575758 0.0183574468866174
6728.41454545455 0.0180794060607219
6811.21151515151 0.017808401127846
6894.00848484848 0.0175441799335056
6976.80545454545 0.0172865020317575
7059.60242424242 0.0170351380182238
7142.39939393939 0.0167898689080511
7225.19636363636 0.016550485555317
7307.99333333333 0.0163167881107011
7390.7903030303 0.0160885855145146
7473.58727272727 0.0158656950224332
7556.38424242424 0.0156479417615001
7639.18121212121 0.015435158314174
7721.97818181818 0.0152271843283798
7804.77515151515 0.0150238661516889
7887.57212121212 0.0148250564879064
7970.36909090909 0.0146306140744857
8053.16606060606 0.0144404033793122
8135.96303030303 0.0142542943155159
8218.76 0.0140721619730776
};
\addplot [very thick, purple11522131]
table {%
80.24 0.662599260630172
137.611313131313 0.481234030521112
194.982626262626 0.387533945650539
252.353939393939 0.328488619956897
309.725252525253 0.287196823565709
367.096565656566 0.256385608527054
424.467878787879 0.232349048655107
481.839191919192 0.21297833541332
539.210505050505 0.19697562679543
596.581818181818 0.183493840411323
653.953131313131 0.17195419530666
711.324444444445 0.161946434100585
768.695757575758 0.153170851473926
826.067070707071 0.145402913080479
883.438383838384 0.13847076169867
940.809696969697 0.132240415121526
998.18101010101 0.126605734041313
1055.55232323232 0.121481446901088
1112.92363636364 0.116798190634015
1170.29494949495 0.112498914479575
1227.66626262626 0.108536226116077
1285.03757575758 0.104870402220545
1342.40888888889 0.101467875886651
1399.7802020202 0.0983000717941519
1457.15151515152 0.0953424986791072
1514.52282828283 0.0925740347103233
1571.89414141414 0.0899763592510135
1629.26545454545 0.0875334969430088
1686.63676767677 0.0852314488630168
1744.00808080808 0.083057891818358
1801.37939393939 0.0810019314361977
1858.75070707071 0.0790538980687352
1916.12202020202 0.0772051770373838
1973.49333333333 0.0754480666139893
2030.86464646465 0.0737756585562884
2088.23595959596 0.0721817370984179
2145.60727272727 0.0706606931314916
2202.97858585859 0.0692074509564791
2260.3498989899 0.0678174054974209
2317.72121212121 0.0664863682610231
2375.09252525253 0.065210520643919
2432.46383838384 0.0639863734401019
2489.83515151515 0.0628107316024051
2547.20646464646 0.0616806634742183
2604.57777777778 0.0605934738391544
2661.94909090909 0.0595466802434773
2719.3204040404 0.0585379921337522
2776.69171717172 0.0575652924242095
2834.06303030303 0.0566266211678012
2891.43434343434 0.0557201610542225
2948.80565656566 0.054844224499225
3006.17696969697 0.0539972421238305
3063.54828282828 0.0531777524508136
3120.9195959596 0.0523843926700208
3178.29090909091 0.0516158903445279
3235.66222222222 0.0508710559469478
3293.03353535354 0.0501487761299108
3350.40484848485 0.0494480076472793
3407.77616161616 0.0487677718533743
3465.14747474747 0.0481071497166811
3522.51878787879 0.0474652772923977
3579.8901010101 0.0468413416049933
3637.26141414141 0.0462345768978268
3694.63272727273 0.0456442612119637
3752.00404040404 0.0450697132607511
3809.37535353535 0.0445102895705571
3866.74666666667 0.0439653818614314
3924.11797979798 0.0434344146443778
3981.48929292929 0.0429168430144895
4038.86060606061 0.0424121506214568
4096.23191919192 0.0419198478009276
4153.60323232323 0.041439469851949
4210.97454545455 0.0409705754472572
4268.34585858586 0.0405127451645368
4325.71717171717 0.0400655801279797
4383.08848484848 0.0396287007505396
4440.4597979798 0.0392017455682265
4497.83111111111 0.0387843701586279
4555.20242424242 0.0383762461366006
4612.57373737374 0.0379770602207419
4669.94505050505 0.0375865133648548
4727.31636363636 0.0372043199491554
4784.68767676768 0.0368302070264529
4842.05898989899 0.0364639136189675
4899.4303030303 0.0361051900618349
4956.80161616162 0.0357537973897008
5014.17292929293 0.0354095067631211
5071.54424242424 0.0350720989317681
5128.91555555556 0.0347413637316997
5186.28686868687 0.0344170996141823
5243.65818181818 0.0340991132037657
5301.0294949495 0.0337872188835011
5358.40080808081 0.0334812384053653
5415.77212121212 0.0331810005241114
5473.14343434343 0.0328863406529085
5530.51474747475 0.0325971005392648
5587.88606060606 0.0323131279598443
5645.25737373737 0.0320342764328976
5702.62868686869 0.0317604049471255
5760 0.0314913777058822
};
\addplot [very thick, black18]
table {%
22.66 0.842885927453242
106.52 0.281383549079575
190.38 0.175929995327203
274.24 0.128857547201051
358.1 0.101816473315486
441.96 0.0841595330457741
525.82 0.0716873950457654
609.68 0.062393886191136
693.54 0.0551947288783036
777.4 0.0494507439639529
861.26 0.0447599456621718
945.12 0.0408564991369651
1028.98 0.0375573995505146
1112.84 0.0347324486262278
1196.7 0.0322864374421377
1280.56 0.0301481029558451
1364.42 0.0282630276347616
1448.28 0.0265889291313012
1532.14 0.0250924497381261
1616 0.0237469157011821
1699.86 0.0225307404506456
1783.72 0.0214262654192905
1867.58 0.0204189044617502
1951.44 0.0194965028649979
2035.3 0.018648850599105
2119.16 0.0178673081268595
2203.02 0.0171445154987819
2286.88 0.0164741638579386
2370.74 0.0158508142579494
2454.6 0.0152697527354743
2538.46 0.0147268734396362
2622.32 0.0142185836746533
2706.18 0.0137417262040211
2790.04 0.013293515260705
2873.9 0.012871483521456
2957.76 0.0124734379132328
3041.62 0.012097422580998
3125.48 0.0117416876980572
3209.34 0.0114046630707109
3293.2 0.0110849356986579
3377.06 0.0107812306162015
3460.92 0.0104923944678478
3544.78 0.0102173813735098
3628.64 0.00995524071937042
3712.5 0.00970510657512251
3796.36 0.00946618849032388
3880.22 0.00923776346466299
3964.08 0.00901916892110703
4047.94 0.00880979653880466
4131.8 0.00860908682549671
4215.66 0.00841652432803424
4299.52 0.00823163339518859
4383.38 0.00805397441987978
4467.24 0.00788314049873518
4551.1 0.00771875445591206
4634.96 0.00756046618569227
4718.82 0.00740795027473462
4802.68 0.0072609038702613
4886.54 0.00711904476502207
4970.4 0.00698210967376455
5054.26 0.00684985267924936
5138.12 0.00672204382868034
5221.98 0.00659846786384692
5305.84 0.00647892307036159
5389.7 0.00636322023317314
5473.56 0.0062511816870885
5557.42 0.00614264045238075
5641.28 0.00603743944672669
5725.14 0.0059354307657325
5809 0.0058364750251897
5892.86 0.00574044075897587
5976.72 0.00564720386719051
6060.58 0.00555664710970874
6144.44 0.00546865964085618
6228.3 0.00538313658136616
6312.16 0.00529997862418477
6396.02 0.00521909167104545
6479.88 0.00514038649705073
6563.74 0.00506377844077839
6647.6 0.00498918711767734
6731.46 0.0049165361547393
6815.32 0.00484575294462871
6899.18 0.00477676841762877
6983.04 0.0047095168299174
7066.9 0.00464393556682719
7150.76 0.00457996495986855
7234.62 0.00451754811640725
7318.48 0.00445663076098885
7402.34 0.00439716108739266
7486.2 0.00433908962057963
7570.06 0.00428236908777208
7653.92 0.00422695429796945
7737.78 0.00417280202926396
7821.64 0.00411987092337464
7905.5 0.00406812138686666
7989.36 0.00401751549856781
8073.22 0.00396801692273399
8157.08 0.00391959082755231
8240.94 0.00387220380860357
8324.8 0.00382582381693623
};
\addplot [very thick, darkgray153]
table {%
22.66 0.524351442892499
113.272121212121 0.212130741931243
203.884242424242 0.141537653338433
294.496363636364 0.107689815461345
385.108484848485 0.0873634181432352
475.720606060606 0.073662434743049
566.332727272727 0.0637445463267901
656.944848484848 0.0562066059363203
747.55696969697 0.0502702512743468
838.169090909091 0.0454666649191305
928.781212121212 0.0414955706915653
1019.39333333333 0.0381552294597607
1110.00545454545 0.035304815255599
1200.61757575758 0.0328428887185417
1291.2296969697 0.030694439708764
1381.84181818182 0.0288027531360408
1472.45393939394 0.0271241184735245
1563.06606060606 0.0256242829768663
1653.67818181818 0.0242760107357748
1744.2903030303 0.0230573638277731
1834.90242424242 0.0219504672369845
1925.51454545455 0.0209406052911165
2016.12666666667 0.0200155499141225
2106.73878787879 0.019165053936361
2197.35090909091 0.0183804638625019
2287.96303030303 0.0176544203837042
2378.57515151515 0.0169806242143914
2469.18727272727 0.0163536511658714
2559.79939393939 0.015768804753767
2650.41151515151 0.0152219977181876
2741.02363636364 0.0147096560318181
2831.63575757576 0.0142286405561392
2922.24787878788 0.0137761826634693
3012.86 0.0133498309970391
3103.47212121212 0.012947407178634
3194.08424242424 0.012566968753212
3284.69636363636 0.0122067780244574
3375.30848484848 0.0118652757145002
3465.92060606061 0.0115410585966554
3556.53272727273 0.011232860417759
3647.14484848485 0.0109395355580486
3737.75696969697 0.0106600449801247
3828.36909090909 0.0103934441007153
3918.98121212121 0.0101388722845602
4009.59333333333 0.00989554371238531
4100.20545454545 0.00966273941741976
4190.81757575758 0.00943980031936875
4281.4296969697 0.00922612111283883
4372.04181818182 0.00902114489020745
4462.65393939394 0.00882435839784008
4553.26606060606 0.00863528784017757
4643.87818181818 0.00845349515916922
4734.4903030303 0.00827857472730935
4825.10242424242 0.00811015040154527
4915.71454545455 0.00794787289288021
5006.32666666667 0.00779141741285222
5096.93878787879 0.00764048156343728
5187.55090909091 0.00749478344147118
5278.16303030303 0.0073540599325456
5368.77515151515 0.00721806517262471
5459.38727272727 0.00708656915843933
5549.99939393939 0.00695935649012486
5640.61151515152 0.00683622523163777
5731.22363636364 0.00671698587626801
5821.83575757576 0.00660146040610299
5912.44787878788 0.00648948143563031
6003.06 0.00638089143082168
6093.67212121212 0.00627554199604423
6184.28424242424 0.00617329322202111
6274.89636363636 0.00607401308882594
6365.50848484848 0.00597757691856545
6456.12060606061 0.00588386687298904
6546.73272727273 0.00579277149177991
6637.34484848485 0.005704185267734
6727.95696969697 0.00561800825543295
6818.56909090909 0.00553414571036944
6909.18121212121 0.00545250775579486
6999.79333333333 0.0053730090748361
7090.40545454545 0.0052955686256727
7181.01757575758 0.00522010937778427
7271.6296969697 0.00514655806747158
7362.24181818182 0.00507484497102795
7452.85393939394 0.00500490369409206
7543.46606060606 0.00493667097585137
7634.07818181818 0.00487008650688889
7724.6903030303 0.00480509275957726
7815.30242424242 0.0047416348300231
7905.91454545455 0.00467966029065484
7996.52666666667 0.0046191190526269
8087.13878787879 0.00455996323728658
8177.75090909091 0.00450214705601469
8268.36303030303 0.00444562669781076
8358.97515151515 0.00439036022404672
8449.58727272727 0.00433630746986174
8540.19939393939 0.00428342995171446
8630.81151515151 0.00423169078064891
8721.42363636364 0.00418105458086663
8812.03575757576 0.00413148741323016
8902.64787878788 0.00408295670335328
8993.26 0.00403543117396033
};
\addplot [very thick, saddlebrown1356716]
table {%
351.04 0.223175960116258
436.334545454545 0.158757317633032
521.629090909091 0.121160389213895
606.923636363636 0.0969755713979919
692.218181818182 0.0803210320900577
777.512727272727 0.0682596038103069
862.807272727273 0.0591797461955205
948.101818181818 0.0521315762043809
1033.39636363636 0.0465227168075471
1118.69090909091 0.0419665084494589
1203.98545454545 0.0382008896888524
1289.28 0.0350425453377588
1374.57454545455 0.0323597476661611
1459.86909090909 0.0300556188110859
1545.16363636364 0.0280574580665851
1630.45818181818 0.0263097320082378
1715.75272727273 0.0247693493311265
1801.04727272727 0.0234024018231811
1886.34181818182 0.0221818701535498
1971.63636363636 0.021085978996202
2056.93090909091 0.0200969980729528
2142.22545454545 0.0192003550558922
2227.52 0.0183839702111521
2312.81454545455 0.0176377511042292
2398.10909090909 0.0169532044513044
2483.40363636364 0.0163231348031372
2568.69818181818 0.01574140835042
2653.99272727273 0.0152027661000791
2739.28727272727 0.0147026748597232
2824.58181818182 0.0142372074476132
2909.87636363636 0.0138029456918196
2995.17090909091 0.0133969013452852
3080.46545454545 0.0130164511937082
3165.76 0.0126592834878488
3251.05454545455 0.0123233534727903
3336.34909090909 0.0120068462714738
3421.64363636364 0.011708145749495
3506.93818181818 0.0114258082721972
3592.23272727273 0.0111585404849431
3677.52727272727 0.0109051804187674
3762.82181818182 0.0106646813579934
3848.11636363636 0.0104360980124445
3933.41090909091 0.0102185746210788
4018.70545454545 0.0100113346810768
4104 0.00981367205035591
4189.29454545455 0.00962494321498815
4274.58909090909 0.00944456054826938
4359.88363636364 0.00927198641690043
4445.17818181818 0.00910672801323308
4530.47272727273 0.0089483328118266
4615.76727272727 0.0087963845644749
4701.06181818182 0.00865049976104014
4786.35636363636 0.00851032449438109
4871.65090909091 0.00837553167679819
4956.94545454545 0.00824581856306357
5042.24 0.00812090454152695
5127.53454545455 0.00800052916019638
5212.82909090909 0.00788445035926828
5298.12363636364 0.00777244288545469
5383.41818181818 0.00766429686675315
5468.71272727273 0.00755981652911305
5554.00727272727 0.00745881903885384
5639.30181818182 0.00736113345674945
5724.59636363636 0.00726659979146146
5809.89090909091 0.00717506814152686
5895.18545454545 0.00708639791642174
5980.48 0.0070004571283607
6065.77454545455 0.0069171217474778
6151.06909090909 0.00683627511389461
6236.36363636364 0.00675780740092634
6321.65818181818 0.00668161512433096
6406.95272727273 0.00660760069307508
6492.24727272727 0.00653567199759111
6577.54181818182 0.00646574203193885
6662.83636363636 0.00639772854666925
6748.13090909091 0.0063315537295296
6833.42545454546 0.00626714391144814
6918.72 0.00620442929550133
7004.01454545455 0.00614334370680198
7089.30909090909 0.00608382436145465
7174.60363636364 0.00602581165290887
7259.89818181818 0.00596924895420618
7345.19272727273 0.00591408243476241
7430.48727272727 0.00586026089045823
7515.78181818182 0.00580773558592685
7601.07636363636 0.00575646010803282
7686.37090909091 0.00570639022962908
7771.66545454545 0.00565748378276318
7856.96 0.0056097005405794
7942.25454545455 0.00556300210723073
8027.54909090909 0.00551735181517565
8112.84363636364 0.00547271462929031
8198.13818181818 0.00542905705727503
8283.43272727273 0.00538634706588037
8368.72727272727 0.00534455400251718
8454.02181818182 0.00530364852185247
8539.31636363636 0.00526360251702609
8624.61090909091 0.00522438905515319
8709.90545454546 0.00518598231680502
8795.2 0.00514835753918521
};
\addplot [draw=black, fill=black, mark=x, very thick, mark size=2.5pt, only marks]
table{%
x  y
89.28 0.665775923240667
351.04 0.289670262204927
1466.88 0.110924073157526
5760 0.0332925439690836
};
