# Supplementary material for: Swarm Reinforcement Learning For Adaptive Mesh Refinement
Source: arXiv:2304.00818 source file (2023-10-09)
Supplement: Supplementary file 14 [file group_additional_metrics_r3.tex]

\nextgroupplot[
ylabel shift = -0.2cm,
title style={yshift=-0.2cm},
height=4.5cm,
width=0.50\textwidth,
ylabel={Top $0.1\,\%$ Error},
xlabel={\empty},
title={Stokes Flow},
scaled x ticks=false,
clip marker paths=true,
legend cell align={left},
legend style={fill opacity=0.8, draw opacity=1, text opacity=1, draw=lightgray204},
log basis y={10},
tick align=outside,
tick pos=left,
x grid style={darkgray176},
xmajorgrids,
xmin=-459.63, xmax=10384.39,
xtick style={color=black},
xtick={-2000,0,2000,4000,6000,8000,10000,12000},
xticklabels={-2.0,0.0,2.0,4.0,6.0,8.0,10.0,12.0},
y grid style={darkgray176},
ymajorgrids,
ymin=0.00464212859342024, ymax=3.04913301150162,
ymode=log,
ytick style={color=black},
ytick={0.0001,0.001,0.01,0.1,1,10,100},
yticklabels={
  \(\displaystyle {10^{-4}}\),
  \(\displaystyle {10^{-3}}\),
  \(\displaystyle {10^{-2}}\),
  \(\displaystyle {10^{-1}}\),
  \(\displaystyle {10^{0}}\),
  \(\displaystyle {10^{1}}\),
  \(\displaystyle {10^{2}}\)
}
]
\addplot [
  draw=royalblue28108204,
  fill=royalblue28108204,
  forget plot,
  mark=*, mark size=1,
  only marks,
  draw opacity=0,
 fill opacity=0.5
]
table{%
x  y
33.28 0.999999999999987
63.94 0.847063196856177
64.42 0.872047243731223
86.94 0.784340088623371
88.68 0.683949724912878
99.24 0.650089001531512
99.62 0.741131056620274
110.6 0.591892053010926
115.36 0.582780834138439
138.2 0.567158324394811
166.5 0.446118221504217
185.28 0.403837933307522
186.32 0.368068484164752
192.5 0.390144298001054
192.94 0.392202658995571
203.74 0.36676574503082
217.04 0.338614819809818
219.78 0.320626418529269
245.78 0.318599081898504
268.74 0.360574598916247
422 0.223501748206569
458.78 0.183508251094649
459.5 0.189940190142768
497.96 0.185385624444007
517.68 0.171515564024501
523.34 0.190147481648301
523.44 0.170473689630248
546.52 0.171683666747789
551.96 0.168194809743852
612.1 0.164670437127895
725.88 0.127827036325908
732.78 0.146217625600547
751.44 0.13114157653825
762.32 0.129569927457276
808.52 0.147495516484827
821.42 0.113020512217299
853.82 0.125838600054192
869.14 0.123536670253313
879.42 0.104246793282596
959.88 0.144063542607433
1228.24 0.0878585926700957
1284.52 0.0850264910670188
1329.32 0.0891109384972309
1337.94 0.0828512829685525
1406.74 0.0865791503463098
1418.84 0.0903063634106228
1508.02 0.0792508148955093
1532.8 0.0700380711055524
1571 0.0900662602970942
1628 0.074128186596107
1642.7 0.0859272913970526
1703.02 0.0778781904853337
1732.9 0.0763834272383229
1794.64 0.0765997806806557
1961.84 0.068624023304656
1981.14 0.0658769474521567
1985.14 0.0618519694173647
1997.1 0.0625011077519678
2029.54 0.0602737565745948
2403.66 0.0593291329552006
2535.1 0.0539856176742372
2542.02 0.054349653273913
2670.78 0.041091980755572
2721.74 0.0574952142127208
2747.38 0.0554565884201765
2799.9 0.0612060913796723
2912.72 0.0530625710092218
2999.54 0.0542195176780015
3062.18 0.0580957884867177
3073.18 0.0464674106846214
3169.52 0.0477922220989807
3190.84 0.0480599544703074
3495.42 0.0390298661224937
3618.02 0.0398727800730123
3817.38 0.0489472873342816
3912.72 0.0437196563329265
3923.78 0.0434120353781719
3937.52 0.0395247947561496
3999.78 0.0490039268403263
4225.44 0.034687817458708
4306.14 0.0296074820840675
4438 0.0363928648207622
4475.72 0.0314125069546382
4510.48 0.0327818489292368
4614.06 0.0380601489417684
4664.78 0.035154622406971
4774.58 0.0424959867516408
5153.04 0.0370842006220099
5286.82 0.0318775669449673
5580.48 0.0375304792531128
5746.54 0.0321265624348405
5864.32 0.0330405122001958
5898.28 0.0351792865561993
5899.36 0.0301333855313015
6467.38 0.0309027560846105
6639.64 0.0324001476896846
6661.94 0.027142559895271
6785.94 0.0294926837766949
7752.06 0.0310677974928168
8415.78 0.0274136316754735
};
\addplot [
  draw=cadetblue80178158,
  fill=cadetblue80178158,
  forget plot,
  mark=*, mark size=1,
  only marks,
  draw opacity=0,
 fill opacity=0.5
]
table{%
x  y
213.3 0.547309953635612
216.7 0.527604450156726
222.34 0.520250344351412
222.36 0.55402271512848
222.62 0.480001074424327
222.74 0.531346587920729
224.28 0.492213217801926
225.28 0.479702823241293
232.56 0.461944860859209
261.98 0.439093943765626
417.88 0.400462218699709
418.28 0.378321998031912
425.44 0.587303687366392
442.5 0.572377477679023
447.4 0.749449064415906
456 0.416718372418708
493.52 0.684842722127334
501.22 0.65583837151484
513.28 0.622592297354923
516.7 0.616143898121574
584.28 0.312582446362746
623.28 0.306471491493557
630.1 0.402632361020752
646.06 0.404121472004083
666.4 0.609533789087912
683.56 0.407074855651339
698.04 0.720154629369764
718.28 0.629126388308538
770.8 0.673584386590184
796.8 0.769943482445009
822 0.308577662875258
855.28 0.335755314774078
858.52 0.265612851220087
882.18 0.427849259892986
919.74 0.19734364726664
941.22 0.384481594650035
957.82 0.540521132313517
1067.26 0.39734694463036
1076.04 0.918498530772015
1080.28 0.294763267109566
1098.28 0.295421215576064
1187.18 0.371524236201436
1236.2 0.539766744584805
1251.14 0.237961303493166
1265.14 0.190834065958976
1365.26 0.24036564506011
1419.74 0.346418469136763
1428.52 0.148478006864226
1448.38 0.768692086938254
1456.26 0.486453546223888
1501.36 0.724542468952794
1603.02 0.859230722104131
1617.96 0.19107537530756
1621.12 0.428197174066175
1635.18 0.310264741078973
1703.34 0.495189631564612
1752.1 0.714774229692026
1767.32 0.395903464979433
1776.86 0.0997502938813169
1811.84 0.683295828174568
1814.48 0.480372678457004
1825.14 0.385960043629178
1867.46 0.352854598458486
1912.92 0.19245977938249
2062.92 0.313182911896868
2148.3 0.100719749817966
2171.32 0.474896292287855
2329.9 0.705473532131503
2501.52 0.216099305151947
2512.24 0.12925555957622
2549.6 0.560742927572535
2622.94 0.402025883798127
2669.18 0.527785835471632
2698.26 0.234244122632565
2714.62 0.290511383643282
2718.62 0.300885521726221
2733.86 0.230728466219224
2810.84 0.840959366065921
2831.6 0.0953756485343849
2953.1 0.0799328801751998
3018.52 0.157729837916863
3039.98 0.214156664601953
3089.34 0.375027247256235
3151.9 0.296046918625908
3169.1 0.516440485268957
3170.96 0.0487510814433582
3254.64 0.116707244705217
3384.6 0.032811458261675
3403.22 0.408580068057528
3478.84 0.054544406981397
3509.96 0.84845478508905
3565.64 0.0324027995568425
3791.16 0.648936195053158
4049.06 0.384622506730842
};
\addplot [
  draw=chocolate21910927,
  fill=chocolate21910927,
  forget plot,
  mark=*, mark size=1,
  only marks,
  draw opacity=0,
 fill opacity=0.5
]
table{%
x  y
33.28 0.999999999999987
33.28 0.999999999999987
33.28 0.999999999999987
33.28 0.999999999999987
33.28 0.999999999999987
33.28 0.999999999999987
33.28 0.999999999999987
33.28 0.999999999999987
33.28 0.999999999999987
33.28 0.999999999999987
33.28 0.999999999999987
33.28 0.999999999999987
33.28 0.999999999999987
33.28 0.999999999999987
33.28 0.999999999999987
33.28 0.999999999999987
33.28 0.999999999999987
33.28 0.999999999999987
33.28 0.999999999999987
33.28 0.999999999999987
33.28 0.999999999999987
33.28 0.999999999999987
33.28 0.999999999999987
33.28 0.999999999999987
33.28 0.999999999999987
33.28 0.999999999999987
33.28 0.999999999999987
33.28 0.999999999999987
33.28 0.999999999999987
33.28 0.999999999999987
33.28 0.999999999999987
33.28 0.999999999999987
33.28 0.999999999999987
33.28 0.999999999999987
33.28 0.999999999999987
33.28 0.999999999999987
38.56 0.997729182404904
39.2 0.984849258241686
50.92 0.981817395582385
88.84 0.751544237294604
94.3 0.761797612924315
96.9 0.713630814325106
97.16 0.713633885703802
99.02 0.712853354015517
100.74 0.88775527297186
102.32 0.727736279467767
103.5 0.799041949555851
108.94 0.738330875128206
109.32 0.699126035987029
109.94 0.695786065832267
119.76 0.718118698323982
120.64 0.580510140005816
125.56 0.657930062628596
126.8 0.54399043546157
134.16 0.512138129689778
136.96 0.626261294992572
147.48 0.682922269764471
149.84 0.757904563539639
155.42 0.599306903396343
156.4 0.602691116964726
157.28 0.524086336489761
167.48 0.953880943985062
180.06 0.536052328068988
196.92 0.525424537621461
212 0.645091902958358
288.52 0.462904161912982
298.64 0.728784175190991
334.96 0.301899614087422
337.52 0.436329797655464
379.26 0.745634181751746
428.56 0.396436735403814
467.9 0.308654439546697
492.16 0.340452482301948
496 0.309934261190631
668.08 0.310510516835974
900.28 0.358887524267874
991.5 0.307227899615002
1148.88 0.229812329275308
1285.14 0.426028786429757
1459.32 0.249644549071724
1491.24 0.226388707274787
1617.4 0.157769248909657
1754.3 0.144495363512218
1871.72 0.1609211830463
2110.62 0.645668646322035
2613.06 0.155209539812172
2670.9 0.0873448006279129
3487.96 0.0787482984056366
3775.28 0.143256836997194
4373.44 0.0678912412189048
4640.5 0.511826442182648
4748.32 0.0209232758101636
6533.18 0.40428118241349
7029.72 0.0367739925000208
};
\addplot [draw=purple11522131, fill=purple11522131, forget plot, mark=*, mark size=1, only marks, draw opacity=0,
 fill opacity=0.5]
table{%
x  y
108.56 0.655184594706507
109.1 0.670750425353893
118.62 0.604436835242952
122.16 0.588813668319999
139.9 0.571936884840828
149.62 0.519111776570412
153.4 0.495352131940824
155.16 0.514951845230839
156.44 0.500941377761559
163.16 0.487885190740794
168.76 0.449983016992478
171.26 0.512965330052733
180.98 0.444820819991638
191.6 0.420861120579872
212.74 0.410780673674922
272.94 0.375750134581229
297.38 0.411466565065733
317.1 0.417914524870657
359.64 0.429143560398377
386.36 0.366215609471911
396.46 0.333724254466367
422.88 0.407771632957865
447.26 0.292233513837448
454.62 0.304612017948606
494.8 0.28632458882477
523.84 0.281204075045399
533.34 0.281569803563562
533.84 0.281217121953912
534.16 0.281225756178549
534.2 0.281216992356439
534.4 0.281227458058025
534.48 0.281688062082103
534.94 0.28130710444141
534.98 0.28122725359437
535.58 0.281231560652367
535.58 0.281231740982616
535.68 0.281233504882666
535.68 0.281233504882666
535.68 0.281233504882666
535.68 0.281233504882666
2003.06 0.153224344514309
2111.32 0.155751675046152
2140.04 0.151453297649429
2143.68 0.15156686101454
2154.12 0.151491367946884
2155.52 0.151491396387582
2156.68 0.151491712146279
2156.8 0.151491008792608
2156.8 0.151491008792608
2156.8 0.151491008792608
2156.8 0.151491008792608
2156.8 0.151491008792608
2156.8 0.151491008792608
2156.8 0.151491008792608
2156.8 0.151491008792608
2156.8 0.151491008792608
2156.8 0.151491008792608
2156.8 0.151491008792608
2156.8 0.151491008792608
2156.8 0.151491008792608
2160.38 0.148732960578484
2172.16 0.145738766384494
2172.16 0.145738766384494
2172.16 0.145738766384494
2172.16 0.145738766384494
2172.16 0.145738766384494
2172.16 0.145738766384494
2172.16 0.145738766384494
2172.16 0.145738766384494
2246.44 0.146642824878241
8289.98 0.0638786577695335
8390.62 0.0638781811992894
8507.84 0.0639787188380412
8561.24 0.0638785305076429
8591.36 0.063878407048926
8591.36 0.063878407048926
8591.36 0.063878407048926
8591.36 0.063878407048926
8591.36 0.063878407048926
8591.36 0.063878407048926
8594.8 0.0642222744563151
8612.72 0.063555777801622
8628.92 0.0635563102961478
8631.76 0.0635558272890683
8633.48 0.0635558428923543
8637.44 0.0635558272818954
8637.44 0.0635558272818954
8637.44 0.0635558272818954
8637.44 0.0635558272818954
8637.44 0.0635558272818954
8637.44 0.0635558272818954
8637.44 0.0635558272818954
8637.44 0.0635558272818954
8637.44 0.0635558272818954
8637.44 0.0635558272818954
8637.44 0.0635558272818954
8637.44 0.0635558272818954
8637.44 0.0635558272818954
8637.44 0.0635558272818954
8637.44 0.0635558272818954
};
\addplot [draw=black18, fill=black18, forget plot, mark=*, mark size=1, only marks, draw opacity=0,
 fill opacity=0.5]
table{%
x  y
33.28 0.999999999999987
80.66 0.63051663908474
82.82 0.624523746317382
84.86 0.617215895866087
87.5 0.602925003286525
92.02 0.588187435133276
94.4 0.575460388553724
95.92 0.567997033142342
99.34 0.55817555921455
104.56 0.545025668882633
109.64 0.526875863729828
113 0.518073094124221
118.3 0.51098619814612
121.6 0.502543331330403
126.98 0.489421687342437
132.26 0.474125642895436
137.32 0.464667000040414
142.78 0.445427555259931
147.92 0.433961380673747
155.06 0.417620904510089
157.24 0.408709465431909
166 0.39900811642989
168.52 0.396249426364928
173.56 0.389508824722704
184.22 0.370842461473522
193.18 0.359753822655023
204.26 0.351977390325953
211.08 0.337073247848579
215.4 0.342435872897696
221.32 0.329437990768017
225.7 0.322062385526006
232.96 0.314521984615716
249.1 0.304633125089145
260.04 0.298338087313075
280.2 0.287482137561916
289.2 0.281522911448582
304.18 0.274356519510807
315.92 0.264488181943987
327.44 0.254921500769665
343.3 0.243555982018336
357.22 0.235250365787367
369.78 0.231391079580692
387.84 0.219092001640703
417.02 0.210820235187468
436.28 0.203337445212595
465.64 0.192703482962414
485.44 0.182617398778325
494.88 0.179757238085235
519.2 0.17496639272796
537.4 0.16773568409134
588.6 0.158950829053737
620.96 0.153229535189942
688.74 0.133493678999161
689.78 0.139964632387175
725.92 0.129351025173678
753.76 0.125971759849449
817.98 0.1168391415015
865.82 0.113294945476424
932.86 0.107701659134625
1004.88 0.102114307566946
1075.68 0.0945173479067756
1148.82 0.089351461966316
1210.6 0.0839526621931307
1274.04 0.0733641483058043
1464.38 0.0648531544020818
1573.96 0.0609846336333175
1738.96 0.0552706559055602
1865.64 0.0499369043343936
1974.42 0.0472190596925316
2099.82 0.0428228198902326
2233.04 0.0400424440922038
2307.9 0.0378761897793681
2656.66 0.0316406835207748
2952.38 0.0278815793785705
3432.4 0.0234550433638636
3852.1 0.0198309899679377
4101.44 0.0185299787756883
4551.72 0.0166930378751213
5160.34 0.0155091444515635
5687.6 0.0148628565276624
6218.28 0.0143513611359012
6856.72 0.0140932727420857
7216.06 0.0138205733167974
7775.2 0.0136476029309281
8273.02 0.0136333791799738
8871.22 0.0134797229145641
9144.08 0.0134565086586405
9550.8 0.0134438210773873
};
\addplot [draw=darkgray153, fill=darkgray153, forget plot, mark=*, mark size=1, only marks, draw opacity=0,
 fill opacity=0.5]
table{%
x  y
33.28 0.999999999999987
108.44 0.494557237497499
116.8 0.461647846132929
121.76 0.439138406301615
128.82 0.408688569842913
136.88 0.386593639771843
149.44 0.369400827666873
161.36 0.345277675569942
170.72 0.330154304100249
177.7 0.315567950847947
189.34 0.298223307245224
204.36 0.276205898042563
216.3 0.263783223395724
239.18 0.247406724196697
253.4 0.227835540441303
271.36 0.212841741965385
293.3 0.205432516133416
309.88 0.193384275644575
327.22 0.179831771319523
348 0.169518967495804
374.78 0.162614502208757
383.9 0.15403959174478
409.62 0.144149182594875
424.06 0.135187575452717
449.2 0.129234960518811
479.38 0.122615475904587
519.58 0.111193222321838
537.48 0.104859842007888
564.32 0.0989507618956206
580.68 0.090886746106207
600 0.087390116015532
610.82 0.0832806629089657
653.48 0.0797082844450195
686.18 0.0764733249480097
722.12 0.0719520058632466
768.2 0.0681285986610165
794.84 0.0635502929429955
809.96 0.058274331219553
810.06 0.0620428211790891
857.96 0.0559342979656176
884.42 0.054110084897612
910.24 0.0527700238170326
940.06 0.0500802998065232
967.6 0.0491908405432847
1004.36 0.0466850568407993
1027.46 0.0446159936433894
1058.74 0.0418671606755335
1085.86 0.0410647827742171
1106.84 0.0392944018777244
1139 0.0380030261243793
1161.04 0.0366646375172055
1194.3 0.0358235434153954
1249.74 0.0340752634308788
1268.74 0.0333162312565988
1291.86 0.0320522333065856
1319.96 0.0309960001625436
1344.26 0.0301160291775356
1370 0.0291909020255255
1402.12 0.0281834944712783
1450.56 0.0273977226153648
1471.24 0.0263208153138806
1506.86 0.0240690978150721
1521.86 0.0247488857196413
1533.94 0.0256531418209979
1577.6 0.0235614515283259
1607.88 0.0229841564825643
1639.98 0.0223454598312341
1645.36 0.0217945834171514
1688.84 0.0212322396677449
1727.92 0.0209058568797103
1738.44 0.0200413385268518
1788.82 0.019909551979305
1824.8 0.0195226280697845
1833.1 0.0190675896568215
1898.24 0.0186043885265509
1922.32 0.018106412505596
1979.28 0.0177216045278635
2044.88 0.0174701843537201
2111.36 0.0169843371058018
2140.9 0.0165631282322102
2216.36 0.016050860963287
2250.04 0.0158819464441621
2349.1 0.0156250063908199
2467.54 0.0152514269402236
2618.1 0.0150104021838664
2699.62 0.0148221576137822
2813.64 0.0145323798323532
3072.7 0.0142181455725219
3272.62 0.014127942113123
3642.48 0.0139234660507029
3986.54 0.0138159560379929
4349.52 0.0137708079486999
4885.62 0.0137073335380093
5536.96 0.01369298206211
6494.12 0.0136938053019767
8029.94 0.0136999359310756
};
\addplot [
  draw=saddlebrown1356716,
  fill=saddlebrown1356716,
  forget plot,
  mark=*, mark size=1,
  only marks,
  draw opacity=0,
 fill opacity=0.5
]
table{%
x  y
535.68 0.281233504882655
610.5 0.214696020334182
614.3 0.208215120769519
623.12 0.200023361557179
627.06 0.195643141364255
633.88 0.190609471495326
650.9 0.187372571350605
660.3 0.18365800608986
663.68 0.167265579157913
665.36 0.17755751411569
665.58 0.175296404999668
675.46 0.161196403533528
691.44 0.154049017236997
706.98 0.148978456971039
711.94 0.143018611399274
745 0.136544021805486
769.74 0.130451649574222
788.52 0.124433960671998
799.04 0.12046420588819
820.96 0.115597131018195
835.5 0.111613629356551
850.26 0.107727867271078
866.34 0.103435275845675
900.08 0.0968491198376711
916.32 0.0930254288859606
918.02 0.0899778123490247
935.72 0.0828235128649115
948.54 0.0800693366232642
979.26 0.0758547148863149
998.94 0.0730454022303282
1027.44 0.0669665746430323
1027.86 0.0708327065157198
1047.82 0.0642196337617684
1078.3 0.0617882481217325
1099.7 0.0607454907778592
1121.36 0.0587328118866051
1133.3 0.058164660836265
1167.88 0.0561603258177782
1187.38 0.0544766014477646
1228.88 0.0487598887609536
1246.78 0.0472414385035595
1295.24 0.0448566761080397
1338 0.0426182400521863
1386.8 0.0398991430527854
1493.08 0.0358352724821631
1563.32 0.0339579855504944
1606.36 0.0334918052558052
1667.5 0.0313413296513258
1732.72 0.0287506877695661
1845.3 0.0265462208280407
1898.12 0.025613185490645
1969.42 0.0252080509246835
2028.86 0.0243013988872103
2109.52 0.0238669102889723
2164.64 0.0231875757191672
2236.16 0.0223732301729748
2296.26 0.0216310748103106
2364.8 0.0212262901616547
2495.28 0.0206018197913895
2583.56 0.0199685040619012
2687.76 0.0192698218789622
2792.34 0.0186263730089841
2873.02 0.0181915682457762
2976.3 0.0176721761557347
3066.98 0.0173507262769427
3094.32 0.016813265714045
3247.22 0.0166510294529019
3325.26 0.0164019884650318
3472.46 0.0160976428109177
3589.66 0.0159713240627377
3613.06 0.0157796974661543
3811.18 0.0155541615920306
3951.4 0.0153890485229263
4106.66 0.0152442388452042
4243.16 0.015152032165086
4384.22 0.0150065455175067
4490.6 0.0145775729219364
4498.2 0.0147175438558447
4596.12 0.0144614526646295
4750.96 0.0143973938365635
4844.82 0.0142682945599247
5035.28 0.0142353081603749
5213.1 0.0142020885657303
5446.58 0.014104918861042
5718.62 0.0140181889697036
6040.8 0.0139908951402111
6270.9 0.0139850362802892
6495.22 0.0139691291459643
6789.18 0.0139161740266682
7036.2 0.013878694365198
7328.3 0.0138660140917624
7590 0.0138502662343962
7973.5 0.0138154568347472
8272.46 0.0138146185032018
8570.9 0.0138135598712782
8881.44 0.0138118577695099
9220 0.0138084158863372
9554.72 0.0138015461209849
9891.48 0.0137990028854779
};
\addplot [very thick, royalblue28108204]
table {%
33.28 1.46160712158083
117.951717171717 0.546901461564724
202.623434343434 0.362416684035986
287.295151515152 0.278687651793844
371.966868686869 0.229793525807664
456.638585858586 0.197329145993385
541.310303030303 0.174012700840931
625.98202020202 0.156352366047384
710.653737373737 0.142452323899987
795.325454545455 0.131189188121647
879.997171717172 0.12185244765671
964.668888888889 0.113969420999994
1049.34060606061 0.10721268186154
1134.01232323232 0.101347799436292
1218.68404040404 0.0962022356133337
1303.35575757576 0.0916460061076485
1388.02747474747 0.0875792048343004
1472.69919191919 0.0839236985056514
1557.37090909091 0.0806174449794611
1642.04262626263 0.0776105130247536
1726.71434343434 0.0748622349992508
1811.38606060606 0.0723391317415958
1896.05777777778 0.0700133748928028
1980.7294949495 0.0678616302883881
2065.40121212121 0.0658641761345194
2150.07292929293 0.0640042223681133
2234.74464646465 0.0622673793714239
2319.41636363636 0.0606412389790117
2404.08808080808 0.0591150409003264
2488.7597979798 0.0576794048143914
2573.43151515152 0.0563261134595854
2658.10323232323 0.0550479356871412
2742.77494949495 0.0538384811019455
2827.44666666667 0.052692079869471
2912.11838383838 0.0516036827226738
2996.7901010101 0.0505687772960173
3081.46181818182 0.0495833177428442
3166.13353535354 0.0486436652263757
3250.80525252525 0.0477465373634464
3335.47696969697 0.046888965079804
3420.14868686869 0.0460682556328747
3504.8204040404 0.0452819607918824
3589.49212121212 0.0445278493506836
3674.16383838384 0.0438038832965886
3758.83555555556 0.0431081970770737
3843.50727272727 0.0424390795019552
3928.17898989899 0.0417949578961519
4012.85070707071 0.0411743841813375
4097.52242424242 0.040576022616498
4182.19414141414 0.0399986389699195
4266.86585858586 0.0394410909302444
4351.53757575758 0.0389023195933364
4436.20929292929 0.038381341885927
4520.88101010101 0.0378772438072619
4605.55272727273 0.0373891743869409
4690.22444444444 0.0369163402714349
4774.89616161616 0.0364580008638264
4859.56787878788 0.0360134639515362
4944.2395959596 0.0355820817654844
5028.91131313131 0.0351632474215331
5113.58303030303 0.0347563917013807
5198.25474747475 0.0343609801355009
5282.92646464646 0.0339765103553773
5367.59818181818 0.0336025096862955
5452.2698989899 0.0332385329554259
5536.94161616162 0.0328841604929291
5621.61333333333 0.0325389963064203
5706.28505050505 0.0322026664113989
5790.95676767677 0.0318748173022211
5875.62848484848 0.0315551145499208
5960.3002020202 0.0312432415146961
6044.97191919192 0.0309388981622006
6129.64363636364 0.0306417999739478
6214.31535353535 0.0303516769431578
6298.98707070707 0.030068272648284
6383.65878787879 0.0297913433972556
6468.33050505051 0.0295206574361781
6553.00222222222 0.029255994216864
6637.67393939394 0.0289971437181212
6722.34565656566 0.0287439058162236
6807.01737373737 0.0284960897004302
6891.68909090909 0.0282535133298126
6976.36080808081 0.0280160029280026
7061.03252525253 0.0277833925127894
7145.70424242424 0.0275555234577746
7230.37595959596 0.0273322440835502
7315.04767676768 0.0271134092760898
7399.71939393939 0.0268988801302515
7484.39111111111 0.0266885236164707
7569.06282828283 0.0264822122688934
7653.73454545455 0.0262798238933463
7738.40626262626 0.0260812412936777
7823.07797979798 0.0258863520151276
7907.7496969697 0.0256950481034943
7992.42141414141 0.025507225878968
8077.09313131313 0.0253227857235937
8161.76484848485 0.0251416318814067
8246.43656565657 0.0249636722703651
8331.10828282828 0.0247888183052664
8415.78 0.0246169847309054
};
\addplot [very thick, cadetblue80178158]
table {%
213.3 0.494507146162741
252.045050505051 0.50741787889522
290.790101010101 0.514594523249591
329.535151515151 0.517797168699659
368.280202020202 0.518186472876935
407.025252525253 0.516554300802587
445.770303030303 0.513455783468592
484.515353535354 0.509288757792182
523.260404040404 0.504343525259766
562.005454545455 0.498835087855976
600.750505050505 0.49292463661968
639.495555555555 0.486734230738203
678.240606060606 0.480357039773903
716.985656565656 0.473864623667084
755.730707070707 0.467312192288974
794.475757575758 0.460742460569764
833.220808080808 0.454188510802674
871.965858585859 0.447675942409288
910.710909090909 0.4412245033162
949.455959595959 0.434849339518879
988.20101010101 0.428561960263054
1026.94606060606 0.422370989241518
1065.69111111111 0.416282753270005
1104.43616161616 0.410301746470046
1143.18121212121 0.404430998337666
1181.92626262626 0.398672367070233
1220.67131313131 0.393026774383622
1259.41636363636 0.38749439424491
1298.16141414141 0.382074805101255
1336.90646464646 0.376767113042499
1375.65151515152 0.371570051707946
1414.39656565657 0.366482063503494
1453.14161616162 0.36150136573729
1491.88666666667 0.356626004539832
1530.63171717172 0.351853898855842
1569.37676767677 0.347182876341782
1608.12181818182 0.342610702645446
1646.86686868687 0.338135105261077
1685.61191919192 0.333753792928277
1724.35696969697 0.329464471362928
1763.10202020202 0.325264855963951
1801.84707070707 0.321152682023257
1840.59212121212 0.317125712872138
1879.33717171717 0.313181746320883
1918.08222222222 0.309318619686179
1956.82727272727 0.305534213649976
1995.57232323232 0.30182645515185
2034.31737373737 0.298193319482599
2073.06242424242 0.294632831718647
2111.80747474747 0.291143067613447
2150.55252525252 0.287722154042832
2189.29757575758 0.284368269085201
2228.04262626263 0.281079641804136
2266.78767676768 0.277854551789908
2305.53272727273 0.274691328507133
2344.27777777778 0.271588350488018
2383.02282828283 0.268544044404207
2421.76787878788 0.265556884044797
2460.51292929293 0.262625389223502
2499.25797979798 0.259748124634132
2538.00303030303 0.256923698670345
2576.74808080808 0.254150762222869
2615.49313131313 0.251428007465159
2654.23818181818 0.24875416663649
2692.98323232323 0.246128010829884
2731.72828282828 0.243548348790889
2770.47333333333 0.241014025732101
2809.21838383838 0.238523922167305
2847.96343434343 0.236076952768345
2886.70848484848 0.233672065247115
2925.45353535354 0.23130823926448
2964.19858585859 0.228984485367494
3002.94363636364 0.226699843955828
3041.68868686869 0.224453384278012
3080.43373737374 0.222244203457815
3119.17878787879 0.220071425550848
3157.92383838384 0.217934200631271
3196.66888888889 0.215831703908363
3235.41393939394 0.213763134872548
3274.15898989899 0.211727716470394
3312.90404040404 0.209724694308012
3351.64909090909 0.207753335882212
3390.39414141414 0.205812929838738
3429.13919191919 0.203902785256859
3467.88424242424 0.202022230959561
3506.62929292929 0.200170614848592
3545.37434343434 0.198347303263571
3584.11939393939 0.196551680364406
3622.86444444444 0.194783147536227
3661.60949494949 0.193041122816079
3700.35454545455 0.191325040340619
3739.0995959596 0.189634349814073
3777.84464646465 0.187968515995713
3816.5896969697 0.186327018206163
3855.33474747475 0.184709349851809
3894.0797979798 0.18311501796667
3932.82484848485 0.181543542771048
3971.5698989899 0.179994457246336
4010.31494949495 0.178467306725354
4049.06 0.176961648497632
};
\addplot [very thick, chocolate21910927]
table {%
33.28 1.00138821214449
103.951111111111 0.724138428946857
174.622222222222 0.602412658740389
245.293333333333 0.527428683326229
315.964444444444 0.474671569492779
386.635555555556 0.434722197581258
457.306666666667 0.403010757533478
527.977777777778 0.376994126893693
598.648888888889 0.3551211599319
669.32 0.336381172393174
739.991111111111 0.320081861676756
810.662222222222 0.305730019070605
881.333333333333 0.292962957061432
952.004444444445 0.281506901454929
1022.67555555556 0.271150605628285
1093.34666666667 0.261727991062314
1164.01777777778 0.253106365017098
1234.68888888889 0.245178206861587
1305.36 0.237855307705766
1376.03111111111 0.23106450312337
1446.70222222222 0.224744509480435
1517.37333333333 0.218843540559255
1588.04444444444 0.213317486035435
1658.71555555556 0.208128501199055
1729.38666666667 0.203243902169714
1800.05777777778 0.198635291118082
1870.72888888889 0.194277856794707
1941.4 0.190149810183522
2012.07111111111 0.186231925388368
2082.74222222222 0.182507163257499
2153.41333333333 0.178960360635627
2224.08444444444 0.175577972099243
2294.75555555556 0.172347853984503
2365.42666666667 0.169259082738859
2436.09777777778 0.166301801314933
2506.76888888889 0.163467088618028
2577.44 0.160746848017393
2648.11111111111 0.158133711709085
2718.78222222222 0.15562095832816
2789.45333333333 0.153202441689661
2860.12444444445 0.150872528920785
2930.79555555556 0.148626046552847
3001.46666666667 0.146458233388119
3072.13777777778 0.144364699155888
3142.80888888889 0.142341388134236
3213.48 0.14038454704651
3284.15111111111 0.138490696650263
3354.82222222222 0.13665660652622
3425.49333333333 0.134879272649179
3496.16444444445 0.13315589738465
3566.83555555556 0.131483871606707
3637.50666666667 0.129860758675867
3708.17777777778 0.128284280052292
3778.84888888889 0.126752302350371
3849.52 0.12526282566688
3920.19111111111 0.12381397303705
3990.86222222222 0.122403980891812
4061.53333333333 0.121031190405653
4132.20444444444 0.119694039638384
4202.87555555556 0.118391056386054
4273.54666666667 0.117120851666526
4344.21777777778 0.115882113774126
4414.88888888889 0.114673602845479
4485.56 0.113494145885351
4556.23111111111 0.112342632207132
4626.90222222222 0.111218009247695
4697.57333333333 0.11011927872081
4768.24444444444 0.109045493077195
4838.91555555556 0.107995752242711
4909.58666666667 0.106969200609218
4980.25777777778 0.105965024255276
5050.92888888889 0.104982448376218
5121.6 0.104020734905188
5192.27111111111 0.103079180308607
5262.94222222222 0.102157113541124
5333.61333333333 0.101253894146617
5404.28444444444 0.100368910493037
5474.95555555556 0.0995015781301216
5545.62666666667 0.0986513382599621
5616.29777777778 0.0978176563113911
5686.96888888889 0.0970000206099538
5757.64 0.0961979411359806
5828.31111111111 0.0954109483639466
5898.98222222222 0.0946385921769024
5969.65333333333 0.0938804408503058
6040.32444444444 0.0931360801000699
6110.99555555556 0.0924051121900878
6181.66666666667 0.0916871550948899
6252.33777777778 0.0909818417134563
6323.00888888889 0.0902888191305304
6393.68 0.0896077479220794
6464.35111111111 0.0889383015018194
6535.02222222222 0.0882801655059643
6605.69333333333 0.0876330372135871
6676.36444444444 0.0869966250001823
6747.03555555556 0.0863706478222064
6817.70666666667 0.0857548347305423
6888.37777777778 0.0851489244109902
6959.04888888889 0.0845526647500293
7029.72 0.0839658124242245
};
\addplot [very thick, purple11522131]
table {%
108.56 0.5875765862952
194.710303030303 0.465787199995216
280.860606060606 0.398657530581777
367.010909090909 0.354106512781819
453.161212121212 0.321600498379906
539.311515151515 0.2964605813751
625.461818181818 0.276231640589639
711.612121212121 0.25947896696697
797.762424242424 0.245298028602904
883.912727272727 0.233085324555801
970.06303030303 0.222420102010551
1056.21333333333 0.212998515114807
1142.36363636364 0.20459472839076
1228.51393939394 0.197036802855444
1314.66424242424 0.190191137668465
1400.81454545455 0.183952088396552
1486.96484848485 0.178234837463722
1573.11515151515 0.172970374730711
1659.26545454545 0.168101886042981
1745.41575757576 0.163582104550269
1831.56606060606 0.159371334789818
1917.71636363636 0.155435956039152
2003.86666666667 0.151747273050231
2090.01696969697 0.148280622526671
2176.16727272727 0.145014670558944
2262.31757575758 0.14193085449058
2348.46787878788 0.139012935317949
2434.61818181818 0.136246635600916
2520.76848484849 0.133619344188351
2606.91878787879 0.131119873633019
2693.06909090909 0.128738259512897
2779.21939393939 0.126465593348378
2865.3696969697 0.124293882652998
2951.52 0.122215933050498
3037.6703030303 0.120225248454018
3123.82060606061 0.118315946119998
3209.97090909091 0.116482684022154
3296.12121212121 0.114720598484768
3382.27151515152 0.113025250402824
3468.42181818182 0.11139257868382
3554.57212121212 0.10981885979086
3640.72242424242 0.108300672462762
3726.87272727273 0.106834866845001
3813.02303030303 0.105418537393369
3899.17333333333 0.104048999016585
3985.32363636364 0.102723766009436
4071.47393939394 0.101440533398282
4157.62424242424 0.100197160378714
4243.77454545455 0.0989916555733024
4329.92484848485 0.0978221638774032
4416.07515151515 0.0966869546945303
4502.22545454546 0.0955844113908933
4588.37575757576 0.0945130218224007
4674.52606060606 0.0934713698074413
4760.67636363636 0.0924581274357334
4846.82666666667 0.0914720481179706
4932.97696969697 0.0905119602933157
5019.12727272727 0.0895767617223368
5105.27757575758 0.0886654143020335
5191.42787878788 0.0877769393473854
5277.57818181818 0.0869104132905723
5363.72848484849 0.0860649637548383
5449.87878787879 0.0852397659649966
5536.02909090909 0.0844340394609694
5622.17939393939 0.0836470450845604
5708.3296969697 0.0828780822129986
5794.48 0.0821264862157058
5880.6303030303 0.0813916261132944
5966.78060606061 0.0806729024200539
6052.93090909091 0.0799697451531573
6139.08121212121 0.0792816119935654
6225.23151515152 0.0786079865851502
6311.38181818182 0.0779483769599169
6397.53212121212 0.077302314078423
6483.68242424243 0.0766693504755575
6569.83272727273 0.0760490590028089
6655.98303030303 0.0754410316589961
6742.13333333333 0.0748448785021997
6828.28363636364 0.0742602266363108
6914.43393939394 0.0736867192662219
7000.58424242424 0.0731240148162325
7086.73454545455 0.0725717861067269
7172.88484848485 0.0720297195846279
7259.03515151515 0.0714975146035221
7345.18545454546 0.0709748827497112
7431.33575757576 0.0704615472107654
7517.48606060606 0.0699572421834477
7603.63636363636 0.0694617123181394
7689.78666666667 0.0689747121971366
7775.93696969697 0.0684960058444039
7862.08727272727 0.0680253662645694
7948.23757575758 0.0675625750091188
8034.38787878788 0.0671074217679146
8120.53818181818 0.0666597039843113
8206.68848484849 0.0662192264922709
8292.83878787879 0.0657858011740108
8378.98909090909 0.0653592466368207
8465.13939393939 0.0649393879077991
8551.2896969697 0.0645260561453404
8637.44 0.0641190883663028
};
\addplot [very thick, black18]
table {%
33.28 1.11323436041709
129.416565656566 0.479515151944606
225.553131313131 0.321865474451895
321.689696969697 0.245403465927115
417.826262626263 0.19932515491282
513.962828282828 0.16822333816551
610.099393939394 0.14569539784181
706.235959595959 0.128568056253987
802.372525252525 0.115077296954862
898.509090909091 0.104159382145684
994.645656565656 0.0951325407116323
1090.78222222222 0.0875385619078237
1186.91878787879 0.0810575285079928
1283.05535353535 0.0754589814592544
1379.19191919192 0.0705725046335177
1475.32848484848 0.0662692507024877
1571.46505050505 0.0624499220216208
1667.60161616162 0.0590367114827861
1763.73818181818 0.0559677555337825
1859.87474747475 0.0531932279852701
1956.01131313131 0.0506725331995126
2052.14787878788 0.0483722527326626
2148.28444444444 0.0462646188524406
2244.42101010101 0.044326363203389
2340.55757575758 0.0425378369736854
2436.69414141414 0.0408823304779597
2532.83070707071 0.0393455411953215
2628.96727272727 0.0379151536950522
2725.10383838384 0.0365805048497359
2821.2404040404 0.0353323147415695
2917.37696969697 0.0341624686600478
3013.51353535353 0.0330638391922405
3109.6501010101 0.0320301400378581
3205.78666666667 0.0310558051235902
3301.92323232323 0.0301358880397255
3398.0597979798 0.0292659779126657
3494.19636363636 0.0284421286554137
3590.33292929293 0.0276607991727313
3686.46949494949 0.0269188025876174
3782.60606060606 0.0262132629368374
3878.74262626263 0.0255415780817128
3974.87919191919 0.0249013878157028
4071.01575757576 0.0242905463370132
4167.15232323232 0.0237070984034671
4263.28888888889 0.0231492586064596
4359.42545454545 0.0226153932973135
4455.56202020202 0.0221040047776091
4551.69858585858 0.0216137174288407
4647.83515151515 0.0211432655089672
4743.97171717172 0.0206914823863666
4840.10828282828 0.0202572910171707
4936.24484848485 0.0198396955013612
5032.38141414141 0.0194377735774912
5128.51797979798 0.019050669936347
5224.65454545454 0.0186775902510212
5320.79111111111 0.0183177958352966
5416.92767676768 0.0179705988544241
5513.06424242424 0.0176353580226988
5609.20080808081 0.0173114747309982
5705.33737373737 0.0169983895549186
5801.47393939394 0.0166955791005251
5897.6105050505 0.0164025531501934
5993.74707070707 0.016118852075724
6089.88363636363 0.0158440444899466
6186.0202020202 0.0155777251115292
6282.15676767677 0.0153195128207255
6378.29333333333 0.0150690488864144
6474.4298989899 0.0148259953470682
6570.56646464646 0.0145900335302652
6666.70303030303 0.0143608626971019
6762.83959595959 0.0141381987993712
6858.97616161616 0.0139217733387067
6955.11272727273 0.0137113323180571
7051.24929292929 0.0135066352768841
7147.38585858586 0.0133074544023838
7243.52242424242 0.0131135737098262
7339.65898989899 0.0129247882858234
7435.79555555555 0.0127409035889542
7531.93212121212 0.0125617348027376
7628.06868686869 0.0123871062364361
7724.20525252525 0.0122168507696139
7820.34181818182 0.0120508093367648
7916.47838383838 0.0118888304486777
8012.61494949495 0.0117307697475178
8108.75151515151 0.0115764895928858
8204.88808080808 0.0114258586763663
8301.02464646465 0.0112787516623032
8397.16121212121 0.0111350488527436
8493.29777777778 0.0109946358746734
8589.43434343434 0.010857403387834
8685.57090909091 0.0107232468115564
8781.70747474747 0.0105920660691838
8877.84404040404 0.0104637653487766
8973.9806060606 0.010338252878901
9070.11717171717 0.0102154407184049
9166.25373737374 0.0100952445591722
9262.3903030303 0.00997758354093165
9358.52686868687 0.00986238007726863
9454.66343434343 0.00974955969205754
9550.8 0.00963905086559423
};
\addplot [very thick, darkgray153]
table {%
33.28 2.27044006803571
114.054343434343 0.498338900666367
194.828686868687 0.266875483316725
275.60303030303 0.180095336544522
356.377373737374 0.135331564356205
437.151717171717 0.108208640861344
517.926060606061 0.0900849827035493
598.700404040404 0.0771490540488488
679.474747474747 0.0674667206633093
760.249090909091 0.0599550793106954
841.023434343434 0.05396184273884
921.797777777778 0.0490712351170877
1002.57212121212 0.0450059982601087
1083.34646464646 0.0415742974832808
1164.12080808081 0.03863926269486
1244.89515151515 0.0361006695161274
1325.66949494949 0.033883475094776
1406.44383838384 0.0319303961504517
1487.21818181818 0.0301969610985768
1567.99252525253 0.0286481260781022
1648.76686868687 0.0272559078504719
1729.54121212121 0.0259976945688074
1810.31555555556 0.0248550185637986
1891.0898989899 0.0238126503433601
1971.86424242424 0.0228579199457422
2052.63858585859 0.0219802018414502
2133.41292929293 0.0211705192336
2214.18727272727 0.0204212367078676
2294.96161616162 0.0197258190709874
2375.73595959596 0.0190786403436129
2456.5103030303 0.0184748311597975
2537.28464646465 0.0179101558653706
2618.05898989899 0.0173809127909163
2698.83333333333 0.0168838527617676
2779.60767676768 0.016416112073149
2860.38202020202 0.0159751570238088
2941.15636363636 0.0155587377498071
3021.93070707071 0.0151648495902938
3102.70505050505 0.0147917005908365
3183.47939393939 0.0144376840370703
3264.25373737374 0.0141013551338102
3345.02808080808 0.0137814111181674
3425.80242424242 0.0134766742313133
3506.57676767677 0.0131860770810557
3587.35111111111 0.0129086500128337
3668.12545454545 0.01264351017503
3748.8997979798 0.0123898520193763
3829.67414141414 0.0121469390215556
3910.44848484848 0.0119140964430914
3991.22282828283 0.0116907049849571
4071.99717171717 0.0114761952073888
4152.77151515151 0.0112700426101623
4233.54585858586 0.0110717632839439
4314.3202020202 0.0108809100568813
4395.09454545455 0.010697069071889
4475.86888888889 0.0105198567395174
4556.64323232323 0.0103489170192053
4637.41757575758 0.0101839189883713
4718.19191919192 0.0100245546644211
4798.96626262626 0.0098705370495025
4879.74060606061 0.00972159837188609
4960.51494949495 0.0095774885012873
5041.28929292929 0.00943797351838996
5122.06363636364 0.00930283442134876
5202.83797979798 0.00917186595421127
5283.61232323232 0.00904487554406232
5364.38666666667 0.00892168233530106
5445.16101010101 0.00880211631085164
5525.93535353535 0.00868601749131287
5606.7096969697 0.00857323520410163
5687.48404040404 0.00846362741555524
5768.25838383838 0.00835706011975604
5849.03272727273 0.00825340677853625
5929.80707070707 0.00815254780773206
6010.58141414141 0.00805437010529116
6091.35575757576 0.00795876661730893
6172.1301010101 0.00786563593848369
6252.90444444444 0.00777488194384712
6333.67878787879 0.007686413448951
6414.45313131313 0.00760014389597634
6495.22747474747 0.00751599106348751
6576.00181818182 0.0074338767977784
6656.77616161616 0.00735372676395912
6737.55050505051 0.00727547021511163
6818.32484848485 0.00719903977800169
6899.09919191919 0.00712437125397799
6979.87353535353 0.00705140343381713
7060.64787878788 0.00698007792538766
7141.42222222222 0.00691033899310925
7222.19656565657 0.00684213340827574
7302.97090909091 0.00677541030939328
7383.74525252525 0.0067101210717606
7464.5195959596 0.00664621918558509
7545.29393939394 0.00658366014198993
7626.06828282828 0.00652240132632233
7706.84262626263 0.00646240191822279
7787.61696969697 0.00640362279796073
7868.39131313131 0.00634602645858254
7949.16565656566 0.00628957692345517
8029.94 0.00623423966882292
};
\addplot [very thick, saddlebrown1356716]
table {%
535.68 0.291075943566755
630.18303030303 0.195782198618141
724.686060606061 0.142286607897732
819.189090909091 0.109348416028158
913.692121212121 0.0876314021224371
1008.19515151515 0.0725407812816666
1102.69818181818 0.0616111357186632
1197.20121212121 0.0534262086063791
1291.70424242424 0.0471262577688326
1386.20727272727 0.042165039775786
1480.7103030303 0.0381819656678763
1575.21333333333 0.0349311302917558
1669.71636363636 0.0322400755206815
1764.21939393939 0.0299848725641173
1858.72242424242 0.0280745440820109
1953.22545454545 0.0264410304673941
2047.72848484848 0.0250325545478559
2142.23151515151 0.0238091295342428
2236.73454545455 0.0227394533804742
2331.23757575758 0.0217987206506514
2425.74060606061 0.0209670542012342
2520.24363636364 0.0202283634631192
2614.74666666667 0.0195695013762503
2709.2496969697 0.0189796336831603
2803.75272727273 0.0184497613955024
2898.25575757576 0.017972355208019
2992.75878787879 0.0175410727323194
3087.26181818182 0.0171505376971599
3181.76484848485 0.0167961660017409
3276.26787878788 0.0164740275428637
3370.77090909091 0.0161807356073394
3465.27393939394 0.015913357687038
3559.77696969697 0.0156693430769085
3654.28 0.0154464637206907
3748.78303030303 0.0152427655882651
3843.28606060606 0.015056528481704
3937.78909090909 0.0148862326298263
4032.29212121212 0.0147305307830697
4126.79515151515 0.0145882247903019
4221.29818181818 0.0144582458474544
4315.80121212121 0.0143396377697233
4410.30424242424 0.0142315427656713
4504.80727272727 0.0141331892911849
4599.3103030303 0.0140438816400954
4693.81333333333 0.0139629909910267
4788.31636363636 0.0138899476802487
4882.81939393939 0.0138242345107001
4977.32242424242 0.0137653809399701
5071.82545454545 0.0137129580165261
5166.32848484849 0.0136665739550753
5260.83151515152 0.0136258702596335
5355.33454545455 0.0135905183174318
5449.83757575758 0.013560216398786
5544.34060606061 0.0135346870080151
5638.84363636364 0.0135136745387668
5733.34666666667 0.0134969431940072
5827.8496969697 0.0134842751367273
5922.35272727273 0.0134754688422635
6016.85575757576 0.0134703376272338
6111.35878787879 0.0134687083335433
6205.86181818182 0.0134704201488548
6300.36484848485 0.0134753235474062
6394.86787878788 0.0134832793371865
6489.37090909091 0.0134941578013019
6583.87393939394 0.0135078379229131
6678.37696969697 0.0135242066844713
6772.88 0.013543158433126
6867.38303030303 0.0135645943051742
6961.88606060606 0.0135884217032808
7056.38909090909 0.0136145538209463
7150.89212121212 0.0136429092093436
7245.39515151515 0.0136734113822096
7339.89818181818 0.0137059884549747
7434.40121212121 0.0137405728147343
7528.90424242424 0.0137771008180508
7623.40727272727 0.0138155125139011
7717.9103030303 0.0138557513893761
7812.41333333333 0.0138977641359938
7906.91636363636 0.0139415004347133
8001.41939393939 0.0139869127579367
8095.92242424242 0.0140339561869624
8190.42545454546 0.0140825882435061
8284.92848484848 0.0141327687340505
8379.43151515151 0.0141844596059033
8473.93454545455 0.0142376248139524
8568.43757575758 0.0142922301972095
8662.94060606061 0.0143482433643161
8757.44363636364 0.0144056335872658
8851.94666666667 0.0144643717026677
8946.4496969697 0.0145244300199344
9040.95272727273 0.0145857822358407
9135.45575757576 0.0146484033549435
9229.95878787879 0.0147122696154013
9324.46181818182 0.0147773584197736
9418.96484848485 0.014843648270416
9513.46787878788 0.0149111187091202
9607.97090909091 0.0149797502606788
9702.47393939394 0.0150495243800813
9796.97696969697 0.0151204234030734
9891.48 0.015192430499833
};
\addplot [draw=black, fill=black, mark=x, very thick, mark size=2.5pt, only marks]
table{%
x  y
132.32 0.512227225941859
535.68 0.281233504882655
2156.8 0.151491008792566
8637.44 0.0635558272818851
};
