# Supplementary material for: Swarm Reinforcement Learning For Adaptive Mesh Refinement
Source: arXiv:2304.00818 source file (2023-10-09)
Supplement: Supplementary file 15 [file group_additional_metrics_r4.tex]

\nextgroupplot[
ylabel shift = -0.2cm,
title style={yshift=-0.2cm},
height=4.5cm,
width=0.50\textwidth,
ylabel={Top $0.1\,\%$ Error},
xlabel={\empty},
title={Linear Elasticity},
scaled x ticks=false,
clip marker paths=true,
legend cell align={left},
legend style={fill opacity=0.8, draw opacity=1, text opacity=1, draw=lightgray204},
log basis y={10},
tick align=outside,
tick pos=left,
x grid style={darkgray176},
xmajorgrids,
xmin=-551.85, xmax=12054.81,
xtick style={color=black},
xtick={-2000,0,2000,4000,6000,8000,10000,12000,14000},
xticklabels={-2.0,0.0,2.0,4.0,6.0,8.0,10.0,12.0,14.0},
y grid style={darkgray176},
ymajorgrids,
ymin=0.0103946166250114, ymax=2.21905261272719,
ymode=log,
ytick style={color=black},
ytick={0.001,0.01,0.1,1,10,100},
yticklabels={
  \(\displaystyle {10^{-3}}\),
  \(\displaystyle {10^{-2}}\),
  \(\displaystyle {10^{-1}}\),
  \(\displaystyle {10^{0}}\),
  \(\displaystyle {10^{1}}\),
  \(\displaystyle {10^{2}}\)
}
]
\addplot [
  draw=royalblue28108204,
  fill=royalblue28108204,
  forget plot,
  mark=*, mark size=1,
  only marks,
  draw opacity=0,
 fill opacity=0.5
]
table{%
x  y
264.32 0.427806859780253
364.66 0.444484009311907
375.3 0.355660128667664
386.96 0.343269432991974
406.26 0.307975019059864
412.92 0.306670432331304
414.46 0.321158902719232
422.04 0.316356471077144
477.92 0.29074580675798
492.1 0.258273265081772
525.6 0.286387857021987
577.88 0.229272184801334
603.68 0.249404916408026
646.9 0.215582589134184
655.62 0.246369034305385
663.16 0.213280916168751
680.32 0.269784524044676
681.38 0.223308123115972
703.32 0.254020549891311
712.76 0.214238398224871
734.82 0.305916645928531
842.5 0.191659770974329
878.82 0.212730496984118
895.08 0.169383145898107
896.18 0.198709599964222
920.54 0.201474006298875
921.18 0.213465778327465
944.22 0.161668220887707
947.26 0.19350092085524
1086.08 0.177884809961145
1292.92 0.114032964316025
1294.28 0.122232678326655
1311.62 0.140488118570914
1326.3 0.115775625816309
1335.52 0.126485850008039
1423.28 0.121756570498947
1527.06 0.101222321634329
1638.22 0.0914435251825029
1659.02 0.112308698996691
1681.02 0.124990263012421
1736.86 0.085004181221538
1788.42 0.0880294786678716
1864.72 0.1071255685429
1911.2 0.0941001430080199
2080.34 0.0942326776384423
2100.48 0.104968085634367
2106.6 0.0943971246438057
2137.34 0.0872012783270749
2168.36 0.0897027409697891
2239.42 0.0808977415261108
2254.76 0.0816676929639913
2741.72 0.0798552480329176
2800.92 0.0570858062805065
2858.7 0.0603175493069252
2903.2 0.0633275228895684
2921.94 0.0598693098106491
2922.96 0.0657165373102141
2976.72 0.0613484752207961
3132.3 0.0629950121729971
3249.68 0.0615751892690854
3361.6 0.0452681258083442
3390.72 0.0515935648738026
3483.68 0.0470107685023736
3503.92 0.0532721138350081
3537.3 0.0461916811890175
3633.28 0.0559393579859902
3658.06 0.0448141295606094
3773.7 0.0560370682564066
3804.7 0.0531052767684115
4338.36 0.0405165659943221
4682.5 0.0403121698352036
4686.5 0.0368146690032345
4750.18 0.0400579283701412
4780.32 0.0362380577500318
4938.9 0.0392359927142959
4987.68 0.0313075068803643
4996.68 0.0383964329848947
5132.22 0.0374219277763844
5151.16 0.038020342677017
5415.56 0.0393364528201517
5575.22 0.033111821864268
5902.62 0.0342799802830101
6146.52 0.028761221210953
6212.6 0.0296684963960002
6456.06 0.0310588406494166
6863.24 0.0302571060046817
7269.2 0.0231857228865868
7366.32 0.0249146875726063
7374.08 0.0290723974680064
7805.46 0.025601114219245
8259.56 0.0293411592828646
8422.98 0.0242354462739304
8447.4 0.0182411551706714
9029.1 0.0182316252597657
9055.6 0.0157253646186244
9120.3 0.0201769120515845
10038.94 0.0154774705051151
10216.84 0.017594467773593
10421.32 0.0146626340808566
10920.18 0.0132644252424656
};
\addplot [
  draw=cadetblue80178158,
  fill=cadetblue80178158,
  forget plot,
  mark=*, mark size=1,
  only marks,
  draw opacity=0,
 fill opacity=0.5
]
table{%
x  y
208.36 0.633565898770519
209.16 0.632295593995823
215.3 0.599892893298719
217.66 0.622326007770062
225.08 0.6744632040443
227.9 0.572193990432501
253.64 0.571519500404337
275.68 0.707840420119435
285.84 0.706876442475177
332.44 0.560726018518014
387.18 0.493429287974948
419.16 0.519460268611052
419.38 0.437119316906443
431.24 0.537605925008045
448.7 0.447312267597527
454.08 0.826783371314551
467.22 0.752759114349074
514.26 0.337717246807563
534.86 0.331902931129634
538.62 0.414987519497441
539.1 0.397939748155169
548 0.357168100364044
569.92 0.495395640801326
585.96 0.577021028458707
604.74 0.664422492480486
613.54 0.617801365189046
630.28 0.406208989241479
636.16 0.401090994601074
674.86 0.462242406345924
727.8 0.403105327142812
730.26 0.507130232426748
736.6 0.287286578245708
755.42 0.404520883073846
864.56 0.33144349243178
877.72 0.460696607827565
906.3 0.293547277217866
921.8 0.275256860361307
928.08 0.617887130952524
933.1 0.307981574812877
949.12 0.272302485643738
960.26 0.267583927208973
1007.02 0.652514191239317
1021.54 0.521779312427989
1030.84 0.368702736332838
1079.06 0.740895615128913
1158.72 0.206106580820354
1179.12 0.332064323552109
1184.88 0.204167750418212
1201.58 0.311646057922124
1216.36 0.196750744314694
1257.6 0.47086445420117
1265.04 0.192961621434776
1294.16 0.170952400991235
1303.14 0.207717688921075
1325.6 0.162853704284028
1373.94 0.183199868111773
1378.98 0.189149791656871
1387.68 0.310702209042084
1389.92 0.667971858308513
1434.46 0.184855651913156
1434.66 0.155325358758436
1497.06 0.226461569608793
1507.86 0.179754455265573
1523.14 0.149500498383539
1563.88 0.280818661236397
1575.36 0.358149772397896
1587.24 0.36608681340116
1640.8 0.21647350782017
1641.88 0.252646159727974
1649.46 0.232944052023958
1651.88 0.133921492725585
1669.36 0.160831378726541
1673.66 0.205642339811112
1697.28 0.152541243224909
1701.46 0.157699202751613
1731.98 0.149653091682013
1734.02 0.156387275621278
1848.24 0.149418944575703
1877.22 0.34880206090982
1889.86 0.219572215735439
1932.1 0.134296677042373
1944.82 0.190818309708066
1945.66 0.200682771087242
1963.42 0.430959052595397
2057.04 0.28055766995807
2130.94 0.247093433778835
2194.44 0.130108609678431
2256.76 0.124977852823093
2304.56 0.398785672378767
2315.72 0.120144394535708
2379 0.142981615767565
2459.4 0.102619338361055
2707.8 0.141716469158639
2717.16 0.108050048437716
2750.54 0.168595509766076
2782.56 0.123293149291423
2887.26 0.187867425303112
2926.04 0.129318850654978
3082.9 0.191793746619034
3514.08 0.308329439058006
};
\addplot [
  draw=chocolate21910927,
  fill=chocolate21910927,
  forget plot,
  mark=*, mark size=1,
  only marks,
  draw opacity=0,
 fill opacity=0.5
]
table{%
x  y
21.18 0.99999999999978
23.44 0.999999999999857
23.48 0.99999999999986
23.56 0.999999999999854
23.88 0.999999999999863
23.88 0.999999999999863
24 0.999999999999862
24 0.999999999999862
24.1 0.999999999999865
24.1 0.999999999999865
24.1 0.999999999999865
24.1 0.999999999999865
24.1 0.999999999999865
24.1 0.999999999999865
24.1 0.999999999999865
24.1 0.999999999999865
24.1 0.999999999999865
24.1 0.999999999999865
24.1 0.999999999999865
24.1 0.999999999999865
24.1 0.999999999999865
24.1 0.999999999999865
24.1 0.999999999999865
24.1 0.999999999999865
24.1 0.999999999999865
24.1 0.999999999999865
24.1 0.999999999999865
24.1 0.999999999999865
24.1 0.999999999999865
24.1 0.999999999999865
24.1 0.999999999999865
24.1 0.999999999999865
24.1 0.999999999999865
24.1 0.999999999999865
24.1 0.999999999999865
24.1 0.999999999999865
24.1 0.999999999999865
24.1 0.999999999999865
24.1 0.999999999999865
24.1 0.999999999999865
30.48 1.00052997859207
56.44 0.892324337966214
65.96 0.790001785527894
77.64 0.74695721860881
111.68 0.797488452666468
120.22 0.630178111425087
129.76 0.693580938604459
156.72 0.972421867617079
193.1 0.709405691395951
209.6 0.630283607773187
221.28 0.577208109578358
226 0.735128082014352
233.52 0.476548166029283
236.74 0.480009168536489
268.18 0.906799608266314
278.98 0.47632323208656
346.04 0.493206538516545
400.44 0.597782677109018
423.22 0.462734412289465
427.78 0.450387714719575
446.94 0.403587734002728
455.88 0.383796593479486
456.44 0.297033050463181
511.02 0.561843007373489
548.48 0.555647714446305
560.94 0.32643684300428
594.82 0.437514064728061
633.06 0.264373085804833
664.56 0.416802720686476
754.42 0.319613212524695
760.46 0.458194933564034
944.74 0.512923461957536
1050.08 0.401930684756733
1184.7 0.234744790844635
1849.18 0.212502736207382
1917.4 0.552851927350736
2405.32 0.266720165077975
2442.16 0.517737246640793
2759.6 0.185979485709651
2789.46 0.320824280276505
2805.28 0.17420762946784
3791.16 0.246487278312724
4664.42 0.13971763946185
5389.16 0.136865565556043
6821.96 0.0373848538713827
8805.82 0.101492815540953
9754.34 0.130014843883942
};
\addplot [draw=purple11522131, fill=purple11522131, forget plot, mark=*, mark size=1, only marks, draw opacity=0,
 fill opacity=0.5]
table{%
x  y
318.22 0.506636649106128
364.52 0.500230484483383
374.38 0.48961258005109
376.26 0.513712378588516
383.8 0.457268724559049
401.02 0.474402369862907
436.8 0.475307677788005
438.08 0.46551087959822
462.62 0.395840257116506
493.36 0.452925067721991
919.12 0.353854282742153
1180.56 0.349666148351689
1201.16 0.365059169102206
1217.42 0.351797639510464
1223.98 0.422613497439609
1254.94 0.352472406592
1298.96 0.351648725178012
1331.14 0.35156021259453
1391.42 0.35164624409805
1418.48 0.349507379569627
1430.72 0.351874312752732
1434.54 0.363560759957797
1466.06 0.351358411266588
1468.06 0.351386408528851
1468.16 0.351386498700002
1468.16 0.351386498700002
1468.16 0.351386498700002
1468.52 0.351171385290678
1478.4 0.351342988880393
1478.54 0.351009375814841
1771.4 0.255828277532696
1836.14 0.263675715743399
1983.76 0.291059274510748
2191.28 0.296163449183721
2228.84 0.257998917347481
2257.9 0.340368563117911
2565.46 0.253877235024851
2867.38 0.252815593739864
3430.04 0.240493132222737
3529.28 0.211140521925032
3844.74 0.250687870508332
4037.1 0.250645789024279
4238.08 0.250612612223631
4863.16 0.211676197719397
4893.54 0.234650509324946
5617.32 0.216660037056147
5880.06 0.211456897475416
5890.22 0.211452613978539
5893 0.211452700411454
5893.12 0.211452709236125
5893.12 0.211452709236125
5893.12 0.211452709236125
5893.12 0.211452709236125
5893.12 0.211452709236125
5893.12 0.211452709236125
5893.12 0.211452709236125
5893.12 0.211452709236125
5893.12 0.211452709236125
5893.12 0.211452709236125
5893.12 0.211452709236125
5893.12 0.211452709236125
5893.12 0.211452709236125
5893.12 0.211452709236125
5893.12 0.211452709236125
5893.12 0.211452709236125
5893.12 0.211452709236125
5893.12 0.211452709236125
5893.12 0.211452709236125
5893.12 0.211452709236125
5893.12 0.211452709236125
5913.12 0.211460131460274
5995.52 0.209016060058814
5995.52 0.209016060058814
5995.52 0.209016060058814
5995.52 0.209016060058814
5995.52 0.209016060058814
5995.52 0.209016060058814
5995.52 0.209016060058814
5995.52 0.209016060058814
5995.52 0.209016060058814
5995.52 0.209016060058814
6975.08 0.18903796542284
6982.94 0.189050210569553
6983.68 0.18903793162047
6983.68 0.18903793162047
6983.68 0.18903793162047
6983.68 0.18903793162047
6983.68 0.18903793162047
6983.68 0.18903793162047
6983.68 0.18903793162047
7227.62 0.112621968195402
9882.46 0.119868476967011
};
\addplot [draw=black18, fill=black18, forget plot, mark=*, mark size=1, only marks, draw opacity=0,
 fill opacity=0.5]
table{%
x  y
24.1 0.999999999999865
70.3 0.685106717010937
72.18 0.680219986351619
74.78 0.67070955602341
76.56 0.669194087716129
79.76 0.652009677361207
81.16 0.648065798574816
83.92 0.637249999128466
85.54 0.623847179185065
88.8 0.626579403497279
92.26 0.617621922325458
95.48 0.61106867892368
98.2 0.609489955554655
101.32 0.603751133295828
103.74 0.594315140041451
105.34 0.58897756349978
111.94 0.583662500339519
116.82 0.578083528607985
120.86 0.57495244490658
125.84 0.568004648035821
128.56 0.558662326749403
132.02 0.556960178004963
134.22 0.54620215815071
140.42 0.539022862071154
144.08 0.527033778346122
150.54 0.514568784210452
167.02 0.49617952171966
169.52 0.492283248252622
173.9 0.481532358775813
185.14 0.468241911389809
190.22 0.456439754205673
200.94 0.443222079867523
207.02 0.435778137455672
215.8 0.427073392849934
227.62 0.419523789990323
236.98 0.414111513303146
246.26 0.407070472426135
263.04 0.395681771427877
281.56 0.386902985031692
290.2 0.376483594313575
314.3 0.362929057986722
323.64 0.348799181647151
333.92 0.341840602800968
355.26 0.330516853697789
370.04 0.32072229639127
401.96 0.297432696536708
417.32 0.29341259274819
439.72 0.279690809313861
497.2 0.263986993398039
536.36 0.254226549840377
542.12 0.243499735456981
591.42 0.22809613077329
613.38 0.219608100808268
676.1 0.199386326190842
697.18 0.194139423144587
736.22 0.185995508006419
806.76 0.178056248121189
846.78 0.166012266926309
963.62 0.153715524556284
1040.76 0.14549103463653
1083.56 0.142710236557795
1192.1 0.133224753580415
1301.58 0.127943137191366
1371.92 0.121409164605994
1436.68 0.116341964606295
1560.24 0.108288209048434
1608.92 0.103553154250901
1774.46 0.0961885119248831
1911.92 0.0876885263916435
2047.24 0.0813939885611151
2279.56 0.0757442855427076
2445.4 0.0704508997303385
2597.08 0.0656240948760418
2903.04 0.0606860263146079
3144.4 0.0550513973656187
3393.58 0.0479636853092477
3402.06 0.0517527352329034
3574.74 0.0459563238696212
4165.7 0.0416752487355907
4315.76 0.0400149135437421
4646.02 0.0372153335644535
5045.08 0.0334240530235503
5263.54 0.0314967324136304
5600.38 0.0299660885396439
6100.22 0.0275371465624002
6365.12 0.0258058619003401
6574.3 0.024508818997451
6912.7 0.0235748735634764
7468.64 0.0217585611519573
8006.26 0.0204411551875431
8405.4 0.0194520134341562
8890.78 0.0184294395035241
9392.06 0.0169398406445714
10549.02 0.0154334594190087
11481.78 0.0141997821432888
};
\addplot [draw=darkgray153, fill=darkgray153, forget plot, mark=*, mark size=1, only marks, draw opacity=0,
 fill opacity=0.5]
table{%
x  y
24.1 0.999999999999865
89.22 0.66302551573666
93.08 0.650410024530336
96.54 0.637488781797378
101.6 0.623844778009743
103.28 0.612006271755144
103.88 0.604135800993837
107.02 0.596905797815724
109.96 0.58339849263793
111.16 0.577900589921813
117.08 0.556682063557954
121.22 0.553210317778731
122.28 0.545978354476654
128.8 0.53874443469635
133.76 0.526318267887272
135.66 0.512458816579924
140.74 0.492431243396607
145.16 0.474689724329361
150.52 0.462799732596474
153.72 0.454051530938315
159.84 0.445243242758082
162.64 0.439846648574943
171.5 0.436645180042312
173.78 0.427988114588441
178.24 0.417395053626677
187.06 0.402758895900046
190.78 0.397540799887907
198.76 0.387222971535263
201.32 0.38916432752737
205.56 0.372120168479059
211.16 0.359612407182607
213.44 0.340393109995639
214.62 0.351932537483533
221.4 0.330726375057947
222.54 0.323164147462008
232.38 0.313543566182197
238.2 0.303449280369032
245.94 0.296616260665276
246.82 0.295225182450907
249.8 0.287923190268168
250.28 0.292546934724288
256.3 0.284488355282073
257.16 0.279415195946391
261.54 0.273524736561566
266.18 0.268414802573172
271.64 0.263954413778363
279.14 0.262587096318812
287.16 0.246485067261199
289.4 0.252064851833604
290.62 0.25889650985389
291.18 0.254620518715762
295.68 0.242543693622524
306.68 0.236366695099645
307.9 0.234013059508945
316.86 0.233346686937706
320.24 0.228802557583674
330.78 0.224269295776204
343.1 0.219314514917017
350.08 0.212775934877151
350.64 0.213224771255316
366.84 0.208501708038017
370.38 0.20591201903157
376.48 0.201185990903807
392.98 0.197956405946795
403.58 0.193691889767506
422.22 0.188978479770342
425.22 0.18530328118697
433.98 0.183696699545922
442.58 0.178494445095205
446 0.173362062807796
463 0.166907777381684
492.54 0.163799428238791
506.42 0.159005584761284
529.74 0.150570738436235
537.64 0.155095626879248
544.7 0.144150019903425
569.16 0.137329187698749
569.5 0.142174817000799
594.76 0.132757311991524
621.16 0.128274265039561
663.86 0.122456977286003
720.92 0.119528255436939
726.38 0.116304684927457
764.68 0.112496290500115
817.88 0.106154432270077
869.52 0.09948281437232
999.26 0.0935161852961517
1032.7 0.0887022842207346
1050.22 0.0846676555481492
1216.52 0.0782952772432562
1346.32 0.0714995054301827
1559.1 0.0649935724587566
1798.92 0.0575154667237924
2122.46 0.0506588825128073
2610.96 0.044350650005459
3327.84 0.0378538073562757
4280.02 0.0294762130976259
5733.92 0.0231340744666008
8577.22 0.0166014215469998
};
\addplot [
  draw=saddlebrown1356716,
  fill=saddlebrown1356716,
  forget plot,
  mark=*, mark size=1,
  only marks,
  draw opacity=0,
 fill opacity=0.5
]
table{%
x  y
375.36 0.516914016590904
421.64 0.437847766614225
421.9 0.433923364797401
427.7 0.429565820534802
429.24 0.425432804847826
435.84 0.418537219213063
439.18 0.415359703830104
443.24 0.403765595705311
443.64 0.396546820906386
452.96 0.387587921113165
455.68 0.374182526627961
460.26 0.377705590836546
472.62 0.356605588642063
480.98 0.347856367585566
487.94 0.332787961601512
500.24 0.324495027623478
506.46 0.315552084404071
522.74 0.310531394157134
532.64 0.302154771422671
551.08 0.29074624960949
574.82 0.28327166912214
584.4 0.265345879530833
607.92 0.254039927677155
622.86 0.24502420685115
644.06 0.238009222650772
665.66 0.228086444096535
697.9 0.213544386147411
702.82 0.204027518203201
731.78 0.189431058616626
763.56 0.177720895644471
768.34 0.170607942879518
798.82 0.16337836618299
820.04 0.158160913677792
834.84 0.153824770992494
868.14 0.148666822327679
900.04 0.147882736336847
932.62 0.14052459029364
944.36 0.133674725994743
966.74 0.130626937029648
995.4 0.12119360177604
1033.24 0.11838746937042
1090.5 0.115462579932347
1099.96 0.112468273677544
1127.88 0.11015341724387
1167.94 0.106849066504645
1177.7 0.105914973303467
1215.8 0.103559776373589
1234.56 0.100274485143733
1245.56 0.0971255376603645
1298.4 0.0929857913883158
1326.58 0.0906752923957337
1401.2 0.0858210780352794
1445.28 0.0825617229124751
1503.14 0.0807658011450964
1571.88 0.0778092119870903
1601.36 0.0757211129451405
1669.14 0.0737013947175062
1774 0.0715357388348069
1816.2 0.0709454453500374
1838.14 0.0692897864021775
1881.32 0.0634670547921319
1885 0.0660776910809798
2000.1 0.0616274824782506
2166.96 0.058935587434457
2194 0.0573062203242847
2280.76 0.0552453170019738
2336.54 0.0532384512297571
2510.64 0.0505125292605886
2536.56 0.048888687513162
2655.32 0.0475113761725774
2737.06 0.0457364701940395
2851.6 0.0442690418241429
2875.54 0.0426323113549072
3083.66 0.0411788563385927
3195.94 0.0402226560775179
3385.02 0.0376133424827729
3434.98 0.0389447347027832
3564.56 0.0364327558623579
3616.56 0.0352061758122012
3822.44 0.0340284694980253
4082.86 0.0330578970831364
4180.78 0.0314797703570108
4294.18 0.0304267975947862
4437.14 0.0299637110908754
4613.96 0.0288428240335884
4751.76 0.0276643389429212
4975.98 0.0271071087230791
5155.66 0.0260055972653924
5374.78 0.0253934463018442
5662.74 0.0246159234805905
5970.6 0.023776122317647
6015.52 0.0229174863580978
6293.98 0.0222174626895817
6477.04 0.0210211804923276
6532 0.0215910749657251
6856.42 0.0206387864340862
7246.32 0.020255103269617
7720.8 0.0194919279355704
8054.06 0.0189465535074979
8463.74 0.0181922078049376
};
\addplot [very thick, royalblue28108204]
table {%
264.32 0.448163854855411
371.954949494949 0.356933753216909
479.589898989899 0.298159181377111
587.224848484849 0.256679892646525
694.859797979798 0.225642928986524
802.494747474748 0.2014481451079
910.129696969697 0.182004857676805
1017.76464646465 0.166008146995874
1125.3995959596 0.152597809316332
1233.03454545455 0.141181940611267
1340.66949494949 0.131338894875886
1448.30444444444 0.122759596857735
1555.93939393939 0.115211978964163
1663.57434343434 0.108518188725145
1771.20929292929 0.102539492264011
1878.84424242424 0.0971659886733443
1986.47919191919 0.0923094281335774
2094.11414141414 0.0878980881581215
2201.74909090909 0.0838730479551454
2309.38404040404 0.080185433093327
2417.01898989899 0.0767943465536091
2524.65393939394 0.0736652937305697
2632.28888888889 0.0707689684540739
2739.92383838384 0.0680803066174904
2847.55878787879 0.0655777407346183
2955.19373737374 0.0632426071475344
3062.82868686869 0.0610586704696909
3170.46363636364 0.0590117389691465
3278.09858585859 0.0570893511500987
3385.73353535354 0.0552805185573074
3493.36848484848 0.053575513334243
3601.00343434343 0.0519656916723037
3708.63838383838 0.0504433462452232
3816.27333333333 0.0490015822053343
3923.90828282828 0.0476342124512919
4031.54323232323 0.0463356687496586
4139.17818181818 0.045100925970266
4246.81313131313 0.0439254372249656
4354.44808080808 0.0428050781163341
4462.08303030303 0.0417360986331861
4569.71797979798 0.0407150814930034
4677.35292929293 0.0397389059423961
4784.98787878788 0.0388047161967866
4892.62282828283 0.0379098938382913
5000.25777777778 0.0370520336029617
5107.89272727273 0.0362289220803114
5215.52767676768 0.0354385189234671
5323.16262626263 0.0346789402305121
5430.79757575758 0.0339484438091598
5538.43252525253 0.0332454160797955
5646.06747474747 0.0325683604077538
5753.70242424242 0.03191588668572
5861.33737373737 0.0312867020124033
5968.97232323232 0.0306796023349331
6076.60727272727 0.0300934649404733
6184.24222222222 0.0295272416978657
6291.87717171717 0.0289799529631632
6399.51212121212 0.0284506820740551
6507.14707070707 0.0279385703677356
6614.78202020202 0.0274428126649611
6722.41696969697 0.0269626531701034
6830.05191919192 0.0264973817430972
6937.68686868687 0.0260463305044519
7045.32181818182 0.0256088707390726
7152.95676767677 0.0251844100686065
7260.59171717172 0.0247723898654961
7368.22666666667 0.0243722828849413
7475.86161616162 0.0239835910936175
7583.49656565657 0.023605843676316
7691.13151515151 0.0232385952037049
7798.76646464646 0.0228814239462039
7906.40141414141 0.0225339303205427
8014.03636363636 0.0221957354569671
8121.67131313131 0.0218664798762901
8229.30626262626 0.0215458222670799
8336.94121212121 0.0212334383542428
8444.57616161616 0.0209290198511241
8552.21111111111 0.0206322734880167
8659.84606060606 0.0203429201106504
8767.48101010101 0.0200606938428469
8875.11595959596 0.0197853413080714
8982.75090909091 0.019516620905101
9090.38585858586 0.0192543021334689
9198.02080808081 0.0189981649647365
9305.65575757576 0.0187479992560008
9413.29070707071 0.0185036042023614
9520.92565656566 0.0182647878253611
9628.56060606061 0.0180313664946702
9736.19555555556 0.0178031644805214
9843.8305050505 0.0175800135346128
9951.46545454545 0.0173617524973872
10059.1004040404 0.0171482269297724
10166.7353535354 0.0169392887676215
10274.3703030303 0.0167347959972383
10382.0052525253 0.0165346123505013
10489.6402020202 0.0163386070182193
10597.2751515152 0.016146654380459
10704.9101010101 0.0159586337526841
10812.5450505051 0.0157744291466348
10920.18 0.0155939290449582
};
\addplot [very thick, cadetblue80178158]
table {%
208.36 0.688296988436722
241.751111111111 0.652667367611376
275.142222222222 0.621054060567482
308.533333333333 0.592786151955219
341.924444444444 0.567329289436614
375.315555555556 0.54425690114169
408.706666666667 0.523225784253552
442.097777777778 0.503957146658179
475.488888888889 0.486222263513235
508.88 0.469831676019579
542.271111111111 0.454627024611385
575.662222222222 0.440474825795859
609.053333333333 0.427261685796508
642.444444444444 0.414890583214745
675.835555555556 0.403277953862011
709.226666666667 0.392351383162695
742.617777777778 0.382047763133807
776.008888888889 0.372311807945171
809.4 0.363094848765356
842.791111111111 0.354353848025238
876.182222222222 0.346050587488822
909.573333333333 0.3381509950789
942.964444444444 0.330624583292913
976.355555555555 0.323443977988623
1009.74666666667 0.316584520836472
1043.13777777778 0.310023932196036
1076.52888888889 0.303742023845599
1109.92 0.297720453071562
1143.31111111111 0.291942511251638
1176.70222222222 0.286392941348713
1210.09333333333 0.281057779750268
1243.48444444444 0.275924218700884
1276.87555555556 0.270980486227837
1310.26666666667 0.266215740986601
1343.65777777778 0.261619979880588
1377.04888888889 0.257183956658194
1410.44 0.252899109976057
1443.83111111111 0.24875749965273
1477.22222222222 0.244751750031602
1510.61333333333 0.240874999533477
1544.00444444444 0.237120855613987
1577.39555555556 0.233483354453754
1610.78666666667 0.229956924803981
1644.17777777778 0.226536355489987
1677.56888888889 0.223216766142786
1710.96 0.219993580786105
1744.35111111111 0.216862503955093
1777.74222222222 0.213819499064618
1811.13333333333 0.210860768780747
1844.52444444444 0.20798273717969
1877.91555555556 0.205182033504843
1911.30666666667 0.202455477355405
1944.69777777778 0.199800065159722
1978.08888888889 0.197212957803696
2011.48 0.194691469299412
2044.87111111111 0.192233056392177
2078.26222222222 0.189835309015475
2111.65333333333 0.187495941513266
2145.04444444444 0.185212784557802
2178.43555555556 0.182983777698729
2211.82666666667 0.180806962486064
2245.21777777778 0.17868047611552
2278.60888888889 0.176602545549963
2312 0.17457148207541
2345.39111111111 0.172585676254148
2378.78222222222 0.170643593241185
2412.17333333333 0.168743768433557
2445.56444444444 0.166884803424903
2478.95555555556 0.165065362240339
2512.34666666667 0.163284167828975
2545.73777777778 0.161539998793527
2579.12888888889 0.159831686338325
2612.52 0.158158111418704
2645.91111111111 0.156518202076291
2679.30222222222 0.154910930946029
2712.69333333333 0.153335312922042
2746.08444444444 0.151790402970525
2779.47555555556 0.15027529407885
2812.86666666667 0.148789115331006
2846.25777777778 0.147331030100272
2879.64888888889 0.145900234350803
2913.04 0.144495955040466
2946.43111111111 0.143117448617879
2979.82222222222 0.141763999607176
3013.21333333333 0.140434919274511
3046.60444444444 0.139129544370799
3079.99555555556 0.137847235945604
3113.38666666667 0.136587378227474
3146.77777777778 0.135349377566376
3180.16888888889 0.134132661434214
3213.56 0.132936677479704
3246.95111111111 0.13176089263415
3280.34222222222 0.130604792264933
3313.73333333333 0.129467879373726
3347.12444444444 0.128349673836682
3380.51555555556 0.127249711684038
3413.90666666667 0.12616754441673
3447.29777777778 0.125102738357812
3480.68888888889 0.124054874036606
3514.08 0.123023545603653
};
\addplot [very thick, chocolate21910927]
table {%
21.18 1.00880678779584
119.494747474747 0.739236170135995
217.809494949495 0.622828762569519
316.124242424242 0.550877604196276
414.43898989899 0.49988291747397
512.753737373737 0.460974298542207
611.068484848485 0.429868518453984
709.383232323232 0.404181960636924
807.69797979798 0.382457830454264
906.012727272727 0.363744121764653
1004.32747474747 0.347386531467374
1102.64222222222 0.332917279505363
1200.95696969697 0.319991156672476
1299.27171717172 0.308346669626546
1397.58646464646 0.297781358419414
1495.90121212121 0.288135525459199
1594.21595959596 0.279281168340787
1692.53070707071 0.271114247566438
1790.84545454545 0.263549157142502
1889.1602020202 0.256514689123175
1987.47494949495 0.249951035015306
2085.7896969697 0.243807521687189
2184.10444444444 0.238040877177489
2282.41919191919 0.23261388510888
2380.73393939394 0.227494328332329
2479.04868686869 0.222654150747912
2577.36343434343 0.218068785729207
2675.67818181818 0.213716613201956
2773.99292929293 0.209578517099611
2872.30767676768 0.205637521880485
2970.62242424242 0.201878491866853
3068.93717171717 0.198287880910563
3167.25191919192 0.194853522682018
3265.56666666667 0.191564453983013
3363.88141414141 0.188410765083836
3462.19616161616 0.185383472312546
3560.51090909091 0.182474409074101
3658.82565656566 0.17967613221745
3757.1404040404 0.176981841250303
3855.45515151515 0.174385308361206
3953.7698989899 0.171880817574662
4052.08464646465 0.169463111658221
4150.39939393939 0.167127345636692
4248.71414141414 0.164869045959919
4347.02888888889 0.162684074526373
4445.34363636364 0.160568596892299
4543.65838383838 0.158519054100981
4641.97313131313 0.156532137653268
4740.28787878788 0.154604767212344
4838.60262626263 0.15273407069552
4936.91737373737 0.150917366455886
5035.23212121212 0.149152147298646
5133.54686868687 0.147436066112327
5231.86161616162 0.145766922924975
5330.17636363636 0.144142653220828
5428.49111111111 0.142561317374513
5526.80585858586 0.141021091078271
5625.12060606061 0.139520256653477
5723.43535353535 0.138057195151253
5821.7501010101 0.136630379158644
5920.06484848485 0.135238366236886
6018.3795959596 0.133879792927
6116.69434343434 0.1325533692655
6215.00909090909 0.131257873759584
6313.32383838384 0.129992148776872
6411.63858585859 0.128755096309809
6509.95333333333 0.127545674079161
6608.26808080808 0.126362891944937
6706.58282828283 0.125205808596411
6804.89757575758 0.124073528495889
6903.21232323232 0.122965199053519
7001.52707070707 0.121880008012722
7099.84181818182 0.120817181027917
7198.15656565657 0.119775979418005
7296.47131313131 0.118755698080711
7394.78606060606 0.117755663554324
7493.10080808081 0.116775232214656
7591.41555555556 0.115813788596194
7689.7303030303 0.114870743827442
7788.04505050505 0.113945534171375
7886.3597979798 0.113037619662739
7984.67454545455 0.112146482834692
8082.98929292929 0.111271627527921
8181.30404040404 0.110412577776006
8279.61878787879 0.109568876761294
8377.93353535354 0.108740085836086
8476.24828282828 0.107925783604347
8574.56303030303 0.107125565059558
8672.87777777778 0.106339040774698
8771.19252525253 0.105565836140661
8869.50727272727 0.104805590649724
8967.82202020202 0.104057957220942
9066.13676767677 0.103322601564598
9164.45151515152 0.10259920158306
9262.76626262626 0.10188744680561
9361.08101010101 0.101187037854979
9459.39575757576 0.10049768594351
9557.71050505051 0.0998191123970247
9656.02525252525 0.0991510482046045
9754.34 0.0984932335926346
};
\addplot [very thick, purple11522131]
table {%
318.22 0.490748449619504
414.828484848485 0.467870377420038
511.43696969697 0.448534162503357
608.045454545455 0.431859914998674
704.653939393939 0.417244151703105
801.262424242424 0.404262241189159
897.870909090909 0.392606143353013
994.479393939394 0.382046040503643
1091.08787878788 0.37240623068721
1187.69636363636 0.363549525058715
1284.30484848485 0.355366841080315
1380.91333333333 0.347770065555171
1477.52181818182 0.340687036199279
1574.1303030303 0.334057933360746
1670.73878787879 0.327832633639617
1767.34727272727 0.321968734294031
1863.95575757576 0.316430054814234
1960.56424242424 0.311185484071843
2057.17272727273 0.306208081831659
2153.78121212121 0.301474370261795
2250.3896969697 0.296963769277367
2346.99818181818 0.292658142109774
2443.60666666667 0.2885414262988
2540.21515151515 0.28459933157199
2636.82363636364 0.280819090598366
2733.43212121212 0.277189251908755
2830.04060606061 0.273699506719229
2926.64909090909 0.270340543221432
3023.25757575758 0.26710392328363
3119.86606060606 0.263981977558557
3216.47454545455 0.260967715803491
3313.08303030303 0.258054749845842
3409.69151515151 0.255237227118294
3506.3 0.252509773074002
3602.90848484848 0.249867441098828
3699.51696969697 0.247305668782141
3796.12545454545 0.244820239604147
3892.73393939394 0.242407249256367
3989.34242424242 0.240063075940724
4085.95090909091 0.23778435409794
4182.55939393939 0.23556795110227
4279.16787878788 0.233410946530802
4375.77636363636 0.231310613674485
4472.38484848485 0.229264403007131
4568.99333333333 0.227269927369556
4665.60181818182 0.225324948660421
4762.2103030303 0.223427365854198
4858.81878787879 0.221575204191167
4955.42727272727 0.219766605404996
5052.03575757576 0.217999818871119
5148.64424242424 0.216273193574112
5245.25272727273 0.214585170805148
5341.86121212121 0.212934277511651
5438.4696969697 0.211319120230745
5535.07818181818 0.209738379546338
5631.68666666667 0.208190805016739
5728.29515151515 0.206675210525887
5824.90363636364 0.205190470016625
5921.51212121212 0.203735513569111
6018.12060606061 0.202309323791557
6114.72909090909 0.200910932494047
6211.33757575758 0.199539417619322
6307.94606060606 0.198193900407195
6404.55454545455 0.196873542771659
6501.16303030303 0.195577544871943
6597.77151515152 0.194305142860619
6694.38 0.193055606793581
6790.98848484849 0.191828238688208
6887.59696969697 0.190622370717332
6984.20545454545 0.189437363527836
7080.81393939394 0.188272604673753
7177.42242424242 0.187127507154689
7274.03090909091 0.186001508051224
7370.63939393939 0.184894067249719
7467.24787878788 0.183804666249623
7563.85636363636 0.182732807047
7660.46484848485 0.181678011088527
7757.07333333333 0.180639818290731
7853.68181818182 0.179617786119661
7950.2903030303 0.178611488726617
8046.89878787879 0.177620516135896
8143.50727272727 0.176644473480882
8240.11575757576 0.175682980285078
8336.72424242424 0.174735669784959
8433.33272727273 0.173802188291792
8529.94121212121 0.172882194589761
8626.5496969697 0.171975359367977
8723.15818181818 0.171081364684113
8819.76666666667 0.170199903457596
8916.37515151515 0.16933067899042
9012.98363636364 0.168473404513826
9109.59212121212 0.16762780275918
9206.20060606061 0.166793605551541
9302.80909090909 0.165970553424495
9399.41757575758 0.165158395254944
9496.02606060606 0.164356887916634
9592.63454545454 0.16356579595128
9689.24303030303 0.162784891256241
9785.85151515151 0.162013952787758
9882.46 0.161252766278836
};
\addplot [very thick, black18]
table {%
24.1 0.927140390577046
139.834141414141 0.531376597343618
255.568282828283 0.389346838008955
371.302424242424 0.311397014116397
487.036565656566 0.260874260498005
602.770707070707 0.225027185833285
718.504848484849 0.198083250343291
834.23898989899 0.176999832138306
949.973131313131 0.160003295931198
1065.70727272727 0.145982403796363
1181.44141414141 0.134201977240052
1297.17555555556 0.124154435562755
1412.9096969697 0.115477074427599
1528.64383838384 0.107903261986511
1644.37797979798 0.101232271849312
1760.11212121212 0.0953098986585024
1875.84626262626 0.0900155868249197
1991.5804040404 0.0852536401055122
2107.31454545455 0.0809470698118155
2223.04868686869 0.0770331965028959
2338.78282828283 0.0734604453203794
2454.51696969697 0.0701859713692976
2570.25111111111 0.067173873385383
2685.98525252525 0.0643938315260655
2801.71939393939 0.0618200556856132
2917.45353535354 0.059430464368274
3033.18767676768 0.0572060369467582
3148.92181818182 0.0551302978452593
3264.65595959596 0.0531889021861391
3380.3901010101 0.0513693002510883
3496.12424242424 0.0496604637284883
3611.85838383838 0.0480526608126557
3727.59252525253 0.0465372702362507
3843.32666666667 0.0451066265618032
3959.06080808081 0.0437538907455443
4074.79494949495 0.0424729412665993
4190.52909090909 0.0412582820937866
4306.26323232323 0.0401049645174697
4421.99737373737 0.0390085204607671
4537.73151515152 0.0379649053437323
4653.46565656566 0.0369704489360168
4769.1997979798 0.0360218129205014
4884.93393939394 0.0351159541193092
5000.66808080808 0.0342500925172925
5116.40222222222 0.0334216833662488
5232.13636363636 0.0326283927732669
5347.87050505051 0.0318680762745015
5463.60464646465 0.0311387599758232
5579.33878787879 0.0304386239077001
5695.07292929293 0.0297659872961005
5810.80707070707 0.0291192954963473
5926.54121212121 0.0284971083744319
6042.27535353535 0.0278980899516993
6158.0094949495 0.0273209991551535
6273.74363636364 0.0267646815377937
6389.47777777778 0.026228061852109
6505.21191919192 0.0257101373757094
6620.94606060606 0.0252099719015397
6736.6802020202 0.0247266903166047
6852.41434343434 0.0242594737029385
6968.14848484849 0.0238075549029632
7083.88262626263 0.0233702144986007
7199.61676767677 0.0229467771597287
7315.35090909091 0.0225366083229423
7431.08505050505 0.0221391111662387
7546.81919191919 0.0217537238492754
7662.55333333333 0.0213799169923666
7778.28747474748 0.0210171913704386
7894.02161616162 0.02066507580084
8009.75575757576 0.0203231252062389
8125.4898989899 0.0199909188358911
8241.22404040404 0.019668058630364
8356.95818181818 0.0193541677163879
8472.69232323232 0.0190488890199036
8588.42646464647 0.0187518839866108
8704.16060606061 0.018462831400415
8819.89474747475 0.0181814262911396
8935.62888888889 0.01790737892373
9051.36303030303 0.01764041386194
9167.09717171717 0.0173802691001741
9282.83131313131 0.0171266952577652
9398.56545454545 0.0168794548305101
9514.2995959596 0.0166383214947701
9630.03373737374 0.0164030794598803
9745.76787878788 0.0161735228649987
9861.50202020202 0.0159494552168779
9977.23616161616 0.0157306888653561
10092.9703030303 0.01551704451365
10208.7044444444 0.0153083507607819
10324.4385858586 0.0151044436737124
10440.1727272727 0.0149051663869499
10555.9068686869 0.0147103687276029
10671.641010101 0.0145199068640084
10787.3751515152 0.0143336429762268
10903.1092929293 0.0141514449468302
11018.8434343434 0.0139731860705448
11134.5775757576 0.013798744781418
11250.3117171717 0.0136280043962902
11366.0458585859 0.0134608528734465
11481.78 0.0132971825854111
};
\addplot [very thick, darkgray153]
table {%
24.1 1.73895217911013
110.495151515152 0.553132515451985
196.890303030303 0.352477764460546
283.285454545455 0.264188919073136
369.680606060606 0.213468235326972
456.075757575758 0.180181882833078
542.470909090909 0.15650083871116
628.866060606061 0.138711331001461
715.261212121212 0.124812804410497
801.656363636364 0.113627162925767
888.051515151515 0.10441318254689
974.446666666667 0.0966800040481425
1060.84181818182 0.090089009923422
1147.23696969697 0.0843986744103366
1233.63212121212 0.0794318650812775
1320.02727272727 0.0750555805046091
1406.42242424242 0.071167918917173
1492.81757575758 0.0676894273471094
1579.21272727273 0.0645571991888597
1665.60787878788 0.0617207495430776
1752.00303030303 0.0591390715047093
1838.39818181818 0.056778495615912
1924.79333333333 0.0546111071076648
2011.18848484848 0.052613557851312
2097.58363636364 0.0507661623793149
2183.97878787879 0.0490522015012227
2270.37393939394 0.0474573797566651
2356.76909090909 0.0459693983293677
2443.16424242424 0.044577615638289
2529.55939393939 0.0432727752284272
2615.95454545455 0.0420467858364302
2702.3496969697 0.0408925422800855
2788.74484848485 0.0398037785652798
2875.14 0.0387749466223949
2961.53515151515 0.037801115584066
3047.9303030303 0.0368778876418401
3134.32545454545 0.036001327371717
3220.72060606061 0.0351679020696686
3307.11575757576 0.0343744311395909
3393.51090909091 0.0336180429651135
3479.90606060606 0.0328961380006489
3566.30121212121 0.0322063570561794
3652.69636363636 0.031546553939605
3739.09151515152 0.0309147717712848
3825.48666666667 0.030309222406223
3911.88181818182 0.0297282684966757
3998.27696969697 0.0291704078067665
4084.67212121212 0.0286342594548262
4171.06727272727 0.0281185518116099
4257.46242424242 0.02762211182561
4343.85757575758 0.0271438555822048
4430.25272727273 0.0266827799328102
4516.64787878788 0.0262379550546627
4603.04303030303 0.0258085178222919
4689.43818181818 0.0253936658888454
4775.83333333333 0.0249926523898153
4862.22848484849 0.0246047811938486
4948.62363636364 0.0242294026355893
5035.01878787879 0.0238659096742202
5121.41393939394 0.0235137344287893
5207.80909090909 0.0231723450477436
5294.20424242424 0.0228412428755221
5380.59939393939 0.0225199598837126
5466.99454545455 0.0222080563382935
5553.3896969697 0.0219051186779371
5639.78484848485 0.0216107575813479
5726.18 0.0213246062042041
5812.57515151515 0.0210463185685262
5898.9703030303 0.0207755680892617
5985.36545454545 0.0205120462245908
6071.76060606061 0.0202554612379562
6158.15575757576 0.0200055370611366
6244.55090909091 0.0197620122488379
6330.94606060606 0.0195246390162885
6417.34121212121 0.0192931823522263
6503.73636363636 0.0190674192004492
6590.13151515152 0.0188471377038039
6676.52666666667 0.0186321365051055
6762.92181818182 0.0184222241000316
6849.31696969697 0.0182172182375207
6935.71212121212 0.0180169453636422
7022.10727272727 0.0178212401052919
7108.50242424242 0.0176299447904126
7194.89757575758 0.0174429090017511
7281.29272727273 0.017259989161437
7367.68787878788 0.0170810481439209
7454.08303030303 0.0169059549150293
7540.47818181818 0.0167345841950974
7626.87333333333 0.0165668161443187
7713.26848484849 0.0164025360686162
7799.66363636364 0.016241634144483
7886.05878787879 0.0160840051613772
7972.45393939394 0.0159295482803725
8058.84909090909 0.0157781668078765
8145.24424242424 0.0156297679833268
8231.63939393939 0.0154842627798643
8318.03454545455 0.0153415657170641
8404.4296969697 0.0152015946848789
8490.82484848485 0.0150642707780169
8577.22 0.0149295181400368
};
\addplot [very thick, saddlebrown1356716]
table {%
375.36 0.502449612458438
457.060808080808 0.375029311279734
538.761616161616 0.296349903538581
620.462424242424 0.243660085295679
702.163232323232 0.206254049129969
783.86404040404 0.178505045452515
865.564848484849 0.15720235718272
947.265656565657 0.140393539344294
1028.96646464646 0.12682950571267
1110.66727272727 0.115677345591335
1192.36808080808 0.106362181360526
1274.06888888889 0.0984755007765902
1355.7696969697 0.0917196790021804
1437.47050505051 0.0858731440688625
1519.17131313131 0.0807677979553804
1600.87212121212 0.0762739699485817
1682.57292929293 0.0722901417597953
1764.27373737374 0.068735777529337
1845.97454545455 0.0655462227559041
1927.67535353535 0.062669011518059
2009.37616161616 0.0600611508668282
2091.07696969697 0.0576870951247341
2172.77777777778 0.055517215031336
2254.47858585859 0.0535266269855003
2336.17939393939 0.0516942878200444
2417.8802020202 0.050002287778698
2499.58101010101 0.0484352931127052
2581.28181818182 0.0469801028068006
2662.98262626263 0.0456252932102655
2744.68343434343 0.0443609309882905
2826.38424242424 0.0431783396216011
2908.08505050505 0.0420699082085757
2989.78585858586 0.0410289339339238
3071.48666666667 0.0400494915178733
3153.18747474748 0.0391263244295943
3234.88828282828 0.0382547537657688
3316.58909090909 0.0374306015510806
3398.2898989899 0.0366501258779756
3479.99070707071 0.0359099658164779
3561.69151515152 0.0352070944265932
3643.39232323232 0.0345387785221625
3725.09313131313 0.0339025440856255
3806.79393939394 0.0332961464327943
3888.49474747475 0.0327175443866589
3970.19555555556 0.0321648778480252
4051.89636363636 0.031636448254979
4133.59717171717 0.0311307015079024
4215.29797979798 0.0306462130059542
4296.99878787879 0.0301816744976948
4378.6995959596 0.0297358824952794
4460.4004040404 0.0293077280403191
4542.10121212121 0.0288961876415914
4623.80202020202 0.0285003152315441
4705.50282828283 0.0281192350108798
4787.20363636364 0.027752135069287
4868.90444444444 0.027398261686163
4950.60525252525 0.0270569142285239
5032.30606060606 0.0267274405745799
5114.00686868687 0.0264092330010596
5195.70767676768 0.0261017244805383
5277.40848484848 0.0258043853420065
5359.10929292929 0.0255167202538992
5440.8101010101 0.0252382654939411
5522.51090909091 0.0249685864745849
5604.21171717172 0.0247072754966335
5685.91252525253 0.0244539497069393
5767.61333333333 0.0242082492389305
5849.31414141414 0.0239698355172042
5931.01494949495 0.0237383897095856
6012.71575757576 0.0235136113119405
6094.41656565657 0.0232952168526815
6176.11737373737 0.0230829387053498
6257.81818181818 0.0228765239989223
6339.51898989899 0.0226757336166132
6421.2197979798 0.0224803412749139
6502.92060606061 0.022290132675488
6584.62141414141 0.0221049047232979
6666.32222222222 0.0219244648050213
6748.02303030303 0.0217486301224131
6829.72383838384 0.0215772270758037
6911.42464646465 0.0214100906933987
6993.12545454545 0.0212470641024653
7074.82626262626 0.0210879980388712
7156.52707070707 0.0209327503917746
7238.22787878788 0.0207811857805665
7319.92868686869 0.0206331751614373
7401.62949494949 0.0204885954611779
7483.3303030303 0.0203473292360469
7565.03111111111 0.0202092643537263
7646.73191919192 0.0200742936965686
7728.43272727273 0.0199423148844898
7810.13353535354 0.0198132300160146
7891.83434343434 0.0196869454260991
7973.53515151515 0.0195633714594819
8055.23595959596 0.0194424222584145
8136.93676767677 0.0193240155637187
8218.63757575758 0.0192080725282083
8300.33838383839 0.0190945175415878
8382.03919191919 0.0189832780660132
8463.74 0.0188742844815681
};
\addplot [draw=black, fill=black, mark=x, very thick, mark size=2.5pt, only marks]
table{%
x  y
95.36 0.721864865467604
375.36 0.516914016590902
1468.16 0.351386498699998
5893.12 0.211452709236117
};
