# Supplementary material for: Swarm Reinforcement Learning For Adaptive Mesh Refinement
Source: arXiv:2304.00818 source file (2023-10-09)
Supplement: Supplementary file 16 [file group_additional_metrics_r5.tex]

\nextgroupplot[
ylabel shift = -0.2cm,
title style={yshift=-0.2cm},
height=4.5cm,
width=0.50\textwidth,
ylabel={Top $0.1\,\%$ Error},
title={Heat Diffusion},
scaled x ticks=false,
clip marker paths=true,
legend cell align={left},
legend style={fill opacity=0.8, draw opacity=1, text opacity=1, draw=lightgray204},
log basis y={10},
tick align=outside,
tick pos=left,
x grid style={darkgray176},
xlabel={Elements \(\displaystyle (\times 10^3)\)},
xmajorgrids,
xmin=-308.119, xmax=6823.819,
xtick style={color=black},
xtick={-1000,0,1000,2000,3000,4000,5000,6000,7000},
xticklabels={-1.0,0.0,1.0,2.0,3.0,4.0,5.0,6.0,7.0},
y grid style={darkgray176},
ymajorgrids,
ymin=0.00147569754614594, ymax=1.37394249050127,
ymode=log,
ytick style={color=black},
ytick={0.0001,0.001,0.01,0.1,1,10,100},
yticklabels={
  \(\displaystyle {10^{-4}}\),
  \(\displaystyle {10^{-3}}\),
  \(\displaystyle {10^{-2}}\),
  \(\displaystyle {10^{-1}}\),
  \(\displaystyle {10^{0}}\),
  \(\displaystyle {10^{1}}\),
  \(\displaystyle {10^{2}}\)
}
]
\addplot [
  draw=royalblue28108204,
  fill=royalblue28108204,
  forget plot,
  mark=*, mark size=1,
  only marks,
  draw opacity=0,
 fill opacity=0.5
]
table{%
x  y
139.38 0.141727507812422
139.76 0.146098427726618
141.48 0.140651100188536
143.58 0.133244298855064
150.68 0.1432470564131
155.14 0.132705303702269
162.66 0.123596182468722
164.36 0.114937991634248
167.18 0.120494646374273
186.18 0.113704084595436
206.44 0.126145643346103
208.62 0.10999465457548
233.56 0.0957984160018061
243.4 0.0906388743214112
257.16 0.0890373864140342
259.46 0.0909390418418387
261.2 0.109093604107314
261.48 0.112978103624495
263.66 0.0926765565482452
266.12 0.100208685519237
273.46 0.0722093474901027
274.54 0.0805749124499016
281.58 0.0939895344618702
286.96 0.0866910611955713
289.96 0.0816672787947995
308.42 0.0703620031422089
309.22 0.0686088846766927
315.16 0.0886063694778614
372.08 0.0756260945317814
383.48 0.0639622968589339
386.5 0.0643612029241434
401.98 0.0730347827761346
403 0.085032501595148
405.76 0.0543242290037206
414.72 0.0484776807351366
433.62 0.0632304269151397
440.96 0.0479996257359117
448.68 0.050282267990018
450.14 0.0447905915294338
485.02 0.0627838862070099
501.06 0.0429890567878646
520.14 0.0503903536024616
520.24 0.048650141148878
595.92 0.041686288088318
628.98 0.0419459821316719
683.56 0.0341401717550158
733.04 0.0285572776103424
738.38 0.028580114400961
757.18 0.0324712851393253
781.6 0.0289414267208989
940.74 0.0589563674956909
974.4 0.0786174499327058
1146.74 0.0203306118188853
1284.9 0.0201918138673393
1457.46 0.0148459275476776
1475.72 0.0134822917825276
1484.38 0.0143904866210667
1541.72 0.0141496840615824
1542.8 0.0148647367669682
1583.88 0.0160650697980993
1586.52 0.0150683740670143
1617.4 0.0145085282014121
1634.2 0.015364750152466
1660.52 0.0129807489608926
1670.38 0.0135296672313349
1670.7 0.0124668476449629
1702.86 0.0169347387304768
1705.1 0.0117003006180989
1706.36 0.0175079785248327
1809.68 0.0110163276770069
1828.42 0.0123739921345036
1856.34 0.0117724278092487
1887.16 0.0123304571932539
1915.96 0.0142067936243893
1935.02 0.0105213367063816
1966.22 0.0104541029676051
1997.3 0.0103142198582272
2033.56 0.0115521800383865
2110.38 0.0139105219485084
2124.98 0.0107063784312344
2439.72 0.00846559336431377
2493.26 0.00847989403722164
2543.38 0.0107204779476644
2579.36 0.00776785178702926
2620.94 0.00792196338359935
2704.12 0.00707025243524385
2747.04 0.0071501750174229
3027.82 0.00617902723506304
3196 0.00600093016877692
3464.8 0.00620071205033952
3658.9 0.00519663546453967
3757.52 0.00691652746647009
3786.44 0.00550448419876258
3996.06 0.00468802014005906
4047.26 0.00541388385968218
4074.66 0.00491618480925913
4599.46 0.0031413118079678
4998.14 0.00259224488145436
5613.52 0.00307735309404263
6090.12 0.00278185784646552
};
\addplot [
  draw=cadetblue80178158,
  fill=cadetblue80178158,
  forget plot,
  mark=*, mark size=1,
  only marks,
  draw opacity=0,
 fill opacity=0.5
]
table{%
x  y
242.32 0.1945219747471
245.4 0.243423587944335
247.56 0.188611633183378
286.9 0.14057997935202
286.98 0.0885330637556009
287.54 0.136713285440175
293.02 0.135842765539463
293.74 0.0844047095776221
395.68 0.131573476253579
426.28 0.35240684872857
460.28 0.229522362208384
461.96 0.171350003612784
462.12 0.337737950001751
464.06 0.0627442031858307
495.86 0.235669425239463
526.62 0.0758182955668507
536.2 0.512444397220981
540.66 0.0519777009918873
554.04 0.86793271468937
620.9 0.137262042786301
651.16 0.995195195280983
654 0.177414120039451
670.46 0.053552568013378
691.08 0.970017283931867
706.78 0.112223768822454
762.16 0.0454477221353362
764.74 0.0844578370463863
767.24 0.0481752811154967
808.86 0.0550632038904193
815.68 0.367668794393357
862.96 0.188246255806186
876.52 0.115961474882203
899.58 0.78679470517965
937.32 0.0496598705829914
937.34 0.668872449601249
955.66 0.774935180637719
956.38 0.0584751714486061
976.28 0.157741471852876
981.74 0.0457697950982278
994.42 0.6641331753224
1017.1 0.0750187920313802
1132.94 0.0853602156451196
1149.86 0.785850239325987
1245.3 0.039301322972614
1258.88 0.973744356231774
1270.2 0.0693515799073105
1342.54 0.973877217427833
1379.98 0.0345826536666355
1447.88 0.0545091678144899
1473.56 0.0407195041644876
1504.64 0.315251555933901
1507.62 0.0582324054487679
1521.48 0.0356753512427671
1539.92 0.161760360791573
1575.44 0.528561919560952
1661.78 0.0378436377217798
1703.38 0.135008472067348
1707.74 0.15782790934669
1729.36 0.0370108090057358
1792.22 0.513840121922117
1798.56 0.107192108812614
1838.14 0.0876364636963236
1923.96 0.519447269069614
1950.76 0.0476464103935431
1992.18 0.018475927831853
2018.72 0.0721302431698834
2042.8 0.036784713039492
2050.32 0.0247449878285115
2063.54 0.803163728917941
2080.16 0.0334592392185084
2219.7 0.114383185351833
2233.16 0.0932208361496233
2267.76 0.195562520016029
2361 0.0477417487838961
2373.84 0.29649888760577
2387.2 0.0694857148285228
2440.46 0.0952676665224623
2506.52 0.311957875447897
2529.86 0.106101612506956
2561.16 0.0349249429093728
2561.54 0.0558605741872915
2576.26 0.0200127970083414
2592.92 0.0156655184758531
2647.78 0.0328645884322873
2684.38 0.97409861366514
2742.38 0.332737763434993
2781.26 0.147622560800177
2831.14 0.0608147265934151
2858.52 0.0201502158347111
2871.6 0.0731922837772703
2937.7 0.312285365280101
2973.3 0.0965307734941501
3075.48 0.24138833435633
3080.46 0.143376835704505
3124.96 0.0268262297210182
3330.94 0.0167673398416977
3465.84 0.0238346849568994
3633 0.0253010143564197
3915.74 0.453012422254192
4272.26 0.0645941748853561
};
\addplot [
  draw=chocolate21910927,
  fill=chocolate21910927,
  forget plot,
  mark=*, mark size=1,
  only marks,
  draw opacity=0,
 fill opacity=0.5
]
table{%
x  y
16.06 1
16.24 1
16.24 1
16.66 1
16.8 1
16.8 1
16.82 1
16.82 1
16.82 1
16.82 1
16.82 1
16.82 1
16.82 1
16.82 1
16.82 1
16.82 1
16.82 1
16.88 1
16.94 1
17 1
20.32 0.986056845500349
21.68 0.948024469851983
100.44 0.494531419533209
139.92 0.575163258807544
143.84 0.460984148284679
143.96 0.754305208547402
145.98 0.457627538960249
158.1 0.282377979319802
192.22 0.24414449654951
211.94 0.607882710528389
212 0.259919949109248
222.02 0.275304543316824
230.42 0.19328861759322
248.94 0.207790104745744
249.94 0.156297722476548
249.94 0.110847016228203
251.26 0.187632363461772
254.24 0.22931905145206
264.02 0.250282914574948
276.94 0.220280573916835
293.14 0.198354732517172
303.22 0.148566400780147
312.72 0.136406921771602
314.38 0.161845634558212
334.66 0.697054178059788
343.44 0.116800756539275
351.14 0.144027868030027
373.8 0.109913579871302
434.18 0.178238673362368
442.12 0.115400327461551
573.94 0.125175259672463
613.4 0.0999969737658401
657.84 0.140288676420836
675.54 0.061728859700068
1046.62 0.265422951250188
1143.8 0.047471560270549
1190.3 0.0830691705331972
1456.2 0.0682223390783192
1470.14 0.0194667928285893
1474.02 0.0789223484960348
1562.2 0.146910879032738
1625.1 0.0272717855114321
1803.16 0.0188960844836412
1854.22 0.0239263668628018
1858.38 0.658898657917658
1950.72 0.0203218304618662
2223.6 0.0442288087612144
2571.6 0.0443604853039198
2730.86 0.0263621234961013
2785.36 0.0170477958284114
2838.7 0.00962129070429314
2935.16 0.0134681623648101
3747.56 0.00557103978925508
4105.34 0.0177924332529879
4161.76 0.0170528664902634
4325.78 0.0107971017592927
5432.8 0.00861127999939088
5560 0.0275000006938961
5725.64 0.00304235537698422
6292.12 0.00747789845608525
6499.64 0.00569136612256112
};
\addplot [draw=purple11522131, fill=purple11522131, forget plot, mark=*, mark size=1, only marks, draw opacity=0,
 fill opacity=0.5]
table{%
x  y
268.04 0.463628762201193
317.18 0.269963201532649
321.42 0.369840174701447
326.18 0.248475083890285
338.66 0.302059868156884
342.22 0.200737273703276
362.9 0.280970965582814
366.22 0.258043538592631
397.04 0.33297911912432
434.5 0.337785018537337
470.56 0.221366492604883
486.08 0.254039494348984
490.62 0.251874817063328
527.48 0.221631239079798
757.56 0.230504592378457
764.72 0.220518683892182
769.14 0.28347184911805
781.52 0.222117588739723
804.72 0.233253409623309
858.12 0.209591067615067
858.46 0.218540816736385
996.64 0.21208786685001
1052.76 0.217328870014399
1077.42 0.212721569691579
1085.84 0.215521356347815
1087.64 0.212721571263577
1088.56 0.212721571269467
1089.8 0.199112362565288
1091.9 0.201651188432606
1096.28 0.215521356347778
1096.6 0.215521356347795
1096.92 0.215521356347795
1096.96 0.215521356347795
1096.96 0.215521356347795
1140.78 0.198766861687049
1141.82 0.215175888812431
1144.02 0.186818737819639
1147.68 0.212403626275007
1245.04 0.161680107084868
1266.8 0.163862303451444
2190.44 0.113561682223704
3040.34 0.0757302511892367
3518.34 0.0764402752244729
3711.08 0.0758458319705526
3724.78 0.0756150538608281
3735.24 0.0761445334857371
4077.5 0.0756081204824626
4126.1 0.0884523215102685
4128.86 0.0742222987781644
4162.5 0.0742200706121965
4168.64 0.0756081156093478
4193.28 0.0756081156093447
4216.04 0.0745721324413031
4256.12 0.0742200693852109
4281.38 0.0742200693739087
4286.76 0.0747931199973852
4289.86 0.0744792081547657
4305.56 0.0742200693741012
4308.84 0.0742200693740979
4324.52 0.074220069374092
4330.38 0.074220069374092
4332.82 0.074221541625413
4357.12 0.074220069374092
4357.12 0.074220069374092
4357.12 0.074220069374092
4357.12 0.074220069374092
4357.12 0.074220069374092
4357.12 0.074220069374092
4357.12 0.074220069374092
4357.12 0.074220069374092
4445.14 0.073647474106507
4454.4 0.073647474106507
4454.4 0.073647474106507
4454.4 0.073647474106507
4454.4 0.073647474106507
4454.4 0.073647474106507
4454.4 0.073647474106507
4454.4 0.073647474106507
4454.4 0.073647474106507
4454.4 0.073647474106507
5232.78 0.0567896083566733
5571.64 0.0561401823297562
5635.36 0.0561401915968345
5707.68 0.0561392140784589
5717.78 0.0561392140657238
5731.76 0.0561392148784166
5734.4 0.0561392140657238
5734.4 0.0561392140657238
5734.4 0.0561392140657238
5734.4 0.0561392140657238
};
\addplot [draw=black18, fill=black18, forget plot, mark=*, mark size=1, only marks, draw opacity=0,
 fill opacity=0.5]
table{%
x  y
16.82 1
78.52 0.352406864634089
79.52 0.343617523819217
81.82 0.335873510469019
83.98 0.329462636533082
86.24 0.320434074852608
86.96 0.316130599146267
88.88 0.313637940621528
89.52 0.309795769235189
91.96 0.302079301876991
93.94 0.296723883528843
96.92 0.297220383726747
99.4 0.295228524829219
103.36 0.296265905332989
105.34 0.289604951799693
110.98 0.276400632076965
116.08 0.269552350218998
117.64 0.264842961955508
121.36 0.264150854497973
125.26 0.262915300704947
129.18 0.247779824201428
129.64 0.25263211960199
134.54 0.24175800551591
137.16 0.236424907750126
140.64 0.230475979885843
144.36 0.222120692206102
147.3 0.210238128510474
153.34 0.208249800484106
159.12 0.198970396810122
163.56 0.194914646604832
172.48 0.194201676302788
175.88 0.189359558501058
182.28 0.183220160853646
194.14 0.17854722863673
194.64 0.174518100765147
206.66 0.170406418602505
206.76 0.164389890108926
219.36 0.15342981135071
234.02 0.149271680708446
238.26 0.144805442357256
249.4 0.137770529678871
268.4 0.134303009881153
268.9 0.129450325666821
287.6 0.127154350726344
302.36 0.123091308472638
325.04 0.119065458351604
326.44 0.11524767630968
338.92 0.111808104246352
359.56 0.104007724744732
365.26 0.101788054521189
396.48 0.0969864696937784
405.08 0.0962240943380343
419.36 0.0899958430935284
431.04 0.090025372993765
455.7 0.0846874256362099
472.32 0.0792453333058815
506.3 0.0752286662184685
512.4 0.0722794669154851
524.74 0.06863177496487
559.4 0.065244496504746
582.4 0.0602787969826986
633 0.0554677709074053
664.48 0.0518068469103507
739.64 0.0468817428789428
760.22 0.0450231970206735
784.46 0.0428741549192849
808.32 0.042260348651274
873.7 0.0393437384790014
891.12 0.0378747946250103
1014.26 0.0349144314332351
1101.9 0.0335051211015261
1139.68 0.0327386990151712
1194.4 0.0315862344736213
1297.34 0.0282555092141506
1387.48 0.0263526417643002
1542.58 0.0238357673367063
1655.52 0.0207749814628984
1833.8 0.0196953140379937
1846.62 0.0180147290240576
2044.74 0.0161650868227532
2249.44 0.0143828577591726
2521.58 0.011844416209044
2616.94 0.0113563525063623
2829.94 0.0100368049382516
3040.76 0.00916593814495429
3312.78 0.00844518462685504
3634.98 0.00739122544578433
3885.2 0.00705681043713627
4153.58 0.00611588855069067
4721.94 0.00523719061100103
5153.98 0.00461256968369267
5648.28 0.0042489201860652
6054.88 0.00391533538423359
6424.72 0.00346620018977536
};
\addplot [draw=darkgray153, fill=darkgray153, forget plot, mark=*, mark size=1, only marks, draw opacity=0,
 fill opacity=0.5]
table{%
x  y
16.82 1
124.74 0.133268092835812
130.56 0.127261001270772
140.42 0.122130182717036
142.82 0.118716494315573
144.42 0.114623607663328
147.54 0.11082734040265
150.08 0.109160873588763
153.86 0.108194426789855
155.98 0.106112267405133
163.06 0.100275732858161
169.6 0.0978102279374639
175.58 0.0936685289253109
176.12 0.0924550294301424
181.44 0.0900365762462394
187.4 0.0875675854408009
196.72 0.0852212767252972
202.02 0.0834708179183686
211.02 0.0819361814822101
215.36 0.0799416137063562
221.8 0.0780794862410057
227.9 0.075974069547764
236.4 0.0732106035704651
238.56 0.0725881362923155
253.04 0.0687555922898438
264.16 0.0654944386547324
278 0.0645846100202051
279.66 0.0633952801291083
298.98 0.0621704400407094
300.96 0.0615850686027572
308.26 0.0595948717597626
321.36 0.0580971144052208
326.36 0.0565368284322324
342.64 0.0542132018953953
356.46 0.0532877431373862
361.9 0.0513774958402645
372.26 0.0504123830932258
400.84 0.0474264912136916
417.4 0.0458489335870729
427.36 0.0438830820658574
445.44 0.0424919734585621
456.66 0.0411401612209637
474.08 0.0403792868246142
486.98 0.0378283442468803
489.16 0.038771249040496
511.24 0.0361227396567082
526.94 0.0358133350342303
553.8 0.0342508267297126
561.42 0.034161371285608
572.86 0.0329618346975396
598.28 0.0312648460491836
601.44 0.0321840822901551
614.6 0.0308821127155452
660.88 0.0298172837152069
673.94 0.0297914199898323
699.12 0.0278497884802016
725.14 0.0265692888560997
758.9 0.0260796218755583
789.54 0.0246056395851363
805.76 0.0240125231495172
823.48 0.0219828126010447
830.12 0.0237886807692866
858.26 0.0214758299795345
859.12 0.0211035405706784
896.96 0.0200799176851056
953.42 0.0191154449152691
955.32 0.0183232566711519
1013.44 0.0177025808119158
1051.06 0.0166314274248366
1087.56 0.0158436530479346
1138.32 0.0157096400518087
1175.78 0.0144899536523155
1218.88 0.014217504509935
1236.24 0.0143698292460652
1293.46 0.0137399872747504
1384.94 0.0129446210965155
1447.24 0.0123440343459865
1515.82 0.0117320422690034
1530.72 0.0111856751295082
1546.76 0.0106113931588243
1688.62 0.00986942215172925
1776.34 0.00914660093929309
1917.1 0.00876225509011145
2002 0.00850379431431339
2019.68 0.00808242771192422
2106.2 0.00744004450560531
2346.68 0.0066805793898825
2415.02 0.00620589080390916
2478.54 0.00585976624718794
2822.22 0.00550184865820004
3083.12 0.00487120019152001
3402.28 0.00440215242012226
3643.14 0.0038684489631508
3930.64 0.00347939165301242
4314.8 0.00297138131232652
5040.16 0.00251202571483294
5824.38 0.00201349516679291
};
\addplot [
  draw=saddlebrown1356716,
  fill=saddlebrown1356716,
  forget plot,
  mark=*, mark size=1,
  only marks,
  draw opacity=0,
 fill opacity=0.5
]
table{%
x  y
277.76 0.466282954121135
340.52 0.125473237148267
343.1 0.12246643163678
346.22 0.115830624090172
351.02 0.111908494316199
353.12 0.108908399262491
362.5 0.102400050951877
373 0.0977990613126176
373.88 0.0930720528234326
374.86 0.095219400934919
378.18 0.0892170564473306
388.58 0.0881429649793577
390.18 0.0851456057299144
401.8 0.08212029191033
411.08 0.0792717945958325
426.44 0.0775171912823767
434.74 0.0754905076971218
447.58 0.0723172038001679
465.74 0.0707391922581567
486.16 0.0673727205928332
501.68 0.065947445255234
508.86 0.0645718471001186
521.3 0.0642959158929115
540.46 0.0639671947483639
562.06 0.0633123313917946
573.68 0.062610281804693
595.3 0.0608484403968491
622.62 0.059774701945911
638.78 0.0590416611021697
654.52 0.0566812392319918
658.46 0.057252722054146
674.88 0.0555970422862214
686.1 0.0548722780747896
711.32 0.054016577933665
725.04 0.0528122701631741
742.6 0.0516910293819871
763 0.0518142554662167
778.52 0.0504581017169793
790.68 0.050013335444624
814.78 0.0488462140984589
833.04 0.0472906959193093
855.8 0.0462675707141757
881.96 0.0456582014853014
915.24 0.0443897801278166
932.52 0.0445332391512188
953.28 0.0434647969707767
967.9 0.0432953969664676
999.66 0.0428843734938093
1039.88 0.0417221658579803
1050.74 0.0401747451435038
1057.9 0.0410851357601881
1074.86 0.0383119402074389
1130.2 0.0370494416870747
1156.14 0.0367520069380685
1192.04 0.0365460872284678
1241.26 0.0358820978110363
1252.14 0.0354798147943327
1287.52 0.0342988477446523
1315.48 0.0330140068232053
1363.7 0.0319812996787525
1410 0.0316700404395148
1459.92 0.0312417354226361
1507.54 0.0305599003927687
1563.22 0.0293183619546203
1593.36 0.0290700922116714
1624 0.0275795238231562
1665.14 0.0273123344047003
1694.3 0.0272387259690467
1741.96 0.026472622902696
1795.4 0.0249938093304947
1855.18 0.0240281612028345
1899.72 0.0245035070579799
1941.92 0.0234141662328361
2009.6 0.0227076299269046
2089.88 0.022689737722979
2135.6 0.0217706609615634
2183.84 0.0211448576399366
2240.58 0.0210343696759014
2308.28 0.020414158938075
2357.86 0.0191089830023983
2422.56 0.0185033986868606
2519.66 0.0178011841563917
2590.26 0.0175380267961728
2639.46 0.0168888815765715
2693.18 0.0163851580400982
2749.82 0.0160293064941525
2798.62 0.0157208205733829
2868.48 0.0144986334074072
2931.46 0.0140224355161308
3038.06 0.0136043448997332
3175.04 0.0126799318780959
3245.46 0.0121077863636076
3348.32 0.0119547789350979
3439.6 0.0116216501462064
3567.24 0.0113825734608513
3615.38 0.0109529307020395
3702.42 0.0106235303394306
3831.18 0.0100197279869929
3940.86 0.00952110007376304
4131.92 0.00909416355746522
};
\addplot [very thick, royalblue28108204]
table {%
139.38 0.142508664833603
199.488484848485 0.111092745432698
259.59696969697 0.090898046514584
319.705454545455 0.0767439577435771
379.813939393939 0.0662460407424954
439.922424242424 0.0581407626242701
500.030909090909 0.0516915313705986
560.139393939394 0.0464381147146202
620.247878787879 0.0420773461975422
680.356363636364 0.0384010125353622
740.464848484849 0.0352611915684355
800.573333333333 0.0325498064519755
860.681818181818 0.0301860049807133
920.790303030303 0.0281080677894124
980.898787878788 0.0262680503623102
1041.00727272727 0.0246281355157528
1101.11575757576 0.02315808970082
1161.22424242424 0.0218334511137308
1221.33272727273 0.0206342146392814
1281.44121212121 0.0195438612853033
1341.5496969697 0.0185486310207688
1401.65818181818 0.0176369705320976
1461.76666666667 0.0167991086229286
1521.87515151515 0.0160267260661196
1581.98363636364 0.0153126962422343
1642.09212121212 0.0146508794507898
1702.20060606061 0.0140359583572594
1762.30909090909 0.0134633052813436
1822.41757575758 0.012928874359486
1882.52606060606 0.0124291133055544
1942.63454545455 0.0119608907359636
2002.74303030303 0.01152143594787
2062.85151515152 0.0111082887305332
2122.96 0.0107192573130755
2183.06848484848 0.0103523829510245
2243.17696969697 0.0100059099610579
2303.28545454545 0.00967826025130827
2363.39393939394 0.00936801158031831
2423.50242424242 0.0090738789236783
2483.61090909091 0.00879469844279507
2543.71939393939 0.00852941364206781
2603.82787878788 0.00827706337422161
2663.93636363636 0.0080367714126634
2724.04484848485 0.0078077373575299
2784.15333333333 0.00758922868094887
2844.26181818182 0.0073805737487574
2904.3703030303 0.00718115568194036
2964.47878787879 0.00699040694248495
3024.58727272727 0.00680780454607389
3084.69575757576 0.00663286581876088
3144.80424242424 0.00646514462704018
3204.91272727273 0.00630422802098714
3265.02121212121 0.0061497332387612
3325.1296969697 0.00600130502802007
3385.23818181818 0.00585861324592509
3445.34666666667 0.00572135070461474
3505.45515151515 0.00558923123344113
3565.56363636364 0.00546198793303089
3625.67212121212 0.00533937159945138
3685.78060606061 0.0052211492995243
3745.88909090909 0.00510710308069953
3805.99757575758 0.00499702880094725
3866.10606060606 0.00489073506589027
3926.21454545455 0.0047880422619271
3986.32303030303 0.00468878167542188
4046.43151515152 0.00459279468918992
4106.54 0.00449993204851211
4166.64848484849 0.00441005318978857
4226.75696969697 0.00432302562570918
4286.86545454545 0.00423872438149152
4346.97393939394 0.00415703147732714
4407.08242424242 0.00407783545269735
4467.19090909091 0.00400103092867761
4527.29939393939 0.00392651820475429
4587.40787878788 0.00385420288703519
4647.51636363636 0.00378399554505255
4707.62484848485 0.00371581139463821
4767.73333333333 0.00364957000460037
4827.84181818182 0.00358519502515475
4887.9503030303 0.00352261393625975
4948.05878787879 0.00346175781418374
5008.16727272727 0.00340256111478968
5068.27575757576 0.00334496147216428
5128.38424242424 0.00328889951134614
5188.49272727273 0.00323431867402039
5248.60121212121 0.0031811650561505
5308.7096969697 0.00312938725660953
5368.81818181818 0.00307893623595619
5428.92666666667 0.00302976518457565
5489.03515151515 0.00298182939947302
5549.14363636364 0.0029350861690679
5609.25212121212 0.00288949466539404
5669.36060606061 0.00284501584315803
5729.46909090909 0.00280161234515609
5789.57757575758 0.00275924841358982
5849.68606060606 0.00271788980685838
5909.79454545455 0.00267750372143924
5969.90303030303 0.00263805871850044
6030.01151515152 0.00259952465491527
6090.12 0.00256187261837657
};
\addplot [very thick, cadetblue80178158]
table {%
242.32 0.158790439250481
283.026464646465 0.165350371050145
323.732929292929 0.169666911687341
364.439393939394 0.172332607822478
405.145858585859 0.173766298281346
445.852323232323 0.174270579301541
486.558787878788 0.174068169360541
527.265252525252 0.173325611866454
567.971717171717 0.172169139147569
608.678181818182 0.170695542040182
649.384646464646 0.168979773570235
690.091111111111 0.167080366756844
730.797575757576 0.165043358636561
771.50404040404 0.162905174249426
812.210505050505 0.16069477425077
852.91696969697 0.158435273195512
893.623434343434 0.156145172070549
934.329898989899 0.153839306178834
975.036363636364 0.151529580576294
1015.74282828283 0.149225545288906
1056.44929292929 0.146934848537222
1097.15575757576 0.144663596253947
1137.86222222222 0.142416639035078
1178.56868686869 0.140197802472289
1219.27515151515 0.13801007300115
1259.98161616162 0.135855748572753
1300.68808080808 0.133736561341403
1341.39454545455 0.131653777965694
1382.10101010101 0.129608281907287
1422.80747474747 0.12760064118265
1463.51393939394 0.125631164306506
1504.2204040404 0.123699946609583
1544.92686868687 0.121806908678795
1585.63333333333 0.119951828326808
1626.3397979798 0.11813436722837
1667.04626262626 0.11635409314683
1707.75272727273 0.114610498503537
1748.45919191919 0.112903015905972
1789.16565656566 0.111231031140305
1829.87212121212 0.109593894045022
1870.57858585859 0.107990927609984
1911.28505050505 0.106421435586388
1951.99151515152 0.104884708844954
1992.69797979798 0.103380030680193
2033.40444444444 0.101906681226056
2074.11090909091 0.100463941121458
2114.81737373737 0.0990510945419335
2155.52383838384 0.0976674316952346
2196.2303030303 0.0963122508632974
2236.93676767677 0.0949848600602021
2277.64323232323 0.0936845783650057
2318.3496969697 0.0924107369793298
2359.05616161616 0.0911626800520258
2399.76262626263 0.0899397653068634
2440.46909090909 0.0887413645038173
2481.17555555556 0.0875668637599794
2521.88202020202 0.0864156637522732
2562.58848484848 0.085287179820883
2603.29494949495 0.0841808419895343
2644.00141414141 0.0830960949164003
2684.70787878788 0.0820323977873972
2725.41434343434 0.0809892241619129
2766.12080808081 0.0799660617795492
2806.82727272727 0.0789624123351995
2847.53373737374 0.0779777912287141
2888.2402020202 0.0770117272944809
2928.94666666667 0.0760637625154645
2969.65313131313 0.0751334517255662
3010.3595959596 0.0742203623035849
3051.06606060606 0.073324073861567
3091.77252525253 0.0724441779298919
3132.47898989899 0.071580277641082
3173.18545454545 0.070731987414002
3213.89191919192 0.0698989326398415
3254.59838383838 0.0690807493710406
3295.30484848485 0.0682770840141167
3336.01131313131 0.0674875930271758
3376.71777777778 0.0667119426227454
3417.42424242424 0.0659498084764378
3458.13070707071 0.0652008754418417
3498.83717171717 0.0644648372719488
3539.54363636364 0.0637413963473419
3580.2501010101 0.0630302634113
3620.95656565657 0.0623311573119245
3661.66303030303 0.061643804751334
3702.3694949495 0.0609679400419382
3743.07595959596 0.0603033048697669
3783.78242424242 0.0596496480647983
3824.48888888889 0.0590067253782084
3865.19535353535 0.0583742992664431
3905.90181818182 0.0577521386819968
3946.60828282828 0.0571400188707702
3987.31474747475 0.0565377211758692
4028.02121212121 0.0559450328476952
4068.72767676768 0.0553617468601762
4109.43414141414 0.05478766173298
4150.14060606061 0.0542225813595483
4190.84707070707 0.053666314840791
4231.55353535354 0.0531186763242742
4272.26 0.0525794848487435
};
\addplot [very thick, chocolate21910927]
table {%
16.06 1.00696718582534
81.5507070707071 0.527684366403782
147.041414141414 0.367972538491158
212.532121212121 0.283910339326002
278.022828282828 0.231140483829237
343.513535353535 0.194666491577329
409.004242424242 0.167855807533057
474.49494949495 0.147281562553441
539.985656565657 0.130980883744146
605.476363636364 0.117743149866548
670.967070707071 0.106778777870914
736.457777777778 0.0975497110131091
801.948484848485 0.0896760904788814
867.439191919192 0.0828818004341586
932.929898989899 0.0769611542512997
998.420606060606 0.0717576948457971
1063.91131313131 0.0671502463096878
1129.40202020202 0.0630434700260827
1194.89272727273 0.059361309701768
1260.38343434343 0.056042341379424
1325.87414141414 0.0530364106538524
1391.36484848485 0.0503021586772282
1456.85555555556 0.0478051738192279
1522.34626262626 0.0455165914562301
1587.83696969697 0.0434120198046015
1653.32767676768 0.0414707063724998
1718.81838383838 0.0396748843067777
1784.30909090909 0.0380092548449818
1849.7997979798 0.0364605738741541
1915.29050505051 0.0350173189287174
1980.78121212121 0.0336694189238373
2046.27191919192 0.0324080332433701
2111.76262626263 0.0312253699704752
2177.25333333333 0.0301145353969124
2242.74404040404 0.0290694087039508
2308.23474747475 0.0280845370346949
2373.72545454545 0.0271550471884401
2439.21616161616 0.0262765709440053
2504.70686868687 0.0254451816198047
2570.19757575758 0.0246573399467821
2635.68828282828 0.023909847697922
2701.17898989899 0.0231998078084244
2766.6696969697 0.0225245899514098
2832.1604040404 0.0218818007185006
2897.65111111111 0.0212692577029084
2963.14181818182 0.0206849669024693
3028.63252525253 0.0201271029573661
3094.12323232323 0.0195939918166563
3159.61393939394 0.0190840954927913
3225.10464646465 0.0185959986168709
3290.59535353535 0.0181283965516496
3356.08606060606 0.0176800848560525
3421.57676767677 0.0172499499255673
3487.06747474747 0.0168369606584679
3552.55818181818 0.0164401610192997
3618.04888888889 0.0160586633891309
3683.5395959596 0.0156916426073446
3749.0303030303 0.0153383306226782
3814.52101010101 0.0149980116822141
3880.01171717172 0.0146700179963886
3945.50242424242 0.0143537258260964
4010.99313131313 0.0140485519448288
4076.48383838384 0.0137539504346768
4141.97454545455 0.0134694097801094
4207.46525252525 0.0131944502278237
4272.95595959596 0.0129286213847519
4338.44666666667 0.0126715000296098
4403.93737373737 0.0124226881162257
4469.42808080808 0.0121818109493869
4534.91878787879 0.0119485155161144
4600.4094949495 0.0117224689571812
4665.9002020202 0.0115033571653604
4731.39090909091 0.0112908834983504
4796.88161616162 0.0110847675956198
4862.37232323232 0.0108847442895447
4927.86303030303 0.0106905626022199
4993.35373737374 0.0105019848202082
5058.84444444444 0.0103187856402816
5124.33515151515 0.0101407513799036
5189.82585858586 0.00996767924682099
5255.31656565657 0.00979937666268765
5320.80727272727 0.00963566063613067
5386.29797979798 0.0094763571811119
5451.78868686869 0.00932130077682682
5517.2793939394 0.00917033386573579
5582.7701010101 0.00902330638663629
5648.26080808081 0.00888007533996762
5713.75151515152 0.00874050438279285
5779.24222222222 0.00860446345113154
5844.73292929293 0.00847182840752172
5910.22363636364 0.00834248071187562
5975.71434343434 0.00821630711386071
6041.20505050505 0.00809319936518919
6106.69575757576 0.00797305395033576
6172.18646464647 0.0078557718343276
6237.67717171717 0.00774125822636342
6303.16787878788 0.00762942235811973
6368.65858585859 0.00752017727569634
6434.14929292929 0.00741343964423623
6499.64 0.00730912956433339
};
\addplot [very thick, purple11522131]
table {%
268.04 0.304768118296189
323.255757575758 0.297968190836828
378.471515151515 0.289968533031165
433.687272727273 0.281526452180638
488.90303030303 0.273032856637268
544.118787878788 0.264693720639103
599.334545454545 0.256616410971349
654.550303030303 0.248853684380854
709.766060606061 0.24142731804789
764.981818181818 0.234341323022847
820.197575757576 0.22758956369272
875.413333333333 0.221160252648401
930.629090909091 0.21503864350253
985.844848484848 0.209208657094159
1041.06060606061 0.203653863147822
1096.27636363636 0.198358066146697
1151.49212121212 0.193305645362015
1206.70787878788 0.188481741131935
1261.92363636364 0.183872344835752
1317.13939393939 0.179464328843514
1372.35515151515 0.175245439568567
1427.57090909091 0.171204268456929
1482.78666666667 0.167330210452805
1538.00242424242 0.163613416064985
1593.21818181818 0.160044740939206
1648.43393939394 0.156615695390378
1703.6496969697 0.153318395396861
1758.86545454545 0.150145515934582
1814.08121212121 0.147090247120527
1869.29696969697 0.144146253370222
1924.51272727273 0.141307635604469
1979.72848484848 0.138568896434836
2034.94424242424 0.135924908194175
2090.16 0.133370883643214
2145.37575757576 0.130902349167678
2200.59151515152 0.128515120275735
2255.80727272727 0.126205279208568
2311.02303030303 0.123969154484499
2366.23878787879 0.121803302207419
2421.45454545455 0.119704488981948
2476.6703030303 0.117669676289863
2531.88606060606 0.115696006194413
2587.10181818182 0.113780788250753
2642.31757575758 0.111921487511742
2697.53333333333 0.110115713528564
2752.74909090909 0.108361210255137
2807.96484848485 0.106655846773915
2863.18060606061 0.104997608768604
2918.39636363636 0.103384590676486
2973.61212121212 0.101814988459541
3028.82787878788 0.100287092939413
3084.04363636364 0.098799283646566
3139.25939393939 0.0973500231387337
3194.47515151515 0.0959378517480411
3249.69090909091 0.0945613827200573
3304.90666666667 0.0932192977114849
3360.12242424242 0.0919103426163237
3415.33818181818 0.0906333236931507
3470.55393939394 0.0893871039686874
3525.7696969697 0.0881705998950953
3580.98545454545 0.0869827782404978
3636.20121212121 0.0858226531940667
3691.41696969697 0.0846892836686846
3746.63272727273 0.0835817707856945
3801.84848484848 0.0824992555276083
3857.06424242424 0.0814409165458723
3912.28 0.0804059681119059
3967.49575757576 0.0793936582006235
4022.71151515151 0.0784032666965766
4077.92727272727 0.0774341037136656
4133.14303030303 0.0764855080201325
4188.35878787879 0.0755568455612208
4243.57454545454 0.0746475080725123
4298.7903030303 0.0737569117775141
4354.00606060606 0.0728844961635811
4409.22181818182 0.0720297228307303
4464.43757575758 0.0711920744083299
4519.65333333333 0.0703710535350334
4574.86909090909 0.0695661818976917
4630.08484848485 0.0687769993252937
4685.30060606061 0.0680030629342937
4740.51636363636 0.067243946321948
4795.73212121212 0.0664992388045429
4850.94787878788 0.0657685446976169
4906.16363636364 0.0650514826354989
4961.37939393939 0.064347684927673
5016.59515151515 0.0636567969496618
5071.81090909091 0.0629784765662821
5127.02666666667 0.0623123935852784
5182.24242424242 0.0616582292394829
5237.45818181818 0.0610156756957687
5292.67393939394 0.0603844355891973
5347.8896969697 0.0597642215808533
5403.10545454545 0.059154755937975
5458.32121212121 0.0585557701350755
5513.53696969697 0.0579670044748338
5568.75272727273 0.0573882077276253
5623.96848484848 0.0568191367886217
5679.18424242424 0.0562595563514725
5734.4 0.055709238597633
};
\addplot [very thick, black18]
table {%
16.82 0.882888714341397
81.5462626262626 0.346058181011084
146.272525252525 0.22208900731908
210.998787878788 0.163738697527132
275.725050505051 0.129371207453474
340.451313131313 0.106620883249069
405.177575757576 0.0904235043829743
469.903838383838 0.0782995094916571
534.630101010101 0.0688853762422148
599.356363636364 0.0613670068930106
664.082626262626 0.055227444417618
728.808888888889 0.0501222687845429
793.535151515152 0.0458129938985186
858.261414141414 0.0421291728273752
922.987676767677 0.0389457154038037
987.71393939394 0.0361687280501454
1052.4402020202 0.0337263543995961
1117.16646464646 0.0315626678507881
1181.89272727273 0.0296334905402962
1246.61898989899 0.0279034644235098
1311.34525252525 0.0263439573576678
1376.07151515152 0.024931538825948
1440.79777777778 0.0236468522227107
1505.52404040404 0.0224737682703625
1570.2503030303 0.0213987410316872
1634.97656565657 0.0204103121087846
1699.70282828283 0.0194987247109943
1764.42909090909 0.0186556201991972
1829.15535353535 0.0178737972532952
1893.88161616162 0.0171470190911039
1958.60787878788 0.0164698579179169
2023.33414141414 0.0158375684842386
2088.0604040404 0.0152459845931454
2152.78666666667 0.0146914338440234
2217.51292929293 0.014170666973955
2282.23919191919 0.0136807989645642
2346.96545454546 0.0132192596929666
2411.69171717172 0.01278375237199
2476.41797979798 0.012372218383951
2541.14424242424 0.0119828073907919
2605.87050505051 0.011613851820907
2670.59676767677 0.0112638450040049
2735.32303030303 0.0109314223606636
2800.04929292929 0.0106153451609263
2864.77555555556 0.0103144864524835
2929.50181818182 0.0100278188283581
2994.22808080808 0.00975440376011921
3058.95434343434 0.00949338226826108
3123.68060606061 0.00924396673863119
3188.40686868687 0.00900543372434383
3253.13313131313 0.00877711759778699
3317.85939393939 0.00855840493814866
3382.58565656566 0.00834872955717866
3447.31191919192 0.00814756808031205
3512.03818181818 0.00795443601233585
3576.76444444445 0.00776888422689926
3641.49070707071 0.00759049582769131
3706.21696969697 0.00741888333630997
3770.94323232323 0.00725368616795089
3835.6694949495 0.00709456836123106
3900.39575757576 0.00694121653288593
3965.12202020202 0.00679333803185902
4029.84828282828 0.00665065927054406
4094.57454545455 0.00651292421372365
4159.30080808081 0.0063798930081485
4224.02707070707 0.00625134073777244
4288.75333333333 0.00612705629145168
4353.4795959596 0.00600684133147289
4418.20585858586 0.00589050935262684
4482.93212121212 0.00577788482272342
4547.65838383838 0.00566880239647206
4612.38464646465 0.00556310619555256
4677.11090909091 0.00546064914848971
4741.83717171717 0.00536129238463815
4806.56343434343 0.00526490467719365
4871.2896969697 0.00517136193068414
4936.01595959596 0.0050805467088679
5000.74222222222 0.00499234779938639
5065.46848484849 0.00490665981188995
5130.19474747475 0.00482338280668521
5194.92101010101 0.00474242195124486
5259.64727272727 0.00466368720218236
5324.37353535354 0.00458709301052537
5389.0997979798 0.00451255804832985
5453.82606060606 0.00444000495486159
5518.55232323232 0.00436936010073825
5583.27858585859 0.00430055336857314
5648.00484848485 0.00423351794879599
5712.73111111111 0.004168190149445
5777.45737373737 0.00410450921883321
5842.18363636364 0.00404241718008847
5906.9098989899 0.0039818586766546
5971.63616161616 0.00392278082791964
6036.36242424242 0.00386513309420938
6101.08868686869 0.00380886715044829
6165.81494949495 0.00375393676784887
6230.54121212121 0.0037002977030436
6295.26747474748 0.00364790759412163
6359.99373737374 0.0035967258630764
6424.72 0.00354671362420995
};
\addplot [very thick, darkgray153]
table {%
16.82 0.727785818616711
75.4822222222222 0.218130953694854
134.144444444444 0.130747330372027
192.806666666667 0.0933185116176789
251.468888888889 0.0723877988749081
310.131111111111 0.0589893189449207
368.793333333333 0.0496721715673338
427.455555555556 0.0428183632624153
486.117777777778 0.0375666308718994
544.78 0.0334157211221637
603.442222222222 0.0300538495905846
662.104444444445 0.0272768175652708
720.766666666667 0.0249452563052303
779.428888888889 0.0229607770541183
838.091111111111 0.0212519358541093
896.753333333333 0.0197656002156946
955.415555555556 0.018461436807428
1014.07777777778 0.0173082779508317
1072.74 0.0162816596461517
1131.40222222222 0.0153621127543073
1190.06444444444 0.014533951494923
1248.72666666667 0.0137843981806912
1307.38888888889 0.0131029401162309
1366.05111111111 0.0124808498540468
1424.71333333333 0.0119108223640953
1483.37555555556 0.0113866971772126
1542.03777777778 0.0109032431612238
1600.7 0.0104559900588827
1659.36222222222 0.0100410953523302
1718.02444444444 0.00965523810663343
1776.68666666667 0.00929553362535707
1835.34888888889 0.0089594643110224
1894.01111111111 0.00864482325292815
1952.67333333333 0.00834966789211214
2011.33555555556 0.00807228172552537
2069.99777777778 0.00781114246912245
2128.66 0.00756489544476443
2187.32222222222 0.0073323312184637
2245.98444444444 0.00711236671894441
2304.64666666667 0.00690402922118702
2363.30888888889 0.00670644270083028
2421.97111111111 0.00651881616030297
2480.63333333333 0.00634043360249806
2539.29555555556 0.00617064538728106
2597.95777777778 0.00600886075360619
2656.62 0.00585454132812826
2715.28222222222 0.00570719547195342
2773.94444444444 0.00556637334211376
2832.60666666667 0.0054316625646743
2891.26888888889 0.00530268443301754
2949.93111111111 0.00517909055852767
3008.59333333333 0.00506055991218837
3067.25555555556 0.00494679620496767
3125.91777777778 0.00483752556265024
3184.58 0.00473249445728181
3243.24222222222 0.00463146786283961
3301.90444444444 0.00453422760732725
3360.56666666667 0.00444057089735798
3419.22888888889 0.00435030899456389
3477.89111111111 0.00426326602594558
3536.55333333333 0.0041792779126427
3595.21555555556 0.00409819140362466
3653.87777777778 0.00401986320252918
3712.54 0.00394415917736072
3771.20222222222 0.00387095364403717
3829.86444444444 0.0038001287158747
3888.52666666667 0.00373157371205321
3947.18888888889 0.00366518461893006
4005.85111111111 0.00360086359878682
4064.51333333333 0.00353851854121784
4123.17555555556 0.00347806265291393
4181.83777777778 0.00341941408207012
4240.5 0.00336249557406352
4299.16222222222 0.00330723415541273
4357.82444444444 0.00325356084335183
4416.48666666667 0.00320141037863538
4475.14888888889 0.00315072097944016
4533.81111111111 0.00310143411445053
4592.47333333333 0.00305349429340971
4651.13555555556 0.00300684887359238
4709.79777777778 0.00296144788080791
4768.46 0.00291724384368057
4827.12222222222 0.00287419164007485
4885.78444444444 0.00283224835464269
4944.44666666667 0.00279137314656683
5003.10888888889 0.0027515271266611
5061.77111111111 0.00271267324306655
5120.43333333333 0.00267477617485207
5179.09555555556 0.00263780223289071
5237.75777777778 0.00260171926743963
5296.42 0.00256649658190206
5355.08222222222 0.00253210485229558
5413.74444444444 0.00249851605199226
5472.40666666667 0.00246570338133373
5531.06888888889 0.00243364120175752
5589.73111111111 0.00240230497410212
5648.39333333333 0.00237167120078574
5707.05555555556 0.00234171737157847
5765.71777777778 0.0023124219127112
5824.38 0.00228376413908458
};
\addplot [very thick, saddlebrown1356716]
table {%
277.76 0.131258750094658
316.690909090909 0.116829080888006
355.621818181818 0.105344822838787
394.552727272727 0.0959762171966474
433.483636363636 0.0881805315514451
472.414545454545 0.0815873214678799
511.345454545455 0.0759348056867734
550.276363636364 0.0710325758163827
589.207272727273 0.0667387197532304
628.138181818182 0.0629452393416108
667.069090909091 0.0595684466209008
706 0.0565424582610516
744.930909090909 0.0538146791676634
783.861818181818 0.0513425985701105
822.792727272727 0.0490914732153307
861.723636363636 0.0470326231305792
900.654545454545 0.0451421585638242
939.585454545454 0.0434000157049631
978.516363636364 0.041789217016216
1017.44727272727 0.0402952972826006
1056.37818181818 0.0389058535308389
1095.30909090909 0.0376101886436136
1134.24 0.0363990266272776
1173.17090909091 0.0352642832343375
1212.10181818182 0.0341988797526658
1251.03272727273 0.0331965907518512
1289.96363636364 0.0322519187599191
1328.89454545455 0.0313599904604406
1367.82545454545 0.0305164702094822
1406.75636363636 0.0297174875849892
1445.68727272727 0.0289595763766372
1484.61818181818 0.0282396229581708
1523.54909090909 0.0275548223974193
1562.48 0.0269026409811982
1601.41090909091 0.0262807840850004
1640.34181818182 0.0256871685169681
1679.27272727273 0.025119898624244
1718.20363636364 0.0245772455765819
1757.13454545455 0.0240576293439958
1796.06545454545 0.0235596029675649
1834.99636363636 0.0230818387893733
1873.92727272727 0.0226231163621205
1912.85818181818 0.0221823118036604
1951.78909090909 0.0217583883985415
1990.72 0.0213503882790619
2029.65090909091 0.0209574250436145
2068.58181818182 0.0205786771911517
2107.51272727273 0.0202133822682027
2146.44363636364 0.0198608316396521
2185.37454545455 0.0195203658069328
2224.30545454545 0.0191913702077952
2263.23636363636 0.0188732714407291
2302.16727272727 0.0185655338646835
2341.09818181818 0.0182676565311924
2380.02909090909 0.0179791704115313
2418.96 0.0176996358862657
2457.89090909091 0.0174286404686191
2496.82181818182 0.0171657967365974
2535.75272727273 0.0169107404518311
2574.68363636364 0.0166631288457235
2613.61454545455 0.0164226390557681
2652.54545454545 0.0161889666968758
2691.47636363636 0.0159618245542836
2730.40727272727 0.0157409413861202
2769.33818181818 0.0155260608250249
2808.26909090909 0.0153169403693733
2847.2 0.0151133504556829
2886.13090909091 0.014915073604662
2925.06181818182 0.0147219036341609
2963.99272727273 0.0145336449329764
3002.92363636364 0.0143501117900829
3041.85454545455 0.0141711277744075
3080.78545454545 0.013996525160753
3119.71636363636 0.0138261443979063
3158.64727272727 0.0136598336153526
3197.57818181818 0.0134974481653605
3236.50909090909 0.0133388501975084
3275.44 0.0131839082629992
3314.37090909091 0.0130324969463526
3353.30181818182 0.0128844965222877
3392.23272727273 0.0127397926358055
3431.16363636364 0.0125982760036576
3470.09454545455 0.0124598421355502
3509.02545454545 0.0123243910735744
3547.95636363636 0.0121918271484864
3586.88727272727 0.0120620587515775
3625.81818181818 0.0119349981209806
3664.74909090909 0.0118105611413575
3703.68 0.0116886671559982
3742.61090909091 0.0115692387904418
3781.54181818182 0.0114522017868029
3820.47272727273 0.0113374848480509
3859.40363636364 0.0112250194915521
3898.33454545455 0.0111147399112347
3937.26545454545 0.0110065828477918
3976.19636363636 0.0109004874663782
4015.12727272727 0.0107963952413011
4054.05818181818 0.010694249847242
4092.98909090909 0.0105939970565806
4131.92 0.0104955846424261
};
\addplot [draw=black, fill=black, mark=x, very thick, mark size=2.5pt, only marks]
table{%
x  y
68.72 0.802580756712449
277.76 0.466927426982489
1096.96 0.215521356347796
4357.12 0.074220069374092
};
