# Supplementary material for: Swarm Reinforcement Learning For Adaptive Mesh Refinement
Source: arXiv:2304.00818 source file (2023-10-09)
Supplement: Supplementary file 17 [file group_baselines_1.tex]

\nextgroupplot[
ylabel shift = -0.2cm,
clip marker paths=true,
width=0.52\textwidth,
height=4.5cm,
title style={yshift=-0.2cm},
scaled x ticks=false,
legend cell align={left},
legend style={fill opacity=0.8, draw opacity=1, text opacity=1, draw=lightgray204},
log basis y={10},
tick align=outside,
tick pos=left,
title={Poisson - PPO and DQN},
x grid style={darkgray176},
xlabel={Elements \(\displaystyle (\times 10^3)\)},
xmajorgrids,
xmin=-359.444, xmax=8030.124,
xtick style={color=black},
xtick={-1000,0,1000,2000,3000,4000,5000,6000,7000,8000,9000},
xticklabels={-1.0,0.0,1.0,2.0,3.0,4.0,5.0,6.0,7.0,8.0,9.0},
y grid style={darkgray176},
ylabel={Squared Error},
ymajorgrids,
ymin=3.20971195110356e-06, ymax=2.0984975199912,
ymode=log,
ytick style={color=black},
ytick={1e-07,1e-06,1e-05,0.0001,0.001,0.01,0.1,1,10,100},
yticklabels={
  \(\displaystyle {10^{-7}}\),
  \(\displaystyle {10^{-6}}\),
  \(\displaystyle {10^{-5}}\),
  \(\displaystyle {10^{-4}}\),
  \(\displaystyle {10^{-3}}\),
  \(\displaystyle {10^{-2}}\),
  \(\displaystyle {10^{-1}}\),
  \(\displaystyle {10^{0}}\),
  \(\displaystyle {10^{1}}\),
  \(\displaystyle {10^{2}}\)
}
]
\addplot [
  draw=royalblue28108204,
  fill=royalblue28108204,
  forget plot,
  mark=*, mark size=1,
  only marks,
  draw opacity=0,
 fill opacity=0.5
]
table{%
x  y
219.22 0.0116380025783674
236.58 0.00893751131252496
255.06 0.00757221773421185
266.3 0.00695152587324572
277.02 0.00870449843080493
289.06 0.00650849332548639
301.82 0.00650772537377039
309.02 0.00632830538267971
313.48 0.00852456067483164
317.48 0.00503420224308783
366.78 0.00472734343816265
384.24 0.00384945126787151
427.52 0.00440570193112838
431.14 0.00387196288409598
433.8 0.0031068838328975
438.92 0.0033561305566538
446.06 0.00325148782214415
485 0.00270934352590588
524.5 0.0019590317268996
530.98 0.0024847849713976
530.98 0.0024462804500235
542.2 0.00339373662958677
568.26 0.00191195330793864
569.1 0.00200759214947172
579.8 0.00192121084682089
587.66 0.00166535004820132
612.06 0.00170099739413765
628 0.00142557999535175
636.98 0.00193167521782833
648.04 0.00147630841918046
648.78 0.00196488850395651
684.76 0.00192456325257735
704.12 0.00152017798836435
708.02 0.00171515266408961
724.56 0.00106290863523144
740.7 0.00145038634314574
740.82 0.00126611233262213
754.68 0.0010958404611985
776.14 0.00136681288549904
861 0.00122261947029662
866.82 0.0012376456173406
951.18 0.000684639740045543
978.82 0.000682995459645206
1030.58 0.000639142132617508
1031.2 0.000608987227553708
1080.16 0.000534351174466062
1116.56 0.000522936657826564
1126.22 0.00047220578013082
1173.32 0.000587407673606018
1183.24 0.000496992672901857
1212.6 0.000433759599768057
1270.84 0.000477030829124065
1271.28 0.00057574970357699
1312.64 0.000295338105933881
1334.88 0.0003688460635094
1390.92 0.000632823129081481
1414.42 0.000439822660083419
1465.2 0.000380405825070989
1546.18 0.000259777992401812
1645.64 0.000189432782231567
1650.1 0.00040730379394757
1712.26 0.000225696747843442
1799.62 0.000205137266591349
1800.64 0.000149688394684308
1820.82 0.00022968203197516
1908.42 0.000134858938308452
1925.1 0.000231468966668099
2020.12 0.000123482420852495
2156.38 0.000114435638078513
2168.78 0.000132258579214635
2169 0.000101440195225082
2212 0.000202015930911123
2238.3 0.000100444720362762
2307.32 0.00010430451268494
2321.26 0.000101348576943888
2363.12 7.85396281013735e-05
2399.82 8.97496755911525e-05
2432.68 0.000175103698214891
2457.16 9.48685731254995e-05
2655.7 7.07642905549767e-05
2715.22 5.85765922707877e-05
3044.4 5.85685554721719e-05
3414.76 4.01750628140733e-05
3545.46 3.80019302781983e-05
3591.66 3.62548169075136e-05
3997.22 3.19018762058348e-05
4033.6 2.70246768067793e-05
4075.94 2.55319826966762e-05
4148.74 2.90210310242148e-05
4304.56 2.36833753484687e-05
4311.96 4.28165553247746e-05
4611.22 2.13677683411378e-05
5764.26 1.3085878413959e-05
6013.74 1.0832458588431e-05
6168.52 9.73742044189171e-06
6591.82 8.02970379055727e-06
6800.42 8.43665609892419e-06
6819.78 8.29434337198603e-06
7381.26 8.13257734004449e-06
7648.78 6.34432528857979e-06
};
\addplot [
  draw=deepskyblue33188255,
  fill=deepskyblue33188255,
  forget plot,
  mark=*, mark size=1,
  only marks,
  draw opacity=0,
 fill opacity=0.5
]
table{%
x  y
67.12 0.274932892587417
69.96 0.342723365162031
72.88 0.314279445369378
74 0.374849486341033
76.54 0.360590354581867
81.3 0.280761761190646
82.02 0.297311536511093
83 0.245092346344684
115.78 0.180782101761938
127.48 0.0543698416446811
139.68 0.0556973545314571
161.24 0.0280664719273081
167.56 0.0189963467331159
183.32 0.016692860765121
183.48 0.0141410870278135
211.88 0.0131662464444706
222.68 0.0107078782657071
222.82 0.0104504203934784
224.2 0.0097667456654264
226.16 0.00889764113033695
227.8 0.0105370727097946
230.62 0.00961740137535413
233 0.0110310414501627
242.64 0.0108643021103302
245.36 0.00815729518883757
267.88 0.007054897957978
278.52 0.00778970732239858
293.24 0.00585470732846399
301.6 0.00615197924972588
305.2 0.00555355672499418
308.36 0.00640557383232012
318.72 0.00502319640621388
319 0.00585132572676869
336.12 0.00562202106895174
357.74 0.0060544352316222
377.12 0.00402801406813961
378.68 0.00358847340063646
390.86 0.00373844419723932
398.3 0.00483505017377062
458.98 0.00356399726932389
469.76 0.0027410241713925
491.02 0.00344853088089428
504.64 0.00269577763259578
540.94 0.00357182468584512
545.36 0.00284614864616167
557.58 0.00237596105254284
569.76 0.00223136659105867
616.92 0.00168541443694532
677.84 0.00214427574731812
701.72 0.00194158349932435
723.92 0.001958035102238
762.02 0.00162451584839585
888.52 0.00356102070285189
957.72 0.00121188428129852
1005.98 0.00657887872200523
1029.9 0.00107714625445396
1587.78 0.000283735537225628
1601.54 0.00230958801314524
1619.84 0.000642928879226042
1658.04 0.0036552564079319
1694.84 0.00526189479381342
1714.48 0.000370429239380156
1748.04 0.000488947162849054
1880.9 0.000481418916735077
2075.14 0.00196924393577724
2129.9 0.00345285296214634
2156.64 0.00137862081590548
2328.06 0.000957717008711116
2351.28 0.000402768900861255
2359.26 0.00227748273789986
2485.76 0.000543220117972678
2527.62 0.00208399837827023
2728.82 0.000276054713098941
2909 0.000362776379695944
2956.48 0.000682271123883172
2969.56 0.00024480490889658
3250.08 0.000270102187395557
3339.06 0.000441881124425598
3436.78 0.000272866752993649
3489 0.000319621838905127
3502.6 0.000134096606688546
3740.96 0.000277534912921662
3952.22 0.000163795770233056
4810.02 7.10054033455952e-05
5018.84 0.000219262416081652
5355.54 0.000180119023385072
5693.36 0.000150174263963767
5783.3 0.000122989187748913
6106.08 8.40403457368597e-05
6238.5 7.09746632561938e-05
6693.94 3.90790296381896e-05
7234.5 4.2105903839035e-05
7238.42 4.8545210778773e-05
7282.34 4.38843545726443e-05
7511.94 4.30176005565315e-05
7606 4.14067695224761e-05
7677.68 3.79374261222289e-05
8027.04 2.40439875989482e-05
};
\addplot [
  draw=cadetblue80178158,
  fill=cadetblue80178158,
  forget plot,
  mark=*, mark size=1,
  only marks,
  draw opacity=0,
 fill opacity=0.5
]
table{%
x  y
238.86 0.0314591256860586
259.2 0.0279614216442924
266.94 0.0440459298859297
270.78 0.0318815823464054
275.54 0.0593514293437776
292.74 0.0207354951700831
293.06 0.0221127116170605
307.06 0.0209106646236632
330.7 0.0702922818937551
350.14 0.0807482460346126
387.32 0.0620047069674773
426.5 0.00592632357712872
441.78 0.00526383493362311
449.52 0.00894098739715834
502.08 0.0128625751437315
527.28 0.00764885638127966
564.38 0.0278710432660707
581.08 0.00737865073205254
607.64 0.0116848347806724
657.88 0.0259621669592313
679.92 0.00755933491914977
695 0.00257071214077956
695.84 0.00395982101856514
702.54 0.0352949317001577
710.8 0.00739388781093521
765.8 0.00489009062296662
780.24 0.0120847799816269
789.02 0.00435340001031618
797.66 0.0791101360827437
870.48 0.215947865448271
877.5 0.202251458564746
953.76 0.00785133509905537
959.74 0.00230121519966155
963.22 0.00206243086349683
964.68 0.0083785913521835
1000.26 0.00346978020975467
1009.96 0.004142049657295
1047.06 0.00225157380159124
1122.86 0.003062103305598
1139.62 0.0020778500532229
1194.2 0.149376206797811
1203.38 0.00109219342001367
1237.52 0.017414815893132
1269.76 0.00153445767684243
1308.66 0.0101006962225929
1343.88 0.00195426204490739
1403.68 0.186316022036712
1474.82 0.00518823390213346
1483.06 0.00137966614553141
1508.22 0.00241542593084506
1533.24 0.108028873012002
1558.36 0.00154318317939186
1623.28 0.00324453968222031
1652.94 0.00306113530930337
1683.24 0.00136663132183301
1769.66 0.00043475425513794
1780.54 0.000525754510912481
1972.86 0.000937671471083318
1977.3 0.00144378189022144
2010.66 0.000830648873741841
2054.24 0.00866340439454498
2158.24 0.000664382562999057
2213.06 0.000443453811901927
2247.66 0.00487431109654702
2270.74 0.00172876918014416
2334.56 0.000310206885374613
2362.8 0.263314397040719
2473.06 0.00119230634636316
2481.1 0.000386263868361426
2492.44 0.000349575358333937
2507.76 0.00122087231252026
2526.96 0.00072060660227723
2528.42 0.000359101194848207
2681.3 0.00184721059179259
2719.26 0.0056335828642175
2783.24 0.000464571417157986
2793.82 0.000547802481503746
2812.56 0.122094542705312
2814.86 0.000552381231239201
2914.52 0.000395045921821014
2958.5 0.026449141273229
2974 0.00147822884589543
2979.64 0.0154154293281526
3023.04 0.00117847278133127
3044.12 0.00771705726110193
3145.88 0.000208994471589525
3162.34 0.00085605260280606
3183.74 0.0238842006531611
3285.24 0.000110283822470742
3285.78 0.000164999251045578
3304.3 0.000293792721768415
3309.32 0.000517710651832717
3351.3 0.000455257895227682
3373.9 0.000130315097348245
3462.92 0.0001628222984189
3705.6 0.000490453853139452
3714.04 0.000242224384089039
3748.38 0.0332845233781071
3834.84 0.000446808641735386
4033.74 0.00301583029691757
};
\addplot [
  draw=yellowgreen18420623,
  fill=yellowgreen18420623,
  forget plot,
  mark=*, mark size=1,
  only marks,
  draw opacity=0,
 fill opacity=0.5
]
table{%
x  y
244.32 0.090075782688065
244.88 0.109434139301195
245.08 0.0257485802076113
246.66 0.0319417364482202
246.68 0.0548414670190473
257.62 0.0184315460486026
275.78 0.0233197970492585
305.24 0.00992524200971177
351.18 0.0175573457720558
415.96 0.0159193397204821
463.3 0.0406281150085113
465.04 0.0363616124201708
467.22 0.0149392295395897
467.28 0.0463968487277582
481.46 0.00644705255039603
500.76 0.00980600717282935
538.1 0.0044633500103474
550.04 0.0082477616334409
696.98 0.0238174719516775
710.02 0.0226813281819729
711.2 0.011943111407373
732.94 0.00304851814596999
737.94 0.0622659741655246
758.66 0.0036070851654307
766.48 0.0088618915315481
796.02 0.00261507735918053
800.1 0.197816347921407
871.56 0.280022302517727
878.34 0.00736867959357902
908.5 0.069594799734745
960.82 0.0659449739818918
1052.48 0.087120647001372
1098.14 0.0187108634446874
1109.36 0.0363869001640209
1128.72 0.253279861452165
1133.84 0.0305863002559521
1157.46 0.205195693139551
1206.22 0.00241511394310093
1216.3 0.00180977353045468
1249.64 0.00470878817219607
1257.7 0.0137983162875369
1260.42 0.0172895964946628
1272.7 0.00202877948911481
1301.5 0.00312475809324292
1321.06 0.0248122369459888
1333.36 0.00336762978361213
1355.6 0.0679735125493375
1367.24 0.0696604349292033
1382.4 0.00204078974368802
1522.78 0.0727738032747131
1572.82 0.0240896253184665
1708.44 0.00264819906538342
1804.54 0.0122247258638785
1806.72 0.288307608218984
1883.96 0.000892923776330306
1894.3 0.0155009807613662
1909.44 0.0290652752507714
2139.68 0.00889350201319023
2141.38 0.342028428061974
2219.72 0.0379310567065358
2276.28 0.0112003406009744
2283.28 0.0101019676756105
2312.88 0.00125647547512504
2425.26 0.00197250228679418
2675.86 0.0166840787855928
2684.42 0.00316133603912716
2726.06 0.0778058664657079
2753.92 0.00229044061456281
2828.42 0.00381723315047638
2954.98 0.0898560499270886
3043.14 0.0165622765711776
3097.74 0.00161791497467868
3108.82 0.00132867969616638
3177.82 0.00872916076733772
3200.28 0.00305058820682227
3213.94 0.131598248865593
3226.86 0.140073511150775
3230.76 0.000531245217366844
3243.48 0.0061275690395519
3261.36 0.00885273674728312
3293.22 0.000842474495452092
3422.14 0.00488261390579161
3556.4 0.000539546486964627
3593.72 0.054974313837116
3912.88 0.020326272409881
3946.86 0.0220496406891058
4005.22 0.00434961061247644
4076.6 0.0042031886078477
4130.68 0.185027081425596
4294.94 0.0128992555213749
4320.4 0.148319285997057
4636.56 0.161414509596417
4686.52 0.0160638169882923
4806.56 0.00325384806681742
4833.72 0.00501434624656875
4989.44 0.00249675694532084
5050.16 0.00548111671174564
5069.26 0.0456408292869426
5805.02 0.00535089865642049
6598.36 0.213086945268102
};
\addplot [
  draw=chocolate21910927,
  fill=chocolate21910927,
  forget plot,
  mark=*, mark size=1,
  only marks,
  draw opacity=0,
 fill opacity=0.5
]
table{%
x  y
21.9 0.999999998927878
21.9 0.999999998927878
21.92 0.999999998950274
21.92 0.999999998950274
21.92 0.999999998950274
21.92 0.999999998950274
21.92 0.999999998950274
21.92 0.999999998950274
21.92 0.999999998950274
21.92 0.999999998950274
21.92 0.999999998950274
21.92 0.999999998950274
21.92 0.999999998950274
21.92 0.999999998950274
21.92 0.999999998950274
21.92 0.999999998950274
21.92 0.999999998950274
21.92 0.999999998950274
21.92 0.999999998950274
21.92 0.999999998950274
21.92 0.999999998950274
21.92 0.999999998950274
21.92 0.999999998950274
21.92 0.999999998950274
21.92 0.999999998950274
21.92 0.999999998950274
21.92 0.999999998950274
21.92 0.999999998950274
21.92 0.999999998950274
21.92 0.999999998950274
21.92 0.999999998950274
21.92 0.999999998950274
21.94 0.999999998905941
21.94 0.999999998905941
21.94 0.999999998905941
21.94 0.999999998905941
22 0.999999998889839
22.02 0.999999998899304
22.16 0.999999998640609
22.28 0.999999998477158
26.5 0.970894204249672
32.62 0.924277946638112
34.96 0.862638850036096
91.4 0.720312311243077
94.9 0.18919499810567
108.74 0.71958749216895
134.98 0.0689210131272957
136.1 0.0613824673087774
155.44 0.0559306313583098
208.3 0.197146125458646
249.98 0.0499246702086478
271.24 0.0325903579711196
274.72 0.0511839347070228
283.88 0.043017706650582
308.14 0.288765844789137
329.14 0.0162289718257283
338.64 0.034337015545152
357.98 0.0101646670694072
386.82 0.0167657064564419
395.32 0.0042305451504377
403.3 0.0119398370592536
430.36 0.0289122109821289
531.96 0.11696073594285
595.12 0.58453985126498
642.3 0.00386796707321375
670.92 0.00302893160661771
695.68 0.00347257940790675
722.02 0.0391289662856242
762.26 0.00451677919851355
1152.26 0.0261976517911636
1233.2 0.000998733802377771
1272.96 0.000876420935487872
1282.64 0.00102417788068937
1315.36 0.000594576789097483
1410.32 0.00146055096768862
1658.3 0.0267799322922428
1817.54 0.222864808756589
1978.66 0.000274269869038731
2059.9 0.00791404372976221
2070.98 0.000261190457505995
2305.2 0.225290493210452
3213.16 0.000133900698026789
3434.82 0.000663721741809451
4206.7 0.000806185856602349
4447.52 0.000113588426911867
4668.8 0.000258317240468995
5045.36 4.79021802088747e-05
7591.98 3.04719971098142e-05
};
\addplot [
  draw=indianred19152101,
  fill=indianred19152101,
  forget plot,
  mark=*, mark size=1,
  only marks,
  draw opacity=0,
 fill opacity=0.5
]
table{%
x  y
21.9 0.999999998927878
21.92 0.999999998950274
21.92 0.999999998950274
21.92 0.999999998950274
21.92 0.999999998950274
21.92 0.999999998950274
21.92 0.999999998950274
21.92 0.999999998950274
21.92 0.999999998950274
21.92 0.999999998950274
21.92 0.999999998950274
21.92 0.999999998950274
21.92 0.999999998950274
21.92 0.999999998950274
21.92 0.999999998950274
21.92 0.999999998950274
21.94 0.999999998905941
22.38 0.999999998494591
86.16 0.352216255032009
86.7 0.328547431631386
87.62 0.333654605600169
87.82 0.327681198323879
88.02 0.278882512794496
88.48 0.331261231703773
98.84 0.335670490636036
106.34 0.241557736491125
140.92 0.148468863169787
156.9 0.170137577476667
289.68 0.105000482512224
304.32 0.12291727942287
310.04 0.0607944562954501
328.7 0.0759163945619775
337.14 0.0512447073997889
339.8 0.040078161734014
342.54 0.0337325032274052
344 0.0365478747195187
348.34 0.028434513304812
351.52 0.0356325093723456
353.08 0.030532771021612
541.1 0.842374535290012
604 0.847835186553072
1066.6 0.719452089607114
1161.2 0.71149606072708
1241.9 0.628152527619007
1300.1 0.622316725184108
1371.64 0.00698772015796695
1382.84 0.00744094377942691
1394.46 0.00577677810582207
1413.48 0.00453148829487134
1416.12 0.0049413720239298
1464.54 0.62118803329771
1531.92 0.0148022976249967
1540.94 0.563534779091307
1543.56 0.54399752624644
1661.74 0.571031223733867
1692.52 0.456822063532561
1753.86 0.511927198179604
1815.12 0.510281719283338
1826.28 0.532736890524313
1836.16 0.0139742540562555
1972.88 0.488244891128931
2005.12 0.0852287293132581
2010.78 0.474055521200355
2018.06 0.497930576781945
2068.12 0.403685355389766
2085.48 0.451446348939405
2113.92 0.414092602236795
2190 0.084093059681537
2235.3 0.381732205329873
2418.2 0.413228171556552
2420.1 0.41892685011743
2426.32 0.0588653508481712
2454.64 0.0558491051519919
2475.16 0.383542144648091
2499.44 0.0113230297192077
2529.36 0.0516671835662763
2532.8 0.0526988047949506
2827.84 0.00901071062612392
2836.6 0.0657179888381315
2841.06 0.313361505311296
3010.8 0.0526385785718605
3096.32 0.00727159705070947
3099.4 0.0474182263176894
3260.16 0.00737793041954566
3443.18 0.227858206416832
3484.24 0.131416343069701
3508.8 0.00650174839867577
3511.04 0.00727476484986376
4037.28 0.00626809931282519
4569.52 0.00220340056657374
4866.56 0.00095351629334446
4887.2 0.00682488843617527
5201.6 0.000876717946282604
6030.08 0.000706079536671927
6155.52 0.000759127934097835
6275.84 0.000695731218746723
6695.68 0.000681034516802472
};
\addplot [draw=purple11522131, fill=purple11522131, forget plot, mark=*, mark size=1, only marks, draw opacity=0,
 fill opacity=0.5]
table{%
x  y
78.58 0.301493427330464
85.08 0.274455743146065
85.76 0.247059957310875
104.82 0.127743695311313
116.6 0.135439329155988
118.2 0.174983189580105
120.4 0.0964925082987315
121.34 0.0988675248837244
135.02 0.112585768954093
197.68 0.0829814200198853
210.46 0.0645671680607277
223.72 0.0607998674259802
241.1 0.0504275656964269
297.98 0.0553802062154436
311.14 0.0404930406669039
323.64 0.022991687600625
333.94 0.0274936611138742
341.18 0.0269801010301793
341.2 0.028156653231875
342.48 0.00992160065898382
343.86 0.0267192329551306
346.56 0.0261208939579781
349.9 0.0251530914362062
351.26 0.0227907233444659
352.64 0.0239397173789617
355.92 0.0191090303397534
364.18 0.0218794329430158
370.24 0.0200638785751326
376.04 0.0136155573179307
381.9 0.0146785342366676
385.72 0.012640642012926
409 0.0129078349935975
418.96 0.00933051668986954
447.7 0.00934748444519734
452.28 0.0229373947300776
493.02 0.0056858045394716
499.32 0.00694086566029311
552.38 0.00895209879479779
572.84 0.00505305561248642
786.28 0.00258348532329224
833.92 0.00320550253911646
1257.9 0.00215555030491081
1339.34 0.00195086299350352
1353.52 0.00209068490575845
1356.5 0.00222798967646156
1396.46 0.00190324922233753
1421.5 0.00176630035985534
1422.22 0.00180824419903394
1425.32 0.001896163401944
1426.54 0.00176777019284238
1429.28 0.00170450464911716
1429.56 0.00189968336381655
1432.82 0.00177489483284763
1449.28 0.00189240844296632
1449.38 0.00189070300363587
1450.16 0.00193782213005509
1450.24 0.00189066552594398
1456.6 0.00190102776276496
1456.6 0.00190102776276496
1462.96 0.00198042805162412
1469.72 0.00162821515839203
1482.54 0.00132975900752616
1516.94 0.00106385341758505
1527.66 0.00105963343820681
1574.24 0.000997338909699857
1613.18 0.000647274604876434
1892.02 0.000604202070923351
1919.8 0.000576682497257652
1930.46 0.000710916067721463
2102.78 0.000469878926949001
2190.92 0.00081450106318767
2593.9 0.000243552880772975
3084.76 0.000263576696379211
3435.3 0.000184887847662381
3657.84 0.000203971119068862
3703.24 0.000186005272034085
3759.92 0.000197947946581525
3996.78 0.000188218954708874
4612.32 0.000214224514655938
5706.3 0.000144931275103409
5716.12 0.000155178357462367
5718.68 0.000144788209431815
5744.66 0.000144619952836946
5765.12 0.000144604747120997
5765.12 0.000144604747120997
5765.12 0.000144604747120997
5765.12 0.000144604747120997
5765.12 0.000144604747120997
5765.12 0.000144604747120997
5765.12 0.000144604747120997
5765.12 0.000144604747120997
5765.12 0.000144604747120997
5765.12 0.000144604747120997
5765.12 0.000144604747120997
5765.12 0.000144604747120997
5765.12 0.000144604747120997
5765.12 0.000144604747120997
5765.12 0.000144604747120997
5765.12 0.000144604747120997
5765.12 0.000144604747120997
};
\addplot [draw=plum223165229, fill=plum223165229, forget plot, mark=*, mark size=1, only marks, draw opacity=0,
 fill opacity=0.5]
table{%
x  y
296.9 0.0358713532833776
300.96 0.059667815878781
310.18 0.0246002598763836
324.32 0.0254690408326361
335.44 0.0252901770260925
338.94 0.0351965556839638
345.8 0.0256987816474409
347.42 0.0278380917362482
348.18 0.0259587621937394
351.36 0.0259470568426135
367.14 0.0244078530873143
407.04 0.018338722781902
407.68 0.0183284468300385
407.68 0.0183284468300385
407.68 0.0183284468300385
407.68 0.0183284468300385
407.68 0.0183284468300385
407.68 0.0183284468300385
407.68 0.0183284468300385
418.84 0.0183461801310535
484.44 0.00464487734480351
563.02 0.00545977619112424
618.84 0.0050701184583912
660.36 0.00504450302121668
889.08 0.00410483805752702
930.02 0.00238949194633018
943.82 0.00618046910583975
1001.86 0.00395759903055264
1014.86 0.00241242495362745
1233.78 0.00221174766337112
1291.2 0.0048699598223877
1302.08 0.0031415816177967
1302.08 0.0031415816177967
1302.08 0.0031415816177967
1352.82 0.00207709975505853
1412.3 0.00193380207474083
1442.56 0.0019158615610468
1450.24 0.00189066552594398
1450.24 0.00189066552594398
1450.24 0.00189066552594398
1450.24 0.00189066552594398
1450.24 0.00189066552594398
1450.24 0.00189066552594398
1450.24 0.00189066552594398
1450.24 0.00189066552594398
1450.24 0.00189066552594398
1450.24 0.00189066552594398
1450.24 0.00189066552594398
1450.24 0.00189066552594398
1450.24 0.00189066552594398
1453.28 0.00164964024886823
1458.86 0.00163651067158695
1474.56 0.00160526611830022
1474.56 0.00160526611830022
1474.56 0.00160526611830022
1474.56 0.00160526611830022
1474.56 0.00160526611830022
1474.56 0.00160526611830022
1474.56 0.00160526611830022
1474.56 0.00160526611830022
1737.8 0.000886671338028735
4017.88 0.000557434410574582
4119.04 0.000379207314951963
4119.04 0.000379207314951963
4119.04 0.000379207314951963
4119.04 0.000379207314951963
4119.04 0.000379207314951963
4119.04 0.000379207314951963
4119.04 0.000379207314951963
4119.04 0.000379207314951963
5652.16 0.000648542524741823
5670.42 0.000526149494892928
5673.92 0.000384987211300264
5693.38 0.000339874579145489
5729.78 0.000565570668288296
5749.56 0.000572141093437812
5765.12 0.000144604747120997
5765.12 0.000144604747120997
5765.12 0.000144604747120997
5765.12 0.000144604747120997
5765.12 0.000144604747120997
5765.12 0.000144604747120997
5765.12 0.000144604747120997
5765.12 0.000144604747120997
5765.12 0.000144604747120997
5765.12 0.000144604747120997
5765.12 0.000144604747120997
5765.12 0.000144604747120997
5765.12 0.000144604747120997
5765.12 0.000144604747120997
5765.12 0.000144604747120997
5765.12 0.000144604747120997
5765.12 0.000144604747120997
5765.12 0.000144604747120997
5765.12 0.000144604747120997
5765.12 0.000144604747120997
5765.12 0.000144604747120997
5765.12 0.000144604747120997
5765.12 0.000144604747120997
5767.06 0.000582506940661614
};
\addplot [very thick, royalblue28108204]
table {%
219.22 0.011036362330508
294.266060606061 0.00683752177615596
369.312121212121 0.00464144864349475
444.358181818182 0.00334666716525019
519.404242424242 0.0025193038327363
594.450303030303 0.00195898836228103
669.496363636364 0.00156242272863255
744.542424242424 0.00127184853740656
819.588484848485 0.00105288309708372
894.634545454545 0.000884011430865333
969.680606060606 0.000751210162546177
1044.72666666667 0.000645022898528129
1119.77272727273 0.000558886634562944
1194.81878787879 0.000488132454642395
1269.86484848485 0.000429366813814566
1344.91090909091 0.000380076270852898
1419.95696969697 0.000338367971794018
1495.00303030303 0.0003027951072934
1570.04909090909 0.000272236981973959
1645.09515151515 0.000245815016365929
1720.14121212121 0.000222832893735278
1795.18727272727 0.000202733241627402
1870.23333333333 0.000185065832838411
1945.27939393939 0.000169463938324359
2020.32545454545 0.000155626532140522
2095.37151515152 0.000143304752953709
2170.41757575758 0.00013229149937599
2245.46363636364 0.000122413358503866
2320.5096969697 0.00011352428972744
2395.55575757576 0.00010550064185257
2470.60181818182 9.82371921850629e-05
2545.64787878788 9.16439755603686e-05
2620.69393939394 8.56437288176314e-05
2695.74 8.01698183332399e-05
2770.78606060606 7.51645493600184e-05
2845.83212121212 7.05777791330937e-05
2920.87818181818 6.63657731597201e-05
2995.92424242424 6.24902573397632e-05
3070.9703030303 5.89176286642295e-05
3146.01636363636 5.56182950054424e-05
3221.06242424242 5.25661205236171e-05
3296.10848484848 4.97379578968152e-05
3371.15454545455 4.71132522503113e-05
3446.20060606061 4.46737045530535e-05
3521.24666666667 4.24029845402706e-05
3596.29272727273 4.02864850465218e-05
3671.33878787879 3.83111110946094e-05
3746.38484848485 3.64650982610337e-05
3821.43090909091 3.47378557882919e-05
3896.47696969697 3.31198306849694e-05
3971.52303030303 3.16023896826275e-05
4046.56909090909 3.01777164323574e-05
4121.61515151515 2.88387217459749e-05
4196.66121212121 2.75789650348172e-05
4271.70727272727 2.63925853870252e-05
4346.75333333333 2.52742409632466e-05
4421.79939393939 2.42190555898078e-05
4496.84545454546 2.32225715948118e-05
4571.89151515152 2.22807080720926e-05
4646.93757575758 2.13897238752291e-05
4721.98363636364 2.05461847426933e-05
4797.0296969697 1.97469340388092e-05
4872.07575757576 1.89890666660709e-05
4947.12181818182 1.8269905764614e-05
5022.16787878788 1.75869818659648e-05
5097.21393939394 1.69380142120492e-05
5172.26 1.63208939879861e-05
5247.30606060606 1.57336692494166e-05
5322.35212121212 1.51745313528374e-05
5397.39818181818 1.46418027212986e-05
5472.44424242424 1.41339257984621e-05
5547.4903030303 1.3649453061884e-05
5622.53636363636 1.31870379818742e-05
5697.58242424242 1.2745426825751e-05
5772.62848484848 1.23234512190284e-05
5847.67454545455 1.19200213852963e-05
5922.72060606061 1.15341199954871e-05
5997.76666666667 1.1164796565038e-05
6072.81272727273 1.08111623443141e-05
6147.85878787879 1.04723856536745e-05
6222.90484848485 1.0147687619861e-05
6297.95090909091 9.83633827504848e-06
6372.99696969697 9.53765298401601e-06
6448.04303030303 9.25098916853041e-06
6523.08909090909 8.97574330125288e-06
6598.13515151515 8.71134814433109e-06
6673.18121212121 8.45727021036785e-06
6748.22727272727 8.21300742570822e-06
6823.27333333333 7.97808697798452e-06
6898.31939393939 7.75206333164318e-06
6973.36545454545 7.53451639676642e-06
7048.41151515152 7.32504983792122e-06
7123.45757575758 7.12328951103846e-06
7198.50363636364 6.92888201746202e-06
7273.5496969697 6.74149336532551e-06
7348.59575757576 6.56080772932964e-06
7423.64181818182 6.38652630081431e-06
7498.68787878788 6.21836622075785e-06
7573.73393939394 6.05605958900093e-06
7648.78 5.89935254359227e-06
};
\addplot [very thick, deepskyblue33188255]
table {%
67.12 0.194322905301588
147.523232323232 0.0389603315259027
227.926464646465 0.0169469869460534
308.329696969697 0.00972867351573159
388.732929292929 0.006438431315139
469.136161616162 0.00464402553206365
549.539393939394 0.00354798173698328
629.942626262626 0.00282408629883527
710.345858585859 0.00231786037768443
790.749090909091 0.00194807726625454
871.152323232323 0.00166852510764028
951.555555555556 0.00145124337331692
1031.95878787879 0.00127845659188188
1112.36202020202 0.00113839559003991
1192.76525252525 0.00102299856647704
1273.16848484849 0.000926581587501575
1353.57171717172 0.000845036589235003
1433.97494949495 0.00077532979367625
1514.37818181818 0.000715178037747631
1594.78141414141 0.000662834112027694
1675.18464646465 0.000616940914282565
1755.58787878788 0.000576430206018487
1835.99111111111 0.000540450967220817
1916.39434343434 0.000508317811121294
1996.79757575758 0.000479473255881079
2077.20080808081 0.000453459734939425
2157.60404040404 0.000429898560213252
2238.00727272727 0.000408473921176177
2318.4105050505 0.000388920579891792
2398.81373737374 0.000371014311833598
2479.21696969697 0.000354564409694729
2559.6202020202 0.000339407753451538
2640.02343434343 0.000325404081153939
2720.42666666667 0.00031243218859151
2800.8298989899 0.000300386853637571
2881.23313131313 0.000289176330460305
2961.63636363636 0.000278720295206705
3042.0395959596 0.000268948151872447
3122.44282828283 0.000259797627428269
3202.84606060606 0.000251213600689982
3283.24929292929 0.000243147121186416
3363.65252525253 0.00023555458332851
3444.05575757576 0.000228397028190359
3524.45898989899 0.000221639550676393
3604.86222222222 0.000215250794135265
3685.26545454545 0.000209202517864381
3765.66868686869 0.000203469225634956
3846.07191919192 0.00019802784551143
3926.47515151515 0.000192857452959394
4006.87838383838 0.000187939030623401
4087.28161616162 0.000183255259280066
4167.68484848485 0.000178790335386748
4248.08808080808 0.000174529811394009
4328.49131313131 0.000170460455604067
4408.89454545455 0.000166570128863534
4489.29777777778 0.000162847675797474
4569.70101010101 0.00015928282863956
4650.10424242424 0.000155866122002997
4730.50747474748 0.000152588817179231
4810.91070707071 0.0001494428347549
4891.31393939394 0.000146420694508691
4971.71717171717 0.000143515461694329
5052.1204040404 0.000140720698938356
5132.52363636364 0.000138030423085344
5212.92686868687 0.000135439066411716
5293.3301010101 0.000132941441705023
5373.73333333333 0.000130532710770187
5454.13656565657 0.000128208355979864
5534.5397979798 0.000125964154533839
5614.94303030303 0.000123796155133617
5695.34626262626 0.00012170065681401
5775.7494949495 0.000119674189704388
5856.15272727273 0.000117713497519075
5936.55595959596 0.00011581552159968
6016.95919191919 0.000113977386352474
6097.36242424242 0.000112196385941701
6177.76565656566 0.000110469972115215
6258.16888888889 0.000108795743052482
6338.57212121212 0.000107171433136945
6418.97535353535 0.000105594903565253
6499.37858585859 0.000104064133715172
6579.78181818182 0.00010257721320216
6660.18505050505 0.00010113233456183
6740.58828282828 9.97277865019539e-05
6820.99151515152 9.83619476733479e-05
6901.39474747475 9.70332809140165e-05
6981.79797979798 9.57403279254586e-05
7062.20121212121 9.44817043440272e-05
7142.60444444445 9.32560951738035e-05
7223.00767676768 9.20622505506693e-05
7303.41090909091 9.08989818100815e-05
7383.81414141414 8.9765157833645e-05
7464.21737373737 8.86597016518467e-05
7544.62060606061 8.75815872824091e-05
7625.02383838384 8.65298367855362e-05
7705.42707070707 8.55035175190291e-05
7785.8303030303 8.45017395777254e-05
7866.23353535354 8.35236534030924e-05
7946.63676767677 8.25684475500184e-05
8027.04 8.16353465989585e-05
};
\addplot [very thick, cadetblue80178158]
table {%
238.86 0.0371374481061499
277.192121212121 0.0322000316184874
315.524242424242 0.0282624616721036
353.856363636364 0.0250580922872224
392.188484848485 0.0224064835106428
430.520606060606 0.0201812887720372
468.852727272727 0.0182914747845647
507.184848484848 0.016669844278446
545.51696969697 0.0152657537975013
583.849090909091 0.0140403420348959
622.181212121212 0.0129633147503883
660.513333333333 0.0120107250241012
698.845454545454 0.0111634074274614
737.177575757576 0.0104058522094566
775.509696969697 0.00972538193957077
813.841818181818 0.00911154005704565
852.173939393939 0.00855563045879386
890.506060606061 0.00805036643012686
928.838181818182 0.00758959986164248
967.170303030303 0.00716811018461701
1005.50242424242 0.00678143825649987
1043.83454545455 0.00642575445201471
1082.16666666667 0.00609775304768537
1120.49878787879 0.00579456700770791
1158.83090909091 0.00551369873762725
1197.16303030303 0.00525296343738564
1235.49515151515 0.00501044247138204
1273.82727272727 0.00478444475907143
1312.15939393939 0.0045734746303699
1350.49151515152 0.00437620492455909
1388.82363636364 0.00419145436721583
1427.15575757576 0.0040181684569062
1465.48787878788 0.00385540324650919
1503.82 0.00370231152374397
1542.15212121212 0.0035581309896647
1580.48424242424 0.00342217410845265
1618.81636363636 0.00329381936120919
1657.14848484848 0.00317250368399148
1695.48060606061 0.00305771590859552
1733.81272727273 0.00294899105554222
1772.14484848485 0.00284590535387844
1810.47696969697 0.00274807188294508
1848.80909090909 0.00265513674810783
1887.14121212121 0.00256677571631694
1925.47333333333 0.0024826912488297
1963.80545454545 0.00240260987794709
2002.13757575758 0.00232627988254352
2040.4696969697 0.00225346922379642
2078.80181818182 0.0021839637080805
2117.13393939394 0.00211756534866958
2155.46606060606 0.00205409090183766
2193.79818181818 0.00199337055629402
2232.1303030303 0.00193524675772654
2270.46242424242 0.00187957315264525
2308.79454545455 0.00182621363778243
2347.12666666667 0.00177504150307335
2385.45878787879 0.00172593865775849
2423.79090909091 0.00167879493045382
2462.12303030303 0.00163350743516096
2500.45515151515 0.00158997999616274
2538.78727272727 0.00154812262559225
2577.11939393939 0.00150785104819604
2615.45151515152 0.0014690862684486
2653.78363636364 0.00143175417573071
2692.11575757576 0.00139578518376931
2730.44787878788 0.00136111390096089
2768.78 0.00132767882857287
2807.11212121212 0.00129542208414423
2845.44424242424 0.00126428914769447
2883.77636363636 0.0012342286286035
2922.10848484848 0.00120519205124912
2960.44060606061 0.00117713365768683
2998.77272727273 0.00115001022583179
3037.10484848485 0.00112378090175885
3075.43696969697 0.0010984070448744
3113.76909090909 0.00107385208483706
3152.10121212121 0.00105008138921367
3190.43333333333 0.00102706214095502
3228.76545454545 0.00100476322486284
3267.09757575758 0.000983155122298061
3305.4296969697 0.000962209813450126
3343.76181818182 0.000941900686550061
3382.09393939394 0.00092220245346633
3420.42606060606 0.000903091071173305
3458.75818181818 0.000884543668627683
3497.0903030303 0.000866538478629445
3535.42242424242 0.000849054774280971
3573.75454545455 0.000832072809691459
3612.08666666667 0.000815573764604143
3650.41878787879 0.000799539692651157
3688.75090909091 0.000783953472965809
3727.08303030303 0.000768798764904497
3765.41515151515 0.000754059965651053
3803.74727272727 0.000739722170494791
3842.07939393939 0.000725771135590503
3880.41151515151 0.000712193243024061
3918.74363636364 0.000698975468021236
3957.07575757576 0.00068610534815025
3995.40787878788 0.000673570954380143
4033.74 0.000661360863867796
};
\addplot [very thick, yellowgreen18420623]
table {%
244.32 0.035630807450352
308.502222222222 0.0294413515643555
372.684444444444 0.0255628538649915
436.866666666667 0.0229113436549781
501.048888888889 0.0209879993258665
565.231111111111 0.0195318774769819
629.413333333333 0.0183933926981825
693.595555555556 0.0174806915583863
757.777777777778 0.0167342641773153
821.96 0.0161138609356391
886.142222222222 0.0155912815193929
950.324444444444 0.0151461771197999
1014.50666666667 0.0147634931804609
1078.68888888889 0.0144318506658943
1142.87111111111 0.0141424872361988
1207.05333333333 0.0138885447067617
1271.23555555556 0.0136645774837913
1335.41777777778 0.0134662059360778
1399.6 0.0132898671651464
1463.78222222222 0.013132632658814
1527.96444444444 0.0129920727727379
1592.14666666667 0.0128661545765765
1656.32888888889 0.0127531638519505
1720.51111111111 0.0126516448274273
1784.69333333333 0.0125603531125976
1848.87555555556 0.0124782185740557
1913.05777777778 0.0124043157839462
1977.24 0.0123378402962127
2041.42222222222 0.0122780894508404
2105.60444444444 0.0122244467276664
2169.78666666667 0.0121763689059111
2233.96888888889 0.0121333754587008
2298.15111111111 0.012095039740899
2362.33333333333 0.0120609816256721
2426.51555555556 0.0120308613189314
2490.69777777778 0.0120043741372154
2554.88 0.0119812460781124
2619.06222222222 0.011961230046142
2683.24444444444 0.0119441026234915
2747.42666666667 0.0119296612958529
2811.60888888889 0.0119177220601342
2875.79111111111 0.0119081173539959
2939.97333333333 0.0119006942577313
3004.15555555556 0.0118953129275284
3068.33777777778 0.0118918452260488
3132.52 0.0118901735218849
3196.70222222222 0.0118901896340463
3260.88444444444 0.0118917939014086
3325.06666666667 0.011894894360171
3389.24888888889 0.0118994060149513
3453.43111111111 0.0119052501912954
3517.61333333333 0.0119123539591687
3581.79555555556 0.0119206496185018
3645.97777777778 0.011930074239122
3710.16 0.0119405692484703
3774.34222222222 0.0119520800614034
3838.52444444444 0.0119645557471451
3902.70666666667 0.0119779487291034
3966.88888888889 0.0119922145138264
4031.07111111111 0.0120073114458439
4095.25333333333 0.012023200485553
4159.43555555556 0.0120398450076555
4223.61777777778 0.0120572106179605
4287.8 0.0120752649866259
4351.98222222222 0.0120939776961418
4416.16444444444 0.0121133201025555
4480.34666666667 0.01213326520861
4544.52888888889 0.0121537875476188
4608.71111111111 0.0121748630770307
4672.89333333333 0.0121964690807525
4737.07555555556 0.0122185840794001
4801.25777777778 0.0122411877477371
4865.44 0.0122642608386362
4929.62222222222 0.0122877851129707
4993.80444444444 0.0123117432749026
5057.98666666667 0.0123361189120887
5122.16888888889 0.0123608964403737
5186.35111111111 0.0123860610525818
5250.53333333333 0.0124115986710574
5314.71555555556 0.0124374959036372
5378.89777777778 0.0124637400027692
5443.08 0.0124903188275169
5507.26222222222 0.0125172208082169
5571.44444444444 0.0125444349135726
5635.62666666667 0.0125719506199937
5699.80888888889 0.0125997578830018
5763.99111111111 0.0126278471105435
5828.17333333333 0.0126562091380634
5892.35555555555 0.0126848352052027
5956.53777777778 0.0127137169340017
6020.72 0.0127428463084938
6084.90222222222 0.0127722156555891
6149.08444444444 0.0128018176271522
6213.26666666667 0.0128316451831899
6277.44888888889 0.0128616915760677
6341.63111111111 0.012891950335684
6405.81333333333 0.0129224152555333
6469.99555555556 0.0129530803795988
6534.17777777778 0.0129839399900155
6598.36 0.0130149885954526
};
\addplot [very thick, chocolate21910927]
table {%
21.9 1.0078570427758
98.3654545454546 0.2191050322673
174.830909090909 0.103686045815564
251.296363636364 0.0617251706835256
327.761818181818 0.0412646564516899
404.227272727273 0.0296207811034494
480.692727272727 0.0223193659311728
557.158181818182 0.0174232049026206
633.623636363636 0.0139736957749938
710.089090909091 0.0114492767714463
786.554545454546 0.00954521391587949
863.02 0.00807326725451775
939.485454545455 0.00691183157566669
1015.95090909091 0.00597939843250849
1092.41636363636 0.00521962002514998
1168.88181818182 0.00459250384210468
1245.34727272727 0.00406901417330281
1321.81272727273 0.00362764933933606
1398.27818181818 0.0032522074678756
1474.74363636364 0.00293029043161332
1551.20909090909 0.00265227924085705
1627.67454545455 0.00241061810260261
1704.14 0.0021993050831932
1780.60545454545 0.00201352383119329
1857.07090909091 0.00184937335174151
1933.53636363636 0.00170366705468494
2010.00181818182 0.00157378147649931
2086.46727272727 0.00145754110887291
2162.93272727273 0.00135312980232053
2239.39818181818 0.00125902195620536
2315.86363636364 0.00117392859876608
2392.32909090909 0.00109675478400001
2468.79454545455 0.00102656566940986
2545.26 0.000962559310194387
2621.72545454545 0.000904044692029398
2698.19090909091 0.000850423880746343
2774.65636363636 0.00080117743043952
2851.12181818182 0.000755852387835003
2927.58727272727 0.000714052378396769
3004.05272727273 0.000675429371582583
3080.51818181818 0.000639676808172313
3156.98363636364 0.000606523838382434
3233.44909090909 0.000575730470443258
3309.91454545455 0.000547083469046607
3386.38 0.000520392874236015
3462.84545454545 0.000495489035898439
3539.31090909091 0.000472220078521697
3615.77636363636 0.000450449726437509
3692.24181818182 0.000430055432238308
3768.70727272727 0.000410926761097904
3845.17272727273 0.000392963991851128
3921.63818181818 0.000376076902290521
3998.10363636364 0.000360183711527083
4074.56909090909 0.000345210156677772
4151.03454545454 0.000331088684775047
4227.5 0.000317757743793077
4303.96545454545 0.000305161159170793
4380.43090909091 0.000293247584278782
4456.89636363636 0.000281970015001416
4533.36181818182 0.000271285360048972
4609.82727272727 0.000261154059826313
4686.29272727273 0.000251539747705227
4762.75818181818 0.000242408948409414
4839.22363636364 0.000233730808951008
4915.68909090909 0.000225476858177422
4992.15454545454 0.000217620791515058
5068.62 0.000210138277946928
5145.08545454545 0.000203006786646667
5221.55090909091 0.000196205431022106
5298.01636363636 0.000189714828205715
5374.48181818182 0.000183516972274177
5450.94727272727 0.000177595119690793
5527.41272727273 0.000171933685647355
5603.87818181818 0.000166518150140791
5680.34363636364 0.000161334972757693
5756.80909090909 0.000156371515259816
5833.27454545455 0.000151615971168234
5909.74 0.000147057301635264
5986.20545454545 0.000142685176973253
6062.67090909091 0.000138489923279466
6139.13636363636 0.000134462473657898
6215.60181818182 0.000130594323593043
6292.06727272727 0.000126877490078347
6368.53272727273 0.000123304474144248
6444.99818181818 0.000119868226467895
6521.46363636364 0.00011656211577962
6597.92909090909 0.000113379899810427
6674.39454545455 0.000110315698550695
6750.86 0.000107363969613341
6827.32545454545 0.000104519485515184
6903.79090909091 0.000101777312708554
6980.25636363636 9.91327922114865e-05
7056.72181818182 9.65815216994116e-05
7133.18727272727 9.41193389343082e-05
7209.65272727273 9.17423064189557e-05
7286.11818181818 8.94466971743869e-05
7362.58363636364 8.72289815480577e-05
7439.04909090909 8.50858149686914e-05
7515.51454545455 8.30140265713605e-05
7591.98 8.10106086232193e-05
};
\addplot [very thick, indianred19152101]
table {%
21.9 0.697249134110895
89.3119191919192 0.558771852563526
156.723838383838 0.438663151977154
224.135757575758 0.359288923028068
291.547676767677 0.303321184043088
358.959595959596 0.261715903067723
426.371515151515 0.229550676511369
493.783434343434 0.203932280241939
561.195353535354 0.183047327591418
628.607272727273 0.165699487502708
696.019191919192 0.151066319912956
763.431111111111 0.138563056662377
830.84303030303 0.127762113462392
898.25494949495 0.1183433649872
965.666868686869 0.110062247764314
1033.07878787879 0.102728631411424
1100.49070707071 0.0961924296417323
1167.90262626263 0.0903335616813401
1235.31454545455 0.0850547985616458
1302.72646464646 0.0802765684834894
1370.13838383838 0.0759331209535986
1437.5503030303 0.0719696513058228
1504.96222222222 0.0683401156560565
1572.37414141414 0.0650055499045469
1639.78606060606 0.0619327618895816
1707.19797979798 0.0590933033327964
1774.6098989899 0.0564626540398092
1842.02181818182 0.0540195688620435
1909.43373737374 0.0517455507114383
1976.84565656566 0.0496244221000263
2044.25757575758 0.0476419743481763
2111.6694949495 0.0457856785088794
2179.08141414141 0.0440444456973288
2246.49333333333 0.0424084272463756
2313.90525252525 0.0408688471756461
2381.31717171717 0.0394178610401132
2448.72909090909 0.0380484364381969
2516.14101010101 0.0367542514009485
2583.55292929293 0.0355296076190625
2650.96484848485 0.0343693560424299
2718.37676767677 0.0332688328442185
2785.78868686869 0.0322238041054382
2853.20060606061 0.0312304178673089
2920.61252525253 0.0302851624332679
2988.02444444444 0.0293848299921829
3055.43636363636 0.0285264847885997
3122.84828282828 0.027707435191869
3190.2602020202 0.0269252091193895
3257.67212121212 0.0261775323544153
3325.08404040404 0.0254623093693766
3392.49595959596 0.0247776063242331
3459.90787878788 0.02412163595821
3527.3197979798 0.0234927441341412
3594.73171717172 0.022889397828956
3662.14363636364 0.0223101743927661
3729.55555555556 0.021753751923449
3796.96747474748 0.0212189006243442
3864.37939393939 0.0207044750303067
3931.79131313131 0.0202094070023835
3999.20323232323 0.019732699404239
4066.61515151515 0.0192734203844684
4134.02707070707 0.0188306981984193
4201.43898989899 0.0184037165113004
4268.85090909091 0.0179917101314147
4336.26282828283 0.017593961128459
4403.67474747475 0.0172097952971348
4471.08666666667 0.0168385789309243
4538.49858585859 0.0164797158749047
4605.9105050505 0.0161326448299829
4673.32242424242 0.0157968368840042
4740.73434343434 0.0154717932478821
4808.14626262626 0.0151570431772616
4875.55818181818 0.0148521420623099
4942.9701010101 0.0145566696700649
5010.38202020202 0.0142702285253929
5077.79393939394 0.0139924424180382
5145.20585858586 0.0137229550245234
5212.61777777778 0.0134614286347806
5280.0296969697 0.0132075429743993
5347.44161616162 0.01296099411427
5414.85353535354 0.0127214934601939
5482.26545454545 0.0124887668157433
5549.67737373737 0.0122625535122886
5617.08929292929 0.0120426056006789
5684.50121212121 0.0118286870995706
5751.91313131313 0.0116205732958554
5819.32505050505 0.0114180500930525
5886.73696969697 0.0112209134038957
5954.14888888889 0.0110289685836821
6021.56080808081 0.0108420299012487
6088.97272727273 0.0106599200447124
6156.38464646465 0.010482469659358
6223.79656565657 0.0103095169152764
6291.20848484848 0.0101409071025596
6358.6204040404 0.00997649225203871
6426.03232323232 0.0098161307797189
6493.44424242424 0.00965968715321413
6560.85616161616 0.00950703157862156
6628.26808080808 0.00935803970640039
6695.68 0.00921259235493324
};
\addplot [very thick, purple11522131]
table {%
78.58 0.326366197778146
136.019797979798 0.114904585930215
193.459595959596 0.0591928259361639
250.899393939394 0.0364060990579827
308.339191919192 0.0248142212219854
365.77898989899 0.0180866836016719
423.218787878788 0.013820663503719
480.658585858586 0.010937541390112
538.098383838384 0.00889305587153157
595.538181818182 0.00738774147931236
652.97797979798 0.0062454354965921
710.417777777778 0.0053568423572965
767.857575757576 0.00465114148972796
825.297373737374 0.00408075383888628
882.737171717172 0.00361272262496554
940.17696969697 0.00322361392283262
997.616767676768 0.00289638266952223
1055.05656565657 0.00261838226659018
1112.49636363636 0.0023800637364572
1169.93616161616 0.0021741038286741
1227.37595959596 0.00199480740712344
1284.81575757576 0.00183768956365928
1342.25555555556 0.00169917810852568
1399.69535353535 0.00157639829311947
1457.13515151515 0.00146701472036622
1514.57494949495 0.00136911367741607
1572.01474747475 0.00128111446795355
1629.45454545455 0.00120170183479506
1686.89434343434 0.00112977391434277
1744.33414141414 0.00106440176281152
1801.77393939394 0.0010047975969685
1859.21373737374 0.000950289663494821
1916.65353535354 0.000900302197488431
1974.09333333333 0.000854339322275723
2031.53313131313 0.000811972026526085
2088.97292929293 0.000772827562481692
2146.41272727273 0.000736580762756145
2203.85252525253 0.000702946887778833
2261.29232323232 0.000671675702209853
2318.73212121212 0.000642546544072073
2376.17191919192 0.000615364200350834
2433.61171717172 0.000589955441307265
2491.05151515152 0.000566166095590236
2548.49131313131 0.000543858571511084
2605.93111111111 0.000522909748119033
2663.37090909091 0.00050320917414397
2720.81070707071 0.000484657524329757
2778.25050505051 0.000467165271826443
2835.6903030303 0.000450651542646948
2893.1301010101 0.000435043124109204
2950.5698989899 0.000420273603976131
3008.0096969697 0.000406282620903847
3065.44949494949 0.000393015209993712
3122.88929292929 0.000380421229856704
3180.32909090909 0.000368454859750987
3237.76888888889 0.000357074157132807
3295.20868686869 0.000346240667437425
3352.64848484848 0.000335919079136169
3410.08828282828 0.000326076918142894
3467.52808080808 0.000316684276504141
3524.96787878788 0.000307713571031175
3582.40767676768 0.000299139328142719
3639.84747474747 0.000290937991703576
3697.28727272727 0.000283087751082422
3754.72707070707 0.000275568387024628
3812.16686868687 0.000268361133253742
3869.60666666667 0.000261448551986861
3927.04646464646 0.000254814421782037
3984.48626262626 0.000248443636335862
4041.92606060606 0.000242322113021638
4099.36585858586 0.000236436710107235
4156.80565656566 0.000230775151720356
4214.24545454545 0.000225325959740368
4271.68525252525 0.000220078391892723
4329.12505050505 0.000215022385406243
4386.56484848485 0.000210148505667059
4444.00464646465 0.000205447899367154
4501.44444444444 0.000200912251701726
4558.88424242424 0.000196533747218818
4616.32404040404 0.000192305033967953
4673.76383838384 0.000188219190632639
4731.20363636364 0.000184269696365136
4788.64343434343 0.000180450403071528
4846.08323232323 0.000176755509921354
4903.52303030303 0.000173179539879235
4960.96282828283 0.000169717318076524
5018.40262626263 0.000166363951859274
5075.84242424242 0.000163114812365074
5133.28222222222 0.000159965517495777
5190.72202020202 0.000156911916166062
5248.16181818182 0.000153950073719282
5305.60161616162 0.000151076258412391
5363.04141414141 0.000148286928880929
5420.48121212121 0.000145578722503368
5477.92101010101 0.000142948444591506
5535.36080808081 0.000140393058340296
5592.80060606061 0.000137909675476477
5650.2404040404 0.000135495547550813
5707.6802020202 0.000133148057823578
5765.12 0.000130864713697377
};
\addplot [very thick, plum223165229]
table {%
296.9 0.0328259389614535
352.154141414141 0.0236212288028073
407.408282828283 0.0178960696414048
462.662424242424 0.0140829815795394
517.916565656566 0.0114094494553119
573.170707070707 0.00945837899756401
628.424848484849 0.0079881891380589
683.67898989899 0.00685092543176566
738.933131313131 0.00595176124425122
794.187272727273 0.0052275826970051
849.441414141414 0.00463502325887067
904.695555555556 0.00414346188045826
959.949696969697 0.00373076114921271
1015.20383838384 0.00338058365176078
1070.45797979798 0.0030806513815155
1125.71212121212 0.00282158704593866
1180.96626262626 0.00259612474367692
1236.2204040404 0.00239856107934645
1291.47454545455 0.00222436635196389
1346.72868686869 0.00206990449519622
1401.98282828283 0.00193222826925696
1457.23696969697 0.00180892739918844
1512.49111111111 0.00169801453736371
1567.74525252525 0.00159783862709234
1622.99939393939 0.00150701837323743
1678.25353535354 0.00142439064356379
1733.50767676768 0.00134897007965259
1788.76181818182 0.00127991721001969
1844.01595959596 0.00121651307359165
1899.2701010101 0.00115813887279979
1954.52424242424 0.00110425954476429
2009.77838383838 0.00105441040856626
2065.03252525253 0.00100818624530607
2120.28666666667 0.00096523231549298
2175.54080808081 0.000925236929280804
2230.79494949495 0.000887925269040491
2286.04909090909 0.000853054227804858
2341.30323232323 0.000820408076321901
2396.55737373737 0.000789794809515841
2451.81151515152 0.000761043052794724
2507.06565656566 0.000733999431869509
2562.3197979798 0.000708526328058016
2617.57393939394 0.000684499955561732
2672.82808080808 0.000661808708772348
2728.08222222222 0.000640351736933978
2783.33636363636 0.000620037710949832
2838.59050505051 0.000600783753159474
2893.84464646465 0.000582514505818648
2949.09878787879 0.000565161318017849
3004.35292929293 0.000548661534057215
3059.60707070707 0.000532957868995414
3114.86121212121 0.000517997859320569
3170.11535353535 0.000503733378540041
3225.3694949495 0.000490120209024283
3280.62363636364 0.000477117662724103
3335.87777777778 0.000464688244456341
3391.13191919192 0.000452797352356692
3446.38606060606 0.000441413010860099
3501.6402020202 0.000430505632213084
3556.89434343434 0.000420047803068173
3612.14848484849 0.000410014093174573
3667.40262626263 0.00040038088357481
3722.65676767677 0.000391126212054883
3777.91090909091 0.000382229633885223
3833.16505050505 0.000373672096138154
3888.41919191919 0.00036543582408184
3943.67333333333 0.00035750421833513
3998.92747474748 0.000349861761627589
4054.18161616162 0.000342493934147223
4109.43575757576 0.000335387136578623
4164.6898989899 0.000328528620038776
4219.94404040404 0.000321906422208924
4275.19818181818 0.00031550930904047
4330.45232323232 0.000309326721482577
4385.70646464647 0.000303348726740226
4440.96060606061 0.000297565973625077
4496.21474747475 0.000291969651608722
4551.46888888889 0.000286551453229476
4606.72303030303 0.000281303539540558
4661.97717171717 0.000276218508320009
4717.23131313131 0.000271289364791299
4772.48545454545 0.000266509494629267
4827.7395959596 0.000261872639048441
4882.99373737374 0.00025737287179105
4938.24787878788 0.000253004577849945
4993.50202020202 0.000248762433777556
5048.75616161616 0.000244641389446398
5104.0103030303 0.000240636651139293
5159.26444444444 0.000236743665858988
5214.51858585859 0.000232958106757041
5269.77272727273 0.000229275859591066
5325.02686868687 0.00022569301012769
5380.28101010101 0.000222205832415986
5435.53515151515 0.000218810777862887
5490.78929292929 0.000215504465048072
5546.04343434343 0.000212283670221299
5601.29757575758 0.000209145318430079
5656.55171717172 0.00020608647523003
5711.80585858586 0.000203104338934294
5767.06 0.000200196233362059
};
\addplot [draw=black, fill=black, mark=x, very thick, mark size=2.5pt, only marks]
table{%
x  y
87.6 0.272343533408822
351.36 0.0259470568426133
1450.24 0.00189066552594397
5765.12 0.000144604747120979
};
