# Supplementary material for: Swarm Reinforcement Learning For Adaptive Mesh Refinement
Source: arXiv:2304.00818 source file (2023-10-09)
Supplement: Supplementary file 18 [file group_baselines_2.tex]

\nextgroupplot[
ylabel shift = -0.2cm,
clip marker paths=true,
width=0.52\textwidth,
height=4.5cm,
title style={yshift=-0.2cm},
scaled x ticks=false,
legend cell align={left},
legend style={fill opacity=0.8, draw opacity=1, text opacity=1, draw=lightgray204},
log basis y={10},
tick align=outside,
tick pos=left,
title={Poisson - MPN and GAT},
x grid style={darkgray176},
xlabel={Elements \(\displaystyle (\times 10^3)\)},
xmajorgrids,
xmin=-379.071, xmax=8427.331,
xtick style={color=black},
xtick={-1000,0,1000,2000,3000,4000,5000,6000,7000,8000,9000},
xticklabels={-1.0,0.0,1.0,2.0,3.0,4.0,5.0,6.0,7.0,8.0,9.0},
y grid style={darkgray176},
ylabel={\empty},
ymajorgrids,
ymin=3.20971195110356e-06, ymax=2.0984975199912,
ymode=log,
ytick style={color=black},
ytick={1e-07,1e-06,1e-05,0.0001,0.001,0.01,0.1,1,10,100},
yticklabels={
  \empty
  % \(\displaystyle {10^{-7}}\),
  % \(\displaystyle {10^{-6}}\),
  % \(\displaystyle {10^{-5}}\),
  % \(\displaystyle {10^{-4}}\),
  % \(\displaystyle {10^{-3}}\),
  % \(\displaystyle {10^{-2}}\),
  % \(\displaystyle {10^{-1}}\),
  % \(\displaystyle {10^{0}}\),
  % \(\displaystyle {10^{1}}\),
  % \(\displaystyle {10^{2}}\)
}
]
\addplot [draw=black18, fill=black18, forget plot, mark=*, mark size=1, only marks, draw opacity=0,
 fill opacity=0.5]
table{%
x  y
252.04 0.00910196105003992
273.28 0.00656161386290537
277.44 0.00685819598447156
280.6 0.00773051123156303
282.14 0.00677802160319427
295.64 0.00677772626953998
298.14 0.0069369837008831
305.18 0.00573005623074585
313.08 0.00595485940219031
355.76 0.00542021034747742
375.66 0.00432372328766738
382.88 0.00378469930986426
402.96 0.00365498460727189
427.18 0.00299894405523269
430.78 0.00334804343149355
443.56 0.00261308599626255
448.76 0.00255512591513487
458.12 0.00211928676948892
475.54 0.00232857265058521
501.28 0.00202170217916782
531.36 0.0017116840552977
535.7 0.00164036325111721
549.2 0.00165989975981073
557.18 0.00166766953581634
564.7 0.00145346474536877
576.1 0.00152294321015519
579.5 0.00187585829182461
611.24 0.00143096846603181
647.72 0.00123711708707717
679.62 0.00129048530384763
694.1 0.00108648705609372
716.6 0.00129442421237454
720.62 0.000869049520849834
732.08 0.00112160777906218
737.44 0.000941213074178068
775.34 0.000839090790670215
787.48 0.000836134920530711
802.9 0.000852780259947504
886.62 0.000592540044742646
928.56 0.000481666299898572
974.24 0.000633482868509968
1049 0.000603170351023298
1064.9 0.000508433367874507
1090.36 0.00048758591274521
1134.44 0.000438550228139679
1143.3 0.000394661607022297
1183.56 0.000435044366848108
1206.56 0.000338651347310387
1238.16 0.000355361702292142
1255.7 0.00036395139079347
1280.56 0.000368882599500474
1295.98 0.000301009929862845
1299.7 0.000398298083523274
1321.14 0.000258383709023031
1348.16 0.000263829815860464
1431 0.000250133324082547
1462.46 0.000235860368451126
1470.28 0.000307810411743672
1508.16 0.000198579319777823
1551.78 0.000220138672037778
1634.64 0.000216867940883727
1694.28 0.000161562752095687
1731.66 0.000154872724199736
1875.8 0.000143304754344995
1888.1 0.000136954317317247
1939.54 0.000138943274931016
1959.34 0.000114835079199504
2035.56 0.000109739140249297
2306.72 0.000101212301194016
2320.12 8.20085304179235e-05
2330.04 8.632486708504e-05
2427.78 9.66884442316103e-05
2437.1 0.00010546659620646
2521.56 8.75315976106771e-05
2535.82 7.72965691141353e-05
2668.24 6.96587819880897e-05
2672.24 6.54929742313365e-05
2702.16 8.32565656675997e-05
2723.72 6.81000267967975e-05
2816.66 6.16540165580413e-05
2886 6.91114983588215e-05
2910.72 4.82339582074195e-05
2925.06 6.35743981499529e-05
2939.2 4.88579025275278e-05
2980.64 5.25976602679367e-05
3057.68 4.71887605320183e-05
3333.54 4.38258985260279e-05
3536.8 4.0436114880334e-05
3981.24 3.01363859546903e-05
4279.76 2.60878652639343e-05
4495.2 2.48310959741839e-05
4555.3 2.51809674235956e-05
4973.3 2.16693417262563e-05
5033.82 2.13571006835526e-05
5560.66 1.51364535850379e-05
6171.32 1.10038628286692e-05
6378.4 1.15228481929327e-05
6422.4 1.25383138781389e-05
6558.44 1.07004519382148e-05
6871.74 1.1017486097863e-05
};
\addplot [
  draw=royalblue28108204,
  fill=royalblue28108204,
  forget plot,
  mark=*, mark size=1,
  only marks,
  draw opacity=0,
 fill opacity=0.5
]
table{%
x  y
219.22 0.0116380025783674
236.58 0.00893751131252496
255.06 0.00757221773421185
266.3 0.00695152587324572
277.02 0.00870449843080493
289.06 0.00650849332548639
301.82 0.00650772537377039
309.02 0.00632830538267971
313.48 0.00852456067483164
317.48 0.00503420224308783
366.78 0.00472734343816265
384.24 0.00384945126787151
427.52 0.00440570193112838
431.14 0.00387196288409598
433.8 0.0031068838328975
438.92 0.0033561305566538
446.06 0.00325148782214415
485 0.00270934352590588
524.5 0.0019590317268996
530.98 0.0024847849713976
530.98 0.0024462804500235
542.2 0.00339373662958677
568.26 0.00191195330793864
569.1 0.00200759214947172
579.8 0.00192121084682089
587.66 0.00166535004820132
612.06 0.00170099739413765
628 0.00142557999535175
636.98 0.00193167521782833
648.04 0.00147630841918046
648.78 0.00196488850395651
684.76 0.00192456325257735
704.12 0.00152017798836435
708.02 0.00171515266408961
724.56 0.00106290863523144
740.7 0.00145038634314574
740.82 0.00126611233262213
754.68 0.0010958404611985
776.14 0.00136681288549904
861 0.00122261947029662
866.82 0.0012376456173406
951.18 0.000684639740045543
978.82 0.000682995459645206
1030.58 0.000639142132617508
1031.2 0.000608987227553708
1080.16 0.000534351174466062
1116.56 0.000522936657826564
1126.22 0.00047220578013082
1173.32 0.000587407673606018
1183.24 0.000496992672901857
1212.6 0.000433759599768057
1270.84 0.000477030829124065
1271.28 0.00057574970357699
1312.64 0.000295338105933881
1334.88 0.0003688460635094
1390.92 0.000632823129081481
1414.42 0.000439822660083419
1465.2 0.000380405825070989
1546.18 0.000259777992401812
1645.64 0.000189432782231567
1650.1 0.00040730379394757
1712.26 0.000225696747843442
1799.62 0.000205137266591349
1800.64 0.000149688394684308
1820.82 0.00022968203197516
1908.42 0.000134858938308452
1925.1 0.000231468966668099
2020.12 0.000123482420852495
2156.38 0.000114435638078513
2168.78 0.000132258579214635
2169 0.000101440195225082
2212 0.000202015930911123
2238.3 0.000100444720362762
2307.32 0.00010430451268494
2321.26 0.000101348576943888
2363.12 7.85396281013735e-05
2399.82 8.97496755911525e-05
2432.68 0.000175103698214891
2457.16 9.48685731254995e-05
2655.7 7.07642905549767e-05
2715.22 5.85765922707877e-05
3044.4 5.85685554721719e-05
3414.76 4.01750628140733e-05
3545.46 3.80019302781983e-05
3591.66 3.62548169075136e-05
3997.22 3.19018762058348e-05
4033.6 2.70246768067793e-05
4075.94 2.55319826966762e-05
4148.74 2.90210310242148e-05
4304.56 2.36833753484687e-05
4311.96 4.28165553247746e-05
4611.22 2.13677683411378e-05
5764.26 1.3085878413959e-05
6013.74 1.0832458588431e-05
6168.52 9.73742044189171e-06
6591.82 8.02970379055727e-06
6800.42 8.43665609892419e-06
6819.78 8.29434337198603e-06
7381.26 8.13257734004449e-06
7648.78 6.34432528857979e-06
};
\addplot [
  draw=chocolate21910927,
  fill=chocolate21910927,
  forget plot,
  mark=*, mark size=1,
  only marks,
  draw opacity=0,
 fill opacity=0.5
]
table{%
x  y
21.9 0.999999998927878
21.9 0.999999998927878
21.92 0.999999998950274
21.92 0.999999998950274
21.92 0.999999998950274
21.92 0.999999998950274
21.92 0.999999998950274
21.92 0.999999998950274
21.92 0.999999998950274
21.92 0.999999998950274
21.92 0.999999998950274
21.92 0.999999998950274
21.92 0.999999998950274
21.92 0.999999998950274
21.92 0.999999998950274
21.92 0.999999998950274
21.92 0.999999998950274
21.92 0.999999998950274
21.92 0.999999998950274
21.92 0.999999998950274
21.92 0.999999998950274
21.92 0.999999998950274
21.92 0.999999998950274
21.92 0.999999998950274
21.92 0.999999998950274
21.92 0.999999998950274
21.92 0.999999998950274
21.92 0.999999998950274
21.92 0.999999998950274
21.92 0.999999998950274
21.92 0.999999998950274
21.92 0.999999998950274
21.94 0.999999998905941
21.94 0.999999998905941
21.94 0.999999998905941
21.94 0.999999998905941
22 0.999999998889839
22.02 0.999999998899304
22.16 0.999999998640609
22.28 0.999999998477158
26.5 0.970894204249672
32.62 0.924277946638112
34.96 0.862638850036096
91.4 0.720312311243077
94.9 0.18919499810567
108.74 0.71958749216895
134.98 0.0689210131272957
136.1 0.0613824673087774
155.44 0.0559306313583098
208.3 0.197146125458646
249.98 0.0499246702086478
271.24 0.0325903579711196
274.72 0.0511839347070228
283.88 0.043017706650582
308.14 0.288765844789137
329.14 0.0162289718257283
338.64 0.034337015545152
357.98 0.0101646670694072
386.82 0.0167657064564419
395.32 0.0042305451504377
403.3 0.0119398370592536
430.36 0.0289122109821289
531.96 0.11696073594285
595.12 0.58453985126498
642.3 0.00386796707321375
670.92 0.00302893160661771
695.68 0.00347257940790675
722.02 0.0391289662856242
762.26 0.00451677919851355
1152.26 0.0261976517911636
1233.2 0.000998733802377771
1272.96 0.000876420935487872
1282.64 0.00102417788068937
1315.36 0.000594576789097483
1410.32 0.00146055096768862
1658.3 0.0267799322922428
1817.54 0.222864808756589
1978.66 0.000274269869038731
2059.9 0.00791404372976221
2070.98 0.000261190457505995
2305.2 0.225290493210452
3213.16 0.000133900698026789
3434.82 0.000663721741809451
4206.7 0.000806185856602349
4447.52 0.000113588426911867
4668.8 0.000258317240468995
5045.36 4.79021802088747e-05
7591.98 3.04719971098142e-05
};
\addplot [
  draw=indianred19152101,
  fill=indianred19152101,
  forget plot,
  mark=*, mark size=1,
  only marks,
  draw opacity=0,
 fill opacity=0.5
]
table{%
x  y
21.9 0.999999998927878
21.92 0.999999998950274
21.92 0.999999998950274
21.92 0.999999998950274
21.92 0.999999998950274
21.92 0.999999998950274
21.92 0.999999998950274
21.92 0.999999998950274
21.92 0.999999998950274
21.92 0.999999998950274
21.92 0.999999998950274
21.92 0.999999998950274
21.92 0.999999998950274
21.92 0.999999998950274
21.92 0.999999998950274
21.92 0.999999998950274
21.94 0.999999998905941
22.38 0.999999998494591
86.16 0.352216255032009
86.7 0.328547431631386
87.62 0.333654605600169
87.82 0.327681198323879
88.02 0.278882512794496
88.48 0.331261231703773
98.84 0.335670490636036
106.34 0.241557736491125
140.92 0.148468863169787
156.9 0.170137577476667
289.68 0.105000482512224
304.32 0.12291727942287
310.04 0.0607944562954501
328.7 0.0759163945619775
337.14 0.0512447073997889
339.8 0.040078161734014
342.54 0.0337325032274052
344 0.0365478747195187
348.34 0.028434513304812
351.52 0.0356325093723456
353.08 0.030532771021612
541.1 0.842374535290012
604 0.847835186553072
1066.6 0.719452089607114
1161.2 0.71149606072708
1241.9 0.628152527619007
1300.1 0.622316725184108
1371.64 0.00698772015796695
1382.84 0.00744094377942691
1394.46 0.00577677810582207
1413.48 0.00453148829487134
1416.12 0.0049413720239298
1464.54 0.62118803329771
1531.92 0.0148022976249967
1540.94 0.563534779091307
1543.56 0.54399752624644
1661.74 0.571031223733867
1692.52 0.456822063532561
1753.86 0.511927198179604
1815.12 0.510281719283338
1826.28 0.532736890524313
1836.16 0.0139742540562555
1972.88 0.488244891128931
2005.12 0.0852287293132581
2010.78 0.474055521200355
2018.06 0.497930576781945
2068.12 0.403685355389766
2085.48 0.451446348939405
2113.92 0.414092602236795
2190 0.084093059681537
2235.3 0.381732205329873
2418.2 0.413228171556552
2420.1 0.41892685011743
2426.32 0.0588653508481712
2454.64 0.0558491051519919
2475.16 0.383542144648091
2499.44 0.0113230297192077
2529.36 0.0516671835662763
2532.8 0.0526988047949506
2827.84 0.00901071062612392
2836.6 0.0657179888381315
2841.06 0.313361505311296
3010.8 0.0526385785718605
3096.32 0.00727159705070947
3099.4 0.0474182263176894
3260.16 0.00737793041954566
3443.18 0.227858206416832
3484.24 0.131416343069701
3508.8 0.00650174839867577
3511.04 0.00727476484986376
4037.28 0.00626809931282519
4569.52 0.00220340056657374
4866.56 0.00095351629334446
4887.2 0.00682488843617527
5201.6 0.000876717946282604
6030.08 0.000706079536671927
6155.52 0.000759127934097835
6275.84 0.000695731218746723
6695.68 0.000681034516802472
};
\addplot [
  draw=saddlebrown1356716,
  fill=saddlebrown1356716,
  forget plot,
  mark=*, mark size=1,
  only marks,
  draw opacity=0,
 fill opacity=0.5
]
table{%
x  y
21.22 0.999999998638705
21.32 0.9999999987968
21.44 0.999999998638142
21.54 0.999999998519937
21.54 0.999999998576536
21.7 0.999999998725199
21.82 0.999999998815059
21.9 0.999999998927878
21.92 0.999999998950274
21.92 0.999999998950274
21.92 0.999999998950274
21.92 0.999999998950274
21.92 0.999999998950274
21.92 0.999999998950274
21.92 0.999999998950274
21.92 0.999999998950274
21.92 0.999999998950274
21.92 0.999999998950274
21.92 0.999999998950274
21.92 0.999999998950274
21.92 0.999999998950274
21.92 0.999999998950274
21.92 0.999999998950274
21.92 0.999999998950274
21.92 0.999999998950274
21.92 0.999999998950274
21.92 0.999999998950274
21.92 0.999999998950274
21.92 0.999999998950274
21.92 0.999999998950274
21.92 0.999999998950274
21.92 0.999999998950274
21.92 0.999999998950274
21.92 0.999999998950274
21.92 0.999999998950274
21.92 0.999999998950274
21.92 0.999999998950274
21.92 0.999999998950274
21.92 0.999999998950274
21.92 0.999999998950274
21.92 0.999999998950274
21.92 0.999999998950274
21.92 0.999999998950274
21.92 0.999999998950274
21.92 0.999999998950274
21.92 0.999999998950274
21.92 0.999999998950274
21.92 0.999999998950274
21.92 0.999999998950274
21.92 0.999999998950274
21.92 0.999999998950274
21.92 0.999999998950274
21.92 0.999999998950274
21.92 0.999999998950274
21.94 0.999999998905941
21.94 0.999999998905941
21.94 0.999999998905941
21.94 0.999999998905941
21.94 0.999999998839691
22.22 0.999999998879079
22.22 0.999999998879079
22.8 0.99214160459336
27 0.948576937353043
30.58 0.910277260690132
37.36 0.922208239117144
42.6 0.958848675322946
43.78 0.891483120089124
84.94 0.304540870621995
86.68 0.699310750664895
87.6 0.272343533408822
88.12 0.326641083846708
90.66 0.271352983663013
95.82 0.24118720044671
114.72 0.182932855414954
115.18 0.134105106512937
137.04 0.123167606710403
175.28 0.0883336080092325
176 0.116128704248637
215.56 0.0559673373889906
268 0.052311975185703
296.32 0.0466862625810785
349.52 0.023414422687462
353.7 0.0156481297589054
357.18 0.034538998443672
386.16 0.0183617538955718
394.98 0.0157024568177718
452.88 0.00836381933141826
525.56 0.00941112603941016
623.26 0.0177509349262807
825.9 0.0031883742042153
1048.32 0.022811899540685
1316.24 0.00110705567320756
3732.02 0.0016193745502732
4824.58 0.402800073995199
};
\addplot [draw=gray127, fill=gray127, forget plot, mark=*, mark size=1, only marks, draw opacity=0,
 fill opacity=0.5]
table{%
x  y
21.92 0.999999998950274
21.92 0.999999998950274
21.92 0.999999998950274
21.92 0.999999998950274
21.92 0.999999998950274
21.92 0.999999998950274
21.92 0.999999998950274
21.92 0.999999998950274
21.92 0.999999998950274
21.92 0.999999998950274
21.92 0.999999998950274
21.92 0.999999998950274
21.92 0.999999998950274
21.94 0.999999998905941
21.98 0.9999999984671
25.86 0.958017636801588
27.6 0.973265145333709
30.86 0.971868025922772
63.78 0.945304973896075
68.6 0.654562478295675
69.6 0.468621121810736
74.26 0.579984484186438
79.66 0.464906346274448
79.92 0.492481415964878
81.02 0.448239371240755
81.36 0.445422614813312
83.86 0.402516608079812
85.06 0.388333222498122
85.18 0.394102082310633
87.3 0.335161675387104
88.04 0.694605632740939
96.98 0.452542295782466
102.02 0.45000029674486
128.82 0.449093228399761
257.48 0.328453916298973
266.86 0.132000896082082
310.18 0.165677884465963
338.68 0.0966931623457143
425.66 0.809543235906963
660.04 0.813419470257131
701.38 0.00348158749741144
965.94 0.484516214839435
1034.86 0.733473763102572
1236.3 0.291571824409724
1320.92 0.268775614048381
1351.78 0.517647561581119
1361.42 0.00523719019070079
1463.12 0.146432372714328
1604.08 0.183814178977991
1605.1 0.604135856733488
1647.28 0.260230390407011
1675.84 0.124803881868056
1688.48 0.127991737731854
1692.8 0.0895991286546235
1706.84 0.541163532431216
1739.2 0.132306430978429
1770.84 0.198728207112211
1790.88 0.620306489545248
1861.52 0.116377396536795
1998.5 0.596716573241798
2098.72 0.120347149521646
2134.72 0.0118598271336505
2166.56 0.3034977498602
2218.84 0.263987835762511
2265.64 0.520393432739672
2316.68 0.464494227236885
2561.82 0.415453263399015
2608.72 0.10861023195418
2864.02 0.487187693118623
3169.28 0.254480387911335
3307.08 0.0302023932481449
3678.36 0.402945948279588
3885.92 0.00375465158523396
3898 0.00118779353178663
4031.36 0.00104958722645467
4432.88 0.00137827785916709
4693.86 0.174739174816624
5123.76 0.0298486959641629
5336.92 0.000543789749780029
5379.98 0.000466310134228927
5495.68 0.000467688233594919
5739.96 0.000541870799302601
6662.42 0.000112745564835767
6948.96 0.001202367948894
7663.3 0.0125279911732456
};
\addplot [very thick, black18]
table {%
252.04 0.00884668258903063
318.905656565657 0.00547110320553025
385.771313131313 0.00370842303327339
452.63696969697 0.00267503451224727
519.502626262626 0.002018472972376
586.368282828283 0.00157588305539618
653.233939393939 0.00126365708273425
720.099595959596 0.00103531927163257
786.965252525252 0.000863374401412206
853.830909090909 0.000730719311971115
920.696565656566 0.000626266405574419
987.562222222222 0.000542574553399
1054.42787878788 0.000474500531673836
1121.29353535354 0.00041839803222704
1188.15919191919 0.00037162424486734
1255.02484848485 0.000332226142861872
1321.8905050505 0.000298735421994908
1388.75616161616 0.000270031141407527
1455.62181818182 0.00024524568838135
1522.48747474747 0.000223699133938246
1589.35313131313 0.00020485259459006
1656.21878787879 0.000188274565188921
1723.08444444444 0.000173616260269577
1789.9501010101 0.00016059331235421
1856.81575757576 0.000148972022074672
1923.68141414141 0.000138558911568659
1990.54707070707 0.000129192704911438
2057.41272727273 0.000120738112303706
2124.27838383838 0.000113080969110881
2191.14404040404 0.000106124402675499
2258.0096969697 9.97857860060751e-05
2324.87535353535 9.39942991246825e-05
2391.74101010101 8.86889634804249e-05
2458.60666666667 8.38170474523061e-05
2525.47232323232 7.93327650331635e-05
2592.33797979798 7.51962077067966e-05
2659.20363636364 7.13724629869488e-05
2726.06929292929 6.78308832723516e-05
2792.93494949495 6.45444764401773e-05
2859.80060606061 6.14893955672312e-05
2926.66626262626 5.86445097828537e-05
2993.53191919192 5.59910418493624e-05
3060.39757575758 5.35122608787752e-05
3127.26323232323 5.11932208103691e-05
3194.12888888889 4.90205370287743e-05
3260.99454545455 4.69821948999806e-05
3327.8602020202 4.50673851212779e-05
3394.72585858586 4.32663616808388e-05
3461.59151515152 4.15703189495796e-05
3528.45717171717 3.99712850179223e-05
3595.32282828283 3.84620288709365e-05
3662.18848484848 3.70359793888872e-05
3729.05414141414 3.56871544835561e-05
3795.9197979798 3.4410098947373e-05
3862.78545454545 3.31998298131331e-05
3929.65111111111 3.205178820542e-05
3996.51676767677 3.09617968176761e-05
4063.38242424242 2.99260222766299e-05
4130.24808080808 2.89409417629735e-05
4197.11373737374 2.8003313347351e-05
4263.97939393939 2.71101495768126e-05
4330.84505050505 2.6258693911264e-05
4397.71070707071 2.54463996640829e-05
4464.57636363636 2.46709111475386e-05
4531.44202020202 2.39300467633088e-05
4598.30767676768 2.32217838122691e-05
4665.17333333333 2.25442448267973e-05
4732.03898989899 2.1895685253788e-05
4798.90464646465 2.1274482338067e-05
4865.7703030303 2.06791250744487e-05
4932.63595959596 2.01082051127106e-05
4999.50161616162 1.95604085136687e-05
5066.36727272727 1.90345082666029e-05
5133.23292929293 1.85293574887851e-05
5200.09858585859 1.80438832370188e-05
5266.96424242424 1.75770808690911e-05
5333.8298989899 1.71280089000385e-05
5400.69555555556 1.6695784304251e-05
5467.56121212121 1.62795782198305e-05
5534.42686868687 1.58786120163434e-05
5601.29252525252 1.54921536912857e-05
5668.15818181818 1.51195145642505e-05
5735.02383838384 1.4760046241041e-05
5801.8894949495 1.4413137822849e-05
5868.75515151515 1.40782133381651e-05
5935.62080808081 1.37547293773516e-05
6002.48646464646 1.34421729118194e-05
6069.35212121212 1.3140059281537e-05
6136.21777777778 1.28479303361983e-05
6203.08343434343 1.25653527167954e-05
6269.94909090909 1.22919162656162e-05
6336.81474747475 1.20272325538217e-05
6403.6804040404 1.17709335167797e-05
6470.54606060606 1.15226701882411e-05
6537.41171717172 1.12821115252695e-05
6604.27737373737 1.10489433165677e-05
6671.14303030303 1.08228671675116e-05
6738.00868686869 1.06035995557969e-05
6804.87434343434 1.03908709521453e-05
6871.74 1.01844250010005e-05
};
\addplot [very thick, royalblue28108204]
table {%
219.22 0.011036362330508
294.266060606061 0.00683752177615596
369.312121212121 0.00464144864349475
444.358181818182 0.00334666716525019
519.404242424242 0.0025193038327363
594.450303030303 0.00195898836228103
669.496363636364 0.00156242272863255
744.542424242424 0.00127184853740656
819.588484848485 0.00105288309708372
894.634545454545 0.000884011430865333
969.680606060606 0.000751210162546177
1044.72666666667 0.000645022898528129
1119.77272727273 0.000558886634562944
1194.81878787879 0.000488132454642395
1269.86484848485 0.000429366813814566
1344.91090909091 0.000380076270852898
1419.95696969697 0.000338367971794018
1495.00303030303 0.0003027951072934
1570.04909090909 0.000272236981973959
1645.09515151515 0.000245815016365929
1720.14121212121 0.000222832893735278
1795.18727272727 0.000202733241627402
1870.23333333333 0.000185065832838411
1945.27939393939 0.000169463938324359
2020.32545454545 0.000155626532140522
2095.37151515152 0.000143304752953709
2170.41757575758 0.00013229149937599
2245.46363636364 0.000122413358503866
2320.5096969697 0.00011352428972744
2395.55575757576 0.00010550064185257
2470.60181818182 9.82371921850629e-05
2545.64787878788 9.16439755603686e-05
2620.69393939394 8.56437288176314e-05
2695.74 8.01698183332399e-05
2770.78606060606 7.51645493600184e-05
2845.83212121212 7.05777791330937e-05
2920.87818181818 6.63657731597201e-05
2995.92424242424 6.24902573397632e-05
3070.9703030303 5.89176286642295e-05
3146.01636363636 5.56182950054424e-05
3221.06242424242 5.25661205236171e-05
3296.10848484848 4.97379578968152e-05
3371.15454545455 4.71132522503113e-05
3446.20060606061 4.46737045530535e-05
3521.24666666667 4.24029845402706e-05
3596.29272727273 4.02864850465218e-05
3671.33878787879 3.83111110946094e-05
3746.38484848485 3.64650982610337e-05
3821.43090909091 3.47378557882919e-05
3896.47696969697 3.31198306849694e-05
3971.52303030303 3.16023896826275e-05
4046.56909090909 3.01777164323574e-05
4121.61515151515 2.88387217459749e-05
4196.66121212121 2.75789650348172e-05
4271.70727272727 2.63925853870252e-05
4346.75333333333 2.52742409632466e-05
4421.79939393939 2.42190555898078e-05
4496.84545454546 2.32225715948118e-05
4571.89151515152 2.22807080720926e-05
4646.93757575758 2.13897238752291e-05
4721.98363636364 2.05461847426933e-05
4797.0296969697 1.97469340388092e-05
4872.07575757576 1.89890666660709e-05
4947.12181818182 1.8269905764614e-05
5022.16787878788 1.75869818659648e-05
5097.21393939394 1.69380142120492e-05
5172.26 1.63208939879861e-05
5247.30606060606 1.57336692494166e-05
5322.35212121212 1.51745313528374e-05
5397.39818181818 1.46418027212986e-05
5472.44424242424 1.41339257984621e-05
5547.4903030303 1.3649453061884e-05
5622.53636363636 1.31870379818742e-05
5697.58242424242 1.2745426825751e-05
5772.62848484848 1.23234512190284e-05
5847.67454545455 1.19200213852963e-05
5922.72060606061 1.15341199954871e-05
5997.76666666667 1.1164796565038e-05
6072.81272727273 1.08111623443141e-05
6147.85878787879 1.04723856536745e-05
6222.90484848485 1.0147687619861e-05
6297.95090909091 9.83633827504848e-06
6372.99696969697 9.53765298401601e-06
6448.04303030303 9.25098916853041e-06
6523.08909090909 8.97574330125288e-06
6598.13515151515 8.71134814433109e-06
6673.18121212121 8.45727021036785e-06
6748.22727272727 8.21300742570822e-06
6823.27333333333 7.97808697798452e-06
6898.31939393939 7.75206333164318e-06
6973.36545454545 7.53451639676642e-06
7048.41151515152 7.32504983792122e-06
7123.45757575758 7.12328951103846e-06
7198.50363636364 6.92888201746202e-06
7273.5496969697 6.74149336532551e-06
7348.59575757576 6.56080772932964e-06
7423.64181818182 6.38652630081431e-06
7498.68787878788 6.21836622075785e-06
7573.73393939394 6.05605958900093e-06
7648.78 5.89935254359227e-06
};
\addplot [very thick, chocolate21910927]
table {%
21.9 1.0078570427758
98.3654545454546 0.2191050322673
174.830909090909 0.103686045815564
251.296363636364 0.0617251706835256
327.761818181818 0.0412646564516899
404.227272727273 0.0296207811034494
480.692727272727 0.0223193659311728
557.158181818182 0.0174232049026206
633.623636363636 0.0139736957749938
710.089090909091 0.0114492767714463
786.554545454546 0.00954521391587949
863.02 0.00807326725451775
939.485454545455 0.00691183157566669
1015.95090909091 0.00597939843250849
1092.41636363636 0.00521962002514998
1168.88181818182 0.00459250384210468
1245.34727272727 0.00406901417330281
1321.81272727273 0.00362764933933606
1398.27818181818 0.0032522074678756
1474.74363636364 0.00293029043161332
1551.20909090909 0.00265227924085705
1627.67454545455 0.00241061810260261
1704.14 0.0021993050831932
1780.60545454545 0.00201352383119329
1857.07090909091 0.00184937335174151
1933.53636363636 0.00170366705468494
2010.00181818182 0.00157378147649931
2086.46727272727 0.00145754110887291
2162.93272727273 0.00135312980232053
2239.39818181818 0.00125902195620536
2315.86363636364 0.00117392859876608
2392.32909090909 0.00109675478400001
2468.79454545455 0.00102656566940986
2545.26 0.000962559310194387
2621.72545454545 0.000904044692029398
2698.19090909091 0.000850423880746343
2774.65636363636 0.00080117743043952
2851.12181818182 0.000755852387835003
2927.58727272727 0.000714052378396769
3004.05272727273 0.000675429371582583
3080.51818181818 0.000639676808172313
3156.98363636364 0.000606523838382434
3233.44909090909 0.000575730470443258
3309.91454545455 0.000547083469046607
3386.38 0.000520392874236015
3462.84545454545 0.000495489035898439
3539.31090909091 0.000472220078521697
3615.77636363636 0.000450449726437509
3692.24181818182 0.000430055432238308
3768.70727272727 0.000410926761097904
3845.17272727273 0.000392963991851128
3921.63818181818 0.000376076902290521
3998.10363636364 0.000360183711527083
4074.56909090909 0.000345210156677772
4151.03454545454 0.000331088684775047
4227.5 0.000317757743793077
4303.96545454545 0.000305161159170793
4380.43090909091 0.000293247584278782
4456.89636363636 0.000281970015001416
4533.36181818182 0.000271285360048972
4609.82727272727 0.000261154059826313
4686.29272727273 0.000251539747705227
4762.75818181818 0.000242408948409414
4839.22363636364 0.000233730808951008
4915.68909090909 0.000225476858177422
4992.15454545454 0.000217620791515058
5068.62 0.000210138277946928
5145.08545454545 0.000203006786646667
5221.55090909091 0.000196205431022106
5298.01636363636 0.000189714828205715
5374.48181818182 0.000183516972274177
5450.94727272727 0.000177595119690793
5527.41272727273 0.000171933685647355
5603.87818181818 0.000166518150140791
5680.34363636364 0.000161334972757693
5756.80909090909 0.000156371515259816
5833.27454545455 0.000151615971168234
5909.74 0.000147057301635264
5986.20545454545 0.000142685176973253
6062.67090909091 0.000138489923279466
6139.13636363636 0.000134462473657898
6215.60181818182 0.000130594323593043
6292.06727272727 0.000126877490078347
6368.53272727273 0.000123304474144248
6444.99818181818 0.000119868226467895
6521.46363636364 0.00011656211577962
6597.92909090909 0.000113379899810427
6674.39454545455 0.000110315698550695
6750.86 0.000107363969613341
6827.32545454545 0.000104519485515184
6903.79090909091 0.000101777312708554
6980.25636363636 9.91327922114865e-05
7056.72181818182 9.65815216994116e-05
7133.18727272727 9.41193389343082e-05
7209.65272727273 9.17423064189557e-05
7286.11818181818 8.94466971743869e-05
7362.58363636364 8.72289815480577e-05
7439.04909090909 8.50858149686914e-05
7515.51454545455 8.30140265713605e-05
7591.98 8.10106086232193e-05
};
\addplot [very thick, indianred19152101]
table {%
21.9 0.697249134110895
89.3119191919192 0.558771852563526
156.723838383838 0.438663151977154
224.135757575758 0.359288923028068
291.547676767677 0.303321184043088
358.959595959596 0.261715903067723
426.371515151515 0.229550676511369
493.783434343434 0.203932280241939
561.195353535354 0.183047327591418
628.607272727273 0.165699487502708
696.019191919192 0.151066319912956
763.431111111111 0.138563056662377
830.84303030303 0.127762113462392
898.25494949495 0.1183433649872
965.666868686869 0.110062247764314
1033.07878787879 0.102728631411424
1100.49070707071 0.0961924296417323
1167.90262626263 0.0903335616813401
1235.31454545455 0.0850547985616458
1302.72646464646 0.0802765684834894
1370.13838383838 0.0759331209535986
1437.5503030303 0.0719696513058228
1504.96222222222 0.0683401156560565
1572.37414141414 0.0650055499045469
1639.78606060606 0.0619327618895816
1707.19797979798 0.0590933033327964
1774.6098989899 0.0564626540398092
1842.02181818182 0.0540195688620435
1909.43373737374 0.0517455507114383
1976.84565656566 0.0496244221000263
2044.25757575758 0.0476419743481763
2111.6694949495 0.0457856785088794
2179.08141414141 0.0440444456973288
2246.49333333333 0.0424084272463756
2313.90525252525 0.0408688471756461
2381.31717171717 0.0394178610401132
2448.72909090909 0.0380484364381969
2516.14101010101 0.0367542514009485
2583.55292929293 0.0355296076190625
2650.96484848485 0.0343693560424299
2718.37676767677 0.0332688328442185
2785.78868686869 0.0322238041054382
2853.20060606061 0.0312304178673089
2920.61252525253 0.0302851624332679
2988.02444444444 0.0293848299921829
3055.43636363636 0.0285264847885997
3122.84828282828 0.027707435191869
3190.2602020202 0.0269252091193895
3257.67212121212 0.0261775323544153
3325.08404040404 0.0254623093693766
3392.49595959596 0.0247776063242331
3459.90787878788 0.02412163595821
3527.3197979798 0.0234927441341412
3594.73171717172 0.022889397828956
3662.14363636364 0.0223101743927661
3729.55555555556 0.021753751923449
3796.96747474748 0.0212189006243442
3864.37939393939 0.0207044750303067
3931.79131313131 0.0202094070023835
3999.20323232323 0.019732699404239
4066.61515151515 0.0192734203844684
4134.02707070707 0.0188306981984193
4201.43898989899 0.0184037165113004
4268.85090909091 0.0179917101314147
4336.26282828283 0.017593961128459
4403.67474747475 0.0172097952971348
4471.08666666667 0.0168385789309243
4538.49858585859 0.0164797158749047
4605.9105050505 0.0161326448299829
4673.32242424242 0.0157968368840042
4740.73434343434 0.0154717932478821
4808.14626262626 0.0151570431772616
4875.55818181818 0.0148521420623099
4942.9701010101 0.0145566696700649
5010.38202020202 0.0142702285253929
5077.79393939394 0.0139924424180382
5145.20585858586 0.0137229550245234
5212.61777777778 0.0134614286347806
5280.0296969697 0.0132075429743993
5347.44161616162 0.01296099411427
5414.85353535354 0.0127214934601939
5482.26545454545 0.0124887668157433
5549.67737373737 0.0122625535122886
5617.08929292929 0.0120426056006789
5684.50121212121 0.0118286870995706
5751.91313131313 0.0116205732958554
5819.32505050505 0.0114180500930525
5886.73696969697 0.0112209134038957
5954.14888888889 0.0110289685836821
6021.56080808081 0.0108420299012487
6088.97272727273 0.0106599200447124
6156.38464646465 0.010482469659358
6223.79656565657 0.0103095169152764
6291.20848484848 0.0101409071025596
6358.6204040404 0.00997649225203871
6426.03232323232 0.0098161307797189
6493.44424242424 0.00965968715321413
6560.85616161616 0.00950703157862156
6628.26808080808 0.00935803970640039
6695.68 0.00921259235493324
};
\addplot [very thick, saddlebrown1356716]
table {%
21.22 1.14174776291221
69.7387878787879 0.195466308142931
118.257575757576 0.100755761065442
166.776363636364 0.0681135674801398
215.295151515152 0.0519726362644293
263.813939393939 0.0424302396756762
312.332727272727 0.0361510621745955
360.851515151515 0.0317134541757426
409.370303030303 0.0284134581051069
457.889090909091 0.0258640767754427
506.407878787879 0.0238354532740645
554.926666666667 0.0221826761924588
603.445454545455 0.0208099514170848
651.964242424242 0.0196514604329014
700.48303030303 0.0186605064266298
749.001818181818 0.0178030500802754
797.520606060606 0.017053697665636
846.039393939394 0.016393122093579
894.558181818182 0.0158063540972328
943.07696969697 0.0152816196629324
991.595757575757 0.0148095305038776
1040.11454545455 0.0143825086373756
1088.63333333333 0.0139943697774407
1137.15212121212 0.0136400166882847
1185.67090909091 0.0133152100839586
1234.1896969697 0.0130163951312729
1282.70848484848 0.0127405684293275
1331.22727272727 0.0124851748636661
1379.74606060606 0.0122480267908771
1428.26484848485 0.0120272401101293
1476.78363636364 0.0118211832431826
1525.30242424242 0.0116284360804962
1573.82121212121 0.0114477566932651
1622.34 0.011278054149304
1670.85878787879 0.0111183661651675
1719.37757575758 0.0109678406190929
1767.89636363636 0.0108257201679165
1816.41515151515 0.0106913293760809
1864.93393939394 0.0105640638904498
1913.45272727273 0.0104433812910301
1961.97151515151 0.0103287933222401
2010.4903030303 0.0102198592674141
2059.00909090909 0.0101161802747588
2107.52787878788 0.0100173944789022
2156.04666666667 0.00992317279070501
2204.56545454545 0.00983321525078578
2253.08424242424 0.00974724786051065
2301.60303030303 0.00966501981896471
2350.12181818182 0.00958630110640796
2398.64060606061 0.00951088036448681
2447.15939393939 0.00943856303147151
2495.67818181818 0.00936916969737081
2544.19696969697 0.00930253464920889
2592.71575757576 0.00923850458125746
2641.23454545455 0.00917693744876658
2689.75333333333 0.00911770144687311
2738.27212121212 0.00906067409899405
2786.79090909091 0.00900574144122278
2835.3096969697 0.00895279729111354
2883.82848484848 0.00890174259081974
2932.34727272727 0.00885248481589422
2980.86606060606 0.00880493744220323
3029.38484848485 0.00875901946438303
3077.90363636364 0.00871465496010419
3126.42242424242 0.00867177269512849
3174.94121212121 0.00863030576476093
3223.46 0.00859019126783466
3271.97878787879 0.00855137000982797
3320.49757575758 0.00851378623211398
3369.01636363636 0.00847738736469155
3417.53515151515 0.0084421238000498
3466.05393939394 0.00840794868608345
3514.57272727273 0.00837481773620755
3563.09151515151 0.0083426890550239
3611.6103030303 0.0083115229780693
3660.12909090909 0.00828128192433286
3708.64787878788 0.00825193026036767
3757.16666666667 0.00822343417494452
3805.68545454545 0.00819576156330329
3854.20424242424 0.00816888192015281
3902.72303030303 0.00814276624065563
3951.24181818182 0.00811738692870892
3999.76060606061 0.00809271771190032
4048.27939393939 0.00806873356257708
4096.79818181818 0.00804541062452052
4145.31696969697 0.00802272614476551
4193.83575757576 0.00800065841014755
4242.35454545455 0.00797918668819801
4290.87333333333 0.00795829117204328
4339.39212121212 0.00793795292899351
4387.91090909091 0.00791815385253547
4436.4296969697 0.00789887661746839
4484.94848484848 0.00788010463794474
4533.46727272727 0.0078618220281981
4581.98606060606 0.00784401356575904
4630.50484848485 0.00782666465697619
4679.02363636364 0.00780976130467573
4727.54242424242 0.00779329007780482
4776.06121212121 0.0077772380829191
4824.58 0.00776159293738334
};
\addplot [very thick, gray127]
table {%
21.92 0.625698935818945
99.1056565656566 1.03563366315929
176.291313131313 0.897706153317603
253.47696969697 0.745835407734477
330.662626262626 0.621506093953132
407.848282828283 0.523407202354208
485.033939393939 0.445811576849736
562.219595959596 0.383731569670545
639.405252525253 0.333414172773651
716.590909090909 0.292114363530882
793.776565656566 0.257821795730983
870.962222222222 0.229048531101515
948.147878787879 0.204678461230951
1025.33353535354 0.183862756103749
1102.51919191919 0.165947209755718
1179.70484848485 0.150421285076581
1256.89050505051 0.136881932616928
1334.07616161616 0.12500755535566
1411.26181818182 0.114539023634749
1488.44747474747 0.105265652566849
1565.63313131313 0.0970147181915848
1642.81878787879 0.0896435293439657
1720.00444444444 0.0830333678268718
1797.1901010101 0.0770848101753968
1874.37575757576 0.0717140822325848
1951.56141414141 0.0668501937139689
2028.74707070707 0.062432667490085
2105.93272727273 0.0584097264144623
2183.11838383838 0.0547368351450021
2260.30404040404 0.0513755195840006
2337.4896969697 0.0482924050517742
2414.67535353535 0.0454584280135362
2491.86101010101 0.0428481864265256
2569.04666666667 0.0404394015004605
2646.23232323232 0.0382124695354444
2723.41797979798 0.0361500869962508
2800.60363636364 0.0342369354474593
2877.78929292929 0.0324594156638916
2954.97494949495 0.0308054223321162
3032.16060606061 0.0292641524102663
3109.34626262626 0.0278259415188662
3186.53191919192 0.0264821237729732
3263.71757575758 0.0252249112950273
3340.90323232323 0.0240472903135827
3418.08888888889 0.0229429312903181
3495.27454545455 0.0219061109531922
3572.4602020202 0.0209316444681701
3649.64585858586 0.0200148262718307
3726.83151515152 0.0191513783251307
3804.01717171717 0.0183374047447263
3881.20282828283 0.0175693519304635
3958.38848484849 0.0168439734423223
4035.57414141414 0.0161582989922751
4112.7597979798 0.0155096070102765
4189.94545454545 0.0148954003222119
4267.13111111111 0.0143133845437472
4344.31676767677 0.0137614488497883
4421.50242424242 0.0132376488264415
4498.68808080808 0.0127401911523876
4575.87373737374 0.0122674198906229
4653.05939393939 0.011817804200557
4730.24505050505 0.011389927305271
4807.43070707071 0.0109824765700155
4884.61636363636 0.0105942345662978
4961.80202020202 0.0102240710116416
5038.98767676768 0.00987093548867547
5116.17333333333 0.00953385085894898
5193.35898989899 0.00921190729704406
5270.54464646465 0.00890425687938515
5347.7303030303 0.00861010866983449
5424.91595959596 0.00832872425085713
5502.10161616162 0.00805941365489057
5579.28727272727 0.00780153165567055
5656.47292929293 0.00755447438374995
5733.65858585859 0.00731767623438396
5810.84424242424 0.00709060703941877
5888.0298989899 0.00687276947786722
5965.21555555556 0.00666369670254846
6042.40121212121 0.00646295016254256
6119.58686868687 0.00627011760331522
6196.77252525253 0.0060848112282313
6273.95818181818 0.0059066660068288
6351.14383838384 0.00573533811669566
6428.3294949495 0.00557050350709816
6505.51515151515 0.0054118565736759
6582.70080808081 0.00525910893455691
6659.88646464647 0.00511198829917603
6737.07212121212 0.00497023742190997
6814.25777777778 0.00483361313338547
6891.44343434344 0.00470188544298531
6968.62909090909 0.00457483670667433
7045.81474747475 0.00445226085480569
7123.0004040404 0.00433396267505243
7200.18606060606 0.0042197571460437
7277.37171717172 0.00410946881767913
7354.55737373737 0.00400293123444896
7431.74303030303 0.00389998639840765
7508.92868686869 0.00380048426873882
7586.11434343434 0.00370428229511132
7663.3 0.00361124498226378
};
\addplot [draw=black, fill=black, mark=x, very thick, mark size=2.5pt, only marks]
table{%
x  y
87.6 0.272343533408822
351.36 0.0259470568426133
1450.24 0.00189066552594397
5765.12 0.000144604747120979
};
