# Supplementary material for: Swarm Reinforcement Learning For Adaptive Mesh Refinement
Source: arXiv:2304.00818 source file (2023-10-09)
Supplement: Supplementary file 19 [file group_generalization_runtime_1.tex]

\nextgroupplot[
ylabel shift = -0.2cm,
clip marker paths=true,
width=0.52\textwidth,
height=5.5cm,
scaled x ticks=false,
legend cell align={left},
legend style={fill opacity=0.8, draw opacity=1, text opacity=1, draw=lightgray204},
log basis x={10},
log basis y={10},
tick align=outside,
tick pos=left,
x grid style={darkgray176},
xlabel={Number of Elements},
xmajorgrids,
xmin=153.149074140696, xmax=143762.242818218,
xmode=log,
xtick style={color=black},
xtick={10,
100,200,500,
1000,2000,5000, 
10000,20000,50000, 
100000,200000,500000,
1000000,10000000},
xticklabels={
  \(\displaystyle {10^{1}}\),
  \(\displaystyle {10^{2}}\),
  \empty,
  \empty,
  \(\displaystyle {10^{3}}\),
  \empty,
  \empty,
  \(\displaystyle {10^{4}}\),
  \empty,
  \empty,
  \(\displaystyle {10^{5}}\),
  \empty,
  \empty,
  \(\displaystyle {10^{6}}\),
  \(\displaystyle {10^{7}}\)
},
y grid style={darkgray176},
ylabel={Squared Error},
ymajorgrids,
ymin=1.62801568293142e-06, ymax=2.08899185322288,
ymode=log,
ytick style={color=black},
ytick={1e-07,1e-06,1e-05,0.0001,0.001,0.01,0.1,1,10,100},
yticklabels={
  \(\displaystyle {10^{-7}}\),
  \(\displaystyle {10^{-6}}\),
  \(\displaystyle {10^{-5}}\),
  \(\displaystyle {10^{-4}}\),
  \(\displaystyle {10^{-3}}\),
  \(\displaystyle {10^{-2}}\),
  \(\displaystyle {10^{-1}}\),
  \(\displaystyle {10^{0}}\),
  \(\displaystyle {10^{1}}\),
  \(\displaystyle {10^{2}}\)
}
]
\addplot [
  draw=yellowgreen18420623,
  fill=yellowgreen18420623,
  forget plot,
  mark=*, mark size=1,
  only marks,
  draw opacity=0,
 fill opacity=0.5
]
table{%
x  y
209.04 0.654603877981477
209.32 0.582769724327232
216.22 0.609075119410975
235.72 0.563644999334164
242.64 0.528545483383789
261.46 0.466062572776632
264.18 0.466143352513158
266.92 0.551767847708456
269.88 0.558997675360308
285.84 0.574226339791752
299.22 0.499641091829033
326.82 0.547959710608015
333.16 0.549168172286927
379.86 0.518889530077008
383.58 0.476162570572269
397.7 0.49676816962886
413.34 0.44852546432235
458.54 0.440468594751043
609.12 0.201925600812304
748.06 0.0212336695841358
748.84 0.485567109549858
752.72 0.023468813071803
833.86 0.0152893045797151
881.98 0.0754313322537534
1123.6 0.00992313511340333
1208.8 0.0125449019384659
1288.52 0.00530458833020674
1297.2 0.0052695179130891
1299.26 0.00641243360579778
1347.54 0.00532965891687446
1396.44 0.00942896933089814
1425 0.00547851461590557
1562.46 0.00359028769197063
1796.7 0.00424759936113774
1862.96 0.00396647199301236
1895.04 0.00263335035824297
1906.7 0.00280636202037642
1936 0.0032044171663161
2193.56 0.00404684412397678
2264.44 0.00154984436829784
2411.22 0.00178238642969343
2578.04 0.00246490735068358
2600.9 0.00145335680436517
2676.1 0.00156341855083769
2841 0.00134715912815036
2882.62 0.00259874823935188
2987.36 0.00252208313067378
3118.58 0.0014973004537065
3165.54 0.00192503480735069
3308.76 0.00211845477789352
3330.52 0.000850798545468596
3340.7 0.00162147410058379
3431.06 0.00321632357612079
3446.76 0.00134373549865324
3565.12 0.00273031897456253
3581.62 0.00129892418093781
3754.42 0.00157423294629498
4308.62 0.000842418206731547
4466.06 0.000677676545088417
4723.96 0.000888535800839461
4898.66 0.000465405453538527
4920.06 0.000910877286159001
4989.86 0.000829966984162294
5258.22 0.00108155048403284
5285.98 0.0018858665144861
5531.64 0.000821729583591592
5601.68 0.000790979864438914
5646.26 0.000686725342318379
5677.16 0.00101464807037224
5965.08 0.00151574052099415
6301.14 0.00070787517461147
6509.24 0.000536015636792632
6743.46 0.000659625140444814
6976.84 0.000278008380538961
6981.7 0.000651000948699942
7816.44 0.000262504189262798
7834.6 0.000517050618498649
8440.86 0.000266483546858912
8644.98 0.000259134154272534
8667.8 0.000416732307474054
8890.72 0.000181550219633748
8927 0.000471627354770734
9036.46 0.000217474113031577
9426.34 0.000305105212344172
9541.62 0.000316380974042025
9691.26 0.000179991146907934
10099.5 0.000196316314711687
10203.36 0.000222151237164181
12210.98 0.000105071488826693
12737 0.000127365367963212
13639.7 0.000121988802173655
14911.26 7.94136857802901e-05
15058.3 7.25428613840203e-05
15328.6 7.56310968805507e-05
15358.04 0.00010114239730337
17250.42 9.24503328410993e-05
18933.88 3.34726785626599e-05
19241.9 2.70492862557171e-05
19965.94 2.56607797214613e-05
19986.98 3.14112275460309e-05
};
\addplot [
  draw=royalblue28108204,
  fill=royalblue28108204,
  forget plot,
  mark=*, mark size=1,
  only marks,
  draw opacity=0,
 fill opacity=0.5
]
table{%
x  y
427.62 0.385448378278534
453 0.422880041496415
465.5 0.377469916079197
479.56 0.311193590158296
487.12 0.349923005452532
541.16 0.32027536690775
569.78 0.315281016254934
585.52 0.155070777860909
594 0.193152372612715
628.66 0.240463226011996
718.1 0.277491457991627
743.46 0.169845972917647
753.08 0.24435618259018
799.26 0.194208585272808
801.04 0.258820611497489
807.32 0.227924325858863
899.28 0.130473113799921
1101.88 0.0638808096452007
1183.38 0.00935767827369261
1223.36 0.013260421568095
1239.5 0.010459423520965
1314.6 0.0112221227273586
1356.54 0.00776642335249954
1488.58 0.1529790387158
1689.96 0.00513386538079793
1756.4 0.00536333675121329
1864.64 0.00369460654298402
1921.52 0.00535281828003167
1933.12 0.00309662087778322
1970.46 0.00281690595658789
2023.08 0.00307828252520292
2070.34 0.00246195976046226
2365 0.00255069174209309
2370.84 0.00204461902808237
2591.36 0.00208356887774582
2661.22 0.00194917222521076
2689.2 0.00154954520319426
2726.28 0.00216067602726981
2755.96 0.00150239036837535
3292.2 0.00103745610349442
3368.7 0.000847339030752058
3484.86 0.000958406362176768
3489.3 0.000879983243300399
3773.72 0.00143738940887855
4032.22 0.000931777228912853
4034.76 0.00129799225561294
4078.58 0.0012795694020956
4119.98 0.00103137374112648
4125.4 0.00187209860033862
4132.84 0.00135048913386285
4168.36 0.000935552453006354
4204.12 0.00151799087582136
4559.78 0.000750409847095814
4648.28 0.000657672175532177
4698.44 0.00043610833424646
4740.38 0.000847592335034262
4754.1 0.000694689277652733
5820.08 0.00038434626257987
5945.1 0.000516031894571503
6191.96 0.00111689930803193
6374.28 0.000594052537707896
6532.24 0.000450089501296404
6577.92 0.00053420446261686
6592.24 0.000487752975191699
6789.98 0.000275257137480383
6896.06 0.000460884773013631
6975.3 0.000847208507863084
7098.96 0.000615702073620268
7263.24 0.000454966843740212
7522.34 0.000397591416995036
8121.74 0.00039310069456425
8200.28 0.000418950900107447
8253.12 0.000305933122373966
8585.46 0.000398983438099097
9035.24 0.000164935807804934
9635.98 0.000312960485407968
9873.08 0.000159549728370575
10596.5 0.000248146688099551
10668.36 0.000156893493824015
10796.46 0.000270532787493189
10831.44 0.000155199283836927
11108.26 0.000135568020422663
11335.78 0.00017235909788411
11351.2 0.000101526987148932
11622.34 0.000175920086574345
12221.88 0.000107636567538962
12913.54 0.000116208113323496
13097.22 0.000112008004476805
15957.22 5.82278996569072e-05
19068.98 6.98318291226892e-05
20292.34 6.80987323763023e-05
21525.14 4.36072497132602e-05
21639.7 6.02002078341832e-05
21711.82 4.41822927604527e-05
22459.14 4.23434244399274e-05
23743.4 5.13425869534069e-05
27460.28 1.82026973171664e-05
27764.16 1.82991229385739e-05
27974.52 1.55880687206445e-05
28972.38 1.42597503396678e-05
};
\addplot [draw=purple11522131, fill=purple11522131, forget plot, mark=*, mark size=1, only marks, draw opacity=0,
 fill opacity=0.5]
table{%
x  y
631.56 0.365381011690037
655.2 0.363379940484318
674.92 0.355899214024967
706.68 0.289616999962278
719.42 0.335825614030616
773.2 0.300923026603344
829.34 0.293233132126374
887.36 0.159115085227579
897.12 0.206453106572818
965.8 0.224138338515277
1038.26 0.258241263288338
1084.98 0.258159456199574
1105.46 0.199854954304654
1112.36 0.200928379438473
1142.08 0.223577706997601
1164.88 0.221435166395192
1249.34 0.146911026937622
1510.8 0.0648803188140402
1748.54 0.00538258844357775
1853.88 0.00731058959519297
1880.78 0.00517081664793154
1912.18 0.166030029905019
1964.2 0.00766883540162038
2020.92 0.00419789412793461
2352.36 0.0026019727816818
2398.86 0.002682199441479
2559.84 0.00198409492947015
2663.82 0.00240145621008484
2695.84 0.00181241547270147
2711.22 0.00179470714450008
2731.14 0.00167155772330103
2833.62 0.00144622059143479
3161.8 0.00147404518542208
3176.22 0.00124506672414402
3469.88 0.00120006719434552
3503.6 0.000885194605773223
3532.8 0.00112323330616889
3547.36 0.00123169302227247
3656.28 0.000853579372132922
4152.68 0.000637923351900684
4401.92 0.000566716914925743
4505.46 0.000588465377626234
4557.18 0.000844654286200446
4719.12 0.000486415001696008
4867.58 0.000610100507588738
4959.96 0.000597437804277416
4984.52 0.0007861159872843
5001.22 0.000629709814586056
5018.68 0.000928159289534977
5082.02 0.000967353223658496
5233.62 0.00076819474599588
5385.28 0.000453278922009693
5697.04 0.0004977242249999
5877.6 0.00037630676422881
6073.38 0.000821460081086797
6260.34 0.00025058766292939
7068.56 0.00065750746362473
7141.06 0.000401061139245871
7234.06 0.000231177440117648
7344.78 0.000360729701742853
7861.44 0.000251007363177405
7890 0.000514650804378014
8178.38 0.000271733899282265
8181.76 0.000325144594116453
8806.94 0.000332950536940306
8818.82 0.000283721795468052
9212.26 0.000371567470295169
9496.5 0.000272287774967767
9533.66 0.000160922599955212
9841.74 0.000224548111632921
10445.8 0.000269043407143566
10549.32 0.000228129910172768
10632.24 0.000179978280574799
10792.88 0.00024013064808721
11601.62 9.58933824811274e-05
11967.38 0.00019564763136277
12665.36 9.68890725420216e-05
13205.9 0.00014660437515264
13241.58 9.46180757976473e-05
13384.98 8.99350000508273e-05
13657.08 0.000156813047972738
13929.26 8.09975661073911e-05
14210.8 9.74045105228679e-05
14288.58 0.000100862515843504
14775 5.91905647088322e-05
15411.76 6.24317535774569e-05
16050.18 6.76301892323872e-05
16155.78 6.54667764756907e-05
19855.44 3.35433147216603e-05
27678.98 3.99178492936137e-05
28736.7 3.88968234070403e-05
30118.02 2.63025360731635e-05
30128.76 3.45339546545149e-05
30646.42 2.46880665254165e-05
31349.02 2.49603847344226e-05
32664.2 2.77622856622207e-05
37806.1 1.064055872233e-05
38726.24 1.01725482609675e-05
39471.8 9.05380456376319e-06
40496.88 8.04191358525413e-06
};
\addplot [
  draw=indianred19152101,
  fill=indianred19152101,
  forget plot,
  mark=*, mark size=1,
  only marks,
  draw opacity=0,
 fill opacity=0.5
]
table{%
x  y
869.92 0.31230395116569
878.2 0.310534992647468
910.1 0.324803205335026
961.12 0.316123079364651
961.68 0.260568619046331
1042.82 0.264947207114043
1091.48 0.267917386713916
1192.08 0.17263236440829
1197.68 0.152384804912319
1231.08 0.208533723266397
1306.48 0.231676041866881
1398.68 0.242554276996938
1405.52 0.206952137080318
1427.34 0.186636856252232
1430.92 0.212466322190101
1530.3 0.17223109310557
1583.76 0.133025550756279
2020.96 0.0394111784150557
2258.98 0.157101720075077
2406 0.0101064272086791
2434.2 0.00571718225982475
2619.82 0.0111829207044167
2655.62 0.00448505629612148
2820.54 0.00378370607171491
3033.12 0.00266350000401671
3187.66 0.00223156645653986
3384.72 0.00170432230874816
3490.56 0.00212715890453444
3611.82 0.00133031154715985
3657.4 0.00143670706971002
3748.38 0.00127746416507218
3811.22 0.00107610136357754
4055.76 0.00110458723954148
4381.28 0.000868800119607656
4421.34 0.000891259149194897
4467.96 0.00104378966566926
4503.54 0.000898200114387117
4530.22 0.000667396203093932
4803.64 0.000616557352465874
5372.5 0.000472169848747238
5618.62 0.000630406209934014
5618.78 0.000431368544861592
5678.84 0.000438749440226141
5849.04 0.000627235218322285
6038.46 0.0006872987642348
6065.24 0.000745848938091346
6083.42 0.00045866067484573
6090.68 0.000457552410392512
6201.64 0.000446043601001775
6226.16 0.000349299041953682
6750.5 0.000540589028354801
6793.1 0.000388032750273551
6823.12 0.000336792882235294
7334.24 0.000268558580447468
8042.76 0.000520448439040162
8148.6 0.000171795268428962
8688.94 0.000564788997835264
8774.94 0.000267709126598969
8946.7 0.000167963902626184
9524.08 0.000183233985797378
9552.46 0.000355980392770936
10041.5 0.000193883320257118
10084.5 0.000288112609486946
11057.32 0.000240803360414163
11722.8 0.000242323019931402
11805.2 0.000202073239343453
12007.24 0.000268673496256755
12362.24 0.000194088642742945
12760.84 0.00011638307971639
13000.42 0.000157122209262551
13380.6 0.000200754816603859
13517.88 0.00016164005596104
13762.5 0.000126501306111728
14001.04 0.000171001464656114
15071.54 6.79425121470694e-05
15144.12 0.000141485520136654
16369.28 7.12936726747518e-05
17116.14 0.000102159505724137
17222.64 6.79078985837699e-05
17253.7 0.000107195188294882
17545.24 6.46241320018052e-05
17728.44 5.9430194726256e-05
18239.92 6.98683528767877e-05
18382.48 6.68810000221926e-05
18997.76 4.14508229960856e-05
19742.02 4.40865054947455e-05
20649.12 4.50266438934158e-05
20720.92 4.60988246636191e-05
25086.34 2.33875234059197e-05
39625.32 2.85731003725263e-05
40581.76 2.76339851138465e-05
41766.96 1.88597273994776e-05
42071.98 2.38477802647249e-05
42781.1 1.70222267586084e-05
44012.88 1.6804059858734e-05
44711.54 1.87111683744864e-05
50632.14 7.63769767444339e-06
52384.58 7.05034951239003e-06
53933.42 6.37184364462913e-06
54364.58 5.72949236177777e-06
};
\addplot [
  draw=chocolate21910927,
  fill=chocolate21910927,
  forget plot,
  mark=*, mark size=1,
  only marks,
  draw opacity=0,
 fill opacity=0.5
]
table{%
x  y
1105.74 0.276269163147787
1120.24 0.268983541725035
1193.3 0.254094041506849
1222.92 0.223681208462993
1248.48 0.270579166282593
1317.54 0.224275933698004
1365.64 0.215976087621831
1523.64 0.155312227640429
1542 0.16858617501018
1563.74 0.130691423193455
1623.54 0.189246402531713
1725.72 0.171115508560284
1746.76 0.16908601864928
1768.02 0.149286535853603
1770.9 0.184674704883669
1937.1 0.149431066885602
2114.92 0.107599296330346
2518.18 0.0275910214243664
2685.6 0.117192933854814
3194.14 0.00244555284414065
3218.16 0.00358461552191202
3532.34 0.00239166371976149
3532.62 0.00732668468102966
3725.94 0.00199914551107942
3866.88 0.00140763013982319
4162.44 0.00127626355572251
4372.5 0.001019472225018
4379.58 0.00117937978987247
4580.26 0.000900434870993333
4622.28 0.000908392274799965
4778.76 0.000816372115624383
4831.8 0.000701626210274094
4991.76 0.000746091365836276
5440.62 0.000570077101147648
5472.14 0.000594363721462894
5486.82 0.000608906830733275
5577.22 0.000572881898436397
5649.12 0.000445666775221802
6058.56 0.000407503251563097
6557.2 0.000298378090760722
6731.18 0.000409254234534266
6811.86 0.000271651799492409
6815.88 0.000404300561183724
6951.56 0.000283407496159307
7181.08 0.000455982067290481
7211.16 0.000412981003067983
7299.3 0.000301516520999779
7312.74 0.000280659078205908
7506.36 0.000287424859065888
7901.66 0.000231339973459206
7927.94 0.000245292732752038
7950.64 0.000217917664275794
8599.12 0.000321106523023278
8727.02 0.000174154679445307
9007.86 0.000328476318966453
9955.76 0.000113021573994408
10120.56 0.000163578327061767
10662.28 0.000109431424743773
11081.08 0.000231182747565638
11364.38 0.000116096524249062
11422.46 0.000127875530893769
11736.46 0.000365054205437297
13503.92 0.000180083128409039
14350.2 0.000159852839267168
14964.04 0.000164467935817055
14981.12 0.000183045275479168
15083.78 0.000130894222862547
15690.24 0.000124154061290112
16201.42 7.97652497809167e-05
16332.64 0.000102642983696348
16445.38 0.000135606084821428
16754.56 0.000104626665359281
16844.74 8.35145420753915e-05
16885.46 0.000113986108542149
18243.14 9.33356398814075e-05
18345.02 4.56079242024324e-05
19945.34 4.92355242973045e-05
20477.3 6.61641398524118e-05
20797.2 4.54129216263566e-05
20893.3 6.84963416745985e-05
21304.04 4.32491191912671e-05
21306.64 4.08255706366745e-05
21566.5 4.5556828448363e-05
22104.08 4.32932731912078e-05
23258.44 2.69991721273969e-05
23917.62 2.9837103609224e-05
24519.18 3.02794154353449e-05
24745.82 2.91902643168851e-05
30108.1 1.47416334547747e-05
52084.02 1.913879522884e-05
53203.28 1.81902378508822e-05
54641.68 1.27205711958154e-05
54792.94 1.60064830792935e-05
55907.76 1.08360262989491e-05
57232.12 1.0504264365848e-05
57745.26 1.19928089840148e-05
64609.34 5.02060309026677e-06
66366.46 4.59342170238898e-06
68483.4 3.77649984120898e-06
69120.68 4.12721622984901e-06
};
\addplot [
  draw=saddlebrown1356716,
  fill=saddlebrown1356716,
  forget plot,
  mark=*, mark size=1,
  only marks,
  draw opacity=0,
 fill opacity=0.5
]
table{%
x  y
1406.64 0.319389597182295
1444.98 0.297711255412551
1533.66 0.310613180033839
1578.84 0.268626937360337
1598.82 0.303846028698328
1648.3 0.268584654719919
1718.32 0.273711260041157
1880.04 0.228039477623516
1907.58 0.18464701285081
1944.62 0.145136440968834
1974.92 0.259606118215738
2066.74 0.231833670677216
2108.2 0.222832429301748
2140.94 0.251010644384737
2176.76 0.188819559720547
2416.84 0.175202268961884
2444.04 0.159451192512517
3116.32 0.148945009836886
3264.84 0.0405475363960824
3998.48 0.00334980384832795
4089.52 0.00210811643037562
4632.66 0.00204490236688823
4650.42 0.00115058879582229
4737.02 0.00993183629130148
4852.24 0.00208686657232068
5290.9 0.00111195032573906
5474.16 0.000880663333556275
5507.04 0.00103311789829294
5794.9 0.000705925354164077
5801.88 0.000762266056758419
6103.16 0.000567509149604142
6150.64 0.000664317571696486
6188.04 0.000603221799148467
6652.4 0.000501905561264934
6694.32 0.000490796788558348
6773.44 0.000462415519358879
6949.84 0.000366366389445426
7111.18 0.000467636616117393
7618.72 0.000335223136826732
8065.56 0.000250664309121769
8140.76 0.000333232936434826
8282.38 0.000338069527825242
8306.98 0.000234847318172977
8460.22 0.00036569120616471
8503.34 0.000241943881137073
8551.88 0.000351379329122643
8628.1 0.000236049570948135
8806.32 0.000257539837235425
9070.84 0.000246433212289747
9434.64 0.00020653333955828
9553.82 0.000183536036148704
9646.2 0.000202382304054197
10328.08 0.000140046251586396
10414.12 0.000266427419234044
10672.74 0.000260521091208189
11766.64 0.00014449420392311
12025.42 9.63833449518542e-05
12771.28 9.66000028128474e-05
13053.3 0.000195779028159536
13131.4 9.90553301839005e-05
13530.18 0.000112253348577057
15566.6 0.000301732498430617
17691.64 0.000154412886192847
18545.28 0.000138236111663341
19134.76 0.000150773688599151
19260.54 0.000137759137000627
19312.86 0.000109603648127093
20002 0.000105186105714267
20577.98 6.70430398703451e-05
20631.66 8.2917202556555e-05
20691.14 0.000116175683472105
21123.44 8.93434623373923e-05
21261.16 6.94948308501961e-05
21267.3 9.48459050779686e-05
22314.72 3.78951132455437e-05
22760.4 8.08870985260245e-05
24665.76 4.22557472248159e-05
24930.46 5.55637189458248e-05
25207.5 3.82290315683488e-05
25517.4 5.66641696728795e-05
25696 3.47993149488656e-05
25826.4 3.63757668692358e-05
26028.2 3.78252372419015e-05
26935.1 3.58420239575613e-05
28409.96 2.26500386537967e-05
28538.12 2.48116166071802e-05
29313.38 2.5330990859222e-05
29533.24 2.42746860620815e-05
35407.36 1.24707451526235e-05
69238.02 1.64433501221248e-05
70191.08 1.52780525360734e-05
71595.62 1.04880959977126e-05
71632 1.30524511786246e-05
72729.08 8.76674847148926e-06
74096.54 8.7575172893321e-06
74738.08 9.32590336354384e-06
81486.48 4.10542488391062e-06
84096.48 3.72577962055073e-06
86182.26 3.08537240936141e-06
87565.88 3.44022758336781e-06
};
\addplot [draw=black18, fill=black18, forget plot, mark=*, mark size=1, only marks, draw opacity=0,
 fill opacity=0.5]
table{%
x  y
1648.2 0.340532709117366
1650 0.343495016538461
1835.4 0.280012326436764
1877 0.280569878862033
1918.8 0.172612052251009
2022.2 0.233739926707236
2090.8 0.227472436040243
2311.6 0.0769692379512679
2411 0.137920507238948
2436.6 0.158573303688796
2587.6 0.0269684210222804
2632.6 0.136199024940898
2660.8 0.134154705709882
2682 0.155011962547538
2832.6 0.105610761919391
3031.2 0.117298585396121
3281.6 0.0444463919098803
3846 0.100416438777728
3869.4 0.00386948592472434
4911 0.00315179546252802
4919.2 0.00274400711677113
5653.2 0.00144287412581414
5773.2 0.002188684162659
5872 0.0158401642037021
5988.6 0.0016761068598992
6473 0.00129245169700966
6580.2 0.00126447626519376
6662.4 0.00104990466243681
6871.6 0.000702734126230265
6895 0.000703465103111041
7057.6 0.000616630568608566
7138.8 0.000707231959387349
7239.4 0.000607445902882223
7402.6 0.000589351587460201
7644 0.000493432016644157
7753 0.000483550304362254
7976 0.000361595067999578
8143.8 0.000492789060138816
8593.6 0.000347069357444556
9036.4 0.00025597801450793
9043.8 0.000343117259395124
9064.6 0.000340366349888505
9362.4 0.000244238050054011
9466.2 0.000360680533844759
9547.6 0.000247675974642974
9625.6 0.00024120314996946
9629 0.000356292864887336
9822.8 0.00026426174945453
10201.2 0.000239806405294172
10312.2 0.000205896781922519
10532.2 0.000194066045639245
11186.8 0.000218648718055449
11301.2 0.000148670553686126
11353.2 0.000258763002591494
12515.6 0.000281555801899407
12787.2 0.000157212096101165
13291.2 0.000102868689383539
14001.6 9.91548077544266e-05
14277.2 0.000104565460231859
14701 0.000117752846886909
15081.2 0.000199120575010023
19222.2 0.000311731081787238
22108.4 0.000161701036497274
23020 0.00014117585332934
23205 0.000154562799062982
23618 0.000141536509194176
23796.4 0.000114426873708962
24353 0.00010966868839383
24892.8 7.0333031663019e-05
25129.8 8.54603830405158e-05
25206.8 0.000117207566911859
25272.6 7.230988832025e-05
25301.2 9.65938221587444e-05
25494.8 9.47301229817765e-05
25604.8 3.7018922507216e-05
26888.2 8.49185462428493e-05
28699 4.35541714734506e-05
29291.6 4.00064551981063e-05
29363 5.83931286111274e-05
29574 3.83868471892033e-05
29872.4 3.64462119861039e-05
29961.2 3.69116814957769e-05
29975 5.7760132037966e-05
31201.6 3.65802569313934e-05
32510 2.30023853167503e-05
32695.2 2.53184935852108e-05
33100.4 2.51434510891358e-05
33693.4 2.4626044681979e-05
39459 1.30501476649835e-05
87162.4 1.71645006521647e-05
88035 1.60224259501968e-05
89329.4 1.11261828002477e-05
89526.8 1.29265718931913e-05
90730.2 9.13208441203441e-06
92386.6 9.82194880226024e-06
92396 9.07656044449038e-06
99135 4.21908560510371e-06
102001.2 3.91880386326471e-06
103312.6 3.164228441159e-06
105324.6 3.54024107506776e-06
};
\addplot [very thick, yellowgreen18420623]
table {%
209.04 1.10226936892416
408.817171717172 0.195380991071543
608.594343434343 0.0732219178977929
808.371515151515 0.0371032335010517
1008.14868686869 0.0221225340648818
1207.92585858586 0.0145989975200604
1407.70303030303 0.0103239414865185
1607.4802020202 0.00767555909072921
1807.25737373737 0.00592674444197881
2007.03454545455 0.00471384402540334
2206.81171717172 0.00383925469483754
2406.58888888889 0.00318837358142619
2606.36606060606 0.00269114635687591
2806.14323232323 0.00230285271334944
3005.9204040404 0.0019938871636907
3205.69757575758 0.00174403417683965
3405.47474747475 0.00153911683910016
3605.25191919192 0.00136895949915942
3805.02909090909 0.00122610796061999
4004.80626262626 0.00110500212593563
4204.58343434343 0.00100142739092847
4404.36060606061 0.000912142563180326
4604.13777777778 0.000834622344449384
4803.91494949495 0.000766875821634287
5003.69212121212 0.000707316399724999
5203.46929292929 0.000654667184696671
5403.24646464646 0.000607891201372615
5603.02363636364 0.000566139274021034
5802.80080808081 0.000528710643980216
6002.57797979798 0.000495022890348502
6202.35515151515 0.000464588726364046
6402.13232323232 0.000436997933481566
6601.90949494949 0.000411903173835891
6801.68666666667 0.00038900875844472
7001.46383838384 0.00036806168812433
7201.24101010101 0.000348844456556011
7401.01818181818 0.000331169230372948
7600.79535353535 0.000314873113261734
7800.57252525253 0.00029981426936074
8000.3496969697 0.000285868732298376
8200.12686868687 0.000272927764707837
8399.90404040404 0.000260895662300265
8599.68121212121 0.000249687918960816
8799.45838383838 0.000239229686581884
8999.23555555556 0.000229454476729908
9199.01272727273 0.00022030306168938
9398.7898989899 0.000211722540632303
9598.56707070707 0.000203665543141867
9798.34424242424 0.000196089547465517
9998.12141414141 0.000188956294980878
10197.8985858586 0.000182231285653963
10397.6757575758 0.000175883341925831
10597.4529292929 0.000169884230615209
10797.2301010101 0.00016420833417427
10997.0072727273 0.00015883236406373
11196.7844444444 0.000153735110185226
11396.5616161616 0.000148897221273512
11596.3387878788 0.000144301011947993
11796.115959596 0.000139930292784016
11995.8931313131 0.000135770220314248
12195.6703030303 0.000131807164329527
12395.4474747475 0.000128028590233154
12595.2246464646 0.00012442295452556
12795.0018181818 0.000120979611768568
12994.778989899 0.000117688731608449
13194.5561616162 0.000114541224632007
13394.3333333333 0.000111528675995525
13594.1105050505 0.000108643285907588
13793.8876767677 0.00010587781616737
13993.6648484848 0.000103225542063174
14193.442020202 0.000100680209024633
14393.2191919192 9.82359934982206e-05
14592.9963636364 9.58874675814104e-05
14792.7735353535 9.36295670076387e-05
14992.5507070707 9.14575621233952e-05
15192.3278787879 8.93670315414371e-05
15392.1050505051 8.73538381912155e-05
15591.8822222222 8.54141075199394e-05
15791.6593939394 8.35442076258965e-05
15991.4365656566 8.17407311303148e-05
16191.2137373737 8.0000478615665e-05
16390.9909090909 7.83204434772562e-05
16590.7680808081 7.66977980516377e-05
16790.5452525253 7.5129880899996e-05
16990.3224242424 7.36141851376822e-05
17190.0995959596 7.21483477124108e-05
17389.8767676768 7.07301395438078e-05
17589.6539393939 6.93574564459216e-05
17789.4311111111 6.80283107622618e-05
17989.2082828283 6.67408236499996e-05
18188.9854545455 6.54932179562315e-05
18388.7626262626 6.42838116348131e-05
18588.5397979798 6.31110116572627e-05
18788.316969697 6.19733083756893e-05
18988.0941414141 6.08692702996981e-05
19187.8713131313 5.9797539252784e-05
19387.6484848485 5.87568258769468e-05
19587.4256565657 5.77459054571197e-05
19787.2028282828 5.67636140395986e-05
19986.98 5.58088448209783e-05
};
\addplot [very thick, royalblue28108204]
table {%
427.62 0.631417063344921
715.950909090909 0.117437547843278
1004.28181818182 0.0418009901709474
1292.61272727273 0.0200739430729886
1580.94363636364 0.0114370868438442
1869.27454545455 0.00727255026306344
2157.60545454545 0.00499017903310614
2445.93636363636 0.00362008029275953
2734.26727272727 0.00273974218553605
3022.59818181818 0.00214350935605459
3310.92909090909 0.0017223995216774
3599.26 0.00141464184970913
3887.59090909091 0.00118326087731765
4175.92181818182 0.00100510052063012
4464.25272727273 0.000865097211344702
4752.58363636364 0.000753128716920478
5040.91454545455 0.000662200133837547
5329.24545454545 0.000587358272732876
5617.57636363636 0.00052501963340274
5905.90727272727 0.00047254188101367
6194.23818181818 0.000427943327107376
6482.56909090909 0.000389714951215767
6770.9 0.000356691764308235
7059.23090909091 0.000327963099296516
7347.56181818182 0.000302808966386321
7635.89272727273 0.000280654189329924
7924.22363636364 0.00026103487946464
8212.55454545455 0.00024357360506156
8500.88545454546 0.00022796077726002
8789.21636363637 0.000213940539560056
9077.54727272728 0.000201299960010102
9365.87818181818 0.000189860673068185
9654.20909090909 0.000179472357716706
9942.54 0.000170007605638762
10230.8709090909 0.000161357851418717
10519.2018181818 0.000153430121173871
10807.5327272727 0.000146144417026922
11095.8636363636 0.000139431599343721
11384.1945454545 0.000133231661453683
11672.5254545455 0.000127492315944088
11960.8563636364 0.000122167829889524
12249.1872727273 0.000117218060181777
12537.5181818182 0.000112607650634342
12825.8490909091 0.000108305360593422
13114.18 0.000104283501007588
13402.5109090909 0.000100517458741415
13690.8418181818 9.69852936967713e-05
13979.1727272727 9.36673962765936e-05
14267.5036363636 9.05461950755738e-05
14555.8345454545 8.76059065500828e-05
14844.1654545455 8.48323199122444e-05
15132.4963636364 8.22126116916682e-05
15420.8272727273 7.97351853752928e-05
15709.1581818182 7.73895323193886e-05
15997.4890909091 7.51661107655641e-05
16285.82 7.30562403138558e-05
16574.1509090909 7.10520096336308e-05
16862.4818181818 6.91461955453439e-05
17150.8127272727 6.73321918973753e-05
17439.1436363636 6.56039469038051e-05
17727.4745454545 6.39559078101122e-05
18015.8054545455 6.23829719217708e-05
18304.1363636364 6.08804431715052e-05
18592.4672727273 5.94439935192425e-05
18880.7981818182 5.80696285785606e-05
19169.1290909091 5.67536569477226e-05
19457.46 5.54926627948816e-05
19745.7909090909 5.42834813077869e-05
20034.1218181818 5.3123176670113e-05
20322.4527272727 5.2009022270768e-05
20610.7836363636 5.09384828904422e-05
20899.1145454545 4.99091986421838e-05
21187.4454545455 4.89189704707892e-05
21475.7763636364 4.79657470399366e-05
21764.1072727273 4.70476128568648e-05
22052.4381818182 4.61627775024791e-05
22340.7690909091 4.5309565850438e-05
22629.1 4.44864091724374e-05
22917.4309090909 4.36918370387848e-05
23205.7618181818 4.2924469933743e-05
23494.0927272727 4.21830125141859e-05
23782.4236363636 4.14662474480781e-05
24070.7545454545 4.07730297762594e-05
24359.0854545455 4.0102281747154e-05
24647.4163636364 3.94529880794282e-05
24935.7472727273 3.88241916123906e-05
25224.0781818182 3.82149893081345e-05
25512.4090909091 3.76245285731505e-05
25800.74 3.70520038704407e-05
26089.0709090909 3.64966535960943e-05
26377.4018181818 3.59577571968865e-05
26665.7327272727 3.54346325077821e-05
26954.0636363636 3.49266332902929e-05
27242.3945454545 3.44331469544716e-05
27530.7254545455 3.39535924489844e-05
27819.0563636364 3.34874183051628e-05
28107.3872727273 3.30341008222689e-05
28395.7181818182 3.25931423823799e-05
28684.0490909091 3.21640698843685e-05
28972.38 3.17464332874039e-05
};
\addplot [very thick, purple11522131]
table {%
631.56 0.723756473452037
1034.24 0.102707773631961
1436.92 0.0310441009973273
1839.6 0.0133556201065377
2242.28 0.00703162574814445
2644.96 0.00421437975804864
3047.64 0.00276270932776156
3450.32 0.00193334751473953
3853 0.0014216582869403
4255.68 0.00108665573222923
4658.36 0.000856743046959926
5061.04 0.000692795292826335
5463.72 0.000572124237760758
5866.4 0.000480911543652854
6269.08 0.000410386978268575
6671.76 0.000354785370895648
7074.44 0.000310200551656981
7477.12 0.000273915292958019
7879.8 0.000243995209644804
8282.48 0.00021903475250242
8685.16 0.000197993842587664
9087.84 0.000180090161792612
9490.52 0.000164726541686889
9893.2 0.00015144102278217
10295.88 0.000139871877072866
10698.56 0.000129732702641482
11101.24 0.000120794420368653
11503.92 0.000112872078569759
11906.6 0.000105815057556823
12309.28 9.94997120432018e-05
12711.96 9.38237841206142e-05
13114.64 8.87021175715917e-05
13517.32 8.40633392802151e-05
13920 7.98472668030726e-05
14322.68 7.60028664705896e-05
14725.36 7.24866326524373e-05
15128.04 6.92612919615121e-05
15530.72 6.62947601613589e-05
15933.4 6.3559297080426e-05
16336.08 6.10308177778755e-05
16738.76 5.86883278388065e-05
17141.44 5.65134579069483e-05
17544.12 5.44900780322695e-05
17946.8 5.26039765791239e-05
18349.48 5.08425916395405e-05
18752.16 4.91947853680294e-05
19154.84 4.76506535761792e-05
19557.52 4.6201364428945e-05
19960.2 4.4839021267634e-05
20362.88 4.35565455207261e-05
20765.56 4.23475764082793e-05
21168.24 4.12063847409453e-05
21570.92 4.0127798592861e-05
21973.6 3.91071390136066e-05
22376.28 3.8140164257344e-05
22778.96 3.72230212619568e-05
23181.64 3.6352203319286e-05
23584.32 3.55245130484627e-05
23987 3.47370299251622e-05
24389.68 3.39870817360372e-05
24792.36 3.32722194242248e-05
25195.04 3.25901948722536e-05
25597.72 3.1938941235912e-05
26000.4 3.13165554989417e-05
26403.08 3.07212829657796e-05
26805.76 3.01515034494875e-05
27208.44 2.96057189457537e-05
27611.12 2.90825426124796e-05
28013.8 2.85806888987776e-05
28416.48 2.809896468796e-05
28819.16 2.7636261336803e-05
29221.84 2.7191547508561e-05
29624.52 2.67638627102278e-05
30027.2 2.63523114557703e-05
30429.88 2.59560579867202e-05
30832.56 2.55743214898849e-05
31235.24 2.52063717591752e-05
31637.92 2.48515252548357e-05
32040.6 2.45091415188351e-05
32443.28 2.41786199099381e-05
32845.96 2.38593966261394e-05
33248.64 2.35509419857832e-05
33651.32 2.32527579418752e-05
34054 2.29643758069005e-05
34456.68 2.26853541679133e-05
34859.36 2.24152769738398e-05
35262.04 2.21537517788414e-05
35664.72 2.19004081272796e-05
36067.4 2.16548960673174e-05
36470.08 2.14168847815116e-05
36872.76 2.11860613239377e-05
37275.44 2.09621294544212e-05
37678.12 2.07448085613899e-05
38080.8 2.05338326656832e-05
38483.48 2.03289494983985e-05
38886.16 2.01299196465141e-05
39288.84 1.99365157606207e-05
39691.52 1.9748521819622e-05
40094.2 1.95657324477408e-05
40496.88 1.9387952279595e-05
};
\addplot [very thick, indianred19152101]
table {%
869.92 0.641315748950197
1410.2701010101 0.0834554010422236
1950.6202020202 0.0238528311000232
2490.9703030303 0.00987228246274636
3031.3204040404 0.00505308361747521
3571.67050505051 0.00296462713429337
4112.02060606061 0.00191153669431589
4652.37070707071 0.00132030164606671
5192.72080808081 0.000960732672543621
5733.07090909091 0.000728135843811245
6273.42101010101 0.000570122478076883
6813.77111111111 0.000458424612217921
7354.12121212121 0.000376829563171414
7894.47131313131 0.000315558077766297
8434.82141414142 0.000268456437974417
8975.17151515152 0.00023151026750586
9515.52161616162 0.000202018236136744
10055.8717171717 0.000178112824058542
10596.2218181818 0.000158471984328711
11136.5719191919 0.000142139989629477
11676.922020202 0.000128412908542833
12217.2721212121 0.000116763519923212
12757.6222222222 0.000106790955485451
13297.9723232323 9.81862299469479e-05
13838.3224242424 9.07082058717734e-05
14378.6725252525 8.41665501043565e-05
14919.0226262626 7.84094608395439e-05
15459.3727272727 7.33147045583477e-05
15999.7228282828 6.87829847509076e-05
16540.0729292929 6.47329767033559e-05
17080.423030303 6.10975683111441e-05
17620.7731313131 5.7820984527144e-05
18161.1232323232 5.48565665528235e-05
18701.4733333333 5.21650412820097e-05
19241.8234343434 4.9713161443117e-05
19782.1735353535 4.74726286218945e-05
20322.5236363636 4.54192340154875e-05
20862.8737373737 4.35321681335099e-05
21403.2238383838 4.17934625944579e-05
21943.5739393939 4.0187535948762e-05
22483.924040404 3.87008219820596e-05
23024.2741414141 3.73214638365345e-05
23564.6242424242 3.60390609748989e-05
24104.9743434343 3.48444588154102e-05
24645.3244444444 3.37295730139369e-05
25185.6745454545 3.26872420252776e-05
25726.0246464646 3.17111028613985e-05
26266.3747474747 3.07954859681526e-05
26806.7248484848 2.99353259306375e-05
27347.074949495 2.91260853402877e-05
27887.4250505051 2.8363689651553e-05
28427.7751515152 2.76444712509191e-05
28968.1252525253 2.69651212778535e-05
29508.4753535354 2.63226479925618e-05
30048.8254545455 2.57143406921804e-05
30589.1755555556 2.51377383450823e-05
31129.5256565657 2.45906022502261e-05
31669.8757575758 2.40708921409654e-05
32210.2258585859 2.35767452453141e-05
32750.575959596 2.31064578911305e-05
33290.9260606061 2.26584693080589e-05
33831.2761616162 2.22313473307969e-05
34371.6262626263 2.18237757522402e-05
34911.9763636364 2.14345431119057e-05
35452.3264646465 2.10625327359568e-05
35992.6765656566 2.0706713871216e-05
36533.0266666667 2.03661337775604e-05
37073.3767676768 2.00399106617476e-05
37613.7268686869 1.97272273515454e-05
38154.076969697 1.94273256225493e-05
38694.4270707071 1.91395011015673e-05
39234.7771717172 1.88630986803301e-05
39775.1272727273 1.85975083817279e-05
40315.4773737374 1.83421616280635e-05
40855.8274747475 1.8096527867069e-05
41396.1775757576 1.78601115168571e-05
41936.5276767677 1.76324491956691e-05
42476.8777777778 1.74131072063371e-05
43017.2278787879 1.7201679248928e-05
43557.577979798 1.69977843381056e-05
44097.9280808081 1.68010649044344e-05
44638.2781818182 1.66111850612048e-05
45178.6282828283 1.64278290204039e-05
45718.9783838384 1.62506996432729e-05
46259.3284848485 1.60795171124669e-05
46799.6785858586 1.59140177142378e-05
47340.0286868687 1.57539527202845e-05
47880.3787878788 1.55990873600044e-05
48420.7288888889 1.54491998748447e-05
48961.078989899 1.53040806472955e-05
49501.4290909091 1.51635313978297e-05
50041.7791919192 1.50273644437632e-05
50582.1292929293 1.48954020146022e-05
51122.4793939394 1.47674756189849e-05
51662.8294949495 1.46434254587881e-05
52203.1795959596 1.45230998864043e-05
52743.5296969697 1.44063549015653e-05
53283.8797979798 1.42930536844327e-05
53824.2298989899 1.4183066161978e-05
54364.58 1.40762686049488e-05
};
\addplot [very thick, chocolate21910927]
table {%
1105.74 0.565215408216468
1792.7595959596 0.0627331416587966
2479.77919191919 0.0164427780087963
3166.79878787879 0.00644400098031338
3853.81838383838 0.00317804196842485
4540.83797979798 0.00181578854592101
5227.85757575757 0.00114822602374481
5914.87717171717 0.000781629052323457
6601.89676767677 0.000562551945108419
7288.91636363636 0.000422830807798551
7975.93595959596 0.000329009975937823
8662.95555555555 0.000263326947239662
9349.97515151515 0.000215733056026218
10036.9947474747 0.000180238006675446
10724.0143434343 0.000153110568144103
11411.0339393939 0.000131938251566154
12098.0535353535 0.000115110321530759
12785.0731313131 0.000101520908697014
13472.0927272727 9.03919559164958e-05
14159.1123232323 8.11640778924721e-05
14846.1319191919 7.3427290212816e-05
15533.1515151515 6.68758860454423e-05
16220.1711111111 6.1278351044289e-05
16907.1907070707 5.64568802499617e-05
17594.2103030303 5.22731656254263e-05
18281.2298989899 4.86183631906632e-05
18968.2494949495 4.54058983401694e-05
19655.2690909091 4.25662315354425e-05
20342.2886868687 4.00429993865197e-05
21029.3082828283 3.77901346942758e-05
21716.3278787879 3.57696926221435e-05
22403.3474747475 3.39501925240422e-05
23090.3670707071 3.2305340675897e-05
23777.3866666667 3.08130373937362e-05
24464.4062626263 2.9454598606688e-05
25151.4258585859 2.82141406669758e-05
25838.4454545455 2.70780905043966e-05
26525.465050505 2.6034792824376e-05
27212.4846464646 2.50741930231429e-05
27899.5042424242 2.41875796136697e-05
28586.5238383838 2.33673737488497e-05
29273.5434343434 2.26069562619941e-05
29960.563030303 2.1900524778895e-05
30647.5826262626 2.12429750753057e-05
31334.6022222222 2.06298020918109e-05
32021.6218181818 2.00570169710304e-05
32708.6414141414 1.9521077220437e-05
33395.661010101 1.90188276796881e-05
34082.6806060606 1.85474504228011e-05
34769.7002020202 1.81044220815561e-05
35456.7197979798 1.76874773588687e-05
36143.7393939394 1.72945777259415e-05
36830.758989899 1.69238844773189e-05
37517.7785858586 1.65737354630985e-05
38204.7981818182 1.6242624934907e-05
38891.8177777778 1.59291860375547e-05
39578.8373737374 1.56321755560264e-05
40265.856969697 1.53504605911041e-05
40952.8765656566 1.50830068892562e-05
41639.8961616161 1.48288685956041e-05
42326.9157575757 1.45871792345276e-05
43013.9353535353 1.43571437521988e-05
43700.9549494949 1.41380314801043e-05
44387.9745454545 1.39291698993402e-05
45074.9941414141 1.37299391028686e-05
45762.0137373737 1.35397668675528e-05
46449.0333333333 1.33581242601557e-05
47136.0529292929 1.31845217119412e-05
47823.0725252525 1.30185055054058e-05
48510.0921212121 1.28596546242218e-05
49197.1117171717 1.27075779239256e-05
49884.1313131313 1.25619115864031e-05
50571.1509090909 1.24223168259536e-05
51258.1705050505 1.22884778187844e-05
51945.1901010101 1.21600998312874e-05
52632.2096969697 1.20369075254784e-05
53319.2292929293 1.19186434225933e-05
54006.2488888889 1.18050665081094e-05
54693.2684848485 1.16959509634282e-05
55380.2880808081 1.15910850111721e-05
56067.3076767677 1.14902698625515e-05
56754.3272727273 1.13933187565558e-05
57441.3468686869 1.13000560818783e-05
58128.3664646464 1.12103165734828e-05
58815.386060606 1.11239445766038e-05
59502.4056565656 1.10407933717488e-05
60189.4252525252 1.09607245549579e-05
60876.4448484848 1.08836074681749e-05
61563.4644444444 1.08093186751256e-05
62250.484040404 1.0737741478564e-05
62937.5036363636 1.06687654751754e-05
63624.5232323232 1.06022861447902e-05
64311.5428282828 1.05382044709012e-05
64998.5624242424 1.04764265897636e-05
65685.582020202 1.04168634656324e-05
66372.6016161616 1.03594305899129e-05
67059.6212121212 1.03040477022225e-05
67746.6408080808 1.02506385315446e-05
68433.6604040404 1.01991305558229e-05
69120.68 1.0149454778501e-05
};
\addplot [very thick, saddlebrown1356716]
table {%
1406.64 0.714377421244587
2276.93535353535 0.0668587203291745
3147.23070707071 0.0159123915702076
4017.52606060606 0.00585711252703453
4887.82141414141 0.00276437157452962
5758.11676767677 0.00152922454573698
6628.41212121212 0.000943607294336271
7498.70747474748 0.000630253246342437
8369.00282828283 0.000446873887434088
9239.29818181818 0.000331915957962755
10109.5935353535 0.000255825096694617
10979.8888888889 0.000203198464256743
11850.1842424242 0.00016545960051945
12720.4795959596 0.000137565687341505
13590.7749494949 0.000116413228720606
14461.0703030303 0.000100016789639928
15331.3656565657 8.70631977035414e-05
16201.661010101 7.66584384001315e-05
17071.9563636364 6.81782486281828e-05
17942.2517171717 6.11768663193628e-05
18812.5470707071 5.53295981585747e-05
19682.8424242424 5.03956932242077e-05
20553.1377777778 4.61937625056659e-05
21423.4331313131 4.25851509225907e-05
22293.7284848485 3.94624680233409e-05
23164.0238383838 3.67415358474079e-05
24034.3191919192 3.43556439157034e-05
24904.6145454545 3.22513892826529e-05
25774.9098989899 3.03856231268635e-05
26645.2052525253 2.87231812825445e-05
27515.5006060606 2.7235177771742e-05
28385.795959596 2.58977077950604e-05
29256.0913131313 2.46908520212645e-05
30126.3866666667 2.35979050188589e-05
30996.682020202 2.26047721382576e-05
31866.9773737374 2.16994942028646e-05
32737.2727272727 2.08718700434021e-05
33607.5680808081 2.01131545670043e-05
34477.8634343434 1.94158156015813e-05
35348.1587878788 1.87733368165279e-05
36218.4541414141 1.81800570195843e-05
37088.7494949495 1.76310383635173e-05
37959.0448484848 1.71219576740508e-05
38829.3402020202 1.66490163803743e-05
39699.6355555556 1.62088654978837e-05
40569.9309090909 1.57985428563283e-05
41440.2262626263 1.54154203412631e-05
42310.5216161616 1.50571593637966e-05
43180.816969697 1.47216731234913e-05
44051.1123232323 1.44070945046925e-05
44921.4076767677 1.41117486645264e-05
45791.703030303 1.38341295442382e-05
46661.9983838384 1.35728796742347e-05
47532.2937373737 1.33267727546276e-05
48402.5890909091 1.3094698583039e-05
49272.8844444444 1.28756499743821e-05
50143.1797979798 1.26687113767207e-05
51013.4751515152 1.24730489358981e-05
51883.7705050505 1.22879018014841e-05
52754.0658585859 1.21125744994596e-05
53624.3612121212 1.19464302242197e-05
54494.6565656566 1.17888849250429e-05
55364.9519191919 1.16394020809443e-05
56235.2472727273 1.14974880735376e-05
57105.5426262626 1.13626880806731e-05
57975.837979798 1.12345824246887e-05
58846.1333333333 1.11127833184334e-05
59716.4286868687 1.09969319601076e-05
60586.724040404 1.08866959346594e-05
61457.0193939394 1.07817668851583e-05
62327.3147474748 1.06818584224172e-05
63197.6101010101 1.0586704245282e-05
64067.9054545455 1.04960564475513e-05
64938.2008080808 1.04096839905454e-05
65808.4961616162 1.03273713229642e-05
66678.7915151515 1.02489171319382e-05
67549.0868686869 1.0174133211136e-05
68419.3822222222 1.01028434334881e-05
69289.6775757576 1.00348828175589e-05
70159.9729292929 9.97009667787824e-06
71030.2682828283 9.9083398506649e-06
71900.5636363636 9.84947598734427e-06
72770.858989899 9.79337690912138e-06
73641.1543434343 9.7399220166121e-06
74511.4496969697 9.68899774919699e-06
75381.7450505051 9.64049708933746e-06
76252.0404040404 9.59431910760129e-06
77122.3357575758 9.55036854459788e-06
77992.6311111111 9.50855542641289e-06
78862.9264646465 9.46879471049137e-06
79733.2218181818 9.43100595922459e-06
80603.5171717172 9.39511303877034e-06
81473.8125252525 9.36104384089029e-06
82344.1078787879 9.3287300257958e-06
83214.4032323232 9.29810678419841e-06
84084.6985858586 9.26911261692785e-06
84954.9939393939 9.24168913064134e-06
85825.2892929293 9.2157808482828e-06
86695.5846464646 9.19133503307931e-06
87565.88 9.16830152497056e-06
};
\addplot [very thick, black18]
table {%
1648.2 0.531641144110067
2695.43636363636 0.0519913141962213
3742.67272727273 0.0128571649999296
4789.90909090909 0.00487953549601193
5837.14545454545 0.00236059630516175
6884.38181818182 0.00133273249257079
7931.61818181818 0.000836557497292362
8978.85454545455 0.000566977478658349
10026.0909090909 0.000407124694347868
11073.3272727273 0.000305757254483162
12120.5636363636 0.000237978774093704
13167.8 0.00019067688211975
14215.0363636364 0.000156481367116471
15262.2727272727 0.000131021643731077
16309.5090909091 0.000111587049539147
17356.7454545455 9.64311609722713e-05
18403.9818181818 8.43913629021722e-05
19451.2181818182 7.46713829634051e-05
20498.4545454545 6.67121121149065e-05
21545.6909090909 6.01122452100421e-05
22592.9272727273 5.45780596474055e-05
23640.1636363636 4.98907843716507e-05
24687.4 4.58848920023658e-05
25734.6363636364 4.2433347817389e-05
26781.8727272727 3.94373918075414e-05
27829.1090909091 3.68193362186055e-05
28876.3454545455 3.45174071991406e-05
29923.5818181818 3.24819961549532e-05
30970.8181818182 3.06728987879211e-05
32018.0545454545 2.90572562829286e-05
33065.2909090909 2.76080024115105e-05
34112.5272727273 2.63026797322811e-05
35159.7636363636 2.51225282049771e-05
36207 2.40517770402784e-05
37254.2363636364 2.30770897090356e-05
38301.4727272727 2.21871254655824e-05
39348.7090909091 2.13721902940943e-05
40395.9454545455 2.0623957057893e-05
41443.1818181818 1.9935239623687e-05
42490.4181818182 1.92998093948104e-05
43537.6545454545 1.87122453984768e-05
44584.8909090909 1.81678110961947e-05
45632.1272727273 1.76623526101318e-05
46679.3636363636 1.71922142139577e-05
47726.6 1.67541678198082e-05
48773.8363636364 1.63453538724696e-05
49821.0727272727 1.5963231588138e-05
50868.3090909091 1.56055368852355e-05
51915.5454545455 1.52702466763473e-05
52962.7818181818 1.49555484438992e-05
54010.0181818182 1.46598142232375e-05
55057.2545454545 1.43815782770095e-05
56104.4909090909 1.41195178730672e-05
57151.7272727273 1.38724366814218e-05
58198.9636363636 1.3639250389278e-05
59246.2 1.34189742010017e-05
60293.4363636364 1.32107119451844e-05
61340.6727272727 1.30136465562535e-05
62387.9090909091 1.28270317353119e-05
63435.1454545455 1.26501846256106e-05
64482.3818181818 1.24824793634998e-05
65529.6181818182 1.23233413868472e-05
66576.8545454546 1.21722424005472e-05
67624.0909090909 1.20286959134866e-05
68671.3272727273 1.18922532737217e-05
69718.5636363636 1.17625001390288e-05
70765.8 1.1639053328799e-05
71813.0363636364 1.15215580106843e-05
72860.2727272727 1.14096851817369e-05
73907.5090909091 1.13031294091528e-05
74954.7454545455 1.12016068003353e-05
76001.9818181818 1.1104853175917e-05
77049.2181818182 1.10126224227554e-05
78096.4545454545 1.09246850068054e-05
79143.6909090909 1.08408266282796e-05
80190.9272727273 1.07608470036568e-05
81238.1636363636 1.06845587609633e-05
82285.4 1.0611786436378e-05
83332.6363636364 1.05423655616056e-05
84379.8727272727 1.04761418327015e-05
85427.1090909091 1.04129703520853e-05
86474.3454545455 1.03527149364261e-05
87521.5818181818 1.02952474838877e-05
88568.8181818182 1.0240447394954e-05
89616.0545454545 1.01882010416661e-05
90663.2909090909 1.01384012806774e-05
91710.5272727273 1.0090947006003e-05
92757.7636363636 1.00457427377874e-05
93805 1.0002698243783e-05
94852.2363636364 9.9617281905822e-06
95899.4727272727 9.92275182193411e-06
96946.7090909091 9.88569266175347e-06
97993.9454545455 9.85047823966155e-06
99041.1818181818 9.81703983710824e-06
100088.418181818 9.7853122523195e-06
101135.654545455 9.75523358247516e-06
102182.890909091 9.72674502167978e-06
103230.127272727 9.69979067341679e-06
104277.363636364 9.67431737630384e-06
105324.6 9.65027454207259e-06
};
\addplot [draw=yellowgreen18420623, fill=yellowgreen18420623, mark=x, very thick, mark size=2.5pt, only marks]
table{%
x  y
316 0.350877452858023
1264 0.0477626963903647
5056 0.0047454831389641
20224 0.000403666290509671
80896 2.04471304559679e-05
};
\addplot [draw=royalblue28108204, fill=royalblue28108204, mark=x, only marks]
table{%
x  y
700 0.266806992180495
2800 0.0272139058959793
11200 0.00221646713515179
44800 0.000166920961358588
};
\addplot [draw=purple11522131, fill=purple11522131, mark=x, only marks]
table{%
x  y
1236 0.232665775699266
4944 0.018089408041855
19776 0.0011680504235253
79104 7.93395137461677e-05
};
\addplot [draw=indianred19152101, fill=indianred19152101, mark=x, only marks]
table{%
x  y
1940 0.227894739041533
7760 0.0194400262060056
31040 0.000840376368884408
};
\addplot [draw=chocolate21910927, fill=chocolate21910927, mark=x, only marks]
table{%
x  y
2756 0.209280625260255
11024 0.0131613922823717
44096 0.000594500495624545
};
\addplot [draw=saddlebrown1356716, fill=saddlebrown1356716, mark=x, only marks]
table{%
x  y
3832 0.216368351287466
15328 0.0148287655424899
61312 0.000432019850387497
};
\addplot [draw=black18, fill=black18, mark=x, only marks]
table{%
x  y
4968 0.194861622301456
19872 0.0121077143873276
79488 0.000340672697534887
};
