# Supplementary material for: Swarm Reinforcement Learning For Adaptive Mesh Refinement
Source: arXiv:2304.00818 source file (2023-10-09)
Supplement: Supplementary file 20 [file group_generalization_runtime_2.tex]

\nextgroupplot[
ylabel shift = -0.2cm,
clip marker paths=true,
width=0.52\textwidth,
height=5.5cm,
title style={yshift=-0.2cm},
scaled x ticks=false,
legend cell align={left},
legend style={
  fill opacity=0.8,
  draw opacity=1,
  text opacity=1,
  at={(0.97,0.03)},
  anchor=south east,
  draw=lightgray204
},
log basis x={10},
log basis y={10},
tick align=outside,
tick pos=left,
x grid style={darkgray176},
xlabel={Number of Elements},
xmajorgrids,
xminorticks=true,
xmin=146.94548582313, xmax=165138.791872846,
xmode=log,
xtick style={color=black},
xtick={10,
100,200,500,
1000,2000,5000, 
10000,20000,50000, 
100000,200000,500000,
1000000,10000000},
xticklabels={
  \(\displaystyle {10^{1}}\),
  \(\displaystyle {10^{2}}\),
  \empty,
  \empty,
  \(\displaystyle {10^{3}}\),
  \empty,
  \empty,
  \(\displaystyle {10^{4}}\),
  \empty,
  \empty,
  \(\displaystyle {10^{5}}\),
  \empty,
  \empty,
  \(\displaystyle {10^{6}}\),
  \(\displaystyle {10^{7}}\)
},
y grid style={darkgray176},
ylabel={Time \(\displaystyle [s]\)},
ymajorgrids,
ymin=0.025, ymax=130.0,
ymode=log,
ytick style={color=black},
ytick={0.03, 0.1, 0.3, 1, 3, 10, 30, 100, 300},
yticklabels={
  \(\displaystyle {0.03}\),
  \(\displaystyle {0.1}\),
  \(\displaystyle {0.3}\),
  \(\displaystyle {1}\),
  \(\displaystyle {3}\),
  \(\displaystyle {10}\),
  \(\displaystyle {30}\),
  \(\displaystyle {100}\),
  \(\displaystyle {300}\),
},
]
\addplot [
  draw=yellowgreen18420623,
  fill=yellowgreen18420623,
  forget plot,
  mark=*, mark size=1,
  only marks,
  draw opacity=0,
 fill opacity=0.5
]
table{%
x  y
202.22 0.053636736869812
210.1 0.0573659467697144
211.48 0.0549483156204224
222.92 0.0597615814208984
234.74 0.0608407402038574
256.28 0.0578651809692383
259.22 0.0635121774673462
261.68 0.0633667421340942
263 0.0639116477966309
282.98 0.0644068145751953
294.36 0.0640381622314453
329.1 0.0631571578979492
331.3 0.0645194625854492
378.22 0.0665956974029541
383.08 0.0668761968612671
399.78 0.0654444742202759
411.32 0.0665652847290039
454.7 0.0709421825408936
589.22 0.0781143379211426
753.28 0.0787068223953247
757.24 0.0939243745803833
778.26 0.0837820243835449
850.28 0.0975303030014038
868.44 0.0921848964691162
1131.74 0.105889449119568
1225.66 0.108700079917908
1286.9 0.117055883407593
1299.32 0.115205421447754
1306.84 0.114628624916077
1341.6 0.114868803024292
1409.08 0.113009166717529
1445.34 0.115776767730713
1578.46 0.127250208854675
1798.36 0.125349459648132
1861.66 0.135553851127625
1891 0.134897961616516
1912.98 0.136924138069153
1966.86 0.130827040672302
2192.24 0.137252526283264
2307.24 0.155854601860046
2432 0.160648856163025
2606.92 0.166000714302063
2651.8 0.171999988555908
2732.14 0.177660126686096
2851.42 0.188421974182129
2908.06 0.156851816177368
3008.34 0.150284204483032
3115.68 0.177828679084778
3200.1 0.181715927124023
3324.12 0.185469427108765
3332.44 0.175553765296936
3401.7 0.186602010726929
3460.44 0.16089789390564
3466.72 0.168340153694153
3558.72 0.161202158927917
3616.88 0.187781276702881
3851.28 0.213588242530823
4375.32 0.250290460586548
4480.44 0.220999851226807
4865.72 0.253379702568054
4880.76 0.215679936408997
5024.04 0.233472094535828
5099.36 0.208133087158203
5184.38 0.19450822353363
5429.82 0.203638672828674
5544.86 0.228255319595337
5598.82 0.237999429702759
5607.34 0.201364970207214
5652.38 0.240973305702209
5911.78 0.185391044616699
6354.42 0.247724995613098
6540.36 0.25549729347229
6716.56 0.234649543762207
6956.54 0.23590950012207
7023.42 0.291095461845398
7750.72 0.300478177070618
7820.7 0.26608766078949
8352.52 0.305391702651978
8638.7 0.258934350013733
8647.16 0.299160981178284
8815.24 0.337037835121155
8836.14 0.276106781959534
8919.88 0.312163662910461
9140 0.309248647689819
9297.04 0.307952795028686
9433.2 0.353137555122375
10090.58 0.353787231445312
10116.9 0.338459496498108
12183.98 0.420777702331543
12588.02 0.483224387168884
13812.78 0.483576741218567
14987.2 0.528575921058655
15188.84 0.538984618186951
15397.08 0.52943078994751
15593.5 0.538594298362732
17237.88 0.532076959609985
18975.72 0.634843673706055
19384.18 0.697243175506592
20097.06 0.663194346427918
20206.68 0.667125792503357
};
\addplot [
  draw=royalblue28108204,
  fill=royalblue28108204,
  forget plot,
  mark=*, mark size=1,
  only marks,
  draw opacity=0,
 fill opacity=0.5
]
table{%
x  y
402.52 0.0704682540893555
435.36 0.0718180179595947
441.5 0.0709519672393799
454.88 0.0757018709182739
458.98 0.0716204929351807
513.54 0.0755746936798096
547.16 0.0777035331726074
567.14 0.0795207071304321
571.72 0.0847738981246948
616.58 0.0867928600311279
692.5 0.0887960815429688
717.66 0.0929835033416748
739.34 0.0951868200302124
766.68 0.0942276287078857
767.5 0.0911421966552734
782.14 0.0931526899337769
884.96 0.102117552757263
1107.12 0.110220561027527
1190.08 0.116753907203674
1242.02 0.117197642326355
1256.92 0.122020192146301
1317.8 0.12391152381897
1359.32 0.126328210830688
1447.18 0.12678373336792
1699.44 0.150327677726746
1755.96 0.151166644096375
1861.94 0.150204491615295
1931.34 0.154651556015015
1939.54 0.156170020103455
1944.36 0.160857672691345
2016.68 0.156384253501892
2034.64 0.171256709098816
2297.12 0.183210835456848
2343.44 0.16874752998352
2551.26 0.193163390159607
2618.32 0.190509567260742
2666.72 0.177434611320496
2682.3 0.191848640441895
2779.6 0.182764043807983
3210.82 0.21693549156189
3318.6 0.244499821662903
3440.02 0.228876752853394
3475.68 0.213424940109253
3661.06 0.204384965896606
3930.9 0.234412961006165
3975.9 0.249577736854553
3997.82 0.221656250953674
4069.44 0.24421772480011
4104 0.236070618629456
4109.98 0.274984354972839
4183.5 0.221172475814819
4209.7 0.218159804344177
4461.84 0.250472993850708
4651.54 0.254021744728088
4665.94 0.271183199882507
4671.66 0.245224094390869
4717.24 0.311787314414978
5681.54 0.315002088546753
6018.54 0.346827688217163
6136.22 0.266628103256226
6230.7 0.27270911693573
6406.58 0.297216200828552
6568.4 0.341003947257996
6596.16 0.363424401283264
6830.88 0.283860802650452
6876.7 0.261333980560303
6883.72 0.39197286605835
7095.1 0.341534910202026
7221.2 0.373389911651611
7472.62 0.37386700630188
8112.92 0.38486686706543
8220.88 0.390343542098999
8327.02 0.362688031196594
8672.74 0.361634330749512
9022.2 0.438300404548645
9664.3 0.402882499694824
9922.62 0.46316755771637
10617.46 0.470893888473511
10722.56 0.40901593208313
10880.14 0.461041975021362
10955.2 0.427262892723083
11097.1 0.480788474082947
11299.14 0.521810297966003
11453.32 0.462012667655945
11619.8 0.486855983734131
12101.58 0.508190550804138
12875.68 0.50767062664032
13022.34 0.54270161151886
15679.16 0.636257371902466
19206.54 0.902356886863709
20352.3 0.916546902656555
21554.9 0.985163588523865
21689.76 0.978785948753357
21852.42 0.990136098861694
22373.38 1.00491415023804
23858.44 0.962296242713928
27510.76 1.15191871643066
27721.68 1.14290676593781
27956.58 1.19390149116516
29022.26 1.18539229869843
};
\addplot [draw=purple11522131, fill=purple11522131, forget plot, mark=*, mark size=1, only marks, draw opacity=0,
 fill opacity=0.5]
table{%
x  y
600.42 0.085165581703186
639.14 0.0935827732086182
667.28 0.089842267036438
697.88 0.0970381784439087
701.92 0.095571231842041
751.24 0.0941839981079102
805.9 0.103412728309631
849.02 0.108593473434448
865.8 0.110978798866272
914.58 0.109401416778564
996.8 0.112434773445129
1052.56 0.115875763893127
1067.14 0.117640337944031
1083.16 0.125228776931763
1092.86 0.11734992980957
1111.02 0.115926699638367
1236.98 0.12476300239563
1570.24 0.15696918964386
1786.5 0.160687956809998
1843.52 0.150521597862244
1882.24 0.166164846420288
1905.02 0.177295737266541
1948.98 0.160236783027649
2040.5 0.188110399246216
2386.34 0.197156252861023
2400.94 0.202372107505798
2608.76 0.215948972702026
2703.56 0.20698205947876
2705.88 0.215693435668945
2760.26 0.210125460624695
2770.66 0.227339124679565
2835.12 0.228434405326843
3146.92 0.222817587852478
3230.02 0.250319395065308
3421.98 0.252686681747437
3499.34 0.251162486076355
3547.6 0.233490991592407
3582.54 0.239266738891602
3665.86 0.26105845451355
4209.44 0.286132197380066
4434.98 0.301263146400452
4537.9 0.327275929450989
4559.76 0.271038837432861
4746.48 0.33886739730835
4902.96 0.310476279258728
4923.56 0.306554093360901
4951.14 0.329138889312744
5026.5 0.284808759689331
5055.3 0.309725642204285
5088.88 0.29528920173645
5167.06 0.335854868888855
5515.08 0.327336111068726
5710.42 0.371356496810913
5947.92 0.33724889755249
6113.7 0.416377348899841
6303.68 0.405374369621277
7056.22 0.34123731136322
7147.78 0.484664649963379
7189.42 0.42329692363739
7385.2 0.370883951187134
7860.08 0.401361017227173
7958.86 0.352347674369812
8165.58 0.575175800323486
8378.3 0.404710516929626
8865.08 0.50550431728363
8915.78 0.53054750919342
9246.24 0.500489664077759
9554.68 0.585963597297668
9556.38 0.540787086486816
9968.5 0.5517755651474
10504.68 0.528091073036194
10556.72 0.569596943855286
10720.76 0.569930806159973
10990 0.52824022769928
11810.68 0.634174847602844
12022.44 0.574160766601562
12878.46 0.671161069869995
13368.4 0.599211406707764
13526.64 0.689761071205139
13602.84 0.626406803131104
13844.14 0.669623198509216
14116.98 0.694125514030457
14457.94 0.664746413230896
14459.22 0.686324081420898
14779.9 0.761429681777954
15502.38 0.776616516113281
16191.92 0.754957728385925
16521.5 0.785174508094788
19998.18 0.936150712966919
28075.68 1.50594533920288
29188.9 1.49323241710663
30376.78 1.5781475019455
30421.24 1.53149908065796
30932.02 1.56533050537109
31528.98 1.65433809757233
32972.32 1.55786964893341
38016.98 1.9149742937088
38460.18 1.82746377468109
39342.9 1.94984057426453
40363.1 1.9153574180603
};
\addplot [
  draw=indianred19152101,
  fill=indianred19152101,
  forget plot,
  mark=*, mark size=1,
  only marks,
  draw opacity=0,
 fill opacity=0.5
]
table{%
x  y
861.9 0.108184342384338
862.22 0.107191033363342
912.58 0.110956125259399
951.94 0.120313782691956
974.06 0.115554089546204
1015.76 0.11558322429657
1068.6 0.119076352119446
1165.36 0.122906165122986
1190.2 0.1348948097229
1190.44 0.129477825164795
1281.88 0.133990597724915
1375.94 0.139886703491211
1379 0.140690612792969
1385.26 0.135749049186707
1399.44 0.142664909362793
1493.18 0.160684714317322
1587.02 0.157379589080811
2059.36 0.186476120948792
2218.42 0.192800674438477
2412.08 0.209354462623596
2417.2 0.208486113548279
2641.44 0.225485863685608
2673.44 0.208835415840149
2796.92 0.239797868728638
3032.68 0.258871083259583
3193.76 0.275303311347961
3394.06 0.27266592502594
3457.64 0.272995128631592
3589.24 0.294171657562256
3591.6 0.282163701057434
3707.98 0.292550144195557
3763.62 0.312000827789307
4000.24 0.29272253036499
4338.62 0.335978136062622
4380.32 0.33245059967041
4436.3 0.314218010902405
4442.38 0.30621395111084
4506.38 0.330484557151794
4795.22 0.353172445297241
5281.78 0.380964078903198
5564.32 0.396198787689209
5655.12 0.362943472862244
5671.32 0.43681881904602
5820.36 0.399710583686829
6041.28 0.429389314651489
6047.26 0.370688920021057
6052.9 0.405657601356506
6110.48 0.387994585037231
6209.26 0.412103018760681
6226.18 0.473917193412781
6701.4 0.429610834121704
6771.56 0.477750463485718
6791.84 0.435090508460999
7297.1 0.452218580245972
8013.42 0.509006748199463
8060.06 0.43546763420105
8692.92 0.614646916389465
8723.7 0.481887702941895
8858.22 0.553050780296326
9410.38 0.521215209960938
9516.14 0.474068460464478
9897.78 0.5106720495224
10096.24 0.705399374961853
11082.44 0.747259349822998
11768.74 0.728093643188477
11818.82 0.76425461769104
11993.98 0.730766706466675
12472.66 0.776315250396729
12750.9 0.826050996780396
13020.62 0.788284530639648
13378.96 0.747961182594299
13528.18 0.818504133224487
13709.24 0.803660759925842
13944.4 0.744210677146912
14958.58 0.878139200210571
15036.26 0.811384930610657
16353.9 0.946326122283936
16785.22 0.846302676200867
16972.96 0.96594286441803
17053.96 0.901380863189697
17392.98 0.93512845993042
17521.82 0.959441375732422
17950.66 0.927578973770142
18149.9 0.972475070953369
18766.74 1.07321537017822
19397.42 1.03834498405457
20197.92 1.08874293804169
20290.02 1.08006652355194
24633.88 1.34318685531616
39515.5 2.36322745323181
40211.82 2.33583311080933
41643.06 2.42913973808289
41705.62 2.42740437984467
42552.36 2.4445161151886
43514.44 2.53423924922943
44460.04 2.44505354404449
50246.86 2.77670222759247
51688.32 2.87028216838837
53317.06 3.12210227966309
53705.48 2.89686496734619
};
\addplot [
  draw=chocolate21910927,
  fill=chocolate21910927,
  forget plot,
  mark=*, mark size=1,
  only marks,
  draw opacity=0,
 fill opacity=0.5
]
table{%
x  y
1090.24 0.143595151901245
1099.78 0.140095963478088
1191.24 0.132979278564453
1224.52 0.146123094558716
1247.54 0.143194661140442
1316.9 0.15933895111084
1375.46 0.159825925827026
1496.78 0.16682065486908
1513.08 0.16269567489624
1570.46 0.173221073150635
1598.2 0.175653991699219
1702.24 0.174667310714722
1715.78 0.17043740272522
1729.8 0.177181663513184
1762.9 0.180541043281555
1913.72 0.197804841995239
2049.46 0.194874272346497
2596.06 0.249711632728577
2611.66 0.224832406044006
3229.22 0.288589153289795
3231.34 0.290303425788879
3520.82 0.311937699317932
3536.02 0.285612807273865
3743.76 0.339476351737976
3868.68 0.326106905937195
4118.22 0.352856020927429
4338.2 0.370033268928528
4357.04 0.35416663646698
4601.92 0.374425463676453
4631.32 0.405805649757385
4780.9 0.399164042472839
4874.28 0.398734712600708
5017.18 0.380642199516296
5460.98 0.428154988288879
5469.1 0.436597027778625
5475.98 0.42110246181488
5566.84 0.436858410835266
5599.56 0.422896099090576
6029.88 0.45968141078949
6584.04 0.485084381103516
6776.72 0.487227602005005
6828.48 0.478990573883057
6875.44 0.50373167514801
7031.82 0.536423926353455
7175.32 0.479123954772949
7221.44 0.477468495368958
7302.4 0.531308264732361
7390.66 0.516145505905151
7531.34 0.527229170799255
7834.72 0.585216717720032
7954.68 0.574217858314514
7976.78 0.583290872573853
8636.68 0.620740523338318
8640.68 0.567761316299438
9120.28 0.52897301197052
9912.08 0.69051164150238
10176.94 0.700615453720093
10703.34 0.703838796615601
11171.72 0.624676485061646
11222.82 0.683419528007507
11617.34 0.710641374588013
11715.04 0.864341735839844
13513.82 1.07220798969269
14439.04 1.09320982456207
15033.46 0.985084390640259
15039.5 1.00042773246765
15121.66 1.03716609954834
15791.72 1.05079977989197
16265.64 1.20451471805573
16424.1 1.07397742271423
16573.26 1.01890222549438
16922.48 1.12373174190521
16969.86 1.07841244697571
17041.86 1.00317525863647
18370.62 1.09383964538574
18464.24 1.20206883907318
20131.4 1.25602327346802
20573.22 1.15042270183563
20812.3 1.27838348865509
20857.48 1.28684429168701
21195.72 1.25525975227356
21285.88 1.28171223163605
21571.54 1.22499960899353
22172.6 1.29834204673767
23317.76 1.44783720970154
23605.58 1.40891050338745
24371.88 1.41618738174438
24614.46 1.41069275856018
29784.86 1.73327664375305
52296.78 3.38681083679199
53396.56 3.41018114089966
54697.88 3.56349792003632
54733.82 3.40508412361145
55870.68 3.55262710571289
57115.5 3.54657684803009
57755.98 3.51783360004425
64372.74 3.93015883922577
66295.06 3.93671598911285
68357.3 4.06547833919525
69118.12 4.18662621974945
};
\addplot [
  draw=saddlebrown1356716,
  fill=saddlebrown1356716,
  forget plot,
  mark=*, mark size=1,
  only marks,
  draw opacity=0,
 fill opacity=0.5
]
table{%
x  y
1400.16 0.1538898229599
1403.9 0.160232944488525
1495.12 0.163474183082581
1556.66 0.171564054489136
1563.82 0.164247465133667
1626.46 0.170481758117676
1702.6 0.176998739242554
1871.32 0.185873594284058
1899.64 0.186020059585571
1933.68 0.197126898765564
1983.06 0.202471170425415
2022.46 0.19611129283905
2070.96 0.193710193634033
2098.06 0.20398859500885
2184.74 0.212477560043335
2357.68 0.23214882850647
2435.2 0.23908344745636
3123.12 0.286430530548096
3287.28 0.306913251876831
4032 0.367185373306274
4098.44 0.359481892585754
4646.02 0.399083957672119
4663.08 0.419335012435913
4733.78 0.361203517913818
4816.62 0.42745756149292
5234.8 0.477194757461548
5453.22 0.457808928489685
5493.22 0.468798570632935
5798.7 0.514243741035461
5825.88 0.503400650024414
6127.56 0.530479936599731
6135.74 0.55153555393219
6254.64 0.488855233192444
6686.42 0.556084842681885
6755.68 0.538998341560364
6769.02 0.541995768547058
6967.72 0.538021955490112
7099.72 0.561435384750366
7590.78 0.632289905548096
8040.12 0.640460720062256
8127.18 0.606278223991394
8140.04 0.607664017677307
8382.68 0.661746411323547
8477.7 0.615292420387268
8562.14 0.624448246955872
8587.72 0.689075345993042
8634.02 0.676105446815491
8877.18 0.683654680252075
8995.6 0.693898873329163
9364.06 0.724628558158875
9534.18 0.709573903083801
9786.14 0.78679780960083
10364.98 0.752350115776062
10424.5 0.664753584861755
10583.12 0.789841837882996
11744.96 0.845769634246826
11985.84 0.937027869224548
12643.9 0.912307658195496
12993.08 0.865896482467651
13037.58 0.825706872940064
13442.94 0.855752973556519
15542.9 1.21935066699982
17708.6 1.45178325653076
18535.32 1.51013807296753
19192.76 1.41348478794098
19308.4 1.42291082859039
19394.18 1.45163331508636
20022.66 1.4987380361557
20754.86 1.54962675094604
20758.3 1.61330208301544
20788.24 1.43613259792328
21246.2 1.51110463619232
21307.38 1.40606046199799
21512.24 1.58159868240356
22408.84 1.56492406845093
22712.14 1.52206473827362
24799.38 1.71170454025269
25142.72 1.60816630363464
25461.88 1.71560124874115
25611.76 1.63173687934875
25885.9 1.73907833099365
25913.72 1.7193154001236
26102.32 1.65250336170197
27118.14 1.76055206298828
28556.94 1.95691677570343
28684.76 1.87657487392426
29287.44 1.90719216346741
29709.26 1.87525992393494
35544.92 2.23102762699127
69481.6 4.97520615100861
70223.38 4.84426027774811
71680.74 5.03092016220093
71848.72 4.91191035270691
73062.08 5.05334676742554
74313.6 5.17291311264038
75161.58 5.00415619850159
81922.24 5.49320433139801
84668.8 5.7080686378479
86805.3 5.63033801555634
87953.68 5.85072546958923
};
\addplot [draw=black18, fill=black18, forget plot, mark=*, mark size=1, only marks, draw opacity=0,
 fill opacity=0.5]
table{%
x  y
1675.74 0.191374959945679
1724.32 0.202126398086548
1825.04 0.190372681617737
1914.48 0.198753666877747
1917.14 0.207651300430298
2006.3 0.228827199935913
2078.1 0.2261328125
2314.5 0.233203821182251
2352.94 0.245575580596924
2385.5 0.242480430603027
2475.38 0.241179189682007
2524.56 0.259366641044617
2541.3 0.236830811500549
2614.06 0.252888526916504
2690.88 0.26266505241394
2973.82 0.287987542152405
3070.54 0.288032975196838
3837.96 0.335071568489075
4029.62 0.380665712356567
4992.08 0.44663058757782
5079.88 0.445504455566406
5663.98 0.493543648719788
5806.76 0.495180168151855
6010.88 0.44931104183197
6040.34 0.538154320716858
6462.24 0.567782893180847
6587.5 0.552133297920227
6692.32 0.579642043113708
7033.06 0.62339367389679
7072.54 0.591950449943543
7360.18 0.616178855895996
7442.58 0.624505171775818
7449.02 0.588607506752014
7920.18 0.650811514854431
7976.7 0.634398765563965
8078.9 0.649757933616638
8305.54 0.649754447937012
8598.8 0.685247349739075
9152.44 0.744018068313599
9393.66 0.703831324577332
9512.34 0.744160170555115
9603.58 0.759280123710632
9789.42 0.717989106178284
9937 0.746668920516968
10000.92 0.773078155517578
10138.4 0.791556534767151
10197.56 0.81877947807312
10464.16 0.792571501731873
10653.34 0.81092022895813
10821.82 0.843865327835083
11250.72 0.890245490074158
11714.72 0.770893902778625
11886.26 0.924045023918152
11953.56 0.877901320457459
13078.14 1.00694804191589
13417.72 0.959435048103332
14170.68 1.05376270771027
14970.9 1.0499155330658
14982.14 1.10246894836426
15465.92 1.04082404613495
15605.6 1.12307391643524
19464.8 1.52459632396698
22348.46 1.79398089408875
23149.28 1.8698184633255
23223.3 1.7032003068924
23864.82 1.85183483123779
23993.4 1.80451635360718
24621.54 1.80800370693207
25363.24 1.79242597103119
25369.48 1.96604620456696
25460.64 1.84108342170715
25601.9 1.80687724113464
25612.94 1.73021662712097
25772.98 2.02715044021606
26872.8 1.86641075134277
27194.34 1.8683313703537
29686.62 2.07109240055084
30043.56 1.9568909740448
30217.76 2.05113118648529
30539.34 2.03469288349152
30559.98 1.96408385753632
30743.14 2.09446365356445
30900.1 2.05394234657288
32320.5 2.12482105731964
34060.9 2.26171833992004
34212.8 2.3934575176239
34314.12 2.28871839523315
35233.44 2.26250495910645
41650.7 2.78562867641449
87547.36 6.22760702133179
88577.76 5.90024886608124
89665.98 6.2541726064682
89932.44 6.1915953874588
91374.32 6.30757035255432
93013.42 6.42520016670227
93468.4 6.24463422775269
100557.26 6.6682722234726
104257.46 7.08209228992462
105880.52 6.85912087917328
108230.36 7.15615629673004
};
\addplot [very thick, yellowgreen18420623]
table {%
202.22 0.0749113817215524
404.285252525253 0.0805774326246075
606.350505050505 0.086251610099681
808.415757575758 0.091933914146773
1010.48101010101 0.0976243447658833
1212.54626262626 0.103322901957012
1414.61151515152 0.109029585720159
1616.67676767677 0.114744396055325
1818.74202020202 0.120467332962509
2020.80727272727 0.126198396441711
2222.87252525253 0.131937586492932
2424.93777777778 0.137684903116171
2627.00303030303 0.143440346311429
2829.06828282828 0.149203916078705
3031.13353535353 0.154975612417999
3233.19878787879 0.160755435329312
3435.26404040404 0.166543384812643
3637.32929292929 0.172339460867993
3839.39454545455 0.178143663495361
4041.4597979798 0.183955992694747
4243.52505050505 0.189776448466152
4445.5903030303 0.195605030809576
4647.65555555556 0.201441739725017
4849.72080808081 0.207286575212477
5051.78606060606 0.213139537271956
5253.85131313131 0.219000625903453
5455.91656565657 0.224869841106968
5657.98181818182 0.230747182882502
5860.04707070707 0.236632651230054
6062.11232323232 0.242526246149624
6264.17757575758 0.248427967641213
6466.24282828283 0.254337815704821
6668.30808080808 0.260255790340447
6870.37333333333 0.266181891548091
7072.43858585859 0.272116119327753
7274.50383838384 0.278058473679434
7476.56909090909 0.284008954603134
7678.63434343434 0.289967562098851
7880.6995959596 0.295934296166588
8082.76484848485 0.301909156806342
8284.8301010101 0.307892144018115
8486.89535353535 0.313883257801907
8688.9606060606 0.319882498157716
8891.02585858586 0.325889865085545
9093.09111111111 0.331905358585391
9295.15636363636 0.337928978657256
9497.22161616161 0.34396072530114
9699.28686868687 0.350000598517042
9901.35212121212 0.356048598304962
10103.4173737374 0.362104724664901
10305.4826262626 0.368168977596858
10507.5478787879 0.374241357100833
10709.6131313131 0.380321863176827
10911.6783838384 0.386410495824839
11113.7436363636 0.39250725504487
11315.8088888889 0.398612140836919
11517.8741414141 0.404725153200987
11719.9393939394 0.410846292137072
11922.0046464646 0.416975557645177
12124.0698989899 0.4231129497253
12326.1351515151 0.429258468377441
12528.2004040404 0.4354121136016
12730.2656565657 0.441573885397778
12932.3309090909 0.447743783765975
13134.3961616162 0.453921808706189
13336.4614141414 0.460107960218422
13538.5266666667 0.466302238302674
13740.5919191919 0.472504642958944
13942.6571717172 0.478715174187233
14144.7224242424 0.484933831987539
14346.7876767677 0.491160616359865
14548.8529292929 0.497395527304208
14750.9181818182 0.50363856482057
14952.9834343434 0.509889728908951
15155.0486868687 0.516149019569349
15357.1139393939 0.522416436801767
15559.1791919192 0.528691980606202
15761.2444444444 0.534975650982657
15963.3096969697 0.541267447931129
16165.3749494949 0.54756737145162
16367.4402020202 0.553875421544129
16569.5054545455 0.560191598208657
16771.5707070707 0.566515901445203
16973.635959596 0.572848331253767
17175.7012121212 0.57918888763435
17377.7664646465 0.585537570586952
17579.8317171717 0.591894380111571
17781.896969697 0.598259316208209
17983.9622222222 0.604632378876866
18186.0274747475 0.611013568117541
18388.0927272727 0.617402883930234
18590.157979798 0.623800326314946
18792.2232323232 0.630205895271676
18994.2884848485 0.636619590800425
19196.3537373737 0.643041412901192
19398.418989899 0.649471361573977
19600.4842424242 0.655909436818781
19802.5494949495 0.662355638635603
20004.6147474747 0.668809967024444
20206.68 0.675272421985303
};
\addplot [thick, yellowgreen18420623, dashed]
table {%
1 2.7543871307373
120000 2.7543871307373
};
\addplot [very thick, royalblue28108204]
table {%
402.52 0.0901387059766513
691.608282828283 0.100779464392164
980.696565656566 0.111438858686268
1269.78484848485 0.122116888858965
1558.87313131313 0.132813554910254
1847.96141414141 0.143528856840136
2137.0496969697 0.15426279464861
2426.13797979798 0.165015368335676
2715.22626262626 0.175786577901335
3004.31454545455 0.186576423345586
3293.40282828283 0.197384904668429
3582.49111111111 0.208212021869864
3871.57939393939 0.219057774949892
4160.66767676768 0.229922163908512
4449.75595959596 0.240805188745725
4738.84424242424 0.251706849461529
5027.93252525253 0.262627146055927
5317.02080808081 0.273566078528916
5606.10909090909 0.284523646880498
5895.19737373737 0.295499851110672
6184.28565656566 0.306494691219438
6473.37393939394 0.317508167206797
6762.46222222222 0.328540279072748
7051.5505050505 0.339591026817291
7340.63878787879 0.350660410440426
7629.72707070707 0.361748429942154
7918.81535353535 0.372855085322475
8207.90363636364 0.383980376581387
8496.99191919192 0.395124303718892
8786.0802020202 0.406286866734989
9075.16848484848 0.417468065629679
9364.25676767677 0.428667900402961
9653.34505050505 0.439886371054835
9942.43333333333 0.451123477585301
10231.5216161616 0.46237921999436
10520.6098989899 0.473653598282011
10809.6981818182 0.484946612448255
11098.7864646465 0.49625826249309
11387.8747474747 0.507588548416518
11676.963030303 0.518937470218539
11966.0513131313 0.530305027899151
12255.1395959596 0.541691221458356
12544.2278787879 0.553096050896154
12833.3161616162 0.564519516212543
13122.4044444444 0.575961617407525
13411.4927272727 0.587422354481099
13700.581010101 0.598901727433266
13989.6692929293 0.610399736264025
14278.7575757576 0.621916380973376
14567.8458585859 0.63345166156132
14856.9341414141 0.645005578027856
15146.0224242424 0.656578130372984
15435.1107070707 0.668169318596704
15724.198989899 0.679779142699017
16013.2872727273 0.691407602679922
16302.3755555556 0.70305469853942
16591.4638383838 0.714720430277509
16880.5521212121 0.726404797894191
17169.6404040404 0.738107801389466
17458.7286868687 0.749829440763332
17747.816969697 0.761569716015791
18036.9052525253 0.773328627146843
18325.9935353535 0.785106174156486
18615.0818181818 0.796902357044722
18904.1701010101 0.808717175811551
19193.2583838384 0.820550630456971
19482.3466666667 0.832402720980984
19771.4349494949 0.844273447383589
20060.5232323232 0.856162809664787
20349.6115151515 0.868070807824577
20638.6997979798 0.879997441862959
20927.7880808081 0.891942711779933
21216.8763636364 0.9039066175755
21505.9646464646 0.915889159249659
21795.0529292929 0.927890336802411
22084.1412121212 0.939910150233755
22373.2294949495 0.951948599543691
22662.3177777778 0.964005684732219
22951.4060606061 0.97608140579934
23240.4943434343 0.988175762745053
23529.5826262626 1.00028875556936
23818.6709090909 1.01242038427226
24107.7591919192 1.02457064885375
24396.8474747475 1.03673954931383
24685.9357575758 1.0489270856525
24975.024040404 1.06113325786977
25264.1123232323 1.07335806596563
25553.2006060606 1.08560150994008
25842.2888888889 1.09786358979312
26131.3771717172 1.11014430552476
26420.4654545455 1.12244365713499
26709.5537373737 1.13476164462381
26998.642020202 1.14709826799122
27287.7303030303 1.15945352723723
27576.8185858586 1.17182742236183
27865.9068686869 1.18421995336502
28154.9951515151 1.1966311202468
28444.0834343434 1.20906092300717
28733.1717171717 1.22150936164614
29022.26 1.2339764361637
};
\addplot [thick, royalblue28108204, dashed]
table {%
1 6.83080143928528
120000 6.83080143928528
};
\addplot [very thick, purple11522131]
table {%
600.42 0.108871137350879
1002.06323232323 0.126614185614796
1403.70646464646 0.144384788012855
1805.3496969697 0.162182944545056
2206.99292929293 0.180008655211399
2608.63616161616 0.197861920011885
3010.27939393939 0.215742738946512
3411.92262626263 0.233651112015282
3813.56585858586 0.251587039218194
4215.20909090909 0.269550520555248
4616.85232323232 0.287541556026445
5018.49555555556 0.305560145631783
5420.13878787879 0.323606289371264
5821.78202020202 0.341679987244887
6223.42525252525 0.359781239252652
6625.06848484849 0.37791004539456
7026.71171717172 0.396066405670609
7428.35494949495 0.414250320080801
7829.99818181818 0.432461788625135
8231.64141414141 0.450700811303611
8633.28464646465 0.468967388116229
9034.92787878788 0.48726151906299
9436.57111111111 0.505583204143892
9838.21434343434 0.523932443358937
10239.8575757576 0.542309236708124
10641.5008080808 0.560713584191453
11043.144040404 0.579145485808925
11444.7872727273 0.597604941560539
11846.4305050505 0.616091951446294
12248.0737373737 0.634606515466192
12649.716969697 0.653148633620233
13051.3602020202 0.671718305908415
13453.0034343434 0.69031553233074
13854.6466666667 0.708940312887206
14256.2898989899 0.727592647577815
14657.9331313131 0.746272536402566
15059.5763636364 0.76497997936146
15461.2195959596 0.783714976454495
15862.8628282828 0.802477527681673
16264.5060606061 0.821267633042993
16666.1492929293 0.840085292538455
17067.7925252525 0.858930506168059
17469.4357575758 0.877803273931805
17871.078989899 0.896703595829694
18272.7222222222 0.915631471861725
18674.3654545455 0.934586902027898
19076.0086868687 0.953569886328213
19477.6519191919 0.97258042476267
19879.2951515152 0.99161851733127
20280.9383838384 1.01068416403401
20682.5816161616 1.0297773648709
21084.2248484848 1.04889811984192
21485.8680808081 1.06804642894709
21887.5113131313 1.0872222921864
22289.1545454545 1.10642570955985
22690.7977777778 1.12565668106745
23092.441010101 1.14491520670919
23494.0842424242 1.16420128648506
23895.7274747475 1.18351492039509
24297.3707070707 1.20285610843925
24699.0139393939 1.22222485061756
25100.6571717172 1.24162114693
25502.3004040404 1.26104499737659
25903.9436363636 1.28049640195733
26305.5868686869 1.2999753606722
26707.2301010101 1.31948187352122
27108.8733333333 1.33901594050438
27510.5165656566 1.35857756162168
27912.1597979798 1.37816673687312
28313.803030303 1.39778346625871
28715.4462626263 1.41742774977843
29117.0894949495 1.4370995874323
29518.7327272727 1.45679897922032
29920.375959596 1.47652592514247
30322.0191919192 1.49628042519877
30723.6624242424 1.51606247938921
31125.3056565657 1.53587208771379
31526.9488888889 1.55570925017251
31928.5921212121 1.57557396676538
32330.2353535354 1.59546623749238
32731.8785858586 1.61538606235353
33133.5218181818 1.63533344134882
33535.165050505 1.65530837447826
33936.8082828283 1.67531086174183
34338.4515151515 1.69534090313955
34740.0947474747 1.71539849867141
35141.737979798 1.73548364833742
35543.3812121212 1.75559635213756
35945.0244444444 1.77573661007185
36346.6676767677 1.79590442214028
36748.3109090909 1.81609978834285
37149.9541414141 1.83632270867956
37551.5973737374 1.85657318315042
37953.2406060606 1.87685121175542
38354.8838383838 1.89715679449456
38756.5270707071 1.91748993136784
39158.1703030303 1.93785062237526
39559.8135353535 1.95823886751683
39961.4567676768 1.97865466679254
40363.1 1.99909802020239
};
\addplot [thick, purple11522131, dashed]
table {%
1 13.0605303382874
120000 13.0605303382874
};
\addplot [very thick, indianred19152101]
table {%
861.9 0.129307932790709
1395.67353535354 0.156364224207461
1929.44707070707 0.183471710327741
2463.22060606061 0.210630391151547
2996.99414141414 0.23784026667888
3530.76767676768 0.26510133690974
4064.54121212121 0.292413601844127
4598.31474747475 0.319777061482041
5132.08828282828 0.347191715823482
5665.86181818182 0.37465756486845
6199.63535353535 0.402174608616945
6733.40888888889 0.429742847068966
7267.18242424242 0.457362280224515
7800.95595959596 0.485032908083591
8334.7294949495 0.512754730646193
8868.50303030303 0.540527747912323
9402.27656565657 0.568351959881979
9936.0501010101 0.596227366555163
10469.8236363636 0.624153967931873
11003.5971717172 0.65213176401211
11537.3707070707 0.680160754795875
12071.1442424242 0.708240940283166
12604.9177777778 0.736372320473984
13138.6913131313 0.764554895368329
13672.4648484848 0.792788664966201
14206.2383838384 0.8210736292676
14740.0119191919 0.849409788272526
15273.7854545455 0.877797141980979
15807.558989899 0.906235690392959
16341.3325252525 0.934725433508465
16875.1060606061 0.963266371327499
17408.8795959596 0.99185850385006
17942.6531313131 1.02050183107615
18476.4266666667 1.04919635300576
19010.2002020202 1.0779420696389
19543.9737373737 1.10673898097557
20077.7472727273 1.13558708701577
20611.5208080808 1.16448638775949
21145.2943434343 1.19343688320674
21679.0678787879 1.22243857335752
22212.8414141414 1.25149145821182
22746.614949495 1.28059553776965
23280.3884848485 1.30975081203101
23814.162020202 1.33895728099589
24347.9355555556 1.3682149446643
24881.7090909091 1.39752380303624
25415.4826262626 1.4268838561117
25949.2561616162 1.45629510389069
26483.0296969697 1.48575754637321
27016.8032323232 1.51527118355926
27550.5767676768 1.54483601544883
28084.3503030303 1.57445204204193
28618.1238383838 1.60411926333856
29151.8973737374 1.63383767933871
29685.6709090909 1.66360729004239
30219.4444444444 1.6934280954496
30753.217979798 1.72330009556033
31286.9915151515 1.75322329037459
31820.7650505051 1.78319767989238
32354.5385858586 1.8132232641137
32888.3121212121 1.84330004303854
33422.0856565657 1.87342801666691
33955.8591919192 1.9036071849988
34489.6327272727 1.93383754803423
35023.4062626263 1.96411910577318
35557.1797979798 1.99445185821565
36090.9533333333 2.02483580536166
36624.7268686869 2.05527094721119
37158.5004040404 2.08575728376425
37692.2739393939 2.11629481502083
38226.0474747475 2.14688354098094
38759.821010101 2.17752346164458
39293.5945454546 2.20821457701175
39827.3680808081 2.23895688708244
40361.1416161616 2.26975039185666
40894.9151515152 2.3005950913344
41428.6886868687 2.33149098551568
41962.4622222222 2.36243807440048
42496.2357575758 2.3934363579888
43030.0092929293 2.42448583628066
43563.7828282828 2.45558650927604
44097.5563636364 2.48673837697495
44631.3298989899 2.51794143937738
45165.1034343434 2.54919569648334
45698.876969697 2.58050114829283
46232.6505050505 2.61185779480585
46766.424040404 2.64326563602239
47300.1975757576 2.67472467194246
47833.9711111111 2.70623490256606
48367.7446464647 2.73779632789318
48901.5181818182 2.76940894792383
49435.2917171717 2.80107276265801
49969.0652525253 2.83278777209571
50502.8387878788 2.86455397623694
51036.6123232323 2.8963713750817
51570.3858585859 2.92823996862999
52104.1593939394 2.9601597568818
52637.9329292929 2.99213073983714
53171.7064646465 3.024152917496
53705.48 3.0562262898584
};
\addplot [thick, indianred19152101, dashed]
table {%
1 23.3272634887695
120000 23.3272634887695
};
\addplot [very thick, chocolate21910927]
table {%
1090.24 0.154371832153995
1777.3903030303 0.19407995849573
2464.54060606061 0.233822404520195
3151.69090909091 0.273599170227392
3838.84121212121 0.313410255617319
4525.99151515151 0.353255660689976
5213.14181818182 0.393135385445364
5900.29212121212 0.433049429883483
6587.44242424242 0.472997794004333
7274.59272727273 0.512980477807913
7961.74303030303 0.552997481294224
8648.89333333333 0.593048804463265
9336.04363636363 0.633134447315037
10023.1939393939 0.67325440984954
10710.3442424242 0.713408692066773
11397.4945454545 0.753597293966737
12084.6448484848 0.793820215549431
12771.7951515151 0.834077456814857
13458.9454545455 0.874369017763013
14146.0957575758 0.914694898393899
14833.2460606061 0.955055098707516
15520.3963636364 0.995449618703864
16207.5466666667 1.03587845838294
16894.696969697 1.07634161774475
17581.8472727273 1.11683909678929
18268.9975757576 1.15737089551656
18956.1478787879 1.19793701392656
19643.2981818182 1.23853745201929
20330.4484848485 1.27917220979476
21017.5987878788 1.31984128725295
21704.7490909091 1.36054468439387
22391.8993939394 1.40128240121753
23079.0496969697 1.44205443772391
23766.2 1.48286079391303
24453.3503030303 1.52370146978487
25140.5006060606 1.56457646533945
25827.6509090909 1.60548578057676
26514.8012121212 1.64642941549679
27201.9515151515 1.68740737009956
27889.1018181818 1.72841964438506
28576.2521212121 1.76946623835329
29263.4024242424 1.81054715200425
29950.5527272727 1.85166238533794
30637.703030303 1.89281193835436
31324.8533333333 1.93399581105352
32012.0036363636 1.9752140034354
32699.1539393939 2.01646651550001
33386.3042424242 2.05775334724736
34073.4545454545 2.09907449867743
34760.6048484848 2.14042996979024
35447.7551515151 2.18181976058577
36134.9054545454 2.22324387106404
36822.0557575757 2.26470230122504
37509.206060606 2.30619505106876
38196.3563636364 2.34772212059522
38883.5066666667 2.38928350980441
39570.656969697 2.43087921869633
40257.8072727273 2.47250924727098
40944.9575757576 2.51417359552836
41632.1078787879 2.55587226346848
42319.2581818182 2.59760525109132
43006.4084848485 2.63937255839689
43693.5587878788 2.68117418538519
44380.7090909091 2.72301013205623
45067.8593939394 2.76488039840999
45755.0096969697 2.80678498444649
46442.16 2.84872389016572
47129.3103030303 2.89069711556767
47816.4606060606 2.93270466065236
48503.6109090909 2.97474652541978
49190.7612121212 3.01682270986993
49877.9115151515 3.05893321400281
50565.0618181818 3.10107803781842
51252.2121212121 3.14325718131676
51939.3624242424 3.18547064449783
52626.5127272727 3.22771842736163
53313.663030303 3.27000052990816
54000.8133333333 3.31231695213743
54687.9636363636 3.35466769404942
55375.1139393939 3.39705275564414
56062.2642424242 3.4394721369216
56749.4145454545 3.48192583788178
57436.5648484848 3.5244138585247
58123.7151515151 3.56693619885035
58810.8654545454 3.60949285885872
59498.0157575757 3.65208383854983
60185.166060606 3.69470913792367
60872.3163636364 3.73736875698024
61559.4666666667 3.78006269571954
62246.616969697 3.82279095414157
62933.7672727273 3.86555353224633
63620.9175757576 3.90835043003383
64308.0678787879 3.95118164750405
64995.2181818182 3.994047184657
65682.3684848485 4.03694704149269
66369.5187878788 4.0798812180111
67056.6690909091 4.12284971421225
67743.8193939394 4.16585253009612
68430.9696969697 4.20888966566273
69118.12 4.25196112091207
};
\addplot [thick, chocolate21910927, dashed]
table {%
1 36.7181792163849
120000 36.7181792163849
};
\addplot [very thick, saddlebrown1356716]
table {%
1400.16 0.17822761567721
2274.43797979798 0.23545252581402
3148.71595959596 0.292700204140202
4022.99393939394 0.349970650655758
4897.27191919192 0.407263865360686
5771.5498989899 0.464579848254988
6645.82787878788 0.521918599338662
7520.10585858586 0.57928011861171
8394.38383838384 0.636664406074131
9268.66181818182 0.694071461725924
10142.9397979798 0.751501285567091
11017.2177777778 0.80895387759763
11891.4957575758 0.866429237817543
12765.7737373737 0.923927366226829
13640.0517171717 0.981448262825487
14514.3296969697 1.03899192761352
15388.6076767677 1.09655836059092
16262.8856565657 1.1541475617577
17137.1636363636 1.21175953111385
18011.4416161616 1.26939426865938
18885.7195959596 1.32705177439427
19759.9975757576 1.38473204831854
20634.2755555556 1.44243509043218
21508.5535353535 1.5001609007352
22382.8315151515 1.55790947922759
23257.1094949495 1.61568082590935
24131.3874747475 1.67347494078049
25005.6654545455 1.73129182384099
25879.9434343434 1.78913147509087
26754.2214141414 1.84699389453013
27628.4993939394 1.90487908215875
28502.7773737374 1.96278703797675
29377.0553535354 2.02071776198413
30251.3333333333 2.07867125418087
31125.6113131313 2.13664751456699
31999.8892929293 2.19464654314248
32874.1672727273 2.25266833990735
33748.4452525252 2.31071290486159
34622.7232323232 2.3687802380052
35497.0012121212 2.42687033933818
36371.2791919192 2.48498320886054
37245.5571717172 2.54311884657227
38119.8351515152 2.60127725247337
38994.1131313131 2.65945842656385
39868.3911111111 2.71766236884369
40742.6690909091 2.77588907931292
41616.9470707071 2.83413855797151
42491.225050505 2.89241080481948
43365.503030303 2.95070581985682
44239.781010101 3.00902360308353
45114.058989899 3.06736415449962
45988.336969697 3.12572747410508
46862.6149494949 3.18411356189991
47736.8929292929 3.24252241788412
48611.1709090909 3.3009540420577
49485.4488888889 3.35940843442065
50359.7268686869 3.41788559497297
51234.0048484848 3.47638552371467
52108.2828282828 3.53490822064574
52982.5608080808 3.59345368576619
53856.8387878788 3.652021919076
54731.1167676768 3.71061292057519
55605.3947474747 3.76922669026376
56479.6727272727 3.82786322814169
57353.9507070707 3.886522534209
58228.2286868687 3.94520460846568
59102.5066666667 4.00390945091174
59976.7846464646 4.06263706154716
60851.0626262626 4.12138744037197
61725.3406060606 4.18016058738614
62599.6185858586 4.23895650258969
63473.8965656566 4.29777518598261
64348.1745454545 4.3566166375649
65222.4525252525 4.41548085733656
66096.7305050505 4.4743678452976
66971.0084848485 4.53327760144802
67845.2864646465 4.5922101257878
68719.5644444444 4.65116541831696
69593.8424242424 4.71014347903549
70468.1204040404 4.76914430794339
71342.3983838384 4.82816790504067
72216.6763636364 4.88721427032732
73090.9543434343 4.94628340380334
73965.2323232323 5.00537530546874
74839.5103030303 5.06448997532351
75713.7882828283 5.12362741336765
76588.0662626263 5.18278761960117
77462.3442424242 5.24197059402405
78336.6222222222 5.30117633663631
79210.9002020202 5.36040484743795
80085.1781818182 5.41965612642896
80959.4561616162 5.47893017360933
81833.7341414141 5.53822698897909
82708.0121212121 5.59754657253821
83582.2901010101 5.65688892428671
84456.5680808081 5.71625404422459
85330.8460606061 5.77564193235183
86205.124040404 5.83505258866845
87079.402020202 5.89448601317444
87953.68 5.9539422058698
};
\addplot [thick, saddlebrown1356716, dashed]
table {%
1 58.9505964565277
120000 58.9505964565277
};
\addplot [very thick, black18]
table {%
1675.74 0.207702006559532
2752.04929292929 0.280057106501963
3828.35858585859 0.352393972367939
4904.66787878788 0.424712604157462
5980.97717171717 0.497013001870531
7057.28646464646 0.569295165507145
8133.59575757576 0.641559095067305
9209.90505050505 0.713804790551012
10286.2143434343 0.786032251958264
11362.5236363636 0.858241479289063
12438.8329292929 0.930432472543407
13515.1422222222 1.0026052317213
14591.4515151515 1.07475975682273
15667.7608080808 1.14689604784772
16744.0701010101 1.21901410479624
17820.3793939394 1.29111392766832
18896.6886868687 1.36319551646394
19972.997979798 1.4352588711831
21049.3072727273 1.50730399182582
22125.6165656566 1.57933087839207
23201.9258585859 1.65133953088188
24278.2351515152 1.72332994929523
25354.5444444444 1.79530213363212
26430.8537373737 1.86725608389256
27507.163030303 1.93919180007655
28583.4723232323 2.01110928218409
29659.7816161616 2.08300853021517
30736.0909090909 2.15488954416979
31812.4002020202 2.22675232404796
32888.7094949495 2.29859686984968
33965.0187878788 2.37042318157494
35041.3280808081 2.44223125922375
36117.6373737374 2.51402110279611
37193.9466666667 2.58579271229201
38270.255959596 2.65754608771146
39346.5652525253 2.72928122905445
40422.8745454545 2.80099813632099
41499.1838383838 2.87269680951107
42575.4931313131 2.94437724862471
43651.8024242424 3.01603945366188
44728.1117171717 3.08768342462261
45804.421010101 3.15930916150687
46880.7303030303 3.23091666431469
47957.0395959596 3.30250593304605
49033.3488888889 3.37407696770096
50109.6581818182 3.44562976827941
51185.9674747475 3.51716433478141
52262.2767676768 3.58868066720695
53338.5860606061 3.66017876555604
54414.8953535354 3.73165862982868
55491.2046464646 3.80312026002486
56567.5139393939 3.87456365614459
57643.8232323232 3.94598881818787
58720.1325252525 4.01739574615469
59796.4418181818 4.08878444004505
60872.7511111111 4.16015489985897
61949.0604040404 4.23150712559642
63025.3696969697 4.30284111725743
64101.678989899 4.37415687484198
65177.9882828283 4.44545439835008
66254.2975757576 4.51673368778172
67330.6068686869 4.58799474313691
68406.9161616162 4.65923756441564
69483.2254545455 4.73046215161792
70559.5347474748 4.80166850474375
71635.844040404 4.87285662379312
72712.1533333333 4.94402650876603
73788.4626262626 5.0151781596625
74864.7719191919 5.08631157648251
75941.0812121212 5.15742675922607
77017.3905050505 5.22852370789317
78093.6997979798 5.29960242248382
79170.0090909091 5.37066290299801
80246.3183838384 5.44170514943575
81322.6276767677 5.51272916179703
82398.936969697 5.58373494008187
83475.2462626263 5.65472248429024
84551.5555555556 5.72569179442216
85627.8648484849 5.79664287047763
86704.1741414141 5.86757571245665
87780.4834343434 5.93849032035921
88856.7927272727 6.00938669418532
89933.102020202 6.08026483393497
91009.4113131313 6.15112473960817
92085.7206060606 6.22196641120492
93162.0298989899 6.29278984872521
94238.3391919192 6.36359505216904
95314.6484848485 6.43438202153643
96390.9577777778 6.50515075682736
97467.2670707071 6.57590125804183
98543.5763636364 6.64663352517985
99619.8856565657 6.71734755824142
100696.194949495 6.78804335722653
101772.504242424 6.85872092213519
102848.813535354 6.92938025296739
103925.122828283 7.00002134972315
105001.432121212 7.07064421240244
106077.741414141 7.14124884100529
107154.050707071 7.21183523553167
108230.36 7.28240339598161
};
\addplot [thick, black18, dashed]
table {%
1 78.7926025772095
120000 78.7926025772095
};
